# Supplementary material for: Computations of Keller maps over fields with $\tfrac16$
Source: arXiv:1609.09753 ancillary file (2017-11-02)
Supplement: Supplementary file 1 [file dim3detcub.pdf]

```

[ > restart;
> efactors := proc (eq)
>   local F, IF, i, c;
>   F := factors (eq);
>   for i from 1 to nops(F[2]) do
>     c := content (F[2][i][1]);
>     F[2][i][1] := F[2][i][1] / c;
>     F[1] := F[1] * c ^ F[2][i][2];
>   od;
>   IF := ifactors (F[1]);
>   return (IF[1], [op(IF[2]), op(F[2])]);
> end;

```

*efactors* := **proc**(eq)

**local** F, IF, i, c;

F := factors(eq);

**for** i **to** nops(F[2]) **do**

c := content(F[2][i][1]);

F[2][i][1] := F[2][i][1] / c;

F[1] := F[1]\*c^F[2][i][2]

**end do**;

IF := ifactors(F[1]);

**return** IF[1], [op(IF[2]), op(F[2])]

**end proc**

```

[ > psqf := proc (eq)
>   local EF, S, i;
>   EF := efactors (eq);
>   S := EF[1];
>   for i from 1 to nops(EF[2]) do
>     if (EF[2][i][2] > 0) then
>       S := S * EF[2][i][1]
>     fi
>   od;
>   return S
> end;

```

*psqf* := **proc**(eq)

**local** EF, S, i;

EF := efactors(eq);

S := EF[1];

**for** i **to** nops(EF[2]) **do** **if** 0 < EF[2][i][2] **then** S := S\*EF[2][i][1] **end if** **end do**;

**return** S

**end proc**

```

[ > initcases := proc ()
>   global nz, NZ, SV;

```

```

>  if nargs = 0 then
>      nz := 1
>  else
>      nz := args[1];
>      printf ("We assume the following in our calculation:");
>      print (psqf (nz) <> 0);
>  fi;
>  NZ := [convert (nz,string)];
>  SV := [[]];
>  return
> end;

```

*initcases* := **proc**()

**global** *nz, NZ, SV*;

**if** nargs = 0 **then** *nz* := 1

**else**

*nz* := args[ 1 ];

        printf ("We assume the following in our calculation:");

        print(psqf(*nz*) ≠ 0)

**end if**;

*NZ* := [ convert(*nz*, *string*) ];

*SV* := [ [ ] ];

**return**

**end proc**

> **launchNZcase** := **proc** (*nz*)

>     **global** *NZ, SV*;

>     **local** *t*;

>     *NZ* := [seq(*NZ*[*i*], *i*=1..*nops*(*NZ*)), convert (*nz*,*string*)];

>     *SV* := [seq(*SV*[*i*], *i*=1..*nops*(*SV*)), [ ]];

>     printf ("Launching case level %d:", *nops*(*NZ*) - 1);

>     print (*nz* <> 0);

>     printf ("Assume from now on that:");

>     *t* := mul (psqf (parse (*NZ*[*i*],*statement*)), *i*=1..*nops*(*NZ*));

>     print (*t* <> 0)

> **end**;

*launchNZcase* := **proc**(*nz*)

**local** *t*;

**global** *NZ, SV*;

*NZ* := [ seq(*NZ*[ *i* ], *i* = 1 .. *nops*(*NZ*)), convert(*nz*, *string*) ];

*SV* := [ seq(*SV*[ *i* ], *i* = 1 .. *nops*(*SV*)), [ ] ];

    printf ("Launching case level %d:", *nops*(*NZ*) - 1);

    print(*nz* ≠ 0);

    printf ("Assume from now on that:");

```

t := mul(psqf(parse(NZ[i], statement)), i = 1 .. nops(NZ));
print(t ≠ 0)

```

**end proc**

```

> contradict := proc (eq)
>   global NZ, SV, alph;
>   local t, EF, i, sv, nz;
>   t := mul (psqf (parse (NZ[i], statement)), i=1..nops(NZ));
>   EF := efactors (psqf (psqf (eq) / t));
>   if EF[1] = 0 or nops (EF[2]) > 0 then
>     error "No contradiction: 'eq' might be zero!"
>   fi;
>   printf ("Contradiction on case level %d, so:", nops(NZ) - 1);
>   for i from 1 to nops(SV[nops(SV)]) do
>     sv := cat (SV[nops(SV)][i], " := ");
>     sv := cat (sv, SV[nops(SV)][i], "");
>     parse (sv, statement)
>   od;
>   nz := parse (NZ[nops(NZ)], statement);
>   print (nz = 0);
>   if nops(SV[nops(SV)]) > 0 then
>     printf ("Variables to be uneliminated:");
>     for i from 1 to nops(SV[nops(SV)]) do
>       sv := cat (SV[nops(SV)][i], " := ");
>       sv := cat (sv, SV[nops(SV)][i], "");
>       print (sv);
>     od
>   fi;
>   if nops(NZ) <= 1 then
>     printf ("That is all, folks! ");
>     printf ("Check that all variables are uneliminated:");
>     print (alph);
>     return
>   fi;
>   NZ := [seq(NZ[i], i=1..nops(NZ)-1)];
>   SV := [seq(SV[i], i=1..nops(SV)-1)];
>   printf ("Proceed on case level %d with:", nops(NZ) - 1);
>   t := mul (psqf (parse (NZ[i], statement)), i=1..nops(NZ));
>   print (t <> 0);
>   printf ("On account of:");
>   print (nz = 0);
>   if nargs = 1 and nops(indets(nz)) = 1 and degree (nz) = 1 then
>     EF := efactors (psqf (psqf (coeff (nz, indets(nz)[1])) / t));
>     if nops (EF[2]) = 0 then
>       elimsolve(nz, indets(nz)[1]);
>       return
>     fi;
>   fi;

```

```

>   elif nargs > 1 then
>       elimsolve (nz, args[2]);
>       return
>   fi;
>   printf ("the following return value %s",
>           "can be used as an equation:");
>   return nz
> end;

contradict := proc(eq)
local t, EF, i, sv, nz;
global NZ, SV, alph;

    t := mul(psqf(parse(NZ[i], statement)), i = 1 .. nops(NZ));
    EF := efactors(psqf(psqf(eq) / t));
    if EF[1] = 0 or 0 < nops(EF[2]) then error "No contradiction: 'eq' might be zero!"
    end if;
    printf("Contradiction on case level %d, so:", nops(NZ) - 1);
    for i to nops(SV[nops(SV)]) do
        sv := cat(SV[nops(SV)][i], " := ");
        sv := cat(sv, SV[nops(SV)][i], "");
        parse(sv, statement)
    end do;
    nz := parse(NZ[nops(NZ)], statement);
    print(nz = 0);
    if 0 < nops(SV[nops(SV)]) then
        printf("Variables to be uneliminated:");
        for i to nops(SV[nops(SV)]) do
            sv := cat(SV[nops(SV)][i], " := ");
            sv := cat(sv, SV[nops(SV)][i], "");
            print(sv)
        end do
    end if;
    if nops(NZ) ≤ 1 then
        printf("That is all, folks! ");
        printf("Check that all variables are uneliminated:");
        print(alph);
        return
    end if;
    NZ := [seq(NZ[i], i = 1 .. nops(NZ) - 1)];
    SV := [seq(SV[i], i = 1 .. nops(SV) - 1)];
    printf("Proceed on case level %d with:", nops(NZ) - 1);

```

```

t := mul(psqf(parse(NZ[i], statement)), i = 1 .. nops(NZ));
print(t ≠ 0);
printf("On account of:");
print(nz = 0);
if nargs = 1 and nops(indets(nz)) = 1 and degree(nz) = 1 then
    EF := efactors(psqf(psqf(coeff(nz, indets(nz)[1]) / t));
    if nops(EF[2]) = 0 then elimsolve(nz, indets(nz)[1]); return end if
elif 1 < nargs then elimsolve(nz, args[2]); return
end if;
printf("the following return value %s", "can be used as an equation:");
return nz

```

**end proc**

```

> elimsolve := proc (eq, v)
>   global NZ, SV;
>   local t, EF, i, c1, c0, NZref, sv, F;
>   if not ({v} subset indets(v)) then
>     error "Second argument 'v' is not a variable!";
>   fi;
>   t := mul (psqf (parse (NZ[i], statement)), i=1..nops(NZ));
>   EF := efactors (psqf (psqf (eq) / t));
>   if EF[1] = 0 then error "First argument 'eq' is zero!" fi;
>   if nops(EF[2]) = 0 then
>     error "Contradiction: call 'contradict'!"
>   fi;
>   if nops(EF[2]) > 1 then
>     error "'eq' has different factors which may be zero!"
>   fi;
>   if degree (EF[2][1][1], v) <> 1 then
>     error "Degree of 'eq' w.r.t 'v' is not one!"
>   fi;
>   c1 := coeff(EF[2][1][1], v, 1);
>   c0 := coeff(EF[2][1][1], v, 0);
>   EF := efactors (psqf (psqf (c1) / t));
>   if nops(EF[2]) > 0 then
>     error "Coefficient of 'v' in 'eq' might be zero!"
>   fi;
>   EF := efactors (psqf (psqf (denom(eq)) / t));
>   if nops(EF[2]) > 0 then
>     error "Denominator of argument 'eq' may be zero!"
>   fi;
>   print ({c1 <> 0});
>   NZref := false;
>   for i from 1 to nops(NZ) do
>     NZref :=

```

```

>      NZref or ({v} subset indets (parse (NZ[i],statement)));
> od;
> sv := convert (v, string);
> F := factor (-c0/c1);
> SV[nops(SV)] :=
>   [sv, seq(SV[nops(SV)][i], i=1..nops(SV[nops(SV)]))];
> printf ("%s is set to:", sv);
> sv := cat (sv, " := ", convert (F, string));
> print (parse (sv,statement));
> if NZref then
>   printf ("Nonzero constraint refines to:");
>   t := mul (psqf (parse (NZ[i],statement)), i=1..nops (NZ));
>   print (t <> 0)
> fi;
> return
> end;

```

*elimsolve* := **proc**(eq, v)

**local** t, EF, i, c1, c0, NZref, sv, F;

**global** NZ, SV;

**if not** {v} subset indets(v) **then error** "Second argument 'v' is not a variable!" **end if**;

t := mul(psqf(parse(NZ[i], statement)), i = 1 .. nops(NZ));

EF := efactors(psqf(psqf(eq) / t));

**if** EF[1] = 0 **then error** "First argument 'eq' is zero!" **end if**;

**if** nops(EF[2]) = 0 **then error** "Contradiction: call 'contradict'!" **end if**;

**if** 1 < nops(EF[2]) **then error** "'eq' has different factors which may be zero!" **end if**;

**if** degree(EF[2][1][1], v) ≠ 1 **then error** "Degree of 'eq' w.r.t 'v' is not one!" **end if**;

c1 := coeff(EF[2][1][1], v, 1);

c0 := coeff(EF[2][1][1], v, 0);

EF := efactors(psqf(psqf(c1) / t));

**if** 0 < nops(EF[2]) **then error** "Coefficient of 'v' in 'eq' might be zero!" **end if**;

EF := efactors(psqf(psqf(denom(eq)) / t));

**if** 0 < nops(EF[2]) **then error** "Denominator of argument 'eq' may be zero!" **end if**;

print({c1 ≠ 0});

NZref := false;

**for** i **to** nops(NZ) **do** NZref := NZref or {v} subset indets(parse(NZ[i], statement))

**end do**;

sv := convert(v, string);

F := factor(-c0 / c1);

SV[nops(SV)] := [sv, seq(SV[nops(SV)][i], i = 1 .. nops(SV[nops(SV)]))];

printf ("%s is set to:", sv);

sv := cat(sv, " := ", convert(F, string));

```

print(parse(sv, statement));
if NZref then
    printf("Nonzero constraint refines to:");
    t := mul(psqf(parse(NZ[i], statement)), i = 1 .. nops(NZ));
    print(t ≠ 0)
end if;
return

```

end proc

```

> initdtcoeff := proc (dt)
>   global x1, x2, x3, S, n;
>   local i, j, k, dt1, dt2, dt3;
>   S := Array (0..(deg-1)*n, 0..(deg-1)*n,
>               0..(deg-1)*n, storage=sparse);
>   for i from 0 to (deg-1)*n do
>       dt1 := coeff (dt, x1, i);
>       for j from 0 to (deg-1)*n-i do
>           dt2 := coeff (dt1, x2, j);
>           for k from 0 to (deg-1)*n-i-j do
>               S[i,j,k] := coeff (dt2, x3, k);
>           od
>       od
>   od;
>   return
> end;

```

initdtcoeff:=proc(dt)

local i, j, k, dt1, dt2, dt3;

global x1, x2, x3, S, n;

S:=Array(0 .. (deg-1)\*n, 0 .. (deg-1)\*n, 0 .. (deg-1)\*n, storage = sparse);

for i from 0 to (deg-1)\*n do

dt1 := coeff(dt, x1, i);

for j from 0 to (deg-1)\*n-i do

dt2 := coeff(dt1, x2, j);

for k from 0 to (deg-1)\*n-i-j do S[i,j,k] := coeff(dt2, x3, k) end do

end do

end do;

return

end proc

```

> dtcoeff := proc (t)
>   global x1, x2, x3, S;
>   local i, j, k;
>   i := degree (t, x1);
>   j := degree (t, x2);

```

```

> k := degree (t, x3);
> factor (S[i,j,k])
> end;
dtcoeff:=proc(t)
local i,j,k;
global x1,x2,x3,S;
    i:=degree(t,x1);j:=degree(t,x2);k:=degree(t,x3);factor(S[i,j,k])
end proc
> n := 3;
                                n:=3
> deg := 3;
                                deg:=3
> alph :=
> [[a1,b1,c1,d1,e1,f1,g1,h1,i1,j1],
>  [a2,b2,c2,d2,e2,f2,g2,h2,i2,j2],
>  [a3,b3,c3,d3,e3,f3,g3,h3,i3,j3]];
alph:=[[a1,b1,c1,d1,e1,f1,g1,h1,i1,j1],[a2,b2,c2,d2,e2,f2,g2,h2,i2,j2],
       [a3,b3,c3,d3,e3,f3,g3,h3,i3,j3]]
> terms := [x1^3,x1^2*x2,x1^2*x3,x1*x2^2,x1*x2*x3,
>           x1*x3^2,x2^3,x2^2*x3,x2*x3^2,x3^3];
       terms:=[x1^3,x1^2 x2,x1^2 x3,x1 x2^2,x1 x2 x3,x1 x3^2,x2^3,x2^2 x3,x2 x3^2,x3^3]
> M := evalm ([ [1,0,0], [0,1,0], [0,0,0] ]);
                                
$$M:=\begin{bmatrix} 1 & 0 & 0 \\ 0 & 1 & 0 \\ 0 & 0 & 0 \end{bmatrix}$$

> H := Vector (evalm (M &* [seq(terms[k]/degree(terms[k],
>                                [x1,x2,x3][k]),k=1..n)] +
> ['add (alph[1,k]*terms[k],k=n+1..nops(terms))'$1=1..n]));
H:=
$$\left[ \frac{x1^3}{3} + d1 x1 x2^2 + e1 x1 x2 x3 + f1 x1 x3^2 + g1 x2^3 + h1 x2^2 x3 + i1 x2 x3^2 + j1 x3^3, \right.$$


$$x1^2 x2 + d2 x1 x2^2 + e2 x1 x2 x3 + f2 x1 x3^2 + g2 x2^3 + h2 x2^2 x3 + i2 x2 x3^2 + j2 x3^3,$$


$$\left. d3 x1 x2^2 + e3 x1 x2 x3 + f3 x1 x3^2 + g3 x2^3 + h3 x2^2 x3 + i3 x2 x3^2 + j3 x3^3 \right]$$

> with (linalg):
Warning, the protected names norm and trace have been redefined and
unprotected
> JH := jacobian (H,[x1,x2,x3]):
> dt := expand (det (JH)):
> initdtcoeff (dt);
> initcases (6);
We assume the following in our calculation:
                                6 ≠ 0

```



```

> tmp1 := dtcoeff (x1^5*x2);
                                     tmp1 := e3
> elimsolve (tmp1,e3);
                                     {1 ≠ 0}
e3 is set to:
                                     0
> tmp1 := dtcoeff (x1^5*x3);
                                     tmp1 := 2 f3
> elimsolve (tmp1,f3);
                                     {1 ≠ 0}
f3 is set to:
                                     0
> tmp1 := dtcoeff (x1^4*x3^2);
                                     tmp1 := 3 j3
> elimsolve (tmp1,j3);
                                     {1 ≠ 0}
j3 is set to:
                                     0
> tmp1 := dtcoeff (x1^4*x2^2);
                                     tmp1 := h3 - 2 e2 d3
> elimsolve (tmp1,h3);
                                     {-1 ≠ 0}
h3 is set to:
                                     2 e2 d3
> tmp1 := dtcoeff (x1^4*x2*x3);
                                     tmp1 := 2 i3 - 4 f2 d3
> elimsolve (tmp1,i3);
                                     {-1 ≠ 0}
i3 is set to:
                                     2 f2 d3
> launchNZcase (d3);
Launching case level 1:
                                     d3 ≠ 0
Assume from now on that:
                                     6 d3 ≠ 0
> tmp1 := dtcoeff (x1^3*x3^3);
                                     tmp1 := -4 f2^2 d3
> elimsolve (tmp1,f2);
                                     {1 ≠ 0}
f2 is set to:
                                     0
> tmp1 := dtcoeff (x1^3*x2*x3^2);
                                     tmp1 := -6 j2 d3
> elimsolve (tmp1,j2);

```

```

{1 ≠ 0}
j2 is set to:
0
> tmp1 := dtcoeff (x1^3*x2^2*x3);
tmp1 := 2 d3 (3 f1 - e2^2 - 2 i2)
> elimsolve (tmp1,i2);
{-2 ≠ 0}
i2 is set to:
3 f1 - e2^2
2      2
> tmp1 := dtcoeff (x1^3*x2^3);
tmp1 := 4 d2 e2 d3 + 3 d3 e1 - 2 h2 d3 - 3 e2 g3
> elimsolve (tmp1,h2);
{-2 d3 ≠ 0}
h2 is set to:
4 d2 e2 d3 + 3 d3 e1 - 3 e2 g3
2 d3
> tmp1 := dtcoeff (x1^2*x2^2*x3^2);
tmp1 := 3 d3 (3 f1 e2 + e2^3 + 3 j1)
> elimsolve (tmp1,j1);
{3 ≠ 0}
j1 is set to:
e2 (e2^2 + 3 f1)
3
> tmp1 := dtcoeff (x1^2*x2^3*x3^1);
tmp1 := 3 f1 g3 + 3 g3 e2^2 + 6 d3 i1 + 6 e1 e2 d3
> elimsolve (tmp1,i1);
{2 d3 ≠ 0}
i1 is set to:
f1 g3 + g3 e2^2 + 2 e1 e2 d3
2 d3
> tmp1 := dtcoeff (x1^2*x2^4);
tmp1 := - 3 (-4 g2 e2 d3^2 + 4 d1 e2 d3^2 + 4 g3 d2 e2 d3 - e1 g3 d3 - 3 e2 g3^2 - 2 d3^2 h1)
2 d3
> elimsolve (tmp1,h1);
{-2 d3^2 ≠ 0}
h1 is set to:
-4 g2 e2 d3^2 + 4 d1 e2 d3^2 + 4 g3 d2 e2 d3 - e1 g3 d3 - 3 e2 g3^2
2 d3^2
> tmp1 := dtcoeff (x1*x2^2*x3^3);
tmp1 := -9 d3 (f1 + e2^2)^2
> elimsolve (tmp1, f1);

```

```

{1 ≠ 0}
f1 is set to:

$$-e2^2$$

> tmp1 := dtcoeff (x1*x2^4*x3);

$$tmp1 := -\frac{9(e2\,g3 + d3\,e1)^2}{2\,d3}$$

> elimsolve (tmp1,e1);
{d3 ≠ 0}
e1 is set to:

$$-\frac{e2\,g3}{d3}$$

> launchNZcase (e2);
Launching case level 2:
e2 ≠ 0
Assume from now on that:
6 e2 d3 ≠ 0
> tmp1 := dtcoeff (x1*x2^5);

$$tmp1 := \frac{3\,e2\,(3\,d2\,g3^2\,d3 - 3\,d3^3\,g1 - 3\,g3\,g2\,d3^2 + 3\,d1\,g3\,d3^2 - 2\,g3^3)}{d3^2}$$

> elimsolve (tmp1,g1);
{-3 d3^3 ≠ 0}
g1 is set to:

$$\frac{g3\,(3\,g3\,d2\,d3 - 3\,g2\,d3^2 + 3\,d1\,d3^2 - 2\,g3^2)}{3\,d3^3}$$

> tmp1 := dtcoeff (x2^6);

$$tmp1 := \frac{6\,e2\,(-g2\,d3^2 + g3\,d2\,d3 - g3^2)^2}{d3^3}$$

> elimsolve (tmp1,g2);
{-d3^2 ≠ 0}
g2 is set to:

$$\frac{g3\,(d2\,d3 - g3)}{d3^2}$$

> factor (H[1] * H[3] - 1/3*d3 * H[2]^2 +
> 1/3*(2*d2*d3-g3)/d3 * H[2] * H[3] -
> 1/3*(g3^2+3*d1*d3^2+d3^2*d2^2-d2*g3*d3)/d3^3 * H[3]^2);
0
> contradict (1);
Contradiction on case level 2, so:
e2 = 0
Variables to be uneliminated:
" g2 := 'g2'"
" g1 := 'g1'"
Proceed on case level 1 with:

```

|                                            |                    |
|--------------------------------------------|--------------------|
|                                            | $6 d3 \neq 0$      |
| On account of:                             |                    |
|                                            | $e2 = 0$           |
|                                            | $\{1 \neq 0\}$     |
| e2 is set to:                              |                    |
|                                            | 0                  |
| > <b>[seq(diff(H[i],x3),i=1..3)];</b>      |                    |
|                                            | [0, 0, 0]          |
| > <b>contradict (1);</b>                   |                    |
| Contradiction on case level 1, so:         |                    |
|                                            | $d3 = 0$           |
| Variables to be uneliminated:              |                    |
|                                            | "e2 := 'e2'"       |
|                                            | "e1 := 'e1'"       |
|                                            | "f1 := 'f1'"       |
|                                            | "h1 := 'h1'"       |
|                                            | "i1 := 'i1'"       |
|                                            | "j1 := 'j1'"       |
|                                            | "h2 := 'h2'"       |
|                                            | "i2 := 'i2'"       |
|                                            | "j2 := 'j2'"       |
|                                            | "f2 := 'f2'"       |
| Proceed on case level 0 with:              |                    |
|                                            | $6 \neq 0$         |
| On account of:                             |                    |
|                                            | $d3 = 0$           |
|                                            | $\{1 \neq 0\}$     |
| d3 is set to:                              |                    |
|                                            | 0                  |
| > <b>launchNZcase (g3);</b>                |                    |
| Launching case level 1:                    |                    |
|                                            | $g3 \neq 0$        |
| Assume from now on that:                   |                    |
|                                            | $6 g3 \neq 0$      |
| > <b>tmp1 := dtcoeff (x1^2*x2^2*x3^2);</b> |                    |
|                                            | $tmp1 := -9 j2 g3$ |
| > <b>elimsolve (tmp1,j2);</b>              |                    |
|                                            | $\{1 \neq 0\}$     |
| j2 is set to:                              |                    |
|                                            | 0                  |
| > <b>tmp1 := dtcoeff (x1^3*x2^2*x3^1);</b> |                    |
|                                            | $tmp1 := -6 f2 g3$ |
| > <b>elimsolve (tmp1,f2);</b>              |                    |
|                                            | $\{1 \neq 0\}$     |

```

f2 is set to:
0
> tmp1 := dtcoeff (x1^3*x2^3);
tmp1 := -3 e2 g3
> elimsolve (tmp1,e2);
{1 ≠ 0}
e2 is set to:
0
> tmp1 := dtcoeff (x1*x2^3*x3^2);
tmp1 := 18 j1 g3
> elimsolve (tmp1,j1);
{1 ≠ 0}
j1 is set to:
0
> tmp1 := dtcoeff (x1^2*x2^4);
tmp1 := 3 g3 (-h2 + 2 e1)
> elimsolve (tmp1,h2);
{-1 ≠ 0}
h2 is set to:
2 e1
> tmp1 := dtcoeff (x1^2*x2^3*x3);
tmp1 := 6 g3 (-i2 + 2 f1)
> elimsolve (tmp1,i2);
{-1 ≠ 0}
i2 is set to:
2 f1
> tmp1 := dtcoeff (x1*x2^5);
tmp1 := 3 g3 (d2 e1 + 2 h1)
> elimsolve (tmp1,h1);
{2 ≠ 0}
h1 is set to:

$$-\frac{d2 e1}{2}$$

> tmp1 := dtcoeff (x1*x2^4*x3);
tmp1 := 6 g3 (2 i1 + d2 f1)
> elimsolve (tmp1,i1);
{2 ≠ 0}
i1 is set to:

$$-\frac{d2 f1}{2}$$

> tmp1 := dtcoeff (x2^3*x3^3);
tmp1 := -12 f1^2 g3
> elimsolve (tmp1,f1);
{1 ≠ 0}

```

```

f1 is set to:
0
> tmp1 := dtcoeff (x2^5*x3);
                                 $tmp1 := -6 e l^2 g3$ 
> elimsolve (tmp1,e1);
                                {1 ≠ 0}
e1 is set to:
0
> [seq(diff(H[i],x3),i=1..3)];
                                [0,0,0]
> contradict (1);
Contradiction on case level 1, so:
                                 $g3 = 0$ 
Variables to be uneliminated:
                                "e1 := 'e1'"
                                "f1 := 'f1'"
                                "i1 := 'i1'"
                                "h1 := 'h1'"
                                "i2 := 'i2'"
                                "h2 := 'h2'"
                                "j1 := 'j1'"
                                "e2 := 'e2'"
                                "f2 := 'f2'"
                                "j2 := 'j2'"
Proceed on case level 0 with:
                                 $6 \neq 0$ 
On account of:
                                 $g3 = 0$ 
                                {1 ≠ 0}
g3 is set to:
0
> H[3];
0
> contradict (1);
Contradiction on case level 0, so:
                                 $6 = 0$ 
Variables to be uneliminated:
                                "g3 := 'g3'"
                                "d3 := 'd3'"
                                "i3 := 'i3'"
                                "h3 := 'h3'"
                                "j3 := 'j3'"
                                "f3 := 'f3'"

```

"e3 := 'e3'"

That is all, folks! Check that all variables are uneliminated:

$[[a_1, b_1, c_1, d_1, e_1, f_1, g_1, h_1, i_1, j_1], [a_2, b_2, c_2, d_2, e_2, f_2, g_2, h_2, i_2, j_2],$   
 $[a_3, b_3, c_3, d_3, e_3, f_3, g_3, h_3, i_3, j_3]]$

>
