# Supplementary material for: Computations of Keller maps over fields with $\tfrac16$
Source: arXiv:1609.09753 ancillary file (2017-11-02)
Supplement: Supplementary file 2 [file dim3qrt.pdf]

```

[ > restart;
  > efactors := proc (eq)
  >   local F, IF, i, c;
  >   F := factors (eq);
  >   for i from 1 to nops(F[2]) do
  >     c := content (F[2][i][1]);
  >     F[2][i][1] := F[2][i][1] / c;
  >     F[1] := F[1] * c ^ F[2][i][2];
  >   od;
  >   IF := ifactors (F[1]);
  >   return (IF[1], [op(IF[2]), op(F[2])]);
  > end;

```

*efactors* := **proc**(eq)

**local** F, IF, i, c;

F := factors(eq);

**for** i **to** nops(F[2]) **do**

c := content(F[2][i][1]);

F[2][i][1] := F[2][i][1] / c;

F[1] := F[1]\*c^F[2][i][2]

**end do**;

IF := ifactors(F[1]);

**return** IF[1], [op(IF[2]), op(F[2])]

**end proc**

```

[ > psqf := proc (eq)
  >   local EF, S, i;
  >   EF := efactors (eq);
  >   S := EF[1];
  >   for i from 1 to nops(EF[2]) do
  >     if (EF[2][i][2] > 0) then
  >       S := S * EF[2][i][1]
  >     fi
  >   od;
  >   return S
  > end;

```

*psqf* := **proc**(eq)

**local** EF, S, i;

EF := efactors(eq);

S := EF[1];

**for** i **to** nops(EF[2]) **do** **if** 0 < EF[2][i][2] **then** S := S\*EF[2][i][1] **end if** **end do**;

**return** S

**end proc**

```

[ > initcases := proc ()
  >   global nz, NZ, SV;

```

```

>  if nargs = 0 then
>      nz := 1
>  else
>      nz := args[1];
>      printf ("We assume the following in our calculation:");
>      print (psqf (nz) <> 0);
>  fi;
>  NZ := [convert (nz,string)];
>  SV := [[]];
>  return
> end;

```

*initcases* := **proc**()

**global** *nz, NZ, SV*;

**if** nargs = 0 **then** *nz* := 1

**else**

*nz* := args[ 1 ];

        printf ("We assume the following in our calculation:");

        print(psqf(*nz*) ≠ 0)

**end if**;

*NZ* := [ convert(*nz*, *string*) ];

*SV* := [ [ ] ];

**return**

**end proc**

> **launchNZcase** := **proc** (*nz*)

>   **global** *NZ, SV*;

>   **local** *t*;

>   *NZ* := [seq(*NZ*[*i*], *i*=1..*nops*(*NZ*)), convert (*nz*,*string*)];

>   *SV* := [seq(*SV*[*i*], *i*=1..*nops*(*SV*)), [ ]];

>   printf ("Launching case level %d:", *nops*(*NZ*) - 1);

>   print (*nz* <> 0);

>   printf ("Assume from now on that:");

>   *t* := mul (psqf (parse (*NZ*[*i*],*statement*)), *i*=1..*nops*(*NZ*));

>   print (*t* <> 0)

> **end**;

*launchNZcase* := **proc**(*nz*)

**local** *t*;

**global** *NZ, SV*;

*NZ* := [ seq(*NZ*[ *i* ], *i* = 1 .. *nops*(*NZ*)), convert(*nz*, *string*) ];

*SV* := [ seq(*SV*[ *i* ], *i* = 1 .. *nops*(*SV*)), [ ] ];

    printf ("Launching case level %d:", *nops*(*NZ*) - 1);

    print(*nz* ≠ 0);

    printf ("Assume from now on that:");

```

t := mul(psqf(parse(NZ[i], statement)), i = 1 .. nops(NZ));
print(t ≠ 0)

```

**end proc**

```

> contradict := proc (eq)
>   global NZ, SV, alph;
>   local t, EF, i, sv, nz;
>   t := mul (psqf (parse (NZ[i], statement)), i=1..nops(NZ));
>   EF := efactors (psqf (psqf (eq) / t));
>   if EF[1] = 0 or nops (EF[2]) > 0 then
>     error "No contradiction: 'eq' might be zero!"
>   fi;
>   printf ("Contradiction on case level %d, so:", nops(NZ) - 1);
>   for i from 1 to nops(SV[nops(SV)]) do
>     sv := cat (SV[nops(SV)][i], " := ");
>     sv := cat (sv, SV[nops(SV)][i], "");
>     parse (sv, statement)
>   od;
>   nz := parse (NZ[nops(NZ)], statement);
>   print (nz = 0);
>   if nops(SV[nops(SV)]) > 0 then
>     printf ("Variables to be uneliminated:");
>     for i from 1 to nops(SV[nops(SV)]) do
>       sv := cat (SV[nops(SV)][i], " := ");
>       sv := cat (sv, SV[nops(SV)][i], "");
>       print (sv);
>     od
>   fi;
>   if nops(NZ) <= 1 then
>     printf ("That is all, folks! ");
>     printf ("Check that all variables are uneliminated:");
>     print (alph);
>     return
>   fi;
>   NZ := [seq(NZ[i], i=1..nops(NZ)-1)];
>   SV := [seq(SV[i], i=1..nops(SV)-1)];
>   printf ("Proceed on case level %d with:", nops(NZ) - 1);
>   t := mul (psqf (parse (NZ[i], statement)), i=1..nops(NZ));
>   print (t <> 0);
>   printf ("On account of:");
>   print (nz = 0);
>   if nargs = 1 and nops(indets(nz)) = 1 and degree (nz) = 1 then
>     EF := efactors (psqf (psqf (coeff (nz, indets(nz)[1])) / t));
>     if nops (EF[2]) = 0 then
>       elimsolve(nz, indets(nz)[1]);
>       return
>     fi;
>   fi;

```

```

>   elif nargs > 1 then
>       elimsolve (nz, args[2]);
>       return
>   fi;
>   printf ("the following return value %s",
>           "can be used as an equation:");
>   return nz
> end;

contradict := proc(eq)
local t, EF, i, sv, nz;
global NZ, SV, alph;

    t := mul(psqf(parse(NZ[i], statement)), i = 1 .. nops(NZ));
    EF := efactors(psqf(psqf(eq) / t));
    if EF[1] = 0 or 0 < nops(EF[2]) then error "No contradiction: 'eq' might be zero!"
    end if;
    printf("Contradiction on case level %d, so:", nops(NZ) - 1);
    for i to nops(SV[nops(SV)]) do
        sv := cat(SV[nops(SV)][i], " := ");
        sv := cat(sv, SV[nops(SV)][i], "");
        parse(sv, statement)
    end do;
    nz := parse(NZ[nops(NZ)], statement);
    print(nz = 0);
    if 0 < nops(SV[nops(SV)]) then
        printf("Variables to be uneliminated:");
        for i to nops(SV[nops(SV)]) do
            sv := cat(SV[nops(SV)][i], " := ");
            sv := cat(sv, SV[nops(SV)][i], "");
            print(sv)
        end do
    end if;
    if nops(NZ) ≤ 1 then
        printf("That is all, folks! ");
        printf("Check that all variables are uneliminated:");
        print(alph);
        return
    end if;
    NZ := [seq(NZ[i], i = 1 .. nops(NZ) - 1)];
    SV := [seq(SV[i], i = 1 .. nops(SV) - 1)];
    printf("Proceed on case level %d with:", nops(NZ) - 1);

```

```

t := mul(psqf(parse(NZ[i], statement)), i = 1 .. nops(NZ));
print(t ≠ 0);
printf("On account of:");
print(nz = 0);
if nargs = 1 and nops(indets(nz)) = 1 and degree(nz) = 1 then
    EF := efactors(psqf(psqf(coeff(nz, indets(nz)[1]) / t));
    if nops(EF[2]) = 0 then elimsolve(nz, indets(nz)[1]); return end if
elif 1 < nargs then elimsolve(nz, args[2]); return
end if;
printf("the following return value %s", "can be used as an equation:");
return nz

```

**end proc**

```

> elimsolve := proc (eq, v)
>   global NZ, SV;
>   local t, EF, i, c1, c0, NZref, sv, F;
>   if not ({v} subset indets(v)) then
>     error "Second argument 'v' is not a variable!";
>   fi;
>   t := mul (psqf (parse (NZ[i], statement)), i=1..nops(NZ));
>   EF := efactors (psqf (psqf (eq) / t));
>   if EF[1] = 0 then error "First argument 'eq' is zero!" fi;
>   if nops(EF[2]) = 0 then
>     error "Contradiction: call 'contradict'!"
>   fi;
>   if nops(EF[2]) > 1 then
>     error "'eq' has different factors which may be zero!"
>   fi;
>   if degree (EF[2][1][1], v) <> 1 then
>     error "Degree of 'eq' w.r.t 'v' is not one!"
>   fi;
>   c1 := coeff(EF[2][1][1], v, 1);
>   c0 := coeff(EF[2][1][1], v, 0);
>   EF := efactors (psqf (psqf (c1) / t));
>   if nops(EF[2]) > 0 then
>     error "Coefficient of 'v' in 'eq' might be zero!"
>   fi;
>   EF := efactors (psqf (psqf (denom(eq)) / t));
>   if nops(EF[2]) > 0 then
>     error "Denominator of argument 'eq' may be zero!"
>   fi;
>   print ({c1 <> 0});
>   NZref := false;
>   for i from 1 to nops(NZ) do
>     NZref :=

```

```

>      NZref or ({v} subset indets (parse (NZ[i],statement)));
> od;
> sv := convert (v, string);
> F := factor (-c0/c1);
> SV[nops(SV)] :=
>   [sv, seq(SV[nops(SV)][i], i=1..nops(SV[nops(SV)]))];
> printf ("%s is set to:", sv);
> sv := cat (sv, " := ", convert (F, string));
> print (parse (sv,statement));
> if NZref then
>   printf ("Nonzero constraint refines to:");
>   t := mul (psqf (parse (NZ[i],statement)), i=1..nops (NZ));
>   print (t <> 0)
> fi;
> return
> end;

```

*elimsolve* := **proc**(*eq*, *v*)

**local** *t*, *EF*, *i*, *c1*, *c0*, *NZref*, *sv*, *F*;

**global** *NZ*, *SV*;

**if not** { *v* } subset indets(*v*) **then error** "Second argument 'v' is not a variable!" **end if**;

*t* := mul(psqf(parse(*NZ*[*i*], *statement*)), *i* = 1 .. nops(*NZ*));

*EF* := efactors(psqf(psqf(*eq*) / *t*));

**if** *EF*[1] = 0 **then error** "First argument 'eq' is zero!" **end if**;

**if** nops(*EF*[2]) = 0 **then error** "Contradiction: call 'contradict'!" **end if**;

**if** 1 < nops(*EF*[2]) **then error** "'eq' has different factors which may be zero!" **end if**;

**if** degree(*EF*[2][1][1], *v*) ≠ 1 **then error** "Degree of 'eq' w.r.t 'v' is not one!" **end if**;

*c1* := coeff(*EF*[2][1][1], *v*, 1);

*c0* := coeff(*EF*[2][1][1], *v*, 0);

*EF* := efactors(psqf(psqf(*c1*) / *t*));

**if** 0 < nops(*EF*[2]) **then error** "Coefficient of 'v' in 'eq' might be zero!" **end if**;

*EF* := efactors(psqf(psqf(denom(*eq*)) / *t*));

**if** 0 < nops(*EF*[2]) **then error** "Denominator of argument 'eq' may be zero!" **end if**;

print({ *c1* ≠ 0 });

*NZref* := *false*;

**for** *i* to nops(*NZ*) **do** *NZref* := *NZref* or { *v* } subset indets(parse(*NZ*[*i*], *statement*))  
**end do**;

*sv* := convert(*v*, *string*);

*F* := factor(-*c0* / *c1*);

*SV*[nops(*SV*)] := [sv, seq(*SV*[nops(*SV*)] [*i*], *i* = 1 .. nops(*SV*[nops(*SV*)]))];

printf ("%s is set to:", sv);

*sv* := cat(*sv*, " := ", convert(*F*, *string*));

```

print(parse(sv, statement));
if NZref then
    printf("Nonzero constraint refines to:");
    t := mul(psqf(parse(NZ[i], statement)), i = 1 .. nops(NZ));
    print(t ≠ 0)
end if;
return

```

**end proc**

```

> initcpcoeff := proc (cp)
>   global x1, x2, x3, T, S, n;
>   local m, i, j, k, cp1, cp2, cp3;
>   S := Array (0..(deg-1)*n, 0..(deg-1)*n, 0..(deg-1)*n,
>               0..n, storage=sparse);
>   for m from 0 to n-1 do
>     cp1 := coeff (cp, T, m);
>     for i from 0 to (deg-1)*(n-m) do
>       cp2 := coeff (cp1, x1, i);
>       for j from 0 to (deg-1)*(n-m)-i do
>         cp3 := coeff (cp2, x2, j);
>         k := (deg-1)*(n-m)-i-j;
>         S[i,j,k,m] := coeff (cp3, x3, k);
>       od
>     od
>   od;
>   return
> end;

```

*initcpcoeff* := **proc**(cp)

**local** m, i, j, k, cp1, cp2, cp3;

**global** x1, x2, x3, T, S, n;

S := Array(0 .. (deg - 1)\*n, 0 .. (deg - 1)\*n, 0 .. (deg - 1)\*n, 0 .. n, storage = sparse);

**for** m **from** 0 **to** n - 1 **do**

cp1 := coeff(cp, T, m);

**for** i **from** 0 **to** (deg - 1)\*(n - m) **do**

cp2 := coeff(cp1, x1, i);

**for** j **from** 0 **to** (deg - 1)\*(n - m) - i **do**

cp3 := coeff(cp2, x2, j);

k := (deg - 1)\*(n - m) - i - j;

S[i, j, k, m] := coeff(cp3, x3, k)

**end do**

**end do**

**end do**;

**return**

**end proc**

```
> cpcoeff := proc (t)
>   global x1, x2, x3, T, S;
>   local m, i, j, k;
>   m := degree (t, T);
>   i := degree (t, x1);
>   j := degree (t, x2);
>   k := degree (t, x3);
>   factor (S[i,j,k,m])
> end;
```

*cpcoeff* := **proc**(*t*)

**local** *m, i, j, k*;

**global** *x1, x2, x3, T, S*;

*m* := degree(*t*, *T*);

*i* := degree(*t*, *x1*);

*j* := degree(*t*, *x2*);

*k* := degree(*t*, *x3*);

factor(*S*[*i, j, k, m*])

**end proc**

```
> n := 3;
```

*n* := 3

```
> deg := 4;
```

*deg* := 4

```
> alph :=
```

```
> [[a1,b1,c1,d1,e1,f1,g1,h1,i1,j1,k1,l1,m1,n1,o1],
```

```
> [a2,b2,c2,d2,e2,f2,g2,h2,i2,j2,k2,l2,m2,n2,o2],
```

```
> [a3,b3,c3,d3,e3,f3,g3,h3,i3,j3,k3,l3,m3,n3,o3]];
```

*alph* := [[*a1, b1, c1, d1, e1, f1, g1, h1, i1, j1, k1, l1, m1, n1, o1*],

[*a2, b2, c2, d2, e2, f2, g2, h2, i2, j2, k2, l2, m2, n2, o2*],

[*a3, b3, c3, d3, e3, f3, g3, h3, i3, j3, k3, l3, m3, n3, o3*]]

```
> terms := [x1^4,x1^3*x2,x1^3*x3,x1^2*x2^2,x1^2*x2*x3,
```

```
> x1^2*x3^2,x1*x2^3,x1*x2^2*x3,x1*x2*x3^2,x1*x3^3,
```

```
> x2^4,x2^3*x3,x2^2*x3^2,x2*x3^3,x3^4];
```

*terms* := [*x1*<sup>4</sup>,*x1*<sup>3</sup> *x2*,*x1*<sup>3</sup> *x3*,*x1*<sup>2</sup> *x2*<sup>2</sup>,*x1*<sup>2</sup> *x2* *x3*,*x1*<sup>2</sup> *x3*<sup>2</sup>,*x1* *x2*<sup>3</sup>,*x1* *x2*<sup>2</sup> *x3*,*x1* *x2* *x3*<sup>2</sup>,*x1* *x3*<sup>3</sup>,  
*x2*<sup>4</sup>,*x2*<sup>3</sup> *x3*,*x2*<sup>2</sup> *x3*<sup>2</sup>,*x2* *x3*<sup>3</sup>,*x3*<sup>4</sup>]

```
> M := evalm ([ [0,0,0], [1,0,0], [0,1,0] ] );
```

$$M := \begin{bmatrix} 0 & 0 & 0 \\ 1 & 0 & 0 \\ 0 & 1 & 0 \end{bmatrix}$$

```
> H := Vector (evalm (M &* [seq(terms[k]/degree(terms[k]),
```

```
> [x1,x2,x3][k]),k=1..n)] +
```

```
> ['add (alph[l,k]*terms[k],k=n+1..nops(terms))'$l=1..n]));
```



$$H := \left[ d1 x1^2 x2^2 + e1 x1^2 x2 x3 + f1 x1^2 x3^2 + g1 x1 x2^3 + h1 x1 x2^2 x3 + i1 x1 x2 x3^2 \right. \\ + j1 x1 x3^3 + k1 x2^4 + l1 x2^3 x3 + m1 x2^2 x3^2 + n1 x2 x3^3 + o1 x3^4, \frac{x1^4}{4} + d2 x1^2 x2^2 \\ + e2 x1^2 x2 x3 + f2 x1^2 x3^2 + g2 x1 x2^3 + h2 x1 x2^2 x3 + i2 x1 x2 x3^2 + j2 x1 x3^3 + k2 x2^4 \\ + l2 x2^3 x3 + m2 x2^2 x3^2 + n2 x2 x3^3 + o2 x3^4, x1^3 x2 + d3 x1^2 x2^2 + e3 x1^2 x2 x3 + f3 x1^2 x3^2 \\ + g3 x1 x2^3 + h3 x1 x2^2 x3 + i3 x1 x2 x3^2 + j3 x1 x3^3 + k3 x2^4 + l3 x2^3 x3 + m3 x2^2 x3^2 \\ \left. + n3 x2 x3^3 + o3 x3^4 \right]$$

```
> with (linalg):
```

```
Warning, the protected names norm and trace have been redefined and unprotected
```

```
> JH := jacobian (H, [x1,x2,x3]):
```

```
> cp := expand (det (T-JH)-T^n):
```

```
> initcpcoeff (cp);
```

```
> initcases (6);
```

```
We assume the following in our calculation:
```

$$6 \neq 0$$

```
> for i from 2 by -1 to 0 do
```

```
>   for j from 3-i by -1 to 0 do
```

```
>     v := coeff (coeff (coeff (H[3],x1,i),x2,j),x3,4-i-j);
```

```
>     m := cpcoeff (x1^i * x2^j * x3^(3-i-j) * T^2);
```

```
>     elimsolve (m,v);
```

```
>   od;
```

```
> od;
```

$$\{1 \neq 0\}$$

```
e3 is set to:
```

$$-2 d2$$

$$\{2 \neq 0\}$$

```
f3 is set to:
```

$$-\frac{e2}{2}$$

$$\{1 \neq 0\}$$

```
h3 is set to:
```

$$-2 d1 - 3 g2$$

$$\{1 \neq 0\}$$

```
i3 is set to:
```

$$-h2 - e1$$

$$\{3 \neq 0\}$$

```
j3 is set to:
```

$$-\frac{i2}{3} - \frac{2 f1}{3}$$

$$\{1 \neq 0\}$$

l3 is set to:

$$\frac{-4 k^2 - g l}{\{2 \neq 0\}}$$

m3 is set to:

$$-\frac{3 l^2}{2} - \frac{h l}{2}$$
$$\{3 \neq 0\}$$

n3 is set to:

$$-\frac{2 m^2}{3} - \frac{i l}{3}$$
$$\{4 \neq 0\}$$

o3 is set to:

$$-\frac{n^2}{4} - \frac{j l}{4}$$

```
> for i from 2 by -1 to 0 do
>   for j from 3-i by -1 to 0 do
>     v := coeff (coeff (coeff (H[2],x1,i),x2,j),x3,4-i-j);
>     m := cpcoeff (x1^(i+3) * x2^j * x3^(3-i-j) * T);
>     elimsolve (m,v);
>   od;
> od;
```

$$\{1 \neq 0\}$$

e2 is set to:

$$\frac{-2 d l}{\{2 \neq 0\}}$$

f2 is set to:

$$-\frac{e l}{2}$$
$$\{1 \neq 0\}$$

h2 is set to:

$$\frac{-4 d^2 + 4 d l d^3 - 3 g l - 3 e l}{\{1 \neq 0\}}$$

i2 is set to:

$$\frac{2 d^2 d l + d^3 e l - 3 f l - h l}{\{3 \neq 0\}}$$

j2 is set to:

$$-\frac{2 d^2 e l}{3} - \frac{4 d l^2}{3} - \frac{i l}{3}$$
$$\{1 \neq 0\}$$

l2 is set to:

$$\frac{-3 h l + 4 d^3 e l - 4 k l - 8 d^2 d l - 12 g^2 d^2 + 6 d l g^3 + 8 d^3 d^2 - 8 d l d^3 + 6 d^3 g l}{\{2 \neq 0\}}$$

m2 is set to:

$$4 d3 f1 + 2 d1^2 + 8 d2 e1 - 3 i1 - \frac{3 l1}{2} + 12 d2^3 - 16 d2 d1 d3 + 9 g1 d2 + \frac{3 g3 e1}{2} - 2 d3^2 e1 + 2 d3 h1$$

$$\{3 \neq 0\}$$

n2 is set to:

$$-8 d1 d2^2 + \frac{2 d3 i1}{3} - 2 g2 e1 + \frac{4 d2 d3 e1}{3} - \frac{2 m1}{3} - 3 j1 + \frac{4 d2 f1}{3} + \frac{32 d1^2 d3}{3} - 6 d1 g1 - \frac{16 d1 e1}{3}$$

$$\{4 \neq 0\}$$

o2 is set to:

$$-3 f1 d1 - \frac{n1}{4} + \frac{3 e1^2}{4} - \frac{d2 i1}{2} + \frac{3 e1 g1}{4} - d1 h1$$

```
> for i from 2 by -1 to 0 do
>   for j from 3-i by -1 to 0 do
>     v := coeff (coeff (coeff (H[1],x1,i),x2,j),x3,4-i-j);
>     m := cpcoeff (x1^(i+6) * x2^j * x3^(3-i-j));
>     elimsolve (m,v);
>   od;
> od;
```

$$\{1 \neq 0\}$$

e1 is set to:

$$0$$

$$\{1 \neq 0\}$$

f1 is set to:

$$0$$

$$\{1 \neq 0\}$$

h1 is set to:

$$-4 d2 d1$$

$$\{1 \neq 0\}$$

i1 is set to:

$$2 d1^2$$

$$\{1 \neq 0\}$$

j1 is set to:

$$0$$

$$\{1 \neq 0\}$$

l1 is set to:

$$-6 g1 d2 + 4 d1^2 - 6 d1 g2 + 8 d2 d1 d3$$

$$\{1 \neq 0\}$$

m1 is set to:

$$3 d1 (4 d2^2 - 4 d1 d3 + 3 g1)$$

$$\{1 \neq 0\}$$

n1 is set to:

```

                                
$$\begin{matrix} -8\,d2\,d1^2 \\ \{1 \neq 0\} \end{matrix}$$

d1 is set to:
                                
$$d1^3$$

> launchNZcase (d1);
Launching case level 1:
                                
$$d1 \neq 0$$

Assume from now on that:
                                
$$6\,d1 \neq 0$$

> tmp1 := cpcoeff (x1^5*x2*x3^3);
                                
$$tmp1 := 12\,d1^2\,(-8\,d1\,d3 + 8\,d2^2 + 5\,g1)$$

> elimsolve (tmp1, d3);
                                
$$\{-8\,d1 \neq 0\}$$

d3 is set to:
                                
$$\frac{8\,d2^2 + 5\,g1}{8\,d1}$$

> tmp1 := cpcoeff (x1^5*x2^2*x3^2);
                                
$$tmp1 := 6\,d1\,(16\,d1^2 - 9\,d1\,g2 + 32\,d2^3 + 3\,g1\,d2)$$

> elimsolve (tmp1, g2);
                                
$$\{-9\,d1 \neq 0\}$$

g2 is set to:
                                
$$\frac{16\,d1^2 + 32\,d2^3 + 3\,g1\,d2}{9\,d1}$$

> tmp1 := cpcoeff (x1^5*x2^3*x3);
                                
$$tmp1 := \frac{224\,d2\,d1^2}{3} - 48\,g3\,d1^2 + 32\,k1\,d1 + 24\,g1\,d2^2 + \frac{928\,d2^4}{3} - \frac{9\,g1^2}{2}$$

> elimsolve (tmp1, k1);
                                
$$\{192\,d1 \neq 0\}$$

k1 is set to:
                                
$$\frac{-448\,d2\,d1^2 + 288\,g3\,d1^2 - 144\,g1\,d2^2 - 1856\,d2^4 + 27\,g1^2}{192\,d1}$$

> tmp1 := cpcoeff (x1^5*x2^4);
                                
$$tmp1 := -\frac{192\,d1^2\,k2 - 56\,d1^2\,g1 + 80\,d2^3\,g1 - 384\,d2^2\,d1^2 - 2496\,d2^5 + 9\,g1^2\,d2}{24\,d1}$$

> elimsolve (tmp1, k2);
                                
$$\{192\,d1^2 \neq 0\}$$

k2 is set to:
                                
$$-\frac{-56\,d1^2\,g1 + 80\,d2^3\,g1 - 384\,d2^2\,d1^2 - 2496\,d2^5 + 9\,g1^2\,d2}{192\,d1^2}$$

> tmp1 := cpcoeff (x1^2*x2^2*x3^2*T);
                                
$$tmp1 := 48\,d2^4 - \frac{9\,g1^2}{4} + 72\,d2\,d1^2 + 18\,g3\,d1^2$$


```

> **elimsolve** (tmp1,g3);

$$\{-24 d l^2 \neq 0\}$$

g3 is set to:

$$\frac{-64 d^2 + 3 g l^2 - 96 d^2 d l^2}{24 d l^2}$$

> **tmp1 := cpcoeff** (x1^2\*x2^4\*T);

$$tmp1 := (-216 g l^2 d^2 - 15360 d l^4 - 180736 d^6 + 63 g l^3 + 4608 d l^3 k3 - 7872 d^2 g l - 4608 g l d^2 d l^2 - 63488 d^3 d l^2) / (576 d l^2)$$

> **elimsolve** (tmp1,k3);

$$\{4608 d l^3 \neq 0\}$$

k3 is set to:

$$-(-216 g l^2 d^2 - 15360 d l^4 - 180736 d^6 + 63 g l^3 - 7872 d^2 g l - 4608 g l d^2 d l^2 - 63488 d^3 d l^2) / (4608 d l^3)$$

> **tmp1 := cpcoeff** (x1^2\*x3^4\*T);

$$tmp1 := 5 d l^2 (4 d^2 + g l)$$

> **tmp2 := cpcoeff** (x1^2\*x2^3\*x3\*T);

$$tmp2 := -d l (-184 d^2 + 17 g l)$$

> **tmp3 := factor**(3 \* tmp1 + d1 \* tmp2);

$$tmp3 := -2 d l^2 (-122 d^2 + g l)$$

> **elimsolve** (tmp3, g1);

$$\{1 \neq 0\}$$

g1 is set to:

$$122 d^2$$

> **tmp1 := cpcoeff** (x1^5\*x3^4);

$$tmp1 := -20 d^2 d l^3$$

> **tmp2 := cpcoeff** (x1^4\*x3^5);

$$tmp2 := -326 d^2 d l^3$$

> **tmp3 := factor**(tmp2 - 16\*d2 \* tmp1);

$$tmp3 := -6 d^2 d l^3$$

> **elimsolve** (tmp3, d2);

$$\{1 \neq 0\}$$

d2 is set to:

$$0$$

> **tmp1 := cpcoeff** (x1\*x3^5\*T);

$$tmp1 := -32 d l^4$$

> **contradict** (tmp1);

Contradiction on case level 1, so:

$$d l = 0$$

Variables to be uneliminated:

$$"d2 := 'd2'"$$

$$"g1 := 'g1'"$$

```

                                "k3 := 'k3'"
                                "g3 := 'g3'"
                                "k2 := 'k2'"
                                "k1 := 'k1'"
                                "g2 := 'g2'"
                                "d3 := 'd3'"

Proceed on case level 0 with:

                                 $6 \neq 0$ 

On account of:

                                 $d1 = 0$ 
                                 $\{1 \neq 0\}$ 

d1 is set to:

                                0

> launchNZcase (d2);
Launching case level 1:

                                 $d2 \neq 0$ 

Assume from now on that:

                                 $6 d2 \neq 0$ 

> tmp1 := cpcoeff (x1^5*x2^4);
                                 $tmp1 := 12 d3 g1 d2 - 9 g1 g2 - 8 d2 k1$ 

> elimsolve (tmp1,k1);
                                 $\{8 d2 \neq 0\}$ 

k1 is set to:

                                 $\frac{3 g1 (4 d3 d2 - 3 g2)}{8 d2}$ 

> tmp1 := cpcoeff (x1^2*x2^4*T);
                                 $tmp1 := (10 g1 d2^2 - 9 g2^2 d2 + 12 g3 d2^3 + 9 g3 d2 g1 - 9 d3 g1 g2 + 24 d3 g2 d2^2$ 
                                 $- 16 d3^2 d2^3 - 16 k2 d2^2) / d2$ 

> elimsolve (tmp1,k2);
                                 $\{-16 d2^2 \neq 0\}$ 

k2 is set to:

                                 $\frac{10 g1 d2^2 - 9 g2^2 d2 + 12 g3 d2^3 + 9 g3 d2 g1 - 9 d3 g1 g2 + 24 d3 g2 d2^2 - 16 d3^2 d2^3}{16 d2^2}$ 

> launchNZcase (g1);
Launching case level 2:

                                 $g1 \neq 0$ 

Assume from now on that:

                                 $6 g1 d2 \neq 0$ 

> tmp1 := cpcoeff (x1^5*x2^3*x3);
                                 $tmp1 := 6 g1 (8 d2^2 + 3 g1)$ 

> elimsolve (tmp1,g1);
                                 $\{3 \neq 0\}$ 

g1 is set to:

```

$$-\frac{8 d2^2}{3}$$

Nonzero constraint refines to:

$$-12 d2^2 \neq 0$$

**> tmp1 := cpcoeff (x1^2\*x2^2\*x3^2\*T);**

$$tmp1 := 96 d2^4$$

**> contradict (tmp1);**

Contradiction on case level 2, so:

$$g1 = 0$$

Variables to be uneliminated:

"g1 := 'g1'"

Proceed on case level 1 with:

$$6 d2 \neq 0$$

On account of:

$$g1 = 0$$

$$\{1 \neq 0\}$$

g1 is set to:

$$0$$

**> tmp1 := cpcoeff (x1^2\*x2^2\*x3^2\*T);**

$$tmp1 := -96 d2^4$$

**> contradict (tmp1);**

Contradiction on case level 1, so:

$$d2 = 0$$

Variables to be uneliminated:

"g1 := 'g1'"

"k2 := 'k2'"

"k1 := 'k1'"

Proceed on case level 0 with:

$$6 \neq 0$$

On account of:

$$d2 = 0$$

$$\{1 \neq 0\}$$

d2 is set to:

$$0$$

**> tmp1 := cpcoeff (x1^5\*x2^3\*x3);**

$$tmp1 := 18 g1^2$$

**> elimsolve (tmp1,g1);**

$$\{1 \neq 0\}$$

g1 is set to:

$$0$$

**> launchNZcase (g2);**

Launching case level 1:

$$g2 \neq 0$$

Assume from now on that:

$$6 g2 \neq 0$$

```

> tmp1 := cpcoeff (x1^4*x2^5);
                                     tmp1 := -12 g2 k1
> elimsolve (tmp1,k1);
                                     { 1 ≠ 0 }
k1 is set to:
                                     0
> tmp1 := cpcoeff (x1^2*x2^4*T);
                                     tmp1 := -9 g2^2
> contradict (tmp1);
Contradiction on case level 1, so:
                                     g2 = 0
Variables to be uneliminated:
                                     "k1 := 'k1'"
Proceed on case level 0 with:
                                     6 ≠ 0
On account of:
                                     g2 = 0
                                     { 1 ≠ 0 }
g2 is set to:
                                     0
> tmp1 := cpcoeff (x1^3*x2^5*x3);
                                     tmp1 := 48 k1^2
> elimsolve (tmp1,k1);
                                     { 1 ≠ 0 }
k1 is set to:
                                     0
> tmp1 := cpcoeff (x2^6*T);
                                     tmp1 := -16 k2^2
> elimsolve (tmp1,k2);
                                     { 1 ≠ 0 }
k2 is set to:
                                     0
> jacobian(H, [x1,x2,x3]);
                                     0           0           0
                                     x1^3         0           0
[ 3 x1^2 x2 + 2 d3 x1 x2^2 + g3 x2^3  x1^3 + 2 d3 x1^2 x2 + 3 g3 x1 x2^2 + 4 k3 x2^3  0 ]
> contradict (1);
Contradiction on case level 0, so:
                                     6 = 0
Variables to be uneliminated:
                                     "k2 := 'k2'"
                                     "k1 := 'k1'"
                                     "g2 := 'g2'"
                                     "g1 := 'g1'"

```



```

"d2 := 'd2'"
"d1 := 'd1'"
"o1 := 'o1'"
"n1 := 'n1'"
"m1 := 'm1'"
"l1 := 'l1'"
"j1 := 'j1'"
"i1 := 'i1'"
"h1 := 'h1'"
"f1 := 'f1'"
"e1 := 'e1'"
"o2 := 'o2'"
"n2 := 'n2'"
"m2 := 'm2'"
"l2 := 'l2'"
"j2 := 'j2'"
"i2 := 'i2'"
"h2 := 'h2'"
"f2 := 'f2'"
"e2 := 'e2'"
"o3 := 'o3'"
"n3 := 'n3'"
"m3 := 'm3'"
"l3 := 'l3'"
"j3 := 'j3'"
"i3 := 'i3'"
"h3 := 'h3'"
"f3 := 'f3'"
"e3 := 'e3'"

```

That is all, folks! Check that all variables are uneliminated:

```

[[a1,b1,c1,d1,e1,f1,g1,h1,i1,j1,k1,l1,m1,n1,o1],
 [a2,b2,c2,d2,e2,f2,g2,h2,i2,j2,k2,l2,m2,n2,o2],
 [a3,b3,c3,d3,e3,f3,g3,h3,i3,j3,k3,l3,m3,n3,o3]]

```

>
