# Supplementary material for: Computations of Keller maps over fields with $\tfrac16$
Source: arXiv:1609.09753 ancillary file (2017-11-02)
Supplement: Supplementary file 3 [file dim3upoqrt.pdf]

```

[ > restart;
  > efactors := proc (eq)
  >   local F, IF, i, c;
  >   F := factors (eq);
  >   for i from 1 to nops(F[2]) do
  >     c := content (F[2][i][1]);
  >     F[2][i][1] := F[2][i][1] / c;
  >     F[1] := F[1] * c ^ F[2][i][2];
  >   od;
  >   IF := ifactors (F[1]);
  >   return (IF[1], [op(IF[2]), op(F[2])]);
  > end;

```

*efactors* := **proc**(eq)

**local** F, IF, i, c;

F := factors(eq);

**for** i **to** nops(F[2]) **do**

c := content(F[2][i][1]);

F[2][i][1] := F[2][i][1] / c;

F[1] := F[1]\*c^F[2][i][2]

**end do**;

IF := ifactors(F[1]);

**return** IF[1], [op(IF[2]), op(F[2])]

**end proc**

```

[ > psqf := proc (eq)
  >   local EF, S, i;
  >   EF := efactors (eq);
  >   S := EF[1];
  >   for i from 1 to nops(EF[2]) do
  >     if (EF[2][i][2] > 0) then
  >       S := S * EF[2][i][1]
  >     fi
  >   od;
  >   return S
  > end;

```

*psqf* := **proc**(eq)

**local** EF, S, i;

EF := efactors(eq);

S := EF[1];

**for** i **to** nops(EF[2]) **do** **if** 0 < EF[2][i][2] **then** S := S\*EF[2][i][1] **end if** **end do**;

**return** S

**end proc**

```

[ > initcases := proc ()
  >   global nz, NZ, SV;

```

```

>   if nargs = 0 then
>       nz := 1
>   else
>       nz := args[1];
>       printf ("We assume the following in our calculation:");
>       print (psqf (nz) <> 0);
>   fi;
>   NZ := [convert (nz,string)];
>   SV := [[]];
>   return
> end;

```

*initcases* := **proc**()

**global** *nz, NZ, SV*;

**if** nargs = 0 **then** *nz* := 1

**else**

*nz* := args[ 1 ];

        printf ("We assume the following in our calculation:");

        print(psqf(*nz*) ≠ 0)

**end if**;

*NZ* := [ convert(*nz*, *string*) ];

*SV* := [ [ ] ];

**return**

**end proc**

> **launchNZcase** := **proc** (*nz*)

>     **global** *NZ, SV*;

>     **local** *t*;

>     *NZ* := [seq(*NZ*[*i*], *i*=1..*nops*(*NZ*)), convert (*nz*,*string*)];

>     *SV* := [seq(*SV*[*i*], *i*=1..*nops*(*SV*)), [ ]];

>     printf ("Launching case level %d:", *nops*(*NZ*) - 1);

>     print (*nz* <> 0);

>     printf ("Assume from now on that:");

>     *t* := mul (psqf (parse (*NZ*[*i*],*statement*)), *i*=1..*nops*(*NZ*));

>     print (*t* <> 0)

> **end**;

*launchNZcase* := **proc**(*nz*)

**local** *t*;

**global** *NZ, SV*;

*NZ* := [ seq(*NZ*[ *i* ], *i* = 1 .. *nops*(*NZ*)), convert(*nz*, *string*) ];

*SV* := [ seq(*SV*[ *i* ], *i* = 1 .. *nops*(*SV*)), [ ] ];

    printf ("Launching case level %d:", *nops*(*NZ*) - 1);

    print(*nz* ≠ 0);

    printf ("Assume from now on that:");

```

t := mul(psqf(parse(NZ[i], statement)), i = 1 .. nops(NZ));
print(t ≠ 0)

```

**end proc**

```

> contradict := proc (eq)
>   global NZ, SV, alph;
>   local t, EF, i, sv, nz;
>   t := mul (psqf (parse (NZ[i], statement)), i=1..nops(NZ));
>   EF := efactors (psqf (psqf (eq) / t));
>   if EF[1] = 0 or nops (EF[2]) > 0 then
>     error "No contradiction: 'eq' might be zero!"
>   fi;
>   printf ("Contradiction on case level %d, so:", nops(NZ) - 1);
>   for i from 1 to nops(SV[nops(SV)]) do
>     sv := cat (SV[nops(SV)][i], " := ");
>     sv := cat (sv, SV[nops(SV)][i], "");
>     parse (sv, statement)
>   od;
>   nz := parse (NZ[nops(NZ)], statement);
>   print (nz = 0);
>   if nops(SV[nops(SV)]) > 0 then
>     printf ("Variables to be uneliminated:");
>     for i from 1 to nops(SV[nops(SV)]) do
>       sv := cat (SV[nops(SV)][i], " := ");
>       sv := cat (sv, SV[nops(SV)][i], "");
>       print (sv);
>     od
>   fi;
>   if nops(NZ) <= 1 then
>     printf ("That is all, folks! ");
>     printf ("Check that all variables are uneliminated:");
>     print (alph);
>     return
>   fi;
>   NZ := [seq(NZ[i], i=1..nops(NZ)-1)];
>   SV := [seq(SV[i], i=1..nops(SV)-1)];
>   printf ("Proceed on case level %d with:", nops(NZ) - 1);
>   t := mul (psqf (parse (NZ[i], statement)), i=1..nops(NZ));
>   print (t <> 0);
>   printf ("On account of:");
>   print (nz = 0);
>   if nargs = 1 and nops(indets(nz)) = 1 and degree (nz) = 1 then
>     EF := efactors (psqf (psqf (coeff (nz, indets(nz)[1])) / t));
>     if nops (EF[2]) = 0 then
>       elimsolve(nz, indets(nz)[1]);
>       return
>     fi;
>   fi;

```

```

>   elif nargs > 1 then
>       elimsolve (nz, args[2]);
>       return
>   fi;
>   printf ("the following return value %s",
>           "can be used as an equation:");
>   return nz
> end;

contradict := proc(eq)
local t, EF, i, sv, nz;
global NZ, SV, alph;

    t := mul(psqf(parse(NZ[i], statement)), i = 1 .. nops(NZ));
    EF := efactors(psqf(psqf(eq) / t));
    if EF[1] = 0 or 0 < nops(EF[2]) then error "No contradiction: 'eq' might be zero!"
    end if;
    printf("Contradiction on case level %d, so:", nops(NZ) - 1);
    for i to nops(SV[nops(SV)]) do
        sv := cat(SV[nops(SV)][i], " := ");
        sv := cat(sv, SV[nops(SV)][i], "");
        parse(sv, statement)
    end do;
    nz := parse(NZ[nops(NZ)], statement);
    print(nz = 0);
    if 0 < nops(SV[nops(SV)]) then
        printf("Variables to be uneliminated:");
        for i to nops(SV[nops(SV)]) do
            sv := cat(SV[nops(SV)][i], " := ");
            sv := cat(sv, SV[nops(SV)][i], "");
            print(sv)
        end do
    end if;
    if nops(NZ) ≤ 1 then
        printf("That is all, folks! ");
        printf("Check that all variables are uneliminated:");
        print(alph);
        return
    end if;
    NZ := [seq(NZ[i], i = 1 .. nops(NZ) - 1)];
    SV := [seq(SV[i], i = 1 .. nops(SV) - 1)];
    printf("Proceed on case level %d with:", nops(NZ) - 1);

```

```

t := mul(psqf(parse(NZ[i], statement)), i = 1 .. nops(NZ));
print(t ≠ 0);
printf("On account of:");
print(nz = 0);
if nargs = 1 and nops(indets(nz)) = 1 and degree(nz) = 1 then
    EF := efactors(psqf(psqf(coeff(nz, indets(nz)[1])) / t));
    if nops(EF[2]) = 0 then elimsolve(nz, indets(nz)[1]); return end if
elif 1 < nargs then elimsolve(nz, args[2]); return
end if;
printf("the following return value %s", "can be used as an equation:");
return nz

```

**end proc**

```

> elimsolve := proc (eq, v)
>   global NZ, SV;
>   local t, EF, i, c1, c0, NZref, sv, F;
>   if not ({v} subset indets(v)) then
>     error "Second argument 'v' is not a variable!";
>   fi;
>   t := mul (psqf (parse (NZ[i], statement)), i=1..nops(NZ));
>   EF := efactors (psqf (psqf (eq) / t));
>   if EF[1] = 0 then error "First argument 'eq' is zero!" fi;
>   if nops(EF[2]) = 0 then
>     error "Contradiction: call 'contradict'!"
>   fi;
>   if nops(EF[2]) > 1 then
>     error "'eq' has different factors which may be zero!"
>   fi;
>   if degree (EF[2][1][1], v) <> 1 then
>     error "Degree of 'eq' w.r.t 'v' is not one!"
>   fi;
>   c1 := coeff(EF[2][1][1], v, 1);
>   c0 := coeff(EF[2][1][1], v, 0);
>   EF := efactors (psqf (psqf (c1) / t));
>   if nops(EF[2]) > 0 then
>     error "Coefficient of 'v' in 'eq' might be zero!"
>   fi;
>   EF := efactors (psqf (psqf (denom(eq)) / t));
>   if nops(EF[2]) > 0 then
>     error "Denominator of argument 'eq' may be zero!"
>   fi;
>   print ({c1 <> 0});
>   NZref := false;
>   for i from 1 to nops(NZ) do
>     NZref :=

```

```

>      NZref or ({v} subset indets (parse (NZ[i],statement)));
> od;
> sv := convert (v, string);
> F := factor (-c0/c1);
> SV[nops(SV)] :=
>   [sv, seq(SV[nops(SV)][i], i=1..nops(SV[nops(SV)]))];
> printf ("%s is set to:", sv);
> sv := cat (sv, " := ", convert (F, string));
> print (parse (sv,statement));
> if NZref then
>   printf ("Nonzero constraint refines to:");
>   t := mul (psqf (parse (NZ[i],statement)), i=1..nops (NZ));
>   print (t <> 0)
> fi;
> return
> end;

```

*elimsolve* := **proc**(eq, v)

**local** t, EF, i, c1, c0, NZref, sv, F;

**global** NZ, SV;

**if not** {v} subset indets(v) **then error** "Second argument 'v' is not a variable!" **end if**;

t := mul(psqf(parse(NZ[i], statement)), i = 1 .. nops(NZ));

EF := efactors(psqf(psqf(eq) / t));

**if** EF[1] = 0 **then error** "First argument 'eq' is zero!" **end if**;

**if** nops(EF[2]) = 0 **then error** "Contradiction: call 'contradict'!" **end if**;

**if** 1 < nops(EF[2]) **then error** "'eq' has different factors which may be zero!" **end if**;

**if** degree(EF[2][1][1], v) ≠ 1 **then error** "Degree of 'eq' w.r.t 'v' is not one!" **end if**;

c1 := coeff(EF[2][1][1], v, 1);

c0 := coeff(EF[2][1][1], v, 0);

EF := efactors(psqf(psqf(c1) / t));

**if** 0 < nops(EF[2]) **then error** "Coefficient of 'v' in 'eq' might be zero!" **end if**;

EF := efactors(psqf(psqf(denom(eq)) / t));

**if** 0 < nops(EF[2]) **then error** "Denominator of argument 'eq' may be zero!" **end if**;

print({c1 ≠ 0});

NZref := false;

**for** i **to** nops(NZ) **do** NZref := NZref or {v} subset indets(parse(NZ[i], statement))

**end do**;

sv := convert(v, string);

F := factor(-c0 / c1);

SV[nops(SV)] := [sv, seq(SV[nops(SV)][i], i = 1 .. nops(SV[nops(SV)]))];

printf ("%s is set to:", sv);

sv := cat(sv, " := ", convert(F, string));

```

print(parse(sv, statement));
if NZref then
    printf("Nonzero constraint refines to:");
    t := mul(psqf(parse(NZ[i], statement)), i = 1 .. nops(NZ));
    print(t ≠ 0)
end if;
return

```

end proc

```

> initcpcoeff := proc (cp)
>   global x1, x2, x3, T, S, n, deg;
>   local i, j, k, m, cp1, cp2, cp3;
>   S := Array (0..9, 0..9, 0..9, 0..3, storage=sparse);
>   for m from 0 to n-1 do
>       cp1 := coeff (cp, T, m);
>       for i from 0 to (deg-1)*(n-m) do
>           cp2 := coeff (cp1, x1, i);
>           for j from 0 to (deg-1)*(n-m)-i do
>               cp3 := coeff (cp2, x2, j);
>               for k from 0 to (deg-1)*(n-m)-i-j do
>                   S[i,j,k,m] := coeff (cp3, x3, k);
>               od
>           od
>       od
>   od;
>   return;
> end;

```

*initcpcoeff* := **proc**(*cp*)

**local** *i, j, k, m, cp1, cp2, cp3*;

**global** *x1, x2, x3, T, S, n, deg*;

*S* := Array(0 .. 9, 0 .. 9, 0 .. 9, 0 .. 3, *storage* = *sparse*);

**for** *m* **from** 0 **to** *n* - 1 **do**

*cp1* := coeff(*cp*, *T*, *m*);

**for** *i* **from** 0 **to** (*deg* - 1)\*(*n* - *m*) **do**

*cp2* := coeff(*cp1*, *x1*, *i*);

**for** *j* **from** 0 **to** (*deg* - 1)\*(*n* - *m*) - *i* **do**

*cp3* := coeff(*cp2*, *x2*, *j*);

**for** *k* **from** 0 **to** (*deg* - 1)\*(*n* - *m*) - *i* - *j* **do**

*S*[*i, j, k, m*] := coeff(*cp3*, *x3*, *k*)

**end do**

**end do**

**end do**

**end do**;

return

end proc

```
> cpcoeff := proc (t)
>   global x1, x2, x3, x4, T, S;
>   local i, j, k, l, m;
>   i := degree (t, x1);
>   j := degree (t, x2);
>   k := degree (t, x3);
>   m := degree (t, T);
>   factor (S[i,j,k,m]);
> end;
```

*cpcoeff* := **proc**(*t*)

**local** *i, j, k, l, m*;

**global** *x1, x2, x3, x4, T, S*;

*i* := degree(*t*, *x1*);

*j* := degree(*t*, *x2*);

*k* := degree(*t*, *x3*);

*m* := degree(*t*, *T*);

factor(*S*[*i, j, k, m*])

end proc

```
> startnewHcase := proc()
>   global remainingHcases, H, JH, cp, n;
>   local i;
>   if remainingHcases = [] then
>     printf ("No cases for H remaining; %s",
>             "all cases have been evaluated.");
>     return
>   fi;
>   printf ("Starting case H = %s:", remainingHcases[1]);
>   H := parse (remainingHcases[1]):
>   print (H):
>   remainingHcases := [seq(remainingHcases[i],
>                           i=2..nops(remainingHcases))] :
>   JH := jacobian (H, [x1,x2,x3]):
>   cp := expand (det (T-JH)-T^n):
>   initcpcoeff (cp);
> end;
```

*startnewHcase* := **proc**()

**local** *i*;

**global** *remainingHcases, H, JH, cp, n*;

**if** *remainingHcases* = [ ] **then**

printf("No cases for H remaining; %s", "all cases have been evaluated."); **return**

**end if**;

```

printf("Starting case H = %s:", remainingHcases[1]);
H := parse(remainingHcases[1]);
print(H);
remainingHcases := [seq(remainingHcases[i], i = 2 .. nops(remainingHcases))];
JH := jacobian(H, [x1, x2, x3]);
cp := expand(det(T - JH) - T^n);
initpcoeff(cp)
end proc
> n := 3;
n := 3
> deg := 4;
deg := 4
> alph :=
> [[a1, b1, c1, d1, e1, f1, g1, h1, i1, j1, k1, l1, m1, n1, o1, p1, q1, r1, s1],
> [a2, b2, c2, d2, e2, f2, g2, h2, i2, j2, k2, l2, m2, n2, o2, p2, q2, r2, s2],
> [a3, b3, c3, d3, e3, f3, g3, h3, i3, j3, k3, l3, m3, n3, o3, p3, q3, r3, s3]];
alph := [[a1, b1, c1, d1, e1, f1, g1, h1, i1, j1, k1, l1, m1, n1, o1, p1, q1, r1, s1],
[a2, b2, c2, d2, e2, f2, g2, h2, i2, j2, k2, l2, m2, n2, o2, p2, q2, r2, s2],
[a3, b3, c3, d3, e3, f3, g3, h3, i3, j3, k3, l3, m3, n3, o3, p3, q3, r3, s3]]
> terms := [x1^3, x1^2*x2, x1^2*x3, x1^2, x1*x2^2, x1*x2*x3, x1*x2,
> x1*x3^2, x1*x3, x1, x2^3, x2^2*x3, x2^2, x2*x3^2,
> x2*x3, x2, x3^3, x3^2, x3];
terms := [x1^3, x1^2 x2, x1^2 x3, x1^2, x1 x2^2, x1 x2 x3, x1 x2, x1 x3^2, x1 x3, x1, x2^3, x2^2 x3, x2^2,
x2 x3^2, x2 x3, x2, x3^3, x3^2, x3]
> H0 := ['add (alph[1,k]*terms[k], k=1..nops(terms))' $1=1..n];
H0 := [a1 x1^3 + b1 x1^2 x2 + c1 x1^2 x3 + d1 x1^2 + e1 x1 x2^2 + f1 x1 x2 x3 + g1 x1 x2 + h1 x1 x3^2
+ i1 x1 x3 + j1 x1 + k1 x2^3 + l1 x2^2 x3 + m1 x2^2 + n1 x2 x3^2 + o1 x2 x3 + p1 x2 + q1 x3^3
+ r1 x3^2 + s1 x3, a2 x1^3 + b2 x1^2 x2 + c2 x1^2 x3 + d2 x1^2 + e2 x1 x2^2 + f2 x1 x2 x3 + g2 x1 x2
+ h2 x1 x3^2 + i2 x1 x3 + j2 x1 + k2 x2^3 + l2 x2^2 x3 + m2 x2^2 + n2 x2 x3^2 + o2 x2 x3 + p2 x2
+ q2 x3^3 + r2 x3^2 + s2 x3, a3 x1^3 + b3 x1^2 x2 + c3 x1^2 x3 + d3 x1^2 + e3 x1 x2^2 + f3 x1 x2 x3
+ g3 x1 x2 + h3 x1 x3^2 + i3 x1 x3 + j3 x1 + k3 x2^3 + l3 x2^2 x3 + m3 x2^2 + n3 x2 x3^2 + o3 x2 x3
+ p3 x2 + q3 x3^3 + r3 x3^2 + s3 x3]
> H1 := Vector (evalm(H0 + [0, 1/4*x1^4, x1^3*x2
> + u3*x1^2*x2^2+v3*x1*x2^3+w3*x2^4]));
H1 := [a1 x1^3 + b1 x1^2 x2 + c1 x1^2 x3 + d1 x1^2 + e1 x1 x2^2 + f1 x1 x2 x3 + g1 x1 x2 + h1 x1 x3^2
+ i1 x1 x3 + j1 x1 + k1 x2^3 + l1 x2^2 x3 + m1 x2^2 + n1 x2 x3^2 + o1 x2 x3 + p1 x2 + q1 x3^3
+ r1 x3^2 + s1 x3, x1^4/4 + a2 x1^3 + b2 x1^2 x2 + c2 x1^2 x3 + d2 x1^2 + e2 x1 x2^2 + f2 x1 x2 x3

```

$$\begin{aligned}
& + g_2 x_1 x_2 + h_2 x_1 x_3^2 + i_2 x_1 x_3 + j_2 x_1 + k_2 x_2^3 + l_2 x_2^2 x_3 + m_2 x_2^2 + n_2 x_2 x_3^2 + o_2 x_2 x_3 \\
& + p_2 x_2 + q_2 x_3^3 + r_2 x_3^2 + s_2 x_3, x_1^3 x_2 + u_3 x_1^2 x_2^2 + v_3 x_1 x_2^3 + w_3 x_2^4 + a_3 x_1^3 \\
& + b_3 x_1^2 x_2 + c_3 x_1^2 x_3 + d_3 x_1^2 + e_3 x_1 x_2^2 + f_3 x_1 x_2 x_3 + g_3 x_1 x_2 + h_3 x_1 x_3^2 + i_3 x_1 x_3 \\
& + j_3 x_1 + k_3 x_2^3 + l_3 x_2^2 x_3 + m_3 x_2^2 + n_3 x_2 x_3^2 + o_3 x_2 x_3 + p_3 x_2 + q_3 x_3^3 + r_3 x_3^2 + s_3 x_3
\end{aligned}$$

```

> H2 := Vector (evalm (H0 + [0,1/4*x1^4
> + u2*x1^2*x3^2+v2*x1*x3^3+w2*x3^4, 0]));

```

$$\begin{aligned}
H2 := & \left[ a_1 x_1^3 + b_1 x_1^2 x_2 + c_1 x_1^2 x_3 + d_1 x_1^2 + e_1 x_1 x_2^2 + f_1 x_1 x_2 x_3 + g_1 x_1 x_2 + h_1 x_1 x_3^2 \right. \\
& + i_1 x_1 x_3 + j_1 x_1 + k_1 x_2^3 + l_1 x_2^2 x_3 + m_1 x_2^2 + n_1 x_2 x_3^2 + o_1 x_2 x_3 + p_1 x_2 + q_1 x_3^3 \\
& + r_1 x_3^2 + s_1 x_3, \frac{x_1^4}{4} + u_2 x_1^2 x_3^2 + v_2 x_1 x_3^3 + w_2 x_3^4 + a_2 x_1^3 + b_2 x_1^2 x_2 + c_2 x_1^2 x_3 \\
& + d_2 x_1^2 + e_2 x_1 x_2^2 + f_2 x_1 x_2 x_3 + g_2 x_1 x_2 + h_2 x_1 x_3^2 + i_2 x_1 x_3 + j_2 x_1 + k_2 x_2^3 \\
& + l_2 x_2^2 x_3 + m_2 x_2^2 + n_2 x_2 x_3^2 + o_2 x_2 x_3 + p_2 x_2 + q_2 x_3^3 + r_2 x_3^2 + s_2 x_3, a_3 x_1^3 \\
& + b_3 x_1^2 x_2 + c_3 x_1^2 x_3 + d_3 x_1^2 + e_3 x_1 x_2^2 + f_3 x_1 x_2 x_3 + g_3 x_1 x_2 + h_3 x_1 x_3^2 + i_3 x_1 x_3 \\
& \left. + j_3 x_1 + k_3 x_2^3 + l_3 x_2^2 x_3 + m_3 x_2^2 + n_3 x_2 x_3^2 + o_3 x_2 x_3 + p_3 x_2 + q_3 x_3^3 + r_3 x_3^2 + s_3 x_3 \right]
\end{aligned}$$

```

> remainingHcases := ["H1", "H2"];
remainingHcases := ["H1", "H2"]

```

```

> with (linalg):
Warning, the protected names norm and trace have been redefined and
unprotected

```

```

> startnewHcase ();
Starting case H = H1:

```

$$\begin{aligned}
& \left[ a_1 x_1^3 + b_1 x_1^2 x_2 + c_1 x_1^2 x_3 + d_1 x_1^2 + e_1 x_1 x_2^2 + f_1 x_1 x_2 x_3 + g_1 x_1 x_2 + h_1 x_1 x_3^2 \right. \\
& + i_1 x_1 x_3 + j_1 x_1 + k_1 x_2^3 + l_1 x_2^2 x_3 + m_1 x_2^2 + n_1 x_2 x_3^2 + o_1 x_2 x_3 + p_1 x_2 + q_1 x_3^3 \\
& + r_1 x_3^2 + s_1 x_3, \frac{x_1^4}{4} + a_2 x_1^3 + b_2 x_1^2 x_2 + c_2 x_1^2 x_3 + d_2 x_1^2 + e_2 x_1 x_2^2 + f_2 x_1 x_2 x_3 \\
& + g_2 x_1 x_2 + h_2 x_1 x_3^2 + i_2 x_1 x_3 + j_2 x_1 + k_2 x_2^3 + l_2 x_2^2 x_3 + m_2 x_2^2 + n_2 x_2 x_3^2 + o_2 x_2 x_3 \\
& + p_2 x_2 + q_2 x_3^3 + r_2 x_3^2 + s_2 x_3, x_1^3 x_2 + u_3 x_1^2 x_2^2 + v_3 x_1 x_2^3 + w_3 x_2^4 + a_3 x_1^3 \\
& + b_3 x_1^2 x_2 + c_3 x_1^2 x_3 + d_3 x_1^2 + e_3 x_1 x_2^2 + f_3 x_1 x_2 x_3 + g_3 x_1 x_2 + h_3 x_1 x_3^2 + i_3 x_1 x_3 \\
& \left. + j_3 x_1 + k_3 x_2^3 + l_3 x_2^2 x_3 + m_3 x_2^2 + n_3 x_2 x_3^2 + o_3 x_2 x_3 + p_3 x_2 + q_3 x_3^3 + r_3 x_3^2 + s_3 x_3 \right]
\end{aligned}$$

```

> initcases (6);
We assume the following in our calculation:
6 ≠ 0

```

```

> for i from 2 by -1 to 0 do
>   for j from 3-i by -1 to 0 do

```

```

>   for k from 3-i-j by -1 to 1 do
>     v := coeff (coeff (coeff (H[3],x1,i),x2,j),x3,k);
>     m := cpcoeff (x1^i * x2^j * x3^(k-1) * T^2);
>     elimsolve (m,v);
>   od
> od;
> od;

```

c3 is set to:  $\{1 \neq 0\}$

$$-3 a1 - b2$$

$$\{1 \neq 0\}$$

f3 is set to:

$$-2 b1 - 2 e2$$

$$\{2 \neq 0\}$$

h3 is set to:

$$-\frac{f2}{2} - c1$$

$$\{1 \neq 0\}$$

i3 is set to:

$$-2 d1 - g2$$

$$\{1 \neq 0\}$$

l3 is set to:

$$-3 k2 - e1$$

$$\{2 \neq 0\}$$

n3 is set to:

$$-\frac{f1}{2} - l2$$

$$\{1 \neq 0\}$$

o3 is set to:

$$-2 m2 - g1$$

$$\{3 \neq 0\}$$

q3 is set to:

$$-\frac{n2}{3} - \frac{h1}{3}$$

$$\{2 \neq 0\}$$

r3 is set to:

$$-\frac{i1}{2} - \frac{o2}{2}$$

$$\{1 \neq 0\}$$

s3 is set to:

$$-j1 - p2$$

```

> for i from 2 by -1 to 0 do
>   for j from 3-i by -1 to 0 do
>     for k from 3-i-j by -1 to 1 do

```

```

>      v := coeff (coeff (coeff (H[2],x1,i),x2,j),x3,k);
>      m := cpcoeff (x1^(i+3) * x2^j * x3^(k-1) * T);
>      elimsolve (m,v);
>      od
>      od;
>      od;

```

c2 is set to:

$$\{1 \neq 0\}$$

f2 is set to:

$$-b1$$

$$\{1 \neq 0\}$$

h2 is set to:

$$2\ b1\ u3 - 2\ e1 - 3\ c1$$

$$\{2 \neq 0\}$$

i2 is set to:

$$-\frac{f1}{2}$$

$$\{1 \neq 0\}$$

l2 is set to:

$$b1\ b3 - 3\ a1\ b2 - 9\ a1^2 - g1 - 3\ a2\ b1 - 3\ a3\ c1 - b2^2$$

$$\{-1 \neq 0\}$$

n2 is set to:

$$-3\ k1 - 3\ f1 + 4\ u3\ c1 + 3\ b1\ v3 - 4\ b1\ u3^2 + 4\ u3\ e1$$

$$\{-1 \neq 0\}$$

o2 is set to:

$$-3\ h1 + u3\ f1 - l1$$

$$\{-1 \neq 0\}$$

q2 is set to:

$$-6\ a2\ e1 + 2\ u3\ b2^2 + 2\ u3\ g1 + 18\ u3\ a1^2 + 2\ b3\ e1 - 4\ b2\ e2 - 4\ b1\ b2 - 12\ b1\ a1 - 6\ a1\ e2$$

$$- 3\ a3\ f1 - 4\ b3\ b1\ u3 + 6\ u3\ a1\ b2 + 6\ u3\ a2\ b1 + 6\ u3\ a3\ c1 + 2\ b1\ e3 + b3\ c1 - 3\ i1 - 2\ m1$$

$$\{3 \neq 0\}$$

r2 is set to:

$$-\frac{n1}{3}$$

$$\{-2 \neq 0\}$$

s2 is set to:

$$-3\ a3\ h1 - 3\ b1\ u3\ a1 - 2\ b1\ u3\ b2 + 3\ e1\ a1 + 2\ e1\ b2 + \frac{3\ c1\ a1}{2} + 3\ b2\ c1 - b1\ e2 + \frac{b3\ f1}{2}$$

$$-\frac{3\ a2\ f1}{2} - \frac{o1}{2}$$

$$\{-1 \neq 0\}$$

t2 is set to:

$$-3\ a3\ i1 - 3\ a1\ g2 - 2\ d1\ b2 - 3\ a2\ g1 - 2\ d2\ b1 - 2\ d3\ c1 - b1\ b3^2 + 3\ b3\ a1\ b2 + 9\ b3\ a1^2$$

$$+ b3\ g1 + 3\ b3\ a2\ b1 + 3\ b3\ a3\ c1 + b3\ b2^2 - 2\ b2\ g2 - 12\ a1\ d1 + b1\ g3 - p1$$

```

> for i from 2 by -1 to 0 do
>   for j from 3-i by -1 to 0 do
>     for k from 3-i-j by -1 to 1 do
>       v := coeff (coeff (coeff (H[1],x1,i),x2,j),x3,k);
>       m := cpcoeff (x1^(i+6) * x2^j * x3^(k-1));
>       elimsolve (m,v);
>     od
>   od;
> od;

c1 is set to:

$$\{1 \neq 0\}$$

0

f1 is set to:

$$\{1 \neq 0\}$$

0

h1 is set to:

$$\{1 \neq 0\}$$

0

i1 is set to:

$$\{1 \neq 0\}$$


$$-b1(6a1 + b2)$$


$$\{1 \neq 0\}$$


l1 is set to:
0

$$\{1 \neq 0\}$$


n1 is set to:
0

$$\{-1 \neq 0\}$$


o1 is set to:

$$-12e1a1 - 2e1b2 - b1^2 + 12b1u3a1 + 2b1u3b2 - 2b1e2$$


$$\{1 \neq 0\}$$


q1 is set to:
0

$$\{1 \neq 0\}$$


r1 is set to:

$$-b1(-e1 + b1u3)$$


$$\{1 \neq 0\}$$


s1 is set to:

$$-4d1b1 - b1g2 + 6a1b1b3 - 27a1^3 - 6a1g1 + 3a3b1^2 + b1b3b2 - g1b2$$


> tmp1 := cpcoeff(x2^2*x3^2*T);


$$tmp1 := -3(3k1 - 3b1v3 + 4b1u3^2 - 4u3e1)^2$$


> elimsolve (tmp1,k1);

k1 is set to:

$$\{3 \neq 0\}$$


```

$$b l v3 - \frac{4 b l u3^2}{3} + \frac{4 u3 e l}{3}$$

```
> tmp1 := cpcoeff(x1^2*x3^2*T);
```

$$tmp1 := -4(-el + bl u3)^2$$

```
> elimsolve(tmp1,e1);
```

$$\{-1 \neq 0\}$$

e1 is set to:

$$b l u3$$

```
> launchNZcase(b1);
```

Launching case level 1:

$$b l \neq 0$$

Assume from now on that:

$$6 b l \neq 0$$

```
> tmp1 := cpcoeff(x1^5*x2^2);
```

$$tmp1 := -3 b l k2$$

```
> elimsolve(tmp1,k2);
```

$$\{1 \neq 0\}$$

k2 is set to:

$$0$$

```
> tmp1 := cpcoeff(x1*x3^2*T);
```

$$tmp1 := -2 b l^2 e2$$

```
> elimsolve(tmp1,e2);
```

$$\{1 \neq 0\}$$

e2 is set to:

$$0$$

```
> tmp1 := cpcoeff(x2^3*x3*T);
```

$$tmp1 := -4 b l^2 w3$$

```
> elimsolve(tmp1,w3);
```

$$\{1 \neq 0\}$$

w3 is set to:

$$0$$

```
> tmp1 := cpcoeff(x1*x2^2*x3*T);
```

$$tmp1 := 3 b l^2 v3$$

```
> elimsolve(tmp1,v3);
```

$$\{1 \neq 0\}$$

v3 is set to:

$$0$$

```
> tmp1 := cpcoeff(x2^3*x3^2);
```

$$tmp1 := -2 b l^4 u3^2$$

```
> elimsolve(tmp1,u3);
```

$$\{1 \neq 0\}$$

u3 is set to:

$$0$$

```
> tmp1 := cpcoeff (x2*x3^3);
```

$$tmp1 := -2 b1^5$$

```
> contradict (tmp1, 'b1');
```

Contradiction on case level 1, so:

$$b1 = 0$$

Variables to be uneliminated:

"u3 := 'u3'"

"v3 := 'v3'"

"w3 := 'w3'"

"e2 := 'e2'"

"k2 := 'k2'"

Proceed on case level 0 with:

$$6 \neq 0$$

On account of:

$$b1 = 0$$

$$\{1 \neq 0\}$$

b1 is set to:

$$0$$

```
> launchNZcase (e2);
```

Launching case level 1:

$$e2 \neq 0$$

Assume from now on that:

$$6 e2 \neq 0$$

```
> tmp1 := cpcoeff (x1*x2*x3*T);
```

$$tmp1 := -18 k2 a1 b2 - 54 k2 a1^2 - 6 g1 k2 - 6 k2 b2^2 - 4 e2 u3 b2^2 - 4 e2 u3 g1 \\ - 36 e2 u3 a1^2 + 8 b2 e2^2 + 12 a1 e2^2 - 12 e2 u3 a1 b2 + 4 e2 m1$$

```
> elimsolve (tmp1, m1);
```

$$\{-2 e2 \neq 0\}$$

m1 is set to:

$$(9 k2 a1 b2 + 27 k2 a1^2 + 3 g1 k2 + 3 k2 b2^2 + 2 e2 u3 b2^2 + 2 e2 u3 g1 + 18 e2 u3 a1^2 \\ - 4 b2 e2^2 - 6 a1 e2^2 + 6 e2 u3 a1 b2) / (2 e2)$$

```
> launchNZcase (3*a1+b2);
```

Launching case level 2:

$$3 a1 + b2 \neq 0$$

Assume from now on that:

$$6 e2 (3 a1 + b2) \neq 0$$

```
> tmp1 := cpcoeff(x1^5*x2);
```

$$tmp1 := -(-30 a1 b2 e2^2 + 54 a1^3 u3 e2 + 81 k2 a1^2 b2 + 2 e2 u3 b2^3 + 18 a1 g1 k2 \\ + 27 a1 k2 b2^2 + 3 b2 g1 k2 + 2 g1 e2^2 + 54 a1^2 u3 e2 b2 + 18 a1 u3 e2 b2^2 - 36 a1^2 e2^2 \\ + 162 k2 a1^3 + 3 k2 b2^3 - 4 b2^2 e2^2) / e2$$

```
> elimsolve (tmp1, u3);
```

$$\{54 a1^3 e2 + 2 e2 b2^3 + 54 a1^2 e2 b2 + 18 a1 e2 b2^2 \neq 0\}$$

u3 is set to:

$$-(-30 a l b 2 e 2^2 + 81 k 2 a l^2 b 2 + 18 a l g l k 2 + 27 a l k 2 b 2^2 + 3 b 2 g l k 2 + 2 g l e 2^2 - 36 a l^2 e 2^2 + 162 k 2 a l^3 + 3 k 2 b 2^3 - 4 b 2^2 e 2^2) / (2 e 2 (3 a l + b 2)^3)$$

> **launchNZcase (3\*a1\*b2-g1);**

Launching case level 3:

$$3 a l b 2 - g l \neq 0$$

Assume from now on that:

$$6 e 2 (3 a l + b 2) (3 a l b 2 - g l) \neq 0$$

> **tmp1 := cpcoeff(x1^3\*x2^3);**

$$\begin{aligned} tmp1 := & -(-432 w 3 e 2 a l^3 g l b 2 - 48 w 3 e 2 a l g l b 2^3 + 648 w 3 e 2 a l^3 b 2^3 \\ & + 972 w 3 e 2 a l^5 b 2 + 1296 w 3 e 2 a l^4 b 2^2 - 324 w 3 e 2 a l^4 g l - 4 w 3 e 2 g l b 2^4 \\ & - 36 a l e 2^2 k 2 b 2^3 - 648 a l^3 e 2^2 k 2 b 2 - 324 a l^2 e 2^2 k 2 b 2^2 - 243 g l k 2^2 a l^2 b 2 \\ & - 81 g l k 2^2 a l b 2^2 + 54 k 2 g l a l^2 e 2^2 + 6 k 2 b 2^2 g l e 2^2 + 144 a l^2 w 3 e 2 b 2^4 \\ & + 12 a l w 3 e 2 b 2^5 + 8748 a l^5 k 2 v 3 b 2 + 324 a l^2 k 2 v 3 b 2^4 + 5103 a l^4 k 2 v 3 b 2^2 \\ & + 1701 a l^3 k 2 v 3 b 2^3 + 729 a l^4 k 2 v 3 g l + 27 a l k 2 v 3 b 2^5 - 2187 k 2^2 a l^5 \\ & - 216 w 3 e 2 a l^2 g l b 2^2 + 72 k 2 g l a l b 2 e 2^2 - 486 a l^4 e 2^2 k 2 - 243 k 2^2 a l^3 b 2^2 \\ & - 729 g l k 2^2 a l^3 - 9 g l k 2^2 b 2^3 - 54 a l g l^2 k 2^2 - 9 b 2 g l^2 k 2^2 - 6 k 2 g l^2 e 2^2 \\ & + 6561 a l^6 k 2 v 3 + 729 a l^3 k 2 v 3 g l b 2 + 243 a l^2 k 2 v 3 g l b 2^2 + 27 a l k 2 v 3 g l b 2^3 \\ & - 729 k 2^2 a l^4 b 2) / (e 2 (3 a l + b 2)^3) \end{aligned}$$

> **elimsolve (tmp1,w3);**

$$\{-432 e 2 a l^3 g l b 2 - 48 e 2 a l g l b 2^3 + 648 e 2 a l^3 b 2^3 + 972 e 2 a l^5 b 2 + 1296 e 2 a l^4 b 2^2 - 324 e 2 a l^4 g l - 4 e 2 g l b 2^4 + 144 a l^2 e 2 b 2^4 + 12 a l e 2 b 2^5 - 216 e 2 a l^2 g l b 2^2 \neq 0\}$$

w3 is set to:

$$\begin{aligned} -3 k 2 (18 g l a l^2 e 2^2 + 243 a l^3 v 3 g l b 2 - 12 b 2^3 a l e 2^2 - 81 g l k 2 a l^2 b 2 - 27 g l k 2 a l b 2^2 \\ + 24 g l a l b 2 e 2^2 - 216 a l^3 b 2 e 2^2 - 243 k 2 a l^4 b 2 - 81 k 2 a l^3 b 2^2 - 243 g l k 2 a l^3 \\ - 3 g l k 2 b 2^3 + 2 b 2^2 g l e 2^2 - 108 b 2^2 a l^2 e 2^2 - 18 a l g l^2 k 2 - 3 b 2 g l^2 k 2 - 729 k 2 a l^5 \\ - 2 g l^2 e 2^2 - 162 a l^4 e 2^2 + 2916 a l^5 v 3 b 2 + 108 a l^2 v 3 b 2^4 + 1701 a l^4 v 3 b 2^2 \\ + 567 a l^3 v 3 b 2^3 + 243 a l^4 v 3 g l + 9 a l v 3 b 2^5 + 2187 a l^6 v 3 + 81 a l^2 v 3 g l b 2^2 \\ + 9 a l v 3 g l b 2^3) / (4 e 2 (3 a l + b 2)^4 (3 a l b 2 - g l)) \end{aligned}$$

> **tmp1 := cpcoeff(x1^4\*x2^2);**

$$\begin{aligned} tmp1 := & (324 a l^3 v 3 e 2^2 g l b 2 - 36 a l^2 g l e 2^4 + 4 g l^2 e 2^4 + 9 a l k 2 b 2^2 g l e 2^2 \\ & + 36 a l v 3 e 2^2 g l b 2^3 - 135 a l^2 k 2 g l b 2 e 2^2 - 189 a l^2 e 2^2 k 2 b 2^3 - 4 b 2^2 e 2^4 g l \\ & + 3 v 3 e 2^2 g l b 2^4 + 3 k 2 g l e 2^2 b 2^3 + 6 g l^2 e 2^2 k 2 b 2 + 10935 a l^5 k 2^2 b 2 - 729 a l^5 e 2^2 k 2 \\ & + 2916 a l^4 g l k 2^2 + 5832 a l^4 k 2^2 b 2^2 + 1701 a l^3 k 2^2 b 2^3 + 108 a l^3 b 2 e 2^4 + 324 a l^2 k 2^2 b 2^4 \\ & + 108 a l^2 b 2^2 e 2^4 + 162 a l^2 g l^2 k 2^2 + 12 a l b 2^3 e 2^4 + 27 a l k 2^2 b 2^5 + 13122 k 2^2 a l^6 \\ & - 729 a l^5 v 3 e 2^2 b 2 - 1701 a l^4 e 2^2 k 2 b 2 + 243 a l^4 v 3 e 2^2 g l - 972 a l^4 v 3 e 2^2 b 2^2 \\ & + 1458 a l^3 g l k 2^2 b 2 + 243 a l^3 k 2 g l e 2^2 - 567 a l^3 e 2^2 k 2 b 2^2 - 486 a l^3 v 3 e 2^2 b 2^3 \\ & - 108 a l^2 v 3 e 2^2 b 2^4 + 486 a l^2 g l k 2^2 b 2^2 - 18 a l e 2^2 k 2 b 2^4 - 48 a l b 2 e 2^4 g l \end{aligned}$$

$$+ 27 a l b 2 g l^2 k 2^2 + 54 a l g l k 2^2 b 2^3 + 54 a l k 2 g l^2 e 2^2 - 9 a l v 3 e 2^2 b 2^5 \\ + 162 a l^2 v 3 e 2^2 g l b 2^2) / ((3 a l + b 2)^3 e 2^2)$$

> **elimsolve (tmp1,v3);**

$$\{ 324 a l^3 e 2^2 g l b 2 + 36 a l e 2^2 g l b 2^3 + 3 e 2^2 g l b 2^4 - 729 a l^5 e 2^2 b 2 + 243 a l^4 e 2^2 g l \\ - 972 a l^4 e 2^2 b 2^2 - 486 a l^3 e 2^2 b 2^3 - 108 a l^2 e 2^2 b 2^4 - 9 a l e 2^2 b 2^5 + 162 a l^2 e 2^2 g l b 2^2 \neq 0 \\ \}$$

v3 is set to:

$$(-36 a l^2 g l e 2^4 + 4 g l^2 e 2^4 + 9 a l k 2 b 2^2 g l e 2^2 - 135 a l^2 k 2 g l b 2 e 2^2 - 189 a l^2 e 2^2 k 2 b 2^3 \\ - 4 b 2^2 e 2^4 g l + 3 k 2 g l e 2^2 b 2^3 + 6 g l^2 e 2^2 k 2 b 2 + 10935 a l^5 k 2^2 b 2 - 729 a l^5 e 2^2 k 2 \\ + 2916 a l^4 g l k 2^2 + 5832 a l^4 k 2^2 b 2^2 + 1701 a l^3 k 2^2 b 2^3 + 108 a l^3 b 2 e 2^4 + 324 a l^2 k 2^2 b 2^4 \\ + 108 a l^2 b 2^2 e 2^4 + 162 a l^2 g l^2 k 2^2 + 12 a l b 2^3 e 2^4 + 27 a l k 2^2 b 2^5 + 13122 k 2^2 a l^6 \\ - 1701 a l^4 e 2^2 k 2 b 2 + 1458 a l^3 g l k 2^2 b 2 + 243 a l^3 k 2 g l e 2^2 - 567 a l^3 e 2^2 k 2 b 2^2 \\ + 486 a l^2 g l k 2^2 b 2^2 - 18 a l e 2^2 k 2 b 2^4 - 48 a l b 2 e 2^4 g l + 27 a l b 2 g l^2 k 2^2 \\ + 54 a l g l k 2^2 b 2^3 + 54 a l k 2 g l^2 e 2^2) / (3 e 2^2 (3 a l + b 2)^4 (3 a l b 2 - g l))$$

> **launchNZcase (k2);**

Launching case level 4:

$$k 2 \neq 0$$

Assume from now on that:

$$6 e 2 (3 a l + b 2) (3 a l b 2 - g l) k 2 \neq 0$$

> **tmp1 := cpcoeff(x3^2\*T);**

$$tmp1 := - \frac{9 (9 a l^2 + 3 a l b 2 + g l + b 2^2)^2 k 2^2}{e 2^2}$$

> **elimsolve (tmp1,g1);**

$$\{ 1 \neq 0 \}$$

g1 is set to:

$$-9 a l^2 - 3 a l b 2 - b 2^2$$

Nonzero constraint refines to:

$$6 e 2 (3 a l + b 2)^2 k 2 \neq 0$$

> **tmp1 := cpcoeff (x2^4\*T);**

$$tmp1 := -9 k 2^2$$

> **contradict (tmp1,'k2');**

Contradiction on case level 4, so:

$$k 2 = 0$$

Variables to be uneliminated:

$$"g1 := 'g1'"$$

Proceed on case level 3 with:

$$6 e 2 (3 a l + b 2) (3 a l b 2 - g l) \neq 0$$

On account of:

$$k 2 = 0$$

$$\{ 1 \neq 0 \}$$

k2 is set to:

$$0$$

```
> tmp1 := cpcoeff (x1^2*x2^2*T);
```

$$tmp1 := -\frac{4 e^2 (3 a l b 2 - g l)^2}{(3 a l + b 2)^4}$$

```
> contradict (tmp1,'g1');
```

Contradiction on case level 3, so:

$$3 a l b 2 - g l = 0$$

Variables to be uneliminated:

"k2 := 'k2'"

"v3 := 'v3'"

"w3 := 'w3'"

Proceed on case level 2 with:

$$6 (3 a l + b 2) e 2 \neq 0$$

On account of:

$$3 a l b 2 - g l = 0$$

$$\{-1 \neq 0\}$$

g1 is set to:

$$3 a l b 2$$

```
> tmp1 := cpcoeff (x3^2*T);
```

$$tmp1 := -\frac{9 (3 a l + b 2)^4 k 2^2}{e 2^2}$$

```
> elimsolve (tmp1,k2);
```

$$\{1 \neq 0\}$$

k2 is set to:

$$0$$

```
> tmp1 := cpcoeff (x1^2*x3*T);
```

$$tmp1 := -2 e 2 (3 a l + b 2)^2$$

```
> contradict (tmp1,'b2');
```

Contradiction on case level 2, so:

$$3 a l + b 2 = 0$$

Variables to be uneliminated:

"k2 := 'k2'"

"g1 := 'g1'"

"u3 := 'u3'"

Proceed on case level 1 with:

$$6 e 2 \neq 0$$

On account of:

$$3 a l + b 2 = 0$$

$$\{1 \neq 0\}$$

b2 is set to:

$$-3 a l$$

```
> launchNZcase (k2);
```

Launching case level 2:

$$k 2 \neq 0$$

Assume from now on that:

```

|                                      $6 e2 k2 \neq 0$ 
| > tmp1 := cpcoeff (x1^4*x3);
|                                      $tmp1 := \frac{3 k2 (9 a1^2 + g1)^2}{e2}$ 
| > elimsolve (tmp1,g1);
|                                      $\{1 \neq 0\}$ 
| g1 is set to:
|                                      $-9 a1^2$ 
| > tmp1 := cpcoeff (x2^4*T);
|                                      $tmp1 := -9 k2^2$ 
| > contradict (tmp1,'k2');
| Contradiction on case level 2, so:
|                                      $k2 = 0$ 
| Variables to be uneliminated:
|                                     "g1 := 'g1'"
| Proceed on case level 1 with:
|                                      $6 e2 \neq 0$ 
| On account of:
|                                      $k2 = 0$ 
|                                      $\{1 \neq 0\}$ 
| k2 is set to:
|                                     0
| > tmp1 := cpcoeff (x1^2*x3*T);
|                                      $tmp1 := -2 (9 a1^2 + g1) e2$ 
| > elimsolve (tmp1,g1);
|                                      $\{1 \neq 0\}$ 
| g1 is set to:
|                                      $-9 a1^2$ 
| > tmp1 := cpcoeff (x1^2*x2^2*T);
|                                      $tmp1 := -4 e2^2$ 
| > contradict (tmp1,'e2');
| Contradiction on case level 1, so:
|                                      $e2 = 0$ 
| Variables to be uneliminated:
|                                     "g1 := 'g1'"
|                                     "k2 := 'k2'"
|                                     "b2 := 'b2'"
|                                     "m1 := 'm1'"
| Proceed on case level 0 with:
|                                      $6 \neq 0$ 
| On account of:
|                                      $e2 = 0$ 
|                                      $\{1 \neq 0\}$ 
| e2 is set to:

```

```

[
0
> launchNZcase (k2);
Launching case level 1:
k2 ≠ 0
Assume from now on that:
6 k2 ≠ 0
> tmp1 := cpcoeff (x1*x2*x3*T);
tmp1 := -6 k2 (9 a l2 + 3 a l b2 + g l + b22)
> elimsolve (tmp1,g1);
{1 ≠ 0}
g1 is set to:
-9 a l2 - 3 a l b2 - b22
> tmp1 := cpcoeff (x3^2*T);
tmp1 := -4 m l2
> elimsolve (tmp1,m1);
{1 ≠ 0}
m1 is set to:
0
> tmp1 := cpcoeff (x2^4*T);
tmp1 := -9 k22
> contradict (tmp1,'k2');
Contradiction on case level 1, so:
k2 = 0
Variables to be uneliminated:
"m1 := 'm1'"
"g1 := 'g1'"
Proceed on case level 0 with:
6 ≠ 0
On account of:
k2 = 0
{1 ≠ 0}
k2 is set to:
0
> launchNZcase (w3);
Launching case level 1:
w3 ≠ 0
Assume from now on that:
6 w3 ≠ 0
> tmp1 := cpcoeff (x2^4*T);
tmp1 := -8 (u3 b22 + u3 g l + 9 u3 a l2 + 3 u3 a l b2 - m l) w3
> elimsolve (tmp1,m1);
{-1 ≠ 0}
m1 is set to:
u3 (9 a l2 + 3 a l b2 + g l + b22)
> tmp1 := cpcoeff (x1*x2^3*T);

```

```

|                                      $tmp1 := 4 w3 (9 a l^2 + 3 a l b2 + g1 + b2^2)$ 
| > elimsolve (tmp1,g1);
|                                      $\{1 \neq 0\}$ 
| g1 is set to:
|                                      $-9 a l^2 - 3 a l b2 - b2^2$ 
| > tmp1 := cpcoeff (x1*x3*T);
|                                      $tmp1 := 2 (3 a l + b2)^4$ 
| > elimsolve (tmp1,b2);
|                                      $\{1 \neq 0\}$ 
| b2 is set to:
|                                      $-3 a l$ 
| > tmp1 := cpcoeff (x2^3*T);
|                                      $tmp1 := -4 (3 a l g2 - 6 a l d1 + 27 a2 a l^2 - p1) w3$ 
| > elimsolve (tmp1,p1);
|                                      $\{-1 \neq 0\}$ 
| p1 is set to:
|                                      $3 a l (g2 - 2 d1 + 9 a l a2)$ 
| > launchNZcase (a1);
| Launching case level 2:
|                                      $a l \neq 0$ 
| Assume from now on that:
|                                      $6 w3 a l \neq 0$ 
| > tmp1 := cpcoeff (x1^2*x2*T);
|                                      $tmp1 := -3 a l (-2 m2 + 9 a l^2)$ 
| > elimsolve (tmp1,m2);
|                                      $\{-2 \neq 0\}$ 
| m2 is set to:
|                                      $\frac{9 a l^2}{2}$ 
| > tmp1 := cpcoeff (x2^2*T);
|                                      $tmp1 := -81 a l^4$ 
| > contradict (tmp1,'a1');
| Contradiction on case level 2, so:
|                                      $a l = 0$ 
| Variables to be uneliminated:
|                                     "m2 := 'm2'"
| Proceed on case level 1 with:
|                                      $6 w3 \neq 0$ 
| On account of:
|                                      $a l = 0$ 
|                                      $\{1 \neq 0\}$ 
| a1 is set to:
|                                     0
| > tmp1 := cpcoeff (x2^2*T);

```

|                                    |  |                           |
|------------------------------------|--|---------------------------|
| [                                  |  | $tmp1 := -4 m2^2$         |
| > <b>elimsolve</b> (tmp1,m2);      |  | $\{1 \neq 0\}$            |
| m2 is set to:                      |  | 0                         |
| [                                  |  |                           |
| > <b>launchNZcase</b> (j1);        |  |                           |
| Launching case level 2:            |  | $j1 \neq 0$               |
| Assume from now on that:           |  | $6 w3 j1 \neq 0$          |
| [                                  |  |                           |
| > <b>launchNZcase</b> (p2);        |  |                           |
| Launching case level 3:            |  | $p2 \neq 0$               |
| Assume from now on that:           |  | $6 w3 j1 p2 \neq 0$       |
| [                                  |  |                           |
| > <b>tmp1 := cpcoeff</b> (1);      |  |                           |
| [                                  |  | $tmp1 := j1 p2 (j1 + p2)$ |
| > <b>elimsolve</b> (tmp1,p2);      |  | $\{1 \neq 0\}$            |
| p2 is set to:                      |  | $-j1$                     |
| Nonzero constraint refines to:     |  | $-6 w3 j1^2 \neq 0$       |
| [                                  |  |                           |
| > <b>tmp1 := cpcoeff</b> (T);      |  | $tmp1 := -j1^2$           |
| [                                  |  |                           |
| > <b>contradict</b> (tmp1,'p2');   |  |                           |
| Contradiction on case level 3, so: |  | $p2 = 0$                  |
| Variables to be uneliminated:      |  | "p2 := 'p2'"              |
| Proceed on case level 2 with:      |  | $6 w3 j1 \neq 0$          |
| On account of:                     |  | $p2 = 0$                  |
|                                    |  | $\{1 \neq 0\}$            |
| p2 is set to:                      |  | 0                         |
| [                                  |  |                           |
| > <b>tmp1 := cpcoeff</b> (T);      |  | $tmp1 := -j1^2$           |
| [                                  |  |                           |
| > <b>contradict</b> (tmp1,'j1');   |  |                           |
| Contradiction on case level 2, so: |  | $j1 = 0$                  |
| Variables to be uneliminated:      |  | "p2 := 'p2'"              |
| Proceed on case level 1 with:      |  | $6 w3 \neq 0$             |

On account of:

$$j1 = 0$$

$$\{1 \neq 0\}$$

j1 is set to:

$$0$$

> **tmp1 := cpcoeff (T);**

$$tmp1 := -p^2$$

> **elimsolve (tmp1,p2);**

$$\{1 \neq 0\}$$

p2 is set to:

$$0$$

> **launchNZcase (d1);**

Launching case level 2:

$$d1 \neq 0$$

Assume from now on that:

$$6 w3 d1 \neq 0$$

> **launchNZcase (g2);**

Launching case level 3:

$$g2 \neq 0$$

Assume from now on that:

$$6 w3 d1 g2 \neq 0$$

> **tmp1 := cpcoeff (x1^3);**

$$tmp1 := 2 d1 g2 (2 d1 + g2)$$

> **elimsolve (tmp1,g2);**

$$\{1 \neq 0\}$$

g2 is set to:

$$-2 d1$$

Nonzero constraint refines to:

$$-12 w3 d1^2 \neq 0$$

> **tmp1 := cpcoeff (x1^2\*T);**

$$tmp1 := -4 d1^2$$

> **contradict (tmp1,'g2');**

Contradiction on case level 3, so:

$$g2 = 0$$

Variables to be uneliminated:

$$"g2 := 'g2'"$$

Proceed on case level 2 with:

$$6 w3 d1 \neq 0$$

On account of:

$$g2 = 0$$

$$\{1 \neq 0\}$$

g2 is set to:

$$0$$

> **tmp1 := cpcoeff (x1^2\*T);**

$$tmp1 := -4 d1^2$$

```
> contradict (tmp1,'d1');
```

Contradiction on case level 2, so:

$$d1 = 0$$

Variables to be uneliminated:

$$g2 := 'g2'$$

Proceed on case level 1 with:

$$6 w3 \neq 0$$

On account of:

$$d1 = 0$$

$$\{1 \neq 0\}$$

d1 is set to:

$$0$$

```
> tmp1 := cpcoeff (x1^2*T);
```

$$tmp1 := -g2^2$$

```
> elimsolve (tmp1,g2);
```

$$\{1 \neq 0\}$$

g2 is set to:

$$0$$

```
> det(T-jacobian(H,[x1,x2,x3]));
```

$$T^3$$

```
> H;
```

$$\left[ 0, \frac{x1^4}{4} + a2 x1^3 + d2 x1^2 + j2 x1, x1^3 x2 + u3 x1^2 x2^2 + v3 x1 x2^3 + w3 x2^4 + a3 x1^3 + b3 x1^2 x2 + d3 x1^2 + e3 x1 x2^2 + g3 x1 x2 + j3 x1 + k3 x2^3 + m3 x2^2 + p3 x2 \right]$$

```
> jacobian(H,[x1,x2,x3]);
```

$$[0, 0, 0]$$

$$[x1^3 + 3 a2 x1^2 + 2 d2 x1 + j2, 0, 0]$$

$$[3 x1^2 x2 + 2 u3 x1 x2^2 + v3 x2^3 + 3 a3 x1^2 + 2 b3 x1 x2 + 2 d3 x1 + e3 x2^2 + g3 x2 + j3, x1^3$$

$$+ 2 u3 x1^2 x2 + 3 v3 x1 x2^2 + 4 w3 x2^3 + b3 x1^2 + 2 e3 x1 x2 + g3 x1 + 3 k3 x2^2 + 2 m3 x2 + p3$$

$$, 0]$$

```
> contradict (1,'w3');
```

Contradiction on case level 1, so:

$$w3 = 0$$

Variables to be uneliminated:

$$g2 := 'g2'$$

$$d1 := 'd1'$$

$$p2 := 'p2'$$

$$j1 := 'j1'$$

$$m2 := 'm2'$$

$$a1 := 'a1'$$

$$p1 := 'p1'$$

```
"m1 := 'm1'"
```

Proceed on case level 0 with:

$6 \neq 0$

On account of:

$$w_3 = 0$$

$$\{1 \neq 0\}$$

w3 is set to:

0

```
> tmp1 := cpcoeff (x3^2*T);
```

$$tmp1 := -4 (u3 \, b2^2 + u3 \, g1 + 9 \, u3 \, a1^2 + 3 \, u3 \, a1 \, b2 - m1)^2$$

```
> elimsolve (tmp1,m1);
```

$$\{-1 \neq 0\}$$

m1 is set to:

$$u3 (9 a1^2 + 3 a1 b2 + g1 + b2^2)$$

```
> launchNZcase (v3);
```

Launching case level 1:

$$v_3 \neq 0$$

Assume from now on that:

$$6 \nu_3 \neq 0$$

```
> tmp1 := cpcoeff (x1^2*x2^2*T);
```

$$tmp1 := 3 \ v3 \ (9 \ a1^2 + 3 \ a1 \ b2 + g1 + b2^2)$$

```
> elimsolve (tmp1,g1);
```

$$\{1 \neq 0\}$$

g1 is set to:

$$-9 a1^2 - 3 a1 b2 - b2^2$$

```
> tmp1 := cpcoeff (x1*x3*T);
```

$$tmp1 := 2 (3 a1 + b2)^4$$

```
> elimsolve (tmp1,b2);
```

$$\{1 \neq 0\}$$

b2 is set to:

$-3 \ a1$

```
> tmp1 := cpcoeff (x1*x2^2*T);
```

$$tmp1 := -3 (3 a1 g2 - 6 a1 d1 + 27 a2 a1^2 - p1) v3$$

```
> elimsolve (tmp1,p1);
```

$$\{-1 \neq 0\}$$

p1 is set to:

$$3\,a1\,(g2-2\,d1+9\,a1\,a2)$$

```
> launchNZcase (a1);
```

Launching case level 2:

$a_1 \neq 0$

Assume from now on that:

$$6 \, v3 \, a1 \neq 0$$

```

> tmp1 := cpcoeff (x1^2*x2^2);

$$tmp1 := 3 a l (-2 m 2 + 9 a l^2)^2$$

> elimsolve (tmp1,m2);

$$\{-2 \neq 0\}$$

m2 is set to:

$$\frac{9 a l^2}{2}$$

> tmp1 := cpcoeff (x2^2*T);

$$tmp1 := -81 a l^4$$

> contradict (tmp1,'a1');
Contradiction on case level 2, so:

$$a l = 0$$

Variables to be uneliminated:
"m2 := 'm2'"
Proceed on case level 1 with:

$$6 v 3 \neq 0$$

On account of:

$$a l = 0$$


$$\{1 \neq 0\}$$

a1 is set to:

$$0$$

> tmp1 := cpcoeff (x2^2*T);

$$tmp1 := -4 m 2^2$$

> elimsolve (tmp1,m2);

$$\{1 \neq 0\}$$

m2 is set to:

$$0$$

> launchNZcase (j1);
Launching case level 2:

$$j l \neq 0$$

Assume from now on that:

$$6 v 3 j l \neq 0$$

> launchNZcase (p2);
Launching case level 3:

$$p 2 \neq 0$$

Assume from now on that:

$$6 v 3 j l p 2 \neq 0$$

> tmp1 := cpcoeff (1);

$$tmp1 := j l p 2 (j l + p 2)$$

> elimsolve (tmp1,p2);

$$\{1 \neq 0\}$$

p2 is set to:

$$-j l$$

Nonzero constraint refines to:

$$-6 v 3 j l^2 \neq 0$$


```

```

> tmp1 := cpcoeff (T);
                                      $tmp1 := -j1^2$ 
> contradict (tmp1,'p2');
Contradiction on case level 3, so:
                                      $p2 = 0$ 
Variables to be uneliminated:
                                     "p2 := 'p2'"
Proceed on case level 2 with:
                                      $6 \sqrt{3} j1 \neq 0$ 
On account of:
                                      $p2 = 0$ 
                                      $\{1 \neq 0\}$ 
p2 is set to:
                                     0
> tmp1 := cpcoeff (T);
                                      $tmp1 := -j1^2$ 
> contradict (tmp1,'j1');
Contradiction on case level 2, so:
                                      $j1 = 0$ 
Variables to be uneliminated:
                                     "p2 := 'p2'"
Proceed on case level 1 with:
                                      $6 \sqrt{3} \neq 0$ 
On account of:
                                      $j1 = 0$ 
                                      $\{1 \neq 0\}$ 
j1 is set to:
                                     0
> tmp1 := cpcoeff (T);
                                      $tmp1 := -p2^2$ 
> elimsolve (tmp1,p2);
                                      $\{1 \neq 0\}$ 
p2 is set to:
                                     0
> launchNZcase (d1);
Launching case level 2:
                                      $d1 \neq 0$ 
Assume from now on that:
                                      $6 \sqrt{3} d1 \neq 0$ 
> launchNZcase (g2);
Launching case level 3:
                                      $g2 \neq 0$ 
Assume from now on that:
                                      $6 \sqrt{3} d1 g2 \neq 0$ 
> tmp1 := cpcoeff (x1^3);
                                      $tmp1 := 2 d1 g2 (2 d1 + g2)$ 

```

```

> elimsolve (tmp1,g2);
g2 is set to:
Nonzero constraint refines to:
> tmp1 := cpcoeff (x1^2*T);
> contradict (tmp1,'g2');
Contradiction on case level 3, so:
Variables to be uneliminated:
Proceed on case level 2 with:
On account of:
g2 is set to:
> tmp1 := cpcoeff (x1^2*T);
> contradict (tmp1,'d1');
Contradiction on case level 2, so:
Variables to be uneliminated:
Proceed on case level 1 with:
On account of:
d1 is set to:
> tmp1 := cpcoeff (x1^2*T);
> elimsolve (tmp1,g2);
g2 is set to:
> det (T-jacobian (H, [x1,x2,x3])) ;
> H;

```

$$\left[ 0, \frac{x1^4}{4} + a2 x1^3 + d2 x1^2 + j2 x1, x1^3 x2 + u3 x1^2 x2^2 + v3 x1 x2^3 + a3 x1^3 + b3 x1^2 x2 + d3 x1^2 \right]$$

$$+ e3 x1 x2^2 + g3 x1 x2 + j3 x1 + k3 x2^3 + m3 x2^2 + p3 x2 \Big]$$

> **jacobian** (H, [x1,x2,x3]) ;

[0,0,0]

$$[x1^3 + 3 a2 x1^2 + 2 d2 x1 + j2, 0, 0]$$

$$[3 x1^2 x2 + 2 u3 x1 x2^2 + v3 x2^3 + 3 a3 x1^2 + 2 b3 x1 x2 + 2 d3 x1 + e3 x2^2 + g3 x2 + j3,$$

$$x1^3 + 2 u3 x1^2 x2 + 3 v3 x1 x2^2 + b3 x1^2 + 2 e3 x1 x2 + g3 x1 + 3 k3 x2^2 + 2 m3 x2 + p3, 0]$$

> **contradict** (1,'v3') ;

Contradiction on case level 1, so:

$$v3 = 0$$

Variables to be uneliminated:

"g2 := 'g2'"

"d1 := 'd1'"

"p2 := 'p2'"

"j1 := 'j1'"

"m2 := 'm2'"

"a1 := 'a1'"

"p1 := 'p1'"

"b2 := 'b2'"

"g1 := 'g1'"

Proceed on case level 0 with:

$$6 \neq 0$$

On account of:

$$v3 = 0$$

$$\{1 \neq 0\}$$

v3 is set to:

$$0$$

> **launchNZcase** (u3) ;

Launching case level 1:

$$u3 \neq 0$$

Assume from now on that:

$$6 u3 \neq 0$$

> **tmp1 := cpcoeff** (x1^5\*x2) ;

$$tmp1 := -2 u3 (3 a1 + b2)^3$$

> **elimsolve** (tmp1,b2) ;

$$\{1 \neq 0\}$$

b2 is set to:

$$-3 a1$$

> **tmp1 := cpcoeff** (x2\*x3\*T) ;

$$tmp1 := 2 u3 (9 a1^2 + g1)^2$$

> **elimsolve** (tmp1,g1) ;

$$\{1 \neq 0\}$$

g1 is set to:

$$-9 a l^2$$

> **tmp1 := cpcoeff (x1^2\*x2\*T);**

$$tmp1 := -27 a l^3 + 6 a l m2 - 6 u3 a l g2 + 12 u3 a l d1 - 54 u3 a2 a l^2 + 2 u3 p1$$

> **elimsolve (tmp1,p1);**

$$\{-2 u3 \neq 0\}$$

p1 is set to:

$$\frac{3 a l (9 a l^2 - 2 m2 + 2 u3 g2 - 4 u3 d1 + 18 u3 a2 a l)}{2 u3}$$

> **launchNZcase (a1);**

Launching case level 2:

$$a l \neq 0$$

Assume from now on that:

$$6 a l u3 \neq 0$$

> **tmp1 := cpcoeff (x1^4\*x2);**

$$tmp1 := -9 a l^2 (-2 m2 + 9 a l^2)$$

> **elimsolve (tmp1,m2);**

$$\{-2 \neq 0\}$$

m2 is set to:

$$\frac{9 a l^2}{2}$$

> **tmp1 := cpcoeff (x2^2\*T);**

$$tmp1 := -81 a l^4$$

> **contradict (tmp1,'a1');**

Contradiction on case level 2, so:

$$a l = 0$$

Variables to be uneliminated:

$$m2 := 'm2'$$

Proceed on case level 1 with:

$$6 u3 \neq 0$$

On account of:

$$a l = 0$$

$$\{1 \neq 0\}$$

a1 is set to:

$$0$$

> **tmp1 := cpcoeff (x2^2\*T);**

$$tmp1 := -4 m2^2$$

> **elimsolve (tmp1,m2);**

$$\{1 \neq 0\}$$

m2 is set to:

$$0$$

> **launchNZcase (j1);**

Launching case level 2:

$$j1 \neq 0$$

Assume from now on that:

|  |                                     |                           |
|--|-------------------------------------|---------------------------|
|  |                                     | $6 u3 j1 \neq 0$          |
|  | <b>&gt; launchNZcase (p2);</b>      |                           |
|  | Launching case level 3:             |                           |
|  |                                     | $p2 \neq 0$               |
|  | Assume from now on that:            |                           |
|  |                                     | $6 u3 j1 p2 \neq 0$       |
|  | <b>&gt; tmp1 := cpcoeff (1);</b>    |                           |
|  |                                     | $tmp1 := j1 p2 (j1 + p2)$ |
|  | <b>&gt; elimsolve (tmp1,p2);</b>    |                           |
|  |                                     | $\{1 \neq 0\}$            |
|  | p2 is set to:                       |                           |
|  |                                     | $-j1$                     |
|  | Nonzero constraint refines to:      |                           |
|  |                                     | $-6 u3 j1^2 \neq 0$       |
|  | <b>&gt; tmp1 := cpcoeff (T);</b>    |                           |
|  |                                     | $tmp1 := -j1^2$           |
|  | <b>&gt; contradict (tmp1,'p2');</b> |                           |
|  | Contradiction on case level 3, so:  |                           |
|  |                                     | $p2 = 0$                  |
|  | Variables to be uneliminated:       |                           |
|  |                                     | "p2 := 'p2'"              |
|  | Proceed on case level 2 with:       |                           |
|  |                                     | $6 u3 j1 \neq 0$          |
|  | On account of:                      |                           |
|  |                                     | $p2 = 0$                  |
|  |                                     | $\{1 \neq 0\}$            |
|  | p2 is set to:                       |                           |
|  |                                     | 0                         |
|  | <b>&gt; tmp1 := cpcoeff (T);</b>    |                           |
|  |                                     | $tmp1 := -j1^2$           |
|  | <b>&gt; contradict (tmp1,'j1');</b> |                           |
|  | Contradiction on case level 2, so:  |                           |
|  |                                     | $j1 = 0$                  |
|  | Variables to be uneliminated:       |                           |
|  |                                     | "p2 := 'p2'"              |
|  | Proceed on case level 1 with:       |                           |
|  |                                     | $6 u3 \neq 0$             |
|  | On account of:                      |                           |
|  |                                     | $j1 = 0$                  |
|  |                                     | $\{1 \neq 0\}$            |
|  | j1 is set to:                       |                           |
|  |                                     | 0                         |
|  | <b>&gt; tmp1 := cpcoeff (T);</b>    |                           |
|  |                                     | $tmp1 := -p2^2$           |
|  | <b>&gt; elimsolve (tmp1,p2);</b>    |                           |

|                                    |                               |
|------------------------------------|-------------------------------|
|                                    | $\{1 \neq 0\}$                |
| p2 is set to:                      |                               |
|                                    | 0                             |
| > <b>launchNZcase (d1);</b>        |                               |
| Launching case level 2:            |                               |
|                                    | $d1 \neq 0$                   |
| Assume from now on that:           |                               |
|                                    | $6 u3 d1 \neq 0$              |
| > <b>launchNZcase (g2);</b>        |                               |
| Launching case level 3:            |                               |
|                                    | $g2 \neq 0$                   |
| Assume from now on that:           |                               |
|                                    | $6 u3 d1 g2 \neq 0$           |
| > <b>tmp1 := cpcoeff (x1^3);</b>   |                               |
|                                    | $tmp1 := 2 d1 g2 (2 d1 + g2)$ |
| > <b>elimsolve (tmp1,g2);</b>      |                               |
|                                    | $\{1 \neq 0\}$                |
| g2 is set to:                      |                               |
|                                    | $-2 d1$                       |
| Nonzero constraint refines to:     |                               |
|                                    | $-12 u3 d1^2 \neq 0$          |
| > <b>tmp1 := cpcoeff (x1^2*T);</b> |                               |
|                                    | $tmp1 := -4 d1^2$             |
| > <b>contradict (tmp1,'g2');</b>   |                               |
| Contradiction on case level 3, so: |                               |
|                                    | $g2 = 0$                      |
| Variables to be uneliminated:      |                               |
|                                    | "g2 := 'g2'"                  |
| Proceed on case level 2 with:      |                               |
|                                    | $6 u3 d1 \neq 0$              |
| On account of:                     |                               |
|                                    | $g2 = 0$                      |
|                                    | $\{1 \neq 0\}$                |
| g2 is set to:                      |                               |
|                                    | 0                             |
| > <b>tmp1 := cpcoeff (x1^2*T);</b> |                               |
|                                    | $tmp1 := -4 d1^2$             |
| > <b>contradict (tmp1,'d1');</b>   |                               |
| Contradiction on case level 2, so: |                               |
|                                    | $d1 = 0$                      |
| Variables to be uneliminated:      |                               |
|                                    | "g2 := 'g2'"                  |
| Proceed on case level 1 with:      |                               |
|                                    | $6 u3 \neq 0$                 |
| On account of:                     |                               |
|                                    | $d1 = 0$                      |

|                                             |                                                                                                                                                                                                      |
|---------------------------------------------|------------------------------------------------------------------------------------------------------------------------------------------------------------------------------------------------------|
|                                             | $\{1 \neq 0\}$                                                                                                                                                                                       |
| d1 is set to:                               | 0                                                                                                                                                                                                    |
| > <b>tmp1 := cpcoeff (x1^2*T);</b>          |                                                                                                                                                                                                      |
|                                             | $tmp1 := -g2^2$                                                                                                                                                                                      |
| > <b>elimsolve (tmp1,g2);</b>               |                                                                                                                                                                                                      |
|                                             | $\{1 \neq 0\}$                                                                                                                                                                                       |
| g2 is set to:                               | 0                                                                                                                                                                                                    |
| > <b>det (T-jacobian (H, [x1,x2,x3])) ;</b> | $T^3$                                                                                                                                                                                                |
| > <b>H;</b>                                 |                                                                                                                                                                                                      |
|                                             | $\left[ 0, \frac{x1^4}{4} + a2 x1^3 + d2 x1^2 + j2 x1, x1^3 x2 + u3 x1^2 x2^2 + a3 x1^3 + b3 x1^2 x2 + d3 x1^2 + e3 x1 x2^2 \right.$ $\left. + g3 x1 x2 + j3 x1 + k3 x2^3 + m3 x2^2 + p3 x2 \right]$ |
| > <b>jacobian (H, [x1,x2,x3]) ;</b>         |                                                                                                                                                                                                      |
|                                             | $[0, 0, 0]$                                                                                                                                                                                          |
|                                             | $[x1^3 + 3 a2 x1^2 + 2 d2 x1 + j2, 0, 0]$                                                                                                                                                            |
|                                             | $[3 x1^2 x2 + 2 u3 x1 x2^2 + 3 a3 x1^2 + 2 b3 x1 x2 + 2 d3 x1 + e3 x2^2 + g3 x2 + j3,$                                                                                                               |
|                                             | $x1^3 + 2 u3 x1^2 x2 + b3 x1^2 + 2 e3 x1 x2 + g3 x1 + 3 k3 x2^2 + 2 m3 x2 + p3, 0]$                                                                                                                  |
| > <b>contradict (1, 'u3') ;</b>             |                                                                                                                                                                                                      |
| Contradiction on case level 1, so:          |                                                                                                                                                                                                      |
|                                             | $u3 = 0$                                                                                                                                                                                             |
| Variables to be uneliminated:               |                                                                                                                                                                                                      |
|                                             | "g2 := 'g2'"                                                                                                                                                                                         |
|                                             | "d1 := 'd1'"                                                                                                                                                                                         |
|                                             | "p2 := 'p2'"                                                                                                                                                                                         |
|                                             | "j1 := 'j1'"                                                                                                                                                                                         |
|                                             | "m2 := 'm2'"                                                                                                                                                                                         |
|                                             | "a1 := 'a1'"                                                                                                                                                                                         |
|                                             | "p1 := 'p1'"                                                                                                                                                                                         |
|                                             | "g1 := 'g1'"                                                                                                                                                                                         |
|                                             | "b2 := 'b2'"                                                                                                                                                                                         |
| Proceed on case level 0 with:               |                                                                                                                                                                                                      |
|                                             | $6 \neq 0$                                                                                                                                                                                           |
| On account of:                              |                                                                                                                                                                                                      |
|                                             | $u3 = 0$                                                                                                                                                                                             |
|                                             | $\{1 \neq 0\}$                                                                                                                                                                                       |
| u3 is set to:                               | 0                                                                                                                                                                                                    |
| > <b>launchNZcase (k3) ;</b>                |                                                                                                                                                                                                      |

Launching case level 1:

$$k3 \neq 0$$

Assume from now on that:

$$6 k3 \neq 0$$

> **tmp1 := cpcoeff (x1\*x2^2\*T);**

$$tmp1 := 3 (9 a l^2 + 3 a l b2 + g1 + b2^2) k3$$

> **elimsolve (tmp1,g1);**

$$\{1 \neq 0\}$$

g1 is set to:

$$-9 a l^2 - 3 a l b2 - b2^2$$

> **tmp1 := cpcoeff (x1\*x3\*T);**

$$tmp1 := 2 (3 a l + b2)^4$$

> **elimsolve (tmp1,b2);**

$$\{1 \neq 0\}$$

b2 is set to:

$$-3 a l$$

> **launchNZcase (a1);**

Launching case level 2:

$$a1 \neq 0$$

Assume from now on that:

$$6 k3 a1 \neq 0$$

> **tmp1 := cpcoeff (x1^2\*x2\*T);**

$$tmp1 := -3 a l (-2 m2 + 9 a l^2)$$

> **elimsolve (tmp1,m2);**

$$\{-2 \neq 0\}$$

m2 is set to:

$$\frac{9 a l^2}{2}$$

> **tmp1 := cpcoeff (x1^2\*x2^2);**

$$tmp1 := 9 a l (3 a l g2 - 6 a l d1 + 27 a2 a l^2 - p1) k3$$

> **elimsolve (tmp1,p1);**

$$\{-1 \neq 0\}$$

p1 is set to:

$$3 a l (g2 - 2 d1 + 9 a l a2)$$

> **tmp1 := cpcoeff (x2^2\*T);**

$$tmp1 := -81 a l^4$$

> **contradict (tmp1,'a1');**

Contradiction on case level 2, so:

$$a1 = 0$$

Variables to be uneliminated:

$$"p1 := 'p1'"$$

$$"m2 := 'm2'"$$

Proceed on case level 1 with:

$$6 k3 \neq 0$$

On account of:

$$a1 = 0$$

$$\{1 \neq 0\}$$

a1 is set to:

$$0$$

> **tmp1 := cpcoeff (x2^2\*T);**

$$tmp1 := -4 m2^2 + 3 p1 k3$$

> **elimsolve (tmp1,p1);**

$$\{3 k3 \neq 0\}$$

p1 is set to:

$$\frac{4 m2^2}{3 k3}$$

> **tmp1 := cpcoeff (x3\*T);**

$$tmp1 := -\frac{8 m2^3}{3 k3}$$

> **elimsolve (tmp1,m2);**

$$\{1 \neq 0\}$$

m2 is set to:

$$0$$

> **launchNZcase (j1);**

Launching case level 2:

$$j1 \neq 0$$

Assume from now on that:

$$6 k3 j1 \neq 0$$

> **launchNZcase (p2);**

Launching case level 3:

$$p2 \neq 0$$

Assume from now on that:

$$6 k3 j1 p2 \neq 0$$

> **tmp1 := cpcoeff (1);**

$$tmp1 := j1 p2 (j1 + p2)$$

> **elimsolve (tmp1,p2);**

$$\{1 \neq 0\}$$

p2 is set to:

$$-j1$$

Nonzero constraint refines to:

$$-6 k3 j1^2 \neq 0$$

> **tmp1 := cpcoeff (T);**

$$tmp1 := -j1^2$$

> **contradict (tmp1,'p2');**

Contradiction on case level 3, so:

$$p2 = 0$$

Variables to be uneliminated:

$$"p2 := 'p2'"$$

Proceed on case level 2 with:

|                                    |                               |
|------------------------------------|-------------------------------|
|                                    | $6 k3 j1 \neq 0$              |
| On account of:                     |                               |
|                                    | $p2 = 0$                      |
|                                    | $\{1 \neq 0\}$                |
| p2 is set to:                      |                               |
|                                    | 0                             |
| > <b>tmp1 := cpcoeff (T);</b>      |                               |
|                                    | $tmp1 := -j1^2$               |
| > <b>contradict (tmp1,'j1');</b>   |                               |
| Contradiction on case level 2, so: |                               |
|                                    | $j1 = 0$                      |
| Variables to be uneliminated:      |                               |
|                                    | "p2 := 'p2'"                  |
| Proceed on case level 1 with:      |                               |
|                                    | $6 k3 \neq 0$                 |
| On account of:                     |                               |
|                                    | $j1 = 0$                      |
|                                    | $\{1 \neq 0\}$                |
| j1 is set to:                      |                               |
|                                    | 0                             |
| > <b>tmp1 := cpcoeff (T);</b>      |                               |
|                                    | $tmp1 := -p2^2$               |
| > <b>elimsolve (tmp1,p2);</b>      |                               |
|                                    | $\{1 \neq 0\}$                |
| p2 is set to:                      |                               |
|                                    | 0                             |
| > <b>launchNZcase (d1);</b>        |                               |
| Launching case level 2:            |                               |
|                                    | $d1 \neq 0$                   |
| Assume from now on that:           |                               |
|                                    | $6 k3 d1 \neq 0$              |
| > <b>launchNZcase (g2);</b>        |                               |
| Launching case level 3:            |                               |
|                                    | $g2 \neq 0$                   |
| Assume from now on that:           |                               |
|                                    | $6 k3 d1 g2 \neq 0$           |
| > <b>tmp1 := cpcoeff (x1^3);</b>   |                               |
|                                    | $tmp1 := 2 d1 g2 (2 d1 + g2)$ |
| > <b>elimsolve (tmp1,g2);</b>      |                               |
|                                    | $\{1 \neq 0\}$                |
| g2 is set to:                      |                               |
|                                    | $-2 d1$                       |
| Nonzero constraint refines to:     |                               |
|                                    | $-12 k3 d1^2 \neq 0$          |
| > <b>tmp1 := cpcoeff (x1^2*T);</b> |                               |

```

|                                      $tmp1 := -4 d1^2$ 
| > contradict (tmp1,'g2');
| Contradiction on case level 3, so:
|                                      $g2 = 0$ 
| Variables to be uneliminated:
|                                      $"g2 := 'g2'"$ 
| Proceed on case level 2 with:
|                                      $6 k3 d1 \neq 0$ 
| On account of:
|                                      $g2 = 0$ 
|                                      $\{1 \neq 0\}$ 
| g2 is set to:
|                                     0
| > tmp1 := cpcoeff (x1^2*T);
|                                      $tmp1 := -4 d1^2$ 
| > contradict (tmp1,'d1');
| Contradiction on case level 2, so:
|                                      $d1 = 0$ 
| Variables to be uneliminated:
|                                      $"g2 := 'g2'"$ 
| Proceed on case level 1 with:
|                                      $6 k3 \neq 0$ 
| On account of:
|                                      $d1 = 0$ 
|                                      $\{1 \neq 0\}$ 
| d1 is set to:
|                                     0
| > tmp1 := cpcoeff (x1^2*T);
|                                      $tmp1 := -g2^2$ 
| > elimsolve (tmp1,g2);
|                                      $\{1 \neq 0\}$ 
| g2 is set to:
|                                     0
| > det(T-jacobian(H,[x1,x2,x3]));
|                                      $T^3$ 
| > H;
|  $\left[ 0, \frac{x1^4}{4} + a2 x1^3 + d2 x1^2 + j2 x1, \right.$ 
|  $\left. x1^3 x2 + a3 x1^3 + b3 x1^2 x2 + d3 x1^2 + e3 x1 x2^2 + g3 x1 x2 + j3 x1 + k3 x2^3 + m3 x2^2 + p3 x2 \right]$ 
| > jacobian(H,[x1,x2,x3]);
| [0,0,0]
|  $[x1^3 + 3 a2 x1^2 + 2 d2 x1 + j2, 0, 0]$ 
|  $[3 x1^2 x2 + 3 a3 x1^2 + 2 b3 x1 x2 + 2 d3 x1 + e3 x2^2 + g3 x2 + j3,$ 

```

$$x l^3 + b_3 x l^2 + 2 e_3 x l x_2 + g_3 x l + 3 k_3 x_2^2 + 2 m_3 x_2 + p_3, 0]$$

> **contradict** (1, 'k3');

Contradiction on case level 1, so:

$$k_3 = 0$$

Variables to be uneliminated:

$$g_2 := 'g_2'$$

$$d_1 := 'd_1'$$

$$p_2 := 'p_2'$$

$$j_1 := 'j_1'$$

$$m_2 := 'm_2'$$

$$p_1 := 'p_1'$$

$$a_1 := 'a_1'$$

$$b_2 := 'b_2'$$

$$g_1 := 'g_1'$$

Proceed on case level 0 with:

$$6 \neq 0$$

On account of:

$$k_3 = 0$$

$$\{1 \neq 0\}$$

k3 is set to:

$$0$$

> **launchNZcase** (27\*a1^3+6\*g1\*a1+g1\*b2);

Launching case level 1:

$$27 a l^3 + 6 a l g l + g l b_2 \neq 0$$

Assume from now on that:

$$162 a l^3 + 36 a l g l + 6 g l b_2 \neq 0$$

> **tmp1** := **cpcoeff** (x2^2\*T);

$$tmp1 := -2 g l m_2 - 4 m_2^2 - g l^2 + 27 e_3 a l^3 + 6 e_3 a l g l + e_3 g l b_2$$

> **elimsolve** (tmp1,e3);

$$\{27 a l^3 + 6 a l g l + g l b_2 \neq 0\}$$

e3 is set to:

$$\frac{2 g l m_2 + 4 m_2^2 + g l^2}{27 a l^3 + 6 a l g l + g l b_2}$$

> **tmp1** := **cpcoeff** (x2\*T);

$$tmp1 := -g l p_2 + 6 m_3 a l g_2 + 4 m_3 d_1 b_2 + 6 m_3 a_2 g l - 6 m_3 b_3 a l b_2 - 18 m_3 b_3 a l^2 \\ - 2 m_3 b_3 g l - 2 m_3 b_3 b_2^2 + 4 m_3 b_2 g_2 + 24 m_3 a l d_1 + 2 m_3 p_1 - 2 j_1 m_2 - 4 m_2 p_2 \\ - 2 j_1 g l - g_2 p_1 + 27 g_3 a l^3 + 6 g_3 a l g l + g_3 g l b_2$$

> **elimsolve** (tmp1,g3);

$$\{27 a l^3 + 6 a l g l + g l b_2 \neq 0\}$$

g3 is set to:

$$(g l p_2 - 6 m_3 a l g_2 - 4 m_3 d_1 b_2 - 6 m_3 a_2 g l + 6 m_3 b_3 a l b_2 + 18 m_3 b_3 a l^2 + 2 m_3 b_3 g l \\ + 2 m_3 b_3 b_2^2 - 4 m_3 b_2 g_2 - 24 m_3 a l d_1 - 2 m_3 p_1 + 2 j_1 m_2 + 4 m_2 p_2 + 2 j_1 g l + g_2 p_1)$$

$$\big/ (27 a l^3 + 6 a l g l + g l b 2)$$

> **tmp1 := cpcoeff (T);**

$$\begin{aligned} tmp1 := & -j l p 2 - p 2^2 + 3 p 3 a l g 2 + 2 p 3 d l b 2 + 3 p 3 a 2 g l - 3 p 3 b 3 a l b 2 - 9 p 3 b 3 a l^2 \\ & - p 3 b 3 g l - p 3 b 3 b 2^2 + 2 p 3 b 2 g 2 + 12 p 3 a l d l + p 3 p l - j 2 p l + 27 j 3 a l^3 + 6 j 3 a l g l \\ & + j 3 g l b 2 - j l^2 \end{aligned}$$

> **elimsolve (tmp1, j3);**

$$\{27 a l^3 + 6 a l g l + g l b 2 \neq 0\}$$

j3 is set to:

$$\begin{aligned} (j l p 2 + p 2^2 - 3 p 3 a l g 2 - 2 p 3 d l b 2 - 3 p 3 a 2 g l + 3 p 3 b 3 a l b 2 + 9 p 3 b 3 a l^2 + p 3 b 3 g l \\ + p 3 b 3 b 2^2 - 2 p 3 b 2 g 2 - 12 p 3 a l d l - p 3 p l + j 2 p l + j l^2) \big/ (27 a l^3 + 6 a l g l + g l b 2) \end{aligned}$$

> **tmp1 := cpcoeff (x1^5);**

$$\begin{aligned} tmp1 := & 27 b 3 a l^3 - 54 a l^2 d l + 81 a 2 a l^3 - 6 p l a l - g l g 2 - 4 g l d l + b 3 g l b 2 \\ & + 6 b 3 a l g l - b 2 p l \end{aligned}$$

> **elimsolve (tmp1, b3);**

$$\{27 a l^3 + 6 a l g l + g l b 2 \neq 0\}$$

b3 is set to:

$$-\frac{-54 a l^2 d l + 81 a 2 a l^3 - 6 p l a l - g l g 2 - 4 g l d l - b 2 p l}{27 a l^3 + 6 a l g l + g l b 2}$$

> **launchNZcase (2\*m2+g1);**

Launching case level 2:

$$2 m 2 + g l \neq 0$$

Assume from now on that:

$$6 (27 a l^3 + 6 a l g l + g l b 2) (2 m 2 + g l) \neq 0$$

> **tmp1 := cpcoeff (x3^2);**

$$tmp1 := (9 a l^2 + 3 a l b 2 + g l + b 2^2) (27 a l^3 + 6 a l g l + g l b 2) (2 m 2 + g l)$$

> **elimsolve (tmp1, g1);**

$$\{1 \neq 0\}$$

g1 is set to:

$$-9 a l^2 - 3 a l b 2 - b 2^2$$

Nonzero constraint refines to:

$$6 (-3 a l - b 2) (2 m 2 - 9 a l^2 - 3 a l b 2 - b 2^2) \neq 0$$

> **tmp1 := cpcoeff (x1\*x3\*T);**

$$tmp1 := 2 (3 a l + b 2)^4$$

> **contradict (tmp1, 'g1');**

Contradiction on case level 2, so:

$$2 m 2 + g l = 0$$

Variables to be uneliminated:

$$"g1 := 'g1'"$$

Proceed on case level 1 with:

$$162 a l^3 + 36 a l g l + 6 g l b 2 \neq 0$$

On account of:

$$2 m 2 + g l = 0$$

```

{1 ≠ 0}
g1 is set to:
-2 m2
Nonzero constraint refines to:
162 a l^3 - 72 a l m2 - 12 m2 b2 ≠ 0
> tmp1 := cpcoeff(x2^3);
tmp1 := -8 m2^3
> elimsolve (tmp1,m2);
{1 ≠ 0}
m2 is set to:
0
Nonzero constraint refines to:
18 a l ≠ 0
> tmp1 := cpcoeff(x1^2*x2*T);
tmp1 := 81 a l^3
> eq1 := contradict (tmp1);
Contradiction on case level 1, so:
27 a l^3 + 6 a l g1 + g1 b2 = 0
Variables to be uneliminated:
"m2 := 'm2"
"gl := 'gl"
"b3 := 'b3"
"j3 := 'j3"
"g3 := 'g3"
"e3 := 'e3"
Proceed on case level 0 with:
6 ≠ 0
On account of:
27 a l^3 + 6 a l g1 + g1 b2 = 0
the following return value can be used as an equation:
eq1 := 27 a l^3 + 6 a l g1 + g1 b2
> launchNZcase (g1);
Launching case level 1:
gl ≠ 0
Assume from now on that:
6 gl ≠ 0
> elimsolve (eq1,b2);
{gl ≠ 0}
b2 is set to:
- 3 a l (9 a l^2 + 2 g1)
gl
> launchNZcase (m2);
Launching case level 2:
m2 ≠ 0
Assume from now on that:

```

```

[
  > tmp1 := cpcoeff (x1*x3*T);
                                      $6\,g\,l\,m2 \neq 0$ 
                                     
$$tmp1 := -\frac{2\,(g\,l + 9\,a\,l^2)^3\,m2}{g\,l^2}$$

  > elimsolve (tmp1,g1);
                                      $\{1 \neq 0\}$ 
  g1 is set to:
                                      $-9\,a\,l^2$ 
  Nonzero constraint refines to:
                                      $-18\,a\,l\,m2 \neq 0$ 
  > tmp1 := cpcoeff (x1^2*x2^2);
                                     
$$tmp1 := 3\,a\,l\,(-2\,m2 + 9\,a\,l^2)^2$$

  > elimsolve (tmp1,m2);
                                      $\{-2 \neq 0\}$ 
  m2 is set to:
                                     
$$\frac{9\,a\,l^2}{2}$$

  Nonzero constraint refines to:
                                      $-54\,a\,l^2 \neq 0$ 
  > tmp1 := cpcoeff (x2^2*T);
                                     
$$tmp1 := -81\,a\,l^4$$

  > contradict (tmp1,'m2');
  Contradiction on case level 2, so:
                                      $m2 = 0$ 
  Variables to be uneliminated:
                                     "m2 := 'm2'"
                                     "g1 := 'g1'"
  Proceed on case level 1 with:
                                      $6\,g\,l \neq 0$ 
  On account of:
                                      $m2 = 0$ 
                                      $\{1 \neq 0\}$ 
  m2 is set to:
                                     0
  > tmp1 := cpcoeff (x2^2*T);
                                     
$$tmp1 := -g\,l^2$$

  > contradict (tmp1,'g1');
  Contradiction on case level 1, so:
                                      $g\,l = 0$ 
  Variables to be uneliminated:
                                     "m2 := 'm2'"
                                     "b2 := 'b2'"
  Proceed on case level 0 with:

```

|                                       |                                                                                                 |
|---------------------------------------|-------------------------------------------------------------------------------------------------|
|                                       | $6 \neq 0$                                                                                      |
| On account of:                        |                                                                                                 |
|                                       | $g1 = 0$                                                                                        |
|                                       | $\{1 \neq 0\}$                                                                                  |
| g1 is set to:                         |                                                                                                 |
|                                       | 0                                                                                               |
| > <b>elimsolve</b> (eq1,a1);          |                                                                                                 |
|                                       | $\{1 \neq 0\}$                                                                                  |
| a1 is set to:                         |                                                                                                 |
|                                       | 0                                                                                               |
| > <b>tmp1 := cpcoeff</b> (x2^2*T);    |                                                                                                 |
|                                       | $tmp1 := -4 m2^2$                                                                               |
| > <b>elimsolve</b> (tmp1,m2);         |                                                                                                 |
|                                       | $\{1 \neq 0\}$                                                                                  |
| m2 is set to:                         |                                                                                                 |
|                                       | 0                                                                                               |
| > <b>launchNZcase</b> (b2);           |                                                                                                 |
| Launching case level 1:               |                                                                                                 |
|                                       | $b2 \neq 0$                                                                                     |
| Assume from now on that:              |                                                                                                 |
|                                       | $6 b2 \neq 0$                                                                                   |
| > <b>tmp1 := cpcoeff</b> (x3*T);      |                                                                                                 |
|                                       | $tmp1 := b2^2 p1$                                                                               |
| > <b>elimsolve</b> (tmp1,p1);         |                                                                                                 |
|                                       | $\{1 \neq 0\}$                                                                                  |
| p1 is set to:                         |                                                                                                 |
|                                       | 0                                                                                               |
| > <b>tmp1 := cpcoeff</b> (x1^2*x2*T); |                                                                                                 |
|                                       | $tmp1 := 2 b2^2 e3$                                                                             |
| > <b>elimsolve</b> (tmp1,e3);         |                                                                                                 |
|                                       | $\{1 \neq 0\}$                                                                                  |
| e3 is set to:                         |                                                                                                 |
|                                       | 0                                                                                               |
| > <b>tmp1 := cpcoeff</b> (x1*x2*T);   |                                                                                                 |
|                                       | $tmp1 := 2 m3 b2^2$                                                                             |
| > <b>elimsolve</b> (tmp1,m3);         |                                                                                                 |
|                                       | $\{1 \neq 0\}$                                                                                  |
| m3 is set to:                         |                                                                                                 |
|                                       | 0                                                                                               |
| > <b>tmp1 := cpcoeff</b> (x1*T);      |                                                                                                 |
|                                       | $tmp1 := -2 d1 p2 - 2 p2 g2 - j1 g2 + 2 g3 d1 b2 - g3 b3 b2^2 + 2 g3 b2 g2 + p3 b2^2 - 4 j1 d1$ |
| > <b>elimsolve</b> (tmp1,p3);         |                                                                                                 |
|                                       | $\{-b2^2 \neq 0\}$                                                                              |
| p3 is set to:                         |                                                                                                 |

$$\frac{2 d l p 2+2 p 2 g 2+j 1 g 2-2 g 3 d l b 2+g 3 b 3 b 2^2-2 g 3 b 2 g 2+4 j 1 d l}{b 2^2}$$

> **tmp1 := cpcoeff (x1^2\*T);**

$$tmp1 := g 3 b 2^2-2 d l g 2-2 p 2 b 2-4 d l^2+2 b 3 d l b 2-b 3^2 b 2^2+2 b 3 b 2 g 2-j 1 b 2-g 2^2$$

> **elimsolve (tmp1,g3);**

$$\{-b 2^2 \neq 0\}$$

g3 is set to:

$$\frac{2 d l g 2+2 p 2 b 2+4 d l^2-2 b 3 d l b 2+b 3^2 b 2^2-2 b 3 b 2 g 2+j 1 b 2+g 2^2}{b 2^2}$$

> **tmp1 := cpcoeff (x1^3);**

$$tmp1 := -8 d l^3$$

> **elimsolve (tmp1,d1);**

$$\{1 \neq 0\}$$

d1 is set to:

$$0$$

> **launchNZcase (j1);**

Launching case level 2:

$$j 1 \neq 0$$

Assume from now on that:

$$6 j 1 b 2 \neq 0$$

> **launchNZcase (p2\*b2-3\*b3\*b2\*g2+b3^2\*b2^2+2\*g2^2);**

Launching case level 3:

$$p 2 b 2-3 b 3 b 2 g 2+b 3^2 b 2^2+2 g 2^2 \neq 0$$

Assume from now on that:

$$6 b 2 j 1 (p 2 b 2-3 b 3 b 2 g 2+b 3^2 b 2^2+2 g 2^2) \neq 0$$

> **tmp1 := cpcoeff (1);**

tmp1 :=

$$\frac{j 1 (p 2 b 2-3 b 3 b 2 g 2+b 3^2 b 2^2+2 g 2^2) (b 3^2 b 2^2-3 b 3 b 2 g 2+j 1 b 2+p 2 b 2+2 g 2^2)}{b 2^2}$$

> **elimsolve (tmp1,p2);**

$$\{b 2 \neq 0\}$$

p2 is set to:

$$-\frac{b 3^2 b 2^2-3 b 3 b 2 g 2+j 1 b 2+2 g 2^2}{b 2}$$

Nonzero constraint refines to:

$$-6 b 2^2 j 1^2 \neq 0$$

> **tmp1 := cpcoeff (T);**

$$tmp1 := -j 1^2$$

> **contradict (tmp1,'p2');**

Contradiction on case level 3, so:

$$p 2 b 2-3 b 3 b 2 g 2+b 3^2 b 2^2+2 g 2^2=0$$

Variables to be uneliminated:

$$"p 2 := 'p 2'"$$

Proceed on case level 2 with:

$$6 j l b 2 \neq 0$$

On account of:

$$p 2 b 2 - 3 b 3 b 2 g 2 + b 3^2 b 2^2 + 2 g 2^2 = 0$$
$$\{b 2 \neq 0\}$$

p2 is set to:

$$-\frac{(-g 2 + b 2 b 3)(b 2 b 3 - 2 g 2)}{b 2}$$

> **tmp1 := cpcoeff (T);**

$$tmp1 := -j l^2$$

> **contradict (tmp1, 'j1');**

Contradiction on case level 2, so:

$$j l = 0$$

Variables to be uneliminated:

$$"p 2 := 'p 2'"$$

Proceed on case level 1 with:

$$6 b 2 \neq 0$$

On account of:

$$j l = 0$$

$$\{1 \neq 0\}$$

j1 is set to:

$$0$$

> **tmp1 := cpcoeff (T);**

$$tmp1 := -\frac{(p 2 b 2 - 3 b 3 b 2 g 2 + b 3^2 b 2^2 + 2 g 2^2)^2}{b 2^2}$$

> **elimsolve (tmp1, p2);**

$$\{b 2 \neq 0\}$$

p2 is set to:

$$-\frac{(-g 2 + b 2 b 3)(b 2 b 3 - 2 g 2)}{b 2}$$

> **det (T-jacobian (H, [x1, x2, x3])) ;**

$$T^3$$

> **simplify (evalm ([H[1], H[2], H[3]])) ;**

$$[0, (x l^4 b 2 + 4 a 2 x l^3 b 2 + 4 b 2^2 x l^2 x 2 + 4 d 2 x l^2 b 2 + 4 g 2 x l x 2 b 2 - 4 b 2^3 x l x 3$$
$$+ 4 j 2 x l b 2 - 4 x 2 b 3^2 b 2^2 + 12 x 2 b 3 b 2 g 2 - 8 x 2 g 2^2 + 4 b 2^3 x 3 b 3 - 8 b 2^2 x 3 g 2) / (4 b 2),$$
$$(x l^3 x 2 b 2^3 + a 3 x l^3 b 2^3 + b 3 x l^2 x 2 b 2^3 - b 2^4 x l^2 x 3 + d 3 x l^2 b 2^3 - b 2^3 x l x 2 b 3^2$$
$$+ 4 b 2^2 x l x 2 b 3 g 2 - 3 b 2 x l x 2 g 2^2 - g 2 x l x 3 b 2^3 + j 3 x l b 2^3 + 4 x 2 b 2^2 b 3^2 g 2$$
$$- 5 x 2 b 2 b 3 g 2^2 + 2 x 2 g 2^3 - x 2 b 2^3 b 3^3 + b 2^4 x 3 b 3^2 - 3 b 2^3 x 3 b 3 g 2 + 2 b 2^2 x 3 g 2^2) / b 2^3]$$

> **M := evalm ([ [C, 0, 0], [0, -4\*C^4\*b2, 0],**

> **[0, 4\*C^5\*(2\*b3\*b2-3\*g2), -4\*b2^2\*C^5]]);**

$$M := \begin{bmatrix} C & 0 & 0 \\ 0 & -4 C^4 b2 & 0 \\ 0 & 4 C^5 (2 b2 b3 - 3 g2) & -4 b2^2 C^5 \end{bmatrix}$$

> **det(M) ;**

$$16 C^{10} b2^3$$

> **G := simplify(evalm(M&\*subs({seq([x1,x2,x3][i]=  
> evalm(M^(-1)&\*[x1,x2,x3])[i],i=1..n)},H))) ;**

$$G := [0, -(x1^4 C^2 b2^2 + 4 a2 x1^3 C^3 b2^2 - b2^2 x1^2 x2 + 4 d2 x1^2 C^4 b2^2 - 4 g2 x1 x2 C b2 + 2 b2^2 x1 x2 C b3 + b2^2 x1 x3 + 4 j2 x1 C^5 b2^2 - x2 C^2 b3^2 b2^2 + 4 x2 C^2 b3 b2 g2 - 4 x2 C^2 g2^2 - C b2^2 b3 x3 + 2 C g2 x3 b2) / (C^2 b2), (-4 j3 x1 C^6 b2^4 + x1^3 x2 b2^3 - x2 C^3 b2^3 b3^3 + 4 C^2 b3 b2^2 g2 x3 + 6 b2^2 x1^2 x2 C g2 + 3 x1 x2 C^2 b2^3 b3^2 - 12 x1 x2 C^2 b2^2 b3 g2 + 12 x1 x2 C^2 b2 g2^2 - 4 g2 x1 C b2^2 x3 + 6 x2 C^3 b2^2 b3^2 g2 - 12 x2 C^3 b2 b3 g2^2 - C^2 b3^2 b2^3 x3 - 4 C^2 g2^2 x3 b2 - 4 a3 x1^3 C^4 b2^4 - 3 b3 x1^2 x2 C b2^3 - 4 d3 x1^2 C^5 b2^4 - b2^3 x1^2 x3 + 8 x2 C^3 g2^3 + 8 b2^3 b3 d2 x1^2 C^5 + 2 C b2^3 b3 x1 x3 + 8 b2^3 b3 j2 x1 C^6 + 8 b2^3 b3 a2 x1^3 C^4 - 12 g2 a2 x1^3 C^4 b2^2 - 12 g2 d2 x1^2 C^5 b2^2 - 12 g2 j2 x1 C^6 b2^2 + 2 b2^3 b3 x1^4 C^3 - 3 g2 x1^4 C^3 b2^2) / (b2^2 C^2)]$$

> **simplify(jacobian(subs(x1=x1+C\*(b3-2\*g2/b2),evalm(G)), [x2,x3])) ;**

$$\begin{bmatrix} 0 & 0 \\ \frac{b2 x1^2}{C^2} & -\frac{b2 x1}{C^2} \\ \frac{b2 x1^3}{C^2} & -\frac{b2 x1^2}{C^2} \end{bmatrix}$$

> **contradict (1,'b2') ;**

Contradiction on case level 1, so:

$$b2 = 0$$

Variables to be uneliminated:

"p2 := 'p2'"

"j1 := 'j1'"

"d1 := 'd1'"

"g3 := 'g3'"

"p3 := 'p3'"

"m3 := 'm3'"

"e3 := 'e3'"

"p1 := 'p1'"

Proceed on case level 0 with:

$$6 \neq 0$$

On account of:

$$b2 = 0$$

$$\{1 \neq 0\}$$

b2 is set to:

```

[
0
> launchNZcase (p1);
Launching case level 1:

Assume from now on that:
 $p1 \neq 0$ 
 $6 p1 \neq 0$ 
> tmp1 := cpcoeff (x2^2);
 $tmp1 := e3 p1^2$ 
> elimsolve (tmp1,e3);
 $\{1 \neq 0\}$ 
e3 is set to:
0
> tmp1 := cpcoeff (x1^2*x2);
 $tmp1 := 3 p1^2$ 
> contradict (tmp1,'p1');
Contradiction on case level 1, so:
 $p1 = 0$ 
Variables to be uneliminated:
"e3 := 'e3'"
Proceed on case level 0 with:
 $6 \neq 0$ 
On account of:
 $p1 = 0$ 
 $\{1 \neq 0\}$ 
p1 is set to:
0
> launchNZcase (j1);
Launching case level 1:

Assume from now on that:
 $j1 \neq 0$ 
 $6 j1 \neq 0$ 
> launchNZcase (p2);
Launching case level 2:

Assume from now on that:
 $p2 \neq 0$ 
 $6 j1 p2 \neq 0$ 
> tmp1 := cpcoeff (1);
 $tmp1 := j1 p2 (j1 + p2)$ 
> elimsolve (tmp1,p2);
 $\{1 \neq 0\}$ 
p2 is set to:
 $-j1$ 
Nonzero constraint refines to:
 $-6 j1^2 \neq 0$ 
> tmp1 := cpcoeff (T);

```

```

[                                      $tmp1 := -j1^2$ 
> contradict (tmp1,'p2');
Contradiction on case level 2, so:
                                      $p2 = 0$ 
Variables to be uneliminated:
                                     "p2 := 'p2'"
Proceed on case level 1 with:
                                      $6j1 \neq 0$ 
On account of:
                                      $p2 = 0$ 
                                      $\{1 \neq 0\}$ 
p2 is set to:
                                     0
> tmp1 := cpcoeff (T);
[                                      $tmp1 := -j1^2$ 
> contradict (tmp1,'j1');
Contradiction on case level 1, so:
                                      $j1 = 0$ 
Variables to be uneliminated:
                                     "p2 := 'p2'"
Proceed on case level 0 with:
                                      $6 \neq 0$ 
On account of:
                                      $j1 = 0$ 
                                      $\{1 \neq 0\}$ 
j1 is set to:
                                     0
> tmp1 := cpcoeff (T);
[                                      $tmp1 := -p2^2$ 
> elimsolve (tmp1,'p2');
                                      $\{1 \neq 0\}$ 
p2 is set to:
                                     0
> launchNZcase (d1);
Launching case level 1:
                                      $d1 \neq 0$ 
Assume from now on that:
                                      $6d1 \neq 0$ 
> launchNZcase (g2);
Launching case level 2:
                                      $g2 \neq 0$ 
Assume from now on that:
                                      $6d1g2 \neq 0$ 
> tmp1 := cpcoeff (x1^3);
[                                      $tmp1 := 2d1g2(2d1 + g2)$ 
> elimsolve (tmp1,g2);

```

|                                         |                                                                   |
|-----------------------------------------|-------------------------------------------------------------------|
|                                         | $\{1 \neq 0\}$                                                    |
| g2 is set to:                           |                                                                   |
|                                         | $-2\,dl$                                                          |
| Nonzero constraint refines to:          |                                                                   |
|                                         | $-12\,dl^2 \neq 0$                                                |
| > <b>tmp1 := cpcoeff (x1^2*T);</b>      |                                                                   |
|                                         | $tmp1 := -4\,dl^2$                                                |
| > <b>contradict (tmp1,'g2');</b>        |                                                                   |
| Contradiction on case level 2, so:      |                                                                   |
|                                         | $g2 = 0$                                                          |
| Variables to be uneliminated:           |                                                                   |
|                                         | "g2 := 'g2'"                                                      |
| Proceed on case level 1 with:           |                                                                   |
|                                         | $6\,dl \neq 0$                                                    |
| On account of:                          |                                                                   |
|                                         | $g2 = 0$                                                          |
|                                         | $\{1 \neq 0\}$                                                    |
| g2 is set to:                           |                                                                   |
|                                         | 0                                                                 |
| > <b>tmp1 := cpcoeff (x1^2*T);</b>      |                                                                   |
|                                         | $tmp1 := -4\,dl^2$                                                |
| > <b>contradict (tmp1,'d1');</b>        |                                                                   |
| Contradiction on case level 1, so:      |                                                                   |
|                                         | $dl = 0$                                                          |
| Variables to be uneliminated:           |                                                                   |
|                                         | "g2 := 'g2'"                                                      |
| Proceed on case level 0 with:           |                                                                   |
|                                         | $6 \neq 0$                                                        |
| On account of:                          |                                                                   |
|                                         | $dl = 0$                                                          |
|                                         | $\{1 \neq 0\}$                                                    |
| d1 is set to:                           |                                                                   |
|                                         | 0                                                                 |
| > <b>tmp1 := cpcoeff (x1^2*T);</b>      |                                                                   |
|                                         | $tmp1 := -g2^2$                                                   |
| > <b>elimsolve (tmp1,g2);</b>           |                                                                   |
|                                         | $\{1 \neq 0\}$                                                    |
| g2 is set to:                           |                                                                   |
|                                         | 0                                                                 |
| > <b>det(T-jacobian(H,[x1,x2,x3]));</b> |                                                                   |
|                                         | $T^3$                                                             |
| > <b>H;</b>                             |                                                                   |
|                                         | $\left[0, \frac{x1^4}{4} + a2\,x1^3 + d2\,x1^2 + j2\,x1, \right.$ |

$$x_1^3 x_2 + a_3 x_1^3 + b_3 x_1^2 x_2 + d_3 x_1^2 + e_3 x_1 x_2^2 + g_3 x_1 x_2 + j_3 x_1 + m_3 x_2^2 + p_3 x_2$$

> **jacobian**(H, [x1, x2, x3]) ;

[0, 0, 0]

$$[x_1^3 + 3 a_2 x_1^2 + 2 d_2 x_1 + j_2, 0, 0]$$

$$[3 x_1^2 x_2 + 3 a_3 x_1^2 + 2 b_3 x_1 x_2 + 2 d_3 x_1 + e_3 x_2^2 + g_3 x_2 + j_3,$$

$$x_1^3 + b_3 x_1^2 + 2 e_3 x_1 x_2 + g_3 x_1 + 2 m_3 x_2 + p_3, 0]$$

> **contradict** (1) ;

Contradiction on case level 0, so:

$$6 = 0$$

Variables to be uneliminated:

"g2 := 'g2'"

"d1 := 'd1'"

"p2 := 'p2'"

"j1 := 'j1'"

"p1 := 'p1'"

"b2 := 'b2'"

"m2 := 'm2'"

"a1 := 'a1'"

"g1 := 'g1'"

"k3 := 'k3'"

"u3 := 'u3'"

"v3 := 'v3'"

"m1 := 'm1'"

"w3 := 'w3'"

"k2 := 'k2'"

"e2 := 'e2'"

"b1 := 'b1'"

"e1 := 'e1'"

"k1 := 'k1'"

"s1 := 's1'"

"r1 := 'r1'"

"q1 := 'q1'"

"o1 := 'o1'"

"n1 := 'n1'"

"l1 := 'l1'"

"i1 := 'i1'"

"h1 := 'h1'"

"f1 := 'f1'"

```

"c1 := 'c1'"
"s2 := 's2'"
"r2 := 'r2'"
"q2 := 'q2'"
"o2 := 'o2'"
"n2 := 'n2'"
"l2 := 'l2'"
"i2 := 'i2'"
"h2 := 'h2'"
"f2 := 'f2'"
"c2 := 'c2'"
"s3 := 's3'"
"r3 := 'r3'"
"q3 := 'q3'"
"o3 := 'o3'"
"n3 := 'n3'"
"l3 := 'l3'"
"i3 := 'i3'"
"h3 := 'h3'"
"f3 := 'f3'"
"c3 := 'c3'"

```

That is all, folks! Check that all variables are uneliminated:

```

[[a1, b1, c1, d1, e1, f1, g1, h1, i1, j1, k1, l1, m1, n1, o1, p1, q1, r1, s1],
 [a2, b2, c2, d2, e2, f2, g2, h2, i2, j2, k2, l2, m2, n2, o2, p2, q2, r2, s2],
 [a3, b3, c3, d3, e3, f3, g3, h3, i3, j3, k3, l3, m3, n3, o3, p3, q3, r3, s3]]

```

```

> startnewHcase ();

```

Starting case H = H2:

$$\begin{aligned}
 & \left[ a1 x1^3 + b1 x1^2 x2 + c1 x1^2 x3 + d1 x1^2 + e1 x1 x2^2 + f1 x1 x2 x3 + g1 x1 x2 + h1 x1 x3^2 \right. \\
 & \quad + i1 x1 x3 + j1 x1 + k1 x2^3 + l1 x2^2 x3 + m1 x2^2 + n1 x2 x3^2 + o1 x2 x3 + p1 x2 + q1 x3^3 \\
 & \quad + r1 x3^2 + s1 x3, \frac{x1^4}{4} + u2 x1^2 x3^2 + v2 x1 x3^3 + w2 x3^4 + a2 x1^3 + b2 x1^2 x2 + c2 x1^2 x3 \\
 & \quad + d2 x1^2 + e2 x1 x2^2 + f2 x1 x2 x3 + g2 x1 x2 + h2 x1 x3^2 + i2 x1 x3 + j2 x1 + k2 x2^3 \\
 & \quad + l2 x2^2 x3 + m2 x2^2 + n2 x2 x3^2 + o2 x2 x3 + p2 x2 + q2 x3^3 + r2 x3^2 + s2 x3, a3 x1^3 \\
 & \quad + b3 x1^2 x2 + c3 x1^2 x3 + d3 x1^2 + e3 x1 x2^2 + f3 x1 x2 x3 + g3 x1 x2 + h3 x1 x3^2 + i3 x1 x3 \\
 & \quad \left. + j3 x1 + k3 x2^3 + l3 x2^2 x3 + m3 x2^2 + n3 x2 x3^2 + o3 x2 x3 + p3 x2 + q3 x3^3 + r3 x3^2 + s3 x3 \right]
 \end{aligned}$$

```

> initcases (6);

```

We assume the following in our calculation:

$$6 \neq 0$$

```

> for i from 2 by -1 to 0 do
>   for j from 3-i by -1 to 1 do
>     for k from 3-i-j by -1 to 0 do
>       v := coeff (coeff (coeff (H[2],x1,i),x2,j),x3,k);
>       m := cpcoeff (x1^i * x2^(j-1) * x3^k * T^2);
>       elimsolve (m,v);
>     od
>   od;
> od;

```

b2 is set to:

$$\{1 \neq 0\}$$

e2 is set to:

$$-3 a1 - c3$$

$$\{2 \neq 0\}$$

f2 is set to:

$$-\frac{f3}{2} - b1$$

$$\{1 \neq 0\}$$

g2 is set to:

$$-2 h3 - 2 c1$$

$$\{1 \neq 0\}$$

k2 is set to:

$$-2 d1 - i3$$

$$\{3 \neq 0\}$$

l2 is set to:

$$-\frac{l3}{3} - \frac{e1}{3}$$

$$\{2 \neq 0\}$$

m2 is set to:

$$-\frac{f1}{2} - n3$$

$$\{2 \neq 0\}$$

n2 is set to:

$$-\frac{o3}{2} - \frac{g1}{2}$$

$$\{1 \neq 0\}$$

o2 is set to:

$$-3 q3 - h1$$

$$\{1 \neq 0\}$$

p2 is set to:

$$-2 r3 - i1$$

$$\{1 \neq 0\}$$

> for i from 2 by -1 to 0 do

$$-j1 - s3$$

```

> for j from 3-i by -1 to 1 do
>   for k from 3-i-j by -1 to 0 do
>     v := coeff (coeff (coeff (H[1],x1,i),x2,j),x3,k);
>     m := cpcoeff (x1^(i+3) * x2^(j-1) * x3^k * T);
>     elimsolve (m,v);
>   od
> od;
> od;

```

b1 is set to:  $\{1 \neq 0\}$

0

e1 is set to:  $\{1 \neq 0\}$

0

f1 is set to:  $\{1 \neq 0\}$

$-2 u2 b3$

g1 is set to:  $\{1 \neq 0\}$

$-c2 b3 - 3 a1 c3 - c3^2 - 9 a1^2 - 3 a3 c1$

k1 is set to:  $\{1 \neq 0\}$

0

l1 is set to:  $\{1 \neq 0\}$

$-2 u2 e3$

m1 is set to:  $\{2 \neq 0\}$

$3 a3 u2 b3 - \frac{3 a1 f3}{2} - f3 c3 - c2 e3 + b3 h3$

n1 is set to:  $\{1 \neq 0\}$

$-3 v2 b3 - 2 u2 f3$

o1 is set to:  $\{1 \neq 0\}$

$6 a2 u2 b3 - 12 c1 a1 - 4 c1 c3 - 6 a3 h1 - 4 c3 h3 - 6 a1 h3 - 2 u2 g3 - c2 f3 - 2 h2 b3$

p1 is set to:  $\{-1 \neq 0\}$

$-3 a3 i1 - 12 a1 d1 - 3 a1 i3 - 2 d1 c3 - 2 c3 i3 + 3 a2 c2 b3 + 9 a2 a1 c3 + 3 a2 c3^2$   
 $+ 27 a2 a1^2 + 9 a2 a3 c1 - 2 d3 c1 - c2 g3 - i2 b3$

```

> launchNZcase (k3);

```

Launching case level 1:

$k3 \neq 0$

Assume from now on that:

$6 k3 \neq 0$

```

[ > tmp1 := cpcoeff (x2^2*x3^3*T);
                                     tmp1 := -12 w2 k3
[ > elimsolve (tmp1,w2);
                                     {1 ≠ 0}
w2 is set to:
                                     0
[ > tmp1 := cpcoeff (x1*x2^2*x3^2*T);
                                     tmp1 := -9 v2 k3
[ > elimsolve (tmp1,v2);
                                     {1 ≠ 0}
v2 is set to:
                                     0
[ > tmp1 := cpcoeff (x1^2*x2^2*x3*T);
                                     tmp1 := -6 u2 k3
[ > elimsolve (tmp1,u2);
                                     {1 ≠ 0}
u2 is set to:
                                     0
[ > tmp1 := cpcoeff (x1^3*x2^2*x3^2);
                                     tmp1 := -9 q1 k3
[ > elimsolve (tmp1,q1);
                                     {1 ≠ 0}
q1 is set to:
                                     0
[ > tmp1 := cpcoeff (x1^4*x2^2*x3);
                                     tmp1 := -6 h1 k3
[ > elimsolve (tmp1,h1);
                                     {1 ≠ 0}
h1 is set to:
                                     0
[ > tmp1 := cpcoeff (x1^5*x2^2);
                                     tmp1 := -3 c1 k3
[ > elimsolve (tmp1,c1);
                                     {1 ≠ 0}
c1 is set to:
                                     0
[ > tmp1 := cpcoeff (x2^4*T);
                                     tmp1 := 3 n3 k3 - l3^2
[ > elimsolve (tmp1,n3);
                                     {3 k3 ≠ 0}
n3 is set to:
                                      $\frac{l3^2}{3 k3}$ 
[ > tmp1 := cpcoeff (x2^3*x3*T);

```

$$tmp1 := \frac{2(-l^3 + 27 q_3 k^3)}{3 k^3}$$

> **elimsolve** (tmp1,q3);

$$\{27 k^3 \neq 0\}$$

q3 is set to:

$$\frac{l^3}{27 k^3}$$

> **tmp1** := **cpcoeff** (x2^2\*x3^2\*T);

$$tmp1 := -\frac{81 q_2 k^3 + l^4}{9 k^3}$$

> **elimsolve** (tmp1,q2);

$$\{81 k^3 \neq 0\}$$

q2 is set to:

$$-\frac{l^4}{81 k^3}$$

> **tmp1** := **cpcoeff** (x1\*x2^2\*x3\*T);

$$tmp1 := -\frac{54 h_2 k^3 - 4 l^3 e_3 + 9 l^2 f_3 k}{9 k^3}$$

> **elimsolve** (tmp1,h2);

$$\{54 k^3 \neq 0\}$$

h2 is set to:

$$\frac{l^3 (4 l e_3 - 9 f_3 k)}{54 k^3}$$

> **tmp1** := **cpcoeff** (x1\*x2^3\*T);

$$tmp1 := \frac{2(-3 l^3 f_3 k + 9 h_3 k^3 + l^3 e_3)}{3 k^3}$$

> **elimsolve** (tmp1,h3);

$$\{9 k^3 \neq 0\}$$

h3 is set to:

$$-\frac{l^3 (-3 f_3 k + l^3 e_3)}{9 k^3}$$

> **tmp1** := **cpcoeff** (x1^3\*x2^2\*x3);

$$tmp1 := -\frac{6 a l^3 e_3 + 12 l^2 c_2 e_3 k - l^3 b_3 f_3 + 4 c_3 l^3 e_3 - 9 l^3 c_2 f_3 k^2 + 54 r_1 k^3}{9 k^3}$$

> **elimsolve** (tmp1,r1);

$$\{54 k^3 \neq 0\}$$

r1 is set to:

$$-\frac{l^3 (6 a l^3 e_3 + 12 l^3 c_2 e_3 k - l^3 b_3 f_3 + 4 c_3 l^3 e_3 - 9 k^3 f_3 c_2)}{54 k^3}$$

> **tmp1** := **cpcoeff** (x1^4\*x2^2);

$$tmp1 := (-27 l3 k3^3 c3^2 - 27 a1 l3^2 b3 k3^2 + 72 e3 c3 l3 k3^2 f3 - 24 e3 l3^2 b3 f3 k3 - 27 l3 k3^3 c2 b3 + 18 f3^2 k3^2 b3 l3 + 243 a1 c2 k3^4 + 8 l3^3 b3 e3^2 - 54 f3^2 k3^3 c3 - 81 i1 k3^4 + 81 a1 l3 c3 k3^3 - 24 c3 l3^2 k3 e3^2) / (27 k3^3)$$

> **elimsolve (tmp1,i1);**

$$\{-81 k3^4 \neq 0\}$$

i1 is set to:

$$(-27 l3 k3^3 c3^2 - 27 a1 l3^2 b3 k3^2 + 72 e3 c3 l3 k3^2 f3 - 24 e3 l3^2 b3 f3 k3 - 27 l3 k3^3 c2 b3 + 18 f3^2 k3^2 b3 l3 + 243 a1 c2 k3^4 + 8 l3^3 b3 e3^2 - 54 f3^2 k3^3 c3 + 81 a1 l3 c3 k3^3 - 24 c3 l3^2 k3 e3^2) / (81 k3^4)$$

> **tmp1 := cpcoeff (x1^2\*x2^2\*T);**

tmp1 :=

$$- \frac{27 k3^2 l3 a1 + 18 c3 l3 k3^2 + 9 f3^2 k3^2 + 27 k3^3 c2 - 12 l3 e3 f3 k3 + 4 l3^2 e3^2 - 3 l3^2 b3 k3}{9 k3^2}$$

> **elimsolve (tmp1,c2);**

$$\{27 k3^3 \neq 0\}$$

c2 is set to:

$$- \frac{27 k3^2 l3 a1 + 18 c3 l3 k3^2 + 9 f3^2 k3^2 - 12 l3 e3 f3 k3 + 4 l3^2 e3^2 - 3 l3^2 b3 k3}{27 k3^3}$$

> **tmp1 := cpcoeff (x1^3\*x2^3);**

$$tmp1 := \frac{(2 l3 e3 - 3 f3 k3)^3}{27 k3^3}$$

> **elimsolve (tmp1,f3);**

$$\{-3 k3 \neq 0\}$$

f3 is set to:

$$\frac{2 l3 e3}{3 k3}$$

> **tmp1 := cpcoeff (x1\*x2^2\*T);**

$$tmp1 := -(-3 l3^2 g3 k3 + 12 l3 e3 o3 k3 + 18 l3 k3^2 d1 + 18 l3 i3 k3^2 + 27 i2 k3^3 - 36 e3 r3 k3^2 - 4 l3^2 e3 m3) / (9 k3^2)$$

> **elimsolve (tmp1,i2);**

$$\{27 k3^3 \neq 0\}$$

i2 is set to:

$$- \frac{-3 l3^2 g3 k3 + 12 l3 e3 o3 k3 + 18 l3 k3^2 d1 + 18 l3 i3 k3^2 - 36 e3 r3 k3^2 - 4 l3^2 e3 m3}{27 k3^3}$$

> **tmp1 := cpcoeff (x2^2\*x3\*T);**

$$tmp1 := (-162 r2 k3^4 - 27 l3^2 o3 k3^2 - 9 l3^3 a1 b3 k3 - 6 l3^3 b3 c3 k3 + l3^4 b3^2 + 27 l3^2 a1 c3 k3^2 + 9 l3^2 k3^2 c3^2 + 81 l3^2 k3^2 a1^2 + 12 l3^3 m3 k3) / (27 k3^3)$$

> **elimsolve (tmp1,r2);**

$$\{-162 k3^4 \neq 0\}$$

r2 is set to:

$$l3^2 (-27 o3 k3^2 - 9 a1 l3 b3 k3 - 6 b3 l3 c3 k3 + b3^2 l3^2 + 27 a1 c3 k3^2 + 9 k3^2 c3^2 + 81 k3^2 a1^2 + 12 l3 m3 k3) / (162 k3^4)$$

> **tmp1 := cpcoeff (x2^3\*T);**

$$tmp1 := \frac{2 (l3^2 m3 - 3 l3 o3 k3 + 9 r3 k3^2)}{3 k3}$$

> **elimsolve (tmp1,r3);**

$$\{9 k3^2 \neq 0\}$$

r3 is set to:

$$\frac{l3 (-l3 m3 + 3 k3 o3)}{9 k3^2}$$

> **tmp1 := cpcoeff (x1^6);**

$$tmp1 := \frac{(b3 l3 - 3 k3 c3)^3}{27 k3^3}$$

> **elimsolve (tmp1,c3);**

$$\{-3 k3 \neq 0\}$$

c3 is set to:

$$\frac{b3 l3}{3 k3}$$

> **tmp1 := cpcoeff (x1^3\*x2^2);**

$$tmp1 := \frac{a1 l3^2 g3 - 12 a1 l3 k3 d1 - 3 a1 l3 i3 k3 + 9 a1^2 l3^2 a3 + 27 a1^2 l3 k3 a2 - 3 s1 k3^2}{k3}$$

> **elimsolve (tmp1,s1);**

$$\{-3 k3^2 \neq 0\}$$

s1 is set to:

$$\frac{a1 l3 (9 a3 l3 a1 - 12 k3 d1 - 3 i3 k3 + 27 a2 a1 k3 + l3 g3)}{3 k3^2}$$

> **tmp1 := cpcoeff (x2^2\*T);**

$$tmp1 := -(-81 a1^2 k3^2 o3 + 729 k3^2 a1^4 - 3 l3^2 p3 k3 + 27 s2 k3^3 + 4 l3^2 m3^2 - 12 l3 m3 k3 o3 + 54 l3 m3 k3 a1^2 + 9 k3^2 l3 j1 + 18 l3 s3 k3^2 + 9 o3^2 k3^2) / (9 k3^2)$$

> **elimsolve (tmp1,s2);**

$$\{27 k3^3 \neq 0\}$$

s2 is set to:

$$-(-81 a1^2 k3^2 o3 + 729 k3^2 a1^4 - 3 l3^2 p3 k3 + 4 l3^2 m3^2 - 12 l3 m3 k3 o3 + 54 l3 m3 k3 a1^2 + 9 k3^2 l3 j1 + 18 l3 s3 k3^2 + 9 o3^2 k3^2) / (27 k3^3)$$

> **tmp1 := cpcoeff (x2^3);**

$$tmp1 := 729 a1^6$$

> **elimsolve (tmp1,a1);**

$$\{1 \neq 0\}$$

a1 is set to:

$$0$$

> **launchNZcase (3\*o3\*k3-2\*l3\*m3);**

Launching case level 2:

$$3 k3 o3 - 2 l3 m3 \neq 0$$

Assume from now on that:

$$6 k3 (3 k3 o3 - 2 l3 m3) \neq 0$$

> **tmp1 := cpcoeff (x1\*x2\*T);**

$$tmp1 := -\frac{2 (3 k3 o3 - 2 l3 m3) (9 i3 k3^2 + 9 k3^2 d1 - 3 e3 o3 k3 - 3 l3 g3 k3 + 2 l3 e3 m3)}{27 k3^3}$$

> **elimsolve (tmp1,i3);**

$$\{9 k3^2 \neq 0\}$$

i3 is set to:

$$-\frac{9 k3^2 d1 - 3 e3 o3 k3 - 3 l3 g3 k3 + 2 l3 e3 m3}{9 k3^2}$$

> **tmp1 := cpcoeff (x2\*T);**

$$tmp1 := -\frac{(3 k3 o3 - 2 l3 m3) (9 k3^2 j1 + 18 k3^2 s3 - 6 k3 o3 m3 - 6 l3 p3 k3 + 4 l3 m3^2)}{27 k3^3}$$

> **elimsolve (tmp1,s3);**

$$\{18 k3^2 \neq 0\}$$

s3 is set to:

$$-\frac{9 k3^2 j1 - 6 k3 o3 m3 - 6 l3 p3 k3 + 4 l3 m3^2}{18 k3^2}$$

> **tmp1 := cpcoeff (x3\*T);**

$$tmp1 := \frac{(3 k3 o3 - 2 l3 m3)^3}{81 k3^4}$$

> **contradict (tmp1,o3);**

Contradiction on case level 2, so:

$$3 k3 o3 - 2 l3 m3 = 0$$

Variables to be uneliminated:

$$s3 := 's3'$$

$$i3 := 'i3'$$

Proceed on case level 1 with:

$$6 k3 \neq 0$$

On account of:

$$3 k3 o3 - 2 l3 m3 = 0$$

$$\{3 k3 \neq 0\}$$

o3 is set to:

$$\frac{2 l3 m3}{3 k3}$$

> **launchNZcase (6\*k3\*j1+3\*k3\*s3-l3\*p3);**

Launching case level 2:

$$6 k3 j1 + 3 k3 s3 - l3 p3 \neq 0$$

Assume from now on that:

$$6 k3 (6 k3 j1 + 3 k3 s3 - l3 p3) \neq 0$$

> **tmp1 := cpcoeff (x1\*T);**

$$tmp1 := -(9 j1 i3 k3^2 + 2 l3^2 p3 g3 - 6 l3 p3 k3 d1 - 6 l3 p3 i3 k3 - 3 l3 g3 k3 j1 - 6 l3 g3 k3 s3 + 18 i3 k3^2 s3 + 18 d1 s3 k3^2 + 36 k3^2 d1 j1) / (9 k3^2)$$

> **elimsolve** (tmp1,d1);

$$\{-6 l3 p3 k3 + 18 k3^2 s3 + 36 k3^2 j1 \neq 0\}$$

d1 is set to:

$$\frac{(-3 i3 k3 + l3 g3)(6 k3 s3 - 2 l3 p3 + 3 k3 j1)}{6 k3 (6 k3 j1 + 3 k3 s3 - l3 p3)}$$

> **launchNZcase** (3\*k3\*s3+3\*k3\*j1-l3\*p3);

Launching case level 3:

$$3 k3 s3 + 3 k3 j1 - l3 p3 \neq 0$$

Assume from now on that:

$$6 k3 (6 k3 j1 + 3 k3 s3 - l3 p3) (3 k3 s3 + 3 k3 j1 - l3 p3) \neq 0$$

> **launchNZcase** (j1);

Launching case level 4:

$$j1 \neq 0$$

Assume from now on that:

$$6 k3 (6 k3 j1 + 3 k3 s3 - l3 p3) (3 k3 s3 + 3 k3 j1 - l3 p3) j1 \neq 0$$

> **tmp1** := **cpcoeff** (1);

$$tmp1 := \frac{(3 k3 s3 - l3 p3) (3 k3 s3 + 3 k3 j1 - l3 p3) j1}{9 k3^2}$$

> **elimsolve** (tmp1,s3);

$$\{3 k3 \neq 0\}$$

s3 is set to:

$$\frac{l3 p3}{3 k3}$$

Nonzero constraint refines to:

$$108 k3^3 j1^3 \neq 0$$

> **tmp1** := **cpcoeff** (T);

$$tmp1 := -j1^2$$

> **contradict** (tmp1,'j1');

Contradiction on case level 4, so:

$$j1 = 0$$

Variables to be uneliminated:

$$s3 := 's3'$$

Proceed on case level 3 with:

$$6 k3 (6 k3 j1 + 3 k3 s3 - l3 p3) (3 k3 s3 + 3 k3 j1 - l3 p3) \neq 0$$

On account of:

$$j1 = 0$$

$$\{1 \neq 0\}$$

j1 is set to:

$$0$$

Nonzero constraint refines to:

$$6 k3 (3 k3 s3 - l3 p3)^2 \neq 0$$

> **tmp1** := **cpcoeff** (T);

$$tmp1 := -\frac{(3\ k3\ s3 - l3\ p3)^2}{9\ k3^2}$$

> **contradict (tmp1,'s3');**

Contradiction on case level 3, so:

$$3\ k3\ s3 + 3\ k3\ j1 - l3\ p3 = 0$$

Variables to be uneliminated:

$$j1 := j1$$

Proceed on case level 2 with:

$$6\ k3\ (6\ k3\ j1 + 3\ k3\ s3 - l3\ p3) \neq 0$$

On account of:

$$3\ k3\ s3 + 3\ k3\ j1 - l3\ p3 = 0$$

$$\{3\ k3 \neq 0\}$$

s3 is set to:

$$-\frac{3\ k3\ j1 - l3\ p3}{3\ k3}$$

Nonzero constraint refines to:

$$18\ k3^2\ j1 \neq 0$$

> **tmp1 := cpcoeff (T);**

$$tmp1 := -j1^2$$

> **contradict (tmp1,'s3');**

Contradiction on case level 2, so:

$$6\ k3\ j1 + 3\ k3\ s3 - l3\ p3 = 0$$

Variables to be uneliminated:

$$s3 := s3$$

$$d1 := d1$$

Proceed on case level 1 with:

$$6\ k3 \neq 0$$

On account of:

$$6\ k3\ j1 + 3\ k3\ s3 - l3\ p3 = 0$$

$$\{3\ k3 \neq 0\}$$

s3 is set to:

$$-\frac{6\ k3\ j1 - l3\ p3}{3\ k3}$$

> **tmp1 := cpcoeff (T);**

$$tmp1 := -3\ j1^2$$

> **elimsolve (tmp1,j1);**

$$\{1 \neq 0\}$$

j1 is set to:

$$0$$

> **launchNZcase (d1);**

Launching case level 2:

$$d1 \neq 0$$

Assume from now on that:

$$6\ k3\ d1 \neq 0$$

> **launchNZcase (l3\*g3-3\*i3\*k3);**

Launching case level 3:

$$-3 \, i3 \, k3 + l3 \, g3 \neq 0$$

Assume from now on that:

$$6 \, k3 \, d1 \, (-3 \, i3 \, k3 + l3 \, g3) \neq 0$$

> **tmp1 := cpcoeff (x1^3);**

$$tmp1 := -\frac{2 \, d1 \, (-3 \, i3 \, k3 + l3 \, g3) \, (-l3 \, g3 + 6 \, k3 \, d1 + 3 \, i3 \, k3)}{9 \, k3^2}$$

> **elimsolve (tmp1,i3);**

$$\{3 \, k3 \neq 0\}$$

i3 is set to:

$$-\frac{-l3 \, g3 + 6 \, k3 \, d1}{3 \, k3}$$

Nonzero constraint refines to:

$$36 \, k3^2 \, d1^2 \neq 0$$

> **tmp1 := cpcoeff (x1^2\*T);**

$$tmp1 := -4 \, d1^2$$

> **contradict (tmp1,'i3');**

Contradiction on case level 3, so:

$$-3 \, i3 \, k3 + l3 \, g3 = 0$$

Variables to be uneliminated:

$$"i3 := 'i3'"$$

Proceed on case level 2 with:

$$6 \, k3 \, d1 \neq 0$$

On account of:

$$\begin{aligned} -3 \, i3 \, k3 + l3 \, g3 &= 0 \\ \{-3 \, k3 \neq 0\} \end{aligned}$$

i3 is set to:

$$\frac{l3 \, g3}{3 \, k3}$$

> **tmp1 := cpcoeff (x1^2\*T);**

$$tmp1 := -4 \, d1^2$$

> **contradict (tmp1,'d1');**

Contradiction on case level 2, so:

$$d1 = 0$$

Variables to be uneliminated:

$$"i3 := 'i3'"$$

Proceed on case level 1 with:

$$6 \, k3 \neq 0$$

On account of:

$$\begin{aligned} d1 &= 0 \\ \{1 \neq 0\} \end{aligned}$$

d1 is set to:

$$0$$

> **tmp1 := cpcoeff (x1^2\*T);**

$$tmp1 := - \frac{(-3 i3 k3 + l3 g3)^2}{9 k3^2}$$

> **elimsolve (tmp1,i3);**

$$\{-3 k3 \neq 0\}$$

i3 is set to:

$$\frac{l3 g3}{3 k3}$$

> **det(T-jacobian(H,[x1,x2,x3]));**

$$T^3$$

> **H;**

$$\left[ 0, \frac{x1^4}{4} + a2 x1^3 - \frac{b3 l3 x1^2 x2}{3 k3} - \frac{l3^2 b3 x1^2 x3}{9 k3^2} + d2 x1^2 - \frac{l3 e3 x1 x2^2}{3 k3} - \frac{2 l3^2 e3 x1 x2 x3}{9 k3^2} - \frac{l3 g3 x1 x2}{3 k3} - \frac{l3^3 e3 x1 x3^2}{27 k3^3} - \frac{l3^2 g3 x1 x3}{9 k3^2} + j2 x1 - \frac{l3 x2^3}{3} - \frac{l3^2 x2^2 x3}{3 k3} - \frac{l3 m3 x2^2}{3 k3} - \frac{l3^3 x2 x3^2}{9 k3^2} - \frac{2 l3^2 m3 x2 x3}{9 k3^2} - \frac{l3 p3 x2}{3 k3} - \frac{l3^4 x3^3}{81 k3^3} - \frac{l3^3 m3 x3^2}{27 k3^3} - \frac{l3^2 p3 x3}{9 k3^2}, a3 x1^3 + b3 x1^2 x2 + \frac{b3 l3 x1^2 x3}{3 k3} + d3 x1^2 + e3 x1 x2^2 + \frac{2 l3 e3 x1 x2 x3}{3 k3} + g3 x1 x2 + \frac{l3^2 e3 x1 x3^2}{9 k3^2} + \frac{l3 g3 x1 x3}{3 k3} + j3 x1 + k3 x2^3 + l3 x2^2 x3 + m3 x2^2 + \frac{l3^2 x2 x3^2}{3 k3} + \frac{2 l3 m3 x2 x3}{3 k3} + p3 x2 + \frac{l3^3 x3^3}{27 k3^2} + \frac{l3^2 m3 x3^2}{9 k3^2} + \frac{l3 p3 x3}{3 k3} \right]$$

> **M:=evalm([ [1,0,0], [0,1,-l3/3/k3], [0,0,1] ] );**

$$M := \begin{bmatrix} 1 & 0 & 0 \\ 0 & 1 & -\frac{l3}{3 k3} \\ 0 & 0 & 1 \end{bmatrix}$$

> **evalm(simplify(jacobian(evalm(M^(-1)&\***

**subs({seq([x1,x2,x3][i]=evalm(M&\*[x1,x2,x3])[i],i=1..3)},H)),**

**[x1,x2,x3])));**

[0,0,0]

$$\left[ \frac{3 x1^3 k3 + 9 a2 x1^2 k3 + 6 d2 x1 k3 + 3 j2 k3 + 3 l3 a3 x1^2 + 2 l3 d3 x1 + l3 j3}{3 k3}, 0, 0 \right]$$

$$[3 a3 x1^2 + 2 b3 x1 x2 + 2 d3 x1 + e3 x2^2 + g3 x2 + j3,$$

$$b3 x1^2 + 2 e3 x1 x2 + g3 x1 + 3 k3 x2^2 + 2 m3 x2 + p3, 0]$$

> **contradict (1,'k3');**

Contradiction on case level 1, so:

$$k3 = 0$$

Variables to be uneliminated:

$$"i3 := 'i3'"$$

```

"d1 := 'd1'"
"j1 := 'j1'"
"s3 := 's3'"
"o3 := 'o3'"
"a1 := 'a1'"
"s2 := 's2'"
"s1 := 's1'"
"c3 := 'c3'"
"r3 := 'r3'"
"r2 := 'r2'"
"i2 := 'i2'"
"f3 := 'f3'"
"c2 := 'c2'"
"i1 := 'i1'"
"r1 := 'r1'"
"h3 := 'h3'"
"h2 := 'h2'"
"q2 := 'q2'"
"q3 := 'q3'"
"n3 := 'n3'"
"c1 := 'c1'"
"h1 := 'h1'"
"q1 := 'q1'"
"u2 := 'u2'"
"v2 := 'v2'"
"w2 := 'w2'"

```

Proceed on case level 0 with:

$$6 \neq 0$$

On account of:

$$k3 = 0$$

$$\{1 \neq 0\}$$

k3 is set to:

$$0$$

```
> launchNZcase (e3);
```

Launching case level 1:

$$e3 \neq 0$$

Assume from now on that:

$$6 e3 \neq 0$$

```
> tmp1 := cpcoeff (x1^4*x2^3);
```

$$tmp1 := 4 u2 e3^2$$

```
> elimsolve (tmp1,u2);
```

|                                     |                      |
|-------------------------------------|----------------------|
|                                     | $\{1 \neq 0\}$       |
| u2 is set to:                       | 0                    |
| > tmp1 := cpcoeff (x1^6*x2);        |                      |
|                                     | $tmp1 := -2\ c1\ e3$ |
| > elimsolve (tmp1,c1);              |                      |
|                                     | $\{1 \neq 0\}$       |
| c1 is set to:                       | 0                    |
| > tmp1 := cpcoeff (x2^4*T);         |                      |
|                                     | $tmp1 := -l3^2$      |
| > elimsolve (tmp1,l3);              |                      |
|                                     | $\{1 \neq 0\}$       |
| l3 is set to:                       | 0                    |
| > tmp1 := cpcoeff (x1*x2*x3^3*T);   |                      |
|                                     | $tmp1 := -8\ w2\ e3$ |
| > elimsolve (tmp1,w2);              |                      |
|                                     | $\{1 \neq 0\}$       |
| w2 is set to:                       | 0                    |
| > tmp1 := cpcoeff (x1*x2^3*T);      |                      |
|                                     | $tmp1 := 2\ n3\ e3$  |
| > elimsolve (tmp1,n3);              |                      |
|                                     | $\{1 \neq 0\}$       |
| n3 is set to:                       | 0                    |
| > tmp1 := cpcoeff (x1^2*x2*x3^2*T); |                      |
|                                     | $tmp1 := -6\ v2\ e3$ |
| > elimsolve (tmp1,v2);              |                      |
|                                     | $\{1 \neq 0\}$       |
| v2 is set to:                       | 0                    |
| > tmp1 := cpcoeff (x1^4*x2*x3^2);   |                      |
|                                     | $tmp1 := -6\ q1\ e3$ |
| > elimsolve (tmp1,q1);              |                      |
|                                     | $\{1 \neq 0\}$       |
| q1 is set to:                       | 0                    |
| > tmp1 := cpcoeff (x1^5*x2*x3);     |                      |
|                                     | $tmp1 := -4\ e3\ h1$ |
| > elimsolve (tmp1,h1);              |                      |
|                                     | $\{1 \neq 0\}$       |
| h1 is set to:                       |                      |

[illegible]

```

|                                     
$$\frac{b_3 f_3}{2 e^3}$$

|
| > tmp1 := cpcoeff (x2^2*x3*T);
|
|                                     
$$tmp1 := -\frac{f_3^4 b_3 + 6 f_3^3 a_1 e_3 + 4 f_3^2 c_2 e_3^2 + 16 r_1 e_3^3}{8 e_3^2}$$

|
| > elimsolve (tmp1,r1);
|
|                                     
$$\{16 e_3^3 \neq 0\}$$

| r1 is set to:
|                                     
$$-\frac{f_3^2 (b_3 f_3^2 + 6 a_1 f_3 e_3 + 4 c_2 e_3^2)}{16 e_3^3}$$

|
| > tmp1 := cpcoeff (x1^2*x2^3);
|
|                                     
$$tmp1 := \frac{(b_3 f_3^2 + 6 a_1 f_3 e_3 + 4 c_2 e_3^2)^2}{8 e_3^2}$$

|
| > elimsolve (tmp1,c2);
|
|                                     
$$\{4 e_3^2 \neq 0\}$$

| c2 is set to:
|                                     
$$-\frac{(6 a_1 e_3 + b_3 f_3) f_3}{4 e_3^2}$$

|
| > tmp1 := cpcoeff (x1*x2^2*T);
|
|                                     
$$tmp1 := \frac{-2 f_3 o_3 e_3 + 4 r_3 e_3^2 + f_3^2 m_3}{e_3}$$

|
| > elimsolve (tmp1,r3);
|
|                                     
$$\{4 e_3^2 \neq 0\}$$

| r3 is set to:
|                                     
$$\frac{f_3 (2 e_3 o_3 - f_3 m_3)}{4 e_3^2}$$

|
| > tmp1 := cpcoeff (x1*x2*x3*T);
|
|                                     
$$tmp1 := \frac{-3 f_3^2 e_3 o_3 + 2 f_3^3 m_3 - 8 r_2 e_3^3 + 9 e_3 f_3^2 a_1^2}{2 e_3^2}$$

|
| > elimsolve (tmp1,r2);
|
|                                     
$$\{-8 e_3^3 \neq 0\}$$

| r2 is set to:
|                                     
$$\frac{f_3^2 (-3 e_3 o_3 + 2 f_3 m_3 + 9 e_3 a_1^2)}{8 e_3^3}$$

|
| > tmp1 := cpcoeff (x1^4*x2);
|
| 
$$tmp1 := (-4 f_3 i_2 b_3 e_3^2 + 54 a_3 a_1^2 f_3^2 e_3 - 4 d_1 b_3 f_3^2 e_3 - 4 b_3 f_3^2 i_3 e_3 - 24 f_3 a_1 d_1 e_3^2$$

| 
$$+ 24 a_1 i_2 e_3^3 + f_3^3 g_3 b_3 + 12 a_1 f_3 i_3 e_3^2 - 8 s_1 e_3^3 + 108 a_2 a_1^2 e_3^2 f_3) / (4 e_3^2)$$

|
| > elimsolve (tmp1,s1);
|
|                                     
$$\{-8 e_3^3 \neq 0\}$$

| s1 is set to:

```

$$\frac{(-4f_3 i_2 b_3 e_3^2 + 54 a_3 a l^2 f_3^2 e_3 - 4 d l b_3 f_3^2 e_3 - 4 b_3 f_3^2 i_3 e_3 - 24 f_3 a l d l e_3^2 + 24 a l i_2 e_3^3 + f_3^3 g_3 b_3 + 12 a l f_3 i_3 e_3^2 + 108 a_2 a l^2 e_3^2 f_3) / (8 e_3^3)}{}$$

> **tmp1 := cpcoeff (x1^2\*x2\*T);**

$$tmp1 := -\frac{6 a l o_3 e_3 + 4 i_2 e_3^2 - 6 a l f_3 m_3 + 4 f_3 e_3 d l + 4 f_3 i_3 e_3 - f_3^2 g_3}{2 e_3}$$

> **elimsolve (tmp1,i2);**

$$\{4 e_3^2 \neq 0\}$$

i2 is set to:

$$-\frac{6 a l o_3 e_3 - 6 a l f_3 m_3 + 4 f_3 e_3 d l + 4 f_3 i_3 e_3 - f_3^2 g_3}{4 e_3^2}$$

> **launchNZcase (a1);**

Launching case level 2:

$$a l \neq 0$$

Assume from now on that:

$$6 a l e_3 \neq 0$$

> **launchNZcase (-f3\*m3+e3\*o3);**

Launching case level 3:

$$-f_3 m_3 + e_3 o_3 \neq 0$$

Assume from now on that:

$$6 e_3 a l (-f_3 m_3 + e_3 o_3) \neq 0$$

> **tmp1 := cpcoeff (x1^2\*x2^2);**

$$tmp1 := -\frac{3 a l (-f_3 m_3 + e_3 o_3) (-e_3 o_3 + 9 e_3 a l^2 + f_3 m_3)}{e_3^2}$$

> **elimsolve (tmp1,o3);**

$$\{-e_3 \neq 0\}$$

o3 is set to:

$$\frac{9 e_3 a l^2 + f_3 m_3}{e_3}$$

Nonzero constraint refines to:

$$18 a l^2 e_3^2 \neq 0$$

> **tmp1 := cpcoeff (x2^2\*T);**

$$tmp1 := -\frac{81 a l^4}{2}$$

> **contradict (tmp1,'o3');**

Contradiction on case level 3, so:

$$-f_3 m_3 + e_3 o_3 = 0$$

Variables to be uneliminated:

$$"o_3 := 'o_3'"$$

Proceed on case level 2 with:

$$6 a l e_3 \neq 0$$

On account of:

$$-f_3 m_3 + e_3 o_3 = 0$$

$$\{e_3 \neq 0\}$$

o3 is set to:

$$\frac{f3\ m3}{e3}$$

> tmp1 := cpcoeff (x2^2\*T);

$$tmp1 := -81\ a1^4$$

> contradict (tmp1,'a1');

Contradiction on case level 2, so:

$$a1 = 0$$

Variables to be uneliminated:

$$"o3 := 'o3'"$$

Proceed on case level 1 with:

$$6\ e3 \neq 0$$

On account of:

$$a1 = 0$$

$$\{1 \neq 0\}$$

a1 is set to:

$$0$$

> tmp1 := cpcoeff (x2^2\*T);

$$tmp1 := -\frac{(-f3\ m3 + e3\ o3)^2}{e3^2}$$

> elimsolve (tmp1,o3);

$$\{e3 \neq 0\}$$

o3 is set to:

$$\frac{f3\ m3}{e3}$$

> tmp1 := cpcoeff (x1\*x2\*T);

$$tmp1 := -\frac{4\ f3\ s3\ e3 + 2\ f3\ e3\ j1 + 4\ s2\ e3^2 - f3^2\ p3}{2\ e3}$$

> elimsolve (tmp1,s2);

$$\{4\ e3^2 \neq 0\}$$

s2 is set to:

$$-\frac{f3\ (4\ s3\ e3 + 2\ e3\ j1 - f3\ p3)}{4\ e3^2}$$

> launchNZcase (j1);

Launching case level 2:

$$j1 \neq 0$$

Assume from now on that:

$$6\ e3\ j1 \neq 0$$

> launchNZcase (2\*e3\*s3-p3\*f3);

Launching case level 3:

$$2\ s3\ e3 - f3\ p3 \neq 0$$

Assume from now on that:

$$6\ e3\ j1\ (2\ s3\ e3 - f3\ p3) \neq 0$$

> tmp1 := cpcoeff (1);

$$tmp1 := \frac{j1 (2 s3 e3 - f3 p3) (2 s3 e3 + 2 e3 j1 - f3 p3)}{4 e3^2}$$

> **elimsolve** (tmp1,s3);

$$\{2 e3 \neq 0\}$$

s3 is set to:

$$-\frac{2 e3 j1 - f3 p3}{2 e3}$$

Nonzero constraint refines to:

$$-12 e3^2 j1^2 \neq 0$$

> **tmp1 := cpcoeff** (T);

$$tmp1 := -j1^2$$

> **contradict** (tmp1,'s3');

Contradiction on case level 3, so:

$$2 s3 e3 - f3 p3 = 0$$

Variables to be uneliminated:

$$s3 := s3$$

Proceed on case level 2 with:

$$6 e3 j1 \neq 0$$

On account of:

$$2 s3 e3 - f3 p3 = 0$$

$$\{2 e3 \neq 0\}$$

s3 is set to:

$$\frac{f3 p3}{2 e3}$$

> **tmp1 := cpcoeff** (T);

$$tmp1 := -j1^2$$

> **contradict** (tmp1,'j1');

Contradiction on case level 2, so:

$$j1 = 0$$

Variables to be uneliminated:

$$s3 := s3$$

Proceed on case level 1 with:

$$6 e3 \neq 0$$

On account of:

$$j1 = 0$$

$$\{1 \neq 0\}$$

j1 is set to:

$$0$$

> **tmp1 := cpcoeff** (T);

$$tmp1 := -\frac{(2 s3 e3 - f3 p3)^2}{4 e3^2}$$

> **elimsolve** (tmp1,s3);

$$\{2 e3 \neq 0\}$$

s3 is set to:

$$\frac{f_3 p_3}{2 e_3}$$

> **launchNZcase (d1);**

Launching case level 2:

$$d_1 \neq 0$$

Assume from now on that:

$$6 e_3 d_1 \neq 0$$

> **launchNZcase (2\*i3\*e3-f3\*g3);**

Launching case level 3:

$$2 i_3 e_3 - f_3 g_3 \neq 0$$

Assume from now on that:

$$6 e_3 d_1 (2 i_3 e_3 - f_3 g_3) \neq 0$$

> **tmp1 := cpcoeff (x1^3);**

$$tmp1 := \frac{d_1 (2 i_3 e_3 - f_3 g_3) (2 i_3 e_3 + 4 e_3 d_1 - f_3 g_3)}{2 e_3^2}$$

> **elimsolve (tmp1,i3);**

$$\{2 e_3 \neq 0\}$$

i3 is set to:

$$-\frac{4 e_3 d_1 - f_3 g_3}{2 e_3}$$

Nonzero constraint refines to:

$$-12 e_3^2 d_1^2 \neq 0$$

> **tmp1 := cpcoeff (x1^2\*T);**

$$tmp1 := -4 d_1^2$$

> **contradict (tmp1,'i3');**

Contradiction on case level 3, so:

$$2 i_3 e_3 - f_3 g_3 = 0$$

Variables to be uneliminated:

$$"i_3 := 'i_3'"$$

Proceed on case level 2 with:

$$6 e_3 d_1 \neq 0$$

On account of:

$$2 i_3 e_3 - f_3 g_3 = 0$$

$$\{2 e_3 \neq 0\}$$

i3 is set to:

$$\frac{f_3 g_3}{2 e_3}$$

> **tmp1 := cpcoeff (x1^2\*T);**

$$tmp1 := -4 d_1^2$$

> **contradict (tmp1,'d1');**

Contradiction on case level 2, so:

$$d_1 = 0$$

Variables to be uneliminated:

$$"i_3 := 'i_3'"$$

Proceed on case level 1 with:

$$6 e3 \neq 0$$

On account of:

$$d1 = 0$$

$$\{1 \neq 0\}$$

d1 is set to:

$$0$$

> **tmp1 := cpcoeff (x1^2\*T);**

$$tmp1 := -\frac{(2 i3 e3 - f3 g3)^2}{4 e3^2}$$

> **elimsolve (tmp1,i3);**

$$\{2 e3 \neq 0\}$$

i3 is set to:

$$\frac{f3 g3}{2 e3}$$

> **det (T-jacobian (H, [x1,x2,x3])) ;**

$$T^3$$

> **H;**

$$\left[ 0, \frac{x1^4}{4} + a2 x1^3 - \frac{b3 f3 x1^2 x2}{2 e3} - \frac{b3 f3^2 x1^2 x3}{4 e3^2} + d2 x1^2 - \frac{f3 x1 x2^2}{2} - \frac{f3^2 x1 x2 x3}{2 e3} - \frac{f3 g3 x1 x2}{2 e3} - \frac{f3^3 x1 x3^2}{8 e3^2} - \frac{f3^2 g3 x1 x3}{4 e3^2} + j2 x1 - \frac{f3 m3 x2^2}{2 e3} - \frac{f3^2 m3 x2 x3}{2 e3^2} - \frac{f3 p3 x2}{2 e3} - \frac{f3^3 m3 x3^2}{8 e3^3} - \frac{f3^2 p3 x3}{4 e3^2}, a3 x1^3 + b3 x1^2 x2 + \frac{b3 f3 x1^2 x3}{2 e3} + d3 x1^2 + e3 x1 x2^2 + f3 x1 x2 x3 + g3 x1 x2 + \frac{f3^2 x1 x3^2}{4 e3} + \frac{f3 g3 x1 x3}{2 e3} + j3 x1 + m3 x2^2 + \frac{f3 m3 x2 x3}{e3} + p3 x2 + \frac{f3^2 m3 x3^2}{4 e3^2} + \frac{f3 p3 x3}{2 e3} \right]$$

> **M:=evalm([ [1,0,0], [0,1,-f3/2/e3], [0,0,1]]);**

$$M := \begin{bmatrix} 1 & 0 & 0 \\ 0 & 1 & -\frac{f3}{2 e3} \\ 0 & 0 & 1 \end{bmatrix}$$

> **evalm(simplify(jacobian(evalm(M^(-1)&\***

> **subs({seq([x1,x2,x3][i]=evalm(M&\*[x1,x2,x3])[i],i=1..3)},H)),**

> **[x1,x2,x3])));**

[0,0,0]

$$\left[ \frac{2 x1^3 e3 + 6 a2 x1^2 e3 + 4 d2 x1 e3 + 2 j2 e3 + 3 f3 a3 x1^2 + 2 f3 d3 x1 + f3 j3}{2 e3}, 0, 0 \right]$$

$$[3 a3 x1^2 + 2 b3 x1 x2 + 2 d3 x1 + e3 x2^2 + g3 x2 + j3,$$

$$b3 x1^2 + 2 e3 x1 x2 + g3 x1 + 2 m3 x2 + p3, 0]$$

```
> contradict (1, 'e3');
```

Contradiction on case level 1, so:

$$e3 = 0$$

Variables to be uneliminated:

"i3 := 'i3'"

"d1 := 'd1'"

"s3 := 's3'"

"j1 := 'j1'"

"s2 := 's2'"

"o3 := 'o3'"

"a1 := 'a1'"

"i2 := 'i2'"

"s1 := 's1'"

"r2 := 'r2'"

"r3 := 'r3'"

"c2 := 'c2'"

"r1 := 'r1'"

"c3 := 'c3'"

"i1 := 'i1'"

"h3 := 'h3'"

"h2 := 'h2'"

"q2 := 'q2'"

"q3 := 'q3'"

"h1 := 'h1'"

"q1 := 'q1'"

"v2 := 'v2'"

"n3 := 'n3'"

"w2 := 'w2'"

"l3 := 'l3'"

"c1 := 'c1'"

"u2 := 'u2'"

Proceed on case level 0 with:

$$6 \neq 0$$

On account of:

$$e3 = 0$$

$$\{1 \neq 0\}$$

e3 is set to:

$$0$$

```
> tmp1 := cpcoeff (x2^4*T);
```

$$tmp1 := -l3^2$$

```
> elimsolve (tmp1, l3);
```

|                                         |                       |
|-----------------------------------------|-----------------------|
|                                         | $\{1 \neq 0\}$        |
| l3 is set to:                           |                       |
|                                         | 0                     |
| > <b>launchNZcase (b3);</b>             |                       |
| Launching case level 1:                 |                       |
|                                         | $b3 \neq 0$           |
| Assume from now on that:                |                       |
|                                         | $6\ b3 \neq 0$        |
| > <b>tmp1 := cpcoeff (x1^7);</b>        |                       |
|                                         | $tmp1 := -b3\ c1$     |
| > <b>elimsolve (tmp1,c1);</b>           |                       |
|                                         | $\{1 \neq 0\}$        |
| c1 is set to:                           |                       |
|                                         | 0                     |
| > <b>tmp1 := cpcoeff (x1^6*x2);</b>     |                       |
|                                         | $tmp1 := 2\ b3^2\ u2$ |
| > <b>elimsolve (tmp1,u2);</b>           |                       |
|                                         | $\{1 \neq 0\}$        |
| u2 is set to:                           |                       |
|                                         | 0                     |
| > <b>tmp1 := cpcoeff (x1^6*x3);</b>     |                       |
|                                         | $tmp1 := -2\ b3\ h1$  |
| > <b>elimsolve (tmp1,h1);</b>           |                       |
|                                         | $\{1 \neq 0\}$        |
| h1 is set to:                           |                       |
|                                         | 0                     |
| > <b>tmp1 := cpcoeff (x1^5*x2*x3);</b>  |                       |
|                                         | $tmp1 := 6\ b3^2\ v2$ |
| > <b>elimsolve (tmp1,v2);</b>           |                       |
|                                         | $\{1 \neq 0\}$        |
| v2 is set to:                           |                       |
|                                         | 0                     |
| > <b>tmp1 := cpcoeff (x1^2*x3^3*T);</b> |                       |
|                                         | $tmp1 := -4\ w2\ b3$  |
| > <b>elimsolve (tmp1,w2);</b>           |                       |
|                                         | $\{1 \neq 0\}$        |
| w2 is set to:                           |                       |
|                                         | 0                     |
| > <b>tmp1 := cpcoeff (x2^2*x3^2*T);</b> |                       |
|                                         | $tmp1 := -3\ n3^2$    |
| > <b>elimsolve (tmp1,n3);</b>           |                       |
|                                         | $\{1 \neq 0\}$        |
| n3 is set to:                           |                       |
|                                         | 0                     |

```
> tmp1 := cpcoeff (x1^2*x2^2*T);  
tmp1 := -f3^2  
> elimsolve (tmp1,f3);  
{1 ≠ 0}  
f3 is set to:  
0  
> tmp1 := cpcoeff (x1^5*x3^2);  
tmp1 := -3 b3 q1  
> elimsolve (tmp1,q1);  
{1 ≠ 0}  
q1 is set to:  
0  
> tmp1 := cpcoeff (x3^4*T);  
tmp1 := -9 q3^2  
> elimsolve (tmp1,q3);  
{1 ≠ 0}  
q3 is set to:  
0  
> tmp1 := cpcoeff (x2^2*x3*T);  
tmp1 := 4 h3^2 b3  
> elimsolve (tmp1,h3);  
{1 ≠ 0}  
h3 is set to:  
0  
> tmp1 := cpcoeff (x1^5*x2);  
tmp1 := 2 b3^2 h2  
> elimsolve (tmp1,h2);  
{1 ≠ 0}  
h2 is set to:  
0  
> tmp1 := cpcoeff (x1^5*x3);  
tmp1 := -2 b3 r1  
> elimsolve (tmp1,r1);  
{1 ≠ 0}  
r1 is set to:  
0  
> tmp1 := cpcoeff (x1^2*x3^2*T);  
tmp1 := -3 q2 b3  
> elimsolve (tmp1,q2);  
{1 ≠ 0}  
q2 is set to:  
0  
> tmp1 := cpcoeff (x1^6);
```

```

[
    tmp1 := 3 a1 c2 b3 - i1 b3 - c3 c2 b3 - c3^3
> elimsolve (tmp1,i1);
                                     {-b3 ≠ 0}
i1 is set to:
                                     
$$\frac{3 a1 c2 b3 - c3 c2 b3 - c3^3}{b3}$$

> tmp1 := cpcoeff (x1^5);
tmp1 := -(9 a2 b3^2 a1 c2 - 3 a2 b3^2 c3 c2 - 9 a3 c3^2 c2 b3 + c3 i2 b3^2 - 9 a3 c3^3 a1
- 3 a3 c2^2 b3^2 + i3 b3^2 c2 + s1 b3^2 - g3 c3^3 - 6 a3 c3^4 - 3 a1 i2 b3^2 - 2 d1 c2 b3^2
- 3 a2 b3 c3^3 + 3 c3^2 i3 b3) / b3
> elimsolve (tmp1,s1);
                                     {b3^2 ≠ 0}
s1 is set to:
-(9 a2 b3^2 a1 c2 - 3 a2 b3^2 c3 c2 - 9 a3 c3^2 c2 b3 + c3 i2 b3^2 - 9 a3 c3^3 a1 - 3 a3 c2^2 b3^2
+ i3 b3^2 c2 - g3 c3^3 - 6 a3 c3^4 - 3 a1 i2 b3^2 - 2 d1 c2 b3^2 - 3 a2 b3 c3^3 + 3 c3^2 i3 b3) / b3^2
> tmp1 := cpcoeff (x1^2*x3*T);
tmp1 := (-6 a1 r3 b3 + 3 a1 c2 b3 c3 + 6 c3^3 a1 + 5 c3^2 c2 b3 + 3 c3^4 + 2 c2^2 b3^2 - 2 r2 b3^2
- 4 r3 b3 c3 - c2 o3 b3) / b3
> elimsolve (tmp1,r2);
                                     {-2 b3^2 ≠ 0}
r2 is set to:
(-6 a1 r3 b3 + 3 a1 c2 b3 c3 + 6 c3^3 a1 + 5 c3^2 c2 b3 + 3 c3^4 + 2 c2^2 b3^2 - 4 r3 b3 c3
- c2 o3 b3) / (2 b3^2)
> tmp1 := cpcoeff (x1^2*x2*T);
tmp1 := -2 o3 c3 - 3 a1 o3 - 2 c2 m3 - 9 a1^2 c3 - 3 a1 c3^2 - 3 a1 c2 b3 + 2 r3 b3
> elimsolve (tmp1,r3);
                                     {-2 b3 ≠ 0}
r3 is set to:
                                     
$$\frac{2 o3 c3 + 3 a1 o3 + 2 c2 m3 + 9 a1^2 c3 + 3 a1 c3^2 + 3 a1 c2 b3}{2 b3}$$

> launchNZcase (-3*a1*c3-c3^2-c2*b3-9*a1^2);
Launching case level 2:
                                     -c2 b3 - 3 a1 c3 - c3^2 - 9 a1^2 ≠ 0
Assume from now on that:
                                     6 b3 (-c2 b3 - 3 a1 c3 - c3^2 - 9 a1^2) ≠ 0
> tmp1 := cpcoeff (x1^4*x2);
tmp1 := -(-2 c2 b3^2 c3^2 + 9 c2 b3^2 a1^2 + 9 a1^2 b3 o3 + 27 a1^3 b3 c3 - 6 a1 b3 c3^3 + o3 b3^2 c2
+ o3 b3 c3^2 + 6 a1 c2 m3 b3 - 6 c2 b3^2 a1 c3 + 3 a1 b3 o3 c3 - 2 m3 c3 c2 b3 - c2^2 b3^3
- c3^4 b3 - 2 m3 c3^3) / b3
> elimsolve (tmp1,o3);
                                     {9 a1^2 b3 + c2 b3^2 + c3^2 b3 + 3 a1 c3 b3 ≠ 0}

```

o3 is set to:

$$-(-2 c2 b3^2 c3^2 + 9 c2 b3^2 a1^2 + 27 a1^3 b3 c3 - 6 a1 b3 c3^3 + 6 a1 c2 m3 b3 - 6 c2 b3^2 a1 c3 - 2 m3 c3 c2 b3 - c2^2 b3^3 - c3^4 b3 - 2 m3 c3^3) / (b3 (c2 b3 + 3 a1 c3 + c3^2 + 9 a1^2))$$

> **launchNZcase (3\*a1\*b3+m3);**

Launching case level 3:

$$3 a1 b3 + m3 \neq 0$$

Assume from now on that:

$$6 b3 (-c2 b3 - 3 a1 c3 - c3^2 - 9 a1^2) (3 a1 b3 + m3) \neq 0$$

> **tmp1 := cpcoeff (x1^4\*x3);**

$$tmp1 := -\frac{2 (3 a1 c3 + c3^2 + c2 b3)^3 (3 a1 b3 + m3)}{b3^2 (c2 b3 + 3 a1 c3 + c3^2 + 9 a1^2)}$$

> **elimsolve (tmp1,c2);**

$$\{b3 \neq 0\}$$

c2 is set to:

$$-\frac{c3 (3 a1 + c3)}{b3}$$

Nonzero constraint refines to:

$$-18 b3 a1 (3 a1 b3 + m3) \neq 0$$

> **tmp1 := cpcoeff (x2^2\*T);**

$$tmp1 := -81 a1^4$$

> **contradict (tmp1,'m3');**

Contradiction on case level 3, so:

$$3 a1 b3 + m3 = 0$$

Variables to be uneliminated:

$$"c2 := 'c2'"$$

Proceed on case level 2 with:

$$6 b3 (-c2 b3 - 3 a1 c3 - c3^2 - 9 a1^2) \neq 0$$

On account of:

$$3 a1 b3 + m3 = 0$$

$$\{1 \neq 0\}$$

m3 is set to:

$$-3 a1 b3$$

> **launchNZcase (a1);**

Launching case level 3:

$$a1 \neq 0$$

Assume from now on that:

$$6 b3 (-c2 b3 - 3 a1 c3 - c3^2 - 9 a1^2) a1 \neq 0$$

> **tmp1 := cpcoeff (x2^3);**

$$tmp1 := -9 (c2 b3 + 3 a1 c3 + c3^2 + 9 a1^2) (3 a1 c3 + c3^2 + c2 b3) a1^2$$

> **elimsolve (tmp1,c2);**

$$\{b3 \neq 0\}$$

c2 is set to:

$$-\frac{c3 (3 a1 + c3)}{b3}$$

Nonzero constraint refines to:

$$-18 b3 a1^2 \neq 0$$

> **tmp1 := cpcoeff (x2^2\*T);**

$$tmp1 := -81 a1^4$$

> **contradict (tmp1,'a1');**

Contradiction on case level 3, so:

$$a1 = 0$$

Variables to be uneliminated:

$$c2 := c2$$

Proceed on case level 2 with:

$$6 b3 (-c2 b3 - 3 a1 c3 - c3^2 - 9 a1^2) \neq 0$$

On account of:

$$a1 = 0$$

$$\{1 \neq 0\}$$

a1 is set to:

$$0$$

Nonzero constraint refines to:

$$6 b3 (-c3^2 - c2 b3) \neq 0$$

> **tmp1 := cpcoeff (x2^2\*T);**

$$tmp1 := -(c3^2 + c2 b3)^2$$

> **contradict (tmp1,'c2');**

Contradiction on case level 2, so:

$$-c2 b3 - 3 a1 c3 - c3^2 - 9 a1^2 = 0$$

Variables to be uneliminated:

$$a1 := a1$$

$$m3 := m3$$

$$o3 := o3$$

Proceed on case level 1 with:

$$6 b3 \neq 0$$

On account of:

$$-c2 b3 - 3 a1 c3 - c3^2 - 9 a1^2 = 0$$

$$\{b3 \neq 0\}$$

c2 is set to:

$$-\frac{3 a1 c3 + c3^2 + 9 a1^2}{b3}$$

> **launchNZcase (a1);**

Launching case level 2:

$$a1 \neq 0$$

Assume from now on that:

$$6 a1 b3 \neq 0$$

> **tmp1 := cpcoeff (x1^4\*x2);**

$$tmp1 := \frac{54 a1^3 (3 a1 b3 + m3)}{b3}$$

> **elimsolve (tmp1,m3);**

```

{1 ≠ 0}
m3 is set to:
-3 a1 b3
> tmp1 := cpcoeff (x1^4*x3);
tmp1 :=  $\frac{27 a1^3 (9 a1^2 + o3 + 6 a1 c3)}{b3}$ 
> elimsolve (tmp1,o3);
{1 ≠ 0}
o3 is set to:
-3 a1 (2 c3 + 3 a1)
> tmp1 := cpcoeff (x2^2*T);
tmp1 := 81 a1^4
> contradict (tmp1,'a1');
Contradiction on case level 2, so:
a1 = 0
Variables to be uneliminated:
"o3 := 'o3'"
"m3 := 'm3'"
Proceed on case level 1 with:
6 b3 ≠ 0
On account of:
a1 = 0
{1 ≠ 0}
a1 is set to:
0
> tmp1 := cpcoeff (x2^2*T);
tmp1 :=  $-\frac{(-2 m3 c3 + o3 b3)^2}{b3^2}$ 
> elimsolve (tmp1,o3);
{b3 ≠ 0}
o3 is set to:
 $\frac{2 m3 c3}{b3}$ 
> tmp1 := cpcoeff (x1^2*T);
tmp1 :=  $-(2 d1 i3 b3^2 + i3^2 b3^2 - 3 a3 c3 i2 b3^2 - 6 a3 c3^2 i3 b3 + 3 a3 c3^3 g3 - 6 a3 c3^2 d1 b3 + 4 d1^2 b3^2 - 3 a2 b3^3 i2 - 6 a2 b3^2 c3 i3 + 3 a2 b3 g3 c3^2 - 6 a2 b3^2 d1 c3 - c3^2 p3 b3 + i2 g3 b3^2 + c3 b3^2 j1 + 2 c3 s3 b3^2 + s2 b3^3) / b3^2$ 
> elimsolve (tmp1,s2);
{b3^3 ≠ 0}
s2 is set to:
 $-(2 d1 i3 b3^2 + i3^2 b3^2 - 3 a3 c3 i2 b3^2 - 6 a3 c3^2 i3 b3 + 3 a3 c3^3 g3 - 6 a3 c3^2 d1 b3 + 4 d1^2 b3^2 - 3 a2 b3^3 i2 - 6 a2 b3^2 c3 i3 + 3 a2 b3 g3 c3^2 - 6 a2 b3^2 d1 c3 - c3^2 p3 b3$ 

```

$$+ i2 g3 b3^2 + c3 b3^2 j1 + 2 c3 s3 b3^2) / b3^3$$

> **launchNZcase (m3);**

Launching case level 2:

$$m3 \neq 0$$

Assume from now on that:

$$6 b3 m3 \neq 0$$

> **tmp1 := cpcoeff (x1\*x2\*T);**

$$tmp1 := -\frac{2 m3 (i2 b3^2 + 2 c3 i3 b3 - g3 c3^2 + 2 d1 c3 b3)}{b3^2}$$

> **elimsolve (tmp1,i2);**

$$\{b3^2 \neq 0\}$$

i2 is set to:

$$-\frac{c3 (2 i3 b3 - g3 c3 + 2 d1 b3)}{b3^2}$$

> **tmp1 := cpcoeff(x1^3);**

$$tmp1 := -8 d1^3$$

> **elimsolve (tmp1,d1);**

$$\{1 \neq 0\}$$

d1 is set to:

$$0$$

> **tmp1 := cpcoeff (x2\*T);**

$$tmp1 := \frac{2 m3 (i3 b3 - g3 c3)^2}{b3^3}$$

> **elimsolve (tmp1,i3);**

$$\{b3 \neq 0\}$$

i3 is set to:

$$\frac{g3 c3}{b3}$$

> **launchNZcase (j1);**

Launching case level 3:

$$j1 \neq 0$$

Assume from now on that:

$$6 b3 m3 j1 \neq 0$$

> **launchNZcase (-p3\*c3+s3\*b3);**

Launching case level 4:

$$-p3 c3 + s3 b3 \neq 0$$

Assume from now on that:

$$6 b3 m3 j1 (-p3 c3 + s3 b3) \neq 0$$

> **tmp1 := cpcoeff (1);**

$$tmp1 := \frac{j1 (-p3 c3 + s3 b3) (b3 j1 + s3 b3 - p3 c3)}{b3^2}$$

> **elimsolve (tmp1,s3);**

$$\{b3 \neq 0\}$$

s3 is set to:

$$-\frac{b_3 j_1 - p_3 c_3}{b_3}$$

Nonzero constraint refines to:

$$-6 b_3^2 m_3 j_1^2 \neq 0$$

> **tmp1 := cpcoeff (T);**

$$tmp1 := -j_1^2$$

> **contradict (tmp1, 's3');**

Contradiction on case level 4, so:

$$-p_3 c_3 + s_3 b_3 = 0$$

Variables to be uneliminated:

$$s_3 := 's_3'$$

Proceed on case level 3 with:

$$6 b_3 m_3 j_1 \neq 0$$

On account of:

$$-p_3 c_3 + s_3 b_3 = 0$$

$$\{b_3 \neq 0\}$$

s3 is set to:

$$\frac{p_3 c_3}{b_3}$$

> **tmp1 := cpcoeff (T);**

$$tmp1 := -j_1^2$$

> **contradict (tmp1, 'j1');**

Contradiction on case level 3, so:

$$j_1 = 0$$

Variables to be uneliminated:

$$s_3 := 's_3'$$

Proceed on case level 2 with:

$$6 b_3 m_3 \neq 0$$

On account of:

$$j_1 = 0$$

$$\{1 \neq 0\}$$

j1 is set to:

$$0$$

> **tmp1 := cpcoeff (T);**

$$tmp1 := -\frac{(-p_3 c_3 + s_3 b_3)^2}{b_3^2}$$

> **elimsolve (tmp1, s3);**

$$\{b_3 \neq 0\}$$

s3 is set to:

$$\frac{p_3 c_3}{b_3}$$

> **det (T-jacobian (H, [x1, x2, x3]));**

$$T^3$$

> **H;**

$$\left[ 0, \frac{x_1^4}{4} + a_2 x_1^3 - c_3 x_1^2 x_2 - \frac{c_3^2 x_1^2 x_3}{b_3} + d_2 x_1^2 - \frac{g_3 c_3 x_1 x_2}{b_3} - \frac{c_3^2 g_3 x_1 x_3}{b_3^2} + j_2 x_1 \right. \\ \left. - \frac{m_3 c_3 x_2^2}{b_3} - \frac{2 c_3^2 m_3 x_2 x_3}{b_3^2} - \frac{p_3 c_3 x_2}{b_3} - \frac{c_3^3 m_3 x_3^2}{b_3^3} - \frac{c_3^2 p_3 x_3}{b_3^2}, a_3 x_1^3 + b_3 x_1^2 x_2 \right. \\ \left. + c_3 x_1^2 x_3 + d_3 x_1^2 + g_3 x_1 x_2 + \frac{g_3 c_3 x_1 x_3}{b_3} + j_3 x_1 + m_3 x_2^2 + \frac{2 m_3 c_3 x_2 x_3}{b_3} + p_3 x_2 \right. \\ \left. + \frac{c_3^2 m_3 x_3^2}{b_3^2} + \frac{p_3 c_3 x_3}{b_3} \right]$$

> **M:=evalm([ [1,0,0], [0,1,-c3/b3], [0,0,1] ] );**

$$M := \begin{bmatrix} 1 & 0 & 0 \\ 0 & 1 & -\frac{c_3}{b_3} \\ 0 & 0 & 1 \end{bmatrix}$$

> **evalm(simplify(jacobian(evalm(M^(-1))&\***

**subs({seq([x1,x2,x3][i]=evalm(M&\*[x1,x2,x3])[i],i=1..3)},H)),**

**[x1,x2,x3])));**

$$\left[ 0, \frac{x_1^3 b_3 + 3 a_2 x_1^2 b_3 + 2 d_2 x_1 b_3 + j_2 b_3 + 3 c_3 a_3 x_1^2 + 2 c_3 d_3 x_1 + c_3 j_3}{b_3}, 0, 0 \right] \\ \left[ 3 a_3 x_1^2 + 2 b_3 x_1 x_2 + 2 d_3 x_1 + g_3 x_2 + j_3, b_3 x_1^2 + g_3 x_1 + 2 m_3 x_2 + p_3, 0 \right]$$

> **contradict(1,'m3');**

Contradiction on case level 2, so:

$$m_3 = 0$$

Variables to be uneliminated:

"s3 := 's3'"

"j1 := 'j1'"

"i3 := 'i3'"

"d1 := 'd1'"

"i2 := 'i2'"

Proceed on case level 1 with:

$$6 b_3 \neq 0$$

On account of:

$$m_3 = 0$$

$$\{1 \neq 0\}$$

m3 is set to:

$$0$$

> **tmp1 := cpcoeff(x1^2\*x2);**

$$tmp1 := \frac{2 (i_2 b_3^2 + 2 c_3 i_3 b_3 - g_3 c_3^2 + 2 d_1 c_3 b_3)^2}{b_3^2}$$

> **elimsolve(tmp1,i2);**

```

                                 $\{b3^2 \neq 0\}$ 
i2 is set to:
                                
$$-\frac{c3 (2 i3 b3 - g3 c3 + 2 d1 b3)}{b3^2}$$

> tmp1 := cpcoeff (x1^3);
                                 $tmp1 := -8 d1^3$ 
> elimsolve (tmp1,d1);
                                 $\{1 \neq 0\}$ 
d1 is set to:
                                0
> launchNZcase (-c3*g3+i3*b3);
Launching case level 2:
                                 $i3 b3 - g3 c3 \neq 0$ 
Assume from now on that:
                                 $6 b3 (i3 b3 - g3 c3) \neq 0$ 
> tmp1 := cpcoeff (x1*T);
                                
$$tmp1 := -\frac{(i3 b3 - g3 c3) (j1 b3^2 + 2 s3 b3^2 - b3 g3 i3 - 2 p3 c3 b3 + g3^2 c3)}{b3^3}$$

> elimsolve (tmp1,s3);
                                 $\{2 b3^2 \neq 0\}$ 
s3 is set to:
                                
$$-\frac{j1 b3^2 - b3 g3 i3 - 2 p3 c3 b3 + g3^2 c3}{2 b3^2}$$

> tmp1 := cpcoeff (T);
                                
$$tmp1 := -(3 j1^2 b3^4 + b3^2 g3^2 i3^2 + 8 b3^2 g3 i3 p3 c3 - 2 b3 g3^3 i3 c3 - 4 p3 c3^2 b3 g3^2 + g3^4 c3^2 - 4 b3^3 p3 i3^2) / (4 b3^4)$$

> elimsolve (tmp1,p3);
                                 $\{8 b3^2 g3 i3 c3 - 4 c3^2 b3 g3^2 - 4 b3^3 i3^2 \neq 0\}$ 
p3 is set to:
                                
$$\frac{3 j1^2 b3^4 + b3^2 g3^2 i3^2 - 2 b3 g3^3 i3 c3 + g3^4 c3^2}{4 b3 (i3 b3 - g3 c3)^2}$$

> tmp1 := cpcoeff (1);
                                 $tmp1 := -j1^3$ 
> elimsolve (tmp1,j1);
                                 $\{1 \neq 0\}$ 
j1 is set to:
                                0
> det(T-jacobian(H,[x1,x2,x3]));
                                 $T^3$ 
> simplify(evalm([H[1],H[2],H[3]]));
                                 $[0, (-4 i3 x1 x2 b3^3 + 4 a2 x1^3 b3^3 - 4 c3 x1^2 x2 b3^3 + x1^4 b3^3 + 4 j2 x1 b3^3 + 4 d2 x1^2 b3^3$ 

```

$$\begin{aligned} & -4 b^3 x^3 i^3 - 8 b^3 i^3 c^3 x l x^3 - 2 b^3 i^3 g^3 x^2 - 4 c^3 x l^2 x^3 b^3 + 4 b^3 x^3 g^3 c^3 i^3 \\ & + b^3 g^3 x^2 c^3 + 4 b^3 c^3 x l x^3 g^3 - x^3 c^3 g^3) / (4 b^3), (4 b^3 x l^2 x^2 + 4 i^3 x l x^3 b^3 \\ & + 4 d^3 x l^2 b^3 + 4 c^3 x l^2 x^3 b^3 + 4 g^3 x l x^2 b^3 + 4 j^3 x l b^3 + 4 a^3 x l^3 b^3 + 2 b^3 g^3 x^3 i^3 \\ & + g^3 x^2 b^3 - g^3 x^3 c^3) / (4 b^3)] \end{aligned}$$

```
> M := evalm([[-(i3*b3-c3*g3)/b3,0,0],
>             [-1/b3^4*(c3*d3+d2*b3)*(i3*b3-c3*g3)^3,
>             (i3*b3-c3*g3)^4/b3^4,(i3*b3-c3*g3)^4*c3/b3^5],
>             [0,1/2*(i3*b3-c3*g3)^5/b3^6*g3,
>             1/2*(i3*b3-c3*g3)^5*(2*i3*b3-c3*g3)/b3^7]]);
```

$$M := \begin{bmatrix} -\frac{i^3 b^3 - g^3 c^3}{b^3}, & 0, & 0 \\ -\frac{(c^3 d^3 + d^2 b^3)(i^3 b^3 - g^3 c^3)^3}{b^3^4}, & \frac{(i^3 b^3 - g^3 c^3)^4}{b^3^4}, & \frac{(i^3 b^3 - g^3 c^3)^4 c^3}{b^3^5} \\ 0, & \frac{(i^3 b^3 - g^3 c^3)^5 g^3}{2 b^3^6}, & \frac{(i^3 b^3 - g^3 c^3)^5 (2 i^3 b^3 - g^3 c^3)}{2 b^3^7} \end{bmatrix}$$

```
> det (M);
```

$$-\frac{(i^3 b^3 - g^3 c^3)^{11}}{b^3^{12}}$$

```
> G := simplify(evalm(M&*subs({seq([x1,x2,x3][i]=
> evalm(M^(-1)&*[x1,x2,x3])[i],i=1..n)},H)));
```

$$\begin{aligned} G := & [0, (-4 b^4 j^2 x l i^3 - 4 b^4 i^3 a^2 x l^3 - 4 b^4 x^3 + 4 b^4 x l x^2 + b^4 x l^4 \\ & - 4 b^3 c^3 j^3 x l i^3 + 12 b^3 j^2 x l g^3 c^3 i^2 - 4 b^3 c^3 a^3 x l^3 i^3 + 4 b^3 a^2 x l^3 g^3 c^3 \\ & + 12 b^3 j^3 x l g^3 c^3 i^2 - 12 b^3 j^2 x l c^3 g^3 i^3 + 4 b^3 a^3 x l^3 g^3 c^3 \\ & - 12 b^3 j^3 x l c^3 g^3 i^3 + 4 b^3 j^2 x l c^3 g^3 + 4 j^3 x l c^3 g^3) / (4 b^4), (4 j^3 g^5 c^5 \\ & + 16 b^4 i^3 g^3 j^2 c^3 + 4 b^3 g^4 x l c^3 d^3 + 8 b^6 x l x^2 - 8 b^5 j^3 i^5 \\ & - 28 b^4 i^3 g^3 x l c^3 d^3 - 12 b^4 i^3 g^3 d^2 x l c^3 + 20 b^4 i^3 a^3 x l^2 g^3 c^3 \\ & + 8 b^4 i^3 g^3 a^2 x l^2 c^3 + 16 b^4 i^3 g^3 c^3 x l^2 d^3 - 8 b^4 d^2 x l^2 c^3 g^3 \\ & - 64 b^3 j^3 c^3 g^3 i^3 + 36 b^3 i^3 g^3 x l c^3 d^3 - 24 b^3 i^3 g^3 j^2 c^3 \\ & - 16 b^3 i^3 a^3 x l^2 c^3 g^3 + 12 b^3 i^3 g^3 d^2 x l c^3 - 4 b^3 g^3 a^2 x l^2 c^3 \\ & - 8 b^3 g^3 c^3 x l^2 d^3 + 56 b^3 j^3 c^3 g^3 i^2 - 20 b^3 i^3 g^3 x l c^3 d^3 + 16 b^3 i^3 g^3 j^2 c^3 \\ & - 4 b^3 g^3 d^2 x l c^3 + 4 b^3 a^3 x l^2 c^3 g^3 - 24 b^3 j^3 c^4 g^4 i^3 - 4 b^3 g^5 j^2 c^4 \\ & + 4 b^5 i^3 g^3 x l d^2 - 8 b^5 i^3 x l^2 c^3 d^3 - 4 b^5 i^3 g^3 a^2 x l^2 + 16 b^5 d^2 x l^2 g^3 i^3 c^3 \\ & + 36 b^4 j^3 g^3 c^3 i^4 - 8 b^6 d^2 x l^2 i^2 - 8 b^6 x^3 - 4 b^5 i^4 g^3 j^2 + 8 b^5 i^4 d^3 x l \\ & - 8 b^5 i^3 a^3 x l^2 + b^5 i^3 g^3 x l^3 - b^4 g^3 x l^3 c^3) x l / (8 b^6)] \end{aligned}$$

```
> simplify(jacobian(G,[x2,x3]));
```

$$\begin{bmatrix} 0 & 0 \\ x l & -1 \\ x l^2 & -x l \end{bmatrix}$$

> **contradict**(1, 'i3');

Contradiction on case level 2, so:

$$i3 \ b3 - g3 \ c3 = 0$$

Variables to be uneliminated:

$$"j1 := 'j1'"$$

$$"p3 := 'p3'"$$

$$"s3 := 's3'"$$

Proceed on case level 1 with:

$$6 \ b3 \neq 0$$

On account of:

$$i3 \ b3 - g3 \ c3 = 0$$

$$\{b3 \neq 0\}$$

i3 is set to:

$$\frac{g3 \ c3}{b3}$$

> **launchNZcase** (j1);

Launching case level 2:

$$j1 \neq 0$$

Assume from now on that:

$$6 \ j1 \ b3 \neq 0$$

> **launchNZcase** (s3\*b3-c3\*p3);

Launching case level 3:

$$s3 \ b3 - c3 \ p3 \neq 0$$

Assume from now on that:

$$6 \ b3 \ j1 \ (s3 \ b3 - c3 \ p3) \neq 0$$

> **tmp1 := cpcoeff** (1);

$$tmp1 := \frac{j1 \ (s3 \ b3 - c3 \ p3) \ (j1 \ b3 + s3 \ b3 - c3 \ p3)}{b3^2}$$

> **elimsolve** (tmp1, s3);

$$\{b3 \neq 0\}$$

s3 is set to:

$$-\frac{j1 \ b3 - c3 \ p3}{b3}$$

Nonzero constraint refines to:

$$-6 \ b3^2 \ j1^2 \neq 0$$

> **tmp1 := cpcoeff** (T);

$$tmp1 := -j1^2$$

> **contradict** (tmp1, 's3');

Contradiction on case level 3, so:

$$s3 \ b3 - c3 \ p3 = 0$$

Variables to be uneliminated:

$$"s3 := 's3'"$$

Proceed on case level 2 with:

$$6 \ j1 \ b3 \neq 0$$

On account of:

```

s3 b3 - c3 p3 = 0
{b3 ≠ 0}
s3 is set to:

$$\frac{c3 p3}{b3}$$

> tmp1 := cpcoeff (T);

$$tmp1 := -j1^2$$

> contradict (tmp1, 'j1');
Contradiction on case level 2, so:

$$j1 = 0$$

Variables to be uneliminated:
"s3 := 's3'"
Proceed on case level 1 with:

$$6 b3 \neq 0$$

On account of:

$$j1 = 0$$


$$\{1 \neq 0\}$$

j1 is set to:
0
> tmp1 := cpcoeff(T);

$$tmp1 := -\frac{(s3 b3 - c3 p3)^2}{b3^2}$$

> elimsolve (tmp1, s3);
{b3 ≠ 0}
s3 is set to:

$$\frac{c3 p3}{b3}$$

> det(T-jacobian(H, [x1, x2, x3]));

$$T^3$$

> H;

$$\left[ 0, \frac{x1^4}{4} + a2 x1^3 - c3 x1^2 x2 - \frac{c3^2 x1^2 x3}{b3} + d2 x1^2 - \frac{g3 c3 x1 x2}{b3} - \frac{c3^2 g3 x1 x3}{b3^2} + j2 x1 \right.$$


$$\left. - \frac{c3 p3 x2}{b3} - \frac{c3^2 p3 x3}{b3^2}, \right.$$


$$\left. a3 x1^3 + b3 x1^2 x2 + c3 x1^2 x3 + d3 x1^2 + g3 x1 x2 + \frac{g3 c3 x1 x3}{b3} + j3 x1 + p3 x2 + \frac{c3 p3 x3}{b3} \right]$$

> M := evalm ([ [1, 0, 0], [0, 1, -c3/b3], [0, 0, 1] ]);

$$M := \begin{bmatrix} 1 & 0 & 0 \\ 0 & 1 & -\frac{c3}{b3} \\ 0 & 0 & 1 \end{bmatrix}$$

> evalm(simplify(jacobian(evalm(M^(-1)) &*
```

```
> subs ({seq ([x1,x2,x3] [i]=evalm(M&*[x1,x2,x3]) [i] ,i=1..3) },H) ,
> [x1,x2,x3])));
```

$$\begin{bmatrix} 0, & 0, & 0 \\ \frac{x1^3 b3 + 3 a2 x1^2 b3 + 2 d2 x1 b3 + j2 b3 + 3 c3 a3 x1^2 + 2 c3 d3 x1 + c3 j3}{b3}, & 0, & 0 \\ 3 a3 x1^2 + 2 b3 x1 x2 + 2 d3 x1 + g3 x2 + j3, & b3 x1^2 + g3 x1 + p3, & 0 \end{bmatrix}$$

```
> contradict(1,'b3');
```

Contradiction on case level 1, so:

$$b3 = 0$$

Variables to be uneliminated:

```
"s3 := 's3'"
"j1 := 'j1'"
"i3 := 'i3'"
"d1 := 'd1'"
"i2 := 'i2'"
"m3 := 'm3'"
"s2 := 's2'"
"o3 := 'o3'"
"a1 := 'a1'"
"c2 := 'c2'"
"r3 := 'r3'"
"r2 := 'r2'"
"s1 := 's1'"
"i1 := 'i1'"
"q2 := 'q2'"
"r1 := 'r1'"
"h2 := 'h2'"
"h3 := 'h3'"
"q3 := 'q3'"
"q1 := 'q1'"
"f3 := 'f3'"
"n3 := 'n3'"
"w2 := 'w2'"
"v2 := 'v2'"
"h1 := 'h1'"
"u2 := 'u2'"
"c1 := 'c1'"
```

Proceed on case level 0 with:

$$6 \neq 0$$

On account of:

$$b3 = 0$$

|                                   |                    |
|-----------------------------------|--------------------|
|                                   | $\{1 \neq 0\}$     |
| b3 is set to:                     | 0                  |
| > tmp1 := cpcoeff (x1^2*x2^2*T);  |                    |
|                                   | $tmp1 := -f3^2$    |
| > elimsolve (tmp1,f3);            |                    |
|                                   | $\{1 \neq 0\}$     |
| f3 is set to:                     | 0                  |
| > tmp1 := cpcoeff (x2^2*x3^2*T);  |                    |
|                                   | $tmp1 := -3 n3^2$  |
| > elimsolve (tmp1,n3);            |                    |
|                                   | $\{1 \neq 0\}$     |
| n3 is set to:                     | 0                  |
| > launchNZcase (m3);              |                    |
| Launching case level 1:           | $m3 \neq 0$        |
| Assume from now on that:          | $6 m3 \neq 0$      |
| > tmp1 := cpcoeff (x1^5*x2);      |                    |
|                                   | $tmp1 := -2 c1 m3$ |
| > elimsolve (tmp1,c1);            |                    |
|                                   | $\{1 \neq 0\}$     |
| c1 is set to:                     | 0                  |
| > tmp1 := cpcoeff (x2*x3^3*T);    |                    |
|                                   | $tmp1 := -8 w2 m3$ |
| > elimsolve (tmp1,w2);            |                    |
|                                   | $\{1 \neq 0\}$     |
| w2 is set to:                     | 0                  |
| > tmp1 := cpcoeff (x1*x2*x3^2*T); |                    |
|                                   | $tmp1 := -6 v2 m3$ |
| > elimsolve (tmp1,v2);            |                    |
|                                   | $\{1 \neq 0\}$     |
| v2 is set to:                     | 0                  |
| > tmp1 := cpcoeff (x1^2*x2*x3*T); |                    |
|                                   | $tmp1 := -4 u2 m3$ |
| > elimsolve (tmp1,u2);            |                    |
|                                   | $\{1 \neq 0\}$     |
| u2 is set to:                     | 0                  |

```

> tmp1 := cpcoeff (x1^6);
tmp1 := -c3^3
> elimsolve (tmp1,c3);
{1 ≠ 0}
c3 is set to:
0
> tmp1 := cpcoeff (x1^4*x2*x3);
tmp1 := -4 h1 m3
> elimsolve (tmp1,h1);
{1 ≠ 0}
h1 is set to:
0
> tmp1 := cpcoeff (x1^3*x2*x3^2);
tmp1 := -6 q1 m3
> elimsolve (tmp1,q1);
{1 ≠ 0}
q1 is set to:
0
> tmp1 := cpcoeff (x1*x2^2*T);
tmp1 := 4 h3 m3
> elimsolve (tmp1,h3);
{1 ≠ 0}
h3 is set to:
0
> tmp1 := cpcoeff (x3^4*T);
tmp1 := -9 q3^2
> elimsolve (tmp1,q3);
{1 ≠ 0}
q3 is set to:
0
> tmp1 := cpcoeff (x2*x3^2*T);
tmp1 := -6 q2 m3
> elimsolve (tmp1,q2);
{1 ≠ 0}
q2 is set to:
0
> tmp1 := cpcoeff (x1*x2*x3*T);
tmp1 := -4 h2 m3
> elimsolve (tmp1,h2);
{1 ≠ 0}
h2 is set to:
0
> tmp1 := cpcoeff (x1^3*x2*x3);
tmp1 := -4 r1 m3

```

```

> elimsolve (tmp1,r1);
r1 is set to:

$$\{1 \neq 0\}$$


$$0$$

> tmp1 := cpcoeff (x1^4*x2);

$$tmp1 := 2\,m3\,(-i1 + 3\,a1\,c2)$$

> elimsolve (tmp1,i1);
i1 is set to:

$$\{-1 \neq 0\}$$


$$3\,a1\,c2$$

> tmp1 := cpcoeff (x1^2*x2*T);

$$tmp1 := -3\,a1\,o3 - 2\,c2\,m3$$

> elimsolve (tmp1,c2);
c2 is set to:

$$\{2\,m3 \neq 0\}$$


$$-\frac{3\,a1\,o3}{2\,m3}$$

> tmp1 := cpcoeff (x2^2*T);

$$tmp1 := -81\,a1^4 + 4\,r3\,m3 - o3^2$$

> elimsolve (tmp1,r3);
r3 is set to:

$$\{-4\,m3 \neq 0\}$$


$$\frac{81\,a1^4 + o3^2}{4\,m3}$$

> tmp1 := cpcoeff (x1^2*x3*T);

$$tmp1 := -\frac{243\,a1^5}{2\,m3}$$

> elimsolve (tmp1,a1);
a1 is set to:

$$\{1 \neq 0\}$$


$$0$$

> tmp1 := cpcoeff (x1^3*x2);

$$tmp1 := -2\,s1\,m3$$

> elimsolve (tmp1,s1);
s1 is set to:

$$\{1 \neq 0\}$$


$$0$$

> tmp1 := cpcoeff (x2*x3*T);

$$tmp1 := -\frac{8\,r2\,m3^2 + o3^3}{2\,m3}$$

> elimsolve (tmp1,r2);
r2 is set to:

$$\{8\,m3^2 \neq 0\}$$


```

$$-\frac{o3^3}{8\,m3^2}$$

> tmp1 := cpcoeff(1);

$$tmp1 := j1 (s2\,p3 + j1\,s3 + s3^2)$$

> tmp2 := cpcoeff(T);

$$tmp2 := -j1\,s3 - s3^2 - s2\,p3 - j1^2$$

> tmp3 := factor(tmp1 + j1\*tmp2);

$$tmp3 := -j1^3$$

> elimsolve (tmp3,j1);

$$\{1 \neq 0\}$$

j1 is set to:

$$0$$

> tmp1 := cpcoeff(x2\*T);

$$tmp1 := -\frac{4\,s2\,m3^2 - o3^2\,p3 + 4\,s3\,o3\,m3}{2\,m3}$$

> elimsolve (tmp1,s2);

$$\{4\,m3^2 \neq 0\}$$

s2 is set to:

$$-\frac{o3(-o3\,p3 + 4\,s3\,m3)}{4\,m3^2}$$

> tmp1 := cpcoeff (x1\*x2\*T);

$$tmp1 := -\frac{4\,i2\,m3^2 - o3^2\,g3 + 4\,o3\,i3\,m3 + 4\,o3\,m3\,dl}{2\,m3}$$

> elimsolve (tmp1,i2);

$$\{4\,m3^2 \neq 0\}$$

i2 is set to:

$$-\frac{o3(-o3\,g3 + 4\,i3\,m3 + 4\,m3\,dl)}{4\,m3^2}$$

> tmp1 := cpcoeff (T);

$$tmp1 := -\frac{(2\,s3\,m3 - o3\,p3)^2}{4\,m3^2}$$

> elimsolve (tmp1,s3);

$$\{2\,m3 \neq 0\}$$

s3 is set to:

$$\frac{o3\,p3}{2\,m3}$$

> launchNZcase (d1);

Launching case level 2:

$$dl \neq 0$$

Assume from now on that:

$$6\,m3\,dl \neq 0$$

> launchNZcase (o3\*g3-2\*i3\*m3);

Launching case level 3:

$$o3\,g3 - 2\,i3\,m3 \neq 0$$

Assume from now on that:

$$6\,m3\,d1\,(o3\,g3 - 2\,i3\,m3) \neq 0$$

> **tmp1 := cpcoeff (x1^3);**

$$tmp1 := -\frac{d1\,(o3\,g3 - 2\,i3\,m3)\,(-o3\,g3 + 2\,i3\,m3 + 4\,m3\,d1)}{2\,m3^2}$$

> **elimsolve (tmp1,i3);**

$$\{2\,m3 \neq 0\}$$

i3 is set to:

$$-\frac{-o3\,g3 + 4\,m3\,d1}{2\,m3}$$

Nonzero constraint refines to:

$$12\,m3^2\,d1^2 \neq 0$$

> **tmp1 := cpcoeff (x1^2\*T);**

$$tmp1 := -4\,d1^2$$

> **contradict (tmp1,'i3');**

Contradiction on case level 3, so:

$$o3\,g3 - 2\,i3\,m3 = 0$$

Variables to be uneliminated:

$$"i3 := 'i3'"$$

Proceed on case level 2 with:

$$6\,m3\,d1 \neq 0$$

On account of:

$$o3\,g3 - 2\,i3\,m3 = 0$$

$$\{-2\,m3 \neq 0\}$$

i3 is set to:

$$\frac{o3\,g3}{2\,m3}$$

> **tmp1 := cpcoeff (x1^2\*T);**

$$tmp1 := -4\,d1^2$$

> **contradict (tmp1,'d1');**

Contradiction on case level 2, so:

$$d1 = 0$$

Variables to be uneliminated:

$$"i3 := 'i3'"$$

Proceed on case level 1 with:

$$6\,m3 \neq 0$$

On account of:

$$d1 = 0$$

$$\{1 \neq 0\}$$

d1 is set to:

$$0$$

> **tmp1 := cpcoeff (x1^2\*T);**

$$tmp1 := -\frac{(o3\,g3 - 2\,i3\,m3)^2}{4\,m3^2}$$

> **elimsolve** (tmp1,i3);

$$\{-2\,m3 \neq 0\}$$

i3 is set to:

$$\frac{o3\,g3}{2\,m3}$$

> **det**(T-jacobian(H,[x1,x2,x3]));

$$T^3$$

> **H**;

$$\left[ 0, \frac{x1^4}{4} + a2\,x1^3 + d2\,x1^2 - \frac{o3\,g3\,x1\,x2}{2\,m3} - \frac{o3^2\,g3\,x1\,x3}{4\,m3^2} + j2\,x1 - \frac{o3\,x2^2}{2} - \frac{o3^2\,x2\,x3}{2\,m3} \right. \\ \left. - \frac{o3\,p3\,x2}{2\,m3} - \frac{o3^3\,x3^2}{8\,m3^2} - \frac{o3^2\,p3\,x3}{4\,m3^2}, a3\,x1^3 + d3\,x1^2 + g3\,x1\,x2 + \frac{o3\,g3\,x1\,x3}{2\,m3} + j3\,x1 + m3\,x2^2 \right. \\ \left. + o3\,x2\,x3 + p3\,x2 + \frac{o3^2\,x3^2}{4\,m3} + \frac{o3\,p3\,x3}{2\,m3} \right]$$

> **M** := **evalm**([[1,0,0],[0,1,-o3/2/m3],[0,0,1]]);

$$M := \begin{bmatrix} 1 & 0 & 0 \\ 0 & 1 & -\frac{o3}{2\,m3} \\ 0 & 0 & 1 \end{bmatrix}$$

> **evalm**(**simplify**(jacobian(**evalm**(M^(-1)&\***H**),

> **subs**({seq([x1,x2,x3][i]=**evalm**(M&\*[x1,x2,x3])[i],i=1..3)},H),

> [x1,x2,x3])));

$$\begin{bmatrix} 0, & 0, & 0 \\ \frac{2\,x1^3\,m3 + 6\,a2\,x1^2\,m3 + 4\,d2\,x1\,m3 + 2\,j2\,m3 + 3\,o3\,a3\,x1^2 + 2\,o3\,d3\,x1 + o3\,j3}{2\,m3}, & 0, & 0 \\ 3\,a3\,x1^2 + 2\,d3\,x1 + g3\,x2 + j3, & g3\,x1 + 2\,m3\,x2 + p3, & 0 \end{bmatrix}$$

> **contradict** (1,'m3');

Contradiction on case level 1, so:

$$m3 = 0$$

Variables to be uneliminated:

"i3 := 'i3'"

"d1 := 'd1'"

"s3 := 's3'"

"i2 := 'i2'"

"s2 := 's2'"

"j1 := 'j1'"

"r2 := 'r2'"

"s1 := 's1'"

"a1 := 'a1'"

```

"r3 := 'r3'"
"c2 := 'c2'"
"i1 := 'i1'"
"r1 := 'r1'"
"h2 := 'h2'"
"q2 := 'q2'"
"q3 := 'q3'"
"h3 := 'h3'"
"q1 := 'q1'"
"h1 := 'h1'"
"c3 := 'c3'"
"u2 := 'u2'"
"v2 := 'v2'"
"w2 := 'w2'"
"c1 := 'c1'"

```

Proceed on case level 0 with:

$$6 \neq 0$$

On account of:

$$m3 = 0$$

$$\{1 \neq 0\}$$

m3 is set to:

$$0$$

> **launchNZcase (a3);**

Launching case level 1:

$$a3 \neq 0$$

Assume from now on that:

$$6 a3 \neq 0$$

> **tmp1 := cpcoeff (x1^2\*x2\*T);**

$$\begin{aligned}
tmp1 := & c1 g3 + 36 a3 c1 a1 + 9 a3 c1 c3 + 12 a3 c3 h3 + 18 a3 a1 h3 + 6 a3 u2 g3 - 3 a1 c3^2 \\
& + 18 a3^2 h1 - 2 o3 c3 + 2 g3 h3 - 9 a1^2 c3 - c3^3 - 3 a1 o3
\end{aligned}$$

> **elimsolve (tmp1,h1);**

$$\{18 a3^2 \neq 0\}$$

h1 is set to:

$$\begin{aligned}
& -(c1 g3 + 36 a3 c1 a1 + 9 a3 c1 c3 + 12 a3 c3 h3 + 18 a3 a1 h3 + 6 a3 u2 g3 - 3 a1 c3^2 \\
& - 2 o3 c3 + 2 g3 h3 - 9 a1^2 c3 - c3^3 - 3 a1 o3) / (18 a3^2)
\end{aligned}$$

> **tmp1 := cpcoeff (x1^2\*x3^2\*T);**

$$\begin{aligned}
tmp1 := & -(18 a1^2 o3 + 72 h3^2 a3^2 + 72 c1^2 a3^2 + 10 o3 c3^2 - 36 a1 a3 u2 g3 - 30 c3 a3 u2 g3 \\
& - 108 u2 a3^2 a1 c3 + 162 a3^3 q1 + 162 a1 q3 a3^2 + 90 c1 h3 a3^2 + 54 v2 g3 a3^2 \\
& + 36 u2 o3 a3^2 - 216 a3 c1 a1^2 - 6 a1 c1 g3 + 27 a1 o3 c3 - 12 a1 g3 h3 - 45 a3 c1 c3^2 \\
& - 60 a3 c3^2 h3 - 5 c3 c1 g3 - 10 c3 g3 h3 - 36 u2 a3^2 c3^2 - 324 u2 a3^2 a1^2 - 108 u2 a3^3 c1 \\
& + 108 q3 a3^2 c3 + 63 a1^2 c3^2 - 108 a3 a1^2 h3 + 5 c3^4 - 234 a1 a3 c1 c3 - 162 a1 a3 c3 h3
\end{aligned}$$

$$+ 54 a l^3 c 3 + 21 a l c 3^3) / (18 a 3^2)$$

> **elimsolve (tmp1,q1);**

$$\{162 a 3^3 \neq 0\}$$

q1 is set to:

$$\begin{aligned} & - (18 a l^2 o 3 + 72 h 3^2 a 3^2 + 72 c l^2 a 3^2 + 10 o 3 c 3^2 - 36 a l a 3 u 2 g 3 - 30 c 3 a 3 u 2 g 3 \\ & - 108 u 2 a 3^2 a l c 3 + 162 a l q 3 a 3^2 + 90 c l h 3 a 3^2 + 54 v 2 g 3 a 3^2 + 36 u 2 o 3 a 3^2 \\ & - 216 a 3 c l a l^2 - 6 a l c l g 3 + 27 a l o 3 c 3 - 12 a l g 3 h 3 - 45 a 3 c l c 3^2 - 60 a 3 c 3^2 h 3 \\ & - 5 c 3 c l g 3 - 10 c 3 g 3 h 3 - 36 u 2 a 3^2 c 3^2 - 324 u 2 a 3^2 a l^2 - 108 u 2 a 3^3 c l + 108 q 3 a 3^2 c 3 \\ & + 63 a l^2 c 3^2 - 108 a 3 a l^2 h 3 + 5 c 3^4 - 234 a l a 3 c l c 3 - 162 a l a 3 c 3 h 3 + 54 a l^3 c 3 \\ & + 21 a l c 3^3) / (162 a 3^3) \end{aligned}$$

> **tmp1 := cpcoeff (x1^2\*x3\*T);**

$$\begin{aligned} tmp1 := & (27 a 2 a 3^2 c l c 3 - 9 a 2 a 3 c l g 3 + 27 a 2 a 3 a l c 3^2 + 18 a 2 a 3 o 3 c 3 - 18 a 2 a 3 g 3 h 3 \\ & + 81 a 2 a 3 a l^2 c 3 + 27 a 2 a 3 a l o 3 - 36 r 3 a 3^2 c 3 + 54 c 2 a 3^2 a l c 3 + 18 d 3 a 3 c l c 3 \\ & + 24 d 3 a 3 c 3 h 3 + 36 d 3 a 3 a l h 3 + 12 d 3 a 3 u 2 g 3 + 72 d 3 a 3 c l a l - 2 d 3 c 3^3 - 54 a 3^3 r l \\ & - 18 u 2 p 3 a 3^2 - 54 a l r 3 a 3^2 - 36 d l h 3 a 3^2 - 27 c l i 3 a 3^2 - 18 h 2 g 3 a 3^2 - 9 c 2 o 3 a 3^2 \\ & - 27 i l c 3 a 3^2 + 9 a 2 a 3 c 3^3 - 54 a l a 3^2 i l - 72 c l a 3^2 d l + 18 c 2 a 3^2 c 3^2 + 162 c 2 a 3^2 a l^2 \\ & + 54 c 2 a 3^3 c l + 2 d 3 c l g 3 - 6 d 3 a l c 3^2 - 4 d 3 o 3 c 3 + 4 d 3 g 3 h 3 - 18 d 3 a l^2 c 3 \\ & - 6 d 3 a l o 3 - 36 i 3 a 3^2 h 3) / (9 a 3^2) \end{aligned}$$

> **elimsolve (tmp1,r1);**

$$\{-54 a 3^3 \neq 0\}$$

r1 is set to:

$$\begin{aligned} & (27 a 2 a 3^2 c l c 3 - 9 a 2 a 3 c l g 3 + 27 a 2 a 3 a l c 3^2 + 18 a 2 a 3 o 3 c 3 - 18 a 2 a 3 g 3 h 3 \\ & + 81 a 2 a 3 a l^2 c 3 + 27 a 2 a 3 a l o 3 - 36 r 3 a 3^2 c 3 + 54 c 2 a 3^2 a l c 3 + 18 d 3 a 3 c l c 3 \\ & + 24 d 3 a 3 c 3 h 3 + 36 d 3 a 3 a l h 3 + 12 d 3 a 3 u 2 g 3 + 72 d 3 a 3 c l a l - 2 d 3 c 3^3 \\ & - 18 u 2 p 3 a 3^2 - 54 a l r 3 a 3^2 - 36 d l h 3 a 3^2 - 27 c l i 3 a 3^2 - 18 h 2 g 3 a 3^2 - 9 c 2 o 3 a 3^2 \\ & - 27 i l c 3 a 3^2 + 9 a 2 a 3 c 3^3 - 54 a l a 3^2 i l - 72 c l a 3^2 d l + 18 c 2 a 3^2 c 3^2 + 162 c 2 a 3^2 a l^2 \\ & + 54 c 2 a 3^3 c l + 2 d 3 c l g 3 - 6 d 3 a l c 3^2 - 4 d 3 o 3 c 3 + 4 d 3 g 3 h 3 - 18 d 3 a l^2 c 3 \\ & - 6 d 3 a l o 3 - 36 i 3 a 3^2 h 3) / (54 a 3^3) \end{aligned}$$

> **tmp1 := cpcoeff (x1^2\*T);**

$$\begin{aligned} tmp1 := & -i 3^2 - 3 a 3 s l - 2 d 3 i l - j 3 c l + 2 d 2 c 3^2 + 18 d 2 a l^2 - 6 a l j l - 9 a 2^2 c 3^2 \\ & - 81 a 2^2 a l^2 - 2 c 3 s 3 + 9 a 2 a 3 i l + 36 a 2 a l d l - 27 a 2^2 a l c 3 - 27 a 2^2 a 3 c l + 9 a 2 a l i 3 \\ & + 6 a 2 d l c 3 + 6 a 2 c 3 i 3 + 6 a 2 d 3 c l + 3 a 2 c 2 g 3 + 6 d 2 a l c 3 + 6 d 2 a 3 c l - c 2 p 3 - i 2 g 3 \\ & - j l c 3 - 3 a l s 3 - 2 d l i 3 - 4 d l^2 \end{aligned}$$

> **elimsolve (tmp1,s1);**

$$\{3 a 3 \neq 0\}$$

s1 is set to:

$$\begin{aligned} & - (i 3^2 + 2 d 3 i l + j 3 c l - 2 d 2 c 3^2 - 18 d 2 a l^2 + 6 a l j l + 9 a 2^2 c 3^2 + 81 a 2^2 a l^2 + 2 c 3 s 3 \\ & - 9 a 2 a 3 i l - 36 a 2 a l d l + 27 a 2^2 a l c 3 + 27 a 2^2 a 3 c l - 9 a 2 a l i 3 - 6 a 2 d l c 3 \end{aligned}$$

$$-6 a_2 c_3 i_3 - 6 a_2 d_3 c_1 - 3 a_2 c_2 g_3 - 6 d_2 a_1 c_3 - 6 d_2 a_3 c_1 + c_2 p_3 + i_2 g_3 + j_1 c_3 \\ + 3 a_1 s_3 + 2 d_1 i_3 + 4 d_1^2) / (3 a_3)$$

> **launchNZcase (g3);**

Launching case level 2:

$$g_3 \neq 0$$

Assume from now on that:

$$6 a_3 g_3 \neq 0$$

> **tmp1 := cpcoeff (x2\*x3\*T);**

$$\begin{aligned} tmp1 := & (-27 g_3 a_2 a_3 a_1 c_3^2 - 18 g_3 a_2 a_3 o_3 c_3 - 81 g_3 a_2 a_3 a_1^2 c_3 - 27 g_3 a_2 a_3 a_1 o_3 \\ & - 54 g_3 c_2 a_3^2 a_1 c_3 - 18 g_3 d_3 a_3 c_1 c_3 - 24 g_3 d_3 a_3 c_3 h_3 - 36 g_3 d_3 a_3 a_1 h_3 \\ & - 72 g_3 d_3 a_3 c_1 a_1 - 27 g_3 a_2 a_3^2 c_1 c_3 + 162 i_1 a_3^3 a_1 c_3 - 3 p_3 a_3 c_1 g_3 \\ & - 108 p_3 a_3^2 c_1 a_1 - 27 p_3 a_3^2 c_1 c_3 - 36 p_3 a_3^2 c_3 h_3 - 54 p_3 a_3^2 a_1 h_3 + 9 p_3 a_3 a_1 c_3^2 \\ & + 6 p_3 a_3 o_3 c_3 - 6 p_3 a_3 g_3 h_3 + 27 p_3 a_3 a_1^2 c_3 + 9 p_3 a_3 a_1 o_3 - 54 a_3^2 d_1 a_1 c_3^2 \\ & - 36 a_3^2 d_1 o_3 c_3 - 162 a_3^2 d_1 a_1^2 c_3 - 54 a_3^2 d_1 a_1 o_3 - 12 d_3 a_3 u_2 g_3^2 + 54 g_3 a_1 r_3 a_3^2 \\ & + 72 g_3 d_1 h_3 a_3^2 + 27 g_3 c_1 i_3 a_3^2 + 9 g_3 c_2 o_3 a_3^2 + 27 g_3 i_1 c_3 a_3^2 - 9 g_3 a_2 a_3 c_3^3 \\ & + 54 g_3 a_1 a_3^2 i_1 + 90 g_3 c_1 a_3^2 d_1 - 18 g_3 c_2 a_3^2 c_3^2 - 162 g_3 c_2 a_3^2 a_1^2 - 108 g_3 c_2 a_3^3 c_1 \\ & + 6 g_3 d_3 a_1 c_3^2 + 4 g_3 d_3 o_3 c_3 + 18 g_3 d_3 a_1^2 c_3 + 6 g_3 d_3 a_1 o_3 + 36 g_3 i_3 a_3^2 h_3 \\ & - 108 i_3 a_3^3 c_1 c_3 + 36 g_3 r_3 a_3^2 c_3 + 18 h_2 g_3^2 a_3^2 + 18 a_2 a_3 g_3^2 h_3 + 162 r_3 a_3^3 a_1 c_3 \\ & + 9 a_2 a_3 c_1 g_3^2 - 2 d_3 c_1 g_3^2 + 54 r_3 a_3^3 c_3^2 + 486 r_3 a_3^3 a_1^2 + 162 r_3 a_3^4 c_1 - 4 d_3 g_3^2 h_3 \\ & + 2 g_3 d_3 c_3^3 + 54 i_1 a_3^3 c_3^2 + 486 i_1 a_3^3 a_1^2 + 162 p_3 a_3^3 q_3 + 3 p_3 a_3 c_3^3 \\ & + 486 a_3^3 c_1 a_2 a_1 c_3 + 486 a_3^3 h_3 a_2 a_1 c_3 - 54 a_3^3 h_3 c_2 g_3 - 162 a_3^3 c_1 a_1 i_3 \\ & + 162 a_3^3 c_1 a_2 c_3^2 + 1458 a_3^3 c_1 a_2 a_1^2 - 648 a_3^3 c_1 a_1 d_1 - 648 a_3^3 h_3 a_1 d_1 \\ & - 162 a_3^3 h_3 a_1 i_3 - 108 a_3^3 h_3 d_1 c_3 - 108 a_3^3 h_3 c_3 i_3 + 162 a_3^3 h_3 a_2 c_3^2 \\ & + 1458 a_3^3 h_3 a_2 a_1^2 + 486 a_3^4 h_3 a_2 c_1 - 108 a_3^3 h_3 d_3 c_1 - 162 a_3^4 h_3 i_1 + 486 a_3^4 a_2 c_1^2 \\ & - 108 a_3^3 d_3 c_1^2 - 54 r_3 a_3^3 o_3 - 18 a_3^2 d_1 c_3^3 - 162 a_3^3 d_1 c_1 c_3) / (27 a_3^3) \end{aligned}$$

> **elimsolve (tmp1,h2);**

$$\{18 g_3^2 a_3^2 \neq 0\}$$

h2 is set to:

$$\begin{aligned} - & (-27 g_3 a_2 a_3 a_1 c_3^2 - 18 g_3 a_2 a_3 o_3 c_3 - 81 g_3 a_2 a_3 a_1^2 c_3 - 27 g_3 a_2 a_3 a_1 o_3 \\ & - 54 g_3 c_2 a_3^2 a_1 c_3 - 18 g_3 d_3 a_3 c_1 c_3 - 24 g_3 d_3 a_3 c_3 h_3 - 36 g_3 d_3 a_3 a_1 h_3 \\ & - 72 g_3 d_3 a_3 c_1 a_1 - 27 g_3 a_2 a_3^2 c_1 c_3 + 162 i_1 a_3^3 a_1 c_3 - 3 p_3 a_3 c_1 g_3 \\ & - 108 p_3 a_3^2 c_1 a_1 - 27 p_3 a_3^2 c_1 c_3 - 36 p_3 a_3^2 c_3 h_3 - 54 p_3 a_3^2 a_1 h_3 + 9 p_3 a_3 a_1 c_3^2 \\ & + 6 p_3 a_3 o_3 c_3 - 6 p_3 a_3 g_3 h_3 + 27 p_3 a_3 a_1^2 c_3 + 9 p_3 a_3 a_1 o_3 - 54 a_3^2 d_1 a_1 c_3^2 \\ & - 36 a_3^2 d_1 o_3 c_3 - 162 a_3^2 d_1 a_1^2 c_3 - 54 a_3^2 d_1 a_1 o_3 - 12 d_3 a_3 u_2 g_3^2 + 54 g_3 a_1 r_3 a_3^2 \\ & + 72 g_3 d_1 h_3 a_3^2 + 27 g_3 c_1 i_3 a_3^2 + 9 g_3 c_2 o_3 a_3^2 + 27 g_3 i_1 c_3 a_3^2 - 9 g_3 a_2 a_3 c_3^3 \\ & + 54 g_3 a_1 a_3^2 i_1 + 90 g_3 c_1 a_3^2 d_1 - 18 g_3 c_2 a_3^2 c_3^2 - 162 g_3 c_2 a_3^2 a_1^2 - 108 g_3 c_2 a_3^3 c_1 \\ & + 6 g_3 d_3 a_1 c_3^2 + 4 g_3 d_3 o_3 c_3 + 18 g_3 d_3 a_1^2 c_3 + 6 g_3 d_3 a_1 o_3 + 36 g_3 i_3 a_3^2 h_3 \end{aligned}$$

$$\begin{aligned}
& -108 i3 a3^3 c1 c3 + 36 g3 r3 a3^2 c3 + 18 a2 a3 g3^2 h3 + 162 r3 a3^3 a1 c3 + 9 a2 a3 c1 g3^2 \\
& -2 d3 c1 g3^2 + 54 r3 a3^3 c3^2 + 486 r3 a3^3 a1^2 + 162 r3 a3^4 c1 - 4 d3 g3^2 h3 + 2 g3 d3 c3^3 \\
& + 54 i1 a3^3 c3^2 + 486 i1 a3^3 a1^2 + 162 p3 a3^3 q3 + 3 p3 a3 c3^3 + 486 a3^3 c1 a2 a1 c3 \\
& + 486 a3^3 h3 a2 a1 c3 - 54 a3^3 h3 c2 g3 - 162 a3^3 c1 a1 i3 + 162 a3^3 c1 a2 c3^2 \\
& + 1458 a3^3 c1 a2 a1^2 - 648 a3^3 c1 a1 d1 - 648 a3^3 h3 a1 d1 - 162 a3^3 h3 a1 i3 \\
& - 108 a3^3 h3 d1 c3 - 108 a3^3 h3 c3 i3 + 162 a3^3 h3 a2 c3^2 + 1458 a3^3 h3 a2 a1^2 \\
& + 486 a3^4 h3 a2 c1 - 108 a3^3 h3 d3 c1 - 162 a3^4 h3 i1 + 486 a3^4 a2 c1^2 - 108 a3^3 d3 c1^2 \\
& - 54 r3 a3^3 o3 - 18 a3^2 d1 c3^3 - 162 a3^3 d1 c1 c3) / (18 g3^2 a3^2)
\end{aligned}$$

> **tmp1 := cpcoeff (x2\*T);**

$$\begin{aligned}
tmp1 := & (-3 j1 o3 a3 + 18 a3^2 c1 j1 + 9 a3^2 c1 s3 + 6 a3 c3^2 j1 + 3 a3 c3^2 s3 + 54 a3 a1^2 j1 \\
& + 27 a3 a1^2 s3 + 18 a3 a1 c3 j1 + 9 a3 a1 c3 s3 + 3 j3 a3 c1 c3 + 54 d1 a2 a3^2 c1 \\
& + 27 i3 a2 a3^2 c1 - 54 a3 d1 a1 i3 - 18 a3 d1 c3 i3 + 18 a3 d1 a2 c3^2 + 162 a3 d1 a2 a1^2 \\
& - 12 a3 d1 d3 c1 - 6 a3 d1 c2 g3 + 9 a3 i3 a2 c3^2 + 81 a3 i3 a2 a1^2 - 6 a3 i3 d3 c1 \\
& - 3 a3 i3 c2 g3 - 9 g3 a2 a3 i1 - 36 g3 a2 a1 d1 + 27 g3 a2^2 a1 c3 + 27 g3 a2^2 a3 c1 \\
& - 9 g3 a2 a1 i3 - 6 g3 a2 d1 c3 - 6 g3 a2 c3 i3 - 6 g3 a2 d3 c1 + 54 a3 d1 a2 a1 c3 \\
& + 27 a3 i3 a2 a1 c3 + i2 g3^2 + 4 g3 d1^2 - 6 g3 d2 a1 c3 - 6 g3 d2 a3 c1 + g3 c2 p3 + g3 i3^2 \\
& + 3 j3 a1 c3^2 + 2 j3 o3 c3 - 2 j3 g3 h3 + 9 j3 a1^2 c3 + 3 j3 a1 o3 - 18 d1 a3^2 i1 - 9 i3 a3^2 i1 \\
& - 72 a3 a1 d1^2 - 12 a3 d1^2 c3 - 9 a3 a1 i3^2 - 6 a3 c3 i3^2 - 3 a2 c2 g3^2 + 2 g3 d3 i1 \\
& - 2 g3 d2 c3^2 - 18 g3 d2 a1^2 + 6 g3 a1 j1 + 9 g3 a2^2 c3^2 + 81 g3 a2^2 a1^2 + 2 g3 c3 s3 \\
& + g3 j1 c3 + 3 g3 a1 s3 + 2 g3 d1 i3 + 6 p3 a3 r3 + 3 p3 a3 i1 - 6 o3 a3 s3 + j3 c3^3) / (3 a3)
\end{aligned}$$

> **elimsolve (tmp1,i2);**

$$\{g3^2 \neq 0\}$$

i2 is set to:

$$\begin{aligned}
& -(-3 j1 o3 a3 + 18 a3^2 c1 j1 + 9 a3^2 c1 s3 + 6 a3 c3^2 j1 + 3 a3 c3^2 s3 + 54 a3 a1^2 j1 \\
& + 27 a3 a1^2 s3 + 18 a3 a1 c3 j1 + 9 a3 a1 c3 s3 + 3 j3 a3 c1 c3 + 54 d1 a2 a3^2 c1 \\
& + 27 i3 a2 a3^2 c1 - 54 a3 d1 a1 i3 - 18 a3 d1 c3 i3 + 18 a3 d1 a2 c3^2 + 162 a3 d1 a2 a1^2 \\
& - 12 a3 d1 d3 c1 - 6 a3 d1 c2 g3 + 9 a3 i3 a2 c3^2 + 81 a3 i3 a2 a1^2 - 6 a3 i3 d3 c1 \\
& - 3 a3 i3 c2 g3 - 9 g3 a2 a3 i1 - 36 g3 a2 a1 d1 + 27 g3 a2^2 a1 c3 + 27 g3 a2^2 a3 c1 \\
& - 9 g3 a2 a1 i3 - 6 g3 a2 d1 c3 - 6 g3 a2 c3 i3 - 6 g3 a2 d3 c1 + 54 a3 d1 a2 a1 c3 \\
& + 27 a3 i3 a2 a1 c3 + 4 g3 d1^2 - 6 g3 d2 a1 c3 - 6 g3 d2 a3 c1 + g3 c2 p3 + g3 i3^2 \\
& + 3 j3 a1 c3^2 + 2 j3 o3 c3 - 2 j3 g3 h3 + 9 j3 a1^2 c3 + 3 j3 a1 o3 - 18 d1 a3^2 i1 - 9 i3 a3^2 i1 \\
& - 72 a3 a1 d1^2 - 12 a3 d1^2 c3 - 9 a3 a1 i3^2 - 6 a3 c3 i3^2 - 3 a2 c2 g3^2 + 2 g3 d3 i1 \\
& - 2 g3 d2 c3^2 - 18 g3 d2 a1^2 + 6 g3 a1 j1 + 9 g3 a2^2 c3^2 + 81 g3 a2^2 a1^2 + 2 g3 c3 s3 \\
& + g3 j1 c3 + 3 g3 a1 s3 + 2 g3 d1 i3 + 6 p3 a3 r3 + 3 p3 a3 i1 - 6 o3 a3 s3 + j3 c3^3) / g3^2
\end{aligned}$$

> **tmp1 := cpcoeff (x1\*x3^2\*T);**

$$tmp1 := -(84 a3 c3^2 d3 c1 g3^2 - 729 a1^2 c3^3 g3 a2 a3^2 - 81 a1 c3^2 g3 a2 a3^2 o3$$

$$\begin{aligned}
& -1458 a l^3 c^3 g^3 a^2 a^3 + 72 d^3 g^3 a l a^3 u^2 + 60 d^3 g^3 c^3 a^3 u^2 + 162 a^3 a l^2 c^3 g^3 d^3 \\
& + 324 a^3 a l^3 c^3 g^3 d^3 + 162 q^2 g^3 a^3 - 243 a l^2 c^3 g^3 a^2 a^3 o^3 - 1458 a l^2 c^3 g^3 c^2 a^3 \\
& - 324 a l c^3 g^3 d^3 a^3 c l - 324 a l c^3 g^3 d^3 a^3 h^3 - 972 a l^2 c^3 g^3 d^3 a^3 h^3 \\
& - 972 a l^2 c^3 g^3 d^3 a^3 c l + 1458 a l c^3 g^3 a^2 a^3 c l - 459 a l c^3 p^3 a^3 c l g^3 \\
& - 1458 a l^2 c^3 p^3 a^3 c l - 486 a l c^3 p^3 a^3 c l - 486 a l c^3 p^3 a^3 h^3 \\
& - 1458 a l^2 c^3 p^3 a^3 h^3 + 27 a l c^3 p^3 a^3 o^3 - 9 a^3 g^3 i^3 c l - 54 a^3 g^3 i^3 u^2 \\
& - 18 a^3 g^3 i^3 h^3 + 9 a^3 g^3 i^3 c^3 - 324 a^3 g^3 i^3 c l a l - 81 a^3 g^3 i^3 c l c^3 \\
& - 108 a^3 g^3 i^3 c^3 h^3 - 162 a^3 g^3 i^3 a l h^3 + 27 a^3 g^3 i^3 a l c^3 + 18 a^3 g^3 i^3 o^3 c^3 \\
& + 81 a^3 g^3 i^3 a l^2 c^3 + 27 a^3 g^3 i^3 a l o^3 - 432 d l a^3 g^3 c l a l - 36 d l a^3 g^3 c l c^3 \\
& - 216 d l a^3 g^3 a l h^3 + 36 d l a^3 g^3 a l c^3 + 24 d l a^3 g^3 o^3 c^3 + 108 d l a^3 g^3 a l^2 c^3 \\
& + 36 d l a^3 g^3 a l o^3 - 324 c^2 a^3 g^3 c l c^3 - 108 c^2 a^3 g^3 a l c^3 - 72 c^2 a^3 g^3 o^3 c^3 \\
& - 324 c^2 a^3 g^3 a l^2 c^3 - 108 c^2 a^3 g^3 a l o^3 + 9 c^5 p^3 a^3 + 162 c^4 r^3 a^3 \\
& + 162 c^4 i l a^3 - 54 c^5 a^3 d l + 13122 a l^4 r^3 a^3 + 13122 a l^4 i l a^3 + 1458 a^3 c l^2 r^3 \\
& + 4374 a^3 c l^3 a^2 - 972 a^3 c l^3 d^3 - 10 d^3 g^3 c^3 + 216 c l r^3 a^3 g^3 + 324 d l q^3 a^3 g^3 \\
& + 162 v^2 p^3 a^3 g^3 + 162 i l h^3 a^3 g^3 + 36 c^2 a^3 g^3 c l + 72 c^2 a^3 g^3 h^3 \\
& - 36 c^2 a^3 g^3 c^3 + 216 c l a^3 g^3 i l - 12 d l a^3 g^3 c l - 72 d l a^3 g^3 u^2 \\
& - 24 d l a^3 g^3 h^3 + 12 d l a^3 g^3 c^3 - 108 o^3 a^3 a^2 g^3 h^3 - 54 o^3 a^3 a^2 c l g^3 \\
& + 12 o^3 a^3 d^3 c l g^3 - 324 o^3 a^3 i l c^3 - 2916 o^3 a^3 i l a l^2 - 972 o^3 a^3 p^3 q^3 \\
& + 972 o^3 a^3 h^3 i l - 2916 o^3 a^3 a^2 c l^2 + 648 o^3 a^3 d^3 c l^2 + 324 o^3 a^3 r^3 \\
& - 972 o^3 a^3 i l a l c^3 + 18 o^3 a^3 p^3 c l g^3 + 216 o^3 a^3 p^3 c^3 h^3 + 324 o^3 a^3 p^3 a l h^3 \\
& + 36 o^3 a^3 p^3 g^3 h^3 - 324 o^3 a^3 g^3 a l r^3 - 432 o^3 a^3 g^3 d l h^3 - 162 o^3 a^3 g^3 c l i^3 \\
& - 162 o^3 a^3 g^3 i l c^3 - 324 o^3 a^3 g^3 a l i l - 540 o^3 a^3 g^3 c l d l - 24 o^3 a^3 g^3 d^3 c^3 \\
& - 36 o^3 a^3 g^3 d^3 a l - 216 o^3 a^3 g^3 i^3 h^3 + 648 o^3 a^3 i^3 c l c^3 + 108 o^3 a^3 g^3 a^2 c^3 \\
& + 162 o^3 a^3 g^3 a^2 a l + 144 o^3 a^3 g^3 d^3 c^3 h^3 + 216 o^3 a^3 g^3 d^3 a l h^3 \\
& - 324 u^2 a^3 g^3 a l i^3 - 216 u^2 a^3 g^3 d l c^3 - 216 u^2 a^3 g^3 c^3 i^3 \\
& + 972 u^2 a^3 g^3 a^2 a l c^3 + 324 u^2 a^3 g^3 a^2 c^3 + 2916 u^2 a^3 g^3 a^2 a l^2 \\
& + 972 u^2 a^3 g^3 a^2 c l - 324 d^3 g^3 a l q^3 a^3 - 54 d^3 g^3 a l o^3 c^3 - 216 d^3 g^3 q^3 a^3 c^3 \\
& - 1296 u^2 a^3 g^3 a l d l - 216 c^3 a^3 g^3 h^3 c^2 + 648 c^3 a^3 g^3 h^3 a^2 \\
& + 5832 c^3 a^3 g^3 h^3 a^2 a l^2 + 1944 c^3 a^3 g^3 h^3 a^2 c l + 648 c^3 a^3 g^3 p^3 q^3 \\
& - 648 c^3 a^3 g^3 h^3 i l - 432 c^3 a^3 g^3 r^3 o^3 + 1944 c^3 a^3 g^3 h^3 a^2 a l - 12 c^3 a^3 g^3 p^3 c l \\
& + 36 c^3 a^3 g^3 p^3 a l + 24 c^3 a^3 g^3 p^3 o^3 - 24 c^3 a^3 g^3 p^3 h^3 + 108 c^3 a^3 g^3 p^3 a l^2 \\
& + 36 c^3 a^3 g^3 p^3 a l o^3 - 216 c^3 a^3 g^3 d l a l - 144 c^3 a^3 g^3 d l o^3 \\
& - 648 c^3 a^3 g^3 d l a l^2 - 216 c^3 a^3 g^3 d l a l o^3 - 72 c^3 a^3 g^3 u^2 p^3 + 36 a^3 a l c^3 g^3 d^3 \\
& + 24 o^3 a^3 d^3 g^3 h^3 - 2916 o^3 a^3 c l a^2 a l c^3 - 2916 o^3 a^3 h^3 a^2 a l c^3 \\
& + 324 o^3 a^3 h^3 c^2 g^3 + 972 o^3 a^3 c l a l i^3 - 972 o^3 a^3 c l a^2 c^3 - 8748 o^3 a^3 c l a^2 a l^2
\end{aligned}$$

$$\begin{aligned}
& + 3888 o3 a3^4 h3 a1 d1 + 972 o3 a3^4 h3 a1 i3 + 648 o3 a3^4 h3 d1 c3 + 648 o3 a3^4 h3 c3 i3 \\
& - 972 o3 a3^4 h3 a2 c3^2 - 8748 o3 a3^4 h3 a2 a1^2 - 2916 o3 a3^5 h3 a2 c1 + 648 o3 a3^4 h3 d3 c1 \\
& + 486 a3 a1^4 g3 d3 c3 + 162 a3 a1^3 g3 d3 o3 + 378 a3 a1^2 d3 c1 g3^2 + 108 a3 c3^2 d3 g3^2 h3 \\
& + 54 a3 a1^2 c3 g3 d3 o3 + 450 a3 a1 c3 d3 c1 g3^2 + 288 a3 a1 c3 d3 g3^2 h3 \\
& + 18 a3 a1 c3^2 g3 d3 o3 + 108 a3 a1^2 d3 g3^2 h3 + 1458 a3^5 c1 p3 q3 - 1458 a3^5 c1^2 a1 i3 \\
& - 5832 a3^5 c1^2 a1 d1 + 4374 a3^6 c1^2 h3 a2 - 972 a3^5 c1^2 h3 d3 - 1458 a3^6 c1 h3 i1 \\
& - 1458 a3^5 c1 r3 o3 - 1458 a3^5 c1^2 d1 c3 + 6 a3 c3^5 g3 d3 + 12 c3^4 a3 g3 p3 \\
& - 72 c3^4 a3^2 g3 d1 - 36 d3 g3^2 a1^2 o3 - 144 d3 g3^2 h3^2 a3^2 - 20 d3 g3^2 o3 c3^2 \\
& - 108 d3 g3^3 v2 a3^2 + 12 d3 g3^3 a1 c1 + 24 d3 g3^3 a1 h3 + 10 d3 g3^3 c3 c1 + 20 d3 g3^3 c3 h3 \\
& - 126 d3 g3^2 a1^2 c3^2 - 108 d3 g3^2 a1^3 c3 - 42 d3 g3^2 a1 c3^3 - 324 u2 a3^4 g3^2 i1 \\
& - 108 u2 a3^3 g3^3 c2 + 324 i3 a3^3 g3^2 q3 + 432 h3 a3^3 g3^2 r3 - 36 o3^2 a3^2 p3 c3 \\
& - 54 o3^2 a3^2 p3 a1 + 216 o3^2 a3^3 d1 c3 + 324 o3^2 a3^3 d1 a1 - 54 o3^2 a3^3 g3 c2 \\
& - 216 a3^2 c1 d3 g3^2 h3 - 486 a3^5 c1 h3 c2 g3 - 5832 a3^5 c1 h3 a1 d1 - 1458 a3^5 c1 h3 a1 i3 \\
& - 972 a3^5 c1 h3 d1 c3 - 972 a3^5 c1 h3 c3 i3 - 1458 a1^2 a3^4 h3 c2 g3 \\
& + 26244 a1^2 a3^5 h3 a2 c1 - 2916 a1^2 a3^4 h3 d3 c1 - 243 a3^3 c1 g3 a2 a1 o3 \\
& - 594 a3^3 c1^2 g3 d3 c3 - 648 a3^3 c1 g3 d3 c3 h3 - 324 a3^3 c1 g3 d3 a1 h3 \\
& - 648 a3^3 c1^2 g3 d3 a1 + 1701 a3^4 c1^2 g3 a2 c3 + 1458 a3^5 c1 i1 a1 c3 - 324 a3^4 c1 p3 c3 h3 \\
& - 486 a3^4 c1 p3 a1 h3 + 216 a3^3 c1 p3 o3 c3 - 54 a3^3 c1 p3 g3 h3 + 729 a3^3 c1 p3 a1 o3 \\
& + 648 a3^4 c1 d1 o3 c3 + 3402 a3^4 c1 d1 a1 o3 - 108 a3^3 c1 d3 u2 g3^2 + 486 a3^4 c1 g3 a1 r3 \\
& + 648 a3^4 c1 g3 d1 h3 - 4374 a1^2 r3 a3^4 o3 - 27 a3^3 c1^2 p3 g3 - 972 a3^4 c1^2 p3 a1 \\
& - 243 a3^4 c1^2 p3 c3 + 243 a3^4 c1^2 g3 i3 + 810 a3^4 c1^2 g3 d1 - 972 a3^5 c1^2 g3 c2 \\
& - 972 a3^5 c1^2 i3 c3 + 81 a3^3 c1^2 a2 g3^2 - 162 a3^2 c1^2 d3 g3^2 + 486 a3^5 c1 i1 c3^2 \\
& + 4374 a3^5 c1 i1 a1^2 + 108 a1 c3 d3 a3^2 u2 g3^2 - 1944 a1 c3 g3 d1 h3 a3^3 \\
& - 405 a1 c3 g3 c1 i3 a3^3 + 405 a1 c3 g3 c2 o3 a3^3 + 1053 a1 c3^2 g3 i1 a3^3 \\
& - 162 a1 c3^4 g3 a2 a3^2 + 3159 a1^2 c3 g3 a3^3 i1 - 1782 a1 c3 g3 c1 a3^3 d1 \\
& - 324 a1 c3^3 g3 c2 a3^3 - 2916 a1^3 c3 g3 c2 a3^3 - 1458 a1 c3 g3 c2 a3^4 c1 \\
& + 729 a3^4 c1 g3 c2 o3 + 243 a3^4 c1 g3 i1 c3 + 486 a3^4 c1 g3 a1 i1 + 144 a3^2 c1 g3 d3 o3 c3 \\
& + 486 a3^2 c1 g3 d3 a1 o3 + 324 a3^4 c1 g3 i3 h3 + 972 a3^4 c1 g3 r3 c3 + 162 a3^3 c1 a2 g3^2 h3 \\
& + 162 a1 c3 a2 a3^2 g3^2 h3 + 81 a1 c3 a2 a3^2 c1 g3^2 + 2916 a1 c3 r3 a3^5 c1 \\
& + 1458 a1 c3 p3 a3^4 q3 + 13122 a1^2 c3^2 a3^4 c1 a2 + 13122 a1^2 c3^2 a3^4 h3 a2 \\
& - 486 a1 c3 a3^4 h3 c2 g3 - 4374 a1^2 c3 a3^4 c1 i3 + 2916 a1 c3^3 a3^4 c1 a2 \\
& + 26244 a1^3 c3 a3^4 c1 a2 - 3888 a1 c3^2 a3^4 d1 c1 - 2187 a1^4 g3 a2 a3^2 c3 \\
& + 4374 a1^2 c3^2 i1 a3^4 + 486 c3^3 g3 a2 a3^3 c1 - 117 c3^2 p3 a3^2 c1 g3 - 11664 a1^2 c3 a3^4 c1 d1 \\
& - 8748 a1^2 c3 a3^4 h3 d1 - 4374 a1^2 c3 a3^4 h3 i3 - 2916 a1 c3^2 a3^4 h3 d1 \\
& - 1458 a1 c3^2 a3^4 h3 i3 + 2916 a1 c3^3 a3^4 h3 a2 + 26244 a1^3 c3 a3^4 h3 a2
\end{aligned}$$

$$\begin{aligned}
& + 8748 a l c 3 a 3^5 h 3 a 2 c l - 972 a l c 3 a 3^4 h 3 d 3 c l - 1458 a l c 3 a 3^5 h 3 i l \\
& + 8748 a l c 3 a 3^5 a 2 c l^2 - 972 a l c 3 a 3^4 d 3 c l^2 - 1458 a l c 3 r 3 a 3^4 o 3 \\
& - 324 a l c 3 g 3 i 3 a 3^3 h 3 - 1458 a l c 3^2 i 3 a 3^4 c l - 270 a l c 3 p 3 a 3^2 g 3 h 3 \\
& - 72 c 3^3 g 3 d 3 a 3^2 h 3 + 1134 a l c 3^2 g 3 r 3 a 3^3 - 729 a l^3 g 3 a 2 a 3^2 o 3 - 972 a l^3 g 3 d 3 a 3^2 h 3 \\
& - 1944 a l^3 g 3 d 3 a 3^2 c l + 4374 a l^2 g 3 a 2 a 3^3 c l c 3 - 81 a l^2 p 3 a 3^2 c l g 3 \\
& - 162 a l^2 p 3 a 3^2 g 3 h 3 + 324 a l^2 d 3 a 3^2 u 2 g 3^2 + 1944 a l^2 g 3 d l h 3 a 3^3 \\
& + 729 a l^2 g 3 c l i 3 a 3^3 + 1215 a l^2 g 3 c 2 o 3 a 3^3 + 2430 a l^2 g 3 c l a 3^3 d l \\
& - 4374 a l^2 g 3 c 2 a 3^4 c l + 972 a l^2 g 3 i 3 a 3^3 h 3 + 486 a l^2 a 2 a 3^2 g 3^2 h 3 \\
& + 243 a l^2 a 2 a 3^2 c l g 3^2 - 162 a l c 3^2 a 3^3 d l o 3 - 486 a l^2 c 3 a 3^3 d l o 3 \\
& + 3402 a l^2 c 3 g 3 r 3 a 3^3 + 81 a l^2 c 3 p 3 a 3^2 o 3 - 162 c 3^2 a 3^4 h 3 c 2 g 3 + 2916 c 3^2 a 3^5 h 3 a 2 c l \\
& - 324 c 3^2 a 3^4 h 3 d 3 c l - 162 c 3^2 p 3 a 3^2 g 3 h 3 + 36 c 3^2 d 3 a 3^2 u 2 g 3^2 - 216 c 3^2 g 3 d l h 3 a 3^3 \\
& - 351 c 3^2 g 3 c l i 3 a 3^3 + 135 c 3^2 g 3 c 2 o 3 a 3^3 - 378 c 3^2 g 3 c l a 3^3 d l - 486 c 3^2 g 3 c 2 a 3^4 c l \\
& - 324 c 3^2 g 3 i 3 a 3^3 h 3 + 54 c 3^2 a 2 a 3^2 g 3^2 h 3 + 27 c 3^2 a 2 a 3^2 c l g 3^2 - 36 c 3^3 g 3 d 3 a 3^2 c l \\
& - 2916 a l^2 a 3^4 d 3 c l^2 - 1458 a l^2 c 3^3 a 3^3 d l - 2916 a l^3 c 3^2 a 3^3 d l - 486 c 3^2 a 3^5 h 3 i l \\
& - 324 c 3^2 a 3^4 d 3 c l^2 - 486 c 3^2 r 3 a 3^4 o 3 - 648 c 3^3 a 3^4 d l c l - 2916 a l^3 p 3 a 3^3 c l \\
& - 1458 a l^3 p 3 a 3^3 h 3 + 729 a l^4 p 3 a 3^2 c 3 + 243 a l^3 p 3 a 3^2 o 3 - 4374 a l^4 a 3^3 d l c 3 \\
& - 1458 a l^3 a 3^3 d l o 3 + 1458 a l^3 g 3 r 3 a 3^3 + 1458 a l^3 g 3 a 3^3 i l - 4374 a l^4 g 3 c 2 a 3^3 \\
& + 8748 a l^2 r 3 a 3^5 c l + 2916 c 3^2 a 3^5 a 2 c l^2 + 486 c 3^2 p 3 a 3^4 q 3 + 486 c 3^4 a 3^4 c l a 2 \\
& - 324 c 3^3 a 3^4 h 3 d l - 324 c 3^3 a 3^4 h 3 i 3 + 486 c 3^4 a 3^4 h 3 a 2 - 108 c 3^3 p 3 a 3^3 h 3 \\
& + 297 c 3^3 g 3 i l a 3^3 - 27 c 3^5 g 3 a 2 a 3^2 - 54 c 3^4 g 3 c 2 a 3^3 - 324 c 3^3 i 3 a 3^4 c l \\
& + 324 c 3^3 g 3 r 3 a 3^3 + 972 c 3^2 r 3 a 3^5 c l - 54 c 3^3 p 3 a 3^3 c l + 243 a l^2 c 3^3 p 3 a 3^2 \\
& + 486 a l^3 c 3^2 p 3 a 3^2 + 4374 a l^2 c 3^2 r 3 a 3^4 + 972 a l c 3^3 r 3 a 3^4 + 8748 a l^3 c 3 r 3 a 3^4 \\
& + 972 a l c 3^3 i l a 3^4 + 8748 a l^3 c 3 i l a 3^4 + 54 a l c 3^4 p 3 a 3^2 - 324 a l c 3^4 a 3^3 d l \\
& + 4374 a l^2 p 3 a 3^4 q 3 - 4374 a l^3 a 3^4 c l i 3 + 39366 a l^4 a 3^4 c l a 2 - 17496 a l^3 a 3^4 c l d l \\
& - 17496 a l^3 a 3^4 h 3 d l - 4374 a l^3 a 3^4 h 3 i 3 + 39366 a l^4 a 3^4 h 3 a 2 - 4374 a l^2 a 3^5 h 3 i l \\
& + 26244 a l^2 a 3^5 a 2 c l^2) / (54 a 3^3 g 3^2)
\end{aligned}$$

> **elimsolve (tmp1,q2);**

$$\{ 162 g 3^3 a 3^3 \neq 0 \}$$

q2 is set to:

$$\begin{aligned}
& - (84 a 3 c 3^2 d 3 c l g 3^2 - 729 a l^2 c 3^3 g 3 a 2 a 3^2 - 81 a l c 3^2 g 3 a 2 a 3^2 o 3 \\
& - 1458 a l^3 c 3^2 g 3 a 2 a 3^2 + 72 d 3 g 3^3 a l a 3 u 2 + 60 d 3 g 3^3 c 3 a 3 u 2 + 162 a 3 a l^2 c 3^3 g 3 d 3 \\
& + 324 a 3 a l^3 c 3^2 g 3 d 3 - 243 a l^2 c 3 g 3 a 2 a 3^2 o 3 - 1458 a l^2 c 3^2 g 3 c 2 a 3^3 \\
& - 324 a l c 3^2 g 3 d 3 a 3^2 c l - 324 a l c 3^2 g 3 d 3 a 3^2 h 3 - 972 a l^2 c 3 g 3 d 3 a 3^2 h 3 \\
& - 972 a l^2 c 3 g 3 d 3 a 3^2 c l + 1458 a l c 3^2 g 3 a 2 a 3^3 c l - 459 a l c 3 p 3 a 3^2 c l g 3 \\
& - 1458 a l^2 c 3 p 3 a 3^3 c l - 486 a l c 3^2 p 3 a 3^3 c l - 486 a l c 3^2 p 3 a 3^3 h 3 \\
& - 1458 a l^2 c 3 p 3 a 3^3 h 3 + 27 a l c 3^2 p 3 a 3^2 o 3 - 9 a 3 g 3^3 i 3 c l - 54 a 3^2 g 3^3 i 3 u 2
\end{aligned}$$

$$\begin{aligned}
& -18 a3 g3^3 i3 h3 + 9 a3 g3^2 i3 c3^3 - 324 a3^2 g3^2 i3 c1 a1 - 81 a3^2 g3^2 i3 c1 c3 \\
& - 108 a3^2 g3^2 i3 c3 h3 - 162 a3^2 g3^2 i3 a1 h3 + 27 a3 g3^2 i3 a1 c3^2 + 18 a3 g3^2 i3 o3 c3 \\
& + 81 a3 g3^2 i3 a1^2 c3 + 27 a3 g3^2 i3 a1 o3 - 432 d1 a3^2 g3^2 c1 a1 - 36 d1 a3^2 g3^2 c1 c3 \\
& - 216 d1 a3^2 g3^2 a1 h3 + 36 d1 a3 g3^2 a1 c3^2 + 24 d1 a3 g3^2 o3 c3 + 108 d1 a3 g3^2 a1^2 c3 \\
& + 36 d1 a3 g3^2 a1 o3 - 324 c2 a3^3 g3^2 c1 c3 - 108 c2 a3^2 g3^2 a1 c3^2 - 72 c2 a3^2 g3^2 o3 c3 \\
& - 324 c2 a3^2 g3^2 a1^2 c3 - 108 c2 a3^2 g3^2 a1 o3 + 9 c3^5 p3 a3^2 + 162 c3^4 r3 a3^4 \\
& + 162 c3^4 i1 a3^4 - 54 c3^5 a3^3 d1 + 13122 a1^4 r3 a3^4 + 13122 a1^4 i1 a3^4 + 1458 a3^6 c1^2 r3 \\
& + 4374 a3^6 c1^3 a2 - 972 a3^5 c1^3 d3 - 10 d3 g3^2 c3^4 + 216 c1 r3 a3^3 g3^2 + 324 d1 q3 a3^3 g3^2 \\
& + 162 v2 p3 a3^3 g3^2 + 162 i1 h3 a3^3 g3^2 + 36 c2 a3^2 g3^3 c1 + 72 c2 a3^2 g3^3 h3 \\
& - 36 c2 a3^2 g3^2 c3^3 + 216 c1 a3^3 g3^2 i1 - 12 d1 a3 g3^3 c1 - 72 d1 a3^2 g3^3 u2 \\
& - 24 d1 a3 g3^3 h3 + 12 d1 a3 g3^2 c3^3 - 108 o3 a3^2 a2 g3^2 h3 - 54 o3 a3^2 a2 c1 g3^2 \\
& + 12 o3 a3 d3 c1 g3^2 - 324 o3 a3^4 i1 c3^2 - 2916 o3 a3^4 i1 a1^2 - 972 o3 a3^4 p3 q3 \\
& + 972 o3 a3^5 h3 i1 - 2916 o3 a3^5 a2 c1^2 + 648 o3 a3^4 d3 c1^2 + 324 o3^2 a3^4 r3 \\
& - 972 o3 a3^4 i1 a1 c3 + 18 o3 a3^2 p3 c1 g3 + 216 o3 a3^3 p3 c3 h3 + 324 o3 a3^3 p3 a1 h3 \\
& + 36 o3 a3^2 p3 g3 h3 - 324 o3 a3^3 g3 a1 r3 - 432 o3 a3^3 g3 d1 h3 - 162 o3 a3^3 g3 c1 i3 \\
& - 162 o3 a3^3 g3 i1 c3 - 324 o3 a3^3 g3 a1 i1 - 540 o3 a3^3 g3 c1 d1 - 24 o3^2 a3 g3 d3 c3 \\
& - 36 o3^2 a3 g3 d3 a1 - 216 o3 a3^3 g3 i3 h3 + 648 o3 a3^4 i3 c1 c3 + 108 o3^2 a3^2 g3 a2 c3 \\
& + 162 o3^2 a3^2 g3 a2 a1 + 144 o3 a3^2 g3 d3 c3 h3 + 216 o3 a3^2 g3 d3 a1 h3 \\
& - 324 u2 a3^3 g3^2 a1 i3 - 216 u2 a3^3 g3^2 d1 c3 - 216 u2 a3^3 g3^2 c3 i3 \\
& + 972 u2 a3^3 g3^2 a2 a1 c3 + 324 u2 a3^3 g3^2 a2 c3^2 + 2916 u2 a3^3 g3^2 a2 a1^2 \\
& + 972 u2 a3^4 g3^2 a2 c1 - 324 d3 g3^2 a1 q3 a3^2 - 54 d3 g3^2 a1 o3 c3 - 216 d3 g3^2 q3 a3^2 c3 \\
& - 1296 u2 a3^3 g3^2 a1 d1 - 216 c3 a3^3 g3^2 h3 c2 + 648 c3^3 a3^3 g3 h3 a2 \\
& + 5832 c3 a3^3 g3 h3 a2 a1^2 + 1944 c3 a3^4 g3 h3 a2 c1 + 648 c3 a3^3 g3 p3 q3 \\
& - 648 c3 a3^4 g3 h3 i1 - 432 c3 a3^3 g3 r3 o3 + 1944 c3^2 a3^3 g3 h3 a2 a1 - 12 c3 a3 g3^2 p3 c1 \\
& + 36 c3^3 a3 g3 p3 a1 + 24 c3^2 a3 g3 p3 o3 - 24 c3 a3 g3^2 p3 h3 + 108 c3^2 a3 g3 p3 a1^2 \\
& + 36 c3 a3 g3 p3 a1 o3 - 216 c3^3 a3^2 g3 d1 a1 - 144 c3^2 a3^2 g3 d1 o3 \\
& - 648 c3^2 a3^2 g3 d1 a1^2 - 216 c3 a3^2 g3 d1 a1 o3 - 72 c3 a3^2 g3^2 u2 p3 + 36 a3 a1 c3^4 g3 d3 \\
& + 24 o3 a3 d3 g3^2 h3 - 2916 o3 a3^4 c1 a2 a1 c3 - 2916 o3 a3^4 h3 a2 a1 c3 \\
& + 324 o3 a3^4 h3 c2 g3 + 972 o3 a3^4 c1 a1 i3 - 972 o3 a3^4 c1 a2 c3^2 - 8748 o3 a3^4 c1 a2 a1^2 \\
& + 3888 o3 a3^4 h3 a1 d1 + 972 o3 a3^4 h3 a1 i3 + 648 o3 a3^4 h3 d1 c3 + 648 o3 a3^4 h3 c3 i3 \\
& - 972 o3 a3^4 h3 a2 c3^2 - 8748 o3 a3^4 h3 a2 a1^2 - 2916 o3 a3^5 h3 a2 c1 + 648 o3 a3^4 h3 d3 c1 \\
& + 486 a3 a1^4 g3 d3 c3 + 162 a3 a1^3 g3 d3 o3 + 378 a3 a1^2 d3 c1 g3^2 + 108 a3 c3^2 d3 g3^2 h3 \\
& + 54 a3 a1^2 c3 g3 d3 o3 + 450 a3 a1 c3 d3 c1 g3^2 + 288 a3 a1 c3 d3 g3^2 h3 \\
& + 18 a3 a1 c3^2 g3 d3 o3 + 108 a3 a1^2 d3 g3^2 h3 + 1458 a3^5 c1 p3 q3 - 1458 a3^5 c1^2 a1 i3 \\
& - 5832 a3^5 c1^2 a1 d1 + 4374 a3^6 c1^2 h3 a2 - 972 a3^5 c1^2 h3 d3 - 1458 a3^6 c1 h3 i1
\end{aligned}$$

$$\begin{aligned}
& -1458 a^5 c l r_3 o_3 - 1458 a^5 c l^2 d l c_3 + 6 a^3 c^5 g_3 d_3 + 12 c^4 a^3 g_3 p_3 \\
& - 72 c^4 a^3 g_3 d l - 36 d_3 g_3^2 a l^2 o_3 - 144 d_3 g_3^2 h_3^2 a^2 - 20 d_3 g_3^2 o_3 c^2 \\
& - 108 d_3 g_3^3 v_2 a^2 + 12 d_3 g_3^3 a l c l + 24 d_3 g_3^3 a l h_3 + 10 d_3 g_3^3 c_3 c l + 20 d_3 g_3^3 c_3 h_3 \\
& - 126 d_3 g_3^2 a l^2 c^2 - 108 d_3 g_3^2 a l^3 c_3 - 42 d_3 g_3^2 a l c^3 - 324 u_2 a^4 g_3^2 i l \\
& - 108 u_2 a^3 g_3^3 c_2 + 324 i_3 a^3 g_3^2 q_3 + 432 h_3 a^3 g_3^2 r_3 - 36 o_3^2 a^2 p_3 c_3 \\
& - 54 o_3^2 a^2 p_3 a l + 216 o_3^2 a^3 d l c_3 + 324 o_3^2 a^3 d l a l - 54 o_3^2 a^3 g_3 c_2 \\
& - 216 a^2 c l d_3 g_3^2 h_3 - 486 a^5 c l h_3 c_2 g_3 - 5832 a^5 c l h_3 a l d l - 1458 a^5 c l h_3 a l i_3 \\
& - 972 a^5 c l h_3 d l c_3 - 972 a^5 c l h_3 c_3 i_3 - 1458 a l^2 a^4 h_3 c_2 g_3 \\
& + 26244 a l^2 a^5 h_3 a_2 c l - 2916 a l^2 a^4 h_3 d_3 c l - 243 a^3 c l g_3 a_2 a l o_3 \\
& - 594 a^3 c l^2 g_3 d_3 c_3 - 648 a^3 c l g_3 d_3 c_3 h_3 - 324 a^3 c l g_3 d_3 a l h_3 \\
& - 648 a^3 c l^2 g_3 d_3 a l + 1701 a^4 c l^2 g_3 a_2 c_3 + 1458 a^5 c l i l a l c_3 - 324 a^4 c l p_3 c_3 h_3 \\
& - 486 a^4 c l p_3 a l h_3 + 216 a^3 c l p_3 o_3 c_3 - 54 a^3 c l p_3 g_3 h_3 + 729 a^3 c l p_3 a l o_3 \\
& + 648 a^4 c l d l o_3 c_3 + 3402 a^4 c l d l a l o_3 - 108 a^3 c l d_3 u_2 g_3^2 + 486 a^4 c l g_3 a l r_3 \\
& + 648 a^4 c l g_3 d l h_3 - 4374 a l^2 r_3 a^4 o_3 - 27 a^3 c l^2 p_3 g_3 - 972 a^4 c l^2 p_3 a l \\
& - 243 a^4 c l^2 p_3 c_3 + 243 a^4 c l^2 g_3 i_3 + 810 a^4 c l^2 g_3 d l - 972 a^5 c l^2 g_3 c_2 \\
& - 972 a^5 c l^2 i_3 c_3 + 81 a^3 c l^2 a_2 g_3^2 - 162 a^2 c l^2 d_3 g_3^2 + 486 a^5 c l i l c_3^2 \\
& + 4374 a^5 c l i l a l^2 + 108 a l c_3 d_3 a^2 u_2 g_3^2 - 1944 a l c_3 g_3 d l h_3 a^3 \\
& - 405 a l c_3 g_3 c l i_3 a^3 + 405 a l c_3 g_3 c_2 o_3 a^3 + 1053 a l c_3^2 g_3 i l a^3 \\
& - 162 a l c_3^4 g_3 a_2 a^2 + 3159 a l^2 c_3 g_3 a^3 i l - 1782 a l c_3 g_3 c l a^3 d l \\
& - 324 a l c_3^3 g_3 c_2 a^3 - 2916 a l^3 c_3 g_3 c_2 a^3 - 1458 a l c_3 g_3 c_2 a^4 c l \\
& + 729 a^4 c l g_3 c_2 o_3 + 243 a^4 c l g_3 i l c_3 + 486 a^4 c l g_3 a l i l + 144 a^2 c l g_3 d_3 o_3 c_3 \\
& + 486 a^2 c l g_3 d_3 a l o_3 + 324 a^4 c l g_3 i_3 h_3 + 972 a^4 c l g_3 r_3 c_3 + 162 a^3 c l a_2 g_3^2 h_3 \\
& + 162 a l c_3 a_2 a^2 g_3^2 h_3 + 81 a l c_3 a_2 a^2 c l g_3^2 + 2916 a l c_3 r_3 a^5 c l \\
& + 1458 a l c_3 p_3 a^4 q_3 + 13122 a l^2 c_3^2 a^4 c l a_2 + 13122 a l^2 c_3^2 a^4 h_3 a_2 \\
& - 486 a l c_3 a^4 h_3 c_2 g_3 - 4374 a l^2 c_3 a^4 c l i_3 + 2916 a l c_3^3 a^4 c l a_2 \\
& + 26244 a l^3 c_3 a^4 c l a_2 - 3888 a l c_3^2 a^4 d l c l - 2187 a l^4 g_3 a_2 a^2 c_3 \\
& + 4374 a l^2 c_3^2 i l a^4 + 486 c_3^3 g_3 a_2 a^3 c l - 117 c_3^2 p_3 a^2 c l g_3 - 11664 a l^2 c_3 a^4 c l d l \\
& - 8748 a l^2 c_3 a^4 h_3 d l - 4374 a l^2 c_3 a^4 h_3 i_3 - 2916 a l c_3^2 a^4 h_3 d l \\
& - 1458 a l c_3^2 a^4 h_3 i_3 + 2916 a l c_3^3 a^4 h_3 a_2 + 26244 a l^3 c_3 a^4 h_3 a_2 \\
& + 8748 a l c_3 a^5 h_3 a_2 c l - 972 a l c_3 a^4 h_3 d_3 c l - 1458 a l c_3 a^5 h_3 i l \\
& + 8748 a l c_3 a^5 a_2 c l^2 - 972 a l c_3 a^4 d_3 c l^2 - 1458 a l c_3 r_3 a^4 o_3 \\
& - 324 a l c_3 g_3 i_3 a^3 h_3 - 1458 a l c_3^2 i_3 a^4 c l - 270 a l c_3 p_3 a^2 g_3 h_3 \\
& - 72 c_3^3 g_3 d_3 a^2 h_3 + 1134 a l c_3^2 g_3 r_3 a^3 - 729 a l^3 g_3 a_2 a^2 o_3 - 972 a l^3 g_3 d_3 a^2 h_3 \\
& - 1944 a l^3 g_3 d_3 a^2 c l + 4374 a l^2 g_3 a_2 a^3 c l c_3 - 81 a l^2 p_3 a^2 c l g_3 \\
& - 162 a l^2 p_3 a^2 g_3 h_3 + 324 a l^2 d_3 a^2 u_2 g_3^2 + 1944 a l^2 g_3 d l h_3 a^3
\end{aligned}$$

$$\begin{aligned}
& + 729 a l^2 g_3 c l i_3 a_3^3 + 1215 a l^2 g_3 c_2 o_3 a_3^3 + 2430 a l^2 g_3 c l a_3^3 d l \\
& - 4374 a l^2 g_3 c_2 a_3^4 c l + 972 a l^2 g_3 i_3 a_3^3 h_3 + 486 a l^2 a_2 a_3^2 g_3^2 h_3 \\
& + 243 a l^2 a_2 a_3^2 c l g_3^2 - 162 a l c_3^2 a_3^3 d l o_3 - 486 a l^2 c_3 a_3^3 d l o_3 \\
& + 3402 a l^2 c_3 g_3 r_3 a_3^3 + 81 a l^2 c_3 p_3 a_3^2 o_3 - 162 c_3^2 a_3^4 h_3 c_2 g_3 + 2916 c_3^2 a_3^5 h_3 a_2 c l \\
& - 324 c_3^2 a_3^4 h_3 d_3 c l - 162 c_3^2 p_3 a_3^2 g_3 h_3 + 36 c_3^2 d_3 a_3^2 u_2 g_3^2 - 216 c_3^2 g_3 d l h_3 a_3^3 \\
& - 351 c_3^2 g_3 c l i_3 a_3^3 + 135 c_3^2 g_3 c_2 o_3 a_3^3 - 378 c_3^2 g_3 c l a_3^3 d l - 486 c_3^2 g_3 c_2 a_3^4 c l \\
& - 324 c_3^2 g_3 i_3 a_3^3 h_3 + 54 c_3^2 a_2 a_3^2 g_3^2 h_3 + 27 c_3^2 a_2 a_3^2 c l g_3^2 - 36 c_3^3 g_3 d_3 a_3^2 c l \\
& - 2916 a l^2 a_3^4 d_3 c l^2 - 1458 a l^2 c_3^3 a_3^3 d l - 2916 a l^3 c_3^2 a_3^3 d l - 486 c_3^2 a_3^5 h_3 i l \\
& - 324 c_3^2 a_3^4 d_3 c l^2 - 486 c_3^2 r_3 a_3^4 o_3 - 648 c_3^3 a_3^4 d l c l - 2916 a l^3 p_3 a_3^3 c l \\
& - 1458 a l^3 p_3 a_3^3 h_3 + 729 a l^4 p_3 a_3^2 c_3 + 243 a l^3 p_3 a_3^2 o_3 - 4374 a l^4 a_3^3 d l c_3 \\
& - 1458 a l^3 a_3^3 d l o_3 + 1458 a l^3 g_3 r_3 a_3^3 + 1458 a l^3 g_3 a_3^3 i l - 4374 a l^4 g_3 c_2 a_3^3 \\
& + 8748 a l^2 r_3 a_3^5 c l + 2916 c_3^2 a_3^5 a_2 c l^2 + 486 c_3^2 p_3 a_3^4 q_3 + 486 c_3^3 a_3^4 c l a_2 \\
& - 324 c_3^3 a_3^4 h_3 d l - 324 c_3^3 a_3^4 h_3 i_3 + 486 c_3^4 a_3^4 h_3 a_2 - 108 c_3^3 p_3 a_3^3 h_3 \\
& + 297 c_3^3 g_3 i l a_3^3 - 27 c_3^5 g_3 a_2 a_3^2 - 54 c_3^4 g_3 c_2 a_3^3 - 324 c_3^3 i_3 a_3^4 c l \\
& + 324 c_3^3 g_3 r_3 a_3^3 + 972 c_3^2 r_3 a_3^5 c l - 54 c_3^3 p_3 a_3^3 c l + 243 a l^2 c_3^3 p_3 a_3^2 \\
& + 486 a l^3 c_3^2 p_3 a_3^2 + 4374 a l^2 c_3^2 r_3 a_3^4 + 972 a l c_3^3 r_3 a_3^4 + 8748 a l^3 c_3 r_3 a_3^4 \\
& + 972 a l c_3^3 i l a_3^4 + 8748 a l^3 c_3 i l a_3^4 + 54 a l c_3^4 p_3 a_3^2 - 324 a l c_3^4 a_3^3 d l \\
& + 4374 a l^2 p_3 a_3^4 q_3 - 4374 a l^3 a_3^4 c l i_3 + 39366 a l^4 a_3^4 c l a_2 - 17496 a l^3 a_3^4 c l d l \\
& - 17496 a l^3 a_3^4 h_3 d l - 4374 a l^3 a_3^4 h_3 i_3 + 39366 a l^4 a_3^4 h_3 a_2 - 4374 a l^2 a_3^5 h_3 i l \\
& + 26244 a l^2 a_3^5 a_2 c l^2) / (162 g_3^3 a_3^3)
\end{aligned}$$

> **tmp1 := cpccoeff (x1\*x3\*T);**

$$\begin{aligned}
tmp1 := & - (-j_3 g_3^3 c l - 72 c_2 a_3^2 g_3^2 d_3 c l + 81 c_2 a_3^3 g_3^2 a_2 c l + 243 c_2 a_3^2 g_3^2 a_2 a l^2 \\
& + 27 c_2 a_3^2 g_3^2 a_2 c_3^2 - 54 c_2 a_3^2 g_3^2 c_3 i_3 - 54 c_2 a_3^2 g_3^2 a l i_3 - 216 c_2 a_3^2 g_3^2 a l d l \\
& - 162 a_3^4 c_3^2 d l i l + 81 c_2 a_3^2 g_3^2 a_2 a l c_3 + 324 d_3 g_3 a_3^2 h_3 a_2 a l c_3 - 24 j_3 g_3^2 a_3 c_3 h_3 \\
& - 18 j_3 g_3^2 a_3 a l h_3 - 36 j_3 g_3^2 a_3 c l a l - 15 j_3 g_3^2 a_3 c l c_3 - 54 d_2 a_3 g_3^2 a l^2 c_3 \\
& - 18 d_2 a_3 g_3^2 a l o_3 - 12 d_2 a_3 g_3^2 o_3 c_3 - 18 d_2 a_3 g_3^2 a l c_3^2 - 18 d_2 a_3^2 g_3^2 c l c_3 \\
& - 72 c_2 a_3^2 g_3^2 d l c_3 - 6 d_2 a_3 g_3^2 c_3^3 + 12 d_2 a_3 g_3^3 h_3 + 6 d_2 a_3 g_3^3 c l - 54 c_2 a_3^3 g_3^2 i l \\
& - 6 j_3 g_3^3 a_3 u_2 - 72 d_3^2 g_3 a_3^2 c l^2 + 3 j_3 g_3^2 a l o_3 + 9 j_3 g_3^2 a l^2 c_3 + 2 j_3 g_3^2 o_3 c_3 \\
& + 3 j_3 g_3^2 a l c_3^2 + 36 d l a_3^2 g_3^2 i l + 36 c l a_3^2 g_3^2 j l + 18 i l a_3^2 g_3^2 i_3 - 729 a_3^3 a l^2 c_3 i_3^2 \\
& - 243 a_3^3 a l c_3^2 i_3^2 + 2916 a_3^3 a l^3 c_3 j l + 1458 a_3^3 a l^3 c_3 s_3 + 1458 a_3^3 a l^2 c_3^2 j l \\
& + 729 a_3^3 a l^2 c_3^2 s_3 + 324 a_3^3 a l c_3^3 j l + 162 a_3^3 a l c_3^3 s_3 - 972 a_3^3 a l c_3^2 d l^2 \\
& - 2916 a_3^3 a l^2 c_3 d l^2 + 162 a_3^4 c_3^2 c l s_3 + 324 a_3^4 c_3^2 c l j l + 162 a_3^3 c_3^4 d l a_2 \\
& - 81 a_3^3 c_3^2 j l o_3 - 162 a_3^3 c_3^3 d l i_3 + 54 a_3^3 c_3^3 j_3 c l + 81 a_3^3 c_3^4 i_3 a_2 - 81 a_3^4 c_3^2 i_3 i l \\
& - 12 d_3 g_3 a_3 d l c_3^3 - 36 d_3 g_3 r_3 a_3^2 o_3 + 162 d_3 g_3 a_3^3 a_2 c l^2 + 486 d_3 g_3 i l a_3^2 a l^2 \\
& + 36 d_3 g_3 r_3 a_3^2 c_3^2 + 108 d_3 g_3 p_3 a_3^2 q_3 + 108 d_3 g_3 r_3 a_3^3 c l + 324 d_3 g_3 r_3 a_3^2 a l^2
\end{aligned}$$

$$\begin{aligned}
& + 54 d3 g3 i l a3^2 c3^2 + 162 d3 g3 a3^2 c l a2 a l c3 + 12 d3 g3^2 c l a3 d l + 24 d3 g3^2 d l h3 a3 \\
& - 108 d3 g3 a3^3 h3 i l - 108 d3 g3 a3 d l a l^2 c3 - 36 d3 g3 a3 d l a l o3 \\
& - 36 d3 g3 a3 d l a l c3^2 + 162 d3 g3 i l a3^2 a l c3 - 72 d3^2 g3 a3^2 h3 c l - 36 d3 g3^2 a3^2 h3 c2 \\
& + 108 d3 g3 r3 a3^2 a l c3 - 24 d3 g3 a3 d l o3 c3 - 432 d3 g3 a3^2 c l a l d l \\
& - 108 d3 g3 i3 a3^2 c l c3 + 6561 a3^3 a l^4 i3 a2 - 4374 a3^3 a l^3 d l i3 - 108 d3 g3 a3^2 c l a l i3 \\
& + 54 d3 g3 a3^2 c l a2 c3^2 + 13122 a3^3 a l^4 d l a2 + 486 d3 g3 a3^2 c l a2 a l^2 \\
& - 108 d3 g3 a3^2 h3 a l i3 - 72 d3 g3 a3^2 h3 d l c3 - 72 d3 g3 a3^2 h3 c3 i3 \\
& - 180 d3 g3 a3^2 d l c l c3 - 432 d3 g3 a3^2 h3 a l d l + 324 d3 g3 a3^3 h3 a2 c l \\
& + 108 d3 g3 a3^2 h3 a2 c3^2 + 972 d3 g3 a3^2 h3 a2 a l^2 + 243 a3^2 a l^2 g3 c2 p3 \\
& - 162 a3^2 a l^2 j3 g3 h3 - 729 a3^2 a l^3 g3 a2 i3 - 2916 a3^2 a l^3 g3 a2 d l - 18 a3^2 c3^2 j3 g3 h3 \\
& + 27 a3^2 c3^2 g3 c2 p3 - 90 a3^2 c3^2 g3 d l i3 + 54 a3^2 c3^3 g3 a2 d l + 189 a3^2 a l c3^2 g3 j l \\
& + 405 a3^2 a l^2 c3 g3 s3 + 135 a3^2 a l c3^2 g3 s3 + 162 a3^2 a l^2 c3 j3 o3 - 108 a3^2 a l c3^3 g3 d2 \\
& + 486 a3^2 a l c3^3 g3 a2^2 - 972 a3^2 a l^3 c3 g3 d2 + 567 a3^2 a l^2 c3 g3 j l \\
& + 4374 a3^2 a l^3 c3 g3 a2^2 - 324 a3^2 a l c3 g3 d l^2 + 2187 a3^2 a l^2 c3^2 g3 a2^2 \\
& - 27 a3^2 a l c3 g3 i3^2 + 1458 a3^4 a l^2 c l s3 - 486 a3^2 a l^2 c3^2 g3 d2 + 54 a3^2 a l c3^2 j3 o3 \\
& + 162 a3^3 a l c3^2 j3 c l - 2916 a3^3 a l^2 c3 d l i3 - 972 a3^3 a l c3^2 d l i3 + 972 a3^3 a l c3^3 d l a2 \\
& + 8748 a3^3 a l^3 c3 d l a2 + 4374 a3^3 a l^3 c3 i3 a2 + 486 a3^3 a l c3^3 i3 a2 \\
& + 162 a3^2 a l^2 g3 d l i3 - 27 a3^3 c3^2 p3 i l - 81 a3^3 c3^2 o3 s3 - 729 a3^3 a l^2 j l o3 \\
& + 2916 a3^4 a l^2 c l j l - 243 a3^3 a l^2 p3 i l - 729 a3^3 a l^2 o3 s3 + 27 o3^2 a3^3 j l \\
& - 243 a3^4 c l j l o3 + 81 a3^4 c l^2 j3 c3 - 1458 a3^4 a l^2 d l i l + 2187 a3^3 a l^2 c3^2 i3 a2 \\
& - 729 a3^4 a l^2 i3 i l - 486 a3^4 a l c3 d l i l - 243 a3^3 a l c3 j l o3 + 972 a3^4 a l c3 c l j l \\
& + 486 a3^4 a l c3 c l s3 + 729 a3^5 c l^2 i3 a2 + 243 a3^5 c l^2 s3 - 324 a3^4 c l^2 d l d3 \\
& + 486 a3^4 c3^2 i3 a2 c l - 162 a3^4 c l^2 i3 d3 - 108 a3^3 c3^2 d l d3 c l - 243 a3^4 a l c3 i3 i l \\
& + 729 a3^4 c l^2 g3 a2^2 + 486 a3^5 c l^2 j l - 81 a3^3 a l c3 p3 i l + 4374 a3^3 a l^2 c3^2 d l a2 \\
& - 54 a3^3 c3^2 d l c2 g3 - 486 a3^5 c l d l i l + 27 a3^3 c3^4 s3 - 81 a3^3 c3^2 g3 a2 i l \\
& - 243 a3^5 c l i3 i l + 486 a3^3 c3^2 g3 a2^2 c l - 243 a3^3 a l c3 o3 s3 - 1944 a3^4 c l a l d l^2 \\
& - 324 a3^4 c l d l^2 c3 + 54 a3^3 c3^4 j l + 972 a3^4 c3^2 d l a2 c l - 243 a3^4 c l a l i3^2 \\
& - 54 a3^3 c3^3 i3^2 - 162 a3^4 c l c3 i3^2 + 81 a3^4 c l p3 i l - 108 a3^3 c3^3 d l^2 - 243 a3^4 c l o3 s3 \\
& + 1458 a3^5 c l^2 d l a2 - 972 a3^3 a l^2 d l d3 c l - 486 a3^3 a l^2 d l c2 g3 - 243 a3^3 a l^2 i3 c2 g3 \\
& - 729 a3^3 a l^2 g3 a2 i l - 81 a3^2 a l c3^2 g3 a2 i3 - 54 a3^2 a l c3 j3 g3 h3 \\
& - 972 a3^3 a l^2 g3 d2 c l - 486 a3^2 a l^2 c3 g3 a2 d l + 4374 a3^3 a l^2 g3 a2^2 c l \\
& - 486 a3^3 a l^2 i3 d3 c l + 486 a3^3 a l^2 j3 c l c3 + 8748 a3^4 a l^2 d l a2 c l + 4374 a3^4 a l^2 i3 a2 c l \\
& + 108 a3^3 c l g3 d l^2 + 9 a3^2 c3^5 j3 - 162 a3^4 c l^2 g3 d2 - 27 a3^3 c3^2 i3 c2 g3 \\
& + 27 a3^3 c l g3 i3^2 - 108 a3^3 c3^2 g3 d2 c l - 54 a3^3 c3^2 i3 d3 c l + 81 a3^2 a l c3 g3 c2 p3 \\
& - 54 a3^3 c l j3 g3 h3 + 81 a3^3 c l j3 a l o3 + 54 a3^3 c l g3 d3 i l + 162 a3^3 c l g3 a l j l
\end{aligned}$$

$$\begin{aligned}
& -270 a^3 a^2 c^3 g^3 d^2 i^3 + 135 a^3 c^3 g^3 j^2 c^3 + 108 a^3 c^3 g^3 c^3 s^3 + 54 a^3 c^3 g^3 d^2 i^3 \\
& -162 a^3 a^2 c^3 g^3 a^2 d^2 - 243 a^3 a^2 c^3 g^3 a^2 i^3 - 81 a^3 c^3 i^3 c^2 g^3 \\
& -162 a^3 c^3 d^2 c^2 g^3 - 1458 a^3 c^3 d^2 a^2 i^3 + 135 a^3 c^3 g^3 c^2 p^3 - 486 a^3 c^3 d^2 c^3 i^3 \\
& + 81 a^3 c^3 g^3 a^2 s^3 - 243 a^3 c^3 g^3 a^2 i^2 + 27 a^3 c^3 j^3 o^3 c^3 + 243 a^3 a^2 c^3 j^3 \\
& + 1458 a^3 a^2 c^3 g^3 a^2 c^2 - 324 a^3 a^2 c^3 g^3 d^2 c^2 - 972 a^3 c^3 g^3 a^2 a^2 d^2 \\
& + 2916 a^3 a^2 c^3 d^2 a^2 c^2 + 1458 a^3 a^2 c^3 i^3 a^2 c^2 - 27 c^3 a^3 g^3 j^2 o^3 \\
& - 324 a^3 a^2 c^3 d^2 d^3 c^2 + 81 a^3 a^2 c^3 g^3 i^3 + 729 a^3 a^2 c^3 j^3 c^3 + 2187 a^3 a^2 c^3 s^3 \\
& + 243 a^3 a^2 c^3 j^3 o^3 + 4374 a^3 a^2 c^3 j^2 - 1458 a^3 a^2 c^3 g^3 d^2 - 729 a^3 a^2 c^3 i^3 \\
& + 18 c^3 a^3 g^3 j^3 c^2 + 486 a^3 a^2 c^3 g^3 j^2 + 6561 a^3 a^2 c^3 g^3 a^2 - 5832 a^3 a^2 c^3 d^2 \\
& + 243 a^3 a^2 c^3 g^3 s^3 + 9 a^3 c^3 j^3 o^3 - 243 a^3 c^3 g^3 a^2 a^2 i^3 + 162 a^3 c^3 g^3 a^2 d^2 c^3 \\
& - 162 a^3 a^2 c^3 d^2 c^2 g^3 - 162 a^3 a^2 c^3 i^3 d^3 c^2 - 36 a^3 c^3 g^3 d^2 - 27 a^3 c^3 g^3 i^3 \\
& - 81 a^3 a^2 c^3 i^3 c^2 g^3 + 486 a^3 a^2 c^3 c^3 j^3 + 54 a^3 a^2 c^3 j^3 - 243 a^3 a^2 c^3 g^3 a^2 i^2 \\
& - 108 c^3 a^3 g^3 d^2 i^2 + 54 c^3 a^3 g^3 j^3 a^2 + 18 c^3 a^3 g^3 j^3 a^2 + 12 c^3 a^3 g^3 j^3 o^3 \\
& - 18 a^3 c^3 g^3 d^2 + 81 a^3 c^3 g^3 a^2 + 36 a^3 c^3 g^3 s^3 + 45 a^3 c^3 g^3 j^2 \\
& + 324 a^3 a^2 c^3 g^3 d^2 - 54 c^3 a^3 g^3 i^3 i^2 - 9 c^3 a^3 g^3 p^3 i^2 + 6 c^3 a^3 g^3 j^3 \\
& - 54 c^3 a^3 g^3 o^3 s^3 + 36 i^3 a^3 g^3 r^3 + 18 c^3 a^3 g^3 j^3 a^2 o^3 + 36 s^3 a^3 g^3 h^3 \\
& - 486 o^3 a^3 d^2 a^2 c^2 + 54 o^3 a^3 i^3 d^3 c^2 - 486 o^3 a^3 d^2 a^2 a^2 c^3 + 54 o^3 a^3 g^3 a^2 d^3 c^2 \\
& + 54 o^3 a^3 g^3 a^2 c^3 i^3 - 81 o^3 a^3 i^3 a^2 c^3 - 1458 o^3 a^3 d^2 a^2 a^2 \\
& + 54 o^3 a^3 g^3 a^2 d^2 c^3 + 54 o^3 a^3 d^2 c^2 g^3 + 108 o^3 a^3 d^2 d^3 c^2 + 81 o^3 a^3 g^3 a^2 a^2 i^3 \\
& - 243 o^3 a^3 g^3 a^2 a^2 c^3 - 162 o^3 a^3 d^2 a^2 c^3 + 324 o^3 a^3 g^3 a^2 a^2 d^2 \\
& + 486 o^3 a^3 d^2 a^2 i^3 + 162 o^3 a^3 d^2 c^3 i^3 - 243 o^3 a^3 i^3 a^2 c^2 + 54 o^3 a^3 g^3 d^2 c^2 \\
& - 243 o^3 a^3 g^3 a^2 c^2 - 243 o^3 a^3 i^3 a^2 a^2 c^3 - 9 o^3 a^3 g^3 i^3 - 36 o^3 a^3 g^3 d^2 \\
& + 81 o^3 a^3 g^3 a^2 i^2 - 729 o^3 a^3 i^3 a^2 a^2 + 27 o^3 a^3 i^3 c^2 g^3 + 18 o^3 a^3 g^3 d^2 c^3 \\
& - 18 o^3 a^3 g^3 d^3 i^2 + 27 o^3 a^3 a^2 c^2 g^3 + 162 o^3 a^3 d^2 i^2 - 27 o^3 a^3 j^3 a^2 \\
& + 18 r^2 g^3 a^3 + 54 o^3 a^3 g^3 d^2 a^2 c^3 + 18 o^3 a^3 j^3 g^3 h^3 - 18 o^3 a^3 j^3 c^3 \\
& - 18 o^3 a^3 g^3 c^2 p^3 + 3 p^3 a^3 c^2 g^3 + 54 p^3 a^3 d^2 a^2 c^3 - 27 o^3 a^3 p^3 i^2 \\
& - 18 o^3 a^3 g^3 d^2 i^3 + 54 o^3 a^3 s^3 + 54 o^3 a^3 c^3 i^3 + 81 o^3 a^3 a^2 i^3 + 108 o^3 a^3 d^2 c^3 \\
& - 162 p^3 a^3 q^3 - 27 o^3 a^3 g^3 a^2 s^3 - 729 o^3 a^3 g^3 a^2 a^2 - 81 o^3 a^3 g^3 a^2 c^3 \\
& - 54 o^3 a^3 g^3 a^2 j^2 + 648 o^3 a^3 a^2 d^2 - 3 p^3 a^3 c^3 + 81 o^3 a^3 i^3 i^2 - 2 j^3 g^3 h^3 \\
& + 162 o^3 a^3 g^3 d^2 a^2 - 18 c^2 a^3 g^3 + 18 p^3 g^3 a^2 a^3 o^3 c^3 + 27 p^3 g^3 a^2 a^3 a^2 c^3 \\
& - 9 p^3 a^3 a^2 o^3 - 27 p^3 a^3 a^2 c^3 - 54 p^3 g^3 a^2 r^3 a^3 + 6 p^3 a^3 g^3 h^3 - 6 p^3 a^3 o^3 c^3 \\
& + 54 p^3 a^3 d^2 a^2 o^3 - 9 p^3 a^3 a^2 c^3 + 162 p^3 a^3 d^2 a^2 c^3 + 36 p^3 a^3 d^2 o^3 c^3 \\
& + 54 p^3 a^3 a^2 a^2 h^3 + 36 p^3 a^3 c^3 h^3 + 27 p^3 a^3 c^2 c^3 + 108 p^3 a^3 c^2 a^2 \\
& - 90 p^3 g^3 c^2 a^3 d^2 + 27 p^3 g^3 a^2 a^3 c^2 c^3 - 54 p^3 g^3 a^2 a^3 i^2 + 9 p^3 g^3 a^2 a^3 c^3 \\
& - 27 p^3 g^3 c^2 i^3 a^3 - 72 p^3 g^3 d^2 h^3 a^3 + j^3 g^3 c^3 + 27 p^3 g^3 a^2 a^3 a^2 o^3
\end{aligned}$$

$$\begin{aligned}
& + 81 p_3 g_3 a_2 a_3 a l^2 c_3 - 9 p_3 a_2 a_3 c l g_3^2 - 18 p_3 a_2 a_3 g_3^2 h_3 + 108 p_3 i_3 a_3^3 c l c_3 \\
& - 36 p_3 g_3 i_3 a_3^2 h_3 + 54 p_3 a_3^3 h_3 c_2 g_3 - 486 p_3 a_3^4 h_3 a_2 c l - 1458 p_3 a_3^3 h_3 a_2 a l^2 \\
& - 162 p_3 a_3^3 h_3 a_2 c_3^2 + 108 p_3 a_3^3 h_3 d l c_3 + 648 p_3 a_3^3 h_3 a l d l + 162 p_3 a_3^3 h_3 a l i_3 \\
& + 162 p_3 a_3^4 h_3 i l - 162 p_3 a_3^3 c l a_2 c_3^2 + 648 p_3 a_3^3 c l a l d l - 1458 p_3 a_3^3 c l a_2 a l^2 \\
& + 162 p_3 a_3^3 c l a l i_3 - 486 p_3 a_3^3 h_3 a_2 a l c_3 - 486 p_3 a_3^3 c l a_2 a l c_3 + 18 p_3 a_3^2 d l c_3^3 \\
& + 108 p_3 a_3^3 d_3 c l^2 + 162 p_3 a_3^3 d l c l c_3 - 486 p_3 a_3^4 a_2 c l^2 + 108 p_3 a_3^3 h_3 d_3 c l \\
& + 108 p_3 a_3^3 h_3 c_3 i_3 + 18 c l s_3 a_3^2 g_3^2 + 18 j l h_3 a_3^2 g_3^2 + 36 d l r_3 a_3^2 g_3^2) / (9 a_3^2 g_3^2)
\end{aligned}$$

> **elimsolve (tmp1,r2) ;**

$$\{ 18 g_3^3 a_3^2 \neq 0 \}$$

r2 is set to:

$$\begin{aligned}
& - (-j_3 g_3^3 c l - 72 c_2 a_3^2 g_3^2 d_3 c l + 81 c_2 a_3^3 g_3^2 a_2 c l + 243 c_2 a_3^2 g_3^2 a_2 a l^2 \\
& + 27 c_2 a_3^2 g_3^2 a_2 c_3^2 - 54 c_2 a_3^2 g_3^2 c_3 i_3 - 54 c_2 a_3^2 g_3^2 a l i_3 - 216 c_2 a_3^2 g_3^2 a l d l \\
& - 162 a_3^4 c_3^2 d l i l + 81 c_2 a_3^2 g_3^2 a_2 a l c_3 + 324 d_3 g_3 a_3^2 h_3 a_2 a l c_3 - 24 j_3 g_3^2 a_3 c_3 h_3 \\
& - 18 j_3 g_3^2 a_3 a l h_3 - 36 j_3 g_3^2 a_3 c l a l - 15 j_3 g_3^2 a_3 c l c_3 - 54 d_2 a_3 g_3^2 a l^2 c_3 \\
& - 18 d_2 a_3 g_3^2 a l o_3 - 12 d_2 a_3 g_3^2 o_3 c_3 - 18 d_2 a_3 g_3^2 a l c_3^2 - 18 d_2 a_3^2 g_3^2 c l c_3 \\
& - 72 c_2 a_3^2 g_3^2 d l c_3 - 6 d_2 a_3 g_3^2 c_3^3 + 12 d_2 a_3 g_3^3 h_3 + 6 d_2 a_3 g_3^3 c l - 54 c_2 a_3^3 g_3^2 i l \\
& - 6 j_3 g_3^3 a_3 u_2 - 72 d_3^2 g_3 a_3^2 c l^2 + 3 j_3 g_3^2 a l o_3 + 9 j_3 g_3^2 a l^2 c_3 + 2 j_3 g_3^2 o_3 c_3 \\
& + 3 j_3 g_3^2 a l c_3^2 + 36 d l a_3^2 g_3^2 i l + 36 c l a_3^2 g_3^2 j l + 18 i l a_3^2 g_3^2 i_3 - 729 a_3^3 a l^2 c_3 i_3^2 \\
& - 243 a_3^3 a l c_3^2 i_3^2 + 2916 a_3^3 a l^3 c_3 j l + 1458 a_3^3 a l^3 c_3 s_3 + 1458 a_3^3 a l^2 c_3^2 j l \\
& + 729 a_3^3 a l^2 c_3^2 s_3 + 324 a_3^3 a l c_3^3 j l + 162 a_3^3 a l c_3^3 s_3 - 972 a_3^3 a l c_3^2 d l^2 \\
& - 2916 a_3^3 a l^2 c_3 d l^2 + 162 a_3^4 c_3^2 c l s_3 + 324 a_3^4 c_3^2 c l j l + 162 a_3^3 c_3^4 d l a_2 \\
& - 81 a_3^3 c_3^2 j l o_3 - 162 a_3^3 c_3^3 d l i_3 + 54 a_3^3 c_3^3 j_3 c l + 81 a_3^3 c_3^4 i_3 a_2 - 81 a_3^4 c_3^2 i_3 i l \\
& - 12 d_3 g_3 a_3 d l c_3^3 - 36 d_3 g_3 r_3 a_3^2 o_3 + 162 d_3 g_3 a_3^3 a_2 c l^2 + 486 d_3 g_3 i l a_3^2 a l^2 \\
& + 36 d_3 g_3 r_3 a_3^2 c_3^2 + 108 d_3 g_3 p_3 a_3^2 q_3 + 108 d_3 g_3 r_3 a_3^3 c l + 324 d_3 g_3 r_3 a_3^2 a l^2 \\
& + 54 d_3 g_3 i l a_3^2 c_3^2 + 162 d_3 g_3 a_3^2 c l a_2 a l c_3 + 12 d_3 g_3^2 c l a_3 d l + 24 d_3 g_3^2 d l h_3 a_3 \\
& - 108 d_3 g_3 a_3^3 h_3 i l - 108 d_3 g_3 a_3 d l a l^2 c_3 - 36 d_3 g_3 a_3 d l a l o_3 \\
& - 36 d_3 g_3 a_3 d l a l c_3^2 + 162 d_3 g_3 i l a_3^2 a l c_3 - 72 d_3^2 g_3 a_3^2 h_3 c l - 36 d_3 g_3^2 a_3^2 h_3 c_2 \\
& + 108 d_3 g_3 r_3 a_3^2 a l c_3 - 24 d_3 g_3 a_3 d l o_3 c_3 - 432 d_3 g_3 a_3^2 c l a l d l \\
& - 108 d_3 g_3 i_3 a_3^2 c l c_3 + 6561 a_3^3 a l^4 i_3 a_2 - 4374 a_3^3 a l^3 d l i_3 - 108 d_3 g_3 a_3^2 c l a l i_3 \\
& + 54 d_3 g_3 a_3^2 c l a_2 c_3^2 + 13122 a_3^3 a l^4 d l a_2 + 486 d_3 g_3 a_3^2 c l a_2 a l^2 \\
& - 108 d_3 g_3 a_3^2 h_3 a l i_3 - 72 d_3 g_3 a_3^2 h_3 d l c_3 - 72 d_3 g_3 a_3^2 h_3 c_3 i_3 \\
& - 180 d_3 g_3 a_3^2 d l c l c_3 - 432 d_3 g_3 a_3^2 h_3 a l d l + 324 d_3 g_3 a_3^3 h_3 a_2 c l \\
& + 108 d_3 g_3 a_3^2 h_3 a_2 c_3^2 + 972 d_3 g_3 a_3^2 h_3 a_2 a l^2 + 243 a_3^2 a l^2 g_3 c_2 p_3 \\
& - 162 a_3^2 a l^2 j_3 g_3 h_3 - 729 a_3^2 a l^3 g_3 a_2 i_3 - 2916 a_3^2 a l^3 g_3 a_2 d l - 18 a_3^2 c_3^2 j_3 g_3 h_3 \\
& + 27 a_3^2 c_3^2 g_3 c_2 p_3 - 90 a_3^2 c_3^2 g_3 d l i_3 + 54 a_3^2 c_3^3 g_3 a_2 d l + 189 a_3^2 a l c_3^2 g_3 j l \\
& + 405 a_3^2 a l^2 c_3 g_3 s_3 + 135 a_3^2 a l c_3^2 g_3 s_3 + 162 a_3^2 a l^2 c_3 j_3 o_3 - 108 a_3^2 a l c_3^3 g_3 d_2
\end{aligned}$$

$$\begin{aligned}
& + 486 a^3^2 a l c^3^3 g^3 a^2^2 - 972 a^3^2 a l^3 c^3 g^3 d^2 + 567 a^3^2 a l^2 c^3 g^3 j l \\
& + 4374 a^3^2 a l^3 c^3 g^3 a^2^2 - 324 a^3^2 a l c^3 g^3 d l^2 + 2187 a^3^2 a l^2 c^3^2 g^3 a^2^2 \\
& - 27 a^3^2 a l c^3 g^3 i^3^2 + 1458 a^3^4 a l^2 c l s^3 - 486 a^3^2 a l^2 c^3^2 g^3 d^2 + 54 a^3^2 a l c^3^2 j^3 o^3 \\
& + 162 a^3^3 a l c^3^2 j^3 c l - 2916 a^3^3 a l^2 c^3 d l i^3 - 972 a^3^3 a l c^3^2 d l i^3 + 972 a^3^3 a l c^3^3 d l a^2 \\
& + 8748 a^3^3 a l^3 c^3 d l a^2 + 4374 a^3^3 a l^3 c^3 i^3 a^2 + 486 a^3^3 a l c^3^3 i^3 a^2 \\
& + 162 a^3^2 a l^2 g^3 d l i^3 - 27 a^3^3 c^3^2 p^3 i l - 81 a^3^3 c^3^2 o^3 s^3 - 729 a^3^3 a l^2 j l o^3 \\
& + 2916 a^3^4 a l^2 c l j l - 243 a^3^3 a l^2 p^3 i l - 729 a^3^3 a l^2 o^3 s^3 + 27 o^3^2 a^3^3 j l \\
& - 243 a^3^4 c l j l o^3 + 81 a^3^4 c l^2 j^3 c^3 - 1458 a^3^4 a l^2 d l i l + 2187 a^3^3 a l^2 c^3^2 i^3 a^2 \\
& - 729 a^3^4 a l^2 i^3 i l - 486 a^3^4 a l c^3 d l i l - 243 a^3^3 a l c^3 j l o^3 + 972 a^3^4 a l c^3 c l j l \\
& + 486 a^3^4 a l c^3 c l s^3 + 729 a^3^5 c l^2 i^3 a^2 + 243 a^3^5 c l^2 s^3 - 324 a^3^4 c l^2 d l d^3 \\
& + 486 a^3^4 c^3^2 i^3 a^2 c l - 162 a^3^4 c l^2 i^3 d^3 - 108 a^3^3 c^3^2 d l d^3 c l - 243 a^3^4 a l c^3 i^3 i l \\
& + 729 a^3^4 c l^2 g^3 a^2^2 + 486 a^3^5 c l^2 j l - 81 a^3^3 a l c^3 p^3 i l + 4374 a^3^3 a l^2 c^3^2 d l a^2 \\
& - 54 a^3^3 c^3^2 d l c^2 g^3 - 486 a^3^5 c l d l i l + 27 a^3^3 c^3^4 s^3 - 81 a^3^3 c^3^2 g^3 a^2 i l \\
& - 243 a^3^5 c l i^3 i l + 486 a^3^3 c^3^2 g^3 a^2^2 c l - 243 a^3^3 a l c^3 o^3 s^3 - 1944 a^3^4 c l a l d l^2 \\
& - 324 a^3^4 c l d l^2 c^3 + 54 a^3^3 c^3^4 j l + 972 a^3^4 c^3^2 d l a^2 c l - 243 a^3^4 c l a l i^3^2 \\
& - 54 a^3^3 c^3^3 i^3^2 - 162 a^3^4 c l c^3 i^3^2 + 81 a^3^4 c l p^3 i l - 108 a^3^3 c^3^3 d l^2 - 243 a^3^4 c l o^3 s^3 \\
& + 1458 a^3^5 c l^2 d l a^2 - 972 a^3^3 a l^2 d l d^3 c l - 486 a^3^3 a l^2 d l c^2 g^3 - 243 a^3^3 a l^2 i^3 c^2 g^3 \\
& - 729 a^3^3 a l^2 g^3 a^2 i l - 81 a^3^2 a l c^3^2 g^3 a^2 i^3 - 54 a^3^2 a l c^3 j^3 g^3 h^3 \\
& - 972 a^3^3 a l^2 g^3 d^2 c l - 486 a^3^2 a l^2 c^3 g^3 a^2 d l + 4374 a^3^3 a l^2 g^3 a^2^2 c l \\
& - 486 a^3^3 a l^2 i^3 d^3 c l + 486 a^3^3 a l^2 j^3 c l c^3 + 8748 a^3^4 a l^2 d l a^2 c l + 4374 a^3^4 a l^2 i^3 a^2 c l \\
& + 108 a^3^3 c l g^3 d l^2 + 9 a^3^2 c^3^5 j^3 - 162 a^3^4 c l^2 g^3 d^2 - 27 a^3^3 c^3^2 i^3 c^2 g^3 \\
& + 27 a^3^3 c l g^3 i^3^2 - 108 a^3^3 c^3^2 g^3 d^2 c l - 54 a^3^3 c^3^2 i^3 d^3 c l + 81 a^3^2 a l c^3 g^3 c^2 p^3 \\
& - 54 a^3^3 c l j^3 g^3 h^3 + 81 a^3^3 c l j^3 a l o^3 + 54 a^3^3 c l g^3 d^3 i l + 162 a^3^3 c l g^3 a l j l \\
& - 270 a^3^2 a l c^3 g^3 d l i^3 + 135 a^3^3 c l g^3 j l c^3 + 108 a^3^3 c l g^3 c^3 s^3 + 54 a^3^3 c l g^3 d l i^3 \\
& - 162 a^3^2 a l c^3^2 g^3 a^2 d l - 243 a^3^2 a l^2 c^3 g^3 a^2 i^3 - 81 a^3^4 c l i^3 c^2 g^3 \\
& - 162 a^3^4 c l d l c^2 g^3 - 1458 a^3^4 c l d l a l i^3 + 135 a^3^3 c l g^3 c^2 p^3 - 486 a^3^4 c l d l c^3 i^3 \\
& + 81 a^3^3 c l g^3 a l s^3 - 243 a^3^4 c l g^3 a^2 i l + 27 a^3^3 c l j^3 o^3 c^3 + 243 a^3^2 a l^2 c^3^3 j^3 \\
& + 1458 a^3^3 a l c^3 g^3 a^2^2 c l - 324 a^3^3 a l c^3 g^3 d^2 c l - 972 a^3^3 c l g^3 a^2 a l d l \\
& + 2916 a^3^4 a l c^3 d l a^2 c l + 1458 a^3^4 a l c^3 i^3 a^2 c l - 27 c^3 a^3^2 g^3 j l o^3 \\
& - 324 a^3^3 a l c^3 d l d^3 c l + 81 a^3^2 a l^2 g^3 i^3^2 + 729 a^3^2 a l^4 j^3 c^3 + 2187 a^3^3 a l^4 s^3 \\
& + 243 a^3^2 a l^3 j^3 o^3 + 4374 a^3^3 a l^4 j l - 1458 a^3^2 a l^4 g^3 d^2 - 729 a^3^3 a l^3 i^3^2 \\
& + 18 c^3^2 a^3^2 g^3 j^3 c l + 486 a^3^2 a l^3 g^3 j l + 6561 a^3^2 a l^4 g^3 a^2^2 - 5832 a^3^3 a l^3 d l^2 \\
& + 243 a^3^2 a l^3 g^3 s^3 + 9 a^3^2 c^3^3 j^3 o^3 - 243 a^3^3 c l g^3 a^2 a l i^3 + 162 a^3^3 c l g^3 a^2 d l c^3 \\
& - 162 a^3^3 a l c^3 d l c^2 g^3 - 162 a^3^3 a l c^3 i^3 d^3 c l - 36 a^3^2 c^3^2 g^3 d l^2 - 27 a^3^2 c^3^2 g^3 i^3^2 \\
& - 81 a^3^3 a l c^3 i^3 c^2 g^3 + 486 a^3^2 a l^3 c^3^2 j^3 + 54 a^3^2 a l c^3^4 j^3 - 243 a^3^3 a l c^3 g^3 a^2 i l
\end{aligned}$$

$$\begin{aligned}
& -108 c3 a3^3 g3 d1 i1 + 54 c3^2 a3 g3 j3 a1^2 + 18 c3^3 a3 g3 j3 a1 + 12 c3^2 a3 g3 j3 o3 \\
& -18 a3^2 c3^4 g3 d2 + 81 a3^2 c3^4 g3 a2^2 + 36 a3^2 c3^3 g3 s3 + 45 a3^2 c3^3 g3 j1 \\
& + 324 a3^2 a1^2 g3 d1^2 - 54 c3 a3^3 g3 i3 i1 - 9 c3 a3^2 g3 p3 i1 + 6 c3^4 a3 g3 j3 \\
& - 54 c3 a3^2 g3 o3 s3 + 36 i3 a3^2 g3^2 r3 + 18 c3 a3 g3 j3 a1 o3 + 36 s3 a3^2 g3^2 h3 \\
& - 486 o3 a3^4 d1 a2 c1 + 54 o3 a3^3 i3 d3 c1 - 486 o3 a3^3 d1 a2 a1 c3 + 54 o3 a3^2 g3 a2 d3 c1 \\
& + 54 o3 a3^2 g3 a2 c3 i3 - 81 o3 a3^3 i3 a2 c3^2 - 1458 o3 a3^3 d1 a2 a1^2 \\
& + 54 o3 a3^2 g3 a2 d1 c3 + 54 o3 a3^3 d1 c2 g3 + 108 o3 a3^3 d1 d3 c1 + 81 o3 a3^2 g3 a2 a1 i3 \\
& - 243 o3 a3^2 g3 a2^2 a1 c3 - 162 o3 a3^3 d1 a2 c3^2 + 324 o3 a3^2 g3 a2 a1 d1 \\
& + 486 o3 a3^3 d1 a1 i3 + 162 o3 a3^3 d1 c3 i3 - 243 o3 a3^4 i3 a2 c1 + 54 o3 a3^3 g3 d2 c1 \\
& - 243 o3 a3^3 g3 a2^2 c1 - 243 o3 a3^3 i3 a2 a1 c3 - 9 o3 a3^2 g3 i3^2 - 36 o3 a3^2 g3 d1^2 \\
& + 81 o3 a3^3 g3 a2 i1 - 729 o3 a3^3 i3 a2 a1^2 + 27 o3 a3^3 i3 c2 g3 + 18 o3 a3^2 g3 d2 c3^2 \\
& - 18 o3 a3^2 g3 d3 i1 + 27 o3 a3^2 a2 c2 g3^2 + 162 o3 a3^4 d1 i1 - 27 o3^2 a3^2 j3 a1 \\
& + 54 o3 a3^2 g3 d2 a1 c3 + 18 o3 a3^2 j3 g3 h3 - 18 o3^2 a3^2 j3 c3 - 18 o3 a3^2 g3 c2 p3 \\
& + 3 p3^2 a3 c1 g3 + 54 p3 a3^2 d1 a1 c3^2 - 27 o3 a3^3 p3 i1 - 18 o3 a3^2 g3 d1 i3 + 54 o3^2 a3^3 s3 \\
& + 54 o3 a3^3 c3 i3^2 + 81 o3 a3^3 a1 i3^2 + 108 o3 a3^3 d1^2 c3 - 162 p3^2 a3^3 q3 \\
& - 27 o3 a3^2 g3 a1 s3 - 729 o3 a3^2 g3 a2^2 a1^2 - 81 o3 a3^2 g3 a2^2 c3^2 - 54 o3 a3^2 g3 a1 j1 \\
& + 648 o3 a3^3 a1 d1^2 - 3 p3^2 a3 c3^3 + 81 o3 a3^4 i3 i1 - 2 j3 g3^3 h3 + 162 o3 a3^2 g3 d2 a1^2 \\
& - 18 c2^2 a3^2 g3^3 + 18 p3 g3 a2 a3 o3 c3 + 27 p3 g3 a2 a3 a1 c3^2 - 9 p3^2 a3 a1 o3 \\
& - 27 p3^2 a3 a1^2 c3 - 54 p3 g3 a1 r3 a3^2 + 6 p3^2 a3 g3 h3 - 6 p3^2 a3 o3 c3 \\
& + 54 p3 a3^2 d1 a1 o3 - 9 p3^2 a3 a1 c3^2 + 162 p3 a3^2 d1 a1^2 c3 + 36 p3 a3^2 d1 o3 c3 \\
& + 54 p3^2 a3^2 a1 h3 + 36 p3^2 a3^2 c3 h3 + 27 p3^2 a3^2 c1 c3 + 108 p3^2 a3^2 c1 a1 \\
& - 90 p3 g3 c1 a3^2 d1 + 27 p3 g3 a2 a3^2 c1 c3 - 54 p3 g3 a1 a3^2 i1 + 9 p3 g3 a2 a3 c3^3 \\
& - 27 p3 g3 c1 i3 a3^2 - 72 p3 g3 d1 h3 a3^2 + j3 g3^2 c3^3 + 27 p3 g3 a2 a3 a1 o3 \\
& + 81 p3 g3 a2 a3 a1^2 c3 - 9 p3 a2 a3 c1 g3^2 - 18 p3 a2 a3 g3^2 h3 + 108 p3 i3 a3^3 c1 c3 \\
& - 36 p3 g3 i3 a3^2 h3 + 54 p3 a3^3 h3 c2 g3 - 486 p3 a3^4 h3 a2 c1 - 1458 p3 a3^3 h3 a2 a1^2 \\
& - 162 p3 a3^3 h3 a2 c3^2 + 108 p3 a3^3 h3 d1 c3 + 648 p3 a3^3 h3 a1 d1 + 162 p3 a3^3 h3 a1 i3 \\
& + 162 p3 a3^4 h3 i1 - 162 p3 a3^3 c1 a2 c3^2 + 648 p3 a3^3 c1 a1 d1 - 1458 p3 a3^3 c1 a2 a1^2 \\
& + 162 p3 a3^3 c1 a1 i3 - 486 p3 a3^3 h3 a2 a1 c3 - 486 p3 a3^3 c1 a2 a1 c3 + 18 p3 a3^2 d1 c3^3 \\
& + 108 p3 a3^3 d3 c1^2 + 162 p3 a3^3 d1 c1 c3 - 486 p3 a3^4 a2 c1^2 + 108 p3 a3^3 h3 d3 c1 \\
& + 108 p3 a3^3 h3 c3 i3 + 18 c1 s3 a3^2 g3^2 + 18 j1 h3 a3^2 g3^2 + 36 d1 r3 a3^2 g3^2) / (18 g3^3 a3^2)
\end{aligned}$$

> **tmp1 := cpcoeff (x1\*T);**

$$\begin{aligned}
tmp1 := & (3 p3 a3 j3 c3^3 - 6 i3 g3^2 a3 s3 + 3 p3 a3 g3 j1 c3 + 9 p3 a3 g3 a1 s3 \\
& + 6 p3 a3 g3 d1 i3 + 18 p3 a3 g3 a1 j1 + 27 p3 a3 g3 a2^2 c3^2 + 243 p3 a3 g3 a2^2 a1^2 \\
& + 6 p3 a3 g3 c3 s3 - 9 p3 a3 a2 c2 g3^2 - 6 p3 a3 g3 d2 c3^2 - 54 p3 a3 g3 d2 a1^2
\end{aligned}$$

$$\begin{aligned}
& + 18 p^3 a^3 r^3 + 9 p^3 a^3 j^3 a l o^3 - 36 p^3 a^3 d l^2 c^3 - 27 p^3 a^3 a l i^3 - 18 p^3 a^3 c^3 i^3 \\
& - 18 p^3 a^3 o^3 s^3 + 9 p^3 a^3 j^3 a l c^3 + 6 p^3 a^3 j^3 o^3 c^3 - 6 p^3 a^3 j^3 g^3 h^3 \\
& + 27 p^3 a^3 j^3 a l^2 c^3 - 18 p^3 a^3 g^3 a^2 c^3 i^3 - 18 p^3 a^3 g^3 a^2 d^3 c l - 18 p^3 a^3 g^3 d^2 c l \\
& - 18 p^3 a^3 g^3 a^2 d l c^3 + 162 p^3 a^3 d l a^2 a l c^3 + 81 p^3 a^3 i^3 a^2 a l c^3 \\
& - 18 p^3 a^3 g^3 d^2 a l c^3 + 81 p^3 a^3 g^3 a^2 a l c^3 + 81 p^3 a^3 g^3 a^2 c l - 27 p^3 a^3 g^3 a^2 a l i^3 \\
& + 9 p^3 a^3 i^3 l - 18 p^3 a^3 d l c^2 g^3 + 27 p^3 a^3 i^3 a^2 c^3 + 243 p^3 a^3 i^3 a^2 a l^2 \\
& - 18 p^3 a^3 i^3 d^3 c l - 36 p^3 a^3 d l d^3 c l - 9 p^3 a^3 i^3 c^2 g^3 - 27 p^3 a^3 g^3 a^2 i l \\
& - 108 p^3 a^3 g^3 a^2 a l d l - 216 p^3 a^3 a l d l^2 - 162 p^3 a^3 d l a l i^3 - 54 p^3 a^3 d l c^3 i^3 \\
& + 54 p^3 a^3 d l a^2 c^3 + 486 p^3 a^3 d l a^2 a l^2 + 12 p^3 a^3 g^3 d l^2 + 27 p^3 a^3 a l c^3 s^3 \\
& + 9 p^3 a^3 j^3 c l c^3 + 162 p^3 a^3 d l a^2 c l + 81 p^3 a^3 i^3 a^2 c l + 162 p^3 a^3 a l^2 j l \\
& + 81 p^3 a^3 a l^2 s^3 + 3 p^3 a^3 g^3 c^2 + 3 p^3 a^3 g^3 i^3 - 54 p^3 a^3 d l i l - 27 p^3 a^3 i^3 i l \\
& - 9 p^3 a^3 j l o^3 + 54 p^3 a^3 c l j l + 27 p^3 a^3 c l s^3 + 18 p^3 a^3 c^3 j l + 9 p^3 a^3 c^3 s^3 \\
& + 54 p^3 a^3 a l c^3 j l - 6 d l s^3 g^3 a^3 - 3 j^3 i l g^3 a^3 - 162 d^2 a^3 g^3 a^2 a l^2 \\
& - 54 d^2 a^3 g^3 a^2 c l + 12 d^2 a^3 g^3 d^3 c l + 72 d^2 a^3 g^3 a l d l + 18 d^2 a^3 g^3 a l i^3 \\
& + 12 d^2 a^3 g^3 d l c^3 + 12 d^2 a^3 g^3 c^3 i^3 - 18 d^2 a^3 g^3 a^2 c^3 + 3 j^2 g^3 a^3 c^3 \\
& + 27 j^2 g^3 a^3 a l^2 + 9 j^2 g^3 a^3 c l + 18 d^2 a^3 g^3 i l + 6 d^2 a^3 g^3 c^2 + 9 j^2 g^3 a^3 a l c^3 \\
& - 54 d^2 a^3 g^3 a^2 a l c^3 + 24 d^3 g^3 a^3 d l^2 c^3 + 18 d^3 g^3 a^3 a l i^3 + 12 d^3 g^3 a^3 c^3 i^3 \\
& - 12 d^3 g^3 p^3 a^3 r^3 + 12 d^3 g^3 o^3 a^3 s^3 - 108 d^3 g^3 a^3 d l a^2 a l c^3 \\
& - 54 d^3 g^3 a^3 i^3 a^2 a l c^3 - 6 d^3 g^3 j^3 a l c^3 - 4 d^3 g^3 j^3 o^3 c^3 - 18 d^3 g^3 a^3 i^3 a^2 c^3 \\
& - 162 d^3 g^3 a^3 i^3 a^2 a l^2 + 12 d^3 g^3 a^3 i^3 c l - 324 d^3 g^3 a^3 d l a^2 a l^2 + 6 d^3 g^3 a^3 i^3 c^2 \\
& - 18 d^3 g^3 j^3 a l^2 c^3 - 6 d^3 g^3 j^3 a l o^3 + 36 d^3 g^3 d l a^3 i l + 18 d^3 g^3 i^3 a^3 i l \\
& + 144 d^3 g^3 a^3 a l d l^2 - 54 d^3 g^3 i^3 a^2 a^3 c l + 108 d^3 g^3 a^3 d l a l i^3 + 36 d^3 g^3 a^3 d l c^3 i^3 \\
& - 36 d^3 g^3 a^3 d l a^2 c^3 + 12 d^3 g^3 a^3 d l c^2 - 54 d^3 g^3 a^3 a l^2 s^3 - 36 d^3 g^3 a^3 a l c^3 j l \\
& - 18 d^3 g^3 a^3 a l c^3 s^3 - 6 d^3 g^3 j^3 a^3 c l c^3 - 108 d^3 g^3 d l a^2 a^3 c l + 24 d^3 g^3 a^3 d l c l \\
& - 36 d^3 g^3 a^3 c l j l - 18 d^3 g^3 a^3 c l s^3 - 12 d^3 g^3 a^3 c^3 j l - 6 d^3 g^3 a^3 c^3 s^3 \\
& - 108 d^3 g^3 a^3 a l^2 j l - 12 d l g^3 a^3 j l + 2 d^3 g^3 j^3 c l + 4 d^3 g^3 j^3 h^3 - 2 d^3 g^3 j^3 c^3 \\
& + 6 d^3 g^3 j l o^3 a^3 - 3 j l i^3 g^3 a^3 - 3 s^2 g^3 a^3) / (3 g^3 a^3)
\end{aligned}$$

> **elimsolve (tmp1,s2);**

$$\{-3 g^3 a^3 \neq 0\}$$

s2 is set to:

$$\begin{aligned}
& (3 p^3 a^3 j^3 c^3 - 6 i^3 g^3 a^3 s^3 + 3 p^3 a^3 g^3 j l c^3 + 9 p^3 a^3 g^3 a l s^3 + 6 p^3 a^3 g^3 d l i^3 \\
& + 18 p^3 a^3 g^3 a l j l + 27 p^3 a^3 g^3 a^2 c^3 + 243 p^3 a^3 g^3 a^2 a l^2 + 6 p^3 a^3 g^3 c^3 s^3 \\
& - 9 p^3 a^3 a^2 c^2 g^3 - 6 p^3 a^3 g^3 d^2 c^3 - 54 p^3 a^3 g^3 d^2 a l^2 + 18 p^3 a^3 r^3 \\
& + 9 p^3 a^3 j^3 a l o^3 - 36 p^3 a^3 d l^2 c^3 - 27 p^3 a^3 a l i^3 - 18 p^3 a^3 c^3 i^3 - 18 p^3 a^3 o^3 s^3 \\
& + 9 p^3 a^3 j^3 a l c^3 + 6 p^3 a^3 j^3 o^3 c^3 - 6 p^3 a^3 j^3 g^3 h^3 + 27 p^3 a^3 j^3 a l^2 c^3 \\
& - 18 p^3 a^3 g^3 a^2 c^3 i^3 - 18 p^3 a^3 g^3 a^2 d^3 c l - 18 p^3 a^3 g^3 d^2 c l - 18 p^3 a^3 g^3 a^2 d l c^3
\end{aligned}$$

$$\begin{aligned}
& + 162 p_3 a_3^2 d_1 a_2 a_1 c_3 + 81 p_3 a_3^2 i_3 a_2 a_1 c_3 - 18 p_3 a_3 g_3 d_2 a_1 c_3 \\
& + 81 p_3 a_3 g_3 a_2^2 a_1 c_3 + 81 p_3 a_3^2 g_3 a_2^2 c_1 - 27 p_3 a_3 g_3 a_2 a_1 i_3 + 9 p_3^2 a_3^2 i_1 \\
& - 18 p_3 a_3^2 d_1 c_2 g_3 + 27 p_3 a_3^2 i_3 a_2 c_3^2 + 243 p_3 a_3^2 i_3 a_2 a_1^2 - 18 p_3 a_3^2 i_3 d_3 c_1 \\
& - 36 p_3 a_3^2 d_1 d_3 c_1 - 9 p_3 a_3^2 i_3 c_2 g_3 - 27 p_3 a_3^2 g_3 a_2 i_1 - 108 p_3 a_3 g_3 a_2 a_1 d_1 \\
& - 216 p_3 a_3^2 a_1 d_1^2 - 162 p_3 a_3^2 d_1 a_1 i_3 - 54 p_3 a_3^2 d_1 c_3 i_3 + 54 p_3 a_3^2 d_1 a_2 c_3^2 \\
& + 486 p_3 a_3^2 d_1 a_2 a_1^2 + 12 p_3 a_3 g_3 d_1^2 + 27 p_3 a_3^2 a_1 c_3 s_3 + 9 p_3 a_3^2 j_3 c_1 c_3 \\
& + 162 p_3 a_3^3 d_1 a_2 c_1 + 81 p_3 a_3^3 i_3 a_2 c_1 + 162 p_3 a_3^2 a_1^2 j_1 + 81 p_3 a_3^2 a_1^2 s_3 \\
& + 3 p_3^2 a_3 g_3 c_2 + 3 p_3 a_3 g_3 i_3^2 - 54 p_3 a_3^3 d_1 i_1 - 27 p_3 a_3^3 i_3 i_1 - 9 p_3 a_3^2 j_1 o_3 \\
& + 54 p_3 a_3^3 c_1 j_1 + 27 p_3 a_3^3 c_1 s_3 + 18 p_3 a_3^2 c_3^2 j_1 + 9 p_3 a_3^2 c_3^2 s_3 + 54 p_3 a_3^2 a_1 c_3 j_1 \\
& - 6 d_1 s_3 g_3^2 a_3 - 3 j_3 i_1 g_3^2 a_3 - 162 d_2 a_3 g_3^2 a_2 a_1^2 - 54 d_2 a_3^2 g_3^2 a_2 c_1 \\
& + 12 d_2 a_3 g_3^2 d_3 c_1 + 72 d_2 a_3 g_3^2 a_1 d_1 + 18 d_2 a_3 g_3^2 a_1 i_3 + 12 d_2 a_3 g_3^2 d_1 c_3 \\
& + 12 d_2 a_3 g_3^2 c_3 i_3 - 18 d_2 a_3 g_3^2 a_2 c_3^2 + 3 j_2 g_3^2 a_3 c_3^2 + 27 j_2 g_3^2 a_3 a_1^2 \\
& + 9 j_2 g_3^2 a_3^2 c_1 + 18 d_2 a_3^2 g_3^2 i_1 + 6 d_2 a_3 g_3^3 c_2 + 9 j_2 g_3^2 a_3 a_1 c_3 \\
& - 54 d_2 a_3 g_3^2 a_2 a_1 c_3 + 24 d_3 g_3 a_3 d_1^2 c_3 + 18 d_3 g_3 a_3 a_1 i_3^2 + 12 d_3 g_3 a_3 c_3 i_3^2 \\
& - 12 d_3 g_3 p_3 a_3 r_3 + 12 d_3 g_3 o_3 a_3 s_3 - 108 d_3 g_3 a_3 d_1 a_2 a_1 c_3 \\
& - 54 d_3 g_3 a_3 i_3 a_2 a_1 c_3 - 6 d_3 g_3 j_3 a_1 c_3^2 - 4 d_3 g_3 j_3 o_3 c_3 - 18 d_3 g_3 a_3 i_3 a_2 c_3^2 \\
& - 162 d_3 g_3 a_3 i_3 a_2 a_1^2 + 12 d_3^2 g_3 a_3 i_3 c_1 - 324 d_3 g_3 a_3 d_1 a_2 a_1^2 + 6 d_3 g_3^2 a_3 i_3 c_2 \\
& - 18 d_3 g_3 j_3 a_1^2 c_3 - 6 d_3 g_3 j_3 a_1 o_3 + 36 d_3 g_3 d_1 a_3^2 i_1 + 18 d_3 g_3 i_3 a_3^2 i_1 \\
& + 144 d_3 g_3 a_3 a_1 d_1^2 - 54 d_3 g_3 i_3 a_2 a_3^2 c_1 + 108 d_3 g_3 a_3 d_1 a_1 i_3 + 36 d_3 g_3 a_3 d_1 c_3 i_3 \\
& - 36 d_3 g_3 a_3 d_1 a_2 c_3^2 + 12 d_3 g_3^2 a_3 d_1 c_2 - 54 d_3 g_3 a_3 a_1^2 s_3 - 36 d_3 g_3 a_3 a_1 c_3 j_1 \\
& - 18 d_3 g_3 a_3 a_1 c_3 s_3 - 6 d_3 g_3 j_3 a_3 c_1 c_3 - 108 d_3 g_3 d_1 a_2 a_3^2 c_1 + 24 d_3^2 g_3 a_3 d_1 c_1 \\
& - 36 d_3 g_3 a_3^2 c_1 j_1 - 18 d_3 g_3 a_3^2 c_1 s_3 - 12 d_3 g_3 a_3 c_3^2 j_1 - 6 d_3 g_3 a_3 c_3^2 s_3 \\
& - 108 d_3 g_3 a_3 a_1^2 j_1 - 12 d_1 g_3^2 a_3 j_1 + 2 d_3 g_3^2 j_3 c_1 + 4 d_3 g_3^2 j_3 h_3 - 2 d_3 g_3 j_3 c_3^3 \\
& + 6 d_3 g_3 j_1 o_3 a_3 - 3 j_1 i_3 g_3^2 a_3) / (3 g_3^3 a_3)
\end{aligned}$$

> **tmp1 := cpccoeff (x1\*x2\*x3\*T);**

$$\begin{aligned}
\text{tmp1} := & 2 (3 c_1^2 a_3^2 - h_3 a_3 o_3 - 9 a_1^3 c_3 - 3 a_1^2 o_3 + 9 a_3 c_1 a_1^2 - a_1 c_3^3 \\
& - 3 a_1^2 c_3^2 + a_3 c_1 c_3^2 - 2 a_1 o_3 c_3 + 2 a_1 g_3 h_3 + a_1 c_1 g_3) / a_3
\end{aligned}$$

> **elimsolve (tmp1,q3);**

$$\{3 g_3 a_3 \neq 0\}$$

q3 is set to:

$$\begin{aligned}
& - (3 c_1^2 a_3^2 - h_3 a_3 o_3 - 9 a_1^3 c_3 - 3 a_1^2 o_3 + 9 a_3 c_1 a_1^2 - a_1 c_3^3 - 3 a_1^2 c_3^2 + a_3 c_1 c_3^2 \\
& - 2 a_1 o_3 c_3 + 2 a_1 g_3 h_3 + a_1 c_1 g_3) / (3 g_3 a_3)
\end{aligned}$$

> **tmp1 := cpccoeff (x1\*x2\*T);**

$$\begin{aligned}
\text{tmp1} := & 2 (27 a_2 a_3^2 c_1 c_3 + 54 a_2 a_3 a_1 c_3^2 + 162 a_2 a_3 a_1^2 c_3 - 3 d_3 a_3 c_1 c_3 \\
& - 18 d_3 a_3 c_1 a_1 + d_3 c_3^3 - 9 i_1 c_3 a_3^2 + 9 a_2 a_3 c_3^3 - 27 a_1 a_3^2 i_1 + 9 c_1 a_3^2 d_1 - d_3 c_1 g_3 \\
& + 3 d_3 a_1 c_3^2 + 2 d_3 o_3 c_3 - 2 d_3 g_3 h_3 + 9 d_3 a_1^2 c_3 + 3 d_3 a_1 o_3 + 3 p_3 a_3 c_1 + 3 p_3 a_3 h_3 \\
& - 3 i_3 a_3 o_3 - 6 i_3 a_3 c_3^2 - 27 i_3 a_3 a_1^2 + 3 g_3 a_3 r_3 - 27 i_3 a_3 a_1 c_3 + 81 a_1 a_2 a_3^2 c_1
\end{aligned}$$

$$-45 a3 a1 d1 c3 - 3 d1 o3 a3 - 9 a3 a1 c2 g3 - 3 a3 c3 c2 g3 + 243 a3 a2 a1^3 - 81 a3 a1^2 d1 - 3 a3 d1 c3^2) / (3 a3)$$

> **elimsolve (tmp1,r3);**

$$\{3 g3 a3 \neq 0\}$$

r3 is set to:

$$-(27 a2 a3^2 c1 c3 + 54 a2 a3 a1 c3^2 + 162 a2 a3 a1^2 c3 - 3 d3 a3 c1 c3 - 18 d3 a3 c1 a1 + d3 c3^3 - 9 i1 c3 a3^2 + 9 a2 a3 c3^3 - 27 a1 a3^2 i1 + 9 c1 a3^2 d1 - d3 c1 g3 + 3 d3 a1 c3^2 + 2 d3 o3 c3 - 2 d3 g3 h3 + 9 d3 a1^2 c3 + 3 d3 a1 o3 + 3 p3 a3 c1 + 3 p3 a3 h3 - 3 i3 a3 o3 - 6 i3 a3 c3^2 - 27 i3 a3 a1^2 - 27 i3 a3 a1 c3 + 81 a1 a2 a3^2 c1 - 45 a3 a1 d1 c3 - 3 d1 o3 a3 - 9 a3 a1 c2 g3 - 3 a3 c3 c2 g3 + 243 a3 a2 a1^3 - 81 a3 a1^2 d1 - 3 a3 d1 c3^2) / (3 g3 a3)$$

> **tmp1 := cpcoeff (x2\*x3^2\*T);**

$$\begin{aligned} tmp1 := & -(-27 c3 g3^2 a1 o3 - 810 g3 a3 a1^3 c3^2 - 324 g3 a3 a1^3 o3 + 90 h3 g3 a3^2 c3^3 \\ & + 270 h3 g3 a3^3 c1 c3 - 324 g3 a3 a1^2 c3^3 + 270 a1 a3 c3 h3 g3^2 - 21 c3^3 g3^2 a1 \\ & - 10 c3^2 g3^2 o3 + 10 g3^3 c3 h3 + 12 g3^3 a1 h3 + 6 g3^3 c1 a1 + 5 g3^3 c1 c3 - 63 c3^2 g3^2 a1^2 \\ & + 108 g3 a3^2 c3^3 c1 + 216 u2 a3^3 c1 g3^2 + 30 c3 a3 u2 g3^3 - 72 g3 a3 c3^4 a1 \\ & + 378 g3 a3^3 c3 c1^2 - 972 g3 a3 a1^4 c3 + 36 a1 a3 u2 g3^3 + 216 u2 a3^2 a1 c3 g3^2 \\ & + 51 a3 c1 c3^2 g3^2 + 72 a3 c3^2 h3 g3^2 + 72 u2 a3^2 c3^2 g3^2 + 648 u2 a3^2 a1^2 g3^2 \\ & - 54 v2 g3^3 a3^2 - 135 o3 g3 a3 a1 c3^2 - 405 o3 g3 a3 a1^2 c3 + 288 a1 a3 c1 c3 g3^2 \\ & + 54 o3 g3 a3^2 a1 h3 - 15 o3 g3 a3 c3^3 - 9 o3^2 g3 a3 a1 + 324 a3 a1^2 h3 g3^2 \\ & - 144 c1 h3 a3^2 g3^2 + 324 a3 c1 a1^2 g3^2 + 162 o3 g3 a3^2 c1 a1 + 63 o3 g3 a3^2 c1 c3 \\ & + 36 o3 g3 a3^2 c3 h3 - 1458 a3^2 a1^4 o3 - 18 a1^2 o3 g3^2 - 108 h3^2 a3^2 g3^2 - 90 c1^2 a3^2 g3^2 \\ & - 54 a1^3 c3 g3^2 - 162 a3^3 a1 c3 h3 o3 + 3 o3 g3^2 a3 c1 - 18 o3 g3^2 a3^2 u2 - 6 o3^2 g3 a3 c3 \\ & + 6 o3 g3^2 a3 h3 + 486 a3^2 c3^2 a1 g3 h3 + 540 a3^2 c3^2 a1 c1 g3 - 162 a3^4 c1 h3 o3 \\ & - 486 a3^3 c1 a1^2 o3 - 324 a3^3 c1 a1 o3 c3 + 2916 a3^2 a1^3 c1 g3 - 486 a3^3 a1^2 h3 o3 \\ & + 648 a3^3 c1 a1 g3 h3 + 972 a3^3 c1^2 a1 g3 + 1944 a3^2 a1^3 g3 h3 - 54 a3^2 c3^5 a1 \\ & + 1458 a3^2 a1^2 c3 g3 h3 + 1782 a3^2 a1^2 c3 c1 g3 - 54 a3^3 c3^2 h3 o3 + 486 a3^3 c3^2 c1 a1^2 \\ & - 1458 a3^2 a1^3 c3 o3 - 486 a3^2 a1^2 c3^2 o3 - 108 a3^2 c3^3 a1 o3 + 486 a3^4 a1 c3 c1^2 \\ & + 486 a3^5 c1^3 - 5 c3^4 g3^2 + 324 a3^4 c3^2 c1^2 + 54 a3^3 c3^4 c1 + 2916 a3^4 a1^2 c1^2 \\ & + 4374 a3^3 a1^4 c1 - 2916 a3^2 a1^4 c3^2 - 324 a3^2 a1^2 c3^4 - 1458 a3^2 a1^3 c3^3 - 4374 a3^2 a1^5 c3 \\ & - 6 g3 a3 c3^5) / (54 g3 a3^3) \end{aligned}$$

> **elimsolve (tmp1,v2);**

$$\{-54 g3^3 a3^2 \neq 0\}$$

v2 is set to:

$$\begin{aligned} & (-27 c3 g3^2 a1 o3 - 810 g3 a3 a1^3 c3^2 - 324 g3 a3 a1^3 o3 + 90 h3 g3 a3^2 c3^3 \\ & + 270 h3 g3 a3^3 c1 c3 - 324 g3 a3 a1^2 c3^3 + 270 a1 a3 c3 h3 g3^2 - 21 c3^3 g3^2 a1 \\ & - 10 c3^2 g3^2 o3 + 10 g3^3 c3 h3 + 12 g3^3 a1 h3 + 6 g3^3 c1 a1 + 5 g3^3 c1 c3 - 63 c3^2 g3^2 a1^2 \\ & + 108 g3 a3^2 c3^3 c1 + 216 u2 a3^3 c1 g3^2 + 30 c3 a3 u2 g3^3 - 72 g3 a3 c3^4 a1 \end{aligned}$$

$$\begin{aligned}
& + 378 g_3 a_3^3 c_3 c_1^2 - 972 g_3 a_3 a_1^4 c_3 + 36 a_1 a_3 u_2 g_3^3 + 216 u_2 a_3^2 a_1 c_3 g_3^2 \\
& + 51 a_3 c_1 c_3^2 g_3^2 + 72 a_3 c_3^2 h_3 g_3^2 + 72 u_2 a_3^2 c_3^2 g_3^2 + 648 u_2 a_3^2 a_1^2 g_3^2 \\
& - 135 o_3 g_3 a_3 a_1 c_3^2 - 405 o_3 g_3 a_3 a_1^2 c_3 + 288 a_1 a_3 c_1 c_3 g_3^2 + 54 o_3 g_3 a_3^2 a_1 h_3 \\
& - 15 o_3 g_3 a_3 c_3^3 - 9 o_3^2 g_3 a_3 a_1 + 324 a_3 a_1^2 h_3 g_3^2 - 144 c_1 h_3 a_3^2 g_3^2 \\
& + 324 a_3 c_1 a_1^2 g_3^2 + 162 o_3 g_3 a_3^2 c_1 a_1 + 63 o_3 g_3 a_3^2 c_1 c_3 + 36 o_3 g_3 a_3^2 c_3 h_3 \\
& - 1458 a_3^2 a_1^4 o_3 - 18 a_1^2 o_3 g_3^2 - 108 h_3^2 a_3^2 g_3^2 - 90 c_1^2 a_3^2 g_3^2 - 54 a_1^3 c_3 g_3^2 \\
& - 162 a_3^3 a_1 c_3 h_3 o_3 + 3 o_3 g_3^2 a_3 c_1 - 18 o_3 g_3^2 a_3^2 u_2 - 6 o_3^2 g_3 a_3 c_3 + 6 o_3 g_3^2 a_3 h_3 \\
& + 486 a_3^2 c_3^2 a_1 g_3 h_3 + 540 a_3^2 c_3^2 a_1 c_1 g_3 - 162 a_3^4 c_1 h_3 o_3 - 486 a_3^3 c_1 a_1^2 o_3 \\
& - 324 a_3^3 c_1 a_1 o_3 c_3 + 2916 a_3^2 a_1^3 c_1 g_3 - 486 a_3^3 a_1^2 h_3 o_3 + 648 a_3^3 c_1 a_1 g_3 h_3 \\
& + 972 a_3^3 c_1^2 a_1 g_3 + 1944 a_3^2 a_1^3 g_3 h_3 - 54 a_3^2 c_3^5 a_1 + 1458 a_3^2 a_1^2 c_3 g_3 h_3 \\
& + 1782 a_3^2 a_1^2 c_3 c_1 g_3 - 54 a_3^3 c_3^2 h_3 o_3 + 486 a_3^3 c_3^2 c_1 a_1^2 - 1458 a_3^2 a_1^3 c_3 o_3 \\
& - 486 a_3^2 a_1^2 c_3^2 o_3 - 108 a_3^2 c_3^3 a_1 o_3 + 486 a_3^4 a_1 c_3 c_1^2 + 486 a_3^5 c_1^3 - 5 c_3^4 g_3^2 \\
& + 324 a_3^4 c_3^2 c_1^2 + 54 a_3^3 c_3^4 c_1 + 2916 a_3^4 a_1^2 c_1^2 + 4374 a_3^3 a_1^4 c_1 - 2916 a_3^2 a_1^4 c_3^2 \\
& - 324 a_3^2 a_1^2 c_3^4 - 1458 a_3^2 a_1^3 c_3^3 - 4374 a_3^2 a_1^5 c_3 - 6 g_3 a_3 c_3^5) / (54 g_3^3 a_3^2)
\end{aligned}$$

> **tmp1 := cpcoeff (x1\*x3^3\*T) ;**

$$\begin{aligned}
tmp1 := & (2916 a_1 c_3^2 h_3 g_3 a_3^3 c_1 + 12 c_1^2 g_3^4 - 216 w_2 g_3^4 a_3^2 + 54 c_1^3 g_3^2 a_3^3 \\
& + 5 c_1 g_3^3 c_3^3 + 18 c_3^2 g_3^2 o_3^2 - 25 c_3^4 g_3^2 o_3 - 1701 c_3^2 g_3^2 a_1^4 - 1080 c_3^3 g_3^2 a_1^3 \\
& + 72 g_3^3 a_3 c_3 h_3^2 + 648 g_3^3 a_3 a_1 h_3^2 + 24 g_3^4 h_3^2 - 17 c_3^6 g_3^2 + 174 c_1 g_3^3 a_3 c_3 h_3 \\
& + 87 c_1^2 g_3^3 a_3 c_3 + 36 c_1 g_3^4 a_3 u_2 + 21 c_1 g_3^3 a_1 c_3^2 - 33 c_1 g_3^3 o_3 c_3 + 63 c_1 g_3^3 a_1^2 c_3 \\
& - 54 c_1 g_3^3 a_1 o_3 - 1323 c_1 g_3^2 a_3 a_1^2 o_3 + 1242 c_1 g_3^2 a_3 c_3^3 a_1 + 4050 c_1 g_3^2 a_3 c_3^2 a_1^2 \\
& + 1116 c_1 g_3^3 a_3 a_1 h_3 + 36 c_1 g_3^4 h_3 + 1134 c_1^2 g_3^2 a_3^2 a_1^2 + 711 c_1^2 g_3^2 a_3^2 c_3^2 \\
& + 558 c_1^2 g_3^3 a_3 a_1 + 342 c_1 g_3^2 h_3 a_3^2 o_3 + 7290 c_1 g_3^2 a_3 a_1^3 c_3 - 828 c_1 g_3^2 a_3 c_3 a_1 o_3 \\
& - 42 g_3^3 h_3 o_3 c_3 + 234 g_3^3 h_3 a_1^2 c_3 - 72 g_3^3 h_3 a_1 o_3 + 22 g_3^3 h_3 c_3^3 + 78 g_3^3 h_3 a_1 c_3^2 \\
& + 1944 a_1^2 c_3^2 u_2 a_3^2 g_3^2 + 432 a_1 c_3^3 u_2 a_3^2 g_3^2 + 3888 a_1^3 c_3 u_2 a_3^2 g_3^2 \\
& - 3240 c_3^2 g_3 a_1^3 a_3 o_3 + 756 a_1 c_3^4 h_3 g_3 a_3^2 + 4698 c_3^2 g_3 a_1 c_1^2 a_3^3 \\
& + 648 a_1 c_3^4 g_3 a_3^2 c_1 + 1296 a_1 c_3 u_2 a_3^3 c_1 g_3^2 - 4374 a_1^5 c_3 a_3^2 o_3 \\
& - 2916 a_1^3 c_3^3 a_3^3 c_1 - 1458 a_1^4 c_3^2 a_3^2 o_3 + 486 a_1^3 c_3^3 a_3^2 o_3 + 4050 c_3^2 g_3^2 a_1^2 a_3 h_3 \\
& + 450 c_3^2 g_3^3 a_1 a_3 u_2 - 378 c_3^2 g_3^2 a_1^2 o_3 - 12150 c_3^3 g_3 a_1^4 a_3 - 1242 c_3^5 g_3 a_1^2 a_3 \\
& - 342 c_3^3 g_3 h_3 a_3^2 o_3 + 4374 c_3^3 g_3 c_1 a_3^2 a_1^2 - 180 c_3^4 g_3 a_3 a_1 o_3 - 198 c_3^6 g_3 a_3 a_1 \\
& - 5346 c_3^4 g_3 a_1^3 a_3 + 198 c_3^5 g_3 a_3^2 c_1 - 120 c_3^3 g_3^2 a_1 o_3 - 4860 c_3 g_3 a_1^2 h_3 a_3^2 o_3 \\
& + 1242 c_3^3 g_3^2 a_1 a_3 h_3 - 108 c_3^5 g_3^2 a_1 - 495 c_3^4 g_3^2 a_1^2 - 26244 a_1^5 c_3^3 a_3^2 \\
& + 1350 c_3^3 g_3 c_1^2 a_3^3 + 5346 c_3 g_3^2 a_1^3 a_3 h_3 - 1026 c_3 g_3 a_3^3 c_1 h_3 o_3 \\
& - 2322 c_3^2 g_3 a_3^2 c_1 a_1 o_3 + 2214 c_3 g_3^2 a_3^2 c_1^2 a_1 - 945 c_3^3 g_3 a_1^2 a_3 o_3 \\
& + 1674 c_3 g_3^2 a_3^2 c_1 a_1 h_3 + 828 c_3^2 g_3^2 a_3^2 c_1 h_3 - 459 c_3 g_3^2 a_1^3 o_3 \\
& - 1620 c_3^2 g_3 a_1 h_3 a_3^2 o_3 - 54 c_3^2 g_3^2 a_3 c_1 o_3 + 414 c_3 g_3^3 a_3^2 c_1 u_2
\end{aligned}$$

$$\begin{aligned}
& + 1350 c3 g3^3 a1^2 a3 u2 - 6480 c3 g3 a3^2 c1 a1^2 o3 + 17496 c3 g3 a1^2 c1^2 a3^3 \\
& - 4617 c3 g3 a1^4 a3 o3 + 30618 c3 g3 a1^4 c1 a3^2 + 252 c3^4 g3^2 a3 h3 + 138 c3^3 g3^3 a3 u2 \\
& + 180 c3^4 g3^2 a3 c1 + 63 c3 g3^2 o3^2 a1 + 2106 c3 g3 a3^4 c1^3 - 18954 c3^2 g3 a1^5 a3 \\
& - 1008 c3 g3^2 o3 a3 a1 h3 - 66 c3^2 g3^2 o3 a3 h3 + 18 c3 g3^3 o3 a3 u2 + 72 c3^4 u2 a3^2 g3^2 \\
& + 3 c3^5 o3 g3 a3 - 108 c3^2 h3^2 a3^2 g3^2 - 1458 a1^2 c3^2 a3^3 h3 o3 + 378 a1 c3^2 o3^2 g3 a3 \\
& + 432 c3^2 u2 a3^3 c1 g3^2 - 306 c3^3 o3 g3 a3^2 c1 + 540 c3^3 h3 g3 a3^3 c1 - 10206 a1^4 c3^4 a3^2 \\
& - 39366 a1^6 c3^2 a3^2 + 162 a1^2 c3^4 a3^2 o3 + 8748 a1^2 c3^2 a3^4 c1^2 + 2916 a1 c3 a3^5 c1^3 \\
& + 1458 a1 c3^3 a3^4 c1^2 + 13122 a1^3 c3 a3^4 c1^2 + 90 c3^5 h3 g3 a3^2 - 2916 a1^3 c3 a3^3 h3 o3 \\
& + 8748 a1^2 c3 a3^3 c1 g3 h3 + 18954 a1^4 c3 a3^2 g3 h3 + 10692 a1^3 c3^2 a3^2 g3 h3 \\
& + 10692 a1^3 c3^2 a3^2 c1 g3 - 324 a1 c3^3 a3^3 h3 o3 - 2916 a1^3 c3^5 a3^2 \\
& - 702 a1 c3 o3 g3^2 a3^2 u2 - 972 a1 c3 a3^4 c1 h3 o3 + 1134 a1^2 c3 o3^2 g3 a3 \\
& - 324 a1 c3 h3^2 a3^2 g3^2 + 3726 a1^2 c3^3 a3^2 g3 h3 - 8748 a1^3 c3 a3^3 c1 o3 \\
& - 4374 a1^2 c3^2 a3^3 c1 o3 - 486 a1^2 c3^6 a3^2 + 39 c3^3 o3^2 g3 a3 - 54 c3^4 a3^3 h3 o3 \\
& + 54 c3^5 a3^2 a1 o3 + 810 a3^4 c1^2 h3 g3 c3 + 11664 a1^3 a3^3 c1 g3 h3 + 39366 a1^4 a3^4 c1^2 \\
& + 39366 a1^6 a3^3 c1 - 39366 a1^7 a3^2 c3 - 2106 a1^2 o3 g3^2 a3^2 u2 - 5346 a1^3 o3 g3 a3^2 h3 \\
& + 1620 a1^2 c1 h3 a3^2 g3^2 - 8262 a1^3 o3 g3 a3^2 c1 - 1566 a1^2 o3 g3^2 a3 h3 \\
& - 2916 a1^2 a3^4 c1 h3 o3 - 21870 a1^4 a3^3 c1 o3 - 4374 a1^4 a3^3 h3 o3 + 17496 a1^3 a3^3 c1^2 g3 \\
& + 17496 a1^5 a3^2 g3 h3 + 26244 a1^5 a3^2 c1 g3 + 3888 a1^2 u2 a3^3 c1 g3^2 + 5832 a1^4 u2 a3^2 g3^2 \\
& + 891 a1^3 o3^2 g3 a3 + 2916 a1^4 a3 h3 g3^2 + 2916 a1^4 a3 c1 g3^2 - 972 a1^2 h3^2 a3^2 g3^2 \\
& + 108 a1^3 g3^3 h3 - 13122 a1^6 a3^2 o3 - 162 a1^4 o3 g3^2 - 486 a1^5 c3 g3^2 + 13122 a1^2 a3^5 c1^3 \\
& + 54 a1^3 g3^3 c1 + 1458 c3^2 a3^5 c1^3 + 54 c3^6 a3^3 c1 - 6 c3^7 g3 a3 + 486 c3^4 a3^4 c1^2 \\
& - 2916 a1^5 g3 a3 o3 - 8748 a1^6 g3 a3 c3 + 324 a1^3 a3 u2 g3^3 - 234 c3^2 o3 g3^2 a3^2 u2 \\
& - 324 c3^2 a3^4 c1 h3 o3 - 648 c3^3 a3^3 c1 a1 o3 - 54 c3^7 a3^2 a1 - 945 a3^3 c1^2 o3 g3 c3 \\
& + 279 a3^2 c1^2 o3 g3^2 - 10206 a3^4 c1^2 a1^2 o3 - 486 a3^5 c1^2 h3 o3 - 2430 a3^3 c1^2 o3 g3 a1 \\
& - 702 a3^3 c1 o3 g3^2 u2 - 207 a3^2 c1 o3^2 g3 c3 - 2430 a3^4 c1^2 a1 o3 c3 + 2916 a3^4 c1^3 a1 g3 \\
& - 1782 a3^3 c1 o3 g3 a1 h3 - 513 a3^2 c1 o3^2 g3 a1 + 108 a3^2 c1 a1 u2 g3^3 \\
& + 648 a3^4 c1^2 u2 g3^2 + 216 a3^3 c1^2 h3 g3^2 - 324 a3^3 c1 h3^2 g3^2 + 1458 a3^6 c1^4 \\
& + 4374 a3^2 a1^4 o3^2 + 54 a1^2 o3^2 g3^2 + 108 g3^2 h3^2 a3^2 o3 + 1944 a3^4 c1^2 a1 g3 h3 \\
& - 162 o3 a3^3 c3^4 c1 - 972 o3 a3^4 c3^2 c1^2 - 1458 o3 a3^5 c1^3 + 972 a3^3 c1 a1 o3^2 c3 \\
& - 162 o3^2 g3 a3^2 a1 h3 - 108 o3^2 g3 a3^2 c3 h3 + 486 a3^3 a1 c3 h3 o3^2 + 18 o3^3 g3 a3 c3 \\
& - 18 o3^2 g3^2 a3 h3 + 486 a3^4 c1 h3 o3^2 + 1458 a3^3 c1 a1^2 o3^2 + 1458 a3^3 a1^2 h3 o3^2 \\
& + 162 a3^3 c3^2 h3 o3^2 + 4374 a3^2 a1^3 c3 o3^2 + 1458 a3^2 a1^2 c3^2 o3^2 + 324 a3^2 c3^3 a1 o3^2 \\
& + 27 o3^3 g3 a3 a1 - 9 o3^2 g3^2 a3 c1 + 54 o3^2 g3^2 a3^2 u2) / (54 a3^2 g3^3)
\end{aligned}$$

> **elimsolve (tmp1,w2) ;**

$$\{-216 g3^4 a3^2 \neq 0\}$$

w2 is set to:

$$\begin{aligned}
& (2916 a l c^3 h^3 g^3 a^3 c l + 12 c l^2 g^3 + 54 c l^3 g^3 a^3 + 5 c l g^3 c^3 + 18 c^3 g^3 o^3 \\
& - 25 c^3 g^3 o^3 - 1701 c^3 g^3 a l^4 - 1080 c^3 g^3 a l^3 + 72 g^3 a^3 c^3 h^3 + 648 g^3 a^3 a l h^3 \\
& + 24 g^3 h^3 - 17 c^3 g^3 + 174 c l g^3 a^3 c^3 h^3 + 87 c l^2 g^3 a^3 c^3 + 36 c l g^3 a^3 u^2 \\
& + 21 c l g^3 a l c^3 - 33 c l g^3 o^3 c^3 + 63 c l g^3 a l^2 c^3 - 54 c l g^3 a l o^3 \\
& - 1323 c l g^3 a^3 a l^2 o^3 + 1242 c l g^3 a^3 c^3 a l + 4050 c l g^3 a^3 c^3 a l^2 \\
& + 1116 c l g^3 a^3 a l h^3 + 36 c l g^3 h^3 + 1134 c l^2 g^3 a^3 a l^2 + 711 c l^2 g^3 a^3 c^3 \\
& + 558 c l^2 g^3 a^3 a l + 342 c l g^3 h^3 a^3 o^3 + 7290 c l g^3 a^3 a l^3 c^3 - 828 c l g^3 a^3 c^3 a l o^3 \\
& - 42 g^3 h^3 o^3 c^3 + 234 g^3 h^3 a l^2 c^3 - 72 g^3 h^3 a l o^3 + 22 g^3 h^3 c^3 + 78 g^3 h^3 a l c^3 \\
& + 1944 a l^2 c^3 u^2 a^3 g^3 + 432 a l c^3 u^2 a^3 g^3 + 3888 a l^3 c^3 u^2 a^3 g^3 \\
& - 3240 c^3 g^3 a l^3 a^3 o^3 + 756 a l c^3 h^3 g^3 a^3 + 4698 c^3 g^3 a l c l^2 a^3 \\
& + 648 a l c^3 g^3 a^3 c l + 1296 a l c^3 u^2 a^3 c l g^3 - 4374 a l^5 c^3 a^3 o^3 \\
& - 2916 a l^3 c^3 a^3 c l - 1458 a l^4 c^3 a^3 o^3 + 486 a l^3 c^3 a^3 o^3 + 4050 c^3 g^3 a l^2 a^3 h^3 \\
& + 450 c^3 g^3 a l a^3 u^2 - 378 c^3 g^3 a l^2 o^3 - 12150 c^3 g^3 a l^4 a^3 - 1242 c^3 g^3 a l^2 a^3 \\
& - 342 c^3 g^3 h^3 a^3 o^3 + 4374 c^3 g^3 c l a^3 a l^2 - 180 c^3 g^3 a^3 a l o^3 - 198 c^3 g^3 a^3 a l \\
& - 5346 c^3 g^3 a l^3 a^3 + 198 c^3 g^3 a^3 c l - 120 c^3 g^3 a l o^3 - 4860 c^3 g^3 a l^2 h^3 a^3 o^3 \\
& + 1242 c^3 g^3 a l a^3 h^3 - 108 c^3 g^3 a l - 495 c^3 g^3 a l^2 - 26244 a l^5 c^3 a^3 \\
& + 1350 c^3 g^3 c l^2 a^3 + 5346 c^3 g^3 a l^3 a^3 h^3 - 1026 c^3 g^3 a^3 c l h^3 o^3 \\
& - 2322 c^3 g^3 a^3 c l a l o^3 + 2214 c^3 g^3 a^3 c l^2 a l - 945 c^3 g^3 a l^2 a^3 o^3 \\
& + 1674 c^3 g^3 a^3 c l a l h^3 + 828 c^3 g^3 a^3 c l h^3 - 459 c^3 g^3 a l^3 o^3 \\
& - 1620 c^3 g^3 a l h^3 a^3 o^3 - 54 c^3 g^3 a^3 c l o^3 + 414 c^3 g^3 a^3 c l u^2 \\
& + 1350 c^3 g^3 a l^2 a^3 u^2 - 6480 c^3 g^3 a^3 c l a l^2 o^3 + 17496 c^3 g^3 a l^2 c l^2 a^3 \\
& - 4617 c^3 g^3 a l^4 a^3 o^3 + 30618 c^3 g^3 a l^4 c l a^3 + 252 c^3 g^3 a^3 h^3 + 138 c^3 g^3 a^3 u^2 \\
& + 180 c^3 g^3 a^3 c l + 63 c^3 g^3 o^3 a l + 2106 c^3 g^3 a^3 c l^3 - 18954 c^3 g^3 a l^5 a^3 \\
& - 1008 c^3 g^3 o^3 a^3 a l h^3 - 66 c^3 g^3 o^3 a^3 h^3 + 18 c^3 g^3 o^3 a^3 u^2 + 72 c^3 u^2 a^3 g^3 \\
& + 3 c^3 o^3 g^3 a^3 - 108 c^3 h^3 a^3 g^3 - 1458 a l^2 c^3 a^3 h^3 o^3 + 378 a l c^3 o^3 g^3 a^3 \\
& + 432 c^3 u^2 a^3 c l g^3 - 306 c^3 o^3 g^3 a^3 c l + 540 c^3 h^3 g^3 a^3 c l - 10206 a l^4 c^3 a^3 \\
& - 39366 a l^6 c^3 a^3 + 162 a l^2 c^3 a^3 o^3 + 8748 a l^2 c^3 a^3 c l^2 + 2916 a l c^3 a^3 c l^3 \\
& + 1458 a l c^3 a^3 c l^2 + 13122 a l^3 c^3 a^3 c l^2 + 90 c^3 h^3 g^3 a^3 - 2916 a l^3 c^3 a^3 h^3 o^3 \\
& + 8748 a l^2 c^3 a^3 c l g^3 h^3 + 18954 a l^4 c^3 a^3 g^3 h^3 + 10692 a l^3 c^3 a^3 g^3 h^3 \\
& + 10692 a l^3 c^3 a^3 c l g^3 - 324 a l c^3 a^3 h^3 o^3 - 2916 a l^3 c^3 a^3 \\
& - 702 a l c^3 o^3 g^3 a^3 u^2 - 972 a l c^3 a^3 c l h^3 o^3 + 1134 a l^2 c^3 o^3 g^3 a^3 \\
& - 324 a l c^3 h^3 a^3 g^3 + 3726 a l^2 c^3 a^3 g^3 h^3 - 8748 a l^3 c^3 a^3 c l o^3 \\
& - 4374 a l^2 c^3 a^3 c l o^3 - 486 a l^2 c^3 a^3 + 39 c^3 o^3 g^3 a^3 - 54 c^3 a^3 h^3 o^3 \\
& + 54 c^3 a^3 a l o^3 + 810 a^3 c l^2 h^3 g^3 c^3 + 11664 a l^3 a^3 c l g^3 h^3 + 39366 a l^4 a^3 c l^2 \\
& + 39366 a l^6 a^3 c l - 39366 a l^7 a^3 c^3 - 2106 a l^2 o^3 g^3 a^3 u^2 - 5346 a l^3 o^3 g^3 a^3 h^3
\end{aligned}$$

$$\begin{aligned}
& + 1620 a l^2 c l h3 a3^2 g3^2 - 8262 a l^3 o3 g3 a3^2 c l - 1566 a l^2 o3 g3^2 a3 h3 \\
& - 2916 a l^2 a3^4 c l h3 o3 - 21870 a l^4 a3^3 c l o3 - 4374 a l^4 a3^3 h3 o3 + 17496 a l^3 a3^3 c l^2 g3 \\
& + 17496 a l^5 a3^2 g3 h3 + 26244 a l^5 a3^2 c l g3 + 3888 a l^2 u2 a3^3 c l g3^2 + 5832 a l^4 u2 a3^2 g3^2 \\
& + 891 a l^3 o3^2 g3 a3 + 2916 a l^4 a3 h3 g3^2 + 2916 a l^4 a3 c l g3^2 - 972 a l^2 h3^2 a3^2 g3^2 \\
& + 108 a l^3 g3^3 h3 - 13122 a l^6 a3^2 o3 - 162 a l^4 o3 g3^2 - 486 a l^5 c3 g3^2 + 13122 a l^2 a3^5 c l^3 \\
& + 54 a l^3 g3^3 c l + 1458 c3^2 a3^5 c l^3 + 54 c3^6 a3^3 c l - 6 c3^7 g3 a3 + 486 c3^4 a3^4 c l^2 \\
& - 2916 a l^5 g3 a3 o3 - 8748 a l^6 g3 a3 c3 + 324 a l^3 a3 u2 g3^3 - 234 c3^2 o3 g3^2 a3^2 u2 \\
& - 324 c3^2 a3^4 c l h3 o3 - 648 c3^3 a3^3 c l a l o3 - 54 c3^7 a3^2 a l - 945 a3^3 c l^2 o3 g3 c3 \\
& + 279 a3^2 c l^2 o3 g3^2 - 10206 a3^4 c l^2 a l^2 o3 - 486 a3^5 c l^2 h3 o3 - 2430 a3^3 c l^2 o3 g3 a l \\
& - 702 a3^3 c l o3 g3^2 u2 - 207 a3^2 c l o3^2 g3 c3 - 2430 a3^4 c l^2 a l o3 c3 + 2916 a3^4 c l^3 a l g3 \\
& - 1782 a3^3 c l o3 g3 a l h3 - 513 a3^2 c l o3^2 g3 a l + 108 a3^2 c l a l u2 g3^3 \\
& + 648 a3^4 c l^2 u2 g3^2 + 216 a3^3 c l^2 h3 g3^2 - 324 a3^3 c l h3^2 g3^2 + 1458 a3^6 c l^4 \\
& + 4374 a3^2 a l^4 o3^2 + 54 a l^2 o3^2 g3^2 + 108 g3^2 h3^2 a3^2 o3 + 1944 a3^4 c l^2 a l g3 h3 \\
& - 162 o3 a3^3 c3^4 c l - 972 o3 a3^4 c3^2 c l^2 - 1458 o3 a3^5 c l^3 + 972 a3^3 c l a l o3^2 c3 \\
& - 162 o3^2 g3 a3^2 a l h3 - 108 o3^2 g3 a3^2 c3 h3 + 486 a3^3 a l c3 h3 o3^2 + 18 o3^3 g3 a3 c3 \\
& - 18 o3^2 g3^2 a3 h3 + 486 a3^4 c l h3 o3^2 + 1458 a3^3 c l a l^2 o3^2 + 1458 a3^3 a l^2 h3 o3^2 \\
& + 162 a3^3 c3^2 h3 o3^2 + 4374 a3^2 a l^3 c3 o3^2 + 1458 a3^2 a l^2 c3^2 o3^2 + 324 a3^2 c3^3 a l o3^2 \\
& + 27 o3^3 g3 a3 a l - 9 o3^2 g3^2 a3 c l + 54 o3^2 g3^2 a3^2 u2) / (216 g3^4 a3^2)
\end{aligned}$$

> **tmp1 := cpcoeff (x2^2\*T);**

$$\begin{aligned}
tmp1 := & -(27 c l^2 a3^3 + 3 a3 c3^4 - g3 c3^3 + 2 g3^2 h3 + c l g3^2 + 243 a3 a l^4 + 3 o3^2 a3 \\
& - 9 c l o3 a3^2 + 162 a3 a l^3 c3 - 27 a3 a l^2 o3 + 162 c l a3^2 a l^2 + 18 a3 c3^3 a l + 81 a3 c3^2 a l^2 \\
& - 3 a3 c3^2 o3 - 2 g3 o3 c3 - 3 g3 a l o3 + 18 a3^2 c3^2 c l - 9 g3 a l^2 c3 - 9 a3 c3 a l o3 \\
& + 54 c l a3^2 a l c3 - 3 g3 a3 c l c3 - 3 g3 a l c3^2) / (3 a3)
\end{aligned}$$

> **elimsolve (tmp1,h3);**

$$\{2 g3^2 \neq 0\}$$

h3 is set to:

$$\begin{aligned}
& -(27 c l^2 a3^3 + 3 a3 c3^4 - g3 c3^3 + c l g3^2 + 243 a3 a l^4 + 3 o3^2 a3 - 9 c l o3 a3^2 \\
& + 162 a3 a l^3 c3 - 27 a3 a l^2 o3 + 162 c l a3^2 a l^2 + 18 a3 c3^3 a l + 81 a3 c3^2 a l^2 - 3 a3 c3^2 o3 \\
& - 2 g3 o3 c3 - 3 g3 a l o3 + 18 a3^2 c3^2 c l - 9 g3 a l^2 c3 - 9 a3 c3 a l o3 + 54 c l a3^2 a l c3 \\
& - 3 g3 a3 c l c3 - 3 g3 a l c3^2) / (2 g3^2)
\end{aligned}$$

> **launchNZcase (c1);**

Launching case level 3:

$$c l \neq 0$$

Assume from now on that:

$$6 a3 g3 c l \neq 0$$

> **tmp1 := cpcoeff (x1^6);**

$$tmp1 := -9 a3 c l a l - 6 a3 c l c3 - c l g3 - c3^3$$

> **elimsolve (tmp1,a1);**

$$\{9 a3 c1 \neq 0\}$$

a1 is set to:

$$-\frac{6 a3 c1 c3 + c1 g3 + c3^3}{9 a3 c1}$$

> **tmp1 := cpcoeff(x1^5);**

$$\begin{aligned} tmp1 := & -(9 a2 c1^3 g3 a3 + 9 i3 c3^2 c1^2 a3 - 3 a3 i1 c1 c3^3 - 27 a3^2 c2 c3^2 c1^2 \\ & - 9 a3 c2 c3^4 c1 - 2 d3 c1^3 g3 - 2 d3 c1^2 c3^3 - c2 c1 g3 c3^3 + 18 a3^2 c1^3 d1 + 18 a3^2 c1^3 i3 \\ & - c2 c3^6 - 27 a3^3 c2 c1^3 + 3 c1^3 p3 a3) / (3 a3 c1^2) \end{aligned}$$

> **elimsolve (tmp1,d1);**

$$\{18 c1^3 a3^2 \neq 0\}$$

d1 is set to:

$$\begin{aligned} & -(9 a2 c1^3 g3 a3 + 9 i3 c3^2 c1^2 a3 - 3 a3 i1 c1 c3^3 - 27 a3^2 c2 c3^2 c1^2 - 9 a3 c2 c3^4 c1 \\ & - 2 d3 c1^3 g3 - 2 d3 c1^2 c3^3 - c2 c1 g3 c3^3 + 18 a3^2 c1^3 i3 - c2 c3^6 - 27 a3^3 c2 c1^3 \\ & + 3 c1^3 p3 a3) / (18 c1^3 a3^2) \end{aligned}$$

> **tmp1 := cpcoeff (x2^3);**

$$\begin{aligned} tmp1 := & -(-9 o3 c1^2 a3^2 + 27 c3^2 c1^2 a3^2 + 9 a3 c1^2 c3 g3 + 9 a3 c1 c3^4 + c1^2 g3^2 \\ & + 2 c1 g3 c3^3 + c3^6 + 27 a3^3 c1^3) / (729 c1^6 a3^6) \end{aligned}$$

> **elimsolve (tmp1,o3);**

$$\{-9 c1^2 a3^2 \neq 0\}$$

o3 is set to:

$$\frac{27 c3^2 c1^2 a3^2 + 9 a3 c1^2 c3 g3 + 9 a3 c1 c3^4 + c1^2 g3^2 + 2 c1 g3 c3^3 + c3^6 + 27 a3^3 c1^3}{9 c1^2 a3^2}$$

> **launchNZcase (3\*a3\*c1+c3^2);**

Launching case level 4:

$$3 a3 c1 + c3^2 \neq 0$$

Assume from now on that:

$$6 a3 g3 c1 (3 a3 c1 + c3^2) \neq 0$$

> **tmp1 := cpcoeff(x1^5\*x3);**

$$\begin{aligned} tmp1 := & (39366 a3^9 c1^9 - 72 a3 c1^3 c3^{10} g3^2 - 36 a3 c1^4 c3^7 g3^3 - 6 a3 c1^5 c3^4 g3^4 \\ & + 4374 a3^7 u2 c1^7 g3^2 + 4374 a3^6 u2 c1^6 g3^2 c3^2 + 1458 a3^5 u2 c1^5 g3^2 c3^4 \\ & + 162 a3^4 u2 c1^4 g3^2 c3^6 + 40095 c3^3 c1^7 a3^6 g3 + 29160 c3^5 c1^6 a3^5 g3 \\ & + 7533 c3^4 c1^6 a3^4 g3^2 + 1350 c3^9 c1^4 a3^3 g3 + 2295 c3^6 c1^5 a3^3 g3^2 + 1026 c3^3 c1^6 a3^3 g3^3 \\ & + 10125 c3^7 c1^5 a3^4 g3 + 54 c3^2 c1^6 a3^2 g3^4 + 9477 c3^2 c1^7 a3^5 g3^2 - 135 c3^{11} c1^3 a3^2 g3 \\ & + 108 c3^8 c1^4 a3^2 g3^2 + 189 c3^5 c1^5 a3^2 g3^3 - 60 a3 c1^2 c3^{13} g3 + 21870 a3^7 c1^8 c3 g3 \\ & + 1215 a3^4 c1^7 c3 g3^3 - 108 c3^{14} c1^2 a3^2 + 98415 c3^2 c1^8 a3^8 + 61236 c3^6 c1^6 a3^6 \\ & + 104976 c3^4 c1^7 a3^7 + 3402 c3^{10} c1^4 a3^4 + 20412 c3^8 c1^5 a3^5 - 18 a3 c1 c3^{16} \\ & - 10 c1^2 g3^2 c3^{12} + 3645 c1^8 g3^2 a3^6 + 81 c1^7 g3^4 a3^3 - 10 c1^3 g3^3 c3^9 - 5 c1^4 g3^4 c3^6 \\ & - c1^5 g3^5 c3^3 - 5 c1 g3 c3^{15} - c3^{18}) / (243 c1^6 a3^5 g3^2) \end{aligned}$$

> **elimsolve (tmp1,u2);**

$\{4374 a^3 c l^7 g^3 + 4374 a^3 c l^6 g^3 c^2 + 1458 a^3 c l^5 g^3 c^3 + 162 a^3 c l^4 g^3 c^4 + 162 a^3 c l^4 g^3 c^5 \neq 0\}$   
u2 is set to:

$$\begin{aligned}
& - (39366 a^3 c l^9 - 72 a^3 c l^3 c^3 g^2 - 36 a^3 c l^4 c^3 g^3 - 6 a^3 c l^5 c^3 g^4 \\
& + 40095 c^3 c l^7 a^3 g^3 + 29160 c^3 c l^6 a^3 g^3 + 7533 c^3 c l^6 a^3 g^3 + 1350 c^3 c l^4 a^3 g^3 \\
& + 2295 c^3 c l^5 a^3 g^3 + 1026 c^3 c l^6 a^3 g^3 + 10125 c^3 c l^7 a^3 g^3 + 54 c^3 c l^6 a^3 g^3 \\
& + 9477 c^3 c l^7 a^3 g^3 - 135 c^3 c l^3 a^3 g^2 + 108 c^3 c l^4 a^3 g^2 + 189 c^3 c l^5 a^3 g^2 \\
& - 60 a^3 c l^2 c^3 g^3 + 21870 a^3 c l^8 c^3 g^3 + 1215 a^3 c l^7 c^3 g^3 - 108 c^3 c l^2 a^3 g^2 \\
& + 98415 c^3 c l^8 a^3 g^3 + 61236 c^3 c l^6 a^3 g^3 + 104976 c^3 c l^7 a^3 g^3 + 3402 c^3 c l^10 a^3 g^3 \\
& + 20412 c^3 c l^5 a^3 g^3 - 18 a^3 c l c^3 g^3 - 10 c l^2 g^3 c^3 + 3645 c l^8 g^3 a^3 + 81 c l^7 g^3 a^3 \\
& - 10 c l^3 g^3 c^3 - 5 c l^4 g^3 c^3 - c l^5 g^3 c^3 - 5 c l g^3 c^3 - c^3 g^3) / (162 a^3 c l^4 g^3 \\
& (3 a^3 c l + c^3)^3)
\end{aligned}$$

> **launchNZcase** (9\*c1^2\*a3^2+6\*c3^2\*a3\*c1+c3\*c1\*g3+c3^4) ;

Launching case level 5:

$$9 c l^2 a^3 + 6 a^3 c l c^3 + c^3 c l g^3 + c^3^4 \neq 0$$

Assume from now on that:

$$6 a^3 g^3 c l (3 a^3 c l + c^3) (9 c l^2 a^3 + 6 a^3 c l c^3 + c^3 c l g^3 + c^3^4) \neq 0$$

> **elimsolve** (a3+1/3\*var1^2\*c1,a3) ;

$$\{3 \neq 0\}$$

a3 is set to:

$$-\frac{var1^2 c l}{3}$$

Nonzero constraint refines to:

$$\begin{aligned}
& -6 var1 c l^2 g^3 (-var1 c l + c^3) (var1 c l + c^3) (c l^4 var1^4 - 2 var1^2 c l^2 c^3 + c^3 c l g^3 + c^3^4) \\
& \neq 0
\end{aligned}$$

> **launchNZcase**

(-c1\*g3-c3^3-c3^2\*var1\*c1+c3\*var1^2\*c1^2+var1^3\*c1^3) ;

Launching case level 6:

$$-c l g^3 - c^3 - c^3 var1 c l + c^3 var1^2 c l^2 + var1^3 c l^3 \neq 0$$

Assume from now on that:

$$\begin{aligned}
& -6 var1 c l^2 g^3 (-var1 c l + c^3) (var1 c l + c^3) (c l^4 var1^4 - 2 var1^2 c l^2 c^3 + c^3 c l g^3 + c^3^4) \\
& (-c l g^3 - c^3 - c^3 var1 c l + c^3 var1^2 c l^2 + var1^3 c l^3) \neq 0
\end{aligned}$$

> **tmp1 := cpccoeff(x1^4\*x2) ;**

$$tmp1 := -(-c l g^3 - c^3 - c^3 var1 c l + c^3 var1^2 c l^2 + var1^3 c l^3)$$

$$(c l g^3 + c^3 - c^3 var1 c l - c^3 var1^2 c l^2 + var1^3 c l^3)$$

$$(c l^4 var1^4 - 2 var1^2 c l^2 c^3 + c^3 c l g^3 + c^3^4)^3 / (var1^8 c l^{10} g^3^2)$$

> **elimsolve** (tmp1,g3) ;

$$\{c l \neq 0\}$$

g3 is set to:

$$-\frac{(var1 c l + c^3) (var1 c l - c^3)^2}{c l}$$

Nonzero constraint refines to:

$$-12 \text{var}l^3 c l^4 (-\text{var}l c l + c3)^2 (\text{var}l c l + c3)^4 (\text{var}l c l - c3)^2 \neq 0$$

> **tmp1 := cpcoeff(x1^4\*x3^2);**

$$\text{tmp1} := \frac{7 (\text{var}l c l + c3)^3 (\text{var}l c l - c3)^5}{2 c l^5 \text{var}l^7}$$

> **tmp2 := cpcoeff (x1^3\*x3^3);**

$$\text{tmp2} := -\frac{2 (16 \text{var}l c l + 5 c3) (\text{var}l c l + c3)^3 (\text{var}l c l - c3)^5}{3 c l^6 \text{var}l^9}$$

> **tmp3 := factor(4\*c3\*tmp1 + c1\*var1^2\*tmp2);**

$$\text{tmp3} := -\frac{32 (\text{var}l c l + c3)^3 (\text{var}l c l - c3)^6}{3 c l^5 \text{var}l^7}$$

> **contradict (tmp3,'g3');**

Contradiction on case level 6, so:

$$-c l g3 - c3^3 - c3^2 \text{var}l c l + c3 \text{var}l^2 c l^2 + \text{var}l^3 c l^3 = 0$$

Variables to be uneliminated:

$$\text{"g3 := 'g3'"}\text{"}$$

Proceed on case level 5 with:

$$-6 \text{var}l c l^2 g3 (-\text{var}l c l + c3) (\text{var}l c l + c3) (c l^4 \text{var}l^4 - 2 \text{var}l^2 c l^2 c3^2 + c3 c l g3 + c3^4) \neq 0$$

On account of:

$$-c l g3 - c3^3 - c3^2 \text{var}l c l + c3 \text{var}l^2 c l^2 + \text{var}l^3 c l^3 = 0$$
$$\{-c l \neq 0\}$$

g3 is set to:

$$\frac{(\text{var}l c l - c3) (\text{var}l c l + c3)^2}{c l}$$

Nonzero constraint refines to:

$$-6 \text{var}l^2 c l^3 (\text{var}l c l - c3)^2 (\text{var}l c l + c3)^3 (-\text{var}l c l + c3) \neq 0$$

> **tmp1 := cpcoeff(x1^4\*x3^2);**

$$\text{tmp1} := -\frac{7 (\text{var}l c l - c3)^3 (\text{var}l c l + c3)^5}{2 c l^5 \text{var}l^7}$$

> **tmp2 := cpcoeff(x1^3\*x3^3);**

$$\text{tmp2} := -\frac{2 (16 \text{var}l c l - 5 c3) (\text{var}l c l - c3)^3 (\text{var}l c l + c3)^5}{3 c l^6 \text{var}l^9}$$

> **tmp3 := factor(4\*c3\*tmp1 + c1\*var1^2\*tmp2);**

$$\text{tmp3} := -\frac{32 (\text{var}l c l - c3)^3 (\text{var}l c l + c3)^6}{3 c l^5 \text{var}l^7}$$

> **eq1 := contradict (tmp3);**

Contradiction on case level 5, so:

$$9 c l^2 a3^2 + 6 a3 c l c3^2 + c3 c l g3 + c3^4 = 0$$

Variables to be uneliminated:

$$\text{"g3 := 'g3'"}\text{"}$$

"a3 := 'a3'"

Proceed on case level 4 with:

$$6 a3 g3 c1 (3 a3 c1 + c3^2) \neq 0$$

On account of:

$$9 c1^2 a3^2 + 6 a3 c1 c3^2 + c3 c1 g3 + c3^4 = 0$$

the following return value can be used as an equation:

$$eq1 := 9 c1^2 a3^2 + 6 a3 c1 c3^2 + c3 c1 g3 + c3^4$$

> **launchNZcase (c3);**

Launching case level 5:

$$c3 \neq 0$$

Assume from now on that:

$$6 a3 g3 c1 (3 a3 c1 + c3^2) c3 \neq 0$$

> **elimsolve (eq1,g3);**

$$\{c1 c3 \neq 0\}$$

g3 is set to:

$$-\frac{(3 a3 c1 + c3^2)^2}{c1 c3}$$

Nonzero constraint refines to:

$$6 a3 (-3 a3 c1 - c3^2) c1 (3 a3 c1 + c3^2) c3 \neq 0$$

> **launchNZcase (3\*c1\*c3^2\*i1\*a3-4\*d3\*c1^2\*c3^2+c2\*c3^5+i1\*c3^4+**

> **6\*a3\*c2\*c3^3\*c1-3\*c3^3\*c1\*i3-9\*a3\*c1^2\*i3\*c3-**

> **c1^2\*p3\*c3+3\*a2\*c1\*c3^4+18\*a2\*c1^2\*a3\*c3^2-**

> **12\*d3\*c1^3\*a3+9\*a3^2\*c2\*c1^2\*c3+27\*a2\*c1^3\*a3^2);**

Launching case level 6:

$$3 c1 c3^2 i1 a3 - 4 d3 c1^2 c3^2 + c2 c3^5 + i1 c3^4 + 6 a3 c2 c3^3 c1 - 3 c3^3 c1 i3 - 9 a3 c1^2 i3 c3 \\ - c1^2 p3 c3 + 3 a2 c1 c3^4 + 18 a2 c1^2 a3 c3^2 - 12 d3 c1^3 a3 + 9 a3^2 c2 c1^2 c3 + 27 a2 c1^3 a3^2 \\ \neq 0$$

Assume from now on that:

$$6 a3 (-3 a3 c1 - c3^2) c1 (3 a3 c1 + c3^2) c3 (3 c1 c3^2 i1 a3 - 4 d3 c1^2 c3^2 + c2 c3^5 + i1 c3^4 \\ + 6 a3 c2 c3^3 c1 - 3 c3^3 c1 i3 - 9 a3 c1^2 i3 c3 - c1^2 p3 c3 + 3 a2 c1 c3^4 + 18 a2 c1^2 a3 c3^2 \\ - 12 d3 c1^3 a3 + 9 a3^2 c2 c1^2 c3 + 27 a2 c1^3 a3^2) \neq 0$$

> **tmp1 := cpcoeff (x3^4);**

$$tmp1 := -(3 c1 c3^2 i1 a3 - 4 d3 c1^2 c3^2 + c2 c3^5 + i1 c3^4 + 6 a3 c2 c3^3 c1 - 3 c3^3 c1 i3 \\ - 9 a3 c1^2 i3 c3 - c1^2 p3 c3 + 3 a2 c1 c3^4 + 18 a2 c1^2 a3 c3^2 - 12 d3 c1^3 a3 + 9 a3^2 c2 c1^2 c3 \\ + 27 a2 c1^3 a3^2) (-3 i3 c3^2 c1^2 a3 - 3 a3 i1 c1 c3^3 + 9 a3^2 c2 c3^2 c1^2 + 6 a3 c2 c3^4 c1 \\ + 18 a3^2 c1^3 i3 + c2 c3^6 - c3^2 c1^2 p3 - 18 c1^2 c3 i1 a3^2 + 27 c1^3 c3 a2 a3^2 + 18 c1^2 c3^3 a2 a3 \\ + c3^5 i1 - 3 c1 c3^4 i3 + 3 c1 c3^5 a2 - 4 d3 c1^2 c3^3 - 12 c1^3 c3 a3 d3) c1 / (3 c3^6 a3 \\ (3 a3 c1 + c3^2))$$

> **elimsolve (tmp1,p3);**

$$\{-c3^2 c1^2 \neq 0\}$$

p3 is set to:

$$(3 a3 c1 + c3^2) (6 c1^2 i3 a3 + 9 c1^2 c3 a2 a3 - 4 c1^2 c3 d3 + 3 c1 c3^2 c2 a3 - 6 c1 c3 i1 a3$$

$$-3 i3 c1 c3^2 + 3 a2 c3^3 c1 + c3^3 i1 + c3^4 c2) / (c3^2 c1^2)$$

Nonzero constraint refines to:

$$6 a3^2 (-3 a3 c1 - c3^2) c1^2 (3 a3 c1 + c3^2) c3 (-18 a3 c1 - 6 c3^2) (c1 i3 - i1 c3) \neq 0$$

> **tmp1 := cpcoeff (x1^4);**

$$tmp1 := \frac{4 (3 a3 c1 + c3^2)^2 (c1 i3 - i1 c3)^2}{c3^3 c1^2}$$

> **contradict (tmp1, 'p3');**

Contradiction on case level 6, so:

$$\begin{aligned} & 3 c1 c3^2 i1 a3 - 4 d3 c1^2 c3^2 + c2 c3^5 + i1 c3^4 + 6 a3 c2 c3^3 c1 - 3 c3^3 c1 i3 - 9 a3 c1^2 i3 c3 \\ & - c1^2 p3 c3 + 3 a2 c1 c3^4 + 18 a2 c1^2 a3 c3^2 - 12 d3 c1^3 a3 + 9 a3^2 c2 c1^2 c3 + 27 a2 c1^3 a3^2 \\ & = 0 \end{aligned}$$

Variables to be uneliminated:

$$"p3 := 'p3'"$$

Proceed on case level 5 with:

$$6 a3 (-3 a3 c1 - c3^2) c1 (3 a3 c1 + c3^2) c3 \neq 0$$

On account of:

$$\begin{aligned} & 3 c1 c3^2 i1 a3 - 4 d3 c1^2 c3^2 + c2 c3^5 + i1 c3^4 + 6 a3 c2 c3^3 c1 - 3 c3^3 c1 i3 - 9 a3 c1^2 i3 c3 \\ & - c1^2 p3 c3 + 3 a2 c1 c3^4 + 18 a2 c1^2 a3 c3^2 - 12 d3 c1^3 a3 + 9 a3^2 c2 c1^2 c3 + 27 a2 c1^3 a3^2 \\ & = 0 \end{aligned}$$

$$\{-c1^2 c3 \neq 0\}$$

p3 is set to:

$$(3 a3 c1 + c3^2)$$

$$(9 c1^2 a2 a3 - 4 c1^2 d3 + 3 c1 c2 c3 a3 - 3 c1 c3 i3 + 3 c1 a2 c3^2 + c3^2 i1 + c2 c3^3) / (c1^2 c3)$$

> **tmp1 := cpcoeff (x1^3);**

$$tmp1 := - \frac{(c1 i3 - i1 c3)^3}{c1^3}$$

> **elimsolve (tmp1, i1);**

$$\{-c3 \neq 0\}$$

i1 is set to:

$$\frac{c1 i3}{c3}$$

> **launchNZcase (j3\*c1-j1\*c3);**

Launching case level 6:

$$j3 c1 - j1 c3 \neq 0$$

Assume from now on that:

$$6 a3 (-3 a3 c1 - c3^2) c1 (3 a3 c1 + c3^2) c3 (j3 c1 - j1 c3) \neq 0$$

> **launchNZcase (81\*a2^2\*c1^4\*a3^2-54\*a2\*c1^4\*a3\*d3+3\*c1^4\*a3\*j3 +**  
 > **8\*d3^2\*c1^4+54\*a2\*c1^3\*a3^2\*c3\*c2+54\*a2^2\*c1^3\*a3\*c3^2 -**  
 > **18\*d3\*c1^3\*c3\*c2\*a3+3\*c1^3\*a3\*c3\*s3-27\*a2\*c1^3\*a3\*c3\*i3 +**  
 > **c1^3\*j3\*c3^2+8\*d3\*c1^3\*c3\*i3-18\*d3\*c1^3\*c3^2\*a2 +**  
 > **9\*c1^2\*c3^2\*c2^2\*a3^2-9\*c1^2\*c3^2\*c2\*a3\*i3+36\*a2\*c1^2\*a3\*c2\*c3^3**

```

+
> 9*c1^2*c3^4*a2^2+2*c1^2*c3^2*i3^2+c1^2*s3*c3^3-9*c1^2*c3^3*i3*a2
-
> 6*d3*c1^2*c2*c3^3+6*c1*c3^4*c2^2*a3+6*c1*c3^5*a2*c2 -
> 3*c1*c3^4*i3*c2+c2^2*c3^6) ;

```

Launching case level 7:

$$\begin{aligned}
& 81 a^2 c l^4 a^3 - 54 c l^4 a_2 a_3 d_3 + 3 j_3 c l^4 a_3 + 8 c l^4 d_3^2 + 54 c l^3 a_2 a^3 c_2 c_3 \\
& + 54 a^2 c l^3 a_3 c_3^2 - 18 c l^3 d_3 c_2 c_3 a_3 + 3 c l^3 a_3 s_3 c_3 - 27 a_2 c l^3 a_3 i_3 c_3 + j_3 c l^3 c_3^2 \\
& + 8 c l^3 d_3 c_3 i_3 - 18 a_2 d_3 c l^3 c_3^2 + 9 c l^2 c_2^2 c_3^2 a^3 - 9 a_3 i_3 c_2 c l^2 c_3^2 \\
& + 36 c l^2 a_2 a_3 c_2 c_3^3 + 9 c_3^4 a^2 c l^2 + 2 i_3^2 c l^2 c_3^2 + s_3 c l^2 c_3^3 - 9 a_2 i_3 c l^2 c_3^3 \\
& - 6 c l^2 d_3 c_2 c_3^3 + 6 c l c_2^2 c_3^4 a_3 + 6 c l a_2 c_3^5 c_2 - 3 c l c_3^4 i_3 c_2 + c_2^2 c_3^6 \neq 0
\end{aligned}$$

Assume from now on that:

$$\begin{aligned}
& 6 a_3 (-3 a_3 c l - c_3^2) c l (3 a_3 c l + c_3^2) c_3 (j_3 c l - j_1 c_3) (81 a^2 c l^4 a^3 - 54 c l^4 a_2 a_3 d_3 \\
& + 3 j_3 c l^4 a_3 + 8 c l^4 d_3^2 + 54 c l^3 a_2 a^3 c_2 c_3 + 54 a^2 c l^3 a_3 c_3^2 - 18 c l^3 d_3 c_2 c_3 a_3 \\
& + 3 c l^3 a_3 s_3 c_3 - 27 a_2 c l^3 a_3 i_3 c_3 + j_3 c l^3 c_3^2 + 8 c l^3 d_3 c_3 i_3 - 18 a_2 d_3 c l^3 c_3^2 \\
& + 9 c l^2 c_2^2 c_3^2 a^3 - 9 a_3 i_3 c_2 c l^2 c_3^2 + 36 c l^2 a_2 a_3 c_2 c_3^3 + 9 c_3^4 a^2 c l^2 + 2 i_3^2 c l^2 c_3^2 \\
& + s_3 c l^2 c_3^3 - 9 a_2 i_3 c l^2 c_3^3 - 6 c l^2 d_3 c_2 c_3^3 + 6 c l c_2^2 c_3^4 a_3 + 6 c l a_2 c_3^5 c_2 \\
& - 3 c l c_3^4 i_3 c_2 + c_2^2 c_3^6) \neq 0
\end{aligned}$$

```

> tmp1 := cpcoeff (1) ;

```

$$\begin{aligned}
& tmp1 := - (81 a^2 c l^4 a^3 - 54 c l^4 a_2 a_3 d_3 + 3 j_3 c l^4 a_3 + 8 c l^4 d_3^2 + 54 c l^3 a_2 a^3 c_2 c_3 \\
& + 54 a^2 c l^3 a_3 c_3^2 - 18 c l^3 d_3 c_2 c_3 a_3 + 3 c l^3 a_3 s_3 c_3 - 27 a_2 c l^3 a_3 i_3 c_3 + j_3 c l^3 c_3^2 \\
& + 8 c l^3 d_3 c_3 i_3 - 18 a_2 d_3 c l^3 c_3^2 + 9 c l^2 c_2^2 c_3^2 a^3 - 9 a_3 i_3 c_2 c l^2 c_3^2 \\
& + 36 c l^2 a_2 a_3 c_2 c_3^3 + 9 c_3^4 a^2 c l^2 + 2 i_3^2 c l^2 c_3^2 + s_3 c l^2 c_3^3 - 9 a_2 i_3 c l^2 c_3^3 \\
& - 6 c l^2 d_3 c_2 c_3^3 + 6 c l c_2^2 c_3^4 a_3 + 6 c l a_2 c_3^5 c_2 - 3 c l c_3^4 i_3 c_2 + c_2^2 c_3^6) (j_3 c l - j_1 c_3) \\
& (81 a^2 c l^4 a^3 - 54 c l^4 a_2 a_3 d_3 + 8 c l^4 d_3^2 + 54 a^2 c l^3 a_3 c_3^2 + 54 c l^3 a_2 a^3 c_2 c_3 \\
& - 27 a_2 c l^3 a_3 i_3 c_3 - 18 a_2 d_3 c l^3 c_3^2 - 18 c l^3 d_3 c_2 c_3 a_3 + 3 c l^3 a_3 s_3 c_3 + 3 j_1 c l^3 a_3 c_3 \\
& + 8 c l^3 d_3 c_3 i_3 - 9 a_3 i_3 c_2 c l^2 c_3^2 + s_3 c l^2 c_3^3 + 2 i_3^2 c l^2 c_3^2 + j_1 c l^2 c_3^3 - 6 c l^2 d_3 c_2 c_3^3 \\
& + 9 c l^2 c_2^2 c_3^2 a^3 - 9 a_2 i_3 c l^2 c_3^3 + 9 c_3^4 a^2 c l^2 + 36 c l^2 a_2 a_3 c_2 c_3^3 + 6 c l c_2^2 c_3^4 a_3 \\
& + 6 c l a_2 c_3^5 c_2 - 3 c l c_3^4 i_3 c_2 + c_2^2 c_3^6) / (c_3^3 c l^4 (3 a_3 c l + c_3^2)^2)
\end{aligned}$$

```

> elimsolve (tmp1,s3) ;

```

$$\{3 a_3 c_3 c l^3 + c l^2 c_3^3 \neq 0\}$$

s3 is set to:

$$\begin{aligned}
& - (81 a^2 c l^4 a^3 - 54 c l^4 a_2 a_3 d_3 + 8 c l^4 d_3^2 + 54 a^2 c l^3 a_3 c_3^2 + 54 c l^3 a_2 a^3 c_2 c_3 \\
& - 27 a_2 c l^3 a_3 i_3 c_3 - 18 a_2 d_3 c l^3 c_3^2 - 18 c l^3 d_3 c_2 c_3 a_3 + 3 j_1 c l^3 a_3 c_3 + 8 c l^3 d_3 c_3 i_3 \\
& - 9 a_3 i_3 c_2 c l^2 c_3^2 + 2 i_3^2 c l^2 c_3^2 + j_1 c l^2 c_3^3 - 6 c l^2 d_3 c_2 c_3^3 + 9 c l^2 c_2^2 c_3^2 a^3 \\
& - 9 a_2 i_3 c l^2 c_3^3 + 9 c_3^4 a^2 c l^2 + 36 c l^2 a_2 a_3 c_2 c_3^3 + 6 c l c_2^2 c_3^4 a_3 + 6 c l a_2 c_3^5 c_2 \\
& - 3 c l c_3^4 i_3 c_2 + c_2^2 c_3^6) / (c l^2 c_3 (3 a_3 c l + c_3^2))
\end{aligned}$$

Nonzero constraint refines to:

$$6 a^3 (-3 a^3 c l - c^3)^2 c l^2 (3 a^3 c l + c^3)^2 c^3 (j^3 c l - j l c^3)^2 \neq 0$$

> **tmp1 := cpcoeff (T) ;**

$$tmp1 := - \frac{(j^3 c l - j l c^3)^2}{c^3^2}$$

> **contradict (tmp1, 's3') ;**

Contradiction on case level 7, so:

$$\begin{aligned} &81 a^2 c l^4 a^3 - 54 c l^4 a^2 a^3 d^3 + 3 j^3 c l^4 a^3 + 8 c l^4 d^3^2 + 54 c l^3 a^2 a^3^2 c^2 c^3 \\ &+ 54 a^2 c l^3 a^3 c^3^2 - 18 c l^3 d^3 c^2 c^3 a^3 + 3 c l^3 a^3 s^3 c^3 - 27 a^2 c l^3 a^3 i^3 c^3 + j^3 c l^3 c^3^2 \\ &+ 8 c l^3 d^3 c^3 i^3 - 18 a^2 d^3 c l^3 c^3^2 + 9 c l^2 c^2^2 c^3^2 a^3^2 - 9 a^3 i^3 c^2 c l^2 c^3^2 \\ &+ 36 c l^2 a^2 a^3 c^2 c^3^3 + 9 c^3^4 a^2^2 c l^2 + 2 i^3^2 c l^2 c^3^2 + s^3 c l^2 c^3^3 - 9 a^2 i^3 c l^2 c^3^3 \\ &- 6 c l^2 d^3 c^2 c^3^3 + 6 c l c^2^2 c^3^4 a^3 + 6 c l a^2 c^3^5 c^2 - 3 c l c^3^4 i^3 c^2 + c^2^2 c^3^6 = 0 \end{aligned}$$

Variables to be uneliminated:

$$s3 := 's3'$$

Proceed on case level 6 with:

$$6 a^3 (-3 a^3 c l - c^3)^2 c l (3 a^3 c l + c^3)^2 c^3 (j^3 c l - j l c^3) \neq 0$$

On account of:

$$\begin{aligned} &81 a^2 c l^4 a^3 - 54 c l^4 a^2 a^3 d^3 + 3 j^3 c l^4 a^3 + 8 c l^4 d^3^2 + 54 c l^3 a^2 a^3^2 c^2 c^3 \\ &+ 54 a^2 c l^3 a^3 c^3^2 - 18 c l^3 d^3 c^2 c^3 a^3 + 3 c l^3 a^3 s^3 c^3 - 27 a^2 c l^3 a^3 i^3 c^3 + j^3 c l^3 c^3^2 \\ &+ 8 c l^3 d^3 c^3 i^3 - 18 a^2 d^3 c l^3 c^3^2 + 9 c l^2 c^2^2 c^3^2 a^3^2 - 9 a^3 i^3 c^2 c l^2 c^3^2 \\ &+ 36 c l^2 a^2 a^3 c^2 c^3^3 + 9 c^3^4 a^2^2 c l^2 + 2 i^3^2 c l^2 c^3^2 + s^3 c l^2 c^3^3 - 9 a^2 i^3 c l^2 c^3^3 \\ &- 6 c l^2 d^3 c^2 c^3^3 + 6 c l c^2^2 c^3^4 a^3 + 6 c l a^2 c^3^5 c^2 - 3 c l c^3^4 i^3 c^2 + c^2^2 c^3^6 = 0 \\ &\{c l^2 c^3^3 + 3 a^3 c^3 c l^3 \neq 0\} \end{aligned}$$

s3 is set to:

$$\begin{aligned} &-(81 a^2 c l^4 a^3 - 54 c l^4 a^2 a^3 d^3 + 3 j^3 c l^4 a^3 + 8 c l^4 d^3^2 + 54 c l^3 a^2 a^3^2 c^2 c^3 \\ &+ 54 a^2 c l^3 a^3 c^3^2 - 18 c l^3 d^3 c^2 c^3 a^3 - 27 a^2 c l^3 a^3 i^3 c^3 + j^3 c l^3 c^3^2 + 8 c l^3 d^3 c^3 i^3 \\ &- 18 a^2 d^3 c l^3 c^3^2 + 9 c l^2 c^2^2 c^3^2 a^3^2 - 9 a^3 i^3 c^2 c l^2 c^3^2 + 36 c l^2 a^2 a^3 c^2 c^3^3 \\ &+ 9 c^3^4 a^2^2 c l^2 + 2 i^3^2 c l^2 c^3^2 - 9 a^2 i^3 c l^2 c^3^3 - 6 c l^2 d^3 c^2 c^3^3 + 6 c l c^2^2 c^3^4 a^3 \\ &+ 6 c l a^2 c^3^5 c^2 - 3 c l c^3^4 i^3 c^2 + c^2^2 c^3^6) / (c l^2 c^3 (3 a^3 c l + c^3^2)) \end{aligned}$$

> **tmp1 := cpcoeff (T) ;**

$$tmp1 := - \frac{(j^3 c l - j l c^3)^2}{c^3^2}$$

> **contradict (tmp1, 'j1') ;**

Contradiction on case level 6, so:

$$j^3 c l - j l c^3 = 0$$

Variables to be uneliminated:

$$s3 := 's3'$$

Proceed on case level 5 with:

$$6 a^3 (-3 a^3 c l - c^3)^2 c l (3 a^3 c l + c^3)^2 c^3 \neq 0$$

On account of:

$$j^3 c l - j l c^3 = 0$$

$$\{-c3 \neq 0\}$$

j1 is set to:

$$\frac{j3 \, cl}{c3}$$

> **tmp1 := cpcoeff (T) ;**

$$\begin{aligned} tmp1 := & -(81 \, a2^2 \, cl^4 \, a3^2 - 54 \, cl^4 \, a2 \, a3 \, d3 + 3 \, j3 \, cl^4 \, a3 + 8 \, cl^4 \, d3^2 + 54 \, cl^3 \, a2 \, a3^2 \, c2 \, c3 \\ & + 54 \, a2^2 \, cl^3 \, a3 \, c3^2 - 18 \, cl^3 \, d3 \, c2 \, c3 \, a3 + 3 \, cl^3 \, a3 \, s3 \, c3 - 27 \, a2 \, cl^3 \, a3 \, i3 \, c3 + j3 \, cl^3 \, c3^2 \\ & + 8 \, cl^3 \, d3 \, c3 \, i3 - 18 \, a2 \, d3 \, cl^3 \, c3^2 + 9 \, cl^2 \, c2^2 \, c3^2 \, a3^2 - 9 \, a3 \, i3 \, c2 \, cl^2 \, c3^2 \\ & + 36 \, cl^2 \, a2 \, a3 \, c2 \, c3^3 + 9 \, c3^4 \, a2^2 \, cl^2 + 2 \, i3^2 \, cl^2 \, c3^2 + s3 \, cl^2 \, c3^3 - 9 \, a2 \, i3 \, cl^2 \, c3^3 \\ & - 6 \, cl^2 \, d3 \, c2 \, c3^3 + 6 \, cl \, c2^2 \, c3^4 \, a3 + 6 \, cl \, a2 \, c3^5 \, c2 - 3 \, cl \, c3^4 \, i3 \, c2 + c2^2 \, c3^6)^2 / (cl^4 \, c3^2 \\ & (3 \, a3 \, cl + c3^2)^2) \end{aligned}$$

> **elimsolve (tmp1, s3) ;**

$$\{3 \, a3 \, c3 \, cl^3 + cl^2 \, c3^3 \neq 0\}$$

s3 is set to:

$$\begin{aligned} - & (81 \, a2^2 \, cl^4 \, a3^2 - 54 \, cl^4 \, a2 \, a3 \, d3 + 3 \, j3 \, cl^4 \, a3 + 8 \, cl^4 \, d3^2 + 54 \, cl^3 \, a2 \, a3^2 \, c2 \, c3 \\ & + 54 \, a2^2 \, cl^3 \, a3 \, c3^2 - 18 \, cl^3 \, d3 \, c2 \, c3 \, a3 - 27 \, a2 \, cl^3 \, a3 \, i3 \, c3 + j3 \, cl^3 \, c3^2 + 8 \, cl^3 \, d3 \, c3 \, i3 \\ & - 18 \, a2 \, d3 \, cl^3 \, c3^2 + 9 \, cl^2 \, c2^2 \, c3^2 \, a3^2 - 9 \, a3 \, i3 \, c2 \, cl^2 \, c3^2 + 36 \, cl^2 \, a2 \, a3 \, c2 \, c3^3 \\ & + 9 \, c3^4 \, a2^2 \, cl^2 + 2 \, i3^2 \, cl^2 \, c3^2 - 9 \, a2 \, i3 \, cl^2 \, c3^3 - 6 \, cl^2 \, d3 \, c2 \, c3^3 + 6 \, cl \, c2^2 \, c3^4 \, a3 \\ & + 6 \, cl \, a2 \, c3^5 \, c2 - 3 \, cl \, c3^4 \, i3 \, c2 + c2^2 \, c3^6) / (cl^2 \, c3 \, (3 \, a3 \, cl + c3^2)) \end{aligned}$$

> **det (T-jacobian (H, [x1, x2, x3])) ;**

$$T^3$$

> **simplify (evalm ([H[1], H[2], H[3]])) ;**

$$\begin{aligned} [ & (-18 \, cl^3 \, a3^2 \, x2 \, c3^3 \, i3 + x2 \, c3^9 \, c2 - c3^8 \, x3 \, c2^2 + 3 \, cl^3 \, a3 \, i3 \, x1 \, x3 \, c3^3 - cl^3 \, c3^4 \, x3 \, j3 \\ & + 18 \, cl^3 \, a3 \, c3^3 \, x3 \, d3 \, c2 - 54 \, cl^3 \, a3 \, c3^4 \, x3 \, a2^2 - 24 \, cl^3 \, a3 \, x2 \, c3^4 \, d3 + 81 \, cl^3 \, a3^2 \, x2 \, c3^4 \, a2 \\ & + 3 \, cl^3 \, a3 \, x1^2 \, x3 \, c3^4 - 2 \, cl^3 \, c3^5 \, x1 \, x3^2 + 3 \, cl^3 \, a3^2 \, x1^3 \, c3^3 - cl^3 \, c3^4 \, x3^2 \, i3 \\ & - 27 \, cl^3 \, a3^2 \, x1 \, x2 \, c3^4 - 54 \, cl^3 \, a3^2 \, c3^3 \, x3 \, a2 \, c2 - 3 \, cl^4 \, a3 \, c3^2 \, x3^2 \, i3 - cl^4 \, c3^3 \, x3^2 \, d3 \\ & + 27 \, cl^3 \, x2 \, c3^3 \, c2 \, a3^3 + 54 \, cl^4 \, a3 \, c3^2 \, x3 \, a2 \, d3 - 9 \, cl^4 \, a3 \, c3^3 \, x1 \, x3^2 - 3 \, cl^4 \, a3 \, c3^2 \, x3 \, j3 \\ & + cl^4 \, x3^3 \, c3^4 - 81 \, cl^4 \, a3^2 \, c3^2 \, x3 \, a2^2 + 27 \, cl^4 \, a3^2 \, c3^3 \, x2 \, x3 - 8 \, cl^4 \, c3^2 \, x3 \, d3^2 \\ & - 36 \, cl^4 \, a3^2 \, x2 \, c3^2 \, d3 + 81 \, cl^4 \, a3^3 \, x2 \, c3^2 \, a2 - 27 \, cl^4 \, a3^3 \, x1 \, x2 \, c3^2 - 3 \, cl^5 \, a3 \, c3 \, x3^2 \, d3 \\ & - 9 \, cl^5 \, c3 \, x1 \, x3^2 \, a3^2 + 5 \, cl^5 \, a3 \, x3^3 \, c3^2 + 27 \, cl^5 \, c3 \, x2 \, x3 \, a3^3 - 6 \, cl \, c3^7 \, x3 \, a2 \, c2 \\ & - 2 \, cl \, x2 \, c3^7 \, i3 + 3 \, cl \, x2 \, c3^8 \, a2 - cl \, x1 \, x2 \, c3^8 + 3 \, cl \, c3^6 \, x3 \, i3 \, c2 - 6 \, cl \, a3 \, c3^6 \, x3 \, c2^2 \\ & + 9 \, cl \, a3 \, x2 \, c3^7 \, c2 - 2 \, cl^2 \, c3^4 \, x3 \, i3^2 + cl^2 \, d3 \, x1^2 \, c3^5 - 9 \, cl^2 \, c3^6 \, x3 \, a2^2 + cl^2 \, i3 \, x1 \, x3 \, c3^5 \\ & + cl^2 \, x1^2 \, x3 \, c3^6 + cl^2 \, j3 \, x1 \, c3^5 + cl^2 \, c3^7 \, x2 \, x3 + 6 \, cl^2 \, c3^5 \, x3 \, d3 \, c2 + 27 \, cl^2 \, a3 \, x2 \, c3^6 \, a2 \\ & - 4 \, cl^2 \, x2 \, c3^6 \, d3 + 9 \, cl^2 \, c3^5 \, x3 \, a2 \, i3 - 36 \, cl^2 \, a3 \, c3^5 \, x3 \, a2 \, c2 - 12 \, cl^2 \, a3 \, x2 \, c3^5 \, i3 \\ & - 9 \, cl^2 \, a3 \, x1 \, x2 \, c3^6 + 9 \, cl^2 \, a3 \, c3^4 \, x3 \, i3 \, c2 + cl^2 \, a3 \, x1^3 \, c3^5 + 27 \, cl^2 \, a3^2 \, x2 \, c3^5 \, c2 \\ & - 9 \, cl^2 \, a3^2 \, c3^4 \, x3 \, c2^2 + 18 \, cl^3 \, c3^4 \, x3 \, a2 \, d3 + 9 \, cl^3 \, a3 \, c3^5 \, x2 \, x3 - 8 \, cl^3 \, c3^3 \, x3 \, d3 \, i3 \end{aligned}$$

$$\begin{aligned}
& + 3 c l^3 a 3 j 3 x l c 3^3 + 27 c l^3 a 3 c 3^3 x 3 a 2 i 3 + 3 c l^3 a 3 d 3 x l^2 c 3^3 + 6 x 3^3 a 3^2 c l^6) / (c l c 3^4 \\
& (3 a 3 c l + c 3^2)), - (648 c l^4 a 3^2 c 3^6 x l x 3 a 2 c 2 + 81 x 3^4 a 3^3 c l^9 - c l^2 x l^4 c 3^{10} \\
& - 972 c l^6 a 3^2 x 3^2 c 3^4 a 2^2 + 216 c l^5 a 3^2 c 3^5 x l d 2 x 3 - 36 c l^4 a 3 c 3^7 x 3 i 3 x 2 \\
& + 72 c l^4 a 3 x l c 3^7 d 3 x 2 - 96 c l^4 a 3 c 3^8 x l x 3 x 2 + 36 c l^4 a 3 x l c 3^5 i 3^2 x 3 \\
& - 216 c l^4 a 3 x 3^2 c 3^7 a 2 c 2 + 96 c l^4 a 3 x 3^2 c 3^6 i 3 c 2 + 324 c l^4 a 3 c 3^7 x l x 3 a 2^2 \\
& - 864 c l^4 a 3 c 3^6 x 3 i 3 a 2^2 + 648 c l^4 a 3 c 3^7 a 2 d 3 x 2 - 192 c l^4 a 3 c 3^6 d 3 i 3 x 2 \\
& + 180 c l^4 a 3 c 3^5 x 3 i 3^2 a 2 + 72 c l^4 a 3 c 3^7 x l x 3^2 c 2 + 72 c l^4 a 3 c 3^7 x l d 2 x 3 \\
& + 108 c l^4 a 3^3 c 3^5 c 2^2 x l x 3 + 48 c l^4 x l c 3^6 i 3 x 3 d 3 + 240 c l^4 c 3^6 x 3 i 3 a 2 d 3 \\
& - 96 c l^4 c 3^7 x l x 3 a 2 d 3 - 8 c l^4 c 3^8 x 3 d 3 x 2 + 32 c l^4 x 3^2 c 3^7 d 3 c 2 - 288 c l^4 c 3^7 x 3 d 3 a 2^2 \\
& + 80 c l^4 c 3^6 x 3 d 3^2 c 2 - 48 c l^4 c 3^5 x 3 d 3 i 3^2 + 12 c l^4 c 3^8 x 3^2 a 2 x l \\
& + 972 c l^3 a 3^2 c 3^7 x 3 c 2^2 a 2 - 36 c l^3 a 3 c 3^8 j 2 x l - 36 c l^3 a 3 c 3^8 c 2^2 x 3^2 \\
& - 48 c l^3 a 3 c 3^7 i 3^2 x 2 + 48 c l^3 a 3 x l^2 c 3^9 x 2 - 432 c l^3 a 3 c 3^9 a 2^2 x 2 \\
& + 216 c l^3 a 3 c 3^8 x l x 3 a 2 c 2 + 972 c l^3 a 3 c 3^8 x 3 a 2^2 c 2 + 216 c l^3 a 3 c 3^8 d 3 c 2 x 2 \\
& - 192 c l^3 a 3 c 3^7 c 2^2 x 3 d 3 + 324 c l^3 a 3 c 3^8 a 2 i 3 x 2 + 36 c l^3 a 3 x l c 3^8 i 3 x 2 \\
& - 576 c l^3 a 3 c 3^7 x 3 i 3 a 2 c 2 - 96 c l^3 a 3 c 3^7 x l x 3 i 3 c 2 + 60 c l^3 a 3 c 3^6 x 3 i 3^2 c 2 \\
& - 36 c l^3 a 3 c 3^8 x l^2 x 3 c 2 - 432 c l^3 a 3^3 c 3^7 c 2^2 x 2 + 108 c l^3 a 3^3 c 3^6 x 3 c 2^3 \\
& + 108 c l^3 a 3^2 c 3^7 c 2^2 x l x 3 + 324 c l^3 a 3^2 c 3^7 i 3 c 2 x 2 - 1296 c l^3 a 3^2 c 3^8 a 2 c 2 x 2 \\
& - 144 c l^3 a 3^2 c 3^6 c 2^2 x 3 i 3 - 36 c l^3 a 3 c 3^8 x l^2 d 2 + 80 c l^3 c 3^7 x 3 d 3 i 3 c 2 \\
& - 48 c l^3 c 3^8 a 2 i 3 x l x 3 - 32 c l^3 c 3^8 x l x 3 d 3 c 2 - 4 c l^3 c 3^9 x 3 i 3 x 2 - 8 c l^3 c 3^{10} x l x 3 x 2 \\
& + 8 c l^3 x l c 3^9 d 3 x 2 - 32 c l^3 c 3^8 d 3 i 3 x 2 + 36 c l^3 c 3^9 x l x 3 a 2^2 - 24 c l^3 x 3^2 c 3^9 a 2 c 2 \\
& + 16 c l^3 x 3^2 c 3^8 i 3 c 2 - 144 c l^3 c 3^8 x 3 i 3 a 2^2 - 192 c l^3 c 3^8 x 3 d 3 a 2 c 2 + 60 c l^3 c 3^7 x 3 i 3^2 a 2 \\
& + 72 c l^3 c 3^9 a 2 d 3 x 2 + 8 c l^3 c 3^9 x l d 2 x 3 + 8 c l^3 c 3^9 x 3^2 c 2 x l + 108 c l^2 a 3 c 3^9 i 3 c 2 x 2 \\
& + 36 c l^2 a 3 c 3^9 c 2^2 x l x 3 + 324 c l^2 a 3 c 3^9 x 3 c 2^2 a 2 - 96 c l^2 a 3 c 3^8 x 3 i 3 c 2^2 \\
& - 288 c l^2 a 3 c 3^{10} a 2 c 2 x 2 + 108 c l^2 a 3^2 c 3^8 x 3 c 2^3 - 216 c l^2 a 3^2 c 3^9 c 2^2 x 2 \\
& + 108 c l^2 c 3^{10} x 3 a 2^2 c 2 + 24 c l^2 c 3^{10} d 3 c 2 x 2 - 32 c l^2 c 3^9 c 2^2 x 3 d 3 + 36 c l^2 c 3^{10} a 2 i 3 x 2 \\
& + 4 c l^2 x l c 3^{10} i 3 x 2 + 20 c l^2 c 3^8 x 3 i 3^2 c 2 - 4 c l^2 c 3^{10} x l^2 x 3 c 2 - 96 c l^2 c 3^9 x 3 i 3 a 2 c 2 \\
& - 16 c l^2 c 3^9 x l x 3 i 3 c 2 + 36 c l a 3 c 3^{10} x 3 c 2^3 - 48 c l a 3 c 3^{11} c 2^2 x 2 + 36 c l c 3^{11} x 3 c 2^2 a 2 \\
& + 4 c l c 3^{11} c 2^2 x l x 3 + 12 c l c 3^{11} i 3 c 2 x 2 - 24 c l c 3^{12} a 2 c 2 x 2 - 16 c l c 3^{10} x 3 i 3 c 2^2 \\
& - 288 c l^5 a 3^2 c 3^4 x l x 3 d 3 c 2 - 72 c l^5 a 3 c 3^6 x 3 d 3 x 2 + 192 c l^5 a 3 x 3^2 c 3^5 d 3 c 2 \\
& - 1728 c l^5 a 3 c 3^5 x 3 d 3 a 2^2 + 240 c l^5 a 3 c 3^4 x 3 d 3^2 c 2 + 144 c l^5 a 3 x l c 3^4 i 3 x 3 d 3 \\
& - 576 c l^5 a 3 c 3^5 x l x 3 a 2 d 3 + 720 c l^5 a 3 c 3^4 x 3 d 3 a 2 i 3 + 108 c l^5 a 3 c 3^6 x 3^2 a 2 x l \\
& + 288 c l^5 a 3 x 3^2 c 3^5 a 2 i 3 - 3888 c l^5 a 3^3 c 3^5 a 2^2 x 2 - 108 c l^5 a 3^3 c 3^4 j 2 x l \\
& - 108 c l^5 a 3^3 c 3^4 c 2^2 x 3^2 - 108 c l^5 a 3^3 c 3^4 x l^2 d 2 + 432 c l^5 a 3^3 x l^2 c 3^5 x 2 \\
& + 108 c l^5 a 3^2 c 3^5 j 2 x 3 + 2916 c l^5 a 3^2 c 3^5 x 3 a 2^3 + 48 c l^5 a 3 x 3^2 c 3^7 x 2 \\
& + 54 c l^5 a 3 x 3^2 c 3^6 x l^2 - 36 c l^5 a 3 c 3^6 x 3^2 d 2 - 192 c l^5 a 3 c 3^5 d 3^2 x 2 - 36 c l^5 a 3 x 3^2 c 3^4 i 3^2
\end{aligned}$$

$$\begin{aligned}
& -324 c l^5 a^3 x^3 c^3 a^2 - 1944 c l^5 a^3 c^3 a^2 c_2 x_2 + 108 c l^5 a^3 x l c^3 i_3 x_2 \\
& + 2916 c l^5 a^3 c^3 x_3 a^2 c_2 + 972 c l^5 a^3 c^3 a_2 i_3 x_2 + 648 c l^5 a^3 c^3 d_3 c_2 x_2 \\
& + 648 c l^5 a^3 c^3 x l x_3 a_2 c_2 - 108 c l^5 a^3 c_2 x l^2 c^3 x_3 - 108 c l^5 a^3 c^3 x_3 i_3 x_2 \\
& + 216 c l^5 a^3 x l c^3 d_3 x_2 - 432 c l^5 a^3 c^3 x l x_3 x_2 - 648 c l^5 a^3 x^3 c^3 a_2 c_2 \\
& + 144 c l^5 a^3 x^3 c^3 i_3 c_2 + 1944 c l^5 a^3 c^3 a_2 d_3 x_2 - 288 c l^5 a^3 c^3 d_3 i_3 x_2 \\
& + 972 c l^5 a^3 c^3 x l x_3 a_2^2 - 1728 c l^5 a^3 c^3 x_3 d_3 a_2 c_2 - 432 c l^5 a^3 c^3 x l x_3 a_2 i_3 \\
& - 48 c l^5 c^3 x^3 i_3 d_3 + 48 c l^5 x l c^3 d_3^2 x_3 + 240 c l^5 c^3 x_3 d_3^2 a_2 - 96 c l^5 c^3 x_3 d_3^2 i_3 \\
& - 144 c l^4 a^3 c^3 x l x_3 i_3 c_2 - 864 c l^4 a^3 c^3 x_3 i_3 a_2 c_2 + 2916 c l^4 a^3 c^3 x_3 a_2^2 c_2 \\
& + 648 c l^4 a^3 c^3 d_3 c_2 x_2 - 288 c l^4 a^3 c^3 c_2^2 x_3 d_3 + 108 c l^4 a^3 x l c^3 i_3 x_2 \\
& + 972 c l^4 a^3 c^3 a_2 i_3 x_2 - 108 c l^4 a^3 c^3 x l^2 x_3 c_2 - 1152 c l^4 a^3 c^3 x_3 d_3 a_2 c_2 \\
& - 288 c l^4 a^3 c^3 x l x_3 a_2 i_3 - 192 c l^4 a^3 c^3 x l x_3 d_3 c_2 + 240 c l^4 a^3 c^3 x_3 d_3 i_3 c_2 \\
& - 108 c l^4 a^3 c^3 x l^2 d_2 - 108 c l^4 a^3 c^3 j_2 x l - 1944 c l^4 a^3 c^3 a_2^2 x_2 \\
& - 72 c l^4 a^3 c^3 i_3^2 x_2 + 972 c l^4 a^3 c^3 x_3 a_2^3 + 36 c l^4 a^3 c^3 j_2 x_3 - 324 c l^4 c^3 c_2^2 x_2 a_3^4 \\
& + 324 c l^4 a^3 c^3 i_3 c_2 x_2 - 108 c l^4 a^3 c^3 c_2^2 x_3^2 + 216 c l^4 a^3 x l^2 c^3 x_2 \\
& + 972 c l^4 a^3 c^3 x_3 c_2^2 a_2 - 2592 c l^4 a^3 c^3 a_2 c_2 x_2 - 288 c l^6 a^3 c^3 d_3^2 x_2 \\
& - 108 c l^6 a^3 c^3 x^3 d_2 - 72 c l^6 a^3 c^3 x_3 a_2 - 72 c l^6 a^3 x_3^3 c^3 x l \\
& - 1296 c l^5 a^3 c^3 x_3 i_3 a_2^2 + 216 c l^5 a^3 c^3 x l x_3^2 c_2 + 81 c l^8 a^3 x^4 c^3^2 \\
& + 27 c l^7 a^3 x^4 c^3 - 64 c l^6 c^3 x_3 d_3^3 - 48 c l^6 c^3 x^3 d_3^2 - 8 c l^5 x^3 c^3 x l \\
& - 8 c l^5 c^3 x_3^3 a_2 + 4 c l^4 x^3 c^3 x_2 + 6 c l^4 x^3 c^3 x l^2 - 27 c l^4 a^3 x l^4 c^3^6 \\
& - 4 c l^4 c^3 x^3 d_2 - 32 c l^4 c^3 d_3^2 x_2 - 9 c l^3 a^3 x l^4 c^3^8 - 8 c l^3 c^3 x_3 i_3^3 \\
& + 108 c l^3 c^3 x_3 a_2^3 + 4 c l^3 c^3 j_2 x_3 - 4 c l^2 c^3 j_2 x l - 4 c l^2 c^3 c_2^2 x_3^2 - 8 c l^2 c^3 i_3^2 x_2 \\
& + 4 c l^2 x l^2 c^3^11 x_2 - 36 c l^2 c^3^11 a_2^2 x_2 - 4 c l^2 c^3^10 x l^2 d_2 + 324 c l^8 x^3 x_2 c_3 a_3^4 \\
& - 216 c l^8 a^3 x^3 c_3 x l - 216 c l^8 a^3 c_3 x_3^3 a_2 - 648 c l^7 a^3 c^3 x l x_3 x_2 \\
& - 972 c l^7 a^3 x^3 c^3 a_2^2 - 216 c l^7 a^3 c^3 x_3 d_3 x_2 - 108 c l^7 a^3 c^3 x^3 d_2 \\
& + 162 c l^7 a^3 x l^2 c^3 x_3^2 + 432 c l^7 a^3 x^3 c^3 x_2 + 324 c l^7 a^3 c^3 x^3 a_2 x l \\
& - 216 c l^7 a^3 c^3 x_3^3 a_2 - 216 c l^7 a^3 x^3 c^3 x l + 864 c l^7 a^3 x^3 c^3 a_2 d_3 \\
& - 144 c l^7 a^3 c^3 x^3 d_3^2 + 432 c l^6 a^3 x^3 c^3 a_2 i_3 + 288 c l^6 a^3 x^3 c^3 d_3 c_2 \\
& + 324 c l^6 a^3 c^3 x^3 a_2 x l + 720 c l^6 a^3 c^3 x_3 d_3^2 a_2 + 576 c l^6 a^3 x^3 c^3 a_2 d_3 \\
& - 144 c l^6 a^3 x^3 c^3 d_3 i_3 + 144 c l^6 a^3 x l c^3 d_3^2 x_3 + 216 c l^6 a^3 c^3 x^3 c_2 x l \\
& - 864 c l^6 a^3 c^3 x l x_3 x_2 + 1944 c l^6 a^3 c^3 a_2 d_3 x_2 + 216 c l^6 a^3 c^3 x l d_2 x_3 \\
& + 972 c l^6 a^3 c^3 x l x_3 a_2^2 - 648 c l^6 a^3 x^3 c^3 a_2 c_2 - 108 c l^6 a^3 c^3 x_3 i_3 x_2 \\
& + 216 c l^6 a^3 x l c^3 d_3 x_2 - 216 c l^6 a^3 c^3 x_3 d_3 x_2 - 2592 c l^6 a^3 c^3 x_3 d_3 a_2^2 \\
& - 864 c l^6 a^3 c^3 x l x_3 a_2 d_3 - 2916 c l^6 a^3 c^3 a_2^2 x_2 + 324 c l^6 a^3 x l^2 c^3 x_2 \\
& + 108 c l^6 a^3 c^3 j_2 x_3 + 2916 c l^6 a^3 c^3 x_3 a_2^3 + 216 c l^6 a^3 x^3 c^3 x_2 \\
& + 162 c l^6 a^3 x^3 x l^2 c^3 - 4 c^3^13 c_2^2 x_2 + 4 c^3^12 x_3 c_2^3 - 27 c l^5 a^3 x l^4 c^3^4
\end{aligned}$$

$$\begin{aligned}
& -12 c l^4 c^3 x^2 i^2 - 36 c l^4 c^3 x^2 a^2 - 4 c l^4 c^3 x^3 c^2 - 4 c l^2 a^2 x l^3 c^3^{10} \\
& -108 c l^7 a^3 c^3 x^3 c^2 - 108 c l^6 a^3 c^3 x^3 c^2 + 96 c l^5 c^3 x^2 a^2 d^3 + 3 c l^6 x^3 c^3^6 \\
& -108 c l^5 a^3 a^2 x l^3 c^3^4 - 36 c l^5 a^3 c^3 x^3 c^2 + 48 c l^4 c^3 x^2 a^2 i^3 - 108 c l^4 a^3 a^2 x l^3 c^3^6 \\
& + 12 c l^3 c^3 x l x^3 i^2 - 36 c l^3 a^3 a^2 x l^3 c^3^8 + 24 c l^2 c^3^{10} x l x^3 a^2 c^2) / (4 c^3^4 c l^2 \\
& (3 a^3 c l + c^3^2)^3), (-18 c l^3 a^3 x^2 c^3^3 i^3 + x^2 c^3^9 c^2 - c^3^8 x^3 c^2^2 + 3 c l^3 a^3 i^3 x l x^3 c^3^3 \\
& - c l^3 c^3^4 x^3 j^3 + 18 c l^3 a^3 c^3^3 x^3 d^3 c^2 - 54 c l^3 a^3 c^3^4 x^3 a^2^2 - 24 c l^3 a^3 x^2 c^3^4 d^3 \\
& + 81 c l^3 a^3 x^2 c^3^4 a^2 + 3 c l^3 a^3 x l^2 x^3 c^3^4 - 2 c l^3 c^3^5 x l x^3^2 + 3 c l^3 a^3^2 x l^3 c^3^3 \\
& - c l^3 c^3^4 x^2 i^3 - 27 c l^3 a^3 x l x^2 c^3^4 - 54 c l^3 a^3^2 c^3^3 x^3 a^2 c^2 - 3 c l^4 a^3 c^3^2 x^2 i^3 \\
& - c l^4 c^3^3 x^2 d^3 + 27 c l^3 x^2 c^3^3 c^2 a^3^3 + 54 c l^4 a^3 c^3^2 x^3 a^2 d^3 - 9 c l^4 a^3 c^3^3 x l x^3^2 \\
& - 3 c l^4 a^3 c^3^2 x^3 j^3 + c l^4 x^3^3 c^3^4 - 81 c l^4 a^3^2 c^3^2 x^3 a^2^2 + 27 c l^4 a^3^2 c^3^3 x^2 x^3 \\
& - 8 c l^4 c^3^2 x^3 d^3^2 - 36 c l^4 a^3^2 x^2 c^3^2 d^3 + 81 c l^4 a^3^3 x^2 c^3^2 a^2 - 27 c l^4 a^3^3 x l x^2 c^3^2 \\
& - 3 c l^5 a^3 c^3 x^3^2 d^3 - 9 c l^5 c^3 x l x^3^2 a^3^2 + 5 c l^5 a^3 x^3^3 c^3^2 + 27 c l^5 c^3 x^2 x^3 a^3^3 \\
& - 6 c l c^3^7 x^3 a^2 c^2 - 2 c l x^2 c^3^7 i^3 + 3 c l x^2 c^3^8 a^2 - c l x l x^2 c^3^8 + 3 c l c^3^6 x^3 i^3 c^2 \\
& - 6 c l a^3 c^3^6 x^3 c^2^2 + 9 c l a^3 x^2 c^3^7 c^2 - 2 c l^2 c^3^4 x^3 i^3^2 + c l^2 d^3 x l^2 c^3^5 - 9 c l^2 c^3^6 x^3 a^2^2 \\
& + c l^2 i^3 x l x^3 c^3^5 + c l^2 x l^2 x^3 c^3^6 + c l^2 j^3 x l c^3^5 + c l^2 c^3^7 x^2 x^3 + 6 c l^2 c^3^5 x^3 d^3 c^2 \\
& + 27 c l^2 a^3 x^2 c^3^6 a^2 - 4 c l^2 x^2 c^3^6 d^3 + 9 c l^2 c^3^5 x^3 a^2 i^3 - 36 c l^2 a^3 c^3^5 x^3 a^2 c^2 \\
& - 12 c l^2 a^3 x^2 c^3^5 i^3 - 9 c l^2 a^3 x l x^2 c^3^6 + 9 c l^2 a^3 c^3^4 x^3 i^3 c^2 + c l^2 a^3 x l^3 c^3^5 \\
& + 27 c l^2 a^3^2 x^2 c^3^5 c^2 - 9 c l^2 a^3^2 c^3^4 x^3 c^2^2 + 18 c l^3 c^3^4 x^3 a^2 d^3 + 9 c l^3 a^3 c^3^5 x^2 x^3 \\
& - 8 c l^3 c^3^3 x^3 d^3 i^3 + 3 c l^3 a^3 j^3 x l c^3^3 + 27 c l^3 a^3 c^3^3 x^3 a^2 i^3 + 3 c l^3 a^3 d^3 x l^2 c^3^3 \\
& + 6 x^3^3 a^3^2 c l^6) / (c l^2 c^3^3 (3 a^3 c l + c^3^2))]
\end{aligned}$$

> **factor(c3\*H[1]-c1\*H[3]);**

0

> **M := evalm([ [1/c3\*C, 0, -c1\*C/c3^2], [c3^2/C, 0, 0],**  
 > **[0, 3\*a3\*c1+c3^2, (-6\*c1\*c2\*c3\*a3-18\*c1^2\*a2\*a3+**  
 > **6\*c1^2\*d3-2\*c2\*c3^3-6\*c1\*a2\*c3^2+3\*c3\*i3\*c1) /**  
 > **(3\*a3\*c1+c3^2) ] ] );**

M:=

$$\begin{bmatrix} \frac{C}{c^3}, 0, -\frac{c l C}{c^3^2} \\ \frac{c^3^2}{C}, 0, 0 \\ 0, 3 a^3 c l + c^3^2, \\ \frac{-6 c l c^2 c^3 a^3 - 18 c l^2 a^2 a^3 + 6 c l^2 d^3 - 2 c^2 c^3^3 - 6 c l a^2 c^3^2 + 3 c l c^3 i^3}{3 a^3 c l + c^3^2} \end{bmatrix}$$

> **factor(det (M));**

$$-c l (3 a^3 c l + c^3^2)$$

```
> G := simplify(evalm(M&*subs({seq([x1,x2,x3][i]=
> evalm(M^(-1)&*[x1,x2,x3])[i],i=1..n)},H)));
```

$$\begin{aligned}
G := & [0, -(-6cl^5c^4a_2x_2c_2 - 4cl^3c^7C^2c_2x_1i_3 - cl^3c^6C^3c_2x_3 \\
& + 4cl^3c^4C^4c_2x_2i_3 + 2cl^3C^3x_2c_3^6x_1c_2 + 6cl^3a_3c^7C^2c_2^2x_1 + 6cl^3c^8C^2a_2x_1c_2 \\
& - 2cl^3c^9Cx_1^2c_2 + 12cl^2c^3C^4i_3x_2a_2 - 8cl^2c^6C^2d_3x_1c_2 - 6cl^3a_3c^4C^4c_2^2x_2 \\
& + 4cl^2c^5C^2i_3^2x_1 - cl^2c^6x_1^2C^2x_2 - 4cl^2C^3x_2c_3^4x_1i_3 + 6cl^2C^3x_2c_3^5x_1a_2 \\
& - 6cl^2c^8Cx_1^2a_2 + 4cl^2c^7Cx_1^2i_3 - 4cl^2c^3C^4i_3^2x_2 - 12cl^2c^6C^2i_3x_1a_2 \\
& - 12cl^2a_3c^7Cx_1^2c_2 + 2cl^2c^4C^3i_3x_3 - 3cl^2c^5C^3a_2x_3 + 12cl^2a_3C^3x_2c_3^4x_1c_2 \\
& - 6cl^2a_3c^4C^3c_2x_3 - 36cl^2a_3c^3C^4a_2x_2c_2 + 12cl^2a_3c^3C^4c_2x_2i_3 + cl^2c^9x_1^3 \\
& + 36cl^2a_3c^6C^2a_2x_1c_2 - 9cl^2c^4C^4a_2^2x_2 + cl^2c^6C^2x_3x_1 - 9cl^2a_3^2c^3C^4c_2^2x_2 \\
& - 12cl^2a_3c^5C^2c_2x_1i_3 + 9cl^2c^7C^2a_2^2x_1 - 16cl^3c^3C^4d_3x_2i_3 \\
& + 16cl^3c^4C^2d_3x_1i_3 + 8cl^2c^3C^4d_3x_2c_2 + 9cl^2a_3^2c^5C^2c_2^2x_1 \\
& - 54cl^3a_3^2c^3C^4a_2x_2c_2 - 24cl^3c^5C^2d_3x_1a_2 + 24cl^3c^3C^4d_3x_2a_2 \\
& - 9cl^3a_3^2c^3C^3c_2x_3 + 54cl^3a_3^2c^4C^2a_2x_1c_2 - 18cl^3a_3^2c^5Cx_1^2c_2 \\
& - 8cl^3C^3x_2c_3^3x_1d_3 - 12cl^3a_3C^3x_2c_3^2x_1i_3 + 24cl^3a_3c^3C^4d_3x_2c_2 \\
& + 18cl^3a_3^2C^3x_2c_3^2x_1c_2 - 36cl^3a_3c^6Cx_1^2a_2 - 24cl^3a_3c^4C^2d_3x_1c_2 \\
& + 6cl^3a_3c^4C^2x_3x_1 + 6cl^3a_3c^3C^3i_3x_3 - 54cl^3a_3c^3C^4a_2^2x_2 \\
& + 54cl^3a_3c^5C^2a_2^2x_1 - 36cl^3a_3c^4C^2a_2x_1i_3 - 6cl^3a_3C^2x_2c_3^4x_1^2 \\
& + 36cl^3a_3c^3C^4a_2x_2i_3 + 36cl^3a_3C^3x_2c_3^3x_1a_2 - cl^3c^5C^2j_3x_1 + 7cl^3c^6Cx_1^2d_3 \\
& - 18cl^3a_3c^3C^3a_2x_3 + 12cl^3a_3c^5Cx_1^2i_3 - 3cl^4a_3c^3C^2j_3x_1 \\
& + 72cl^4a_3C^4a_2x_2d_3 + 21cl^4a_3c^4Cx_1^2d_3 + 16cl^4c^3C^2d_3^2x_1 + 4cl^3c^3C^3d_3x_3 \\
& - 72cl^4a_3c^3C^2a_2x_1d_3 - 24cl^4a_3C^3x_2c_3x_1d_3 + 12cl^4a_3c^3C^3d_3x_3 \\
& - 27cl^4a_3^2c^3C^3a_2x_3 + 81cl^4a_3^2c^3C^2a_2^2x_1 - 81cl^4a_3^2C^4a_2^2x_2 \\
& + 9cl^4a_3^2c^3C^2x_3x_1 + 54cl^4a_3^2C^3x_2c_3x_1a_2 - 9cl^4a_3^2C^2x_2c_3^2x_1^2 \\
& - 54cl^4a_3^2c^4Cx_1^2a_2 - 16cl^4C^4d_3^2x_2 + 6cl^4a_3^2c^5x_1^3 + 5cl^3a_3c^7x_1^3 \\
& - c^6C^4c_2^2x_2 + c^9C^2c_2^2x_1) / (cl^2c^3(3a_3cl + c^3^2)C^4), -(-4c^3^{12}C^3c_2^3x_1 \\
& + 4c^9C^5c_2^3x_2 + 3cl^3c^{12}x_1^4 - 256cl^6C^5d_3^3x_2 + 81cl^6a_3^3c^6x_1^4 \\
& + 81cl^5a_3^2c^8x_1^4 + 27cl^4a_3c^{10}x_1^4 + 256cl^6c^3C^3d_3^3x_1 + 2916cl^6a_3^3C^5a_2^3x_2 \\
& - 108cl^6a_3^3c^4C^2d_2x_1^2 + 972cl^6a_3^3c^3C^4a_2^2x_3 - 2916cl^6a_3^3c^3C^3a_2^3x_1 \\
& - 2916cl^6a_3^3c^3C^4x_2a_2^2x_1 + 2916cl^6a_3^3c^4C^2a_2^2x_1^2 - 864cl^6a_3^3c^5Cx_1^3a_2 \\
& + 108cl^6a_3^3c^3C^2x_3x_1^2 - 108cl^6a_3^3c^3C^3j_2x_1 - 108cl^6a_3^3C^2x_2c_3^3x_1^3 \\
& - 648cl^6a_3^3a_2c^3C^3x_3x_1 + 972cl^6a_3^3c^3C^3x_2x_1^2a_2 - 864cl^6a_3^2c^3C^4a_2d_3x_3 \\
& + 216cl^6a_3^2a_2c^3C^3j_3x_1 + 360cl^6a_3^2c^5Cx_1^3d_3 + 288cl^6a_3^2c^3C^3d_3x_3x_1 \\
& - 3888cl^6a_3^2C^5a_2^2x_2d_3 + 2592cl^6a_3^2C^4x_2c_3d_3x_1a_2 - 432cl^6a_3^2c^3C^3x_2x_1^2d_3 \\
& - 2376cl^6a_3^2c^4C^2d_3x_1^2a_2 + 3888cl^6a_3^2c^3C^3a_2^2x_1d_3 + 192cl^6a_3c^3C^4d_3^2x_3
\end{aligned}$$

$$\begin{aligned}
& + 504 c l^6 a_3 d_3^2 c_3^4 C^2 x l^2 + 1728 c l^6 a_3 C^5 a_2 d_3^2 x_2 - 72 c l^6 a_3 d_3 c_3^3 C^3 j_3 x l \\
& - 576 c l^6 a_3 d_3^2 C^4 x_2 c_3 x l - 1728 c l^6 a_3 c_3^3 C^3 a_2 d_3^2 x l + 64 c l^5 c_3^3 C^4 d_3^2 x_3 \\
& + 168 c l^5 d_3^2 c_3^6 C^2 x l^2 + 384 c l^5 c_3^4 C^3 d_3^2 x l i_3 - 24 c l^5 d_3 c_3^5 C^3 j_3 x l \\
& - 384 c l^5 c_3 C^5 d_3^2 x_2 i_3 - 192 c l^5 d_3^2 C^4 x_2 c_3^3 x l - 576 c l^5 c_3^5 C^3 a_2 d_3^2 x l \\
& + 576 c l^5 c_3^2 C^5 a_2 d_3^2 x_2 + 648 c l^5 a_3^3 c_3^2 C^4 a_2 c_2 x_3 + 1944 c l^5 a_3^3 c_3^5 C^2 a_2 c_2 x l^2 \\
& - 252 c l^5 a_3^3 c_3^6 C x l^3 c_2 - 2916 c l^5 a_3^3 c_3^4 C^3 a_2^2 x l c_2 - 1944 c l^5 a_3^3 c_3^2 C^4 x_2 c_2 a_2 x l \\
& - 216 c l^5 a_3^3 c_2 c_3^3 C^3 x_3 x l + 2916 c l^5 a_3^3 c_3 C^5 a_2^2 x_2 c_2 + 324 c l^5 a_3^3 c_3^3 C^3 x_2 x l^2 c_2 \\
& - 108 c l^5 a_3^2 c_3^5 C^3 j_2 x l - 936 c l^5 a_3^2 c_3^7 C x l^3 a_2 + 180 c l^5 a_3^2 c_3^6 C x l^3 i_3 \\
& + 972 c l^5 a_3^2 c_3^3 C^4 a_2^2 x_3 - 108 c l^5 a_3^2 c_3^6 C^2 d_2 x l^2 + 2916 c l^5 a_3^2 c_3^6 C^2 a_2^2 x l^2 \\
& - 108 c l^5 a_3^2 C^2 x_2 c_3^5 x l^3 - 2916 c l^5 a_3^2 c_3^5 C^3 a_2^3 x l + 2916 c l^5 a_3^2 c_3^2 C^5 a_2^3 x_2 \\
& + 972 c l^5 a_3^2 c_3^4 C^3 x_2 x l^2 a_2 - 216 c l^5 a_3^2 c_3^3 C^3 x_2 x l^2 i_3 - 1944 c l^5 a_3^2 c_3 C^5 a_2^2 x_2 i_3 \\
& + 1944 c l^5 a_3^2 c_3^4 C^3 a_2^2 x l i_3 - 432 c l^5 a_3^2 c_3^2 C^4 a_2 i_3 x_3 - 2916 c l^5 a_3^2 c_3^3 C^4 x_2 a_2^2 x l \\
& + 72 c l^5 a_3^2 c_2 c_3^4 C^3 j_3 x l - 792 c l^5 a_3^2 c_3^5 C^2 d_3 x l^2 c_2 - 1296 c l^5 a_3^2 c_3^5 C^2 i_3 x l^2 a_2 \\
& - 648 c l^5 a_3^2 a_2 c_3^4 C^3 x_3 x l + 144 c l^5 a_3^2 c_3^3 C^3 i_3 x_3 x l - 288 c l^5 a_3^2 c_3^2 C^4 d_3 c_2 x_3 \\
& + 108 c l^5 a_3^2 c_3^5 C^2 x_3 x l^2 + 2592 c l^5 a_3^2 c_3^4 C^3 a_2 d_3 x l c_2 \\
& + 1296 c l^5 a_3^2 C^4 x_2 c_3^2 i_3 x l a_2 - 2592 c l^5 a_3^2 c_3 C^5 a_2 d_3 x_2 c_2 \\
& + 864 c l^5 a_3^2 C^4 x_2 c_3^2 d_3 x l c_2 + 192 c l^5 a_3 c_3^4 C^3 d_3 x_3 x l - 36 c l^5 a_3 c_3^4 i_3 C^3 j_3 x l \\
& - 576 c l^5 a_3 d_3 C^4 x_2 c_3^2 x l i_3 + 1728 c l^5 a_3 c_3 C^5 a_2 d_3 x_2 i_3 \\
& - 1584 c l^5 a_3 c_3^6 C^2 d_3 x l^2 a_2 - 576 c l^5 a_3 c_3^3 C^4 a_2 d_3 x_3 + 144 c l^5 a_3 a_2 c_3^5 C^3 j_3 x l \\
& + 192 c l^5 a_3 c_3^2 C^4 d_3 i_3 x_3 - 288 c l^5 a_3 c_3^4 C^3 x_2 x l^2 d_3 + 264 c l^5 a_3 c_3^7 C x l^3 d_3 \\
& + 540 c l^5 a_3 d_3 c_3^5 C^2 x l^2 i_3 + 2592 c l^5 a_3 c_3^5 C^3 a_2^2 x l d_3 - 1728 c l^5 a_3 c_3^4 C^3 a_2 d_3 x l i_3 \\
& - 576 c l^5 a_3 c_3^4 C^3 d_3^2 x l c_2 + 576 c l^5 a_3 c_3 C^5 d_3^2 x_2 c_2 + 1728 c l^5 a_3 C^4 x_2 c_3^3 d_3 x l a_2 \\
& - 2592 c l^5 a_3 c_3^2 C^5 a_2^2 x_2 d_3 + 48 c l^4 c_3^9 C x l^3 d_3 - 192 c l^4 c_3^6 C^3 d_3^2 x l c_2 \\
& - 48 c l^4 c_3^6 C^3 x_2 x l^2 d_3 - 96 c l^4 c_3^5 C^4 a_2 d_3 x_3 - 264 c l^4 c_3^8 C^2 d_3 x l^2 a_2 \\
& + 24 c l^4 a_2 c_3^7 C^3 j_3 x l + 192 c l^4 c_3^3 C^5 d_3^2 x_2 c_2 - 192 c l^4 c_3^2 C^5 d_3 i_3^2 x_2 \\
& + 432 c l^4 c_3^7 C^3 a_2^2 x l d_3 + 192 c l^4 c_3^5 C^3 d_3 i_3^2 x l + 288 c l^4 C^4 x_2 c_3^5 d_3 x l a_2 \\
& - 576 c l^4 c_3^6 C^3 a_2 d_3 x l i_3 - 192 c l^4 d_3 C^4 x_2 c_3^4 x l i_3 + 576 c l^4 c_3^3 C^5 a_2 d_3 x_2 i_3 \\
& + 180 c l^4 d_3 c_3^7 C^2 x l^2 i_3 - 432 c l^4 c_3^4 C^5 a_2^2 x_2 d_3 + 32 c l^4 c_3^6 C^3 d_3 x_3 x l \\
& - 12 c l^4 c_3^6 i_3 C^3 j_3 x l + 64 c l^4 c_3^4 C^4 d_3 i_3 x_3 + 108 c l^4 a_3^3 c_3^3 C^4 c_2^2 x_3 \\
& + 972 c l^4 a_3^3 c_3^2 C^5 a_2 c_2^2 x_2 + 324 c l^4 a_3^3 c_3^6 C^2 c_2^2 x l^2 - 324 c l^4 a_3^3 c_3^3 C^4 x_2 c_2^2 x l \\
& - 972 c l^4 a_3^3 c_3^5 C^3 a_2 c_2^2 x l + 2916 c l^4 a_3^2 c_3^3 C^5 a_2^2 x_2 c_2 \\
& - 1296 c l^4 a_3^2 c_3^2 C^5 a_2 c_2 x_2 i_3 - 276 c l^4 a_3^2 c_3^8 C x l^3 c_2 + 1944 c l^4 a_3^2 c_3^7 C^2 a_2 c_2 x l^2 \\
& - 1944 c l^4 a_3^2 c_3^4 C^4 x_2 c_2 a_2 x l + 1296 c l^4 a_3^2 c_3^5 C^3 a_2 c_2 x l i_3 \\
& - 216 c l^4 a_3^2 c_2 c_3^5 C^3 x_3 x l + 432 c l^4 a_3^2 C^4 x_2 c_3^3 i_3 x l c_2 + 324 c l^4 a_3^2 c_3^5 C^3 x_2 x l^2 c_2 \\
& - 432 c l^4 a_3^2 c_3^2 C^5 d_3 c_2^2 x_2 - 432 c l^4 a_3^2 c_3^6 C^2 i_3 x l^2 c_2 + 648 c l^4 a_3^2 c_3^4 C^4 a_2 c_2 x_3
\end{aligned}$$

$$\begin{aligned}
& -144 c l^4 a^3 c^3 C^4 i^3 c_2 x_3 + 432 c l^4 a^3 c^3 C^3 d_3 c_2^2 x_1 - 2916 c l^4 a^3 c^3 C^3 a_2^2 x_1 c_2 \\
& - 336 c l^4 a^3 c^3 C x l^3 a_2 + 132 c l^4 a^3 c^3 C x l^3 i^3 + 36 c l^4 a^3 c^3 C^2 x_3 x l^2 \\
& + 972 c l^4 a^3 c^3 C^5 a_2^3 x_2 + 324 c l^4 a^3 c^3 C^4 a_2^2 x_3 - 36 c l^4 a^3 c^3 C^2 d_2 x l^2 \\
& + 972 c l^4 a^3 c^3 C^2 a_2^2 x l^2 - 36 c l^4 a^3 c^3 C^3 j_2 x_1 + 48 c l^4 a^3 c^3 C^4 i^3 x_3 \\
& + 144 c l^4 a^3 c^3 i^3 C^2 x l^2 - 36 c l^4 a^3 C^2 x_2 c_3^7 x l^3 - 972 c l^4 a^3 c^3 C^3 a_2^3 x_1 \\
& + 576 c l^4 a^3 c^3 C^5 d_3 c_2 x_2 i^3 + 1728 c l^4 a^3 c^3 C^3 a_2 d_3 x_1 c_2 \\
& + 864 c l^4 a^3 C^4 x_2 c_3^4 i^3 x_1 a_2 - 1728 c l^4 a^3 c^3 C^5 a_2 d_3 x_2 c_2 \\
& - 576 c l^4 a^3 c^3 C^3 d_3 c_2 x_1 i^3 - 864 c l^4 a^3 c^3 C^2 i^3 x l^2 a_2 - 216 c l^4 a^3 a_2 c^3 C^3 x_3 x_1 \\
& - 528 c l^4 a^3 c^3 C^2 d_3 x l^2 c_2 + 96 c l^4 a^3 c^3 C^3 i^3 x_3 x_1 - 432 c l^4 a^3 c^3 C^3 a_2 i^3 x_1 \\
& - 192 c l^4 a^3 c^3 C^4 d_3 c_2 x_3 + 48 c l^4 a^3 c_2 c^3 C^3 j_3 x_1 - 144 c l^4 a^3 c^3 i^3 C^4 x_2 x_1 \\
& - 288 c l^4 a^3 c^3 C^4 a_2 i^3 x_3 + 432 c l^4 a^3 c^3 C^5 a_2 i^3 x_2 + 324 c l^4 a^3 c^3 C^3 x_2 x l^2 a_2 \\
& + 1296 c l^4 a^3 c^3 C^3 a_2^2 x_1 i^3 - 972 c l^4 a^3 c^3 C^4 x_2 a_2^2 x_1 - 144 c l^4 a^3 c^3 C^3 x_2 x l^2 i^3 \\
& - 1296 c l^4 a^3 c^3 C^5 a_2^2 x_2 i^3 + 576 c l^4 a^3 C^4 x_2 c_3^4 d_3 x_1 c_2 - 4 c l^3 c^3 x l^3 C^2 x_2 \\
& + 32 c l^3 c^3 C^3 i^3 x_1 + 108 c l^3 c^3 C^5 a_2^3 x_2 + 36 c l^3 c^3 C^4 a_2^2 x_3 - 4 c l^3 c^3 C^2 d_2 x l^2 \\
& + 16 c l^3 c^3 C^4 i^3 x_3 + 48 c l^3 c^3 i^3 C^2 x l^2 - 108 c l^3 c^3 C^3 a_2^3 x_1 - 40 c l^3 c^3 C x l^3 a_2 \\
& + 24 c l^3 c^3 C x l^3 i^3 + 4 c l^3 c^3 C^2 x_3 x l^2 + 108 c l^3 c^3 C^2 a_2^2 x l^2 - 4 c l^3 c^3 C^3 j_2 x_1 \\
& - 32 c l^3 c^3 C^5 i^3 x_2 + 96 c l^3 C^4 x_2 c_3^6 d_3 x_1 c_2 - 192 c l^3 c^3 C^3 d_3 c_2 x_1 i^3 \\
& - 288 c l^3 c^3 C^5 a_2 d_3 x_2 c_2 + 288 c l^3 c^3 C^3 a_2 d_3 x_1 c_2 + 192 c l^3 c^3 C^5 d_3 c_2 x_2 i^3 \\
& + 144 c l^3 C^4 x_2 c_3^6 i^3 x_1 a_2 - 48 c l^3 c^3 i^3 C^4 x_2 x_1 + 216 c l^3 c^3 C^3 a_2^2 x_1 i^3 \\
& - 48 c l^3 c^3 C^4 a_2 i^3 x_3 + 8 c l^3 c_2 c^3 C^3 j_3 x_1 - 24 c l^3 a_2 c^3 C^3 x_3 x_1 \\
& - 88 c l^3 c^3 C^2 d_3 x l^2 c_2 + 16 c l^3 c^3 C^3 i^3 x_3 x_1 - 144 c l^3 c^3 C^3 a_2 i^3 x_1 \\
& - 144 c l^3 c^3 C^2 i^3 x l^2 a_2 - 108 c l^3 c^3 C^4 x_2 a_2^2 x_1 - 32 c l^3 c^3 C^4 d_3 c_2 x_3 \\
& - 24 c l^3 c^3 C^3 x_2 x l^2 i^3 + 144 c l^3 c^3 C^5 a_2 i^3 x_2 - 216 c l^3 c^3 C^5 a_2^2 x_2 i^3 \\
& + 36 c l^3 c^3 C^3 x_2 x l^2 a_2 + 108 c l^3 a_3^3 c^3 C^5 c_2^3 x_2 - 108 c l^3 a_3^3 c^3 C^3 c_2^3 x_1 \\
& + 972 c l^3 a_3^2 c^3 C^5 a_2 c_2^2 x_2 - 972 c l^3 a_3^2 c^3 C^3 a_2 c_2^2 x_1 + 216 c l^3 a_3^2 c^3 C^3 c_2^2 x_1 i^3 \\
& - 324 c l^3 a_3^2 c^3 C^4 x_2 c_2^2 x_1 - 216 c l^3 a_3^2 c^3 C^5 c_2^2 x_2 i^3 + 324 c l^3 a_3^2 c^3 C^2 c_2^2 x l^2 \\
& + 108 c l^3 a_3^2 c^3 C^4 c_2^2 x_3 + 288 c l^3 a_3 C^4 x_2 c_3^5 i^3 x_1 c_2 - 96 c l^3 a_3 c^3 C^4 i^3 c_2 x_3 \\
& + 648 c l^3 a_3 c^3 C^2 a_2 c_2 x l^2 - 288 c l^3 a_3 c^3 C^5 d_3 c_2^2 x_2 - 144 c l^3 a_3 c^3 C^3 i^3 c_2 x_1 \\
& - 864 c l^3 a_3 c^3 C^5 a_2 c_2 x_2 i^3 - 648 c l^3 a_3 c^3 C^4 x_2 c_2 a_2 x_1 + 288 c l^3 a_3 c^3 C^3 d_3 c_2^2 x_1 \\
& - 72 c l^3 a_3 c_2 c^3 C^3 x_3 x_1 - 288 c l^3 a_3 c^3 C^2 i^3 x l^2 c_2 - 972 c l^3 a_3 c^3 C^3 a_2^2 x_1 c_2 \\
& - 100 c l^3 a_3 c^3 C x l^3 c_2 + 144 c l^3 a_3 c^3 C^5 i^3 c_2 x_2 + 216 c l^3 a_3 c^3 C^4 a_2 c_2 x_3 \\
& + 108 c l^3 a_3 c^3 C^3 x_2 x l^2 c_2 + 972 c l^3 a_3 c^3 C^5 a_2^2 x_2 c_2 + 864 c l^3 a_3 c^3 C^3 a_2 c_2 x_1 i^3 \\
& - 12 c l^2 c^3 C x l^3 c_2 - 48 c l^2 c^3 C^5 d_3 c_2^2 x_2 - 144 c l^2 c^3 C^5 a_2 c_2 x_2 i^3 \\
& - 72 c l^2 c^3 C^4 x_2 c_2 a_2 x_1 + 144 c l^2 c^3 C^3 a_2 c_2 x_1 i^3 - 48 c l^2 c^3 C^2 i^3 x l^2 c_2 \\
& - 108 c l^2 c^3 C^3 a_2^2 x_1 c_2 + 108 c l^2 c^3 C^5 a_2^2 x_2 c_2 + 72 c l^2 c^3 C^2 a_2 c_2 x l^2
\end{aligned}$$

$$\begin{aligned}
& + 24 c l^2 c 3^8 C^4 a 2 c 2 x 3 + 12 c l^2 c 3^9 C^3 x 2 x l^2 c 2 + 48 c l^2 c 3^9 C^3 d 3 c 2^2 x l \\
& + 48 c l^2 c 3^5 C^5 i 3^2 c 2 x 2 - 8 c l^2 c 2 c 3^9 C^3 x 3 x l + 48 c l^2 C^4 x 2 c 3^7 i 3 x l c 2 \\
& - 48 c l^2 c 3^8 C^3 i 3^2 c 2 x l - 16 c l^2 c 3^7 C^4 i 3 c 2 x 3 + 108 c l^2 a 3^2 c 3^5 C^5 c 2^3 x 2 \\
& - 108 c l^2 a 3^2 c 3^8 C^3 c 2^3 x l - 108 c l^2 a 3 c 3^7 C^4 x 2 c 2^2 x l + 324 c l^2 a 3 c 3^6 C^5 a 2 c 2^2 x 2 \\
& - 144 c l^2 a 3 c 3^5 C^5 c 2^2 x 2 i 3 + 108 c l^2 a 3 c 3^{10} C^2 c 2^2 x l^2 + 144 c l^2 a 3 c 3^8 C^3 c 2^2 x l i 3 \\
& - 324 c l^2 a 3 c 3^9 C^3 a 2 c 2^2 x l + 36 c l^2 a 3 c 3^7 C^4 c 2^2 x 3 - 36 c l a 3 c 3^{10} C^3 c 2^3 x l \\
& + 36 c l a 3 c 3^7 C^5 c 2^3 x 2 - 24 c l c 3^7 C^5 c 2^2 x 2 i 3 - 36 c l c 3^{11} C^3 a 2 c 2^2 x l \\
& + 4 c l c 3^9 C^4 c 2^2 x 3 + 36 c l c 3^8 C^5 a 2 c 2^2 x 2 + 12 c l c 3^{12} C^2 c 2^2 x l^2 - 12 c l c 3^9 C^4 x 2 c 2^2 x l \\
& + 24 c l c 3^{10} C^3 c 2^2 x l i 3) / (4 c 3^2 c l^3 C^4 (3 a 3 c l + c 3^2)^2)]
\end{aligned}$$

```

> simplify(jacobian(subs(x1=x1-C*
> (-9*c1^2*a2*a3+4*c1^2*d3-3*c1*c2*c3*a3+
> 2*c3*i3*c1-3*c1*a2*c3^2-c2*c3^3)/
> (c3*c1*(3*a3*c1+c3^2)),evalm(G)),[x2,x3]));

```

$$\begin{bmatrix} 0 & 0 \\ \frac{(3 a 3 c l + c 3^2) x l^2 c 3}{C^2} & -\frac{(3 a 3 c l + c 3^2) x l c 3}{C^2} \\ \frac{(3 a 3 c l + c 3^2) x l^3 c 3}{C^2} & -\frac{(3 a 3 c l + c 3^2) x l^2 c 3}{C^2} \end{bmatrix}$$

```

> contradict(1,'c3');

```

Contradiction on case level 5, so:

$$c 3 = 0$$

Variables to be uneliminated:

"s3 := 's3'"

"j1 := 'j1'"

"i1 := 'i1'"

"p3 := 'p3'"

"g3 := 'g3'"

Proceed on case level 4 with:

$$6 a 3 g 3 c l (3 a 3 c l + c 3^2) \neq 0$$

On account of:

$$c 3 = 0$$

$$\{1 \neq 0\}$$

c3 is set to:

$$0$$

Nonzero constraint refines to:

$$18 a 3^2 g 3 c l^2 \neq 0$$

```

> tmp1 := cpcoeff (x1^4*x2);

```

$$tmp1 := \frac{9 c l^2 a 3^2 (g 3^2 + 27 a 3^3 c l)}{g 3^2}$$

```

> elimsolve (tmp1,c1);

```

```

c1 is set to:

$$\{27 a3^3 \neq 0\}$$


$$-\frac{g3^2}{27 a3^3}$$

Nonzero constraint refines to:

$$6 a3 g3^3 \neq 0$$

> tmp1 := cpcoeff (x1^3*x3^3);

$$tmp1 := \frac{32 g3^6}{59049 a3^9}$$

> contradict (tmp1,'c1');
Contradiction on case level 4, so:

$$3 a3 c1 + c3^2 = 0$$

Variables to be uneliminated:
" c1 := 'c1'"
" c3 := 'c3'"
" u2 := 'u2'"
Proceed on case level 3 with:

$$6 a3 g3 c1 \neq 0$$

On account of:

$$3 a3 c1 + c3^2 = 0$$


$$\{3 a3 \neq 0\}$$

c1 is set to:

$$-\frac{c3^2}{3 a3}$$

Nonzero constraint refines to:

$$-6 a3 g3 c3 \neq 0$$

> tmp1 := cpcoeff (x1^5*x3);

$$tmp1 := \frac{c3 g3^3}{81 a3^4}$$

> contradict (tmp1,'c1');
Contradiction on case level 3, so:

$$c1 = 0$$

Variables to be uneliminated:
" c1 := 'c1'"
" o3 := 'o3'"
" d1 := 'd1'"
" a1 := 'a1'"
Proceed on case level 2 with:

$$6 a3 g3 \neq 0$$

On account of:

$$c1 = 0$$


$$\{1 \neq 0\}$$

c1 is set to:

```

```

[
  > tmp1 := cpcoeff (x1^6);
  0
  tmp1 := -c3^3
  > elimsolve (tmp1,c3);
  {1 ≠ 0}
  c3 is set to:
  0
  > tmp1 := cpcoeff (x2^3);
  tmp1 := -(-o3 + 9 a l^2)^3
  > elimsolve (tmp1,o3);
  {-1 ≠ 0}
  o3 is set to:
  9 a l^2
  > tmp1 := cpcoeff (x3^4*T);
  tmp1 := - (6561 a3^2 a l^6 + 2916 g3 a3 a l^5 - 2 u2 g3^4)^2 / (36 g3^6 a3^2)
  > elimsolve (tmp1,u2);
  {-2 g3^4 ≠ 0}
  u2 is set to:
  729 a3 a l^5 (9 a3 a l + 4 g3) / (2 g3^4)
  > launchNZcase (a1);
  Launching case level 3:
  a l ≠ 0
  Assume from now on that:
  6 a3 a l g3 ≠ 0
  > tmp1 := cpcoeff (x1^4*x2);
  tmp1 := 729 a3 a l^5 (g3 + 9 a3 a l) / g3^2
  > elimsolve (tmp1,g3);
  {1 ≠ 0}
  g3 is set to:
  -9 a3 a l
  Nonzero constraint refines to:
  -18 a3^2 a l^2 ≠ 0
  > tmp1 := cpcoeff (x1^4*x3);
  tmp1 := 3 a l^3 (-6 d l a3 - 6 i3 a3 + 27 a3 a2 a l + 9 c2 a3^2 - p3 - 6 d3 a l) / a3^2
  > elimsolve (tmp1,p3);
  {-1 ≠ 0}
  p3 is set to:
  -6 d l a3 - 6 i3 a3 + 27 a3 a2 a l + 9 c2 a3^2 - 6 d3 a l
]

```

> **launchNZcase** (a3\*i1-a1\*i3);

Launching case level 4:

$$a^3 i1 - a1 i3 \neq 0$$

Assume from now on that:

$$-18 a^3 a1^2 (a^3 i1 - a1 i3) \neq 0$$

> **tmp1 := cpcoeff** (x3^4);

$$tmp1 := \frac{6 a1^3 (-a^3 i1 + a1 i3) (2 d3 a1^2 + i3 a3 a1 - 2 a3 a1 d1 - a^3 i1)}{a^3^5}$$

> **elimsolve** (tmp1,i1);

$$\{-a^3^2 \neq 0\}$$

i1 is set to:

$$\frac{a1 (2 d3 a1 + i3 a3 - 2 d1 a3)}{a^3^2}$$

Nonzero constraint refines to:

$$-18 a^3 a1^3 (2 d3 a1 - 2 d1 a3) \neq 0$$

> **tmp1 := cpcoeff** (x1^3);

$$tmp1 := \frac{8 (d3 a1 - d1 a3)^3}{a^3^3}$$

> **contradict** (tmp1,'i1');

Contradiction on case level 4, so:

$$a^3 i1 - a1 i3 = 0$$

Variables to be uneliminated:

$$i1 := i1$$

Proceed on case level 3 with:

$$-18 a^3 a1^2 \neq 0$$

On account of:

$$a^3 i1 - a1 i3 = 0$$

$$\{-a^3 \neq 0\}$$

i1 is set to:

$$\frac{a1 i3}{a^3}$$

> **tmp1 := cpcoeff** (x1^2\*x2);

$$tmp1 := -\frac{36 a1^2 (d3 a1 - d1 a3)^2}{a^3^2}$$

> **elimsolve** (tmp1,d1);

$$\{-a^3 \neq 0\}$$

d1 is set to:

$$\frac{d3 a1}{a^3}$$

> **launchNZcase** (j3\*a1-j1\*a3);

Launching case level 4:

$$j3 a1 - a3 j1 \neq 0$$

Assume from now on that:

$$-18 a^3 d^2 a l^2 (j^3 a l - a^3 j l) \neq 0$$

```
> launchNZcase (3*s3*a3^2*a1+3*j3*a3*a1^2-18*a3^2*c2*a1*d3 +
> 2*a3^2*i3^2+81*a2^2*a3^2*a1^2+8*a1^2*d3^2+9*a3^4*c2^2 -
> 54*a1^2*d3*a2*a3-9*a3^3*c2*i3+54*a3^3*c2*a2*a1-27*a2*a3^2*a1*i3
+
> 8*a1*d3*a3*i3);
```

Launching case level 5:

$$3 a^3 d^2 a l s^3 + 3 j^3 a l^2 a^3 - 18 c^2 a^3 d^3 a l + 2 a^3 d^2 i^3^2 + 81 a^3 d^2 a l^2 a^2 + 8 d^3^2 a l^2 + 9 c^2^2 a^3^4 - 54 a^3 a^2 a l^2 d^3 - 9 a^3^3 i^3 c^2 + 54 a^2 c^2 a^3^3 a l - 27 a^3^2 i^3 a^2 a l + 8 i^3 a^3 d^3 a l \neq 0$$

Assume from now on that:

$$-18 a^3 d^2 a l^2 (j^3 a l - a^3 j l) (3 a^3 d^2 a l s^3 + 3 j^3 a l^2 a^3 - 18 c^2 a^3 d^3 a l + 2 a^3 d^2 i^3^2 + 81 a^3 d^2 a l^2 a^2 + 8 d^3^2 a l^2 + 9 c^2^2 a^3^4 - 54 a^3 a^2 a l^2 d^3 - 9 a^3^3 i^3 c^2 + 54 a^2 c^2 a^3^3 a l - 27 a^3^2 i^3 a^2 a l + 8 i^3 a^3 d^3 a l) \neq 0$$

```
> tmp1 := cpcoeff (1);
```

$$tmp1 := -(3 a^3 d^2 a l s^3 + 3 j^3 a l^2 a^3 - 18 c^2 a^3 d^3 a l + 2 a^3 d^2 i^3^2 + 81 a^3 d^2 a l^2 a^2 + 8 d^3^2 a l^2 + 9 c^2^2 a^3^4 - 54 a^3 a^2 a l^2 d^3 - 9 a^3^3 i^3 c^2 + 54 a^2 c^2 a^3^3 a l - 27 a^3^2 i^3 a^2 a l + 8 i^3 a^3 d^3 a l) (j^3 a l - a^3 j l) (81 a^3 d^2 a l^2 a^2 - 54 a^3 a^2 a l^2 d^3 + 8 d^3^2 a l^2 + 54 a^2 c^2 a^3^3 a l - 27 a^3^2 i^3 a^2 a l + 3 a^3 d^2 a l s^3 - 18 c^2 a^3 d^3 a l + 3 a^3 d^2 a l j l + 8 i^3 a^3 d^3 a l + 9 c^2^2 a^3^4 - 9 a^3^3 i^3 c^2 + 2 a^3 d^2 i^3^2) / (9 a l^2 a^3^5)$$

```
> elimsolve (tmp1,s3);
```

$$\{3 a l a^3^2 \neq 0\}$$

s3 is set to:

$$-(81 a^3 d^2 a l^2 a^2 - 54 a^3 a^2 a l^2 d^3 + 8 d^3^2 a l^2 + 54 a^2 c^2 a^3^3 a l - 27 a^3^2 i^3 a^2 a l - 18 c^2 a^3 d^3 a l + 3 a^3 d^2 a l j l + 8 i^3 a^3 d^3 a l + 9 c^2^2 a^3^4 - 9 a^3^3 i^3 c^2 + 2 a^3 d^2 i^3^2) / (3 a l a^3^2)$$

Nonzero constraint refines to:

$$-18 a^3 d^2 a l^3 (j^3 a l - a^3 j l) (3 j^3 a l - 3 a^3 j l) \neq 0$$

```
> tmp1 := cpcoeff (T);
```

$$tmp1 := -\frac{(j^3 a l - a^3 j l)^2}{a^3^2}$$

```
> contradict (tmp1,'s3');
```

Contradiction on case level 5, so:

$$3 a^3 d^2 a l s^3 + 3 j^3 a l^2 a^3 - 18 c^2 a^3 d^3 a l + 2 a^3 d^2 i^3^2 + 81 a^3 d^2 a l^2 a^2 + 8 d^3^2 a l^2 + 9 c^2^2 a^3^4 - 54 a^3 a^2 a l^2 d^3 - 9 a^3^3 i^3 c^2 + 54 a^2 c^2 a^3^3 a l - 27 a^3^2 i^3 a^2 a l + 8 i^3 a^3 d^3 a l = 0$$

Variables to be uneliminated:

$$"s3 := 's3'"$$

Proceed on case level 4 with:

$$-18 a^3 d^2 a l^2 (j^3 a l - a^3 j l) \neq 0$$

On account of:

$$3 a^3 d^2 a l s^3 + 3 j^3 a l^2 a^3 - 18 c^2 a^3 d^3 a l + 2 a^3 d^2 i^3^2 + 81 a^3 d^2 a l^2 a^2 + 8 d^3^2 a l^2 + 9 c^2^2 a^3^4 - 54 a^3 a^2 a l^2 d^3 - 9 a^3^3 i^3 c^2 + 54 a^2 c^2 a^3^3 a l - 27 a^3^2 i^3 a^2 a l + 8 i^3 a^3 d^3 a l = 0$$

$$\{3 a1 a3^2 \neq 0\}$$

s3 is set to:

$$-(3 j3 a1^2 a3 - 18 c2 a3^2 d3 a1 + 2 a3^2 i3^2 + 81 a3^2 a1^2 a2^2 + 8 d3^2 a1^2 + 9 c2^2 a3^4 - 54 a3 a2 a1^2 d3 - 9 a3^3 i3 c2 + 54 a2 c2 a3^3 a1 - 27 a3^2 i3 a2 a1 + 8 i3 a3 d3 a1) / (3 a1 a3^2)$$

> **tmp1 := cpcoeff (T) ;**

$$tmp1 := - \frac{(j3 a1 - a3 j1)^2}{a3^2}$$

> **contradict (tmp1, 'j1') ;**

Contradiction on case level 4, so:

$$j3 a1 - a3 j1 = 0$$

Variables to be uneliminated:

$$s3 := 's3'$$

Proceed on case level 3 with:

$$-18 a3^2 a1^2 \neq 0$$

On account of:

$$j3 a1 - a3 j1 = 0$$

$$\{-a3 \neq 0\}$$

j1 is set to:

$$\frac{j3 a1}{a3}$$

> **tmp1 := cpcoeff (T) ;**

$$tmp1 := -(3 a3^2 a1 s3 + 3 j3 a1^2 a3 - 18 c2 a3^2 d3 a1 + 2 a3^2 i3^2 + 81 a3^2 a1^2 a2^2 + 8 d3^2 a1^2 + 9 c2^2 a3^4 - 54 a3 a2 a1^2 d3 - 9 a3^3 i3 c2 + 54 a2 c2 a3^3 a1 - 27 a3^2 i3 a2 a1 + 8 i3 a3 d3 a1)^2 / (9 a1^2 a3^4)$$

> **elimsolve (tmp1, s3) ;**

$$\{3 a3^2 a1 \neq 0\}$$

s3 is set to:

$$-(3 j3 a1^2 a3 - 18 c2 a3^2 d3 a1 + 2 a3^2 i3^2 + 81 a3^2 a1^2 a2^2 + 8 d3^2 a1^2 + 9 c2^2 a3^4 - 54 a3 a2 a1^2 d3 - 9 a3^3 i3 c2 + 54 a2 c2 a3^3 a1 - 27 a3^2 i3 a2 a1 + 8 i3 a3 d3 a1) / (3 a3^2 a1)$$

> **det (T-jacobian (H, [x1, x2, x3])) ;**

$$T^3$$

> **simplify (evalm ([H[1], H[2], H[3]])) ;**

$$[(6 a1^4 x3^3 + 27 a1^3 x2 x3 a3^2 + 3 j3 a1 x1 a3^2 - 9 a1^3 x1 x3^2 a3 - 27 a1^2 x1 x2 a3^3 + 3 d3 a1 x1^2 a3^2 - 54 x3 a2 c2 a3^3 a1 + 9 x3 a3^3 i3 c2 - 81 x3 a3^2 a1^2 a2^2 - 3 x3 j3 a1^2 a3 - 8 x3 i3 a3 d3 a1 + 27 x3 a3^2 i3 a2 a1 - 3 a1^2 x3^2 i3 a3 + 54 x3 a3 a2 a1^2 d3 + 27 a1 x2 a3^4 c2 + 81 a1^2 x2 a3^3 a2 + 3 a1 i3 x1 x3 a3^2 + 18 x3 c2 a3^2 d3 a1 - 18 a1 x2 a3^3 i3 - 36 a1^2 x2 a3^2 d3 + 3 a1 x1^3 a3^3 - 2 x3 a3^2 i3^2 - 3 a1^3 x3^2 d3 - 9 x3 c2^2 a3^4 - 8 x3 d3^2 a1^2) / (3 a3^3), (108 a2 x1^3 a3^4 a1^2 + 108 a3^2 a1^4 x3^3 c2$$

$$\begin{aligned}
& + 27 x l^4 a^3 a l^2 + 288 a l^2 x l x^3 a^3 c^2 d^3 - 216 a^3 a l^3 x l d^2 x^3 + 108 a l^2 x l^2 x^3 a^3 c^2 \\
& - 324 a l^4 x l x^3 a^3 a^2 - 216 a l^3 x l x^3 a^3 c^2 + 288 i^3 a^3 d^3 a l^2 x^2 \\
& + 1944 a^2 c^2 a^3 a l^2 x^2 - 972 a^3 i^3 a^2 a l^2 x^2 - 1944 a^3 a^2 a l^3 d^3 x^2 - 324 a^3 i^3 c^2 a l x^2 \\
& + 2916 a^3 a l^3 a^2 x^2 + 324 c^2 a^3 a l x^2 - 324 a l^5 x^3 x^2 a^3 + 36 a l^2 x^3 a^3 i^3 \\
& + 972 a l^4 x^3 a^3 a^2 + 108 a l^2 x^3 c^2 a^3 + 8 x^3 i^3 a^3 + 288 d^3 a l^3 x^2 a^3 \\
& + 648 a l^4 x l x^3 a^3 x^2 - 81 a l^6 x^3 + 64 a l^3 x^3 d^3 + 144 a l^4 x^3 d^3 + 216 a l^5 x l x^3 a^3 \\
& + 108 a^3 a l^2 x l^2 d^2 - 2916 a l^3 x^3 a^3 a^2 - 108 x^3 c^2 a^3 + 108 a l^4 x^3 a^3 d^2 \\
& + 108 j^2 a^3 a l^2 x l - 108 j^2 a^3 a l^3 x^3 - 324 a l^3 x l^2 a^3 x^2 - 162 a l^4 x l^2 a^3 x^2 \\
& + 216 a l^5 x^3 a^3 a^2 + 864 a l x^3 i^3 a^3 a^2 c^2 - 180 a l x^3 i^3 a^3 a^2 - 648 c^2 a^3 d^3 a l^2 x^2 \\
& - 972 a l x^3 c^2 a^3 a^2 - 288 a l^3 x^3 c^2 a^3 d^3 - 864 a l^4 x^3 a^3 a^2 d^3 - 144 a l^2 x^3 a^3 i^3 c^2 \\
& + 648 a l^3 x^3 a^2 c^2 a^3 - 432 a l^3 x^3 a^3 i^3 a^2 + 144 a l^3 x^3 i^3 a^3 d^3 \\
& - 240 a l x^3 d^3 a^3 i^3 c^2 - 216 a^3 a l^3 x l d^3 x^2 - 108 a^3 a l^2 x l i^3 x^2 + 216 a l^4 x^3 d^3 x^2 a^3 \\
& - 240 a l^2 x^3 d^3 c^2 a^3 + 48 a l x^3 d^3 a^3 i^3 + 2592 a l^3 x^3 d^3 a^3 a^2 + 288 a l x^3 d^3 c^2 a^3 \\
& - 720 a l^3 x^3 d^3 a^3 a^2 + 1728 a l^2 x^3 d^3 a^2 c^2 a^3 - 720 a l^2 x^3 d^3 a^3 i^3 a^2 \\
& + 96 a l^2 x^3 d^3 i^3 a^3 + 108 a l^3 x^3 i^3 a^3 x^2 + 1296 a l^2 x^3 i^3 a^3 a^2 + 144 x^3 i^3 a^3 c^2 \\
& - 2916 a l^2 x^3 a^3 a^2 c^2 - 60 x^3 i^3 a^3 c^2 - 36 a l x l x^3 a^3 i^3 - 972 a l^3 x l x^3 a^3 a^2 \\
& - 144 a l^3 x l x^3 a^3 d^3 - 108 a l x l x^3 a^3 c^2 + 864 a l^3 x l x^3 a^3 a^2 d^3 \\
& + 144 a l x l x^3 a^3 i^3 c^2 - 648 a l^2 x l x^3 a^3 a^2 c^2 + 432 a l^2 x l x^3 a^3 i^3 a^2 \\
& - 144 a l^2 x l x^3 a^3 i^3 d^3 + 72 a^3 i^3 a l x^2) / (108 a^3 a l^2), (6 a l^4 x^3 + 27 a l^3 x^2 x^3 a^3 \\
& + 3 j^3 a l x l a^3 - 9 a l^3 x l x^3 a^3 - 27 a l^2 x l x^2 a^3 + 3 d^3 a l x l^2 a^3 - 54 x^3 a^2 c^2 a^3 a l \\
& + 9 x^3 a^3 i^3 c^2 - 81 x^3 a^3 a l^2 a^2 - 3 x^3 j^3 a l^2 a^3 - 8 x^3 i^3 a^3 d^3 a l + 27 x^3 a^3 i^3 a^2 a l \\
& - 3 a l^2 x^3 i^3 a^3 + 54 x^3 a^3 a^2 a l^2 d^3 + 27 a l x^2 a^3 c^2 + 81 a l^2 x^2 a^3 a^2 \\
& + 3 a l i^3 x l x^3 a^3 + 18 x^3 c^2 a^3 d^3 a l - 18 a l x^2 a^3 i^3 - 36 a l^2 x^2 a^3 d^3 + 3 a l x l^3 a^3 \\
& - 2 x^3 a^3 i^3 - 3 a l^3 x^3 d^3 - 9 x^3 c^2 a^3 - 8 x^3 d^3 a l^2) / (3 a^3 a l)]
\end{aligned}$$

> **factor(a3\*H[1]-a1\*H[3]) ;**

0

> **M := evalm([C,0,-C/a3\*a1], [0,0,1], [0,3\*C\*a3,**  
> **-C\*(6\*a3\*a2\*a1+2\*c2\*a3^2-i3\*a3-2\*d3\*a1)/a3/a1]) ;**

$$M := \begin{bmatrix} C & 0 & -\frac{C a l}{a^3} \\ 0 & 0 & 1 \\ 0 & 3 C a^3 & -\frac{C (6 a^3 a^2 a l + 2 c^2 a^3 - i^3 a^3 - 2 d^3 a l)}{a^3 a l} \end{bmatrix}$$

> **G := simplify(evalm(M&\*subs({seq([x1,x2,x3][i]=**  
> **evalm(M^(-1)&\*[x1,x2,x3])[i],i=1..n)},H))) ;**

$$\begin{aligned}
G := & [0, (9 x l^2 a^3 a l^2 x^2 C + 3 C d^3 a l x l^2 a^3 + 24 C^2 d^3 a l^2 x l a^3 x^2 \\
& - 54 a l^2 C^2 x l a^3 x^2 a^2 - 18 a l C^2 x l a^3 x^2 c^2 + 12 a l C^2 x l a^3 x^2 i^3 - 9 a l^2 C x l a^3 x^3
\end{aligned}$$

$$\begin{aligned}
& + 3 j_3 a l C^2 a^3 x l - 12 C^2 d_3 a l^2 x_3 a_3 - 72 C^3 d_3 a l^2 x_2 a_3 a_2 - 24 C^3 d_3 a l x_2 c_2 a^3 \\
& + 16 C^3 d_3 a l x_2 i_3 a_3 - 36 C^3 i_3 a^3 x_2 a_2 a l - 12 C^3 i_3 a^3 x_2 c_2 - 6 C^2 i_3 a^3 x_3 a l \\
& + 81 C^3 a^3 a^2 a l^2 x_2 + 54 C^3 a^3 a_2 a l x_2 c_2 + 27 C^2 a^3 a_2 a l^2 x_3 + 9 C^2 c_2 a^3 x_3 a l \\
& + 16 C^3 d_3^2 a l^2 x_2 + 4 C^3 i_3^2 a^3 x_2 + 9 C^3 c_2^2 a^4 x_2 + 3 a l x l^3 a^3 \big) / (3 a^3 C^3 a l), ( \\
& 27 x l^4 a^4 a l^2 + 216 C^4 c_2^2 a^5 x_2 i_3 + 32 C^4 a^3 i_3^3 x_2 - 108 C^4 c_2^3 a^6 x_2 \\
& + 108 d_2 C^2 a^4 a l^2 x l^2 - 2592 C^3 a l^3 d_3 x l a^3 x_2 a_2 + 108 a l^3 x l^3 a^3 x_2 C \\
& - 108 a_2 C a^4 a l^2 x l^3 - 972 a_2 C^2 a^3 a l^3 x l^2 x_2 - 324 a l^2 C^2 x l^2 a^4 x_2 c_2 \\
& + 216 a l^2 C^2 x l^2 a^3 x_2 i_3 + 432 a l^3 C^2 x l^2 a^3 x_2 d_3 - 108 a l^3 C x l^2 a^3 x_3 \\
& + 36 i_3 a^3 C^2 d_3 a l x l^2 + 36 i_3 a^3 j_3 a l C^3 x l + 72 d_3^2 a l^2 C^2 x l^2 a^3 \\
& + 72 d_3 a l^2 j_3 C^3 a^3 x l - 216 a^3 a_2 a l^2 C^2 d_3 x l^2 + 648 a^3 a_2 a l^3 C^2 x l x_3 \\
& - 216 a^3 a_2 a l^2 j_3 C^3 x l - 72 c_2 a^4 C^2 d_3 a l x l^2 + 216 c_2 a^4 a l^2 C^2 x l x_3 \\
& - 72 c_2 a^4 j_3 a l C^3 x l + 72 C d_3 a l^2 x l^3 a^3 + 36 C a l x l^3 a^4 i_3 - 72 C c_2 x l^3 a^5 a l \\
& - 1728 C^4 a^3 a_2 a l^2 d_3 x_2 i_3 + 1296 C^4 a^4 i_3 c_2 x_2 a_2 a l + 144 C^3 a^4 i_3 c_2 x_3 a l \\
& - 648 C^3 a_2 c_2 a^4 a l^2 x_3 + 432 C^3 a^3 i_3 a_2 a l^2 x_3 - 192 C^3 i_3 a^3 d_3 a l^2 x_3 \\
& + 2592 C^4 c_2 a^3 d_3 a l^2 x_2 a_2 + 288 C^3 c_2 a^3 d_3 a l^2 x_3 - 576 C^4 c_2 a^3 d_3 a l x_2 i_3 \\
& - 576 C^4 c_2 a^3 d_3^2 a l^2 x_2 - 432 C^4 a^3 i_3^2 x_2 a_2 a l - 144 C^4 a^4 i_3^2 x_2 c_2 \\
& + 192 C^4 a^3 i_3^2 x_2 d_3 a l - 2916 C^4 a^3 a l^3 a^2 x_2 - 2916 C^4 a^4 a l^2 a^2 x_2 c_2 \\
& + 1944 C^4 a^3 a l^2 a^2 x_2 i_3 + 3888 C^4 a^3 a l^3 a^2 x_2 d_3 - 1728 C^4 d_3^2 a l^3 x_2 a_3 a_2 \\
& + 384 C^4 d_3^2 a l^2 x_2 i_3 a_3 - 972 C^4 c_2^2 a^5 x_2 a_2 a l + 864 C^3 a^3 a_2 a l^3 d_3 x_3 \\
& + 432 C^4 c_2^2 a^4 d_3 a l x_2 - 48 C^3 a^3 i_3^2 x_3 a l + 256 C^4 d_3^3 a l^3 x_2 \\
& + 324 a l x_2 C^3 c_2^2 a^5 x l + 2916 a l^3 x_2 C^3 a^3 a^2 x l + 1944 a l^2 x_2 C^3 a_2 c_2 a^4 x l \\
& + 108 j_2 C^3 a^4 a l^2 x l - 972 C^3 a^3 a l^3 a^2 x_3 - 192 C^3 d_3^2 a l^3 x_3 a_3 - 108 C^3 c_2^2 a^5 x_3 a l \\
& - 864 C^3 a l^2 d_3 x l a^3 x_2 c_2 + 576 C^3 a l^2 d_3 x l a^3 x_2 i_3 + 576 C^3 a l^3 d_3^2 x l a_3 x_2 \\
& - 288 C^2 a l^3 d_3 x l a^3 x_3 - 1296 C^3 a l^2 i_3 a^3 x l x_2 a_2 - 432 C^3 a l i_3 a^4 x l x_2 c_2 \\
& + 144 C^3 a l i_3^2 a^3 x l x_2 - 144 C^2 a l^2 i_3 a^3 x l x_3 \big) / (36 C^3 a^3 a l^2) ]
\end{aligned}$$

```

> simplify(jacobian(subs(x1=x1+
> 1/3*C*(3*c2*a3^2+9*a3*a2*a1-2*i3*a3-4*d3*a1)/
> (a1*a3),evalm(G)), [x2,x3]));

```

$$\begin{bmatrix} 0 & 0 \\ \frac{3 a l x l^2}{C^2} & -\frac{3 a l x l}{C^2} \\ \frac{3 a l x l^3}{C^2} & -\frac{3 a l x l^2}{C^2} \end{bmatrix}$$

```

> contradict(1,'a1');

```

Contradiction on case level 3, so:

$$a l = 0$$

Variables to be uneliminated:

|                                |                                                                    |
|--------------------------------|--------------------------------------------------------------------|
|                                | "s3 := 's3'"                                                       |
|                                | "j1 := 'j1'"                                                       |
|                                | "d1 := 'd1'"                                                       |
|                                | "i1 := 'i1'"                                                       |
|                                | "p3 := 'p3'"                                                       |
|                                | "g3 := 'g3'"                                                       |
| Proceed on case level 2 with:  |                                                                    |
|                                | $6 a3 g3 \neq 0$                                                   |
| On account of:                 |                                                                    |
|                                | $a1 = 0$                                                           |
|                                | $\{1 \neq 0\}$                                                     |
| a1 is set to:                  |                                                                    |
|                                | 0                                                                  |
| > tmp1 := cpcoeff (x3^2*T);    |                                                                    |
|                                | $tmp1 := -i1^2$                                                    |
| > elimsolve (tmp1,i1);         |                                                                    |
|                                | $\{1 \neq 0\}$                                                     |
| i1 is set to:                  |                                                                    |
|                                | 0                                                                  |
| > tmp1 := cpcoeff (x1^2*x2);   |                                                                    |
|                                | $tmp1 := g3^2 c2^2$                                                |
| > elimsolve (tmp1,c2);         |                                                                    |
|                                | $\{1 \neq 0\}$                                                     |
| c2 is set to:                  |                                                                    |
|                                | 0                                                                  |
| > tmp1 := cpcoeff (x1^3);      |                                                                    |
|                                | $tmp1 := -8 d1^3$                                                  |
| > elimsolve (tmp1,d1);         |                                                                    |
|                                | $\{1 \neq 0\}$                                                     |
| d1 is set to:                  |                                                                    |
|                                | 0                                                                  |
| > launchNZcase (j1);           |                                                                    |
| Launching case level 3:        |                                                                    |
|                                | $j1 \neq 0$                                                        |
| Assume from now on that:       |                                                                    |
|                                | $6 a3 g3 j1 \neq 0$                                                |
| > launchNZcase (-p3*i3+s3*g3); |                                                                    |
| Launching case level 4:        |                                                                    |
|                                | $-p3 i3 + s3 g3 \neq 0$                                            |
| Assume from now on that:       |                                                                    |
|                                | $6 a3 g3 j1 (-p3 i3 + s3 g3) \neq 0$                               |
| > tmp1 := cpcoeff (1);         |                                                                    |
|                                | $tmp1 := \frac{j1 (-p3 i3 + s3 g3) (j1 g3 + s3 g3 - p3 i3)}{g3^2}$ |

> **elimsolve** (tmp1,s3);

s3 is set to:  $\{g^3 \neq 0\}$

$$-\frac{j1\ g^3 - p3\ i3}{g^3}$$

Nonzero constraint refines to:

$$-6\ a3\ g^3^2\ j1^2 \neq 0$$

> **tmp1 := cpcoeff** (T);

$$tmp1 := -j1^2$$

> **contradict** (tmp1,'s3');

Contradiction on case level 4, so:

$$-p3\ i3 + s3\ g3 = 0$$

Variables to be uneliminated:

$$"s3 := 's3'"$$

Proceed on case level 3 with:

$$6\ a3\ g3\ j1 \neq 0$$

On account of:

$$-p3\ i3 + s3\ g3 = 0$$

$$\{g^3 \neq 0\}$$

s3 is set to:

$$\frac{p3\ i3}{g^3}$$

> **tmp1 := cpcoeff** (T);

$$tmp1 := -j1^2$$

> **contradict** (tmp1,'j1');

Contradiction on case level 3, so:

$$j1 = 0$$

Variables to be uneliminated:

$$"s3 := 's3'"$$

Proceed on case level 2 with:

$$6\ a3\ g3 \neq 0$$

On account of:

$$j1 = 0$$

$$\{1 \neq 0\}$$

j1 is set to:

$$0$$

> **tmp1 := cpcoeff** (T);

$$tmp1 := -\frac{(-p3\ i3 + s3\ g3)^2}{g3^2}$$

> **elimsolve** (tmp1,s3);

$$\{g^3 \neq 0\}$$

s3 is set to:

$$\frac{p3\ i3}{g^3}$$

```

> det(T-jacobian(H,[x1,x2,x3]));
T^3
> H;
[ 0,  $\frac{x1^4}{4} + a2 x1^3 + d2 x1^2 - i3 x1 x2 - \frac{i3^2 x1 x3}{g3} + j2 x1 - \frac{p3 i3 x2}{g3} - \frac{p3 i3^2 x3}{g3^2},$ 
 $a3 x1^3 + d3 x1^2 + g3 x1 x2 + i3 x1 x3 + j3 x1 + p3 x2 + \frac{p3 i3 x3}{g3}$  ]
> M := evalm([ [1,0,0], [0,1,-i3/g3], [0,0,1] ]);
M :=  $\begin{bmatrix} 1 & 0 & 0 \\ 0 & 1 & -\frac{i3}{g3} \\ 0 & 0 & 1 \end{bmatrix}$ 
> evalm(simplify(jacobian(evalm(M^(-1) &*
> subs({seq([x1,x2,x3][i]=evalm(M&*[x1,x2,x3])[i],i=1..3)},H)),
> [x1,x2,x3])));
 $\begin{bmatrix} 0 & 0 & 0 \\ \frac{x1^3 g3 + 3 a2 x1^2 g3 + 2 d2 x1 g3 + j2 g3 + 3 i3 a3 x1^2 + 2 i3 d3 x1 + i3 j3}{g3} & 0 & 0 \\ 3 a3 x1^2 + 2 d3 x1 + g3 x2 + j3 & g3 x1 + p3 & 0 \end{bmatrix}$ 
> contradict (1,'g3');
Contradiction on case level 2, so:
g3 = 0
Variables to be uneliminated:
"s3 := 's3'"
"j1 := 'j1'"
"d1 := 'd1'"
"c2 := 'c2'"
"i1 := 'i1'"
"a1 := 'a1'"
"u2 := 'u2'"
"o3 := 'o3'"
"c3 := 'c3'"
"c1 := 'c1'"
"h3 := 'h3'"
"w2 := 'w2'"
"v2 := 'v2'"
"r3 := 'r3'"
"q3 := 'q3'"
"s2 := 's2'"
"r2 := 'r2'"

```

```

"q2 := 'q2'"
"i2 := 'i2'"
"h2 := 'h2'"

Proceed on case level 1 with:

6 a3 ≠ 0

On account of:

g3 = 0
{1 ≠ 0}

g3 is set to:

0

> launchNZcase (c1);
Launching case level 2:

c1 ≠ 0

Assume from now on that:

6 a3 c1 ≠ 0

> tmp1 := cpcoeff (x1^6);
                                     tmp1 := -9 a3 c1 a1 - 6 a3 c1 c3 - c3^3
> elimsolve (tmp1,a1);
                                     {9 a3 c1 ≠ 0}

a1 is set to:

                                     - c3 (6 a3 c1 + c3^2)
                                     -----
                                     9 a3 c1

> tmp1 := cpcoeff (x1^5);
tmp1 := -(3 c1^3 p3 a3 + 18 a3^2 c1^3 d1 + 18 a3^2 c1^3 i3 - c2 c3^6 - 27 a3^3 c2 c1^3
+ 9 c3^2 i3 c1^2 a3 - 3 a3 i1 c3^3 c1 - 27 a3^2 c2 c3^2 c1^2 - 9 a3 c2 c1 c3^4 - 2 d3 c1^2 c3^3) / (3 a3
c1^2)
> elimsolve (tmp1,d1);
                                     {18 a3^2 c1^3 ≠ 0}

d1 is set to:
(-3 c1^3 p3 a3 - 18 a3^2 c1^3 i3 + c2 c3^6 + 27 a3^3 c2 c1^3 - 9 c3^2 i3 c1^2 a3 + 3 a3 i1 c3^3 c1
+ 27 a3^2 c2 c3^2 c1^2 + 9 a3 c2 c1 c3^4 + 2 d3 c1^2 c3^3) / (18 a3^2 c1^3)
> launchNZcase (3*a3*c1+c3^2);
Launching case level 3:

3 a3 c1 + c3^2 ≠ 0

Assume from now on that:

6 a3 c1 (3 a3 c1 + c3^2) ≠ 0

> tmp1 := cpcoeff (x1^4*x2);
tmp1 := -(3 a3 c1 + c3^2)^2 (27 a3^3 c1^3 + 54 a3^3 h3 c1^2 + 18 o3 c1^2 a3^2 + 9 c3^2 c1^2 a3^2
+ 18 c1 h3 a3^2 c3^2 - 3 o3 c1 a3 c3^2 + 3 a3 c1 c3^4 + c3^6) / (27 a3^3 c1^3)
> elimsolve (tmp1,h3);
                                     {54 c1^2 a3^3 + 18 a3^2 c3^2 c1 ≠ 0}

h3 is set to:

```

$$-\frac{27 a^3 c l^3 + 18 o3 c l^2 a^3 + 9 c^3 c l^2 a^3 - 3 o3 c l a^3 c^3 + 3 a^3 c l c^3 + c^3^6}{18 c l a^3 (3 a^3 c l + c^3^2)}$$

> **launchNZcase (o3);**

Launching case level 4:

$$o3 \neq 0$$

Assume from now on that:

$$6 a^3 c l (3 a^3 c l + c^3^2) o3 \neq 0$$

> **tmp1 := cpcoeff (x2^3);**

$$tmp1 := \frac{(3 a^3 c l + c^3^2)^3 (-9 o3 c l^2 a^3 + 27 c^3 c l^2 a^3 + 9 a^3 c l c^3^4 + c^3^6 + 27 a^3 c l^3) o3}{81 a^3 c l^4}$$

> **elimsolve (tmp1,o3);**

$$\{-9 c l^2 a^3 \neq 0\}$$

o3 is set to:

$$\frac{(3 a^3 c l + c^3^2)^3}{9 c l^2 a^3}$$

Nonzero constraint refines to:

$$6 a^3 c l (3 a^3 c l + c^3^2)^2 \neq 0$$

> **tmp1 := cpcoeff (x2^2\*T);**

$$tmp1 := -\frac{(3 a^3 c l + c^3^2)^6}{81 a^3 c l^4}$$

> **contradict (tmp1,'o3');**

Contradiction on case level 4, so:

$$o3 = 0$$

Variables to be uneliminated:

$$"o3 := 'o3'"$$

Proceed on case level 3 with:

$$6 a^3 c l (3 a^3 c l + c^3^2) \neq 0$$

On account of:

$$o3 = 0$$

$$\{1 \neq 0\}$$

o3 is set to:

$$0$$

> **tmp1 := cpcoeff (x2^2\*T);**

$$tmp1 := -\frac{(3 a^3 c l + c^3^2)^6}{81 a^3 c l^4}$$

> **contradict (tmp1,'c1');**

Contradiction on case level 3, so:

$$3 a^3 c l + c^3^2 = 0$$

Variables to be uneliminated:

$$"o3 := 'o3'"$$

$$"h3 := 'h3'"$$

Proceed on case level 2 with:

|                                       |                                                                   |
|---------------------------------------|-------------------------------------------------------------------|
|                                       | $6 a3 c1 \neq 0$                                                  |
| On account of:                        |                                                                   |
|                                       | $3 a3 c1 + c3^2 = 0$                                              |
|                                       | $\{3 a3 \neq 0\}$                                                 |
| c1 is set to:                         |                                                                   |
|                                       | $-\frac{c3^2}{3 a3}$                                              |
| Nonzero constraint refines to:        |                                                                   |
|                                       | $-6 a3 c3 \neq 0$                                                 |
| > <b>tmp1 := cpcoeff (x2^2*T);</b>    |                                                                   |
|                                       | $tmp1 := -o3^2$                                                   |
| > <b>elimsolve (tmp1,o3);</b>         |                                                                   |
|                                       | $\{1 \neq 0\}$                                                    |
| o3 is set to:                         |                                                                   |
|                                       | 0                                                                 |
| > <b>tmp1 := cpcoeff (x1^3*x3^3);</b> |                                                                   |
|                                       | $tmp1 := \frac{8 (3 h3 a3 - c3^2)^3}{27 a3^3}$                    |
| > <b>elimsolve (tmp1,h3);</b>         |                                                                   |
|                                       | $\{3 a3 \neq 0\}$                                                 |
| h3 is set to:                         |                                                                   |
|                                       | $\frac{c3^2}{3 a3}$                                               |
| > <b>tmp1 := cpcoeff (x3^4*T);</b>    |                                                                   |
|                                       | $tmp1 := -\frac{(27 q3 a3^2 - c3^3)^2}{81 a3^4}$                  |
| > <b>elimsolve (tmp1,q3);</b>         |                                                                   |
|                                       | $\{27 a3^2 \neq 0\}$                                              |
| q3 is set to:                         |                                                                   |
|                                       | $\frac{c3^3}{27 a3^2}$                                            |
| > <b>launchNZcase (p3);</b>           |                                                                   |
| Launching case level 3:               |                                                                   |
|                                       | $p3 \neq 0$                                                       |
| Assume from now on that:              |                                                                   |
|                                       | $-6 a3 c3 p3 \neq 0$                                              |
| > <b>tmp1 := cpcoeff (x1*x3^2*T);</b> |                                                                   |
|                                       | $tmp1 := -\frac{p3 (-18 u2 a3^2 c3 - c3^3 + 27 v2 a3^3)}{9 a3^3}$ |
| > <b>elimsolve (tmp1,v2);</b>         |                                                                   |
|                                       | $\{27 a3^3 \neq 0\}$                                              |
| v2 is set to:                         |                                                                   |

$$\frac{c3 (18 u2 a3^2 + c3^2)}{27 a3^3}$$

> **tmp1 := cpcoeff (x3^3\*T);**

$$tmp1 := -\frac{p3 (108 w2 a3^4 - c3^4 - 12 u2 a3^2 c3^2)}{27 a3^4}$$

> **elimsolve (tmp1,w2);**

$$\{108 a3^4 \neq 0\}$$

w2 is set to:

$$\frac{c3^2 (c3^2 + 12 u2 a3^2)}{108 a3^4}$$

> **tmp1 := cpcoeff (x1^4);**

$$tmp1 := -\frac{p3 (-2 d3 c3^2 + 9 c3 i3 a3 - c3 p3 + 18 i1 a3^2)}{9 a3^2}$$

> **elimsolve (tmp1,i1);**

$$\{18 a3^2 \neq 0\}$$

i1 is set to:

$$-\frac{c3 (-2 d3 c3 + 9 i3 a3 - p3)}{18 a3^2}$$

> **tmp1 := cpcoeff (x2\*T);**

$$tmp1 := \frac{p3 (c3 p3 - 6 c3 i3 a3 + 2 d3 c3^2 + 18 r3 a3^2)}{9 a3^2}$$

> **elimsolve (tmp1,r3);**

$$\{18 a3^2 \neq 0\}$$

r3 is set to:

$$\frac{c3 (-p3 + 6 i3 a3 - 2 d3 c3)}{18 a3^2}$$

> **tmp1 := cpcoeff (x1^3\*x3);**

$$tmp1 := \frac{2 c3^2 p3^2}{27 a3^3}$$

> **contradict (tmp1,'p3');**

Contradiction on case level 3, so:

$$p3 = 0$$

Variables to be uneliminated:

"r3 := 'r3'"

"i1 := 'i1'"

"w2 := 'w2'"

"v2 := 'v2'"

Proceed on case level 2 with:

$$-6 a3 c3 \neq 0$$

On account of:

$$p3 = 0$$

```

{1 ≠ 0}
p3 is set to:
0
> tmp1 := cpcoeff (x1^3);
tmp1 := 
$$\frac{(6\,c3\,i3\,a3 + 9\,i1\,a3^2 - 2\,d3\,c3^2)^3}{27\,a3^3\,c3^3}$$

> elimsolve (tmp1,i1);
{9 a3^2 ≠ 0}
i1 is set to:

$$-\frac{2\,c3\,(3\,i3\,a3 - d3\,c3)}{9\,a3^2}$$

> launchNZcase (3*i3*a3-2*d3*c3);
Launching case level 3:
3 i3 a3 - 2 d3 c3 ≠ 0
Assume from now on that:
-6 a3 c3 (3 i3 a3 - 2 d3 c3) ≠ 0
> tmp1 := cpcoeff (x1*x3*T);
tmp1 := 
$$-\frac{2\,(3\,i3\,a3 - 2\,d3\,c3)\,(9\,r3\,a3^2 - 3\,c3\,i3\,a3 + d3\,c3^2)}{27\,a3^3}$$

> elimsolve (tmp1,r3);
{9 a3^2 ≠ 0}
r3 is set to:

$$\frac{c3\,(3\,i3\,a3 - d3\,c3)}{9\,a3^2}$$

> tmp1 := cpcoeff (x1*T);
tmp1 := 
$$\frac{(3\,i3\,a3 - 2\,d3\,c3)\,(-9\,a3^2\,s3 + 9\,a3^2\,j1 + 6\,a3\,d3\,i3 + 6\,j3\,c3\,a3 - 4\,d3^2\,c3)}{27\,a3^3}$$

> elimsolve (tmp1,j1);
{9 a3^2 ≠ 0}
j1 is set to:

$$\frac{9\,a3^2\,s3 - 6\,a3\,d3\,i3 - 6\,j3\,c3\,a3 + 4\,d3^2\,c3}{9\,a3^2}$$

> tmp1 := cpcoeff (x3*T);
tmp1 := 
$$\frac{(3\,i3\,a3 - 2\,d3\,c3)^3}{81\,a3^4}$$

> contradict (tmp1,'i3');
Contradiction on case level 3, so:
3 i3 a3 - 2 d3 c3 = 0
Variables to be uneliminated:
"j1 := 'j1'"
"r3 := 'r3'"
Proceed on case level 2 with:

```

|                                         |                                                                         |
|-----------------------------------------|-------------------------------------------------------------------------|
|                                         | $-6 a3 c3 \neq 0$                                                       |
| On account of:                          |                                                                         |
|                                         | $3 i3 a3 - 2 d3 c3 = 0$                                                 |
|                                         | $\{3 a3 \neq 0\}$                                                       |
| i3 is set to:                           |                                                                         |
|                                         | $\frac{2 d3 c3}{3 a3}$                                                  |
| > <b>tmp1 := cpcoeff (x3^2*T);</b>      |                                                                         |
|                                         | $tmp1 := -\frac{4 (9 r3 a3^2 - d3 c3^2)^2}{81 a3^4}$                    |
| > <b>elimsolve (tmp1,r3);</b>           |                                                                         |
|                                         | $\{9 a3^2 \neq 0\}$                                                     |
| r3 is set to:                           |                                                                         |
|                                         | $\frac{c3^2 d3}{9 a3^2}$                                                |
| > <b>launchNZcase (j1+s3);</b>          |                                                                         |
| Launching case level 3:                 |                                                                         |
|                                         | $j1 + s3 \neq 0$                                                        |
| Assume from now on that:                |                                                                         |
|                                         | $-6 a3 c3 (j1 + s3) \neq 0$                                             |
| > <b>launchNZcase (-j3*c3+3*s3*a3);</b> |                                                                         |
| Launching case level 4:                 |                                                                         |
|                                         | $-j3 c3 + 3 s3 a3 \neq 0$                                               |
| Assume from now on that:                |                                                                         |
|                                         | $-6 a3 c3 (j1 + s3) (-j3 c3 + 3 s3 a3) \neq 0$                          |
| > <b>tmp1 := cpcoeff (1);</b>           |                                                                         |
|                                         | $tmp1 := \frac{(j1 + s3) (-j3 c3 + 3 s3 a3) (3 j1 a3 + j3 c3)}{9 a3^2}$ |
| > <b>elimsolve (tmp1,j1);</b>           |                                                                         |
|                                         | $\{3 a3 \neq 0\}$                                                       |
| j1 is set to:                           |                                                                         |
|                                         | $-\frac{j3 c3}{3 a3}$                                                   |
| Nonzero constraint refines to:          |                                                                         |
|                                         | $-6 a3 c3 (-j3 c3 + 3 s3 a3)^2 \neq 0$                                  |
| > <b>tmp1 := cpcoeff (T);</b>           |                                                                         |
|                                         | $tmp1 := -\frac{(-j3 c3 + 3 s3 a3)^2}{9 a3^2}$                          |
| > <b>contradict (tmp1,'s3');</b>        |                                                                         |
| Contradiction on case level 4, so:      |                                                                         |
|                                         | $-j3 c3 + 3 s3 a3 = 0$                                                  |
| Variables to be uneliminated:           |                                                                         |
|                                         | "j1 := 'j1'"                                                            |

Proceed on case level 3 with:

$$-6 a3 c3 (j1 + s3) \neq 0$$

On account of:

$$\begin{aligned} -j3 c3 + 3 s3 a3 &= 0 \\ \{3 a3 \neq 0\} \end{aligned}$$

s3 is set to:

$$\frac{j3 c3}{3 a3}$$

Nonzero constraint refines to:

$$-6 a3 c3 (3 j1 a3 + j3 c3) \neq 0$$

> **tmp1 := cpcoeff (T);**

$$tmp1 := -\frac{(3 j1 a3 + j3 c3)^2}{9 a3^2}$$

> **contradict (tmp1, 's3');**

Contradiction on case level 3, so:

$$j1 + s3 = 0$$

Variables to be uneliminated:

$$s3 := 's3''$$

Proceed on case level 2 with:

$$-6 a3 c3 \neq 0$$

On account of:

$$\begin{aligned} j1 + s3 &= 0 \\ \{1 \neq 0\} \end{aligned}$$

s3 is set to:

$$-j1$$

> **tmp1 := cpcoeff (T);**

$$tmp1 := -\frac{(3 j1 a3 + j3 c3)^2}{9 a3^2}$$

> **elimsolve (tmp1, j1);**

$$\{3 a3 \neq 0\}$$

j1 is set to:

$$-\frac{j3 c3}{3 a3}$$

> **det (T-jacobian (H, [x1, x2, x3]));**

$$T^3$$

> **H;**

$$\begin{aligned} &\left[ -\frac{c3 x1^3}{3} - \frac{c3^2 x1^2 x3}{3 a3} - \frac{d3 c3 x1^2}{3 a3} - \frac{c3^3 x1 x3^2}{9 a3^2} - \frac{2 c3^2 d3 x1 x3}{9 a3^2} - \frac{j3 c3 x1}{3 a3} - \frac{c3^4 x3^3}{81 a3^3} \right. \\ &\quad \left. - \frac{d3 c3^3 x3^2}{27 a3^3} - \frac{j3 c3^2 x3}{9 a3^2}, \frac{x1^4}{4} + u2 x1^2 x3^2 + v2 x1 x3^3 + w2 x3^4 + a2 x1^3 + c2 x1^2 x3 + d2 x1^2 \right. \\ &\quad \left. + h2 x1 x3^2 + i2 x1 x3 + j2 x1 + q2 x3^3 + r2 x3^2 + s2 x3, a3 x1^3 + c3 x1^2 x3 + d3 x1^2 \right] \end{aligned}$$

$$\left[ \frac{c^3 x_1 x_3^2}{3 a^3} + \frac{2 d_3 c_3 x_1 x_3}{3 a^3} + j_3 x_1 + \frac{c^3 x_3^3}{27 a^3} + \frac{c^3 d_3 x_3^2}{9 a^3} + \frac{j_3 c_3 x_3}{3 a^3} \right]$$

> **factor**(3\*a3\*H[1]+c3\*H[3]);

0

> **M := evalm**([[1,-c3/3/a3,0],[0,0,1],[0,1,0]]);

$$M := \begin{bmatrix} 1 & -\frac{c_3}{3 a^3} & 0 \\ 0 & 0 & 1 \\ 0 & 1 & 0 \end{bmatrix}$$

> **evalm**(**simplify**(**jacobian**(**evalm**(M^(-1) &

> **subs**({**seq**([x1,x2,x3][i]=**evalm**(M&\*[x1,x2,x3])[i],i=1..3)},H)),

> [x1,x2,x3])));

[0,0,0]

$$[3 a^3 x_1^2 + 2 d_3 x_1 + j_3, 0, 0]$$

$$\begin{aligned} & [(27 x_1^3 a^3 - 27 x_1^2 a^3 c_3 x_2 + 9 x_1 a_3 c_3^2 x_2^2 - c_3^3 x_2^3 + 54 u_2 x_2^2 a_3^3 x_1 \\ & - 18 u_2 x_2^3 a_3^2 c_3 + 27 v_2 x_2^3 a_3^3 + 81 a_2 a_3^3 x_1^2 - 54 a_2 a_3^2 x_1 c_3 x_2 + 9 a_2 a_3 c_3^2 x_2^2 \\ & + 54 c_2 x_2 a_3^3 x_1 - 18 c_2 x_2^2 a_3^2 c_3 + 54 d_2 a_3^3 x_1 - 18 d_2 a_3^2 c_3 x_2 + 27 h_2 x_2^2 a_3^3 \\ & + 27 i_2 x_2 a_3^3 + 27 j_2 a_3^3) / (27 a^3), -(27 c_3 x_1^3 a^3 - 243 q_2 x_2^2 a_3^4 - 162 r_2 x_2 a_3^4 \\ & - 81 c_2 a_3^4 x_1^2 - 81 s_2 a_3^4 - 324 w_2 x_2^3 a_3^4 - 27 x_1^2 a_3^2 c_3^2 x_2 + 9 x_1 a_3 c_3^3 x_2^2 \\ & - 36 u_2 x_2^3 c_3^2 a_3^2 - 162 u_2 x_2 a_3^4 x_1^2 - 243 v_2 x_2^2 a_3^4 x_1 - c_3^4 x_2^3 + 81 h_2 c_3 x_2^2 a_3^3 \\ & + 54 i_2 c_3 x_2 a_3^3 + 27 j_2 c_3 a_3^3 + 108 v_2 c_3 x_2^3 a_3^3 - 162 h_2 x_2 a_3^4 x_1 + 54 d_2 c_3 a_3^3 x_1 \\ & - 18 d_2 c_3^2 a_3^2 x_2 - 54 a_2 c_3^2 a_3^2 x_1 x_2 + 108 c_2 x_2 c_3 a_3^3 x_1 + 81 a_2 c_3 a_3^3 x_1^2 \\ & + 9 a_2 c_3^3 a_3 x_2^2 - 27 c_2 x_2^2 c_3^2 a_3^2 + 162 u_2 x_2^2 c_3 a_3^3 x_1 - 81 i_2 a_3^4 x_1) / (81 a^3), 0] \end{aligned}$$

> **contradict**(1,'c1');

Contradiction on case level 2, so:

$$c_1 = 0$$

Variables to be uneliminated:

"j1 := 'j1'"

"s3 := 's3'"

"r3 := 'r3'"

"i3 := 'i3'"

"i1 := 'i1'"

"p3 := 'p3'"

"q3 := 'q3'"

"h3 := 'h3'"

"o3 := 'o3'"

"c1 := 'c1'"

"d1 := 'd1'"

"a1 := 'a1'"

Proceed on case level 1 with:

|                                    |                       |
|------------------------------------|-----------------------|
|                                    | $6 a3 \neq 0$         |
| On account of:                     |                       |
|                                    | $c1 = 0$              |
|                                    | $\{1 \neq 0\}$        |
| c1 is set to:                      |                       |
|                                    | 0                     |
| > tmp1 := cpcoeff (x1^6);          |                       |
|                                    | $tmp1 := -c3^3$       |
| > elimsolve (tmp1,c3);             |                       |
|                                    | $\{1 \neq 0\}$        |
| c3 is set to:                      |                       |
|                                    | 0                     |
| > launchNZcase (a1);               |                       |
| Launching case level 2:            |                       |
|                                    | $a1 \neq 0$           |
| Assume from now on that:           |                       |
|                                    | $6 a3 a1 \neq 0$      |
| > tmp1 := cpcoeff (x1*x2^2*x3);    |                       |
|                                    | $tmp1 := 162 a1^4 h3$ |
| > elimsolve (tmp1,h3);             |                       |
|                                    | $\{1 \neq 0\}$        |
| h3 is set to:                      |                       |
|                                    | 0                     |
| > tmp1 := cpcoeff (x1^4*x2);       |                       |
|                                    | $tmp1 := 9 a1^2 o3$   |
| > elimsolve (tmp1,o3);             |                       |
|                                    | $\{1 \neq 0\}$        |
| o3 is set to:                      |                       |
|                                    | 0                     |
| > tmp1 := cpcoeff (x2^2*T);        |                       |
|                                    | $tmp1 := -81 a1^4$    |
| > contradict (tmp1,'a1');          |                       |
| Contradiction on case level 2, so: |                       |
|                                    | $a1 = 0$              |
| Variables to be uneliminated:      |                       |
|                                    | "o3 := 'o3'"          |
|                                    | "h3 := 'h3'"          |
| Proceed on case level 1 with:      |                       |
|                                    | $6 a3 \neq 0$         |
| On account of:                     |                       |
|                                    | $a1 = 0$              |
|                                    | $\{1 \neq 0\}$        |
| a1 is set to:                      |                       |
|                                    | 0                     |
| > tmp1 := cpcoeff (x2^2*T);        |                       |

```

[                                      $tmp1 := -o3^2$ 
> elimsolve (tmp1,o3);
                                      $\{1 \neq 0\}$ 
o3 is set to:
                                     0
[ > tmp1 := cpcoeff (x1^3*x3^3);
                                      $tmp1 := 8 h3^3$ 
> elimsolve (tmp1,h3);
                                      $\{1 \neq 0\}$ 
h3 is set to:
                                     0
[ > tmp1 := cpcoeff (x3^4*T);
                                      $tmp1 := -9 q3^2$ 
> elimsolve (tmp1,q3);
                                      $\{1 \neq 0\}$ 
q3 is set to:
                                     0
[ > launchNZcase (i1);
Launching case level 2:
                                      $il \neq 0$ 
Assume from now on that:
                                      $6 a3 il \neq 0$ 
> tmp1 := cpcoeff (x1^2*x3^3);
                                      $tmp1 := 36 a3^2 il w2$ 
> elimsolve (tmp1,w2);
                                      $\{1 \neq 0\}$ 
w2 is set to:
                                     0
[ > tmp1 := cpcoeff (x1^3*x3^2);
                                      $tmp1 := 27 a3^2 il v2$ 
> elimsolve (tmp1,v2);
                                      $\{1 \neq 0\}$ 
v2 is set to:
                                     0
[ > tmp1 := cpcoeff (x1^4*x3);
                                      $tmp1 := 18 a3^2 il u2$ 
> elimsolve (tmp1,u2);
                                      $\{1 \neq 0\}$ 
u2 is set to:
                                     0
[ > tmp1 := cpcoeff (x1^2*x3^2);
                                      $tmp1 := 27 a3^2 il q2$ 
> elimsolve (tmp1,q2);

```

|                                    |                                  |
|------------------------------------|----------------------------------|
|                                    | $\{1 \neq 0\}$                   |
| q2 is set to:                      |                                  |
|                                    | 0                                |
| > tmp1 := cpcoeff (x1^2*x2);       |                                  |
|                                    | $tmp1 := -9 a3^2 il (2 r3 + il)$ |
| > elimsolve (tmp1,r3);             |                                  |
|                                    | $\{2 \neq 0\}$                   |
| r3 is set to:                      |                                  |
|                                    | $-\frac{il}{2}$                  |
| > tmp1 := cpcoeff (x3^3);          |                                  |
|                                    | $tmp1 := 3 h2 a3 il^2$           |
| > elimsolve (tmp1,h2);             |                                  |
|                                    | $\{1 \neq 0\}$                   |
| h2 is set to:                      |                                  |
|                                    | 0                                |
| > tmp1 := cpcoeff (x3^2*T);        |                                  |
|                                    | $tmp1 := -il^2$                  |
| > contradict (tmp1,'il');          |                                  |
| Contradiction on case level 2, so: |                                  |
|                                    | $il = 0$                         |
| Variables to be uneliminated:      |                                  |
|                                    | "h2 := 'h2'"                     |
|                                    | "r3 := 'r3'"                     |
|                                    | "q2 := 'q2'"                     |
|                                    | "u2 := 'u2'"                     |
|                                    | "v2 := 'v2'"                     |
|                                    | "w2 := 'w2'"                     |
| Proceed on case level 1 with:      |                                  |
|                                    | $6 a3 \neq 0$                    |
| On account of:                     |                                  |
|                                    | $il = 0$                         |
|                                    | $\{1 \neq 0\}$                   |
| il is set to:                      |                                  |
|                                    | 0                                |
| > launchNZcase (p3);               |                                  |
| Launching case level 2:            |                                  |
|                                    | $p3 \neq 0$                      |
| Assume from now on that:           |                                  |
|                                    | $6 a3 p3 \neq 0$                 |
| > tmp1 := cpcoeff (x3^3*T);        |                                  |
|                                    | $tmp1 := -4 w2 p3$               |
| > elimsolve (tmp1,w2);             |                                  |
|                                    | $\{1 \neq 0\}$                   |

w2 is set to:

$$0$$

> tmp1 := cpcoeff (x1\*x3^2\*T);

$$tmp1 := -3 v2 p3$$

> elimsolve (tmp1,v2);

$$\{1 \neq 0\}$$

v2 is set to:

$$0$$

> tmp1 := cpcoeff (x2\*T);

$$tmp1 := 2 r3 p3$$

> elimsolve (tmp1,r3);

$$\{1 \neq 0\}$$

r3 is set to:

$$0$$

> tmp1 := cpcoeff (x1\*x3^3);

$$tmp1 := \frac{4 u2^2 p3^2}{3 a3}$$

> elimsolve (tmp1,u2);

$$\{1 \neq 0\}$$

u2 is set to:

$$0$$

> tmp1 := cpcoeff (x3^2\*T);

$$tmp1 := -3 q2 p3$$

> elimsolve (tmp1,q2);

$$\{1 \neq 0\}$$

q2 is set to:

$$0$$

> tmp1 := cpcoeff (x1\*x3\*T);

$$tmp1 := -2 h2 p3$$

> elimsolve (tmp1,h2);

$$\{1 \neq 0\}$$

h2 is set to:

$$0$$

> tmp1 := cpcoeff (x1\*T);

$$tmp1 := (-3 j1 i3 a3 - 3 i2 p3 a3 - 6 i3 a3 s3 - 6 d1 s3 a3 - 12 d1 a3 j1 + 2 d3 i3^2 + 2 d3 c2 p3 + 4 d3 d1 i3 + 8 d3 d1^2) / (3 a3)$$

> elimsolve (tmp1,i2);

$$\{-3 a3 p3 \neq 0\}$$

i2 is set to:

$$(-3 j1 i3 a3 - 6 i3 a3 s3 - 6 d1 s3 a3 - 12 d1 a3 j1 + 2 d3 i3^2 + 2 d3 c2 p3 + 4 d3 d1 i3 + 8 d3 d1^2) / (3 a3 p3)$$

> tmp1 := cpcoeff (x3\*T);

$$tmp1 := \frac{-6 r2 p3 a3 + i3^3 + i3 c2 p3 + 2 d1 i3^2 + 4 i3 d1^2}{3 a3}$$

> **elimsolve** (tmp1,r2);

$$\{-6 a3 p3 \neq 0\}$$

r2 is set to:

$$\frac{i3 (i3^2 + c2 p3 + 2 d1 i3 + 4 d1^2)}{6 a3 p3}$$

> **tmp1 := cpcoeff** (T);

tmp1 :=

$$\frac{-3 j1 s3 a3 - 3 s3^2 a3 - 3 s2 p3 a3 - 3 j1^2 a3 + j3 i3^2 + j3 c2 p3 + 2 j3 d1 i3 + 4 j3 d1^2}{3 a3}$$

> **elimsolve** (tmp1,s2);

$$\{-3 a3 p3 \neq 0\}$$

s2 is set to:

$$\frac{-3 j1 s3 a3 - 3 s3^2 a3 - 3 j1^2 a3 + j3 i3^2 + j3 c2 p3 + 2 j3 d1 i3 + 4 j3 d1^2}{3 a3 p3}$$

> **launchNZcase** (2\*d1+i3);

Launching case level 3:

$$2 d1 + i3 \neq 0$$

Assume from now on that:

$$6 a3 p3 (2 d1 + i3) \neq 0$$

> **tmp1 := cpcoeff** (x2);

$$tmp1 := - \frac{(2 d1 + i3) (i3^2 + c2 p3 + 2 d1 i3 + 4 d1^2) p3}{3 a3}$$

> **elimsolve** (tmp1,c2);

$$\{p3 \neq 0\}$$

c2 is set to:

$$- \frac{i3^2 + 2 d1 i3 + 4 d1^2}{p3}$$

> **tmp1 := cpcoeff** (1);

$$tmp1 := -j1^3$$

> **elimsolve** (tmp1,j1);

$$\{1 \neq 0\}$$

j1 is set to:

$$0$$

> **tmp1 := cpcoeff** (x1^3);

$$tmp1 := -8 d1^3$$

> **elimsolve** (tmp1,d1);

$$\{1 \neq 0\}$$

d1 is set to:

$$0$$

Nonzero constraint refines to:

$$6 a3 p3 i3 \neq 0$$

```

> det(T-jacobian(H,[x1,x2,x3]));

$$T^3$$

> H;

$$\left[ 0, \frac{x1^4}{4} + a2 x1^3 - \frac{i3^2 x1^2 x3}{p3} + d2 x1^2 - i3 x1 x2 - \frac{2 i3 s3 x1 x3}{p3} + j2 x1 - s3 x2 - \frac{s3^2 x3}{p3}, \right.$$


$$\left. a3 x1^3 + d3 x1^2 + i3 x1 x3 + j3 x1 + p3 x2 + s3 x3 \right]$$

> M := evalm([[i3,0,0], [0,0,1], [0,-p3,-s3]]);

$$M := \begin{bmatrix} i3 & 0 & 0 \\ 0 & 0 & 1 \\ 0 & -p3 & -s3 \end{bmatrix}$$

> det (M);

$$i3 p3$$

> G := simplify(evalm(M&*subs({seq([x1,x2,x3][i]=evalm(M^(-1)&*[x1,x2,x3])[i],i=1..n)},H)));
>

$$G := \left[ 0, \frac{a3 x1^3 + d3 x1^2 i3 + x1 x2 i3^3 + j3 x1 i3^2 - i3^3 x3}{i3^3}, -x1 (x1^3 p3 + 4 a2 x1^2 i3 p3 \right.$$


$$\left. - 4 x1 x2 i3^4 + 4 d2 x1 i3^2 p3 + 4 i3^4 x3 + 4 j2 i3^3 p3 + 4 i3 s3 a3 x1^2 + 4 i3^2 s3 d3 x1 \right.$$


$$\left. + 4 i3^3 s3 j3) / (4 i3^4) \right]$$

> simplify(jacobian(G,[x2,x3]));

$$\begin{bmatrix} 0 & 0 \\ x1 & -1 \\ x1^2 & -x1 \end{bmatrix}$$

> contradict (1,'i3');
Contradiction on case level 3, so:

$$2 d1 + i3 = 0$$

Variables to be uneliminated:

$$\begin{aligned} "d1" &:= 'd1' \\ "j1" &:= 'j1' \\ "c2" &:= 'c2' \end{aligned}$$

Proceed on case level 2 with:

$$6 a3 p3 \neq 0$$

On account of:

$$2 d1 + i3 = 0$$


$$\{1 \neq 0\}$$

i3 is set to:

$$-2 d1$$

> launchNZcase (4*d1^2+c2*p3);
Launching case level 3:

$$4 d1^2 + c2 p3 \neq 0$$

Assume from now on that:

```

```

[
    6 a3 p3 (4 d1^2 + c2 p3) ≠ 0
> tmp1 := cpcoeff (x1*x3);
    tmp1 := -  $\frac{2 (4 d1^2 + c2 p3) (-c2 p3 + 2 d1^2)}{3 a3}$ 
> elimsolve (tmp1,c2);
    {-p3 ≠ 0}
c2 is set to:
     $\frac{2 d1^2}{p3}$ 
Nonzero constraint refines to:
    36 a3 p3 d1 ≠ 0
> tmp1 := cpcoeff (x1^3);
    tmp1 :=  $\frac{2 d1^2 (2 d1 a3 + p3)}{a3}$ 
> elimsolve (tmp1,p3);
    {1 ≠ 0}
p3 is set to:
    -2 d1 a3
Nonzero constraint refines to:
    -72 a3^2 d1^2 ≠ 0
> tmp1 := cpcoeff (x3);
    tmp1 :=  $\frac{4 d1^3 (-3 j1 a3 + 2 d3 d1)}{a3^2}$ 
> elimsolve (tmp1,j1);
    {-3 a3 ≠ 0}
j1 is set to:
     $\frac{2 d3 d1}{3 a3}$ 
> tmp1 := cpcoeff (x1^2);
    tmp1 := -  $\frac{2 d1^2 (-4 d3 d1 - 3 s3 a3 + 6 a2 d1 a3)}{a3}$ 
> elimsolve (tmp1,s3);
    {-3 a3 ≠ 0}
s3 is set to:
     $\frac{2 d1 (-2 d3 + 3 a2 a3)}{3 a3}$ 
> tmp1 := cpcoeff (1);
    tmp1 :=  $\frac{4 d1^3 (-2 d3^3 - 27 j2 a3^3 + 27 j3 a3^2 a2)}{27 a3^3}$ 
> elimsolve (tmp1,j2);
    {-27 a3^3 ≠ 0}
j2 is set to:

```

$$\frac{-2 d3^3 + 27 j3 a3^2 a2}{27 a3^3}$$

> tmp1 := cpcoeff (x1);

$$tmp1 := \frac{4 d1^3 (-2 d3^2 + 6 d3 a2 a3 + 3 j3 a3 - 6 d2 a3^2)}{3 a3^2}$$

> elimsolve (tmp1,d2);

$$\{-6 a3^2 \neq 0\}$$

d2 is set to:

$$\frac{-2 d3^2 + 6 d3 a2 a3 + 3 j3 a3}{6 a3^2}$$

> det(T-jacobian(H,[x1,x2,x3]));

$$T^3$$

> simplify(evalm([H[1],H[2],H[3]]));

$$\left[ \frac{d1 (3 a3 x1^2 + 2 d3 x1 - 6 d1 x3)}{3 a3}, (27 x1^4 a3^3 + 108 a2 x1^3 a3^3 - 108 d1 x1^2 x3 a3^2 - 36 a3 x1^2 d3^2 + 108 a3^2 x1^2 d3 a2 + 54 a3^2 x1^2 j3 - 216 d1 a2 a3^2 x1 x3 - 8 x1 d3^3 + 108 x1 j3 a3^2 a2 + 72 d1 x2 a3^2 d3 - 216 d1 x2 a3^3 a2 + 108 d1^2 x3^2 a3 + 72 d1 x3 d3^2 - 216 d1 x3 d3 a2 a3 + 216 d1 x3 a2^2 a3^2 - 108 d1 x3 j3 a3) / (108 a3^3), (3 a3^2 x1^3 + 3 d3 x1^2 a3 - 6 d1 x1 x3 a3 + 3 j3 x1 a3 - 6 d1 x2 a3^2 - 4 d1 x3 d3 + 6 d1 x3 a2 a3) / (3 a3) \right]$$

> factor(12\*d1^2\*(3\*a3^2\*H[2]+(d3-3\*a2\*a3)\*H[3]) -

> 9\*a3^2\*H[1]^2 + 2\*d1\*(2\*d3^2-9\*j3\*a3)\*H[1]);

$$0$$

> G := [x2-x1^2, x3+2\*x1\*(x2-x1^2), -(x2-x1^2)^2];

$$G := [x2 - x1^2, x3 + 2 x1 (x2 - x1^2), -(x2 - x1^2)^2]$$

> M := evalm([-d1,0,0], [-2/3\*d3\*d1^2/a3,0,2\*d1^3/a3],

> [2/9\*d1^3\*(-2\*d3^2+9\*j3\*a3)/a3^2,-4\*d1^4,

> 4/3\*d1^4\*(-d3+3\*a2\*a3)/a3^2]);

$$M := \begin{bmatrix} -d1 & 0 & 0 \\ -\frac{2 d3 d1^2}{3 a3} & 0 & \frac{2 d1^3}{a3} \\ \frac{2 d1^3 (-2 d3^2 + 9 j3 a3)}{9 a3^2} & -4 d1^4 & \frac{4 d1^4 (-d3 + 3 a2 a3)}{3 a3^2} \end{bmatrix}$$

> det(M);

$$-\frac{8 d1^8}{a3}$$

> evalm(simplify(evalm(M^(-1)&\*

> subs({seq([x1,x2,x3][i]=evalm(M&\*[x1,x2,x3])[i],i=1..n)}),

```
> evalm(G) - H));
```

$[0, 0, 0]$

```
> G[3] + G[1]^2; rank (jacobian (G, [x1,x2,x3]));
```

0

2

```
> contradict(1, 'c2');
```

Contradiction on case level 3, so:

$$4 d l^2 + c_2 p_3 = 0$$

Variables to be uneliminated:

"d2 := 'd2'"

"j2 := 'j2'"

"s3 := 's3'"

"j1 := 'j1'"

"p3 := 'p3'"

"c2 := 'c2'"

Proceed on case level 2 with:

$$6 a_3 p_3 \neq 0$$

On account of:

$$4 d l^2 + c_2 p_3 = 0$$

$$\{p_3 \neq 0\}$$

c2 is set to:

$$-\frac{4 d l^2}{p_3}$$

```
> tmp1 := cpcoeff (1);
```

$$tmp1 := -j l^3$$

```
> elimsolve (tmp1, j1);
```

$$\{1 \neq 0\}$$

j1 is set to:

0

```
> tmp1 := cpcoeff (x1^3);
```

$$tmp1 := -8 d l^3$$

```
> elimsolve (tmp1, d1);
```

$$\{1 \neq 0\}$$

d1 is set to:

0

```
> det(T-jacobian(H, [x1,x2,x3]));
```

$T^3$

```
> H;
```

$$\left[ 0, \frac{x l^4}{4} + a_2 x l^3 + d_2 x l^2 + j_2 x l - s_3 x_2 - \frac{s_3^2 x_3}{p_3}, a_3 x l^3 + d_3 x l^2 + j_3 x l + p_3 x_2 + s_3 x_3 \right]$$

```
> M := evalm([[1,0,0],[0,1,-s3/p3],[0,0,1]]);
```

$$M := \begin{bmatrix} 1 & 0 & 0 \\ 0 & 1 & -\frac{s^3}{p^3} \\ 0 & 0 & 1 \end{bmatrix}$$

```
> evalm(simplify(jacobian(evalm(M^(-1) &*
> subs({seq([x1,x2,x3][i]=evalm(M&*[x1,x2,x3])[i],i=1..3}),H)),
> [x1,x2,x3])));
```

$$\begin{bmatrix} 0 & 0 & 0 \\ \frac{x_1^3 p^3 + 3 a_2 x_1^2 p^3 + 2 d_2 x_1 p^3 + j_2 p^3 + 3 s_3 a_3 x_1^2 + 2 s_3 d_3 x_1 + s_3 j_3}{p^3} & 0 & 0 \\ 3 a_3 x_1^2 + 2 d_3 x_1 + j_3 & p^3 & 0 \end{bmatrix}$$

```
> contradict (1,'p3');
```

Contradiction on case level 2, so:

$$p^3 = 0$$

Variables to be uneliminated:

"d1 := 'd1'"

"j1 := 'j1'"

"c2 := 'c2'"

"i3 := 'i3'"

"s2 := 's2'"

"r2 := 'r2'"

"i2 := 'i2'"

"h2 := 'h2'"

"q2 := 'q2'"

"u2 := 'u2'"

"r3 := 'r3'"

"v2 := 'v2'"

"w2 := 'w2'"

Proceed on case level 1 with:

$$6 a_3 \neq 0$$

On account of:

$$p^3 = 0$$

$$\{1 \neq 0\}$$

p3 is set to:

$$0$$

```
> tmp1 := cpcoeff (x3^2*T);
```

$$tmp1 := -4 r_3^2$$

```
> elimsolve (tmp1,r3);
```

$$\{1 \neq 0\}$$

r3 is set to:

$$0$$

```
> tmp1 := cpcoeff (x1^3);
```

|                                  |                                    |                                  |
|----------------------------------|------------------------------------|----------------------------------|
| [                                |                                    | $tmp1 := (2\ d1 + i3)^3$         |
| > <b>elimsolve</b> (tmp1,i3);    |                                    | $\{1 \neq 0\}$                   |
|                                  | i3 is set to:                      | $-2\ d1$                         |
| > <b>tmp1 := cpcoeff</b> (x3*T); |                                    | $tmp1 := -\frac{8\ d1^3}{3\ a3}$ |
| > <b>elimsolve</b> (tmp1,d1);    |                                    | $\{1 \neq 0\}$                   |
|                                  | d1 is set to:                      | 0                                |
| > <b>launchNZcase</b> (j1);      |                                    |                                  |
|                                  | Launching case level 2:            | $j1 \neq 0$                      |
|                                  | Assume from now on that:           | $6\ j1\ a3 \neq 0$               |
| > <b>launchNZcase</b> (s3);      |                                    |                                  |
|                                  | Launching case level 3:            | $s3 \neq 0$                      |
|                                  | Assume from now on that:           | $6\ j1\ s3\ a3 \neq 0$           |
| > <b>tmp1 := cpcoeff</b> (1);    |                                    | $tmp1 := j1\ (j1 + s3)\ s3$      |
| > <b>elimsolve</b> (tmp1,s3);    |                                    | $\{1 \neq 0\}$                   |
|                                  | s3 is set to:                      | $-j1$                            |
|                                  | Nonzero constraint refines to:     | $-6\ j1^2\ a3 \neq 0$            |
| > <b>tmp1 := cpcoeff</b> (T);    |                                    | $tmp1 := -j1^2$                  |
| > <b>contradict</b> (tmp1,'s3'); |                                    |                                  |
|                                  | Contradiction on case level 3, so: | $s3 = 0$                         |
|                                  | Variables to be uneliminated:      | "s3 := 's3'"                     |
|                                  | Proceed on case level 2 with:      | $6\ j1\ a3 \neq 0$               |
|                                  | On account of:                     | $s3 = 0$                         |
|                                  |                                    | $\{1 \neq 0\}$                   |
|                                  | s3 is set to:                      | 0                                |
| > <b>tmp1 := cpcoeff</b> (T);    |                                    |                                  |

```

|                                      $tmp1 := -j l^2$ 
| > contradict (tmp1,'j1');
| Contradiction on case level 2, so:
|                                      $j l = 0$ 
| Variables to be uneliminated:
|                                     "s3 := 's3'"
| Proceed on case level 1 with:
|                                      $6 a3 \neq 0$ 
| On account of:
|                                      $j l = 0$ 
|                                      $\{1 \neq 0\}$ 
| j1 is set to:
|                                     0
| > tmp1 := cpcoeff (T);
|                                      $tmp1 := -s3^2$ 
| > elimsolve (tmp1,s3);
|                                      $\{1 \neq 0\}$ 
| s3 is set to:
|                                     0
| > det(T-jacobian(H,[x1,x2,x3]));
|                                      $T^3$ 
| > H;
|  $\left[ 0, \frac{x l^4}{4} + u2 x l^2 x3^2 + v2 x l x3^3 + w2 x3^4 + a2 x l^3 + c2 x l^2 x3 + d2 x l^2 + h2 x l x3^2 + i2 x l x3 \right.$ 
|  $\left. + j2 x l + q2 x3^3 + r2 x3^2 + s2 x3, a3 x l^3 + d3 x l^2 + j3 x l \right]$ 
| > M := evalm([[1,0,0],[0,0,1],[0,1,0]]);
|                                      $M := \begin{bmatrix} 1 & 0 & 0 \\ 0 & 0 & 1 \\ 0 & 1 & 0 \end{bmatrix}$ 
| > evalm(simplify(jacobian(evalm(M^(-1)&*
| > subs ({seq([x1,x2,x3][i]=evalm(M&*[x1,x2,x3])[i],i=1..3)},H)),
| > [x1,x2,x3]));
| [0,0,0]
|  $[3 a3 x l^2 + 2 d3 x l + j3, 0, 0]$ 
|  $[x l^3 + 2 u2 x l x2^2 + v2 x2^3 + 3 a2 x l^2 + 2 c2 x l x2 + 2 d2 x l + h2 x2^2 + i2 x2 + j2,$ 
|  $2 u2 x l^2 x2 + 3 v2 x l x2^2 + 4 w2 x2^3 + c2 x l^2 + 2 h2 x l x2 + i2 x l + 3 q2 x2^2 + 2 r2 x2 + s2, 0]$ 
| > contradict (1,'a3');
| Contradiction on case level 1, so:
|                                      $a3 = 0$ 
| Variables to be uneliminated:
|                                     "s3 := 's3'"
|                                     "j1 := 'j1'"

```

```

"d1 := 'd1'"
"i3 := 'i3'"
"r3 := 'r3'"
"p3 := 'p3'"
"i1 := 'i1'"
"q3 := 'q3'"
"h3 := 'h3'"
"o3 := 'o3'"
"a1 := 'a1'"
"c3 := 'c3'"
"c1 := 'c1'"
"g3 := 'g3'"
"s1 := 's1'"
"r1 := 'r1'"
"q1 := 'q1'"
"h1 := 'h1'"

```

Proceed on case level 0 with:

$$6 \neq 0$$

On account of:

$$a3 = 0$$

$$\{1 \neq 0\}$$

a3 is set to:

$$0$$

> **launchNZcase (g3);**

Launching case level 1:

$$g3 \neq 0$$

Assume from now on that:

$$6 g3 \neq 0$$

> **tmp1 := cpcoeff (x1^6);**

$$tmp1 := -c1 g3 - c3^3$$

> **elimsolve (tmp1,c1);**

$$\{g3 \neq 0\}$$

c1 is set to:

$$-\frac{c3^3}{g3}$$

> **tmp1 := cpcoeff (x1^2\*x2\*T);**

$$tmp1 := -9 a1^2 c3 - 3 a1 c3^2 - 2 c3^3 - 3 a1 o3 - 2 o3 c3 + 2 g3 h3$$

> **elimsolve (tmp1,h3);**

$$\{-2 g3 \neq 0\}$$

h3 is set to:

$$\frac{9 a1^2 c3 + 3 a1 c3^2 + 2 c3^3 + 3 a1 o3 + 2 o3 c3}{2 g3}$$

```

> tmp1 := cpcoeff (x1^4*x2);
      tmp1 := 3 o3 c3^2 + 9 al o3 c3 + 27 al^2 c3^2 + 2 u2 g3^2
> elimsolve (tmp1,u2);
      {2 g3^2 ≠ 0}
u2 is set to:
      - 3 c3 (o3 c3 + 3 al o3 + 9 al^2 c3)
        2 g3^2
> tmp1 := cpcoeff (x1^5*x3);
      tmp1 := - 81 al^3 c3^2 + 3 al c3^4 + 27 al^2 c3 o3 + 9 al c3^2 o3 + 2 g3^2 hl + 2 c3^5 + 2 c3^3 o3
                g3
> elimsolve (tmp1,h1);
      {2 g3^2 ≠ 0}
h1 is set to:
      - c3 (81 al^3 c3 + 3 al c3^3 + 27 al^2 o3 + 9 al o3 c3 + 2 c3^4 + 2 o3 c3^2)
        2 g3^2
> tmp1 := cpcoeff (x1^5);
      tmp1 := (
      -il g3^2 + 4 d3 c3^4 + 3 al c2 g3^2 + 3 a2 c3^3 g3 - 3 c3^2 i3 g3 - c3 c2 g3^2 + 6 d3 c3^3 al + c3^3 p3
      ) / g3
> elimsolve (tmp1,i1);
      {-g3^2 ≠ 0}
i1 is set to:
      4 d3 c3^4 + 3 al c2 g3^2 + 3 a2 c3^3 g3 - 3 c3^2 i3 g3 - c3 c2 g3^2 + 6 d3 c3^3 al + c3^3 p3
      g3^2
> tmp1 := cpcoeff (x1*x2*x3*T);
      tmp1 := - (18 al^2 c3^3 + 6 al c3^4 + 162 al^4 c3 + 54 al^3 o3 + 27 al^2 c3 o3 + 9 al c3^2 o3 + 2 c3^5
      + 2 c3^3 o3 - 6 q3 g3^2 + 3 al o3^2 + 2 o3^2 c3) / g3
> elimsolve (tmp1,q3);
      {-6 g3^2 ≠ 0}
q3 is set to:
      (18 al^2 c3^3 + 6 al c3^4 + 162 al^4 c3 + 54 al^3 o3 + 27 al^2 c3 o3 + 9 al c3^2 o3 + 2 c3^5
      + 2 c3^3 o3 + 3 al o3^2 + 2 o3^2 c3) / (6 g3^2)
> tmp1 := cpcoeff (x1^2*x3^2*T);
      tmp1 := - 3 (2 o3^2 c3^2 + 2 v2 g3^3 + 45 al^2 c3^4 + 162 al^5 c3 + 54 al^4 o3 + 9 al^2 o3^2
      + 162 al^4 c3^2 + 2 c3^4 o3 + 6 al o3^2 c3 + 12 c3^3 al o3 + 18 al^2 c3^2 o3 + 99 c3 al^3 o3
      - 27 al^3 c3^3) / (2 g3^2)
> elimsolve (tmp1,v2);
      {2 g3^3 ≠ 0}
v2 is set to:
      - (2 o3^2 c3^2 + 45 al^2 c3^4 + 162 al^5 c3 + 54 al^4 o3 + 9 al^2 o3^2 + 162 al^4 c3^2 + 2 c3^4 o3

```

$$+ 6 a l o 3^2 c 3 + 12 c 3^3 a l o 3 + 18 a l^2 c 3^2 o 3 + 99 c 3 a l^3 o 3 - 27 a l^3 c 3^3) / (2 g 3^3)$$

> **tmp1 := cpcoeff (x2\*x3^2\*T);**

$$\begin{aligned} tmp1 := & (-2 c 3^7 - 6 q l g 3^3 + 486 a l^5 o 3 + 1458 a l^6 c 3 - 2 c 3^3 o 3^2 - 2 c 3^5 o 3 - 6 a l c 3^6 \\ & - 1215 a l^5 c 3^2 - 54 a l^3 c 3^4 - 243 a l^4 c 3^3 - 9 a l c 3^2 o 3^2 - 27 a l^2 c 3 o 3^2 - 15 a l c 3^4 o 3 \\ & - 72 a l^2 c 3^3 o 3 - 297 a l^3 c 3^2 o 3 - 243 a l^4 c 3 o 3) / (2 g 3^2) \end{aligned}$$

> **elimsolve (tmp1,q1);**

$$\{-6 g 3^3 \neq 0\}$$

q1 is set to:

$$\begin{aligned} & (-2 c 3^7 + 486 a l^5 o 3 + 1458 a l^6 c 3 - 2 c 3^3 o 3^2 - 2 c 3^5 o 3 - 6 a l c 3^6 - 1215 a l^5 c 3^2 \\ & - 54 a l^3 c 3^4 - 243 a l^4 c 3^3 - 9 a l c 3^2 o 3^2 - 27 a l^2 c 3 o 3^2 - 15 a l c 3^4 o 3 - 72 a l^2 c 3^3 o 3 \\ & - 297 a l^3 c 3^2 o 3 - 243 a l^4 c 3 o 3) / (6 g 3^3) \end{aligned}$$

> **tmp1 := cpcoeff (x1^2\*x3\*T);**

$$\begin{aligned} tmp1 := & (8 c 3^3 i 3 g 3 - 18 a l a 2 c 3^3 g 3 + 27 a 2 g 3 a l^2 o 3 + 81 a 2 g 3 a l^3 c 3 + 3 a 2 g 3 o 3 c 3^2 \\ & - 4 d l g 3 o 3 c 3 - 6 d l g 3 a l o 3 - 6 d l g 3 a l c 3^2 - 18 d l g 3 a l^2 c 3 + 3 a l c 3 c 2 g 3^2 \\ & + 12 a l c 3^2 i 3 g 3 + 18 d 3 c 3^2 a l o 3 - 4 i 3 g 3 o 3 c 3 - 6 i 3 g 3 a l o 3 - 18 i 3 g 3 a l^2 c 3 \\ & + 9 c 3 p 3 a l o 3 - 2 h 2 g 3^3 - c 2 o 3 g 3^2 - 6 a l r 3 g 3^2 + 9 a 2 g 3 a l o 3 c 3 - 36 a l d 3 c 3^4 \\ & - 6 a l c 3^3 p 3 - 36 d 3 c 3^3 a l^2 + 4 c 3^3 g 3 d l - 9 a 2 c 3^4 g 3 - 8 d 3 c 3^5 + 5 c 3^2 c 2 g 3^2 - 3 c 3^4 p 3 \\ & + 54 d 3 c 3 a l^2 o 3 + 162 d 3 c 3^2 a l^3 + 4 d 3 c 3^3 o 3 + 3 c 3^2 p 3 o 3 + 27 c 3^2 p 3 a l^2 - 4 r 3 g 3^2 c 3) \\ & / g 3^2 \end{aligned}$$

> **elimsolve (tmp1,h2);**

$$\{-2 g 3^3 \neq 0\}$$

h2 is set to:

$$\begin{aligned} & (8 c 3^3 i 3 g 3 - 18 a l a 2 c 3^3 g 3 + 27 a 2 g 3 a l^2 o 3 + 81 a 2 g 3 a l^3 c 3 + 3 a 2 g 3 o 3 c 3^2 \\ & - 4 d l g 3 o 3 c 3 - 6 d l g 3 a l o 3 - 6 d l g 3 a l c 3^2 - 18 d l g 3 a l^2 c 3 + 3 a l c 3 c 2 g 3^2 \\ & + 12 a l c 3^2 i 3 g 3 + 18 d 3 c 3^2 a l o 3 - 4 i 3 g 3 o 3 c 3 - 6 i 3 g 3 a l o 3 - 18 i 3 g 3 a l^2 c 3 \\ & + 9 c 3 p 3 a l o 3 - c 2 o 3 g 3^2 - 6 a l r 3 g 3^2 + 9 a 2 g 3 a l o 3 c 3 - 36 a l d 3 c 3^4 - 6 a l c 3^3 p 3 \\ & - 36 d 3 c 3^3 a l^2 + 4 c 3^3 g 3 d l - 9 a 2 c 3^4 g 3 - 8 d 3 c 3^5 + 5 c 3^2 c 2 g 3^2 - 3 c 3^4 p 3 \\ & + 54 d 3 c 3 a l^2 o 3 + 162 d 3 c 3^2 a l^3 + 4 d 3 c 3^3 o 3 + 3 c 3^2 p 3 o 3 + 27 c 3^2 p 3 a l^2 - 4 r 3 g 3^2 c 3) \\ & / (2 g 3^3) \end{aligned}$$

> **tmp1 := cpcoeff (x1^4\*x3);**

$$\begin{aligned} tmp1 := & (81 a 2 a l^2 c 3 g 3 o 3 + 81 a 2 a l^3 g 3 o 3 + 12 d 3 c 3^3 a l o 3 + 9 c 2 g 3^2 a l c 3^2 \\ & - c 2 g 3^2 o 3 c 3 - 54 a 2 a l^2 c 3^3 g 3 + 243 a 2 a l^4 g 3 c 3 - 18 a 2 a l c 3^4 g 3 - 15 a l i 3 g 3 o 3 c 3 \\ & - 2 c 3^2 i 3 g 3 o 3 + 162 a 2 a l^3 c 3^2 g 3 + o 3 c 3^3 p 3 - 18 a l^2 d l g 3 o 3 + 27 a l^2 i 3 g 3 c 3^2 \\ & + 15 a l i 3 g 3 c 3^3 - 54 a l^3 i 3 g 3 c 3 + 18 a l d l g 3 c 3^3 + 3 a 2 c 3^3 o 3 g 3 - 24 a l d l g 3 o 3 c 3 \\ & - 18 a l^2 i 3 g 3 o 3 - 2 d l c 3^2 g 3 o 3 - 2 c 3^4 i 3 g 3 + 3 a 2 c 3^5 g 3 - 108 d 3 c 3^4 a l^2 \\ & - 6 a l c 2 o 3 g 3^2 - 54 a l^3 d l g 3 c 3 - 54 a l^2 d l g 3 c 3^2 - 2 r l g 3^3 + 4 d 3 c 3^6 + 9 a l c 3^2 p 3 o 3 \\ & - 6 a l r 3 g 3^2 c 3 + 486 d 3 c 3^2 a l^4 + 81 c 3^2 p 3 a l^3 + 54 d 3 c 3^2 a l^2 o 3 + 27 c 3 p 3 a l^2 o 3) \end{aligned}$$

$$+ 162 d3 c3 a l^3 o3 + c3^5 p3 - 18 a l^2 r3 g3^2 - 18 a l^2 c3^3 p3 - 108 d3 c3^3 a l^3 - 6 a l c3^4 p3 \\ + 2 d3 c3^4 o3 - c2 g3^2 c3^3 - 2 r3 g3^2 c3^2 + 27 a2 a l c3^2 g3 o3) / g3^2$$

> **elimsolve (tmp1,r1);**

$$\{-2 g3^3 \neq 0\}$$

r1 is set to:

$$(81 a2 a l^2 c3 g3 o3 + 81 a2 a l^3 g3 o3 + 12 d3 c3^3 a l o3 + 9 c2 g3^2 a l c3^2 - c2 g3^2 o3 c3 \\ - 54 a2 a l^2 c3^3 g3 + 243 a2 a l^4 g3 c3 - 18 a2 a l c3^4 g3 - 15 a l i3 g3 o3 c3 - 2 c3^2 i3 g3 o3 \\ + 162 a2 a l^3 c3^2 g3 + o3 c3^3 p3 - 18 a l^2 d l g3 o3 + 27 a l^2 i3 g3 c3^2 + 15 a l i3 g3 c3^3 \\ - 54 a l^3 i3 g3 c3 + 18 a l d l g3 c3^3 + 3 a2 c3^3 o3 g3 - 24 a l d l g3 o3 c3 - 18 a l^2 i3 g3 o3 \\ - 2 d l c3^2 g3 o3 - 2 c3^4 i3 g3 + 3 a2 c3^5 g3 - 108 d3 c3^4 a l^2 - 6 a l c2 o3 g3^2 \\ - 54 a l^3 d l g3 c3 - 54 a l^2 d l g3 c3^2 + 4 d3 c3^6 + 9 a l c3^2 p3 o3 - 6 a l r3 g3^2 c3 \\ + 486 d3 c3^2 a l^4 + 81 c3^2 p3 a l^3 + 54 d3 c3^2 a l^2 o3 + 27 c3 p3 a l^2 o3 + 162 d3 c3 a l^3 o3 \\ + c3^5 p3 - 18 a l^2 r3 g3^2 - 18 a l^2 c3^3 p3 - 108 d3 c3^3 a l^3 - 6 a l c3^4 p3 + 2 d3 c3^4 o3 \\ - c2 g3^2 c3^3 - 2 r3 g3^2 c3^2 + 27 a2 a l c3^2 g3 o3) / (2 g3^3)$$

> **tmp1 := cpcoeff (x1^4);**

$$(tmp1 := (-s1 g3^3 + j1 c3^2 g3^2 + 3 p3 c3^2 i3 g3 + p3 c3 c2 g3^2 + 3 a l s3 g3^2 c3 + 6 a l c3 g3^2 j1 \\ + 2 i3 g3^2 d l c3 - i3 g3^3 c2 + 4 d l^2 c3 g3^2 - s3 g3^2 c3^2 + 18 d3 a l c3^2 i3 g3 + 4 d3 c3^2 c2 g3^2 \\ + 3 j3 c3^3 g3 a l - c3^3 p3^2 - 6 d3 c3^4 p3 - 36 d3^2 c3^3 a l^2 + j3 c3^4 g3 - 2 i3^2 g3^2 c3 \\ - 12 d3 a l c3^3 p3 - 36 a l d3^2 c3^4 - 8 d3^2 c3^5 + 4 d3 c3^3 g3 d l + 10 d3 c3^3 g3 i3 \\ - 36 a2 g3 d3 c3^3 a l - 9 a2 i3 g3^2 a l c3 - 12 a2 g3 d3 c3^4 - 9 a2 g3^3 a l c2 + 3 a2 g3^2 c3^2 i3 \\ - 6 d2 c3^2 g3^2 a l - 18 d2 c3 g3^2 a l^2 - 3 a2 c3^3 p3 g3 + 3 a l i2 g3^3 + 2 d l c2 g3^3 \\ - 36 a2 g3^2 c3 a l d l - 6 a2 g3^2 c3^2 d l + 27 a2^2 g3^2 c3^2 a l + 81 a2^2 g3^2 c3 a l^2 \\ + 6 d3 c2 g3^2 a l c3) / g3^2$$

> **elimsolve (tmp1,s1);**

$$\{-g3^3 \neq 0\}$$

s1 is set to:

$$(j1 c3^2 g3^2 + 3 p3 c3^2 i3 g3 + p3 c3 c2 g3^2 + 3 a l s3 g3^2 c3 + 6 a l c3 g3^2 j1 + 2 i3 g3^2 d l c3 \\ - i3 g3^3 c2 + 4 d l^2 c3 g3^2 - s3 g3^2 c3^2 + 18 d3 a l c3^2 i3 g3 + 4 d3 c3^2 c2 g3^2 + 3 j3 c3^3 g3 a l \\ - c3^3 p3^2 - 6 d3 c3^4 p3 - 36 d3^2 c3^3 a l^2 + j3 c3^4 g3 - 2 i3^2 g3^2 c3 - 12 d3 a l c3^3 p3 \\ - 36 a l d3^2 c3^4 - 8 d3^2 c3^5 + 4 d3 c3^3 g3 d l + 10 d3 c3^3 g3 i3 - 36 a2 g3 d3 c3^3 a l \\ - 9 a2 i3 g3^2 a l c3 - 12 a2 g3 d3 c3^4 - 9 a2 g3^3 a l c2 + 3 a2 g3^2 c3^2 i3 - 6 d2 c3^2 g3^2 a l \\ - 18 d2 c3 g3^2 a l^2 - 3 a2 c3^3 p3 g3 + 3 a l i2 g3^3 + 2 d l c2 g3^3 - 36 a2 g3^2 c3 a l d l \\ - 6 a2 g3^2 c3^2 d l + 27 a2^2 g3^2 c3^2 a l + 81 a2^2 g3^2 c3 a l^2 + 6 d3 c2 g3^2 a l c3) / g3^3$$

> **tmp1 := cpcoeff (x1^2\*T);**

$$(tmp1 := -(-6 d2 g3^2 a l c3 - 36 a2 g3^2 a l d l + 9 a2^2 g3^2 c3^2 + 81 a2^2 g3^2 a l^2 + 4 d l^2 g3^2 \\ + 8 d3^2 c3^4 - 2 d2 g3^2 c3^2 + 6 a l g3^2 j1 - 18 d2 g3^2 a l^2 + c2 p3 g3^2 + i2 g3^3 + i3^2 g3^2 \\ - 9 a2 g3^2 a l i3 - 6 a2 g3^2 c3 i3 + 27 a2^2 g3^2 a l c3 + 12 a2 g3 d3 c3^3 - 6 a2 g3^2 d l c3$$

$$+ 6 d3 a1 c2 g3^2 - 6 d3 c3^2 i3 g3 - 2 d3 c3 c2 g3^2 - 3 a2 g3^3 c2 + 12 d3^2 c3^3 a1 + 2 d3 c3^3 p3 \\ + 2 g3^2 c3 s3 + 3 a1 s3 g3^2 + 2 d1 i3 g3^2 + j1 c3 g3^2 - j3 c3^3 g3) / g3^2$$

> **elimsolve (tmp1,i2);**

$$\{g3^3 \neq 0\}$$

i2 is set to:

$$- (-6 d2 g3^2 a1 c3 - 36 a2 g3^2 a1 d1 + 9 a2^2 g3^2 c3^2 + 81 a2^2 g3^2 a1^2 + 4 d1^2 g3^2 + 8 d3^2 c3^4 \\ - 2 d2 g3^2 c3^2 + 6 a1 g3^2 j1 - 18 d2 g3^2 a1^2 + c2 p3 g3^2 + i3^2 g3^2 - 9 a2 g3^2 a1 i3 \\ - 6 a2 g3^2 c3 i3 + 27 a2^2 g3^2 a1 c3 + 12 a2 g3 d3 c3^3 - 6 a2 g3^2 d1 c3 + 6 d3 a1 c2 g3^2 \\ - 6 d3 c3^2 i3 g3 - 2 d3 c3 c2 g3^2 - 3 a2 g3^3 c2 + 12 d3^2 c3^3 a1 + 2 d3 c3^3 p3 + 2 g3^2 c3 s3 \\ + 3 a1 s3 g3^2 + 2 d1 i3 g3^2 + j1 c3 g3^2 - j3 c3^3 g3) / g3^3$$

> **tmp1 := cpcoeff (x1\*x3^2\*T);**

$$tmp1 := - (12 c3^7 d3 + 3 c3^3 a1 c2 g3^2 + 4 c3^3 r3 g3^2 + 3 c2 g3^2 o3 c3^2 - 54 c2 g3^2 a1^3 c3 \\ + 15 c3^6 a2 g3 - 12 c3^5 i3 g3 - 7 c3^4 c2 g3^2 + 72 c3^6 d3 a1 + 6 q2 g3^4 + 5 c3^6 p3 \\ + 243 c3^3 a2 g3 a1^3 + 378 a1^3 c3^3 p3 - 81 a1^2 c3^2 a2 g3 o3 + 54 a1^3 c3^2 d3 o3 \\ + 18 a1 c3^2 r3 g3^2 - 162 a1^3 c3 a2 g3 o3 - 729 a1^4 c3^2 a2 g3 + 54 a1^2 c3^2 p3 o3 \\ + 54 a1^2 c3 r3 g3^2 - 9 a2 c3^4 g3 o3 + 81 c3^3 i3 g3 a1^2 - 27 a2 c3^3 g3 a1 o3 \\ - 90 d3 c3^3 a1^2 o3 - 21 c3^3 p3 a1 o3 - 4 d3 c3^5 o3 - 108 d3 c3^4 a1^3 - 162 c3^4 p3 a1^2 \\ - 5 c3^4 p3 o3 + 1296 a1^4 c3^3 d3 - 27 g3 c3 i3 a1^2 o3 - 48 d3 c3^4 a1 o3 - 162 a2 c3^4 g3 a1^2 \\ + 108 g3 c3 d1 a1^2 o3 - 8 g3 c3^5 d1 - 162 d3 c3^5 a1^2 + 12 g3 c3^3 d1 o3 - 351 g3 c3^2 i3 a1^3 \\ + 4 g3 c3^3 i3 o3 - 72 d1 g3 a1^2 c3^3 + 66 d1 g3 a1 c3^4 + 486 d1 g3 a1^4 c3 + 162 d1 g3 a1^3 o3 \\ - 6 d1 g3 a1 o3^2 - 4 d1 g3 o3^2 c3 + 216 d1 g3 a1^3 c3^2 + 54 d3 a1^2 c3 o3^2 + 2916 d3 a1^6 c3 \\ + 4 d3 c3^3 o3^2 + 18 d3 a1 c3^2 o3^2 - 3888 a1^5 d3 c3^2 - 729 a1^4 c3^2 p3 + 972 d3 a1^5 o3 \\ - 972 a1^4 d3 c3 o3 + 486 a1^4 i3 g3 c3 - 378 a1^3 c3 p3 o3 + 54 a1^3 r3 g3^2 - 243 a1^4 a2 g3 o3 \\ - 729 a1^5 a2 g3 c3 + 162 a1^3 i3 g3 o3 + 6 a2 g3 o3^2 c3^2 - 2 c2 o3^2 g3^2 + 12 r3 g3^2 a1 o3 \\ - 6 i3 g3 a1 o3^2 - 4 i3 g3 o3^2 c3 + 8 r3 g3^2 o3 c3 - 486 p3 a1^5 c3 - 162 p3 a1^4 o3 \\ - 27 p3 a1^2 o3^2 + 18 a2 g3 a1 o3^2 c3 + 54 a2 g3 a1^2 o3^2) / (2 g3^3)$$

> **elimsolve (tmp1,q2);**

$$\{6 g3^4 \neq 0\}$$

q2 is set to:

$$- (12 c3^7 d3 + 3 c3^3 a1 c2 g3^2 + 4 c3^3 r3 g3^2 + 3 c2 g3^2 o3 c3^2 - 54 c2 g3^2 a1^3 c3 \\ + 15 c3^6 a2 g3 - 12 c3^5 i3 g3 - 7 c3^4 c2 g3^2 + 72 c3^6 d3 a1 + 5 c3^6 p3 + 243 c3^3 a2 g3 a1^3 \\ + 378 a1^3 c3^3 p3 - 81 a1^2 c3^2 a2 g3 o3 + 54 a1^3 c3^2 d3 o3 + 18 a1 c3^2 r3 g3^2 \\ - 162 a1^3 c3 a2 g3 o3 - 729 a1^4 c3^2 a2 g3 + 54 a1^2 c3^2 p3 o3 + 54 a1^2 c3 r3 g3^2 \\ - 9 a2 c3^4 g3 o3 + 81 c3^3 i3 g3 a1^2 - 27 a2 c3^3 g3 a1 o3 - 90 d3 c3^3 a1^2 o3 - 21 c3^3 p3 a1 o3 \\ - 4 d3 c3^5 o3 - 108 d3 c3^4 a1^3 - 162 c3^4 p3 a1^2 - 5 c3^4 p3 o3 + 1296 a1^4 c3^3 d3 \\ - 27 g3 c3 i3 a1^2 o3 - 48 d3 c3^4 a1 o3 - 162 a2 c3^4 g3 a1^2 + 108 g3 c3 d1 a1^2 o3 \\ - 8 g3 c3^5 d1 - 162 d3 c3^5 a1^2 + 12 g3 c3^3 d1 o3 - 351 g3 c3^2 i3 a1^3 + 4 g3 c3^3 i3 o3$$

$$\begin{aligned}
& -72 d1 g3 a1^2 c3^3 + 66 d1 g3 a1 c3^4 + 486 d1 g3 a1^4 c3 + 162 d1 g3 a1^3 o3 - 6 d1 g3 a1 o3^2 \\
& -4 d1 g3 o3^2 c3 + 216 d1 g3 a1^3 c3^2 + 54 d3 a1^2 c3 o3^2 + 2916 d3 a1^6 c3 + 4 d3 c3^3 o3^2 \\
& + 18 d3 a1 c3^2 o3^2 - 3888 a1^5 d3 c3^2 - 729 a1^4 c3^2 p3 + 972 d3 a1^5 o3 - 972 a1^4 d3 c3 o3 \\
& + 486 a1^4 i3 g3 c3 - 378 a1^3 c3 p3 o3 + 54 a1^3 r3 g3^2 - 243 a1^4 a2 g3 o3 - 729 a1^5 a2 g3 c3 \\
& + 162 a1^3 i3 g3 o3 + 6 a2 g3 o3^2 c3^2 - 2 c2 o3^2 g3^2 + 12 r3 g3^2 a1 o3 - 6 i3 g3 a1 o3^2 \\
& -4 i3 g3 o3^2 c3 + 8 r3 g3^2 o3 c3 - 486 p3 a1^5 c3 - 162 p3 a1^4 o3 - 27 p3 a1^2 o3^2 \\
& + 18 a2 g3 a1 o3^2 c3 + 54 a2 g3 a1^2 o3^2) / (6 g3^4)
\end{aligned}$$

> **tmp1 := cpcoeff (x1\*x3\*T);**

$$\begin{aligned}
tmp1 := & -(4 d1 r3 g3^3 - j3 c3^5 g3 - 252 d3^2 c3^4 a1^2 + 972 d3^2 c3^2 a1^4 - 108 d3^2 c3^3 a1^3 \\
& -4 d3^2 c3^4 o3 - 16 d3 c3^5 p3 - 5 c3^4 p3^2 + 486 d3 a2 a1^4 g3 c3 - 144 d3 a2 a1 c3^4 g3 \\
& -30 d3 a1 i3 g3 o3 c3 + 2 d3 c3^2 i3 g3 o3 + 324 d3 a2 a1^3 c3^2 g3 - 36 d3 a1^2 d1 g3 o3 \\
& + 96 d3 a1 i3 g3 c3^3 - 108 d3 a1^3 i3 g3 c3 + 60 d3 a1 d1 g3 c3^3 - 6 d3 a2 c3^3 o3 g3 \\
& -48 d3 a1 d1 g3 o3 c3 - 36 d3 a1^2 i3 g3 o3 - 4 d3 d1 c3^2 g3 o3 - 18 d3 a1 c2 o3 g3^2 \\
& -108 d3 a1^3 d1 g3 c3 - 108 d3 a1^2 d1 g3 c3^2 + 36 d3 a1 c3^2 p3 o3 - 12 d3 a1 r3 g3^2 c3 \\
& + 108 d3 c3 p3 a1^2 o3 + 54 d3 a2 a1 c3^2 g3 o3 + g3^2 c3^3 j1 - 9 c3^2 i3^2 g3^2 - 84 a1 c3^5 d3^2 \\
& + 9 c3^4 a2^2 g3^2 + 12 c3^2 d1^2 g3^2 - 2 c3^4 d2 g3^2 + 729 a1^4 a2^2 g3^2 + 36 a1^2 d1^2 g3^2 \\
& + 54 a1^3 g3^2 j1 - 162 a1^4 d2 g3^2 + 9 a1^2 i3^2 g3^2 + 27 a1^3 s3 g3^2 + 4 i3 g3^3 r3 - 4 o3 d1^2 g3^2 \\
& - o3 i3^2 g3^2 - 6 a1 c3^3 p3^2 + 3 c3^2 p3^2 o3 + 27 c3^2 p3^2 a1^2 + 9 c2 g3^3 a2 a1 c3 \\
& -27 j3 c3 g3 a1^2 o3 - 9 j3 c3^2 g3 a1 o3 + 162 d3 a2 a1^2 c3 g3 o3 + 162 d3 a2 a1^3 g3 o3 \\
& + 42 d3 c2 g3^2 a1 c3^2 - 12 c2 g3^3 a1 d1 - 4 c2 g3^3 d1 c3 - 8 c2 g3^3 c3 i3 + 3 c2 g3^3 a2 c3^2 \\
& + 27 c2 g3^3 a2 a1^2 + 8 c2 g3^2 d3 c3^3 - 54 d2 g3^2 a1^3 c3 - 81 j3 c3^2 g3 a1^3 + 6 j3 c3^4 g3 a1 \\
& - j3 c3^3 g3 o3 + 12 d3^2 c3^3 a1 o3 + 108 d3^2 c3^2 a1^2 o3 + 324 d3^2 c3 a1^3 o3 + 4 d3 o3 c3^3 p3 \\
& + 18 d3 c3^4 i3 g3 - 6 d3 a2 c3^5 g3 + 324 d3 c3^2 p3 a1^3 - 36 d3 a1^2 r3 g3^2 - 54 d3 a1^2 c3^3 p3 \\
& -78 d3 a1 c3^4 p3 - 4 d3 r3 g3^2 c3^2 + 24 d1 g3 d3 c3^4 - 6 d1 g3^2 a2 c3^3 - 6 d1 g3^2 c3^2 i3 \\
& + 8 d1 g3 c3^3 p3 - 12 a1 c3^3 d2 g3^2 - 3 a1 c3 i3^2 g3^2 + 243 a1^2 c3^2 a2^2 g3^2 + 9 a1 c3^2 g3^2 s3 \\
& + 27 a1^2 c3 s3 g3^2 + 8 c3^2 c2 p3 g3^2 - 324 a1^3 a2 g3^2 d1 + 9 a1^2 c2 p3 g3^2 - 81 a1^3 a2 g3^2 i3 \\
& + 54 a1^3 d3 c2 g3^2 + 18 a1^2 d1 i3 g3^2 - 9 a1^2 j3 c3^3 g3 - 15 a2 c3^4 p3 g3 + 3 s3 g3^2 a1 o3 \\
& + 2 s3 g3^2 o3 c3 - 9 o3 a2^2 g3^2 c3^2 - 81 o3 a2^2 g3^2 a1^2 - 2 o3 c2 p3 g3^2 + 3 o3 a2 g3^3 c2 \\
& -2 o3 d1 i3 g3^2 + 2 r2 g3^4 - 2 c2^2 g3^4 + 2 c3^3 s3 g3^2 - 18 p3 a1 a2 c3^3 g3 \\
& + 27 p3 a2 g3 a1^2 o3 + 81 p3 a2 g3 a1^3 c3 + 3 p3 a2 g3 o3 c3^2 - 4 p3 d1 g3 o3 c3 \\
& -6 p3 d1 g3 a1 o3 - 6 p3 d1 g3 a1 c3^2 - 18 p3 d1 g3 a1^2 c3 + 12 p3 a1 c3^2 i3 g3 \\
& -4 p3 i3 g3 o3 c3 - 6 p3 i3 g3 a1 o3 - 18 p3 i3 g3 a1^2 c3 + 9 p3 a2 g3 a1 o3 c3 \\
& -27 a1^2 c3 a2 g3^2 i3 - 9 a1 c3^2 a2 g3^2 i3 - 90 a1 c3^2 a2 g3^2 d1 - 36 a1^2 c3 d3 c2 g3^2 \\
& -6 a1 c3 d1 i3 g3^2 + 36 o3 a2 g3^2 a1 d1 + 9 o3 a2 g3^2 a1 i3 + 6 o3 a2 g3^2 c3 i3 \\
& -27 o3 a2^2 g3^2 a1 c3 + 6 o3 a2 g3^2 d1 c3 + 9 c3 p3^2 a1 o3 - 6 p3 a1 r3 g3^2 - 4 p3 r3 g3^2 c3
\end{aligned}$$

$$+ 54 a l^2 c 3 a 2 g 3^2 d l + 6 i 3 a 2 c 3^3 g 3^2 + 16 g 3 i 3 c 3^3 p 3 + 18 j l g 3^2 a l c 3^2 - 3 j l g 3^2 a l o 3 \\ + j l g 3^2 o 3 c 3 - 54 a l^2 c 3^2 d 2 g 3^2 + 54 a l c 3^3 a 2^2 g 3^2 - 12 a l c 3 d l^2 g 3^2) / g 3^3$$

> **elimsolve (tmp1,r2) ;**

$$\{2 g 3^4 \neq 0\}$$

r2 is set to:

$$- (4 d l r 3 g 3^3 - j 3 c 3^5 g 3 - 252 d 3^2 c 3^4 a l^2 + 972 d 3^2 c 3^2 a l^4 - 108 d 3^2 c 3^3 a l^3 \\ - 4 d 3^2 c 3^4 o 3 - 16 d 3 c 3^5 p 3 - 5 c 3^4 p 3^2 + 486 d 3 a 2 a l^4 g 3 c 3 - 144 d 3 a 2 a l c 3^4 g 3 \\ - 30 d 3 a l i 3 g 3 o 3 c 3 + 2 d 3 c 3^2 i 3 g 3 o 3 + 324 d 3 a 2 a l^3 c 3^2 g 3 - 36 d 3 a l^2 d l g 3 o 3 \\ + 96 d 3 a l i 3 g 3 c 3^3 - 108 d 3 a l^3 i 3 g 3 c 3 + 60 d 3 a l d l g 3 c 3^3 - 6 d 3 a 2 c 3^3 o 3 g 3 \\ - 48 d 3 a l d l g 3 o 3 c 3 - 36 d 3 a l^2 i 3 g 3 o 3 - 4 d 3 d l c 3^2 g 3 o 3 - 18 d 3 a l c 2 o 3 g 3^2 \\ - 108 d 3 a l^3 d l g 3 c 3 - 108 d 3 a l^2 d l g 3 c 3^2 + 36 d 3 a l c 3^2 p 3 o 3 - 12 d 3 a l r 3 g 3^2 c 3 \\ + 108 d 3 c 3 p 3 a l^2 o 3 + 54 d 3 a 2 a l c 3^2 g 3 o 3 + g 3^2 c 3^3 j l - 9 c 3^2 i 3^2 g 3^2 - 84 a l c 3^5 d 3^2 \\ + 9 c 3^4 a 2^2 g 3^2 + 12 c 3^2 d l^2 g 3^2 - 2 c 3^4 d 2 g 3^2 + 729 a l^4 a 2^2 g 3^2 + 36 a l^2 d l^2 g 3^2 \\ + 54 a l^3 g 3^2 j l - 162 a l^4 d 2 g 3^2 + 9 a l^2 i 3^2 g 3^2 + 27 a l^3 s 3 g 3^2 + 4 i 3 g 3^3 r 3 - 4 o 3 d l^2 g 3^2 \\ - o 3 i 3^2 g 3^2 - 6 a l c 3^3 p 3^2 + 3 c 3^2 p 3^2 o 3 + 27 c 3^2 p 3^2 a l^2 + 9 c 2 g 3^3 a 2 a l c 3 \\ - 27 j 3 c 3 g 3 a l^2 o 3 - 9 j 3 c 3^2 g 3 a l o 3 + 162 d 3 a 2 a l^2 c 3 g 3 o 3 + 162 d 3 a 2 a l^3 g 3 o 3 \\ + 42 d 3 c 2 g 3^2 a l c 3^2 - 12 c 2 g 3^3 a l d l - 4 c 2 g 3^3 d l c 3 - 8 c 2 g 3^3 c 3 i 3 + 3 c 2 g 3^3 a 2 c 3^2 \\ + 27 c 2 g 3^3 a 2 a l^2 + 8 c 2 g 3^2 d 3 c 3^3 - 54 d 2 g 3^2 a l^3 c 3 - 81 j 3 c 3^2 g 3 a l^3 + 6 j 3 c 3^4 g 3 a l \\ - j 3 c 3^3 g 3 o 3 + 12 d 3^2 c 3^3 a l o 3 + 108 d 3^2 c 3^2 a l^2 o 3 + 324 d 3^2 c 3 a l^3 o 3 + 4 d 3 o 3 c 3^3 p 3 \\ + 18 d 3 c 3^4 i 3 g 3 - 6 d 3 a 2 c 3^5 g 3 + 324 d 3 c 3^2 p 3 a l^3 - 36 d 3 a l^2 r 3 g 3^2 - 54 d 3 a l^2 c 3^3 p 3 \\ - 78 d 3 a l c 3^4 p 3 - 4 d 3 r 3 g 3^2 c 3^2 + 24 d l g 3 d 3 c 3^4 - 6 d l g 3^2 a 2 c 3^3 - 6 d l g 3^2 c 3^2 i 3 \\ + 8 d l g 3 c 3^3 p 3 - 12 a l c 3^3 d 2 g 3^2 - 3 a l c 3 i 3^2 g 3^2 + 243 a l^2 c 3^2 a 2^2 g 3^2 + 9 a l c 3^2 g 3^2 s 3 \\ + 27 a l^2 c 3 s 3 g 3^2 + 8 c 3^2 c 2 p 3 g 3^2 - 324 a l^3 a 2 g 3^2 d l + 9 a l^2 c 2 p 3 g 3^2 - 81 a l^3 a 2 g 3^2 i 3 \\ + 54 a l^3 d 3 c 2 g 3^2 + 18 a l^2 d l i 3 g 3^2 - 9 a l^2 j 3 c 3^3 g 3 - 15 a 2 c 3^4 p 3 g 3 + 3 s 3 g 3^2 a l o 3 \\ + 2 s 3 g 3^2 o 3 c 3 - 9 o 3 a 2^2 g 3^2 c 3^2 - 81 o 3 a 2^2 g 3^2 a l^2 - 2 o 3 c 2 p 3 g 3^2 + 3 o 3 a 2 g 3^3 c 2 \\ - 2 o 3 d l i 3 g 3^2 - 2 c 2^2 g 3^4 + 2 c 3^3 s 3 g 3^2 - 18 p 3 a l a 2 c 3^3 g 3 + 27 p 3 a 2 g 3 a l^2 o 3 \\ + 81 p 3 a 2 g 3 a l^3 c 3 + 3 p 3 a 2 g 3 o 3 c 3^2 - 4 p 3 d l g 3 o 3 c 3 - 6 p 3 d l g 3 a l o 3 \\ - 6 p 3 d l g 3 a l c 3^2 - 18 p 3 d l g 3 a l^2 c 3 + 12 p 3 a l c 3^2 i 3 g 3 - 4 p 3 i 3 g 3 o 3 c 3 \\ - 6 p 3 i 3 g 3 a l o 3 - 18 p 3 i 3 g 3 a l^2 c 3 + 9 p 3 a 2 g 3 a l o 3 c 3 - 27 a l^2 c 3 a 2 g 3^2 i 3 \\ - 9 a l c 3^2 a 2 g 3^2 i 3 - 90 a l c 3^2 a 2 g 3^2 d l - 36 a l^2 c 3 d 3 c 2 g 3^2 - 6 a l c 3 d l i 3 g 3^2 \\ + 36 o 3 a 2 g 3^2 a l d l + 9 o 3 a 2 g 3^2 a l i 3 + 6 o 3 a 2 g 3^2 c 3 i 3 - 27 o 3 a 2^2 g 3^2 a l c 3 \\ + 6 o 3 a 2 g 3^2 d l c 3 + 9 c 3 p 3^2 a l o 3 - 6 p 3 a l r 3 g 3^2 - 4 p 3 r 3 g 3^2 c 3 + 54 a l^2 c 3 a 2 g 3^2 d l \\ + 6 i 3 a 2 c 3^3 g 3^2 + 16 g 3 i 3 c 3^3 p 3 + 18 j l g 3^2 a l c 3^2 - 3 j l g 3^2 a l o 3 + j l g 3^2 o 3 c 3 \\ - 54 a l^2 c 3^2 d 2 g 3^2 + 54 a l c 3^3 a 2^2 g 3^2 - 12 a l c 3 d l^2 g 3^2) / (2 g 3^4)$$

> **tmp1 := cpcoeff (x1\*T) ;**

$$tmp1 := (-s 2 g 3^4 + 9 p 3 a 2^2 g 3^2 c 3^2 + 81 p 3 a 2^2 g 3^2 a l^2 - 2 p 3 d 2 g 3^2 c 3^2 + 6 p 3 a l g 3^2 j l$$

$$\begin{aligned}
& -18 p3 d2 g3^2 a1^2 - 3 p3 a2 g3^3 c2 + 48 p3 d3^2 c3^3 a1 + 2 p3 g3^2 c3 s3 + 3 p3 a1 s3 g3^2 \\
& + 2 p3 d1 i3 g3^2 + p3 j1 c3 g3^2 - 2 p3 j3 c3^3 g3 - 6 j3 g3 d3 c3^4 - 3 j3 g3^3 a1 c2 \\
& - 3 j3 g3^2 a2 c3^3 + 3 j3 g3^2 c3^2 i3 + j3 g3^3 c3 c2 - 8 d3^2 c3^2 c2 g3^2 + 36 d3^2 a1^2 c2 g3^2 \\
& - 8 d3^2 c3^3 g3 d1 - 20 d3^2 c3^3 g3 i3 + 24 a2 g3 d3^2 c3^4 + 486 d3 a2^2 g3^2 a1^3 \\
& + 36 d3 a1^2 g3^2 j1 - 108 d3 d2 g3^2 a1^3 + 24 d3 a1 d1^2 g3^2 - 2 d3 j1 c3^2 g3^2 + 2 d3 i3 g3^3 c2 \\
& - 8 d3 d1^2 c3 g3^2 + 18 d3 a1^2 s3 g3^2 + 2 d3 s3 g3^2 c3^2 + 6 d3 i3^2 g3^2 a1 + 4 d3 i3^2 g3^2 c3 \\
& - 4 d3 d1 c2 g3^3 + 3 j2 g3^3 a1 c3 + 24 d2 g3^3 a1 d1 + 6 d2 g3^3 a1 i3 + 4 d2 g3^3 d1 c3 \\
& + 4 d2 g3^3 c3 i3 - 6 d2 g3^3 a2 c3^2 - 54 d2 g3^3 a2 a1^2 - 4 d2 g3^2 d3 c3^3 \\
& - 216 d3 a2 g3^2 a1^2 d1 + 6 d3 a1 s3 g3^2 c3 - 6 d3 a1 c3 g3^2 j1 + 12 d3 i3 g3^2 a1 d1 \\
& - 4 d3 i3 g3^2 d1 c3 - 18 d3 a2 i3 g3^2 a1 c3 - 6 d3 a2 g3^2 c3^2 i3 - 54 d3 a2 i3 g3^2 a1^2 \\
& + 36 d3 a2 g3^2 c3 a1 d1 + 12 d3 a2 g3^2 c3^2 d1 - 18 d2 g3^3 a2 a1 c3 - 18 j3 g3 d3 c3^3 a1 \\
& - 72 d3^2 a1 c3^2 i3 g3 + 144 a2 g3 d3^2 c3^3 a1 - 36 p3 a2 g3^2 a1 d1 - 9 p3 a2 g3^2 a1 i3 \\
& - 6 p3 a2 g3^2 c3 i3 + 27 p3 a2^2 g3^2 a1 c3 + 18 p3 a2 g3 d3 c3^3 - 6 p3 a2 g3^2 d1 c3 \\
& + 12 p3 d3 a1 c2 g3^2 - 12 p3 d3 c3^2 i3 g3 - 4 p3 d3 c3 c2 g3^2 + 16 d3^3 c3^5 \\
& - 6 p3 d2 g3^2 a1 c3 - 24 d3^2 c2 g3^2 a1 c3 - j1 i3 g3^3 - 2 d1 s3 g3^3 + c2 p3^2 g3^2 + 4 d3 c3^3 p3^2 \\
& + 4 p3 d1^2 g3^2 + 20 p3 d3^2 c3^4 + p3 i3^2 g3^2 - 2 i3 g3^3 s3 - 4 d1 g3^3 j1 + 144 d3^3 c3^3 a1^2 \\
& + 120 a1 d3^3 c3^4 + j2 g3^3 c3^2 + 9 j2 g3^3 a1^2 + 2 d2 g3^4 c2) / g3^3
\end{aligned}$$

> **elimsolve (tmp1,s2) ;**

$$\{-g3^4 \neq 0\}$$

s2 is set to:

$$\begin{aligned}
& (9 p3 a2^2 g3^2 c3^2 + 81 p3 a2^2 g3^2 a1^2 - 2 p3 d2 g3^2 c3^2 + 6 p3 a1 g3^2 j1 - 18 p3 d2 g3^2 a1^2 \\
& - 3 p3 a2 g3^3 c2 + 48 p3 d3^2 c3^3 a1 + 2 p3 g3^2 c3 s3 + 3 p3 a1 s3 g3^2 + 2 p3 d1 i3 g3^2 \\
& + p3 j1 c3 g3^2 - 2 p3 j3 c3^3 g3 - 6 j3 g3 d3 c3^4 - 3 j3 g3^3 a1 c2 - 3 j3 g3^2 a2 c3^3 \\
& + 3 j3 g3^2 c3^2 i3 + j3 g3^3 c3 c2 - 8 d3^2 c3^2 c2 g3^2 + 36 d3^2 a1^2 c2 g3^2 - 8 d3^2 c3^3 g3 d1 \\
& - 20 d3^2 c3^3 g3 i3 + 24 a2 g3 d3^2 c3^4 + 486 d3 a2^2 g3^2 a1^3 + 36 d3 a1^2 g3^2 j1 \\
& - 108 d3 d2 g3^2 a1^3 + 24 d3 a1 d1^2 g3^2 - 2 d3 j1 c3^2 g3^2 + 2 d3 i3 g3^3 c2 - 8 d3 d1^2 c3 g3^2 \\
& + 18 d3 a1^2 s3 g3^2 + 2 d3 s3 g3^2 c3^2 + 6 d3 i3^2 g3^2 a1 + 4 d3 i3^2 g3^2 c3 - 4 d3 d1 c2 g3^3 \\
& + 3 j2 g3^3 a1 c3 + 24 d2 g3^3 a1 d1 + 6 d2 g3^3 a1 i3 + 4 d2 g3^3 d1 c3 + 4 d2 g3^3 c3 i3 \\
& - 6 d2 g3^3 a2 c3^2 - 54 d2 g3^3 a2 a1^2 - 4 d2 g3^2 d3 c3^3 - 216 d3 a2 g3^2 a1^2 d1 \\
& + 6 d3 a1 s3 g3^2 c3 - 6 d3 a1 c3 g3^2 j1 + 12 d3 i3 g3^2 a1 d1 - 4 d3 i3 g3^2 d1 c3 \\
& - 18 d3 a2 i3 g3^2 a1 c3 - 6 d3 a2 g3^2 c3^2 i3 - 54 d3 a2 i3 g3^2 a1^2 + 36 d3 a2 g3^2 c3 a1 d1 \\
& + 12 d3 a2 g3^2 c3^2 d1 - 18 d2 g3^3 a2 a1 c3 - 18 j3 g3 d3 c3^3 a1 - 72 d3^2 a1 c3^2 i3 g3 \\
& + 144 a2 g3 d3^2 c3^3 a1 - 36 p3 a2 g3^2 a1 d1 - 9 p3 a2 g3^2 a1 i3 - 6 p3 a2 g3^2 c3 i3 \\
& + 27 p3 a2^2 g3^2 a1 c3 + 18 p3 a2 g3 d3 c3^3 - 6 p3 a2 g3^2 d1 c3 + 12 p3 d3 a1 c2 g3^2 \\
& - 12 p3 d3 c3^2 i3 g3 - 4 p3 d3 c3 c2 g3^2 + 16 d3^3 c3^5 - 6 p3 d2 g3^2 a1 c3 \\
& - 24 d3^2 c2 g3^2 a1 c3 - j1 i3 g3^3 - 2 d1 s3 g3^3 + c2 p3^2 g3^2 + 4 d3 c3^3 p3^2 + 4 p3 d1^2 g3^2
\end{aligned}$$

$$+ 20 p3 d3^2 c3^4 + p3 i3^2 g3^2 - 2 i3 g3^3 s3 - 4 d1 g3^3 j1 + 144 d3^3 c3^3 al^2 + 120 al d3^3 c3^4 + j2 g3^3 c3^2 + 9 j2 g3^3 al^2 + 2 d2 g3^4 c2) / g3^4$$

> **tmp1 := cpcoeff (x1\*x3^3\*T);**

$$tmp1 := -(-1053 al^5 c3^3 + 162 al^4 c3^4 - 36 c3^3 al^3 o3 + 12 c3^3 al o3^2 + 999 al^4 c3^2 o3 - 9 al^2 c3^4 o3 + 18 al c3^5 o3 + 99 al^2 c3^2 o3^2 + 216 c3 al^3 o3^2 + 3483 c3 al^5 o3 + 6 al o3^3 c3 + 8 w2 g3^4 + 99 c3^6 al^2 + 2 c3^4 o3^2 + 162 c3^5 al^3 + 2 c3^6 o3 + 7776 al^6 c3^2 + 1458 al^7 c3 + 486 al^6 o3 + 243 al^4 o3^2 - 9 al^2 o3^3 + 2 o3^3 c3^2) / (2 g3^3)$$

> **elimsolve (tmp1,w2);**

$$\{8 g3^4 \neq 0\}$$

w2 is set to:

$$-(-1053 al^5 c3^3 + 162 al^4 c3^4 - 36 c3^3 al^3 o3 + 12 c3^3 al o3^2 + 999 al^4 c3^2 o3 - 9 al^2 c3^4 o3 + 18 al c3^5 o3 + 99 al^2 c3^2 o3^2 + 216 c3 al^3 o3^2 + 3483 c3 al^5 o3 + 6 al o3^3 c3 + 99 c3^6 al^2 + 2 c3^4 o3^2 + 162 c3^5 al^3 + 2 c3^6 o3 + 7776 al^6 c3^2 + 1458 al^7 c3 + 486 al^6 o3 + 243 al^4 o3^2 - 9 al^2 o3^3 + 2 o3^3 c3^2) / (8 g3^4)$$

> **tmp1 := cpcoeff (x1\*x2\*T);**

$$tmp1 := (2 r3 g3^2 - 18 i3 g3 al c3 + 6 d3 al o3 c3 + 108 a2 al^2 c3 g3 - 30 al d1 c3 g3 + 36 al a2 c3^2 g3 - 18 i3 g3 al^2 - 2 i3 g3 o3 + 9 p3 al^2 c3 + 3 p3 al c3^2 + 3 p3 al o3 + 2 p3 o3 c3 + 2 d3 o3 c3^2 + 54 d3 al^3 c3 + 18 d3 al^2 o3 - 54 al^2 d1 g3 + 162 a2 al^3 g3 - 2 d1 c3^2 g3 - 2 d1 o3 g3 + 4 d3 c3^4 - 6 al c2 g3^2 + 6 a2 c3^3 g3 - 4 c3^2 i3 g3 - 2 c3 c2 g3^2 + 12 d3 c3^3 al) / g3$$

> **elimsolve (tmp1,r3);**

$$\{2 g3^2 \neq 0\}$$

r3 is set to:

$$-(-18 i3 g3 al c3 + 6 d3 al o3 c3 + 108 a2 al^2 c3 g3 - 30 al d1 c3 g3 + 36 al a2 c3^2 g3 - 18 i3 g3 al^2 - 2 i3 g3 o3 + 9 p3 al^2 c3 + 3 p3 al c3^2 + 3 p3 al o3 + 2 p3 o3 c3 + 2 d3 o3 c3^2 + 54 d3 al^3 c3 + 18 d3 al^2 o3 - 54 al^2 d1 g3 + 162 a2 al^3 g3 - 2 d1 c3^2 g3 - 2 d1 o3 g3 + 4 d3 c3^4 - 6 al c2 g3^2 + 6 a2 c3^3 g3 - 4 c3^2 i3 g3 - 2 c3 c2 g3^2 + 12 d3 c3^3 al) / (2 g3^2)$$

> **launchNZcase (a1);**

Launching case level 2:

$$al \neq 0$$

Assume from now on that:

$$6 g3 al \neq 0$$

> **launchNZcase (c3);**

Launching case level 3:

$$c3 \neq 0$$

Assume from now on that:

$$6 g3 al c3 \neq 0$$

> **tmp1 := cpcoeff (x2^3);**

$$tmp1 := -27 (-o3 + 3 al c3 + c3^2 + 9 al^2) al^3 c3$$

```
> elimsolve (tmp1,o3);
```

$$\{-1 \neq 0\}$$

o3 is set to:

$$3 \, a1 \, c3 + c3^2 + 9 \, a1^2$$

```
> tmp1 := cpcoeff (x2^2*T);
```

$$tmp1 := 27 \, a1^3 \, c3$$

```
> contradict (tmp1,'c3');
```

Contradiction on case level 3, so:

$$c3 = 0$$

Variables to be uneliminated:

$$"o3 := 'o3'"$$

Proceed on case level 2 with:

$$6 \, g3 \, a1 \neq 0$$

On account of:

$$c3 = 0$$

$$\{1 \neq 0\}$$

c3 is set to:

$$0$$

```
> tmp1 := cpcoeff (x1^3*x2*x3);
```

$$tmp1 := -\frac{162 \, a1^4 \, o3}{g3}$$

```
> elimsolve (tmp1,o3);
```

$$\{1 \neq 0\}$$

o3 is set to:

$$0$$

```
> tmp1 := cpcoeff (x2^2*T);
```

$$tmp1 := -81 \, a1^4$$

```
> contradict (tmp1,'a1');
```

Contradiction on case level 2, so:

$$a1 = 0$$

Variables to be uneliminated:

$$"o3 := 'o3'"$$

$$"c3 := 'c3'"$$

Proceed on case level 1 with:

$$6 \, g3 \neq 0$$

On account of:

$$a1 = 0$$

$$\{1 \neq 0\}$$

a1 is set to:

$$0$$

```
> tmp1 := cpcoeff (x2^2*T);
```

$$tmp1 := -(-o3 + c3^2)^2$$

```
> elimsolve (tmp1,o3);
```

$$\{-1 \neq 0\}$$

o3 is set to:

$$c3^2$$

> **launchNZcase (c3);**

Launching case level 2:

$$c3 \neq 0$$

Assume from now on that:

$$6 g3 c3 \neq 0$$

> **tmp1 := cpcoeff (x2\*x3^2);**

$$tmp1 := \frac{c3^4 (2 d1 c3 g3 + c2 g3^2 - 2 d3 c3^3 - 3 a2 c3^2 g3 + 2 c3 i3 g3 - p3 c3^2)^2}{g3^4}$$

> **elimsolve (tmp1,p3);**

$$\{-c3^2 \neq 0\}$$

p3 is set to:

$$\frac{2 d1 c3 g3 + 2 c3 i3 g3 - 3 a2 c3^2 g3 - 2 d3 c3^3 + c2 g3^2}{c3^2}$$

> **tmp1 := cpcoeff (x1^3);**

$$tmp1 := -\frac{8 (d1 g3 + d3 c3^2)^3}{g3^3}$$

> **elimsolve (tmp1,d1);**

$$\{g3 \neq 0\}$$

d1 is set to:

$$-\frac{d3 c3^2}{g3}$$

> **launchNZcase (g3\*j1+j3\*c3^2);**

Launching case level 3:

$$g3 j1 + j3 c3^2 \neq 0$$

Assume from now on that:

$$6 g3 c3 (g3 j1 + j3 c3^2) \neq 0$$

> **launchNZcase (-j3\*c3^5\*g3+s3\*g3^2\*c3^3+2\*g3^2\*c3^2\*i3^2 +**  
> **3\*g3^3\*c3\*i3\*c2-9\*g3^2\*c3^3\*i3\*a2-8\*d3\*i3\*g3\*c3^4 +**  
> **9\*c3^4\*a2^2\*g3^2+8\*c3^6\*d3^2+c2^2\*g3^4-6\*c2\*g3^3\*a2\*c3^2 +**  
> **18\*c3^5\*a2\*g3\*d3-6\*d3\*c2\*g3^2\*c3^3);**

Launching case level 4:

$$-j3 c3^5 g3 + c3^3 s3 g3^2 + 2 c3^2 i3^2 g3^2 + 3 c2 g3^3 c3 i3 - 9 i3 a2 c3^3 g3^2 - 8 d3 c3^4 i3 g3 \\ + 9 c3^4 a2^2 g3^2 + 8 d3^2 c3^6 + c2^2 g3^4 - 6 c2 g3^3 a2 c3^2 + 18 d3 a2 c3^5 g3 - 6 c2 g3^2 d3 c3^3 \neq 0$$

Assume from now on that:

$$6 g3 c3 (g3 j1 + j3 c3^2) (-j3 c3^5 g3 + c3^3 s3 g3^2 + 2 c3^2 i3^2 g3^2 + 3 c2 g3^3 c3 i3 \\ - 9 i3 a2 c3^3 g3^2 - 8 d3 c3^4 i3 g3 + 9 c3^4 a2^2 g3^2 + 8 d3^2 c3^6 + c2^2 g3^4 - 6 c2 g3^3 a2 c3^2 \\ + 18 d3 a2 c3^5 g3 - 6 c2 g3^2 d3 c3^3) \neq 0$$

> **tmp1 := cpcoeff (1);**

$$tmp1 := (-j3 c3^5 g3 + c3^3 s3 g3^2 + 2 c3^2 i3^2 g3^2 + 3 c2 g3^3 c3 i3 - 9 i3 a2 c3^3 g3^2 \\ - 8 d3 c3^4 i3 g3 + 9 c3^4 a2^2 g3^2 + 8 d3^2 c3^6 + c2^2 g3^4 - 6 c2 g3^3 a2 c3^2 + 18 d3 a2 c3^5 g3$$

$$\begin{aligned} & -6 c2 g3^2 d3 c3^3)(g3 j1 + j3 c3^2)(g3^2 c3^3 j1 + 9 c3^4 a2^2 g3^2 + 18 d3 a2 c3^5 g3 \\ & -9 i3 a2 c3^3 g3^2 - 6 c2 g3^3 a2 c3^2 + 8 d3^2 c3^6 - 8 d3 c3^4 i3 g3 - 6 c2 g3^2 d3 c3^3 + c3^3 s3 g3^2 \\ & + 2 c3^2 i3^2 g3^2 + 3 c2 g3^3 c3 i3 + c2^2 g3^4) / (c3^6 g3^5) \end{aligned}$$

> **elimsolve (tmp1,j1);**

$$\{c3^3 g3^2 \neq 0\}$$

j1 is set to:

$$\begin{aligned} & -(9 c3^4 a2^2 g3^2 + 18 d3 a2 c3^5 g3 - 9 i3 a2 c3^3 g3^2 - 6 c2 g3^3 a2 c3^2 + 8 d3^2 c3^6 \\ & - 8 d3 c3^4 i3 g3 - 6 c2 g3^2 d3 c3^3 + c3^3 s3 g3^2 + 2 c3^2 i3^2 g3^2 + 3 c2 g3^3 c3 i3 + c2^2 g3^4) / ( \\ & c3^3 g3^2) \end{aligned}$$

Nonzero constraint refines to:

$$\begin{aligned} & 6 g3 c3 (-9 c3^4 a2^2 g3^2 - 18 d3 a2 c3^5 g3 + 9 i3 a2 c3^3 g3^2 + 6 c2 g3^3 a2 c3^2 - 8 d3^2 c3^6 \\ & + 8 d3 c3^4 i3 g3 + 6 c2 g3^2 d3 c3^3 - c3^3 s3 g3^2 - 2 c3^2 i3^2 g3^2 - 3 c2 g3^3 c3 i3 - c2^2 g3^4 \\ & + j3 c3^5 g3)(-j3 c3^5 g3 + c3^3 s3 g3^2 + 2 c3^2 i3^2 g3^2 + 3 c2 g3^3 c3 i3 - 9 i3 a2 c3^3 g3^2 \\ & - 8 d3 c3^4 i3 g3 + 9 c3^4 a2^2 g3^2 + 8 d3^2 c3^6 + c2^2 g3^4 - 6 c2 g3^3 a2 c3^2 + 18 d3 a2 c3^5 g3 \\ & - 6 c2 g3^2 d3 c3^3) \neq 0 \end{aligned}$$

> **tmp1 := cpcoeff (T);**

$$\begin{aligned} tmp1 := & -(-j3 c3^5 g3 + c3^3 s3 g3^2 + 2 c3^2 i3^2 g3^2 + 3 c2 g3^3 c3 i3 - 9 i3 a2 c3^3 g3^2 \\ & - 8 d3 c3^4 i3 g3 + 9 c3^4 a2^2 g3^2 + 8 d3^2 c3^6 + c2^2 g3^4 - 6 c2 g3^3 a2 c3^2 + 18 d3 a2 c3^5 g3 \\ & - 6 c2 g3^2 d3 c3^3)^2 / (c3^6 g3^4) \end{aligned}$$

> **contradict (tmp1,'j3');**

Contradiction on case level 4, so:

$$\begin{aligned} & -j3 c3^5 g3 + c3^3 s3 g3^2 + 2 c3^2 i3^2 g3^2 + 3 c2 g3^3 c3 i3 - 9 i3 a2 c3^3 g3^2 - 8 d3 c3^4 i3 g3 \\ & + 9 c3^4 a2^2 g3^2 + 8 d3^2 c3^6 + c2^2 g3^4 - 6 c2 g3^3 a2 c3^2 + 18 d3 a2 c3^5 g3 - 6 c2 g3^2 d3 c3^3 = 0 \end{aligned}$$

Variables to be uneliminated:

$$"j1 := 'j1'"$$

Proceed on case level 3 with:

$$6 g3 c3 (g3 j1 + j3 c3^2) \neq 0$$

On account of:

$$\begin{aligned} & -j3 c3^5 g3 + c3^3 s3 g3^2 + 2 c3^2 i3^2 g3^2 + 3 c2 g3^3 c3 i3 - 9 i3 a2 c3^3 g3^2 - 8 d3 c3^4 i3 g3 \\ & + 9 c3^4 a2^2 g3^2 + 8 d3^2 c3^6 + c2^2 g3^4 - 6 c2 g3^3 a2 c3^2 + 18 d3 a2 c3^5 g3 - 6 c2 g3^2 d3 c3^3 = 0 \\ & \{-c3^5 g3 \neq 0\} \end{aligned}$$

j3 is set to:

$$\begin{aligned} & (9 c3^4 a2^2 g3^2 + 18 d3 a2 c3^5 g3 - 9 i3 a2 c3^3 g3^2 - 6 c2 g3^3 a2 c3^2 + 8 d3^2 c3^6 \\ & - 8 d3 c3^4 i3 g3 - 6 c2 g3^2 d3 c3^3 + c3^3 s3 g3^2 + 2 c3^2 i3^2 g3^2 + 3 c2 g3^3 c3 i3 + c2^2 g3^4) / ( \\ & c3^5 g3) \end{aligned}$$

Nonzero constraint refines to:

$$\begin{aligned} & 6 g3 c3 (g3^2 c3^3 j1 + 9 c3^4 a2^2 g3^2 + 18 d3 a2 c3^5 g3 - 9 i3 a2 c3^3 g3^2 - 6 c2 g3^3 a2 c3^2 \\ & + 8 d3^2 c3^6 - 8 d3 c3^4 i3 g3 - 6 c2 g3^2 d3 c3^3 + c3^3 s3 g3^2 + 2 c3^2 i3^2 g3^2 + 3 c2 g3^3 c3 i3 \\ & + c2^2 g3^4) \neq 0 \end{aligned}$$

> **tmp1 := cpcoeff (T) ;**

$$\text{tmp1} := -(g^3 c^3 j_1 + 9 c^4 a^2 g^3 + 18 d_3 a_2 c^5 g^3 - 9 i_3 a_2 c^3 g^3 - 6 c_2 g^3 a_2 c^3 + 8 d_3^2 c^6 - 8 d_3 c^4 i_3 g^3 - 6 c_2 g^3 d_3 c^3 + c^3 s_3 g^3 + 2 c^3 i_3^2 g^3 + 3 c_2 g^3 c_3 i_3 + c^2 g^4)^2 / (c^6 g^4)$$

> **contradict (tmp1, 'j1') ;**

Contradiction on case level 3, so:

$$g^3 j_1 + j_3 c^3 = 0$$

Variables to be uneliminated:

$$j_3 := 'j_3'$$

Proceed on case level 2 with:

$$6 g^3 c^3 \neq 0$$

On account of:

$$g^3 j_1 + j_3 c^3 = 0$$

$$\{g^3 \neq 0\}$$

j1 is set to:

$$-\frac{j_3 c^3}{g^3}$$

> **tmp1 := cpcoeff (T) ;**

$$\text{tmp1} := -(-j_3 c^5 g^3 + c^3 s_3 g^3 + 2 c^3 i_3^2 g^3 + 3 c_2 g^3 c_3 i_3 - 9 i_3 a_2 c^3 g^3 - 8 d_3 c^4 i_3 g^3 + 9 c^4 a^2 g^3 + 8 d_3^2 c^6 + c^2 g^4 - 6 c_2 g^3 a_2 c^3 + 18 d_3 a_2 c^5 g^3 - 6 c_2 g^3 d_3 c^3)^2 / (c^6 g^4)$$

> **elimsolve (tmp1, j3) ;**

$$\{-c^5 g^3 \neq 0\}$$

j3 is set to:

$$(9 c^4 a^2 g^3 + 18 d_3 a_2 c^5 g^3 - 9 i_3 a_2 c^3 g^3 - 6 c_2 g^3 a_2 c^3 + 8 d_3^2 c^6 - 8 d_3 c^4 i_3 g^3 - 6 c_2 g^3 d_3 c^3 + c^3 s_3 g^3 + 2 c^3 i_3^2 g^3 + 3 c_2 g^3 c_3 i_3 + c^2 g^4) / (c^5 g^3)$$

> **det (T-jacobian (H, [x1, x2, x3])) ;**

$$T^3$$

> **simplify (evalm ([H[1], H[2], H[3]])) ;**

$$\begin{aligned} & [-(3 g^4 x_1 c_2 c_3 i_3 + g^5 x_1 c^2 - c^9 x^2 d_3 + 18 g^3 x_1 d_3 a_2 c^5 - 9 g^3 x_1 i_3 a_2 c^3 \\ & - 6 g^4 x_1 c_2 a_2 c^3 - 8 g^3 x_1 d_3 c^4 i_3 - 6 g^3 x_1 c_2 d_3 c^3 + c^{10} x^3 + c^5 s_3 g^3 x^3 \\ & + 9 g^3 x_1 c^4 a^2 + 8 g^3 x_1 d_3^2 c^6 + g^3 x_1 c^3 s_3 + 2 g^3 x_1 c^3 i_3^2 + d_3 c^5 x_1^2 g^3 \\ & + 2 c^8 x_1 x^2 g^3 + c^6 x_1^2 x_3 g^3 + c^5 i_3 g^3 x_1 x_3 + c^7 x_2 x_3 g^3 + c^5 x_1 x_2 g^3 \\ & - 4 x_2 g^3 c^6 d_3 + 2 x_2 g^3 c^4 i_3 - 3 x_2 g^3 c^5 a_2 + x_2 g^4 c^3 c_2 + c^7 x^2 i_3 g^3) / (g^3 c^3), \\ & (-48 x_3 d_3 c^6 i_3 g^3 x_1 + 12 x^2 c^6 i_3^2 g^3 - 8 x_3 c^3 i_3^3 g^3 + 96 x_3 c_2 g^4 c^3 i_3 a_2 \\ & - 16 x_3 c^2 g^5 c_3 i_3 + 4 j_2 g^3 c^6 x_3 - 192 x_3 c_2 g^3 d_3 c^5 a_2 + 80 x_3 c_2 g^3 d_3 c^4 i_3 \\ & + 32 x_3 c^2 g^4 d_3 c^3 - 24 c_2 x_1 x_3 c^4 g^4 a_2 + 4 d_2 x_1^2 c^4 g^4 - 3 c^{12} x^4 \\ & + 4 j_2 g^4 c^4 x_1 - 48 x_3 i_3 a_2 c^5 g^3 x_1 + 288 x_3 d_3 a_2 c^7 g^3 + 96 x_3 d_3 a_2 c^7 g^3 x_1 \end{aligned}$$

$$\begin{aligned}
& + 108 x3 c3^6 a2^3 g3^3 + 4 x3^2 c3^8 d2 g3^2 - 240 x3 d3 c3^6 i3 g3^2 a2 + 64 x3 d3^3 c3^9 \\
& + 48 x3^2 d3^2 c3^{10} - 4 x3 c2^3 g3^6 + x1^4 c3^4 g3^4 + 4 x1^3 c3^4 g3^4 a2 + 4 c3^8 x3^3 c2 g3^2 \\
& - 8 c3^{10} x3^3 a2 g3 - 8 c3^{10} x1 x3^3 g3 - 6 c3^8 x1^2 x3^2 g3^2 - 4 c3^5 x1^2 x2 g3^4 - 4 c3^9 x2 x3^2 g3^2 \\
& + 16 c2 x1 x3 c3^3 g3^4 i3 - 32 c2 x1 x3 c3^5 g3^3 d3 + 8 c3^3 x2 g3^4 i3^2 + 32 c3^7 x2 g3^2 d3^2 \\
& + 36 c3^8 g3^2 x3^2 a2^2 + 4 c3^4 g3^4 x3^2 c2^2 + 8 c3^6 x1 x3^2 g3^3 c2 - 12 c3^8 x1 x3^2 g3^2 a2 \\
& + 4 c2 x1^2 x3 c3^4 g3^4 - 4 c3^4 x1 x2 g3^4 i3 + 8 c3^6 x1 x2 g3^3 d3 - 8 c3^7 x1 x2 g3^3 x3 \\
& + 8 d2 x1 c3^6 g3^3 x3 + 4 c2^2 x1 x3 c3^2 g3^5 - 4 c3^6 x2 x3 g3^3 i3 + 8 c3^8 x2 x3 g3^2 d3 \\
& - 24 c3^4 x2 g3^4 d3 c2 - 32 c3^5 x2 g3^3 d3 i3 + 72 c3^6 x2 g3^3 d3 a2 - 48 c3^7 g3^2 x3^2 a2 i3 \\
& + 96 c3^9 g3 x3^2 a2 d3 + 12 c3^2 x2 g3^5 i3 c2 - 36 c3^4 x2 g3^4 i3 a2 - 24 c3^6 g3^3 x3^2 a2 c2 \\
& + 16 c3^5 g3^3 x3^2 c2 i3 - 32 c3^7 g3^2 x3^2 c2 d3 - 20 x3 c2 g3^4 c3^2 i3^2 - 80 x3 c2 g3^2 d3^2 c3^6 \\
& + 36 x3 c2^2 g3^5 a2 c3^2 - 108 x3 c2 g3^4 a2^2 c3^4 + 48 x3 d3^2 c3^8 x1 g3 - 24 x2 c3^3 g3^5 c2 a2 \\
& + 36 x2 c3^5 g3^4 a2^2 + 4 x2 c3 g3^6 c2^2 - 96 x3 d3^2 c3^7 i3 g3 + 240 x3 d3^2 c3^8 a2 g3 \\
& - 144 x3 c3^5 a2^2 g3^3 i3 + 48 x3 d3 c3^5 i3^2 g3^2 - 48 x3^2 d3 c3^8 i3 g3 + 36 x3 c3^6 a2^2 g3^3 x1 \\
& + 60 x3 c3^4 i3^2 g3^3 a2 + 12 x3 c3^4 i3^2 g3^3 x1) / (4 c3^4 g3^4), (3 g3^4 x1 c2 c3 i3 + g3^5 x1 c2^2 \\
& - c3^9 x3^2 d3 + 18 g3^2 x1 d3 a2 c3^5 - 9 g3^3 x1 i3 a2 c3^3 - 6 g3^4 x1 c2 a2 c3^2 \\
& - 8 g3^2 x1 d3 c3^4 i3 - 6 g3^3 x1 c2 d3 c3^3 + c3^{10} x3^3 + c3^5 s3 g3^2 x3 + 9 g3^3 x1 c3^4 a2^2 \\
& + 8 g3 x1 d3^2 c3^6 + g3^3 x1 c3^3 s3 + 2 g3^3 x1 c3^2 i3^2 + d3 c3^5 x1^2 g3^2 + 2 c3^8 x1 x3^2 g3 \\
& + c3^6 x1^2 x3 g3^2 + c3^5 i3 g3^2 x1 x3 + c3^7 x2 x3 g3^2 + c3^5 x1 x2 g3^3 - 4 x2 g3^2 c3^6 d3 \\
& + 2 x2 g3^3 c3^4 i3 - 3 x2 g3^3 c3^5 a2 + x2 g3^4 c3^3 c2 + c3^7 x3^2 i3 g3) / (g3^2 c3^5)]
\end{aligned}$$

> factor(g3\*H[1]+c3^2\*H[3]);

0

> M := evalm ([ [C,0,C/g3\*c3^2], [1,0,0],  
> [-C\*(-2\*c2\*g3^2-3\*c3\*i3\*g3+6\*a2\*c3^2\*g3+  
> 6\*d3\*c3^3)/g3/c3^2, C\*c3, 0] ] );

$$M := \begin{bmatrix} C & 0 & \frac{C c3^2}{g3} \\ 1 & 0 & 0 \\ -\frac{C(-2 c2 g3^2 - 3 c3 i3 g3 + 6 a2 c3^2 g3 + 6 d3 c3^3)}{g3 c3^2} & C c3 & 0 \end{bmatrix}$$

> det (M);

$$\frac{C^2 c3^3}{g3}$$

> G := simplify(evalm(M&\*subs({seq([x1,x2,x3][i]=  
> evalm(M^(-1)&\*[x1,x2,x3])[i],i=1..n)},H)));

$$\begin{aligned}
G := & [0, -(g3^2 c3^3 C i3 x1^2 - g3 c3^5 C d3 x1^2 + c3^3 s3 g3^2 C^2 x1 - c3^4 x2 g3^2 C x1^2 \\
& - 4 c3^3 i3 g3^2 x2 C^2 x1 - 9 x2 C^3 c3^4 a2^2 g3^2 - 24 x2 C^3 d3 a2 c3^5 g3 + 12 x2 C^3 i3 a2 c3^3 g3^2 \\
& + 6 x2 C^3 c2 g3^3 a2 c3^2 + 16 x2 C^3 d3 c3^4 i3 g3 + 8 x2 C^3 c2 g3^2 d3 c3^3 - 4 x2 C^3 c3^2 i3^2 g3^2
\end{aligned}$$

$$\begin{aligned}
& -4 x_2 C^3 c_2 g_3^3 c_3 i_3 - 2 g_3^3 C^2 c_3^2 x_2 c_2 x_1 + 6 g_3^2 C^2 c_3^4 x_2 a_2 x_1 + 8 g_3 C^2 c_3^5 x_2 d_3 x_1 \\
& + g_3^2 C c_3^4 x_1 x_3 - 4 C^2 d_3 c_3^5 x_3 g_3 + 2 C^2 c_3^3 i_3 g_3^2 x_3 - 3 C^2 a_2 c_3^4 g_3^2 x_3 \\
& + C^2 c_2 g_3^3 x_3 c_3^2 + c_3^4 g_3^2 x_1^3 - 16 x_2 C^3 d_3^2 c_3^6 - x_2 C^3 c_2^2 g_3^4) / (g_3^2 c_3^3 C^3), - ( \\
& 8 c_2 g_3^4 c_3^3 s_3 C^3 x_1 + 8 C^3 c_3^3 i_3^3 g_3^3 x_1 - 4 C^3 j_2 g_3^3 c_3^6 x_1 - 108 C^3 c_3^6 a_2^3 g_3^3 x_1 \\
& + 192 C^3 c_2 g_3^3 d_3 a_2 c_3^5 x_1 - 96 C^3 c_2 g_3^4 i_3 a_2 c_3^3 x_1 + 20 C^3 c_2 g_3^4 c_3^2 i_3^2 x_1 \\
& + 16 C^3 c_2^2 g_3^5 c_3 i_3 x_1 + 240 C^3 d_3 a_2 g_3^2 c_3^6 i_3 x_1 + 96 C^3 d_3^2 c_3^7 g_3 i_3 x_1 \\
& - 240 C^3 a_2 g_3 d_3^2 c_3^8 x_1 - 80 C^3 d_3 i_3 g_3^3 c_2 c_3^4 x_1 - 48 C^3 d_3 i_3^2 g_3^2 c_3^5 x_1 \\
& + 80 C^3 d_3^2 c_3^6 c_2 g_3^2 x_1 - 288 C^3 d_3 c_3^7 a_2^2 g_3^2 x_1 - 8 c_3^3 g_3^4 C^2 c_2 i_3 x_1^2 \\
& + 24 c_3^4 g_3^4 C^2 c_2 a_2 x_1^2 + 24 c_3^5 g_3^3 C^2 c_2 d_3 x_1^2 + 12 c_3^6 g_3^2 C^2 d_3 i_3 x_1^2 \\
& - 72 c_3^7 g_3^2 C^2 d_3 a_2 x_1^2 - 4 c_3^2 g_3^5 C^2 c_2^2 x_1^2 - 24 c_3^8 g_3 C^2 d_3^2 x_1^2 \\
& - 36 c_3^6 g_3^3 C^2 a_2^2 x_1^2 - 4 c_3^6 g_3^3 C^2 d_2 x_1^2 + 144 C^3 i_3 a_2^2 c_3^5 g_3^3 x_1 \\
& + 108 C^3 c_2 g_3^4 c_3^4 a_2^2 x_1 - 36 C^3 c_2^2 g_3^5 a_2 c_3^2 x_1 - 60 C^3 c_3^4 i_3^2 g_3^3 a_2 x_1 \\
& - 32 C^3 c_2^2 g_3^4 d_3 c_3^3 x_1 + 24 c_3^5 g_3^3 C^2 i_3 a_2 x_1^2 - 16 c_3^6 g_3^3 C a_2 x_1^3 + 4 c_3^4 g_3^4 C c_2 x_1^3 \\
& - 64 C^3 d_3 c_3^6 i_3 g_3^2 x_3 + 48 C^4 c_2^2 g_3^4 d_3 c_3^3 x_2 - 32 C^3 c_2 g_3^3 d_3 c_3^5 x_3 \\
& - 48 C^4 c_3^2 i_3^2 g_3^4 x_2 c_2 - 24 C^4 c_2^2 g_3^5 c_3 i_3 x_2 + 16 C^3 c_2 g_3^4 c_3^3 i_3 x_3 \\
& - 108 C^4 c_3^4 a_2^2 g_3^4 x_2 c_2 - 216 C^4 c_3^5 a_2^2 g_3^3 x_2 i_3 + 108 C^4 c_3^6 a_2^3 g_3^3 x_2 \\
& + 432 C^4 c_3^7 a_2^2 g_3^2 x_2 d_3 - 288 C^4 d_3 a_2 c_3^5 g_3^3 x_2 c_2 - 576 C^4 d_3 a_2 c_3^6 g_3^2 x_2 i_3 \\
& + 576 C^4 d_3^2 a_2 c_3^8 g_3 x_2 + 96 C^3 d_3 a_2 c_3^7 g_3^2 x_3 + 144 C^4 i_3 a_2 c_3^3 g_3^4 x_2 c_2 \\
& + 144 C^4 i_3^2 a_2 c_3^4 g_3^3 x_2 - 48 C^3 i_3 a_2 c_3^5 g_3^3 x_3 + 36 C^4 c_2^2 g_3^5 a_2 c_3^2 x_2 \\
& + 36 C^3 c_3^6 a_2^2 g_3^3 x_3 + 64 C^3 d_3^2 c_3^8 x_3 g_3 + 16 C^3 c_3^4 i_3^2 g_3^3 x_3 + 4 C^3 c_2^2 g_3^5 x_3 c_3^2 \\
& - 384 C^4 d_3^2 c_3^7 x_2 i_3 g_3 + 192 C^4 d_3 c_3^4 i_3 g_3^3 x_2 c_2 + 192 C^4 d_3 c_3^5 i_3^2 g_3^2 x_2 \\
& - 32 c_3^7 g_3^2 C^2 d_3 x_3 x_1 + 16 c_3^5 g_3^3 C^2 i_3 x_3 x_1 - 24 C^3 c_2 g_3^4 a_2 c_3^4 x_3 \\
& - 192 C^4 d_3^2 c_3^6 x_2 c_2 g_3^2 - 32 C^4 c_3^3 i_3^3 g_3^3 x_2 + 256 C^4 d_3^3 c_3^9 x_2 - 4 C^4 c_2^3 g_3^6 x_2 \\
& + 4 C^3 c_2^3 g_3^6 x_1 - 64 C^3 d_3^3 c_3^9 x_1 + 96 x_2 g_3^3 C^3 c_3^5 c_2 d_3 x_1 - 48 x_2 g_3^4 C^3 c_3^3 c_2 i_3 x_1 \\
& + 36 c_3^6 g_3^3 x_2 C^2 a_2 x_1^2 - 12 c_3^4 g_3^4 x_2 C^2 c_2 x_1^2 - 4 c_3^6 x_2 g_3^3 C x_1^3 + 3 c_3^6 g_3^3 x_1^4 \\
& + 72 x_2 g_3^4 C^3 c_3^4 c_2 a_2 x_1 - 12 x_2 g_3^5 C^3 c_3^2 c_2^2 x_1 - 192 x_2 g_3 C^3 c_3^8 d_3^2 x_1 \\
& + 192 x_2 g_3^2 C^3 c_3^6 d_3 i_3 x_1 - 288 x_2 g_3^2 C^3 c_3^7 d_3 a_2 x_1 - 108 x_2 g_3^3 C^3 c_3^6 a_2^2 x_1 \\
& - 48 x_2 g_3^3 C^3 c_3^4 i_3^2 x_1 + 144 x_2 g_3^3 C^3 c_3^5 i_3 a_2 x_1 - 24 c_3^5 g_3^3 C^2 x_2 i_3 x_1^2 \\
& + 48 c_3^7 g_3^2 C^2 x_2 d_3 x_1^2 + 4 c_3^6 g_3^3 C x_3 x_1^2 - 24 a_2 c_3^6 g_3^3 C^2 x_1 x_3 \\
& - 24 d_3 c_3^6 s_3 g_3^2 C^3 x_1 - 24 a_2 c_3^5 g_3^3 s_3 C^3 x_1 + 8 c_2 g_3^4 C^2 c_3^4 x_1 x_3 \\
& + 12 c_3^4 i_3 g_3^3 s_3 C^3 x_1 + 12 C c_3^5 i_3 g_3^3 x_1^3 - 24 C d_3 c_3^7 g_3^2 x_1^3) / (4 g_3^3 c_3^5 C^3)]
\end{aligned}$$

> **simplify(jacobian(subs(x1=x1+C/g3\*(-c2\*g3^2-2\*c3\*i3\*g3+3\*a2\*c3^2\*g3+4\*d3\*c3^3)/c3^2,evalm(G)), [x2,x3])) ;**

$$\begin{bmatrix} 0 & 0 \\ \frac{c3 x1^2}{C^2} & -\frac{c3 x1}{C^2} \\ \frac{c3 x1^3}{C^2} & -\frac{c3 x1^2}{C^2} \end{bmatrix}$$

> **contradict** (1,'c3');

Contradiction on case level 2, so:

$$c3 = 0$$

Variables to be uneliminated:

"j3 := 'j3'"

"j1 := 'j1'"

"d1 := 'd1'"

"p3 := 'p3'"

Proceed on case level 1 with:

$$6 g3 \neq 0$$

On account of:

$$c3 = 0$$

$$\{1 \neq 0\}$$

c3 is set to:

$$0$$

> **tmp1 := cpcoeff** (x1^2\*x2);

$$tmp1 := g3^2 c2^2$$

> **elimsolve** (tmp1,c2);

$$\{1 \neq 0\}$$

c2 is set to:

$$0$$

> **tmp1 := cpcoeff** (x1^3);

$$tmp1 := -8 d1^3$$

> **elimsolve** (tmp1,d1);

$$\{1 \neq 0\}$$

d1 is set to:

$$0$$

> **launchNZcase** (j1);

Launching case level 2:

$$j1 \neq 0$$

Assume from now on that:

$$6 g3 j1 \neq 0$$

> **launchNZcase** (g3\*s3-p3\*i3);

Launching case level 3:

$$g3 s3 - p3 i3 \neq 0$$

Assume from now on that:

$$6 g3 j1 (g3 s3 - p3 i3) \neq 0$$

> **tmp1 := cpcoeff** (1);

$$tmp1 := \frac{j1 (g3 s3 - p3 i3) (g3 j1 + g3 s3 - p3 i3)}{g3^2}$$

> **elimsolve** (tmp1,s3);

$$\{g3 \neq 0\}$$

s3 is set to:

$$-\frac{g3 j1 - p3 i3}{g3}$$

Nonzero constraint refines to:

$$-6 g3^2 j1^2 \neq 0$$

> **tmp1 := cpcoeff** (T);

$$tmp1 := -j1^2$$

> **contradict** (tmp1,'s3');

Contradiction on case level 3, so:

$$g3 s3 - p3 i3 = 0$$

Variables to be uneliminated:

$$s3 := s3$$

Proceed on case level 2 with:

$$6 g3 j1 \neq 0$$

On account of:

$$g3 s3 - p3 i3 = 0$$

$$\{g3 \neq 0\}$$

s3 is set to:

$$\frac{p3 i3}{g3}$$

> **tmp1 := cpcoeff** (T);

$$tmp1 := -j1^2$$

> **contradict** (tmp1,'j1');

Contradiction on case level 2, so:

$$j1 = 0$$

Variables to be uneliminated:

$$s3 := s3$$

Proceed on case level 1 with:

$$6 g3 \neq 0$$

On account of:

$$j1 = 0$$

$$\{1 \neq 0\}$$

j1 is set to:

$$0$$

> **tmp1 := cpcoeff** (T);

$$tmp1 := -\frac{(g3 s3 - p3 i3)^2}{g3^2}$$

> **elimsolve** (tmp1,s3);

$$\{g3 \neq 0\}$$

s3 is set to:

```

|
|                                      $\frac{p3 \, i3}{g3}$ 
|
| > det(T-jacobian(H,[x1,x2,x3]));
|                                      $T^3$ 
|
| > H;
|
|  $\left[ 0, \frac{x1^4}{4} + a2 \, x1^3 + d2 \, x1^2 - i3 \, x1 \, x2 - \frac{i3^2 \, x1 \, x3}{g3} + j2 \, x1 - \frac{p3 \, i3 \, x2}{g3} - \frac{p3 \, i3^2 \, x3}{g3^2}, \right.$ 
|
|  $\left. d3 \, x1^2 + g3 \, x1 \, x2 + i3 \, x1 \, x3 + j3 \, x1 + p3 \, x2 + \frac{p3 \, i3 \, x3}{g3} \right]$ 
|
| > M := evalm([ [1,0,0],[0,1,-i3/g3],[0,0,1]]);
|
|  $M := \begin{bmatrix} 1 & 0 & 0 \\ 0 & 1 & -\frac{i3}{g3} \\ 0 & 0 & 1 \end{bmatrix}$ 
|
| > evalm(simplify(jacobian(evalm(M^(-1))&*
| > subs({seq([x1,x2,x3][i]=evalm(M&*[x1,x2,x3])[i],i=1..3)},H)),
| > [x1,x2,x3])));
|
|  $\begin{bmatrix} 0 & 0 & 0 \\ \frac{x1^3 \, g3 + 3 \, a2 \, x1^2 \, g3 + 2 \, d2 \, x1 \, g3 + j2 \, g3 + 2 \, i3 \, d3 \, x1 + i3 \, j3}{g3} & 0 & 0 \\ 2 \, d3 \, x1 + g3 \, x2 + j3 & g3 \, x1 + p3 & 0 \end{bmatrix}$ 
|
| > contradict (1,'g3');
| Contradiction on case level 1, so:
|
|  $g3 = 0$ 
|
| Variables to be uneliminated:
|
| "s3 := 's3'"
| "j1 := 'j1'"
| "d1 := 'd1'"
| "c2 := 'c2'"
| "c3 := 'c3'"
| "o3 := 'o3'"
| "a1 := 'a1'"
| "r3 := 'r3'"
| "w2 := 'w2'"
| "s2 := 's2'"
| "r2 := 'r2'"
| "q2 := 'q2'"
| "i2 := 'i2'"
| "s1 := 's1'"
| "r1 := 'r1'"
| "h2 := 'h2'"

```

|                                    |                     |
|------------------------------------|---------------------|
|                                    | "q1 := 'q1'"        |
|                                    | "v2 := 'v2'"        |
|                                    | "q3 := 'q3'"        |
|                                    | "i1 := 'i1'"        |
|                                    | "h1 := 'h1'"        |
|                                    | "u2 := 'u2'"        |
|                                    | "h3 := 'h3'"        |
|                                    | "c1 := 'c1'"        |
| Proceed on case level 0 with:      |                     |
|                                    | $6 \neq 0$          |
| On account of:                     |                     |
|                                    | $g3 = 0$            |
|                                    | $\{1 \neq 0\}$      |
| g3 is set to:                      |                     |
|                                    | 0                   |
| > tmp1 := cpcoeff (x1^6);          |                     |
|                                    | $tmp1 := -c3^3$     |
| > elimsolve (tmp1,c3);             |                     |
|                                    | $\{1 \neq 0\}$      |
| c3 is set to:                      |                     |
|                                    | 0                   |
| > launchNZcase (a1);               |                     |
| Launching case level 1:            |                     |
|                                    | $a1 \neq 0$         |
| Assume from now on that:           |                     |
|                                    | $6 a1 \neq 0$       |
| > tmp1 := cpcoeff (x1^2*x2^2);     |                     |
|                                    | $tmp1 := 3 a1 o3^2$ |
| > elimsolve (tmp1,o3);             |                     |
|                                    | $\{1 \neq 0\}$      |
| o3 is set to:                      |                     |
|                                    | 0                   |
| > tmp1 := cpcoeff (x2^2*T);        |                     |
|                                    | $tmp1 := -81 a1^4$  |
| > contradict (tmp1,'a1');          |                     |
| Contradiction on case level 1, so: |                     |
|                                    | $a1 = 0$            |
| Variables to be uneliminated:      |                     |
|                                    | "o3 := 'o3'"        |
| Proceed on case level 0 with:      |                     |
|                                    | $6 \neq 0$          |
| On account of:                     |                     |
|                                    | $a1 = 0$            |
|                                    | $\{1 \neq 0\}$      |

```

a1 is set to:
0
> tmp1 := cpcoeff (x2^2*T);
tmp1 := -o3^2
> elimsolve (tmp1,o3);
{1 ≠ 0}
o3 is set to:
0
> launchNZcase (c1);
Launching case level 1:
c1 ≠ 0
Assume from now on that:
6 c1 ≠ 0
> tmp1 := cpcoeff (x1^5);
tmp1 := -c1 p3
> elimsolve (tmp1,p3);
{1 ≠ 0}
p3 is set to:
0
> launchNZcase (h3);
Launching case level 2:
h3 ≠ 0
Assume from now on that:
6 c1 h3 ≠ 0
> tmp1 := cpcoeff (x1^3*x3^3);
tmp1 := 6 c1 (h3 + c1) h3
> elimsolve (tmp1,h3);
{1 ≠ 0}
h3 is set to:
-c1
Nonzero constraint refines to:
-6 c1^2 ≠ 0
> tmp1 := cpcoeff (x1^2*x3^2*T);
tmp1 := -3 c1^2
> contradict (tmp1,'h3');
Contradiction on case level 2, so:
h3 = 0
Variables to be uneliminated:
"h3 := 'h3'"
Proceed on case level 1 with:
6 c1 ≠ 0
On account of:
h3 = 0
{1 ≠ 0}
h3 is set to:

```

```

[
0
> tmp1 := cpcoeff (x1^2*x3^2*T);
                                     tmp1 := -4 c1^2
> contradict (tmp1,'c1');
Contradiction on case level 1, so:
                                     c1 = 0
Variables to be uneliminated:
                                     "h3 := 'h3'"
                                     "p3 := 'p3'"
Proceed on case level 0 with:
                                     6 ≠ 0
On account of:
                                     c1 = 0
                                     {1 ≠ 0}
c1 is set to:
                                     0
> tmp1 := cpcoeff (x1^2*x3^2*T);
                                     tmp1 := -4 h3^2
> elimsolve (tmp1,h3);
                                     {1 ≠ 0}
h3 is set to:
                                     0
> launchNZcase (p3);
Launching case level 1:
                                     p3 ≠ 0
Assume from now on that:
                                     6 p3 ≠ 0
> tmp1 := cpcoeff (x1^3*x3^2);
                                     tmp1 := -3 q1 p3
> elimsolve (tmp1,q1);
                                     {1 ≠ 0}
q1 is set to:
                                     0
> tmp1 := cpcoeff (x1^4);
                                     tmp1 := -i1 p3
> elimsolve (tmp1,i1);
                                     {1 ≠ 0}
i1 is set to:
                                     0
> tmp1 := cpcoeff (x1^4*x3);
                                     tmp1 := -2 h1 p3
> elimsolve (tmp1,h1);
                                     {1 ≠ 0}
h1 is set to:
                                     0
]

```

```

> tmp1 := cpcoeff (x3^4*T);
tmp1 := -9 q3^2

> elimsolve (tmp1,q3);
{1 ≠ 0}
q3 is set to:
0

> tmp1 := cpcoeff (x2*T);
tmp1 := 2 r3 p3

> elimsolve (tmp1,r3);
{1 ≠ 0}
r3 is set to:
0

> tmp1 := cpcoeff (x1^2*x3*T);
tmp1 := -2 u2 p3

> elimsolve (tmp1,u2);
{1 ≠ 0}
u2 is set to:
0

> tmp1 := cpcoeff (x1^3*x3);
tmp1 := -2 r1 p3

> elimsolve (tmp1,r1);
{1 ≠ 0}
r1 is set to:
0

> tmp1 := cpcoeff (x3^3*T);
tmp1 := -4 w2 p3

> elimsolve (tmp1,w2);
{1 ≠ 0}
w2 is set to:
0

> tmp1 := cpcoeff (x1*x3^2*T);
tmp1 := -3 v2 p3

> elimsolve (tmp1,v2);
{1 ≠ 0}
v2 is set to:
0

> tmp1 := cpcoeff (x3^2*T);
tmp1 := -3 q2 p3

> elimsolve (tmp1,q2);
{1 ≠ 0}
q2 is set to:
0

> tmp1 := cpcoeff (x1*x3*T);
tmp1 := -2 h2 p3

```

```

> elimsolve (tmp1,h2);
                                     {1 ≠ 0}
h2 is set to:
                                     0
> tmp1 := cpcoeff (x3*T);
                                     tmp1 := -2 r2 p3 - i3 s1
> elimsolve (tmp1,r2);
                                     {2 p3 ≠ 0}
r2 is set to:
                                     -  $\frac{i3 s1}{2 p3}$ 
> tmp1 := cpcoeff (x1^2*T);
                                     tmp1 := -2 d1 i3 - i3^2 - 4 d1^2 - c2 p3
> elimsolve (tmp1,c2);
                                     {p3 ≠ 0}
c2 is set to:
                                     -  $\frac{2 d1 i3 + i3^2 + 4 d1^2}{p3}$ 
> tmp1 := cpcoeff (x1^3);
                                     tmp1 := -s1 p3 - 8 d1^3
> elimsolve (tmp1,s1);
                                     {p3 ≠ 0}
s1 is set to:
                                     -  $\frac{8 d1^3}{p3}$ 
> tmp1 := cpcoeff (T);
                                     tmp1 :=  $\frac{-j1 s3 p3 - s3^2 p3 - s2 p3^2 - j1^2 p3 + 8 j3 d1^3}{p3}$ 
> elimsolve (tmp1,s2);
                                     {-p3^2 ≠ 0}
s2 is set to:
                                      $\frac{-j1 s3 p3 - s3^2 p3 - j1^2 p3 + 8 j3 d1^3}{p3^2}$ 
> tmp1 := cpcoeff (x2);
                                     tmp1 := -8 (2 d1 + i3) d1^3
> tmp2 := cpcoeff (x1*x3);
                                     tmp2 := -  $\frac{8 d1^3 (i3^2 + 8 d1^2)}{p3}$ 
> tmp3 := factor ((2*d1-i3)*tmp1 + p3*tmp2);
                                     tmp3 := -96 d1^5
> elimsolve (tmp3,d1);
                                     {1 ≠ 0}

```

d1 is set to:

$$0$$

> tmp1 := cpcoeff (1);

$$tmp1 := -j l^3$$

> elimsolve (tmp1,j1);

$$\{1 \neq 0\}$$

j1 is set to:

$$0$$

> tmp1 := cpcoeff (x1\*T);

$$tmp1 := -i2 p3 - 2 s3 i3$$

> elimsolve (tmp1,i2);

$$\{p3 \neq 0\}$$

i2 is set to:

$$-\frac{2 s3 i3}{p3}$$

> launchNZcase (i3);

Launching case level 2:

$$i3 \neq 0$$

Assume from now on that:

$$6 p3 i3 \neq 0$$

> det (T-jacobian (H, [x1,x2,x3])) ;

$$T^3$$

> H;

$$\left[ 0, \frac{x1^4}{4} + a2 x1^3 - \frac{i3^2 x1^2 x3}{p3} + d2 x1^2 - i3 x1 x2 - \frac{2 s3 i3 x1 x3}{p3} + j2 x1 - s3 x2 - \frac{s3^2 x3}{p3}, \right. \\ \left. d3 x1^2 + i3 x1 x3 + j3 x1 + p3 x2 + s3 x3 \right]$$

> M := evalm([[i3,0,0], [0,0,1], [0,-p3,-s3]]);

$$M := \begin{bmatrix} i3 & 0 & 0 \\ 0 & 0 & 1 \\ 0 & -p3 & -s3 \end{bmatrix}$$

> det (M) ;

$$p3 i3$$

> G := simplify(evalm(M&\*subs({seq([x1,x2,x3][i]=

> evalm(M^(-1)&\*[x1,x2,x3])[i],i=1..n)},H));

$$G := \left[ 0, \frac{d3 x1^2 + x1 x2 i3^2 + j3 x1 i3 - i3^2 x3}{i3^2}, -x1 (x1^3 p3 + 4 a2 x1^2 i3 p3 - 4 x1 x2 i3^4 \right. \\ \left. + 4 d2 x1 i3^2 p3 + 4 i3^4 x3 + 4 j2 i3^3 p3 + 4 s3 i3^2 d3 x1 + 4 s3 i3^3 j3) / (4 i3^4) \right]$$

> simplify(jacobian(G, [x2,x3]));

$$\begin{bmatrix} 0 & 0 \\ x1 & -1 \\ x1^2 & -x1 \end{bmatrix}$$

> **contradict** (1,'i3');

Contradiction on case level 2, so:

$$i3 = 0$$

Proceed on case level 1 with:

$$6 p3 \neq 0$$

On account of:

$$i3 = 0$$

$$\{1 \neq 0\}$$

i3 is set to:

$$0$$

> **det**(T-jacobian(H,[x1,x2,x3]));

$$T^3$$

> **H**;

$$\left[ 0, \frac{x1^4}{4} + a2 x1^3 + d2 x1^2 + j2 x1 - s3 x2 - \frac{s3^2 x3}{p3}, d3 x1^2 + j3 x1 + p3 x2 + s3 x3 \right]$$

> **M** := **evalm**([[1,0,0],[0,1,-s3/p3],[0,0,1]]);

$$M := \begin{bmatrix} 1 & 0 & 0 \\ 0 & 1 & -\frac{s3}{p3} \\ 0 & 0 & 1 \end{bmatrix}$$

> **evalm**(**simplify**(**jacobian**(**evalm**(M^(-1) &

> **subs** ({**seq** ([x1,x2,x3][i]=**evalm**(M&\*[x1,x2,x3])[i],i=1..3)},H)),

> [x1,x2,x3])));

$$\begin{bmatrix} 0 & 0 & 0 \\ \frac{x1^3 p3 + 3 a2 x1^2 p3 + 2 d2 x1 p3 + j2 p3 + 2 s3 d3 x1 + s3 j3}{p3} & 0 & 0 \\ 2 d3 x1 + j3 & p3 & 0 \end{bmatrix}$$

> **contradict** (1,'p3');

Contradiction on case level 1, so:

$$p3 = 0$$

Variables to be uneliminated:

"i3 := 'i3'"

"i2 := 'i2'"

"j1 := 'j1'"

"d1 := 'd1'"

"s2 := 's2'"

"s1 := 's1'"

"c2 := 'c2'"

"r2 := 'r2'"

"h2 := 'h2'"

|                                       |                                              |
|---------------------------------------|----------------------------------------------|
|                                       | "q2 := 'q2'"                                 |
|                                       | "v2 := 'v2'"                                 |
|                                       | "w2 := 'w2'"                                 |
|                                       | "r1 := 'r1'"                                 |
|                                       | "u2 := 'u2'"                                 |
|                                       | "r3 := 'r3'"                                 |
|                                       | "q3 := 'q3'"                                 |
|                                       | "h1 := 'h1'"                                 |
|                                       | "i1 := 'i1'"                                 |
|                                       | "q1 := 'q1'"                                 |
| Proceed on case level 0 with:         |                                              |
|                                       | $6 \neq 0$                                   |
| On account of:                        |                                              |
|                                       | $p3 = 0$                                     |
|                                       | $\{1 \neq 0\}$                               |
| p3 is set to:                         |                                              |
|                                       | 0                                            |
| > <b>launchNZcase (d3);</b>           |                                              |
| Launching case level 1:               |                                              |
|                                       | $d3 \neq 0$                                  |
| Assume from now on that:              |                                              |
|                                       | $6 d3 \neq 0$                                |
| > <b>tmp1 := cpcoeff (x1^2*x3*T);</b> |                                              |
|                                       | $tmp1 := -4 d3 h1$                           |
| > <b>elimsolve (tmp1,h1);</b>         |                                              |
|                                       | $\{1 \neq 0\}$                               |
| h1 is set to:                         |                                              |
|                                       | 0                                            |
| > <b>tmp1 := cpcoeff (x3^4*T);</b>    |                                              |
|                                       | $tmp1 := -9 q3^2$                            |
| > <b>elimsolve (tmp1,q3);</b>         |                                              |
|                                       | $\{1 \neq 0\}$                               |
| q3 is set to:                         |                                              |
|                                       | 0                                            |
| > <b>tmp1 := cpcoeff (x1*x3^2*T);</b> |                                              |
|                                       | $tmp1 := -6 d3 q1$                           |
| > <b>elimsolve (tmp1,q1);</b>         |                                              |
|                                       | $\{1 \neq 0\}$                               |
| q1 is set to:                         |                                              |
|                                       | 0                                            |
| > <b>tmp1 := cpcoeff (x1^2*T);</b>    |                                              |
|                                       | $tmp1 := -2 d1 i3 - i3^2 - 4 d1^2 - 2 d3 i1$ |
| > <b>elimsolve (tmp1,i1);</b>         |                                              |

|                                  |                                                                      |
|----------------------------------|----------------------------------------------------------------------|
|                                  | $\{2 d3 \neq 0\}$                                                    |
| i1 is set to:                    | $-\frac{2 d1 i3 + i3^2 + 4 d1^2}{2 d3}$                              |
| > tmp1 := cpcoeff (x1^3);        | $tmp1 := (2 d1 + i3)^3$                                              |
| > elimsolve (tmp1,d1);           | $\{2 \neq 0\}$                                                       |
| d1 is set to:                    | $-\frac{i3}{2}$                                                      |
| > tmp1 := cpcoeff (x1*x3*T);     | $tmp1 := -4 d3 r1 - 2 i3 r3$                                         |
| > elimsolve (tmp1,r1);           | $\{2 d3 \neq 0\}$                                                    |
| r1 is set to:                    | $-\frac{i3 r3}{2 d3}$                                                |
| > tmp1 := cpcoeff (x3^2*T);      | $tmp1 := -\frac{(4 r3 d3 - i3^2)^2}{4 d3^2}$                         |
| > elimsolve (tmp1,r3);           | $\{4 d3 \neq 0\}$                                                    |
| r3 is set to:                    | $\frac{i3^2}{4 d3}$                                                  |
| > tmp1 := cpcoeff (x1*T);        | $tmp1 := \frac{2 j1 i3 d3 - 2 s3 i3 d3 + j3 i3^2 - 4 d3^2 s1}{2 d3}$ |
| > elimsolve (tmp1,s1);           | $\{-4 d3^2 \neq 0\}$                                                 |
| s1 is set to:                    | $\frac{i3 (2 j1 d3 - 2 s3 d3 + i3 j3)}{4 d3^2}$                      |
| > launchNZcase (j1+s3);          |                                                                      |
| Launching case level 2:          | $j1 + s3 \neq 0$                                                     |
| Assume from now on that:         | $6 d3 (j1 + s3) \neq 0$                                              |
| > launchNZcase (-i3*j3+2*d3*s3); |                                                                      |
| Launching case level 3:          | $-i3 j3 + 2 s3 d3 \neq 0$                                            |
| Assume from now on that:         |                                                                      |

```

[
  6 d3 (j1 + s3) (-i3 j3 + 2 s3 d3) ≠ 0
> tmp1 := cpcoeff (1);
      (j1 + s3) (-i3 j3 + 2 s3 d3) (2 j1 d3 + i3 j3)
      tmp1 := -----
                4 d32
> elimsolve (tmp1, j1);
      { 2 d3 ≠ 0 }
j1 is set to:
      - i3 j3
      - ----
        2 d3
Nonzero constraint refines to:
      6 d3 (-i3 j3 + 2 s3 d3)2 ≠ 0
> tmp1 := cpcoeff (T);
      (-i3 j3 + 2 s3 d3)2
      tmp1 := - ----
                4 d32
> contradict (tmp1, 's3');
Contradiction on case level 3, so:
      -i3 j3 + 2 s3 d3 = 0
Variables to be uneliminated:
      "j1 := 'j1'"
Proceed on case level 2 with:
      6 d3 (j1 + s3) ≠ 0
On account of:
      -i3 j3 + 2 s3 d3 = 0
      { 2 d3 ≠ 0 }
s3 is set to:
      i3 j3
      ----
      2 d3
Nonzero constraint refines to:
      6 d3 (2 j1 d3 + i3 j3) ≠ 0
> tmp1 := cpcoeff (T);
      (2 j1 d3 + i3 j3)2
      tmp1 := - ----
                4 d32
> contradict (tmp1, 's3');
Contradiction on case level 2, so:
      j1 + s3 = 0
Variables to be uneliminated:
      "s3 := 's3'"
Proceed on case level 1 with:
      6 d3 ≠ 0
On account of:
      j1 + s3 = 0
      { 1 ≠ 0 }
s3 is set to:
      -j1

```

```
> tmp1 := cpcoeff (T);
```

$$tmp1 := -\frac{(2j1\,d3 + i3\,j3)^2}{4\,d3^2}$$

```
> elimsolve (tmp1,j1);
```

$$\{2\,d3 \neq 0\}$$

```
j1 is set to:
```

$$-\frac{i3\,j3}{2\,d3}$$

```
> det(T-jacobian(H,[x1,x2,x3]));
```

$$T^3$$

```
> H;
```

$$\left[ -\frac{i3\,x1^2}{2} - \frac{i3^2\,x1\,x3}{2\,d3} - \frac{i3\,j3\,x1}{2\,d3} - \frac{i3^3\,x3^2}{8\,d3^2} - \frac{i3^2\,j3\,x3}{4\,d3^2}, \frac{x1^4}{4} + u2\,x1^2\,x3^2 + v2\,x1\,x3^3 + w2\,x3^4 \right. \\ \left. + a2\,x1^3 + c2\,x1^2\,x3 + d2\,x1^2 + h2\,x1\,x3^2 + i2\,x1\,x3 + j2\,x1 + q2\,x3^3 + r2\,x3^2 + s2\,x3, \right. \\ \left. d3\,x1^2 + i3\,x1\,x3 + j3\,x1 + \frac{i3^2\,x3^2}{4\,d3} + \frac{i3\,j3\,x3}{2\,d3} \right]$$

```
> factor(2*d3*H[1]+i3*H[3]);
```

$$0$$

```
> M := evalm([ [1,-i3/2/d3,0], [0,0,1], [0,1,0] ] );
```

$$M := \begin{bmatrix} 1 & -\frac{i3}{2\,d3} & 0 \\ 0 & 0 & 1 \\ 0 & 1 & 0 \end{bmatrix}$$

```
> evalm(simplify(jacobian(evalm(M^(-1)&*
```

```
> subs({seq([x1,x2,x3][i]=evalm(M&*[x1,x2,x3])[i],i=1..3)},H)),
```

```
> [x1,x2,x3])));
```

```
[0,0,0]
```

$$[2\,d3\,x1 + j3, 0, 0]$$

$$\begin{aligned} & [(8\,d3^3\,x1^3 - 12\,d3^2\,x1^2\,i3\,x2 + 6\,d3\,x1\,i3^2\,x2^2 - i3^3\,x2^3 + 16\,u2\,x2^2\,d3^3\,x1 - 8\,u2\,x2^3\,d3^2\,i3 \\ & + 8\,v2\,x2^3\,d3^3 + 24\,a2\,d3^3\,x1^2 - 24\,a2\,d3^2\,x1\,i3\,x2 + 6\,a2\,d3\,i3^2\,x2^2 + 16\,c2\,x2\,d3^3\,x1 \\ & - 8\,c2\,x2^2\,d3^2\,i3 + 16\,d2\,d3^3\,x1 - 8\,d2\,d3^2\,i3\,x2 + 8\,h2\,x2^2\,d3^3 + 8\,i2\,x2\,d3^3 + 8\,j2\,d3^3) / (8 \\ & d3^3), -(-12\,c2\,x2^2\,i3^2\,d3^2 + 6\,a2\,i3^3\,d3\,x2^2 + 24\,a2\,i3\,d3^3\,x1^2 - 16\,c2\,d3^4\,x1^2 \\ & - 32\,h2\,x2\,d3^4\,x1 + 8\,i3\,d3^3\,x1^3 - 32\,r2\,x2\,d3^4 - 48\,q2\,x2^2\,d3^4 - 8\,d2\,i3^2\,d3^2\,x2 \\ & + 16\,d2\,i3\,d3^3\,x1 - 64\,w2\,x2^3\,d3^4 - i3^4\,x2^3 - 16\,s2\,d3^4 - 16\,i2\,d3^4\,x1 + 8\,j2\,i3\,d3^3 \\ & - 16\,u2\,x2^3\,i3^2\,d3^2 + 6\,d3\,x1\,i3^3\,x2^2 - 12\,d3^2\,x1^2\,i3^2\,x2 - 32\,u2\,x2\,d3^4\,x1^2 - 48\,v2\,x2^2\,d3^4\,x1 \\ & + 32\,v2\,i3\,x2^3\,d3^3 + 16\,i2\,i3\,x2\,d3^3 + 24\,h2\,i3\,x2^2\,d3^3 + 48\,u2\,x2^2\,i3\,d3^3\,x1 \\ & - 24\,a2\,i3^2\,d3^2\,x1\,x2 + 32\,c2\,x2\,i3\,d3^3\,x1) / (16\,d3^4), 0] \end{aligned}$$

```
> contradict (1,'d3');
```

```
Contradiction on case level 1, so:
```

|                                    |                                   |
|------------------------------------|-----------------------------------|
|                                    | $d3 = 0$                          |
| Variables to be uneliminated:      |                                   |
|                                    | "j1 := 'j1'"                      |
|                                    | "s3 := 's3'"                      |
|                                    | "s1 := 's1'"                      |
|                                    | "r3 := 'r3'"                      |
|                                    | "r1 := 'r1'"                      |
|                                    | "d1 := 'd1'"                      |
|                                    | "i1 := 'i1'"                      |
|                                    | "q1 := 'q1'"                      |
|                                    | "q3 := 'q3'"                      |
|                                    | "h1 := 'h1'"                      |
| Proceed on case level 0 with:      |                                   |
|                                    | $6 \neq 0$                        |
| On account of:                     |                                   |
|                                    | $d3 = 0$                          |
|                                    | $\{1 \neq 0\}$                    |
| d3 is set to:                      |                                   |
|                                    | 0                                 |
| > <b>launchNZcase (d1);</b>        |                                   |
| Launching case level 1:            |                                   |
|                                    | $d1 \neq 0$                       |
| Assume from now on that:           |                                   |
|                                    | $6\ d1 \neq 0$                    |
| > <b>launchNZcase (i3);</b>        |                                   |
| Launching case level 2:            |                                   |
|                                    | $i3 \neq 0$                       |
| Assume from now on that:           |                                   |
|                                    | $6\ d1\ i3 \neq 0$                |
| > <b>tmp1 := cpcoeff (x1^3);</b>   |                                   |
|                                    | $tmp1 := 2\ d1\ (2\ d1 + i3)\ i3$ |
| > <b>elimsolve (tmp1,i3);</b>      |                                   |
|                                    | $\{1 \neq 0\}$                    |
| i3 is set to:                      |                                   |
|                                    | $-2\ d1$                          |
| Nonzero constraint refines to:     |                                   |
|                                    | $-12\ d1^2 \neq 0$                |
| > <b>tmp1 := cpcoeff (x1^2*T);</b> |                                   |
|                                    | $tmp1 := -4\ d1^2$                |
| > <b>contradict (tmp1,'i3');</b>   |                                   |
| Contradiction on case level 2, so: |                                   |
|                                    | $i3 = 0$                          |
| Variables to be uneliminated:      |                                   |
|                                    | "i3 := 'i3'"                      |
| Proceed on case level 1 with:      |                                   |

|                                     |                                                        |
|-------------------------------------|--------------------------------------------------------|
|                                     | $6\,dl \neq 0$                                         |
| On account of:                      |                                                        |
|                                     | $i3 = 0$                                               |
|                                     | $\{1 \neq 0\}$                                         |
| i3 is set to:                       |                                                        |
|                                     | 0                                                      |
| > <b>tmp1 := cpcoeff (x1^2*T);</b>  |                                                        |
|                                     | $tmp1 := -4\,dl^2$                                     |
| > <b>contradict (tmp1,'d1');</b>    |                                                        |
| Contradiction on case level 1, so:  |                                                        |
|                                     | $dl = 0$                                               |
| Variables to be uneliminated:       |                                                        |
|                                     | "i3 := 'i3'"                                           |
| Proceed on case level 0 with:       |                                                        |
|                                     | $6 \neq 0$                                             |
| On account of:                      |                                                        |
|                                     | $dl = 0$                                               |
|                                     | $\{1 \neq 0\}$                                         |
| d1 is set to:                       |                                                        |
|                                     | 0                                                      |
| > <b>tmp1 := cpcoeff (x1^2*T);</b>  |                                                        |
|                                     | $tmp1 := -i3^2$                                        |
| > <b>elimsolve (tmp1,i3);</b>       |                                                        |
|                                     | $\{1 \neq 0\}$                                         |
| i3 is set to:                       |                                                        |
|                                     | 0                                                      |
| > <b>launchNZcase (j3);</b>         |                                                        |
| Launching case level 1:             |                                                        |
|                                     | $j3 \neq 0$                                            |
| Assume from now on that:            |                                                        |
|                                     | $6\,j3 \neq 0$                                         |
| > <b>tmp1 := cpcoeff (x1*x3*T);</b> |                                                        |
|                                     | $tmp1 := -2\,j3\,hl$                                   |
| > <b>elimsolve (tmp1,h1);</b>       |                                                        |
|                                     | $\{1 \neq 0\}$                                         |
| h1 is set to:                       |                                                        |
|                                     | 0                                                      |
| > <b>tmp1 := cpcoeff (x1*T);</b>    |                                                        |
|                                     | $tmp1 := -j3\,il$                                      |
| > <b>elimsolve (tmp1,i1);</b>       |                                                        |
|                                     | $\{1 \neq 0\}$                                         |
| i1 is set to:                       |                                                        |
|                                     | 0                                                      |
| > <b>tmp1 := cpcoeff (x3^2*T);</b>  |                                                        |
|                                     | $tmp1 := -3\,jl\,q3 - 6\,q3\,s3 - 4\,r3^2 - 3\,j3\,ql$ |

```

> elimsolve (tmp1,q1);
                                     {3 j3 ≠ 0}
q1 is set to:
                                     -  $\frac{3 j1 q3 + 6 q3 s3 + 4 r3^2}{3 j3}$ 
> tmp1 := cpcoeff (x3*T);
                                     tmp1 := -2 j1 r3 - 4 r3 s3 - 2 j3 r1
> elimsolve (tmp1,r1);
                                     {j3 ≠ 0}
r1 is set to:
                                     -  $\frac{r3 (j1 + 2 s3)}{j3}$ 
> tmp1 := cpcoeff (T);
                                     tmp1 := -j1 s3 - s3^2 - j1^2 - j3 s1
> elimsolve (tmp1,s1);
                                     {j3 ≠ 0}
s1 is set to:
                                     -  $\frac{j1 s3 + s3^2 + j1^2}{j3}$ 
> tmp1 := cpcoeff (1);
                                     tmp1 := (j1 + s3)^3
> elimsolve (tmp1,s3);
                                     {1 ≠ 0}
s3 is set to:
                                     -j1
> tmp1 := cpcoeff (x3^3);
                                     tmp1 := 8 r3^3
> elimsolve (tmp1,r3);
                                     {1 ≠ 0}
r3 is set to:
                                     0
> tmp1 := cpcoeff (x3^4*T);
                                     tmp1 := -9 q3^2
> elimsolve (tmp1,q3);
                                     {1 ≠ 0}
q3 is set to:
                                     0
> det (T-jacobian (H, [x1,x2,x3])) ;
                                     T^3
> H;

$$\left[ j1 x1 - \frac{j1^2 x3}{j3}, \frac{x1^4}{4} + u2 x1^2 x3^2 + v2 x1 x3^3 + w2 x3^4 + a2 x1^3 + c2 x1^2 x3 + d2 x1^2 \right]$$


```

$$+ h2 x1 x3^2 + i2 x1 x3 + j2 x1 + q2 x3^3 + r2 x3^2 + s2 x3, j3 x1 - j1 x3 \Big]$$

> **factor(j3\*H[1]-j1\*H[3]);**

0

> **M := evalm([ [1,j1/j3,0], [0,0,1], [0,1,0] ] );**

$$M := \begin{bmatrix} 1 & \frac{j1}{j3} & 0 \\ 0 & 0 & 1 \\ 0 & 1 & 0 \end{bmatrix}$$

> **evalm(simplify(jacobian(evalm(M^(-1) &\***

**subs({seq([x1,x2,x3][i]=evalm(M&\*[x1,x2,x3])[i], i=1..3)}, H)),**

**[x1,x2,x3])));**

[0,0,0]

[j3,0,0]

$$\begin{aligned} & [(j3^3 x1^3 + 3 j3^2 x1^2 j1 x2 + 3 j3 x1 j1^2 x2^2 + j1^3 x2^3 + 2 u2 x2^2 j3^3 x1 + 2 u2 x2^3 j3^2 j1 \\ & + v2 x2^3 j3^3 + 3 a2 j3^3 x1^2 + 6 a2 j3^2 x1 j1 x2 + 3 a2 j3 j1^2 x2^2 + 2 c2 x2 j3^3 x1 \\ & + 2 c2 x2^2 j3^2 j1 + 2 d2 j3^3 x1 + 2 d2 j3^2 j1 x2 + h2 x2^2 j3^3 + i2 x2 j3^3 + j2 j3^3) / j3^3, (s2 j3^4 \\ & + j1^4 x2^3 + c2 j3^4 x1^2 + i2 j3^4 x1 + 4 v2 j1 x2^3 j3^3 + 3 h2 j1 x2^2 j3^3 + 2 i2 j1 x2 j3^3 \\ & + 3 j3^2 x1^2 j1^2 x2 + 3 j3 x1 j1^3 x2^2 + 4 u2 x2^3 j1^2 j3^2 + 6 u2 x2^2 j1 j3^3 x1 + 2 u2 x2 j3^4 x1^2 \\ & + 3 v2 x2^2 j3^4 x1 + 4 w2 x2^3 j3^4 + 3 q2 x2^2 j3^4 + 2 r2 x2 j3^4 + j1 j3^3 x1^3 + j2 j1 j3^3 \\ & + 6 a2 j1^2 j3^2 x1 x2 + 4 c2 x2 j1 j3^3 x1 + 3 a2 j1 j3^3 x1^2 + 3 a2 j1^3 j3 x2^2 + 3 c2 x2^2 j1^2 j3^2 \\ & + 2 d2 j1 j3^3 x1 + 2 d2 j1^2 j3^2 x2 + 2 h2 x2 j3^4 x1) / j3^4, 0] \end{aligned}$$

> **contradict(1,'j3');**

Contradiction on case level 1, so:

$$j3 = 0$$

Variables to be uneliminated:

"q3 := 'q3'"

"r3 := 'r3'"

"s3 := 's3'"

"s1 := 's1'"

"r1 := 'r1'"

"q1 := 'q1'"

"i1 := 'i1'"

"h1 := 'h1'"

Proceed on case level 0 with:

$$6 \neq 0$$

On account of:

$$j3 = 0$$

$$\{1 \neq 0\}$$

j3 is set to:

0

```

> launchNZcase (j1);
Launching case level 1:

Assume from now on that:
 $j1 \neq 0$ 
 $6j1 \neq 0$ 

> launchNZcase (s3);
Launching case level 2:

Assume from now on that:
 $s3 \neq 0$ 
 $6j1 s3 \neq 0$ 

> tmp1 := cpcoeff (1);
 $tmp1 := j1 (j1 + s3) s3$ 

> elimsolve (tmp1,s3);
 $\{1 \neq 0\}$ 
s3 is set to:
 $-j1$ 
Nonzero constraint refines to:
 $-6j1^2 \neq 0$ 

> tmp1 := cpcoeff (T);
 $tmp1 := -j1^2$ 

> contradict (tmp1,'s3');
Contradiction on case level 2, so:
 $s3 = 0$ 
Variables to be uneliminated:
"s3 := 's3'"
Proceed on case level 1 with:
 $6j1 \neq 0$ 
On account of:
 $s3 = 0$ 
 $\{1 \neq 0\}$ 
s3 is set to:
0

> tmp1 := cpcoeff (T);
 $tmp1 := -j1^2$ 

> contradict (tmp1,'j1');
Contradiction on case level 1, so:
 $j1 = 0$ 
Variables to be uneliminated:
"s3 := 's3'"
Proceed on case level 0 with:
 $6 \neq 0$ 
On account of:
 $j1 = 0$ 
 $\{1 \neq 0\}$ 
j1 is set to:
0

```

```

> tmp1 := cpcoeff (T);
                                      $tmp1 := -s^3$ 
> elimsolve (tmp1,s3);
                                      $\{1 \neq 0\}$ 
s3 is set to:
                                     0
> launchNZcase (i1);
Launching case level 1:
                                      $i1 \neq 0$ 
Assume from now on that:
                                      $6 i1 \neq 0$ 
> launchNZcase (r3);
Launching case level 2:
                                      $r3 \neq 0$ 
Assume from now on that:
                                      $6 i1 r3 \neq 0$ 
> tmp1 := cpcoeff (x3^3);
                                      $tmp1 := 2 i1 (2 r3 + i1) r3$ 
> elimsolve (tmp1,r3);
                                      $\{2 \neq 0\}$ 
r3 is set to:
                                      $-\frac{i1}{2}$ 
Nonzero constraint refines to:
                                      $-6 i1^2 \neq 0$ 
> tmp1 := cpcoeff (x3^2*T);
                                      $tmp1 := -i1^2$ 
> contradict (tmp1,'r3');
Contradiction on case level 2, so:
                                      $r3 = 0$ 
Variables to be uneliminated:
                                     "r3 := 'r3'"
Proceed on case level 1 with:
                                      $6 i1 \neq 0$ 
On account of:
                                      $r3 = 0$ 
                                      $\{1 \neq 0\}$ 
r3 is set to:
                                     0
> tmp1 := cpcoeff (x3^2*T);
                                      $tmp1 := -i1^2$ 
> contradict (tmp1,'i1');
Contradiction on case level 1, so:
                                      $i1 = 0$ 
Variables to be uneliminated:

```

|                                             |                               |
|---------------------------------------------|-------------------------------|
|                                             | <code>"r3 := 'r3'"</code>     |
| Proceed on case level 0 with:               |                               |
|                                             | $6 \neq 0$                    |
| On account of:                              |                               |
|                                             | $il = 0$                      |
|                                             | $\{1 \neq 0\}$                |
| il is set to:                               |                               |
|                                             | 0                             |
| <code>&gt; tmp1 := cpcoeff (x3^2*T);</code> |                               |
|                                             | $tmp1 := -4 r3^2$             |
| <code>&gt; elimsolve (tmp1,r3);</code>      |                               |
|                                             | $\{1 \neq 0\}$                |
| r3 is set to:                               |                               |
|                                             | 0                             |
| <code>&gt; launchNZcase (h1);</code>        |                               |
| Launching case level 1:                     |                               |
|                                             | $h1 \neq 0$                   |
| Assume from now on that:                    |                               |
|                                             | $6 h1 \neq 0$                 |
| <code>&gt; launchNZcase (q3);</code>        |                               |
| Launching case level 2:                     |                               |
|                                             | $q3 \neq 0$                   |
| Assume from now on that:                    |                               |
|                                             | $6 h1 q3 \neq 0$              |
| <code>&gt; tmp1 := cpcoeff (x3^6);</code>   |                               |
|                                             | $tmp1 := 3 h1 (3 q3 + h1) q3$ |
| <code>&gt; elimsolve (tmp1,q3);</code>      |                               |
|                                             | $\{3 \neq 0\}$                |
| q3 is set to:                               |                               |
|                                             | $-\frac{h1}{3}$               |
| Nonzero constraint refines to:              |                               |
|                                             | $-6 h1^2 \neq 0$              |
| <code>&gt; tmp1 := cpcoeff (x3^4*T);</code> |                               |
|                                             | $tmp1 := -h1^2$               |
| <code>&gt; contradict (tmp1,'q3');</code>   |                               |
| Contradiction on case level 2, so:          |                               |
|                                             | $q3 = 0$                      |
| Variables to be uneliminated:               |                               |
|                                             | <code>"q3 := 'q3'"</code>     |
| Proceed on case level 1 with:               |                               |
|                                             | $6 h1 \neq 0$                 |
| On account of:                              |                               |
|                                             | $q3 = 0$                      |
|                                             | $\{1 \neq 0\}$                |
| q3 is set to:                               |                               |

```
> tmp1 := cpcoeff (x3^4*T);
```

$$\text{tmp1} := -hl^2$$

```
> contradict (tmp1,'h1');
Contradiction on case level 1, so:
```

$$hl = 0$$

Variables to be uneliminated:

$$\text{"q3"} := \text{'q3'}$$

Proceed on case level 0 with:

$$6 \neq 0$$

On account of:

$$hl = 0$$

$$\{1 \neq 0\}$$

h1 is set to:

$$0$$

```
> tmp1 := cpcoeff (x3^4*T);
```

$$\text{tmp1} := -9 q3^2$$

```
> elimsolve (tmp1,q3);
```

$$\{1 \neq 0\}$$

q3 is set to:

$$0$$

```
> det(T-jacobian(H,[x1,x2,x3]));
```

$$T^3$$

```
> H;
```

$$\left[ ql x3^3 + rl x3^2 + sl x3, \frac{x1^4}{4} + u2 xl^2 x3^2 + v2 xl x3^3 + w2 x3^4 + a2 xl^3 + c2 xl^2 x3 + d2 xl^2 \right.$$

$$\quad \left. + h2 xl x3^2 + i2 xl x3 + j2 xl + q2 x3^3 + r2 x3^2 + s2 x3, 0 \right]$$

```
> M := evalm([ [0,1,0], [0,0,1], [1,0,0] ]);
```

$$M := \begin{bmatrix} 0 & 1 & 0 \\ 0 & 0 & 1 \\ 1 & 0 & 0 \end{bmatrix}$$

```
> evalm(simplify(jacobian(evalm(M^(-1))&*
> subs({seq([x1,x2,x3][i]=evalm(M&*[x1,x2,x3])[i],i=1..3)},H)),
>      [x1,x2,x3])));
```

$$[0,0,0]$$

$$[3 ql xl^2 + 2 rl xl + sl, 0, 0]$$

$$[2 u2 x2^2 xl + 3 v2 x2 xl^2 + 4 w2 xl^3 + c2 x2^2 + 2 h2 x2 xl + i2 x2 + 3 q2 xl^2 + 2 r2 xl + s2,$$

$$x2^3 + 2 u2 x2 xl^2 + v2 xl^3 + 3 a2 x2^2 + 2 c2 x2 xl + 2 d2 x2 + h2 xl^2 + i2 xl + j2, 0]$$

```
> contradict (1);
Contradiction on case level 0, so:
```

$$6 = 0$$

Variables to be uneliminated:

"q3 := 'q3'"  
"h1 := 'h1'"  
"r3 := 'r3'"  
"i1 := 'i1'"  
"s3 := 's3'"  
"j1 := 'j1'"  
"j3 := 'j3'"  
"i3 := 'i3'"  
"d1 := 'd1'"  
"d3 := 'd3'"  
"p3 := 'p3'"  
"h3 := 'h3'"  
"c1 := 'c1'"  
"o3 := 'o3'"  
"a1 := 'a1'"  
"c3 := 'c3'"  
"g3 := 'g3'"  
"a3 := 'a3'"  
"m3 := 'm3'"  
"n3 := 'n3'"  
"f3 := 'f3'"  
"b3 := 'b3'"  
"l3 := 'l3'"  
"e3 := 'e3'"  
"k3 := 'k3'"  
"p1 := 'p1'"  
"o1 := 'o1'"  
"n1 := 'n1'"  
"m1 := 'm1'"  
"l1 := 'l1'"  
"k1 := 'k1'"  
"g1 := 'g1'"  
"f1 := 'f1'"  
"e1 := 'e1'"  
"b1 := 'b1'"  
"p2 := 'p2'"  
"o2 := 'o2'"  
"n2 := 'n2'"  
"m2 := 'm2'"

"l2 := 'l2'"

"k2 := 'k2'"

"g2 := 'g2'"

"f2 := 'f2'"

"e2 := 'e2'"

"b2 := 'b2'"

That is all, folks! Check that all variables are uneliminated:

$[a1, b1, c1, d1, e1, f1, g1, h1, i1, j1, k1, l1, m1, n1, o1, p1, q1, r1, s1],$

$[a2, b2, c2, d2, e2, f2, g2, h2, i2, j2, k2, l2, m2, n2, o2, p2, q2, r2, s2],$

$[a3, b3, c3, d3, e3, f3, g3, h3, i3, j3, k3, l3, m3, n3, o3, p3, q3, r3, s3]]$

>
