# Supplementary material for: Computations of Keller maps over fields with $\tfrac16$
Source: arXiv:1609.09753 ancillary file (2017-11-02)
Supplement: Supplementary file 4 [file dim4cub.pdf]

```

[ > restart;
  > efactors := proc (eq)
  >   local F, IF, i, c;
  >   F := factors (eq);
  >   for i from 1 to nops(F[2]) do
  >     c := content (F[2][i][1]);
  >     F[2][i][1] := F[2][i][1] / c;
  >     F[1] := F[1] * c ^ F[2][i][2];
  >   od;
  >   IF := ifactors (F[1]);
  >   return (IF[1], [op(IF[2]), op(F[2])]);
  > end;

```

*efactors* := **proc**(eq)

**local** F, IF, i, c;

F := factors(eq);

**for** i **to** nops(F[2]) **do**

c := content(F[2][i][1]);

F[2][i][1] := F[2][i][1] / c;

F[1] := F[1]\*c^F[2][i][2]

**end do**;

IF := ifactors(F[1]);

**return** IF[1], [op(IF[2]), op(F[2])]

**end proc**

```

[ > psqf := proc (eq)
  >   local EF, S, i;
  >   EF := efactors (eq);
  >   S := EF[1];
  >   for i from 1 to nops(EF[2]) do
  >     if (EF[2][i][2] > 0) then
  >       S := S * EF[2][i][1]
  >     fi
  >   od;
  >   return S
  > end;

```

*psqf* := **proc**(eq)

**local** EF, S, i;

EF := efactors(eq);

S := EF[1];

**for** i **to** nops(EF[2]) **do** **if** 0 < EF[2][i][2] **then** S := S\*EF[2][i][1] **end if** **end do**;

**return** S

**end proc**

```

[ > initcases := proc ()
  >   global nz, NZ, SV;

```

```

>  if nargs = 0 then
>      nz := 1
>  else
>      nz := args[1];
>      printf ("We assume the following in our calculation:");
>      print (psqf (nz) <> 0);
>  fi;
>  NZ := [convert (nz,string)];
>  SV := [[]];
>  return
> end;

```

*initcases* := **proc**()

**global** *nz, NZ, SV*;

if nargs = 0 then *nz* := 1

else

*nz* := args[ 1 ];

printf("We assume the following in our calculation:");

print(psqf(*nz*) ≠ 0)

end if;

*NZ* := [convert(*nz*, *string*)];

*SV* := [[ ]];

return

**end proc**

> **launchNZcase** := **proc** (*nz*)

> **global** *NZ, SV*;

> **local** *t*;

> *NZ* := [seq(*NZ*[*i*], *i*=1..*nops*(*NZ*)), convert (*nz*,string)];

> *SV* := [seq(*SV*[*i*], *i*=1..*nops*(*SV*)), [ ]];

> printf ("Launching case level %d:", *nops*(*NZ*) - 1);

> print (*nz* <> 0);

> printf ("Assume from now on that:");

> *t* := mul (psqf (parse (*NZ*[*i*],statement)), *i*=1..*nops*(*NZ*));

> print (*t* <> 0)

> **end**;

*launchNZcase* := **proc**(*nz*)

**local** *t*;

**global** *NZ, SV*;

*NZ* := [seq(*NZ*[*i*], *i* = 1 .. *nops*(*NZ*)), convert(*nz*, *string*)];

*SV* := [seq(*SV*[*i*], *i* = 1 .. *nops*(*SV*)), [ ]];

printf("Launching case level %d:", *nops*(*NZ*) - 1);

print(*nz* ≠ 0);

printf("Assume from now on that:");

```

t := mul(psqf(parse(NZ[i], statement)), i = 1 .. nops(NZ));
print(t ≠ 0)

```

**end proc**

```

> contradict := proc (eq)
>   global NZ, SV, alph;
>   local t, EF, i, sv, nz;
>   t := mul (psqf (parse (NZ[i], statement)), i=1..nops(NZ));
>   EF := efactors (psqf (psqf (eq) / t));
>   if EF[1] = 0 or nops (EF[2]) > 0 then
>     error "No contradiction: 'eq' might be zero!"
>   fi;
>   printf ("Contradiction on case level %d, so:", nops(NZ) - 1);
>   for i from 1 to nops(SV[nops(SV)]) do
>     sv := cat (SV[nops(SV)][i], " := ");
>     sv := cat (sv, SV[nops(SV)][i], "");
>     parse (sv, statement)
>   od;
>   nz := parse (NZ[nops(NZ)], statement);
>   print (nz = 0);
>   if nops(SV[nops(SV)]) > 0 then
>     printf ("Variables to be uneliminated:");
>     for i from 1 to nops(SV[nops(SV)]) do
>       sv := cat (SV[nops(SV)][i], " := ");
>       sv := cat (sv, SV[nops(SV)][i], "");
>       print (sv);
>     od
>   fi;
>   if nops(NZ) <= 1 then
>     printf ("That is all, folks! ");
>     printf ("Check that all variables are uneliminated:");
>     print (alph);
>     return
>   fi;
>   NZ := [seq(NZ[i], i=1..nops(NZ)-1)];
>   SV := [seq(SV[i], i=1..nops(SV)-1)];
>   printf ("Proceed on case level %d with:", nops(NZ) - 1);
>   t := mul (psqf (parse (NZ[i], statement)), i=1..nops(NZ));
>   print (t <> 0);
>   printf ("On account of:");
>   print (nz = 0);
>   if nargs = 1 and nops(indets(nz)) = 1 and degree (nz) = 1 then
>     EF := efactors (psqf (psqf (coeff (nz, indets(nz)[1])) / t));
>     if nops (EF[2]) = 0 then
>       elimsolve(nz, indets(nz)[1]);
>       return
>     fi;
>   fi;

```

```

>   elif nargs > 1 then
>       elimsolve (nz, args[2]);
>       return
>   fi;
>   printf ("the following return value %s",
>           "can be used as an equation:");
>   return nz
> end;

contradict := proc(eq)
local t, EF, i, sv, nz;
global NZ, SV, alph;

    t := mul(psqf(parse(NZ[i], statement)), i = 1 .. nops(NZ));
    EF := efactors(psqf(psqf(eq) / t));
    if EF[1] = 0 or 0 < nops(EF[2]) then error "No contradiction: 'eq' might be zero!"
    end if;
    printf("Contradiction on case level %d, so:", nops(NZ) - 1);
    for i to nops(SV[nops(SV)]) do
        sv := cat(SV[nops(SV)][i], " := ");
        sv := cat(sv, SV[nops(SV)][i], "");
        parse(sv, statement)
    end do;
    nz := parse(NZ[nops(NZ)], statement);
    print(nz = 0);
    if 0 < nops(SV[nops(SV)]) then
        printf("Variables to be uneliminated:");
        for i to nops(SV[nops(SV)]) do
            sv := cat(SV[nops(SV)][i], " := ");
            sv := cat(sv, SV[nops(SV)][i], "");
            print(sv)
        end do
    end if;
    if nops(NZ) ≤ 1 then
        printf("That is all, folks! ");
        printf("Check that all variables are uneliminated:");
        print(alph);
        return
    end if;
    NZ := [seq(NZ[i], i = 1 .. nops(NZ) - 1)];
    SV := [seq(SV[i], i = 1 .. nops(SV) - 1)];
    printf("Proceed on case level %d with:", nops(NZ) - 1);

```

```

t := mul(psqf(parse(NZ[i], statement)), i = 1 .. nops(NZ));
print(t ≠ 0);
printf("On account of:");
print(nz = 0);
if nargs = 1 and nops(indets(nz)) = 1 and degree(nz) = 1 then
    EF := efactors(psqf(psqf(coeff(nz, indets(nz)[1])) / t));
    if nops(EF[2]) = 0 then elimsolve(nz, indets(nz)[1]); return end if
elif 1 < nargs then elimsolve(nz, args[2]); return
end if;
printf("the following return value %s", "can be used as an equation:");
return nz

```

**end proc**

```

> elimsolve := proc (eq, v)
>   global NZ, SV;
>   local t, EF, i, c1, c0, NZref, sv, F;
>   if not ({v} subset indets(v)) then
>     error "Second argument 'v' is not a variable!";
>   fi;
>   t := mul (psqf (parse (NZ[i], statement)), i=1..nops(NZ));
>   EF := efactors (psqf (psqf (eq) / t));
>   if EF[1] = 0 then error "First argument 'eq' is zero!" fi;
>   if nops(EF[2]) = 0 then
>     error "Contradiction: call 'contradict'!"
>   fi;
>   if nops(EF[2]) > 1 then
>     error "'eq' has different factors which may be zero!"
>   fi;
>   if degree (EF[2][1][1], v) <> 1 then
>     error "Degree of 'eq' w.r.t 'v' is not one!"
>   fi;
>   c1 := coeff(EF[2][1][1], v, 1);
>   c0 := coeff(EF[2][1][1], v, 0);
>   EF := efactors (psqf (psqf (c1) / t));
>   if nops(EF[2]) > 0 then
>     error "Coefficient of 'v' in 'eq' might be zero!"
>   fi;
>   EF := efactors (psqf (psqf (denom(eq)) / t));
>   if nops(EF[2]) > 0 then
>     error "Denominator of argument 'eq' may be zero!"
>   fi;
>   print ({c1 <> 0});
>   NZref := false;
>   for i from 1 to nops(NZ) do
>     NZref :=

```

```

>      NZref or ({v} subset indets (parse (NZ[i],statement)));
> od;
> sv := convert (v, string);
> F := factor (-c0/c1);
> SV[nops(SV)] :=
>   [sv, seq(SV[nops(SV)][i], i=1..nops(SV[nops(SV)]))];
> printf ("%s is set to:", sv);
> sv := cat (sv, " := ", convert (F, string));
> print (parse (sv,statement));
> if NZref then
>   printf ("Nonzero constraint refines to:");
>   t := mul (psqf (parse (NZ[i],statement)), i=1..nops (NZ));
>   print (t <> 0)
> fi;
> return
> end;

```

*elimsolve* := **proc**(eq, v)

**local** t, EF, i, c1, c0, NZref, sv, F;

**global** NZ, SV;

**if not** {v} subset indets(v) **then error** "Second argument 'v' is not a variable!" **end if**;

t := mul(psqf(parse(NZ[i], statement)), i = 1 .. nops(NZ));

EF := efactors(psqf(psqf(eq) / t));

**if** EF[1] = 0 **then error** "First argument 'eq' is zero!" **end if**;

**if** nops(EF[2]) = 0 **then error** "Contradiction: call 'contradict'!" **end if**;

**if** 1 < nops(EF[2]) **then error** "'eq' has different factors which may be zero!" **end if**;

**if** degree(EF[2][1][1], v) ≠ 1 **then error** "Degree of 'eq' w.r.t 'v' is not one!" **end if**;

c1 := coeff(EF[2][1][1], v, 1);

c0 := coeff(EF[2][1][1], v, 0);

EF := efactors(psqf(psqf(c1) / t));

**if** 0 < nops(EF[2]) **then error** "Coefficient of 'v' in 'eq' might be zero!" **end if**;

EF := efactors(psqf(psqf(denom(eq)) / t));

**if** 0 < nops(EF[2]) **then error** "Denominator of argument 'eq' may be zero!" **end if**;

print({c1 ≠ 0});

NZref := false;

**for** i **to** nops(NZ) **do** NZref := NZref or {v} subset indets(parse(NZ[i], statement))

**end do**;

sv := convert(v, string);

F := factor(-c0 / c1);

SV[nops(SV)] := [sv, seq(SV[nops(SV)][i], i = 1 .. nops(SV[nops(SV)]))];

printf ("%s is set to:", sv);

sv := cat(sv, " := ", convert(F, string));

```

print(parse(sv, statement));
if NZref then
    printf("Nonzero constraint refines to:");
    t := mul(psqf(parse(NZ[i], statement)), i = 1 .. nops(NZ));
    print(t ≠ 0)
end if;
return

```

end proc

```

> initcpcoeff := proc (cp)
>   global x1, x2, x3, x4, T, S, deg, n;
>   local i, j, k, l, m, cp1, cp2, cp3, cp4;
>   S := Array (0..(deg-1)*n, 0..(deg-1)*n, 0..(deg-1)*n,
>               0..(deg-1)*n, 0..n, storage=sparse);
>   for m from 0 to n-1 do
>       cp1 := coeff (cp, T, m);
>       for i from 0 to (deg-1)*(n-m) do
>           cp2 := coeff (cp1, x1, i);
>           for j from 0 to (deg-1)*(n-m)-i do
>               cp3 := coeff (cp2, x2, j);
>               for k from 0 to (deg-1)*(n-m)-i-j do
>                   cp4 := coeff (cp3, x3, k);
>                   l := (deg-1)*(n-m)-i-j-k;
>                   S[i,j,k,l,m] := coeff (cp4, x4, l);
>               od
>           od
>       od
>   od;
>   return;
> end;

```

initcpcoeff := proc(cp)

local i, j, k, l, m, cp1, cp2, cp3, cp4;

global x1, x2, x3, x4, T, S, deg, n;

S := Array(0 .. (deg - 1)\*n, 0 .. (deg - 1)\*n, 0 .. (deg - 1)\*n, 0 .. (deg - 1)\*n, 0 .. n,  
storage = sparse);

for m from 0 to n - 1 do

cp1 := coeff(cp, T, m);

for i from 0 to (deg - 1)\*(n - m) do

cp2 := coeff(cp1, x1, i);

for j from 0 to (deg - 1)\*(n - m) - i do

cp3 := coeff(cp2, x2, j);

for k from 0 to (deg - 1)\*(n - m) - i - j do

cp4 := coeff(cp3, x3, k);

```

        l := (deg - 1)*(n - m) - i - j - k;
        S[i,j,k,l,m] := coeff(cp4,x4,l)
    end do
end do
end do
end do;
return
end proc

```

```

> cpcoeff := proc (t)
>   global x1, x2, x3, x4, T, S;
>   local i, j, k, l, m;
>   i := degree (t, x1);
>   j := degree (t, x2);
>   k := degree (t, x3);
>   l := degree (t, x4);
>   m := degree (t, T);
>   factor (S[i,j,k,l,m]);
> end;

```

*cpcoeff* := **proc**(*t*)

**local** *i,j,k,l,m*;

**global** *x1,x2,x3,x4,T,S*;

*i* := degree(*t*,*x1*);

*j* := degree(*t*,*x2*);

*k* := degree(*t*,*x3*);

*l* := degree(*t*,*x4*);

*m* := degree(*t*,*T*);

factor(*S*[*i,j,k,l,m*])

**end proc**

```

> startnewHcase := proc()
>   global remainingHcases, H, JH, cp, n;
>   local i;
>   if remainingHcases = [] then
>     printf ("No cases for H remaining; %s",
>             "all cases have been evaluated.");
>     return
>   fi;
>   printf ("Starting case H = %s:", remainingHcases[1]);
>   H := parse (remainingHcases[1]):
>   print (H):
>   remainingHcases := [seq(remainingHcases[i],
>                           i=2..nops(remainingHcases))]:
>   JH := jacobian (H,[x1,x2,x3,x4]):
>   cp := expand (det (T-JH)-T^n):

```



```

> initpccoeff (cp);
> end;

startnewHcase := proc()
local i;
global remainingHcases, H, JH, cp, n;
  if remainingHcases = [ ] then
    printf("No cases for H remaining; %s", "all cases have been evaluated."); return
  end if;
  printf("Starting case H = %s:", remainingHcases[1]);
  H := parse(remainingHcases[1]);
  print(H);
  remainingHcases := [ seq(remainingHcases[i], i = 2 .. nops(remainingHcases)) ];
  JH := jacobian(H, [x1, x2, x3, x4]);
  cp := expand(det(T - JH) - T^n);
  initpccoeff(cp)
end proc

> n := 4;
                                     n := 4

> deg := 3;
                                     deg := 3

> alph :=
> [[a1,b1,c1,d1,e1,f1,g1,h1,i1,j1,k1,l1,m1,n1,o1,p1,q1,r1,s1,t1],
> [a2,b2,c2,d2,e2,f2,g2,h2,i2,j2,k2,l2,m2,n2,o2,p2,q2,r2,s2,t2],
> [a3,b3,c3,d3,e3,f3,g3,h3,i3,j3,k3,l3,m3,n3,o3,p3,q3,r3,s3,t3],
> [a4,b4,c4,d4,e4,f4,g4,h4,i4,j4,k4,l4,m4,n4,o4,p4,q4,r4,s4,t4]];
alph := [[a1,b1,c1,d1,e1,f1,g1,h1,i1,j1,k1,l1,m1,n1,o1,p1,q1,r1,s1,t1],
[a2,b2,c2,d2,e2,f2,g2,h2,i2,j2,k2,l2,m2,n2,o2,p2,q2,r2,s2,t2],
[a3,b3,c3,d3,e3,f3,g3,h3,i3,j3,k3,l3,m3,n3,o3,p3,q3,r3,s3,t3],
[a4,b4,c4,d4,e4,f4,g4,h4,i4,j4,k4,l4,m4,n4,o4,p4,q4,r4,s4,t4]]

> terms :=
[x1^3,x1^2*x2,x1^2*x3,x1^2*x4,x1*x2^2,x1*x2*x3,x1*x2*x4,
> x1*x3^2,x1*x3*x4,x1*x4^2,x2^3,x2^2*x3,x2^2*x4,x2*x3^2,
> x2*x3*x4,x2*x4^2,x3^3,x3^2*x4,x3*x4^2,x4^3];
terms := [x1^3,x1^2 x2,x1^2 x3,x1^2 x4,x1 x2^2,x1 x2 x3,x1 x2 x4,x1 x3^2,x1 x3 x4,x1 x4^2,x2^3,
x2^2 x3,x2^2 x4,x2 x3^2,x2 x3 x4,x2 x4^2,x3^3,x3^2 x4,x3 x4^2,x4^3]

> M1 := evalm ([[0,0,0,0],[1,0,0,0],[0,1,0,0],[0,0,1,0]]);
                                     
$$M1 := \begin{bmatrix} 0 & 0 & 0 & 0 \\ 1 & 0 & 0 & 0 \\ 0 & 1 & 0 & 0 \\ 0 & 0 & 1 & 0 \end{bmatrix}$$


> H1 := Vector (evalm (M1 & [seq(terms[k]/degree(terms[k]),

```

```

>                                     [x1,x2,x3,x4][k]),k=1..n)] +
> ['add (alph[1,k]*terms[k],k=n+1..nops(terms))'$1=1..n))];

H1 := [ e1 x1 x2^2 + f1 x1 x2 x3 + g1 x1 x2 x4 + h1 x1 x3^2 + i1 x1 x3 x4 + j1 x1 x4^2 + k1 x2^3
+ l1 x2^2 x3 + m1 x2^2 x4 + n1 x2 x3^2 + o1 x2 x3 x4 + p1 x2 x4^2 + q1 x3^3 + r1 x3^2 x4 + s1 x3 x4^2
+ t1 x4^3, x1^3/3 + e2 x1 x2^2 + f2 x1 x2 x3 + g2 x1 x2 x4 + h2 x1 x3^2 + i2 x1 x3 x4 + j2 x1 x4^2
+ k2 x2^3 + l2 x2^2 x3 + m2 x2^2 x4 + n2 x2 x3^2 + o2 x2 x3 x4 + p2 x2 x4^2 + q2 x3^3 + r2 x3^2 x4
+ s2 x3 x4^2 + t2 x4^3, x1^2 x2 + e3 x1 x2^2 + f3 x1 x2 x3 + g3 x1 x2 x4 + h3 x1 x3^2 + i3 x1 x3 x4
+ j3 x1 x4^2 + k3 x2^3 + l3 x2^2 x3 + m3 x2^2 x4 + n3 x2 x3^2 + o3 x2 x3 x4 + p3 x2 x4^2 + q3 x3^3
+ r3 x3^2 x4 + s3 x3 x4^2 + t3 x4^3, x1^2 x3 + e4 x1 x2^2 + f4 x1 x2 x3 + g4 x1 x2 x4 + h4 x1 x3^2
+ i4 x1 x3 x4 + j4 x1 x4^2 + k4 x2^3 + l4 x2^2 x3 + m4 x2^2 x4 + n4 x2 x3^2 + o4 x2 x3 x4
+ p4 x2 x4^2 + q4 x3^3 + r4 x3^2 x4 + s4 x3 x4^2 + t4 x4^3 ]

> M2 := evalm ([ [0,0,0,1], [1,0,0,0], [0,1,0,0], [0,0,0,0] ]);

M2 := [ 0  0  0  1
        1  0  0  0
        0  1  0  0
        0  0  0  0 ]

> H2 := Vector (evalm (M2 &* [seq(terms[k]/degree(terms[k]),
>                                     [x1,x2,x3,x4][k]),k=1..n)] +
> ['add (alph[1,k]*terms[k],k=n+1..nops(terms))'$1=1..n))];

H2 := [ x1^2 x4 + e1 x1 x2^2 + f1 x1 x2 x3 + g1 x1 x2 x4 + h1 x1 x3^2 + i1 x1 x3 x4 + j1 x1 x4^2
+ k1 x2^3 + l1 x2^2 x3 + m1 x2^2 x4 + n1 x2 x3^2 + o1 x2 x3 x4 + p1 x2 x4^2 + q1 x3^3 + r1 x3^2 x4
+ s1 x3 x4^2 + t1 x4^3, x1^3/3 + e2 x1 x2^2 + f2 x1 x2 x3 + g2 x1 x2 x4 + h2 x1 x3^2 + i2 x1 x3 x4
+ j2 x1 x4^2 + k2 x2^3 + l2 x2^2 x3 + m2 x2^2 x4 + n2 x2 x3^2 + o2 x2 x3 x4 + p2 x2 x4^2 + q2 x3^3
+ r2 x3^2 x4 + s2 x3 x4^2 + t2 x4^3, x1^2 x2 + e3 x1 x2^2 + f3 x1 x2 x3 + g3 x1 x2 x4 + h3 x1 x3^2
+ i3 x1 x3 x4 + j3 x1 x4^2 + k3 x2^3 + l3 x2^2 x3 + m3 x2^2 x4 + n3 x2 x3^2 + o3 x2 x3 x4
+ p3 x2 x4^2 + q3 x3^3 + r3 x3^2 x4 + s3 x3 x4^2 + t3 x4^3, e4 x1 x2^2 + f4 x1 x2 x3 + g4 x1 x2 x4
+ h4 x1 x3^2 + i4 x1 x3 x4 + j4 x1 x4^2 + k4 x2^3 + l4 x2^2 x3 + m4 x2^2 x4 + n4 x2 x3^2
+ o4 x2 x3 x4 + p4 x2 x4^2 + q4 x3^3 + r4 x3^2 x4 + s4 x3 x4^2 + t4 x4^3 ]

> remainingHcases := ["H1", "H2"];
remainingHcases := ["H1", "H2"]

> with (linalg):
Warning, the protected names norm and trace have been redefined and
unprotected

```

```
> startnewHcase ();
```

Starting case H = H1:

$$\left[ \begin{aligned} &e1 x1 x2^2 + f1 x1 x2 x3 + g1 x1 x2 x4 + h1 x1 x3^2 + i1 x1 x3 x4 + j1 x1 x4^2 + k1 x2^3 + l1 x2^2 x3 \\ &+ m1 x2^2 x4 + n1 x2 x3^2 + o1 x2 x3 x4 + p1 x2 x4^2 + q1 x3^3 + r1 x3^2 x4 + s1 x3 x4^2 + t1 x4^3, \\ &\frac{x1^3}{3} + e2 x1 x2^2 + f2 x1 x2 x3 + g2 x1 x2 x4 + h2 x1 x3^2 + i2 x1 x3 x4 + j2 x1 x4^2 + k2 x2^3 \\ &+ l2 x2^2 x3 + m2 x2^2 x4 + n2 x2 x3^2 + o2 x2 x3 x4 + p2 x2 x4^2 + q2 x3^3 + r2 x3^2 x4 + s2 x3 x4^2 \\ &+ t2 x4^3, x1^2 x2 + e3 x1 x2^2 + f3 x1 x2 x3 + g3 x1 x2 x4 + h3 x1 x3^2 + i3 x1 x3 x4 + j3 x1 x4^2 \\ &+ k3 x2^3 + l3 x2^2 x3 + m3 x2^2 x4 + n3 x2 x3^2 + o3 x2 x3 x4 + p3 x2 x4^2 + q3 x3^3 + r3 x3^2 x4 \\ &+ s3 x3 x4^2 + t3 x4^3, x1^2 x3 + e4 x1 x2^2 + f4 x1 x2 x3 + g4 x1 x2 x4 + h4 x1 x3^2 + i4 x1 x3 x4 \\ &+ j4 x1 x4^2 + k4 x2^3 + l4 x2^2 x3 + m4 x2^2 x4 + n4 x2 x3^2 + o4 x2 x3 x4 + p4 x2 x4^2 + q4 x3^3 \\ &+ r4 x3^2 x4 + s4 x3 x4^2 + t4 x4^3 \end{aligned} \right]$$

```
> initcases (6);
```

We assume the following in our calculation:

$$6 \neq 0$$

```
> for i from 1 by -1 to 0 do
```

```
>   for j from 2-i by -1 to 0 do
```

```
>     for k from 2-i-j by -1 to 0 do
```

```
>       v := coeff (coeff (coeff (coeff (H[4],
```

```
>                                     x1,i),x2,j),x3,k),x4,3-i-j-k);
```

```
>       m := cpcoeff (x1^i * x2^j * x3^k * x4^(2-i-j-k) * T^3);
```

```
>       elimsolve (m,v);
```

```
>     od;
```

```
>   od;
```

```
> od;
```

$$\{1 \neq 0\}$$

g4 is set to:

$$-2 e2 - f3$$

$$\{1 \neq 0\}$$

i4 is set to:

$$-2 h3 - f2$$

$$\{2 \neq 0\}$$

j4 is set to:

$$-\frac{g2}{2} - \frac{i3}{2}$$

$$\{1 \neq 0\}$$

m4 is set to:

$$-l3 - e1 - 3 k2$$

$$\{1 \neq 0\}$$

o4 is set to:

$$\begin{aligned} & -2\,n3 - 2\,l2 - f1 \\ & \{2 \neq 0\} \end{aligned}$$

p4 is set to:

$$\begin{aligned} & -m2 - \frac{gl}{2} - \frac{o3}{2} \\ & \{1 \neq 0\} \end{aligned}$$

r4 is set to:

$$\begin{aligned} & -h1 - n2 - 3\,q3 \\ & \{2 \neq 0\} \end{aligned}$$

s4 is set to:

$$\begin{aligned} & -r3 - \frac{i1}{2} - \frac{o2}{2} \\ & \{3 \neq 0\} \end{aligned}$$

t4 is set to:

$$-\frac{p2}{3} - \frac{j1}{3} - \frac{s3}{3}$$

```
> for i from 1 by -1 to 0 do
>   for j from 2-i by -1 to 0 do
>     for k from 2-i-j by -1 to 0 do
>       v := coeff (coeff (coeff (coeff (H[3],
>                                     x1,i),x2,j),x3,k),x4,3-i-j-k);
>       m := cpcoeff (x1^(i+2) * x2^j * x3^k * x4^(2-i-j-k) *
> T^2);
>       elimsolve (m,v);
>     od;
>   od;
> od;
```

$$\{1 \neq 0\}$$

g3 is set to:

$$\begin{aligned} & -2\,e1 - f2 \\ & \{1 \neq 0\} \end{aligned}$$

i3 is set to:

$$\begin{aligned} & -f1 - 2\,h2 \\ & \{2 \neq 0\} \end{aligned}$$

j3 is set to:

$$\begin{aligned} & -\frac{gl}{2} - \frac{i2}{2} \\ & \{-1 \neq 0\} \end{aligned}$$

m3 is set to:

$$\begin{aligned} & -l2 - 4\,e2^2 - 2\,e2\,f3 + 2\,e1\,f4 + f4\,f2 - f3^2 - 3\,k1 - 2\,f1 - 2\,f2\,e3 - 2\,e4\,g2 \\ & \{-1 \neq 0\} \end{aligned}$$

o3 is set to:

$$\begin{aligned} & -f4\,g2 - 4\,f2\,e2 - 2\,f2\,f3 + f4\,f1 + 2\,h2\,f4 - 4\,h3\,e2 - 4\,h3\,f3 - 4\,h2\,e3 - 2\,e4\,i2 - 4\,h1 - 2\,gl \\ & - 2\,n2 - 2\,l1 + 4\,h4\,e1 + 2\,h4\,f2 \end{aligned}$$

$$\{2 \neq 0\}$$

p3 is set to:

$$\frac{f4 \, i2}{2} - i1 - m1 - \frac{o2}{2} + 2 \, e2 \, h2 - e3 \, i2 + f1 \, f3 - e2 \, g2 + \frac{f4 \, g1}{2} - 2 \, e1 \, h3 + f1 \, e2 + 2 \, h2 \, f3 - h3 \, f2 - 2 \, e4 \, j2$$

$$\{-1 \neq 0\}$$

r3 is set to:

$$-n1 - 2 \, i1 - 2 \, h3 \, f2 - f2^2 + 2 \, h4 \, f1 + 4 \, h4 \, h2 - 4 \, h3^2 - 3 \, q2 - 2 \, h2 \, f3 - f4 \, i2$$

$$\{-2 \neq 0\}$$

s3 is set to:

$$-r2 - \frac{o1}{2} - f4 \, j2 + i2 \, e2 - h3 \, g2 + f1 \, h3 + 2 \, h3 \, h2 - f2 \, g2 + f2 \, h2 + g1 \, h4 + i2 \, h4 - 2 \, j1 + 2 \, h2 \, e1$$

$$\{-3 \neq 0\}$$

t3 is set to:

$$-\frac{p1}{3} - \frac{s2}{3} - \frac{g2^2}{3} + \frac{f1 \, g2}{3} + \frac{2 \, g2 \, h2}{3} - \frac{2 \, h3 \, g1}{3} - \frac{f2 \, g1}{3} - \frac{2 \, i2 \, h3}{3} - \frac{f1^2}{3} - \frac{4 \, f1 \, h2}{3} - \frac{4 \, h2^2}{3} + \frac{2 \, e1 \, i2}{3} + \frac{4 \, j2 \, e2}{3} + \frac{2 \, f3 \, j2}{3}$$

```
> for i from 1 by -1 to 0 do
>   for j from 2-i by -1 to 0 do
>     for k from 2-i-j by -1 to 0 do
>       v := coeff (coeff (coeff (coeff (H[2],
>                                     x1,i),x2,j),x3,k),x4,3-i-j-k);
>       m := cpcoeff (x1^(i+4) * x2^j * x3^k * x4^(2-i-j-k) * T);
>       elimsolve (m,v);
>     od;
>   od;
> od;
```

$$\{1 \neq 0\}$$

g2 is set to:

$$-f1$$

$$\{1 \neq 0\}$$

i2 is set to:

$$-2 \, h1$$

$$\{2 \neq 0\}$$

j2 is set to:

$$-\frac{i1}{2}$$

$$\{1 \neq 0\}$$

m2 is set to:

$$-2 \, g1 - l1 - 8 \, e1 \, e2 - 4 \, f2 \, e2 - 2 \, e4 \, g1 + f4 \, f1 - f2 \, f3$$

$$\{1 \neq 0\}$$

o2 is set to:

$$-2\,il - 2\,e4\,il - 4\,fl\,e2 - 8\,e2\,h2 - 2\,nl - 2\,h3\,f2 - 2\,f2^2 - 4\,e1\,f2 + 2\,h4\,fl - 2\,h2\,f3 \\ + 2\,f4\,hl - f4\,gl$$

$$\{-2 \neq 0\}$$

p2 is set to:

$$-2\,e4\,jl + 2\,e1\,fl - e2\,gl + 4\,hl\,e2 - \frac{ol}{2} + \frac{f3\,gl}{2} + f2\,fl - 2\,jl - fl\,h3 + f2\,h2 + hl\,f3 + \frac{f4\,il}{2}$$

$$\{1 \neq 0\}$$

r2 is set to:

$$-3\,ql - f4\,il - 2\,f2\,fl + 4\,hl\,h4 - 4\,h3\,h2 - 4\,f2\,h2$$

$$\{-2 \neq 0\}$$

s2 is set to:

$$-r1 - f2\,gl + hl\,f2 + 3\,fl\,h2 + 2\,h2^2 + il\,h4 + fl^2 - f4\,jl + e2\,il + \frac{f3\,il}{2}$$

$$\{-3 \neq 0\}$$

t2 is set to:

$$-\frac{sl}{3} + \frac{4\,e2\,jl}{3} + \frac{2\,f3\,jl}{3} + \frac{2\,gl\,fl}{3} - \frac{2\,h3\,il}{3} - \frac{f2\,il}{3} - 2\,hl\,fl - \frac{4\,hl\,h2}{3}$$

```
> for i from 1 by -1 to 0 do
>   for j from 2-i by -1 to 0 do
>     for k from 2-i-j by -1 to 0 do
>       v := coeff (coeff (coeff (coeff (H[1],
>                                     x1,i),x2,j),x3,k),x4,3-i-j-k);
>       m := cpcoeff (x1^(i+6) * x2^j * x3^k * x4^(2-i-j-k));
>       elimsolve (m,v);
>     od;
>   od;
> od;
```

$$\{1 \neq 0\}$$

g1 is set to:

$$0$$

$$\{1 \neq 0\}$$

i1 is set to:

$$0$$

$$\{1 \neq 0\}$$

j1 is set to:

$$0$$

$$\{1 \neq 0\}$$

m1 is set to:

$$-4\,el^2 - 2\,el\,f2 - 2\,fl\,e2 - fl\,f3$$

$$\{1 \neq 0\}$$

o1 is set to:

$$-4\,el\,fl - 2\,f2\,fl - 4\,h2\,el - 2\,fl\,h3 - 4\,hl\,e2 - 2\,hl\,f3$$

$$\{-1 \neq 0\}$$

p1 is set to:

```

                                
$$2 e1 h1 + f1^2 + f1 h2$$

                                
$$\{1 \neq 0\}$$

r1 is set to:

                                
$$-f1^2 - 2 f1 h2 - 4 h1 h3 - 2 h1 f2$$

                                
$$\{-1 \neq 0\}$$

s1 is set to:

                                
$$h1 (3 f1 + 2 h2)$$

                                
$$\{1 \neq 0\}$$

t1 is set to:

                                
$$0$$

> launchNZcase (h1);
Launching case level 1:

                                
$$h1 \neq 0$$

Assume from now on that:

                                
$$6 h1 \neq 0$$

> tmp1 := cpcoeff (x1^5*x4^3);
                                
$$tmp1 := 4 h1 (e1 h1 + 2 f1^2 + 3 f1 h2 + h2^2)$$

> elimsolve (tmp1, e1);
                                
$$\{h1 \neq 0\}$$

e1 is set to:

                                
$$-\frac{(f1 + h2)(2 f1 + h2)}{h1}$$

> tmp1 := cpcoeff (x1^5*x3*x4^2);
                                
$$tmp1 := -24 f1 h3 h1 - 24 h3 h2 h1 - 18 f2 h2 h1 - 24 f2 f1 h1 + 12 h1^2 h4 - 6 q1 h1$$

                                
$$- 6 h1^2 f3 - 12 h1^2 e2 + 84 f1 h2^2 + 99 f1^2 h2 + 39 f1^3 + 24 h2^3$$

> elimsolve (tmp1, q1);
                                
$$\{-2 h1 \neq 0\}$$

q1 is set to:
                                
$$(-8 f1 h3 h1 - 8 h3 h2 h1 - 6 f2 h2 h1 - 8 f2 f1 h1 + 4 h1^2 h4 - 2 h1^2 f3 - 4 h1^2 e2 + 28 f1 h2^2$$

                                
$$+ 33 f1^2 h2 + 13 f1^3 + 8 h2^3) / (2 h1)$$

> tmp1 := cpcoeff (x1^5*x3^2*x4);
                                
$$tmp1 := (16 h2^4 + 66 f1^4 - 56 f1 h3 h1 h2 - 70 f2 h2 h1 f1 - 12 h1^2 h4 h2 - 54 f2 f1^2 h1$$

                                
$$- 26 f2 h2^2 h1 - 24 h3 h2^2 h1 - 42 f1^2 h3 h1 + 6 h1^2 h2 f3 + 4 h1^2 e2 h2 - 12 h1^2 f1 f3$$

                                
$$- 16 h1^2 f1 e2 - 8 f1 h1^2 h4 + 20 h3 f2 h1^2 - 16 h1^3 f4 + 10 n1 h1^2 + 187 f1^3 h2 + 92 f1 h2^3$$

                                
$$+ 197 f1^2 h2^2 + 10 f2^2 h1^2 + 24 h3^2 h1^2 + 12 h1^2 q2) / h1$$

> elimsolve (tmp1, q2);
                                
$$\{12 h1^2 \neq 0\}$$

q2 is set to:
                                
$$-(16 h2^4 + 66 f1^4 - 56 f1 h3 h1 h2 - 70 f2 h2 h1 f1 - 12 h1^2 h4 h2 - 54 f2 f1^2 h1$$

                                
$$- 26 f2 h2^2 h1 - 24 h3 h2^2 h1 - 42 f1^2 h3 h1 + 6 h1^2 h2 f3 + 4 h1^2 e2 h2 - 12 h1^2 f1 f3$$

                                
$$- 16 h1^2 f1 e2 - 8 f1 h1^2 h4 + 20 h3 f2 h1^2 - 16 h1^3 f4 + 10 n1 h1^2 + 187 f1^3 h2 + 92 f1 h2^3$$


```

$$+ 197 f l^2 h^2 + 10 f^2 h l^2 + 24 h^3 h l^2) / (12 h l^2)$$

> **tmp1 := cpcoeff (x1^5\*x3^3);**

$$\begin{aligned} \text{tmp1} := & (4 f l h l^2 e_2 h_2 + 6 f l h l^2 h_2 f_3 + 120 h_3 h_2 h l^2 f_2 - 194 h l f l h_2^2 f_2 \\ & - 452 h l f l^2 h_2 h_3 - 268 h l f l^2 h_2 f_2 - 360 h l f l h_2^2 h_3 + 164 f l h_3 h l^2 f_2 + 16 h l^4 \\ & - 16 h l^2 f l^2 e_2 - 8 h l^2 f l^2 f_3 - 48 h l h_2^3 f_2 - 96 h l h_2^3 h_3 - 132 h l f l^3 f_2 - 198 h l f l^3 h_3 \\ & + 24 h l^3 e_2 f_2 + 48 h l^3 e_2 h_3 + 12 h l^3 f_3 f_2 + 24 h l^3 f_3 h_3 - 8 h l^3 h_4 f_2 - 16 h l^3 h_4 h_3 \\ & + 54 f_2^2 f l h l^2 + 36 f_2^2 h_2 h l^2 + 96 h_3^2 h_2 h l^2 + 120 f l h_3^2 h l^2 + 16 h l^3 f_4 h_2 - 8 n l h l^2 h_2 \\ & + 2 f l n l h l^2 - 24 h l^3 q_3 - 8 h l^3 n_2 + 16 f l h_2^4 + 197 f l^3 h_2^2 + 92 f l^2 h_2^3 + 187 f l^4 h_2 \\ & + 66 f l^5 + 4 f l h l^2 h_4 h_2) / (4 h l^2) \end{aligned}$$

> **elimsolve (tmp1, q3);**

$$\{-24 h l^3 \neq 0\}$$

q3 is set to:

$$\begin{aligned} & (4 f l h l^2 e_2 h_2 + 6 f l h l^2 h_2 f_3 + 120 h_3 h_2 h l^2 f_2 - 194 h l f l h_2^2 f_2 - 452 h l f l^2 h_2 h_3 \\ & - 268 h l f l^2 h_2 f_2 - 360 h l f l h_2^2 h_3 + 164 f l h_3 h l^2 f_2 + 16 h l^4 - 16 h l^2 f l^2 e_2 - 8 h l^2 f l^2 f_3 \\ & - 48 h l h_2^3 f_2 - 96 h l h_2^3 h_3 - 132 h l f l^3 f_2 - 198 h l f l^3 h_3 + 24 h l^3 e_2 f_2 + 48 h l^3 e_2 h_3 \\ & + 12 h l^3 f_3 f_2 + 24 h l^3 f_3 h_3 - 8 h l^3 h_4 f_2 - 16 h l^3 h_4 h_3 + 54 f_2^2 f l h l^2 + 36 f_2^2 h_2 h l^2 \\ & + 96 h_3^2 h_2 h l^2 + 120 f l h_3^2 h l^2 + 16 h l^3 f_4 h_2 - 8 n l h l^2 h_2 + 2 f l n l h l^2 - 8 h l^3 n_2 \\ & + 16 f l h_2^4 + 197 f l^3 h_2^2 + 92 f l^2 h_2^3 + 187 f l^4 h_2 + 66 f l^5 + 4 f l h l^2 h_4 h_2) / (24 h l^3) \end{aligned}$$

> **tmp1 := cpcoeff (x1^3\*x4^3\*T);**

$$\begin{aligned} \text{tmp1} := & -24 f l h_3 h l - 16 h_3 h_2 h l - 4 f_2 h_2 h l - 8 f_2 f l h l + 4 h l^2 e_2 + 28 f l h_2^2 + 16 f l^2 h_2 \\ & + 12 h_2^3 \end{aligned}$$

> **elimsolve (tmp1, e2);**

$$\{h l^2 \neq 0\}$$

e2 is set to:

$$-\frac{-6 f l h_3 h l - 4 h_3 h_2 h l - f_2 h_2 h l - 2 f_2 f l h l + 7 f l h_2^2 + 4 f l^2 h_2 + 3 h_2^3}{h l^2}$$

> **tmp1 := cpcoeff (x1^3\*x3\*x4^2\*T);**

$$\begin{aligned} \text{tmp1} := & -3 (44 h_2^4 + 40 f l^4 - 120 f l h_3 h l h_2 - 74 f_2 h_2 h l f l - 4 h l^2 h_4 h_2 - 52 f_2 f l^2 h l \\ & - 22 f_2 h_2^2 h l - 40 h_3 h_2^2 h l - 82 f l^2 h_3 h l - 6 h l^2 h_2 f_3 - 8 h l^2 f l f_3 - 8 f l h l^2 h_4 \\ & - 4 h_3 f_2 h l^2 - 4 h l^3 f_4 + 2 n l h l^2 + 179 f l^3 h_2 + 184 f l h_2^3 + 279 f l^2 h_2^2 + 2 f_2^2 h l^2 \\ & - 8 h_3^2 h l^2) / (2 h l) \end{aligned}$$

> **elimsolve (tmp1, n1);**

$$\{2 h l^2 \neq 0\}$$

n1 is set to:

$$\begin{aligned} & - (44 h_2^4 + 40 f l^4 - 120 f l h_3 h l h_2 - 74 f_2 h_2 h l f l - 4 h l^2 h_4 h_2 - 52 f_2 f l^2 h l \\ & - 22 f_2 h_2^2 h l - 40 h_3 h_2^2 h l - 82 f l^2 h_3 h l - 6 h l^2 h_2 f_3 - 8 h l^2 f l f_3 - 8 f l h l^2 h_4 \\ & - 4 h_3 f_2 h l^2 - 4 h l^3 f_4 + 179 f l^3 h_2 + 184 f l h_2^3 + 279 f l^2 h_2^2 + 2 f_2^2 h l^2 - 8 h_3^2 h l^2) / (2 \\ & h l^2) \end{aligned}$$



> **tmp1 := cpccoeff (x1^3\*x3^2\*x4\*T) ;**

$$\begin{aligned} \text{tmp1} := & -(4 f1 h1^3 f4 + 14 f1^2 h1^2 h4 + 8 h1^2 h4 h2^2 - 2 f1 h1^2 h2 f3 + 200 h3 h2 h1^2 f2 \\ & - 404 h1 f1 h2^2 f2 - 604 h1 f1^2 h2 h3 - 371 h1 f1^2 h2 f2 - 628 h1 f1 h2^2 h3 + 300 f1 h3 h1^2 f2 \\ & + 10 h1^4 - 142 h1 h2^3 f2 - 208 h1 h2^3 h3 - 100 h1 f1^3 f2 - 170 h1 f1^3 h3 + 12 h1^3 f3 f2 \\ & + 12 h1^3 f3 h3 + 4 h1^3 h4 f2 + 8 h1^3 h4 h3 + 88 f2^2 f1 h1^2 + 50 f2^2 h2 h1^2 + 160 h3^2 h2 h1^2 \\ & + 224 f1 h3^2 h1^2 + 6 h1^3 f4 h2 - 2 h1^3 n2 + 276 f1 h2^4 + 439 f1^3 h2^2 + 510 f1^2 h2^3 + 175 f1^4 h2 \\ & + 56 h2^5 + 26 f1^5 + 24 f1 h1^2 h4 h2) / h1^2 \end{aligned}$$

> **elimsolve (tmp1, n2) ;**

$$\{-2 h1^3 \neq 0\}$$

n2 is set to:

$$\begin{aligned} & (4 f1 h1^3 f4 + 14 f1^2 h1^2 h4 + 8 h1^2 h4 h2^2 - 2 f1 h1^2 h2 f3 + 200 h3 h2 h1^2 f2 \\ & - 404 h1 f1 h2^2 f2 - 604 h1 f1^2 h2 h3 - 371 h1 f1^2 h2 f2 - 628 h1 f1 h2^2 h3 + 300 f1 h3 h1^2 f2 \\ & + 10 h1^4 - 142 h1 h2^3 f2 - 208 h1 h2^3 h3 - 100 h1 f1^3 f2 - 170 h1 f1^3 h3 + 12 h1^3 f3 f2 \\ & + 12 h1^3 f3 h3 + 4 h1^3 h4 f2 + 8 h1^3 h4 h3 + 88 f2^2 f1 h1^2 + 50 f2^2 h2 h1^2 + 160 h3^2 h2 h1^2 \\ & + 224 f1 h3^2 h1^2 + 6 h1^3 f4 h2 + 276 f1 h2^4 + 439 f1^3 h2^2 + 510 f1^2 h2^3 + 175 f1^4 h2 + 56 h2^5 \\ & + 26 f1^5 + 24 f1 h1^2 h4 h2) / (2 h1^3) \end{aligned}$$

> **tmp1 := cpccoeff (x1^3\*x3^3\*T) ;**

$$\begin{aligned} \text{tmp1} := & (-400 h1 h3 h2^4 + 6 f1^2 h1^3 f4 - 50 f1^3 h1^2 h4 + 20 h1^4 h2 + 1344 f1^4 h2^2 \\ & + 2263 f1^3 h2^3 + 415 f1^5 h2 + 1012 f1 h2^5 + 2094 f1^2 h2^4 + 8 h1^4 f1 - 12 h1^4 q4 \\ & + 256 h1^2 h3^2 h2^2 + 648 f1 h3 h2 h1^2 f2 + 200 h2^6 - 64 h1^3 h3^3 - 4 f1^2 h1^2 h2 f3 + 52 f1^6 \\ & - 8 h1^4 h4^2 - 2 f2^3 h1^3 - 4 f4 h1^4 h3 + 12 f3 h1^4 h4 - 88 h3^2 f2 h1^3 - 32 h3 f2^2 h1^3 \\ & + 4 h1^3 f4 h2^2 - 146 h1 f1^4 f2 - 206 h1 f1^4 h3 + 106 f2^2 f1^2 h1^2 + 176 f1^2 h3^2 h1^2 \\ & - 112 h1^2 h4 h2^3 - 260 h1 h2^4 f2 + 90 f2^2 h2^2 h1^2 - 12 h1^2 f3 h2^3 - 4 h1^4 f4 f2 \\ & + 48 h1^3 h4 f2 h2 + 80 h1^3 h4 f2 f1 + 6 h2 f3 h1^3 f2 - 1259 h1 f1^2 h2^2 f2 + 14 h1^3 f4 h2 f1 \\ & - 712 h1 f1^3 h2 f2 - 1010 h1 f1^3 h2 h3 - 14 f1 h1^2 h2^2 f3 - 214 f1^2 h1^2 h4 h2 \\ & + 318 f1^2 h3 h1^2 f2 - 1808 h1 f1^2 h2^2 h3 - 1424 f1 h1 h2^3 h3 - 968 f1 h1 h2^3 f2 \\ & - 284 f1 h1^2 h4 h2^2 + 176 f1 h1^3 h4 h3 - 4 f1 h1^3 f3 h3 + 8 f1 h1^3 f3 f2 + 324 h1^2 h3 f2 h2^2 \\ & + 128 h1^3 h3 h4 h2 + 472 f1 h3^2 h2 h1^2 + 182 f1 f2^2 h2 h1^2) / (2 h1^3) \end{aligned}$$

> **elimsolve (tmp1, q4) ;**

$$\{-12 h1^4 \neq 0\}$$

q4 is set to:

$$\begin{aligned} & (-400 h1 h3 h2^4 + 6 f1^2 h1^3 f4 - 50 f1^3 h1^2 h4 + 20 h1^4 h2 + 1344 f1^4 h2^2 + 2263 f1^3 h2^3 \\ & + 415 f1^5 h2 + 1012 f1 h2^5 + 2094 f1^2 h2^4 + 8 h1^4 f1 + 256 h1^2 h3^2 h2^2 + 648 f1 h3 h2 h1^2 f2 \\ & + 200 h2^6 - 64 h1^3 h3^3 - 4 f1^2 h1^2 h2 f3 + 52 f1^6 - 8 h1^4 h4^2 - 2 f2^3 h1^3 - 4 f4 h1^4 h3 \\ & + 12 f3 h1^4 h4 - 88 h3^2 f2 h1^3 - 32 h3 f2^2 h1^3 + 4 h1^3 f4 h2^2 - 146 h1 f1^4 f2 - 206 h1 f1^4 h3 \\ & + 106 f2^2 f1^2 h1^2 + 176 f1^2 h3^2 h1^2 - 112 h1^2 h4 h2^3 - 260 h1 h2^4 f2 + 90 f2^2 h2^2 h1^2 \\ & - 12 h1^2 f3 h2^3 - 4 h1^4 f4 f2 + 48 h1^3 h4 f2 h2 + 80 h1^3 h4 f2 f1 + 6 h2 f3 h1^3 f2 \end{aligned}$$

$$\begin{aligned}
& -1259 h1 f1^2 h2^2 f2 + 14 h1^3 f4 h2 f1 - 712 h1 f1^3 h2 f2 - 1010 h1 f1^3 h2 h3 \\
& -14 f1 h1^2 h2^2 f3 - 214 f1^2 h1^2 h4 h2 + 318 f1^2 h3 h1^2 f2 - 1808 h1 f1^2 h2^2 h3 \\
& -1424 f1 h1 h2^3 h3 - 968 f1 h1 h2^3 f2 - 284 f1 h1^2 h4 h2^2 + 176 f1 h1^3 h4 h3 - 4 f1 h1^3 f3 h3 \\
& + 8 f1 h1^3 f3 f2 + 324 h1^2 h3 f2 h2^2 + 128 h1^3 h3 h4 h2 + 472 f1 h3^2 h2 h1^2 + 182 f1 f2^2 h2 h1^2 \\
& ) / (12 h1^4)
\end{aligned}$$

> **tmp1 := cpcoeff (x1\*x4^3\*T^2);**

$$\begin{aligned}
tmp1 := & (56 h2^4 + 39 f1^4 - 164 f1 h3 h1 h2 - 68 f2 h2 h1 f1 + 16 h1^2 h4 h2 - 30 f2 f1^2 h1 \\
& - 40 f2 h2^2 h1 - 104 h3 h2^2 h1 - 58 f1^2 h3 h1 + 4 h1^2 h2 f3 + 2 h1^2 f1 f3 + 24 f1 h1^2 h4 \\
& + 16 h3 f2 h1^2 + 131 f1^3 h2 + 172 f1 h2^3 + 208 f1^2 h2^2 + 32 h3^2 h1^2 + 8 e3 h1^3) / (2 h1)
\end{aligned}$$

> **elimsolve (tmp1, e3);**

$$\{8 h1^3 \neq 0\}$$

e3 is set to:

$$\begin{aligned}
& - (56 h2^4 + 39 f1^4 - 164 f1 h3 h1 h2 - 68 f2 h2 h1 f1 + 16 h1^2 h4 h2 - 30 f2 f1^2 h1 \\
& - 40 f2 h2^2 h1 - 104 h3 h2^2 h1 - 58 f1^2 h3 h1 + 4 h1^2 h2 f3 + 2 h1^2 f1 f3 + 24 f1 h1^2 h4 \\
& + 16 h3 f2 h1^2 + 131 f1^3 h2 + 172 f1 h2^3 + 208 f1^2 h2^2 + 32 h3^2 h1^2) / (8 h1^3)
\end{aligned}$$

> **tmp1 := cpcoeff (x1\*x3\*x4^2\*T^2);**

$$\begin{aligned}
tmp1 := & (14 f1 h1^3 f4 + 2 f1^2 h1^2 h4 - 28 h1^2 h2^2 f3 + 40 h1^2 h4 h2^2 + 8 e4 h1^4 \\
& - 78 f1 h1^2 h2 f3 + 28 h3 h2 h1^2 f2 - 624 h1 f1 h2^2 f2 - 2400 h1 f1^2 h2 h3 - 895 h1 f1^2 h2 f2 \\
& - 1784 h1 f1 h2^2 h3 - 20 f1 h3 h1^2 f2 - 8 h1^4 - 54 h1^2 f1^2 f3 - 164 h1 h2^3 f2 - 496 h1 h2^3 h3 \\
& - 460 h1 f1^3 f2 - 1156 h1 f1^3 h3 - 6 h1^3 f3 f2 - 8 h1^3 f3 h3 - 8 h1^3 h4 f2 - 32 h1^3 h4 h3 \\
& - 20 f2^2 f1 h1^2 - 4 f2^2 h2 h1^2 + 64 h3^2 h2 h1^2 + 8 f1 h3^2 h1^2 + 12 h1^3 f4 h2 + 1876 f1 h2^4 \\
& + 4067 f1^3 h2^2 + 3944 f1^2 h2^3 + 1990 f1^4 h2 + 360 h2^5 + 351 f1^5 + 44 f1 h1^2 h4 h2) / (2 h1^2)
\end{aligned}$$

> **elimsolve (tmp1, e4);**

$$\{8 h1^4 \neq 0\}$$

e4 is set to:

$$\begin{aligned}
& - (14 f1 h1^3 f4 + 2 f1^2 h1^2 h4 - 28 h1^2 h2^2 f3 + 40 h1^2 h4 h2^2 - 78 f1 h1^2 h2 f3 \\
& + 28 h3 h2 h1^2 f2 - 624 h1 f1 h2^2 f2 - 2400 h1 f1^2 h2 h3 - 895 h1 f1^2 h2 f2 \\
& - 1784 h1 f1 h2^2 h3 - 20 f1 h3 h1^2 f2 - 8 h1^4 - 54 h1^2 f1^2 f3 - 164 h1 h2^3 f2 - 496 h1 h2^3 h3 \\
& - 460 h1 f1^3 f2 - 1156 h1 f1^3 h3 - 6 h1^3 f3 f2 - 8 h1^3 f3 h3 - 8 h1^3 h4 f2 - 32 h1^3 h4 h3 \\
& - 20 f2^2 f1 h1^2 - 4 f2^2 h2 h1^2 + 64 h3^2 h2 h1^2 + 8 f1 h3^2 h1^2 + 12 h1^3 f4 h2 + 1876 f1 h2^4 \\
& + 4067 f1^3 h2^2 + 3944 f1^2 h2^3 + 1990 f1^4 h2 + 360 h2^5 + 351 f1^5 + 44 f1 h1^2 h4 h2) / (8 h1^4)
\end{aligned}$$

> **tmp1 := cpcoeff (x1\*x3^2\*x4\*T^2);**

$$\begin{aligned}
tmp1 := & - (2816 h1 h3 h2^4 + 12 h1^4 f3^2 + 10 f1^2 h1^3 f4 + 16 f1^3 h1^2 h4 + 24 h1^4 h2 \\
& - 1085 f1^4 h2^2 - 9636 f1^3 h2^3 + 1962 f1^5 h2 - 6768 f1 h2^5 - 12656 f1^2 h2^4 + 48 h1^4 f1 \\
& - 1440 h1^2 h3^2 h2^2 - 3068 f1 h3 h2 h1^2 f2 - 1328 h2^6 - 292 f1^2 h1^2 h2 f3 + 627 f1^6 \\
& - 16 h2 h1 h1^3 - 16 h1^4 h4^2 - 4 f2^3 h1^3 + 32 f4 h1^4 h3 - 16 f3 h1^4 h4 - 48 h3^2 f2 h1^3 \\
& - 48 h3 f2^2 h1^3 - 40 h1^3 f4 h2^2 - 488 h1 f1^4 f2 - 462 h1 f1^4 h3 - 362 f2^2 f1^2 h1^2)
\end{aligned}$$

$$\begin{aligned}
& -2616 f l^2 h^3 h l^2 + 8 h l^4 n^3 - 32 h l^2 h^4 h^2^3 + 1168 h l h^2^4 f^2 - 200 f^2 h^2^2 h l^2 \\
& -190 h l^2 f^3 f l^3 - 16 h l^2 f^3 h^2^3 + 8 h l^4 f^4 f^2 - 24 h l^3 h^4 f^2 h^2 - 116 h l^3 h^4 f^2 f l \\
& -20 h^2 f^3 h l^3 f^2 + 16 h^2 f^3 h l^3 h^3 + 5000 h l f l^2 h^2^2 f^2 - 12 h l^3 f^4 h^2 f l + 1523 h l f l^3 h^2 f^2 \\
& + 5614 h l f l^3 h^2 h^3 - 128 f l h l^2 h^2^2 f^3 + 120 f l^2 h l^2 h^4 h^2 - 2016 f l^2 h^3 h l^2 f^2 \\
& + 14064 h l f l^2 h^2^2 h^3 + 10856 f l h l h^2^3 h^3 + 4184 f l h l h^2^3 f^2 + 64 f l h l^2 h^4 h^2^2 \\
& - 168 f l h l^3 h^4 h^3 + 36 f l h l^3 f^3 h^3 + 26 f l h l^3 f^3 f^2 - 1264 h l^2 h^3 f^2 h^2^2 \\
& - 3648 f l h^3^2 h^2 h l^2 - 578 f l f^2 h^2 h l^2 + 16 h l^4 l^2) / (4 h l^3)
\end{aligned}$$

> **elimsolve (tmp1, l2);**

$$\{16 h l^4 \neq 0\}$$

l2 is set to:

$$\begin{aligned}
& -(2816 h l h^3 h^2^4 + 12 h l^4 f^3^2 + 10 f l^2 h l^3 f^4 + 16 f l^3 h l^2 h^4 + 24 h l^4 h^2 - 1085 f l^4 h^2^2 \\
& - 9636 f l^3 h^2^3 + 1962 f l^5 h^2 - 6768 f l h^2^5 - 12656 f l^2 h^2^4 + 48 h l^4 f l - 1440 h l^2 h^3^2 h^2^2 \\
& - 3068 f l h^3 h^2 h l^2 f^2 - 1328 h^2^6 - 292 f l^2 h l^2 h^2 f^3 + 627 f l^6 - 16 h^2 l l h l^3 - 16 h l^4 h^4^2 \\
& - 4 f^2^3 h l^3 + 32 f^4 h l^4 h^3 - 16 f^3 h l^4 h^4 - 48 h^3^2 f^2 h l^3 - 48 h^3 f^2^2 h l^3 - 40 h l^3 f^4 h^2^2 \\
& - 488 h l f l^4 f^2 - 462 h l f l^4 h^3 - 362 f^2^2 f l^2 h l^2 - 2616 f l^2 h^3^2 h l^2 + 8 h l^4 n^3 - 32 h l^2 h^4 h^2^3 \\
& + 1168 h l h^2^4 f^2 - 200 f^2 h^2^2 h l^2 - 190 h l^2 f^3 f l^3 - 16 h l^2 f^3 h^2^3 + 8 h l^4 f^4 f^2 \\
& - 24 h l^3 h^4 f^2 h^2 - 116 h l^3 h^4 f^2 f l - 20 h^2 f^3 h l^3 f^2 + 16 h^2 f^3 h l^3 h^3 + 5000 h l f l^2 h^2^2 f^2 \\
& - 12 h l^3 f^4 h^2 f l + 1523 h l f l^3 h^2 f^2 + 5614 h l f l^3 h^2 h^3 - 128 f l h l^2 h^2^2 f^3 \\
& + 120 f l^2 h l^2 h^4 h^2 - 2016 f l^2 h^3 h l^2 f^2 + 14064 h l f l^2 h^2^2 h^3 + 10856 f l h l h^2^3 h^3 \\
& + 4184 f l h l h^2^3 f^2 + 64 f l h l^2 h^4 h^2^2 - 168 f l h l^3 h^4 h^3 + 36 f l h l^3 f^3 h^3 + 26 f l h l^3 f^3 f^2 \\
& - 1264 h l^2 h^3 f^2 h^2^2 - 3648 f l h^3^2 h^2 h l^2 - 578 f l f^2 h^2 h l^2) / (16 h l^4)
\end{aligned}$$

> **launchNZcase (3\*f1+2\*h2);**

Launching case level 2:

$$3 f l + 2 h^2 \neq 0$$

Assume from now on that:

$$6 h l (3 f l + 2 h^2) \neq 0$$

> **tmp1 := cpcoeff (x1^4\*x4^4);**

$$\begin{aligned}
& tmp1 := -(3 f l + 2 h^2) (15 f l^3 + 71 f l^2 h^2 - 34 f^2 f l h l - 74 f l h^3 h l + 92 f l h^2^2 \\
& - 20 f^2 h^2 h l - 4 h l^2 f^3 - 52 h^3 h^2 h l + 36 h^2^3) / 2
\end{aligned}$$

> **elimsolve (tmp1, f3);**

$$\{-4 h l^2 \neq 0\}$$

f3 is set to:

$$\frac{15 f l^3 + 71 f l^2 h^2 - 34 f^2 f l h l - 74 f l h^3 h l + 92 f l h^2^2 - 20 f^2 h^2 h l - 52 h^3 h^2 h l + 36 h^2^3}{4 h l^2}$$

> **tmp1 := cpcoeff (x1\*x4^7);**

$$tmp1 := \frac{3 h l (3 f l + 2 h^2)^3 (3 f l^2 + 5 f l h^2 - 2 h l h^3 + 2 h^2^2 - 2 h l f^2)}{4}$$

> **elimsolve (tmp1, h3);**

$$\{-2 h l \neq 0\}$$

h3 is set to:

$$\frac{3 f l^2 + 5 f l h 2 + 2 h 2^2 - 2 h l f 2}{2 h l}$$

> **tmp1 := cpcoeff (x4^8);**

$$\begin{aligned} \text{tmp1} := & 3 (3 f l + 2 h 2)^2 (791 f l^5 + 2504 f l^4 h 2 + 2961 f l^3 h 2^2 - 418 h l f l^3 f 2 - 22 f l^2 h l^2 h 4 \\ & - 837 h l f l^2 h 2 f 2 + 1604 f l^2 h 2^3 - 14 f l h l^3 f 4 + 8 f 2^2 f l h l^2 + 388 f l h 2^4 - 536 h l f l h 2^2 f 2 \\ & - 52 f l h l^2 h 4 h 2 - 116 h l h 2^3 f 2 - 8 h l h l^3 + 32 h 2^5 - 20 h l^4 - 8 f 2^2 h 2 h l^2 - 20 h l^3 f 4 h 2 \\ & - 12 h l^3 h 4 f 2 - 32 h l^2 h 4 h 2^2) / 4 \end{aligned}$$

> **elimsolve (tmp1, l1);**

$$\{-8 h l^3 \neq 0\}$$

l1 is set to:

$$\begin{aligned} & (791 f l^5 + 2504 f l^4 h 2 + 2961 f l^3 h 2^2 - 418 h l f l^3 f 2 - 22 f l^2 h l^2 h 4 - 837 h l f l^2 h 2 f 2 \\ & + 1604 f l^2 h 2^3 - 14 f l h l^3 f 4 + 8 f 2^2 f l h l^2 + 388 f l h 2^4 - 536 h l f l h 2^2 f 2 - 52 f l h l^2 h 4 h 2 \\ & - 116 h l h 2^3 f 2 + 32 h 2^5 - 20 h l^4 - 8 f 2^2 h 2 h l^2 - 20 h l^3 f 4 h 2 - 12 h l^3 h 4 f 2 - 32 h l^2 h 4 h 2^2 \\ & ) / (8 h l^3) \end{aligned}$$

> **tmp1 := cpcoeff (x1^5\*x2\*x3\*x4);**

$$\begin{aligned} \text{tmp1} := & 3 (6 f l h l^3 f 4 - 30 f l^2 h l^2 h 4 - 192 h l f l h 2^2 f 2 - 231 h l f l^2 h 2 f 2 - 12 h l^4 \\ & - 36 h l h 2^3 f 2 - 70 h l f l^3 f 2 + 12 h l^3 h 4 f 2 + 16 f 2^2 f l h l^2 + 24 f 2^2 h 2 h l^2 + 4 h l^3 f 4 h 2 \\ & + 172 f l h 2^4 + 881 f l^3 h 2^2 + 604 f l^2 h 2^3 + 548 f l^4 h 2 + 16 h 2^5 + 115 f l^5 - 28 f l h l^2 h 4 h 2) / \\ & (2 h l^2) \end{aligned}$$

> **elimsolve (tmp1, f4);**

$$\{6 h l^3 f l + 4 h l^3 h 2 \neq 0\}$$

f4 is set to:

$$\begin{aligned} & -(-30 f l^2 h l^2 h 4 - 192 h l f l h 2^2 f 2 - 231 h l f l^2 h 2 f 2 - 12 h l^4 - 36 h l h 2^3 f 2 - 70 h l f l^3 f 2 \\ & + 12 h l^3 h 4 f 2 + 16 f 2^2 f l h l^2 + 24 f 2^2 h 2 h l^2 + 172 f l h 2^4 + 881 f l^3 h 2^2 + 604 f l^2 h 2^3 \\ & + 548 f l^4 h 2 + 16 h 2^5 + 115 f l^5 - 28 f l h l^2 h 4 h 2) / (2 h l^3 (3 f l + 2 h 2)) \end{aligned}$$

> **tmp1 := cpcoeff (x1^2\*x4^4\*T);**

$$\begin{aligned} \text{tmp1} := & -(3 f l + 2 h 2) (71 f l^4 + 144 f l^3 h 2 - 38 f 2 f l^2 h l + 77 f l^2 h 2^2 - 33 f 2 h 2 h l f l \\ & + 18 f l h l^2 h 4 + 2 f 2 h 2^2 h l + 8 f 2^2 h l^2 + 12 h l^2 h 4 h 2 - 4 h 2^4) / (2 h l) \end{aligned}$$

> **elimsolve (tmp1, h4);**

$$\{18 h l^2 f l + 12 h 2 h l^2 \neq 0\}$$

h4 is set to:

$$\begin{aligned} & - ( \\ & 71 f l^4 + 144 f l^3 h 2 - 38 f 2 f l^2 h l + 77 f l^2 h 2^2 - 33 f 2 h 2 h l f l + 2 f 2 h 2^2 h l + 8 f 2^2 h l^2 - 4 h 2^4 \\ & ) / (6 h l^2 (3 f l + 2 h 2)) \end{aligned}$$

> **launchNZcase (f1+h2);**

Launching case level 3:

$$f l + h 2 \neq 0$$

Assume from now on that:

$$6 h l (3 f l + 2 h 2) (f l + h 2) \neq 0$$

> **launchNZcase (2\*f1+h2);**

Launching case level 4:

$$2f1 + h2 \neq 0$$

Assume from now on that:

$$6h1(3f1 + 2h2)(f1 + h2)(2f1 + h2) \neq 0$$

> **tmp1 := cpcoeff (x1\*x2\*x4^6);**

$$\begin{aligned} tmp1 := & (30f1^7 + 2928f1^6h2 + 12128f1^5h2^2 + 981h1f1^5f2 + 3228h1f1^4h2f2 \\ & + 21266f1^4h2^3 + 36f2^2f1^3h1^2 + 4192h1f1^3h2^2f2 + 19916f1^3h2^4 + 10424f1^2h2^5 \\ & - 105f1^2f2^2h2h1^2 + 162h1^4f1^2 + 2512f1^2h1h2^3f2 + 252f1h1^4h2 + 2864f1h2^6 \\ & - 214f1f2^2h2^2h1^2 - 24f1f2^3h1^3 + 608f1h1h2^4f2 + 320h2^7 + 96h1^4h2^2 + 32h1h2^5f2 \\ & - 64f2^2h2^3h1^2) / (2h1) \end{aligned}$$

> **tmp2 := cpcoeff (x1^4\*x2\*x4^3);**

$$\begin{aligned} tmp2 := & -(456f1^7 - 1308f1^6h2 - 1467h1f1^5f2 - 10670f1^5h2^2 - 22202f1^4h2^3 \\ & - 4929h1f1^4h2f2 - 22640f1^3h2^4 - 36f2^2f1^3h1^2 - 6541h1f1^3h2^2f2 - 4114f1^2h1h2^3f2 \\ & - 12512f1^2h2^5 - 162h1^4f1^2 + 105f1^2f2^2h2h1^2 - 252f1h1^4h2 - 3584f1h2^6 \\ & + 214f1f2^2h2^2h1^2 + 24f1f2^3h1^3 - 1148f1h1h2^4f2 + 64f2^2h2^3h1^2 - 96h1^4h2^2 \\ & - 104h1h2^5f2 - 416h2^7) / (3h1^2(3f1 + 2h2)) \end{aligned}$$

> **tmp3 := factor (2\*tmp1 - 3\*h1\*(3\*f1+2\*h2)\*tmp2);**

tmp3 :=

$$\frac{3(f1 + h2)(3f1 + 2h2)^3(6f1^3 + 2f1^2h2 - 8f1h2^2 - 6f2f1h1 - 3f2h2h1 - 4h2^3)}{h1}$$

> **elimsolve (tmp3, f2);**

$$\{-6h1f1 - 3h1h2 \neq 0\}$$

f2 is set to:

$$\frac{2(f1 + h2)(-2h2^2 - 2f1h2 + 3f1^2)}{3(2f1 + h2)h1}$$

> **tmp1 := cpcoeff (x1^4\*x3\*x4^3);**

$$\begin{aligned} tmp1 := & 4(4068f1^8 + 26340f1^7h2 + 74273f1^6h2^2 + 119132f1^5h2^3 + 118890f1^4h2^4 \\ & - 648f1^3h1^4 + 75596f1^3h2^5 - 972f1^2h1^4h2 + 29909f1^2h2^6 + 6732f1h2^7 - 486f1h1^4h2^2 \\ & - 81h1^4h2^3 + 660h2^8) / (27h1(2f1 + h2)^3) \end{aligned}$$

> **tmp2 := cpcoeff (x1^3\*x2\*x4^2\*T);**

$$\begin{aligned} tmp2 := & 2(252f1^8 + 120f1^7h2 - 3983f1^6h2^2 - 13362f1^5h2^3 - 20280f1^4h2^4 + 648f1^3h1^4 \\ & - 17266f1^3h2^5 - 8529f1^2h2^6 + 972f1^2h1^4h2 + 486f1h1^4h2^2 - 2292f1h2^7 - 260h2^8 \\ & + 81h1^4h2^3) / (9h1^2(2f1 + h2)^3) \end{aligned}$$

> **tmp3 := factor (3\*tmp1 + 2\*h1\*tmp2);**

$$tmp3 := \frac{40(5h2 + 8f1)(f1 + h2)^3(3f1 + 2h2)^3}{9(2f1 + h2)^2h1}$$

> **tmp4 := cpcoeff (x4^4\*T^2);**

$$tmp4 := -(3f1 + 2h2)(14976f1^8 + 95460f1^7h2 + 264236f1^6h2^2 + 414756f1^5h2^3$$

$$+ 403692 f l^4 h^4 + 249448 f l^3 h^2^5 + 648 f l^3 h l^4 + 972 f l^2 h l^4 h^2 + 95544 f l^2 h^2^6 \\ + 20736 f l h^2^7 + 486 f l h l^4 h^2^2 + 1952 h^2^8 + 81 h l^4 h^2^3) / (81 h l^2 (2 f l + h^2)^3)$$

> **tmp5 := cpcoeff (x1\*x4^5\*T);**

$$tmp5 := (3 f l + 2 h^2)^2 (3816 f l^8 + 24744 f l^7 h^2 + 69592 f l^6 h^2^2 + 110832 f l^5 h^2^3 \\ + 109272 f l^4 h^2^4 - 648 f l^3 h l^4 + 68264 f l^3 h^2^5 - 972 f l^2 h l^4 h^2 + 26376 f l^2 h^2^6 + 5760 f l h^2^7 \\ - 486 f l h l^4 h^2^2 - 81 h l^4 h^2^3 + 544 h^2^8) / (81 h l^2 (2 f l + h^2)^3)$$

> **tmp6 := factor ((2\*h2+3\*f1)\*tmp4 - tmp5);**

$$tmp6 := - \frac{4 (26 h^2 + 29 f l) (f l + h^2)^3 (3 f l + 2 h^2)^5}{27 (2 f l + h^2)^2 h l^2}$$

> **tmp7 := factor ((2\*h2+3\*f1)^2\*tmp3 + 6\*h1\*tmp6);**

$$tmp7 := \frac{8 (3 f l + 2 h^2)^5 (f l + h^2)^3 (-h^2 + 11 f l)}{9 (2 f l + h^2)^2 h l}$$

> **elimsolve (tmp7, h2);**

$$\{-1 \neq 0\}$$

h2 is set to:

$$11 f l$$

Nonzero constraint refines to:

$$2340 h l f l^3 \neq 0$$

> **tmp1 := cpcoeff (x1^3\*x2\*x4^2\*T);**

$$tmp1 := - \frac{18 (1464240000 f l^5 - 2197 h l^4)}{2197 h l^2}$$

> **tmp2 := cpcoeff (x1^4\*x3\*x4^3);**

$$tmp2 := \frac{12 (4194240000 f l^5 - 2197 h l^4)}{2197 h l}$$

> **tmp3 := cpcoeff (x4^4\*T^2);**

$$tmp3 := - \frac{25 f l (12820320000 f l^5 + 2197 h l^4)}{2197 h l^2}$$

> **tmp4 := factor(100\*f1\*h1\*tmp1 - 1725\*f1\*tmp2 + 900\*h1\*tmp3);**

$$tmp4 := - \frac{377913600000000 f l^6}{2197 h l}$$

> **contradict (tmp4, 'h2');**

Contradiction on case level 4, so:

$$2 f l + h^2 = 0$$

Variables to be uneliminated:

$$"h2 := 'h2'"$$

$$"f2 := 'f2'"$$

Proceed on case level 3 with:

$$6 h l (3 f l + 2 h^2) (f l + h^2) \neq 0$$

On account of:

$$2 f l + h^2 = 0$$

$$\{1 \neq 0\}$$

h2 is set to:

$$-2f1$$

Nonzero constraint refines to:

$$6h1f1^2 \neq 0$$

> tmp1 := cpcoeff (x1^4\*x3\*x4^3);

$$tmp1 := \frac{2(-18h1^4f1 + 63f1^6 + 24f2^3h1^3 + 141h1f1^4f2 + 104f2^2f1^2h1^2)}{3h1f1}$$

> tmp2 := cpcoeff (x1\*x3\*x4^6);

$$tmp2 := 18h1^4f1 - 60f1^6 - 24f2^3h1^3 - 141h1f1^4f2 - 104f2^2f1^2h1^2$$

> tmp3 := factor (3\*f1\*h1\*tmp1 + 2\*tmp2);

$$tmp3 := 6f1^6$$

> contradict (tmp3, f1);

Contradiction on case level 3, so:

$$f1 + h2 = 0$$

Variables to be uneliminated:

$$"h2 := 'h2'"$$

Proceed on case level 2 with:

$$6h1(3f1 + 2h2) \neq 0$$

On account of:

$$f1 + h2 = 0$$

$$\{1 \neq 0\}$$

f1 is set to:

$$-h2$$

Nonzero constraint refines to:

$$-6h1h2 \neq 0$$

> tmp1 := cpcoeff (x1\*x2\*x4^6);

$$tmp1 := \frac{3(2h1^3h2 - 3h2^4f2 + 3f2^2h2^2h1 + 8h1^2f2^3)h2}{2}$$

> tmp2 := cpcoeff (x1^3\*x2\*x4^2\*T);

$$tmp2 := \frac{3(-3f2^2h2^2h1 + 6h1^3h2 + 3h2^4f2 - 8h1^2f2^3)}{h1h2}$$

> tmp3 := factor (2\*tmp1 + h2^2\*h1\*tmp2);

$$tmp3 := 24h1^3h2^2$$

> contradict (tmp3, h2);

Contradiction on case level 2, so:

$$3f1 + 2h2 = 0$$

Variables to be uneliminated:

$$"f1 := 'f1'"$$

$$"h4 := 'h4'"$$

$$"f4 := 'f4'"$$

$$"l1 := 'l1'"$$

$$"h3 := 'h3'"$$

$$"f3 := 'f3'"$$

Proceed on case level 1 with:

$$6\ h1 \neq 0$$

On account of:

$$3\ f1 + 2\ h2 = 0$$
$$\{2 \neq 0\}$$

h2 is set to:

$$-\frac{3\ f1}{2}$$

> **tmp1 := cpcoeff (x1^5\*x2^2\*x4);**

$$\begin{aligned} tmp1 := & -(-4\ h1^4\ f3^2 + 18\ f1^2\ h1^3\ f4 - 42\ f1^3\ h1^2\ h4 - 12\ h1^4\ f1 + 33\ f1^6 - 6\ f1\ l1\ h1^3 \\ & - 12\ k1\ h1^4 - 105\ h1\ f1^4\ f2 - 183\ h1\ f1^4\ h3 - 19\ f2^2\ f1^2\ h1^2 + 152\ f1^2\ h3^2\ h1^2 - 3\ h1^2\ f3\ f1^3 \\ & + 12\ h1^3\ h4\ f2\ f1 + 92\ f1^2\ h3\ h1^2\ f2 + 48\ f1\ h1^3\ h4\ h3 - 16\ f1\ h1^3\ f3\ h3 - 32\ f1\ h1^3\ f3\ f2) / (2 \\ & h1^3) \end{aligned}$$

> **elimsolve (tmp1, k1);**

$$\{-12\ h1^4 \neq 0\}$$

k1 is set to:

$$\begin{aligned} & (-4\ h1^4\ f3^2 + 18\ f1^2\ h1^3\ f4 - 42\ f1^3\ h1^2\ h4 - 12\ h1^4\ f1 + 33\ f1^6 - 6\ f1\ l1\ h1^3 - 105\ h1\ f1^4\ f2 \\ & - 183\ h1\ f1^4\ h3 - 19\ f2^2\ f1^2\ h1^2 + 152\ f1^2\ h3^2\ h1^2 - 3\ h1^2\ f3\ f1^3 + 12\ h1^3\ h4\ f2\ f1 \\ & + 92\ f1^2\ h3\ h1^2\ f2 + 48\ f1\ h1^3\ h4\ h3 - 16\ f1\ h1^3\ f3\ h3 - 32\ f1\ h1^3\ f3\ f2) / (12\ h1^4) \end{aligned}$$

> **tmp1 := cpcoeff (x1\*x2\*x4^2\*T^2);**

$$\begin{aligned} tmp1 := & (-24\ h1^4\ f3^2 + 128\ f1^2\ h1^3\ f4 - 176\ f1^3\ h1^2\ h4 - 192\ h1^4\ f1 - 64\ h1^3\ h3^3 + 52\ f1^6 \\ & - 56\ f1\ l1\ h1^3 - 192\ h3^2\ f2\ h1^3 - 68\ h3\ f2^2\ h1^3 - 889\ h1\ f1^4\ f2 - 982\ h1\ f1^4\ h3 \\ & - 199\ f2^2\ f1^2\ h1^2 + 888\ f1^2\ h3^2\ h1^2 - 16\ h1^4\ n3 - 62\ h1^2\ f3\ f1^3 - 20\ h1^4\ f4\ f2 + 44\ h1^3\ h4\ f2\ f1 \\ & + 718\ f1^2\ h3\ h1^2\ f2 + 176\ f1\ h1^3\ h4\ h3 - 216\ f1\ h1^3\ f3\ h3 - 340\ f1\ h1^3\ f3\ f2) / (4\ h1^3) \end{aligned}$$

> **elimsolve (tmp1, n3);**

$$\{-16\ h1^4 \neq 0\}$$

n3 is set to:

$$\begin{aligned} & (-24\ h1^4\ f3^2 + 128\ f1^2\ h1^3\ f4 - 176\ f1^3\ h1^2\ h4 - 192\ h1^4\ f1 - 64\ h1^3\ h3^3 + 52\ f1^6 - 56\ f1\ l1\ h1^3 \\ & - 192\ h3^2\ f2\ h1^3 - 68\ h3\ f2^2\ h1^3 - 889\ h1\ f1^4\ f2 - 982\ h1\ f1^4\ h3 - 199\ f2^2\ f1^2\ h1^2 \\ & + 888\ f1^2\ h3^2\ h1^2 - 62\ h1^2\ f3\ f1^3 - 20\ h1^4\ f4\ f2 + 44\ h1^3\ h4\ f2\ f1 + 718\ f1^2\ h3\ h1^2\ f2 \\ & + 176\ f1\ h1^3\ h4\ h3 - 216\ f1\ h1^3\ f3\ h3 - 340\ f1\ h1^3\ f3\ f2) / (16\ h1^4) \end{aligned}$$

> **tmp1 := cpcoeff (x1^4\*x3\*x4^3);**

$$\begin{aligned} tmp1 := & (16\ f1\ h1^3\ f4 - 16\ f1^2\ h1^2\ h4 + 28\ f1\ h3\ h1^2\ f2 - 20\ h1^4 + 8\ h1^2\ f1^2\ f3 - 66\ h1\ f1^3\ f2 \\ & - 108\ h1\ f1^3\ h3 - 30\ h1^3\ f3\ f2 - 32\ h1^3\ f3\ h3 + 4\ h1^3\ h4\ f2 + 16\ h1^3\ h4\ h3 - 28\ f2^2\ f1\ h1^2 \\ & + 80\ f1\ h3^2\ h1^2 - 8\ l1\ h1^3 + 17\ f1^5) / h1 \end{aligned}$$

> **elimsolve (tmp1, l1);**

$$\{-8\ h1^3 \neq 0\}$$

l1 is set to:

$$(16\ f1\ h1^3\ f4 - 16\ f1^2\ h1^2\ h4 + 28\ f1\ h3\ h1^2\ f2 - 20\ h1^4 + 8\ h1^2\ f1^2\ f3 - 66\ h1\ f1^3\ f2$$



$$-108 h1 f1^3 h3 - 30 h1^3 f3 f2 - 32 h1^3 f3 h3 + 4 h1^3 h4 f2 + 16 h1^3 h4 h3 - 28 f2^2 f1 h1^2 + 80 f1 h3^2 h1^2 + 17 f1^5) / (8 h1^3)$$

> **tmp1 := cpcoeff (x1^4\*x2\*x4^3);**

$$tmp1 := - \frac{(3 f1^3 + 2 f2 f1 h1 + 2 h1^2 f3 - 2 f1 h3 h1)^2}{h1^2}$$

> **elimsolve (tmp1, f3);**

$$\{2 h1^2 \neq 0\}$$

f3 is set to:

$$- \frac{f1 (3 f1^2 + 2 h1 f2 - 2 h1 h3)}{2 h1^2}$$

> **launchNZcase (3\*f1^2-h1\*f2-4\*h1\*h3);**

Launching case level 2:

$$3 f1^2 - h1 f2 - 4 h1 h3 \neq 0$$

Assume from now on that:

$$6 h1 (3 f1^2 - h1 f2 - 4 h1 h3) \neq 0$$

> **tmp1 := cpcoeff (x1^5\*x2\*x3\*x4);**

$$tmp1 := -3 (-6 f1^2 h1^2 h4 + 15 f1 h3 h1^2 f2 + 6 h1^4 - 12 h1 f1^3 f2 - 29 h1 f1^3 h3 + 2 h1^3 h4 f2 + 8 h1^3 h4 h3 + f2^2 f1 h1^2 + 24 f1 h3^2 h1^2 + 7 f1^5) / h1^2$$

> **elimsolve (tmp1, h4);**

$$\{-6 f1^2 h1^2 + 2 h1^3 f2 + 8 h1^3 h3 \neq 0\}$$

h4 is set to:

$$\frac{15 f1 h3 h1^2 f2 + 6 h1^4 - 12 h1 f1^3 f2 - 29 h1 f1^3 h3 + f2^2 f1 h1^2 + 24 f1 h3^2 h1^2 + 7 f1^5}{2 h1^2 (3 f1^2 - h1 f2 - 4 h1 h3)}$$

> **launchNZcase (5\*h1\*f2+f1^2+4\*h1\*h3);**

Launching case level 3:

$$5 h1 f2 + f1^2 + 4 h1 h3 \neq 0$$

Assume from now on that:

$$6 h1 (3 f1^2 - h1 f2 - 4 h1 h3) (5 h1 f2 + f1^2 + 4 h1 h3) \neq 0$$

> **tmp1 := cpcoeff (x1\*x3^3\*x4^4);**

$$tmp1 := -3 (68 f1^8 - 161 f1^6 h1 f2 - 416 f1^6 h1 h3 + 1348 f1^4 h3 h1^2 f2 + 398 f1^4 f2^2 h1^2 + 1304 f1^4 h3^2 h1^2 - 12 f1^4 h1^3 f4 + 12 f1^3 h1^4 - 3064 f1^2 h3^2 f2 h1^3 - 225 f1^2 f2^3 h1^3 - 1952 f1^2 h1^3 h3^3 - 56 f1^2 h1^4 f4 f2 - 1552 f1^2 h3 f2^2 h1^3 - 32 f1^2 h1^4 f4 h3 + 48 h1^5 f1 h3 + 60 h1^5 f1 f2 + 96 h1^5 f4 f2 h3 + 20 h1^5 f4 f2^2 + 64 h1^5 h3^2 f4 + 28 f2^4 h1^4 + 332 h3 f2^3 h1^4 + 1312 h3^2 f2^2 h1^4 + 1024 h1^4 h3^4 + 1984 h1^4 h3^3 f2) / (4 h1^2)$$

> **elimsolve (tmp1, f4);**

$$\{-12 f1^4 h1^3 - 56 f1^2 h1^4 f2 - 32 f1^2 h1^4 h3 + 96 h1^5 h3 f2 + 20 h1^5 f2^2 + 64 h1^5 h3^2 \neq 0\}$$

f4 is set to:

$$(68 f1^8 - 161 f1^6 h1 f2 - 416 f1^6 h1 h3 + 1348 f1^4 h3 h1^2 f2 + 398 f1^4 f2^2 h1^2 + 1304 f1^4 h3^2 h1^2 + 12 f1^3 h1^4 - 3064 f1^2 h3^2 f2 h1^3 - 225 f1^2 f2^3 h1^3 - 1952 f1^2 h1^3 h3^3 - 1552 f1^2 h3 f2^2 h1^3 + 48 h1^5 f1 h3 + 60 h1^5 f1 f2 + 28 f2^4 h1^4 + 332 h3 f2^3 h1^4$$

$$+ 1312 h^3 f^2 h l^4 + 1024 h l^4 h^3 + 1984 h l^4 h^3 f^2) / (4 h l^3 (5 h l f^2 + f l^2 + 4 h l h^3) (3 f l^2 - h l f^2 - 4 h l h^3))$$

> **launchNZcase (f1^2-h1\*h3);**

Launching case level 4:

$$f l^2 - h l h^3 \neq 0$$

Assume from now on that:

$$6 h l (3 f l^2 - h l f^2 - 4 h l h^3) (5 h l f^2 + f l^2 + 4 h l h^3) (f l^2 - h l h^3) \neq 0$$

> **launchNZcase (h1\*f2+5\*f1^2-4\*h1\*h3);**

Launching case level 5:

$$h l f^2 + 5 f l^2 - 4 h l h^3 \neq 0$$

Assume from now on that:

$$6 h l (3 f l^2 - h l f^2 - 4 h l h^3) (5 h l f^2 + f l^2 + 4 h l h^3) (f l^2 - h l h^3) (h l f^2 + 5 f l^2 - 4 h l h^3) \neq 0$$

> **tmp1 := cpcoeff (x4^4\*T^2);**

$$tmp1 := - \frac{(f l^2 - h l h^3) (f l^2 - 4 h l h^3 - 3 h l f^2) (h l f^2 + 5 f l^2 - 4 h l h^3)}{h l^2}$$

> **elimsolve (tmp1, h3);**

$$\{-4 h l \neq 0\}$$

h3 is set to:

$$\frac{f l^2 - 3 h l f^2}{4 h l}$$

Nonzero constraint refines to:

$$6 h l (2 f l^2 + 2 h l f^2)^3 (3 f l^2 + 3 h l f^2) \neq 0$$

> **tmp1 := cpcoeff (x3\*x4^3\*T^2);**

$$tmp1 := - \frac{(f l^2 + h l f^2) (33 f l^5 + 66 h l f l^3 f^2 + 33 f^2 f l h l^2 + 232 h l^4)}{8 h l^3}$$

> **tmp2 := cpcoeff (x1\*x3^4\*x4^3);**

$$tmp2 := \frac{3 (f l^5 + 2 h l f l^3 f^2 + f^2 f l h l^2 - 152 h l^4) (f l^2 + h l f^2)^2}{4 h l^3}$$

> **tmp3 := cpcoeff (x1\*x2\*x3^2\*x4^4);**

$$tmp3 := \frac{3 (f l^5 + 2 h l f l^3 f^2 + f^2 f l h l^2 - 16 h l^4) (f l^2 + h l f^2)^2}{h l^3}$$

> **tmp4 := factor(24\*(f1^2+h1\*f2)\*tmp1 - 16\*tmp2 + 37\*tmp3);**

$$tmp4 := -648 h l (f l^2 + h l f^2)^2$$

> **contradict (tmp4, 'f2');**

Contradiction on case level 5, so:

$$h l f^2 + 5 f l^2 - 4 h l h^3 = 0$$

Variables to be uneliminated:

$$"h3 := 'h3'"$$

Proceed on case level 4 with:

$$6 h l (3 f l^2 - h l f^2 - 4 h l h^3) (5 h l f^2 + f l^2 + 4 h l h^3) (f l^2 - h l h^3) \neq 0$$

On account of:

$$h1 f2 + 5 f1^2 - 4 h1 h3 = 0$$
$$\{h1 \neq 0\}$$

f2 is set to:

$$-\frac{5 f1^2 - 4 h1 h3}{h1}$$

Nonzero constraint refines to:

$$6 h1 (2 f1^2 - 2 h1 h3) (-6 f1^2 + 6 h1 h3) (f1^2 - h1 h3) \neq 0$$

> tmp1 := cpcoeff (x1\*x2^3\*x4^4);

$$tmp1 := -\frac{576 (f1^5 - 2 h1 f1^3 h3 + f1 h3^2 h1^2 - h1^4) (f1^2 - h1 h3)^2 f1^2}{h1^5}$$

> tmp2 := cpcoeff (x3\*x4^3\*T^2);

$$tmp2 := -\frac{4 (f1^2 - h1 h3) (46 f1^5 - 92 h1 f1^3 h3 + 46 f1 h3^2 h1^2 + 11 h1^4)}{h1^3}$$

> tmp3 := factor (23\*h1^2\*tmp1 + 72\*(-f1^2+h1\*h3)\*f1^2\*tmp2);

$$tmp3 := 16416 (f1^2 - h1 h3)^2 f1^2 h1$$

> tmp4 := cpcoeff (x1\*x3^4\*x4^3);

$$tmp4 := -\frac{96 (82 f1^5 - 164 h1 f1^3 h3 + 82 f1 h3^2 h1^2 + 117 h1^4) (f1^2 - h1 h3)^2}{h1^3}$$

> tmp5 := factor (41\*h1^2\*tmp1 - 3\*f1^2\*tmp4);

$$tmp5 := 57312 (f1^2 - h1 h3)^2 f1^2 h1$$

> tmp6 := factor (7\*tmp3 - 2\*tmp5);

$$tmp6 := 288 (f1^2 - h1 h3)^2 f1^2 h1$$

> elimsolve (tmp6, f1);

$$\{1 \neq 0\}$$

f1 is set to:

$$0$$

Nonzero constraint refines to:

$$72 h1^4 h3^3 \neq 0$$

> tmp1 := cpcoeff (x1\*x2^5\*x4^2);

$$tmp1 := 192 h1^3$$

> contradict (tmp1, 'h3');

Contradiction on case level 4, so:

$$f1^2 - h1 h3 = 0$$

Variables to be uneliminated:

$$"f1 := 'f1'"$$

$$"f2 := 'f2'"$$

Proceed on case level 3 with:

$$6 h1 (3 f1^2 - h1 f2 - 4 h1 h3) (5 h1 f2 + f1^2 + 4 h1 h3) \neq 0$$

On account of:

$$f1^2 - h1 h3 = 0$$

$$\{-h1 \neq 0\}$$

h3 is set to:

$$\frac{f1^2}{h1}$$

Nonzero constraint refines to:

$$6 h1 (-f1^2 - h1 f2) (5 h1 f2 + 5 f1^2) \neq 0$$

> **tmp1 := cpcoeff (x3\*x4^3\*T^2);**

$$tmp1 := \frac{(f1^2 + h1 f2) (3 f1^5 + 6 h1 f1^3 f2 + 3 f2^2 f1 h1^2 - 16 h1^4)}{2 h1^3}$$

> **tmp2 := cpcoeff (x1\*x2^3\*x4^4);**

$$tmp2 := -\frac{15 (f1^5 + 2 h1 f1^3 f2 + f2^2 f1 h1^2 - 4 h1^4) (f1^2 + h1 f2)^2 f1^2}{4 h1^5}$$

> **tmp3 := factor (f1^2\*(5\*h1\*f2+f1^2+4\*h1\*h3)\*tmp1 + 2\*h1^2\*tmp2);**

$$tmp3 := -10 f1^2 (f1^2 + h1 f2)^2 h1$$

> **elimsolve (tmp3, f1);**

$$\{1 \neq 0\}$$

f1 is set to:

$$0$$

Nonzero constraint refines to:

$$-30 h1^3 f2^2 \neq 0$$

> **tmp1 := cpcoeff (x1^4\*x2^3\*x4);**

$$tmp1 := -32 h1^2$$

> **contradict (tmp1, 'h3');**

Contradiction on case level 3, so:

$$5 h1 f2 + f1^2 + 4 h1 h3 = 0$$

Variables to be uneliminated:

$$"f1 := 'f1'"$$

$$"h3 := 'h3'"$$

$$"f4 := 'f4'"$$

Proceed on case level 2 with:

$$6 h1 (3 f1^2 - h1 f2 - 4 h1 h3) \neq 0$$

On account of:

$$5 h1 f2 + f1^2 + 4 h1 h3 = 0$$

$$\{4 h1 \neq 0\}$$

h3 is set to:

$$-\frac{5 h1 f2 + f1^2}{4 h1}$$

Nonzero constraint refines to:

$$6 h1 (2 f1^2 + 2 h1 f2) \neq 0$$

> **tmp1 := cpcoeff (x1\*x3^3\*x4^4);**

$$tmp1 := -\frac{216 (f1^2 + h1 f2)^4}{h1^2}$$

> **contradict** (tmp1, 'h3');

Contradiction on case level 2, so:

$$3 f1^2 - h1 f2 - 4 h1 h3 = 0$$

Variables to be uneliminated:

"h3 := 'h3'"

"h4 := 'h4'"

Proceed on case level 1 with:

$$6 h1 \neq 0$$

On account of:

$$3 f1^2 - h1 f2 - 4 h1 h3 = 0$$

$$\{-4 h1 \neq 0\}$$

h3 is set to:

$$\frac{3 f1^2 - h1 f2}{4 h1}$$

> **tmp1 := cpcoeff** (x4^4\*T^2);

$$tmp1 := \frac{(f1^2 + h1 f2)^3}{h1^2}$$

> **elimsolve** (tmp1, f2);

$$\{h1 \neq 0\}$$

f2 is set to:

$$-\frac{f1^2}{h1}$$

> **tmp1 := cpcoeff** (x1^5\*x2^1\*x3^1\*x4^1);

$$tmp1 := -18 h1^2$$

> **contradict** (tmp1);

Contradiction on case level 1, so:

$$h1 = 0$$

Variables to be uneliminated:

"f2 := 'f2'"

"h3 := 'h3'"

"f3 := 'f3'"

"l1 := 'l1'"

"n3 := 'n3'"

"k1 := 'k1'"

"h2 := 'h2'"

"l2 := 'l2'"

"e4 := 'e4'"

"e3 := 'e3'"

"q4 := 'q4'"

|                                          |                                     |
|------------------------------------------|-------------------------------------|
|                                          | "n2 := 'n2'"                        |
|                                          | "n1 := 'n1'"                        |
|                                          | "e2 := 'e2'"                        |
|                                          | "q3 := 'q3'"                        |
|                                          | "q2 := 'q2'"                        |
|                                          | "q1 := 'q1'"                        |
|                                          | "e1 := 'e1'"                        |
| Proceed on case level 0 with:            |                                     |
|                                          | $6 \neq 0$                          |
| On account of:                           |                                     |
|                                          | $h1 = 0$                            |
|                                          | $\{1 \neq 0\}$                      |
| h1 is set to:                            |                                     |
|                                          | 0                                   |
| > <b>launchNZcase (f1+h2);</b>           |                                     |
| Launching case level 1:                  |                                     |
|                                          | $f1 + h2 \neq 0$                    |
| Assume from now on that:                 |                                     |
|                                          | $6 f1 + 6 h2 \neq 0$                |
| > <b>tmp1 := cpcoeff (x1^3*x4^3*T);</b>  |                                     |
|                                          | $tmp1 := (f1 + h2) (3 f1 + 2 h2)^2$ |
| > <b>elimsolve (tmp1, f1);</b>           |                                     |
|                                          | $\{3 \neq 0\}$                      |
| f1 is set to:                            |                                     |
|                                          | $-\frac{2 h2}{3}$                   |
| Nonzero constraint refines to:           |                                     |
|                                          | $6 h2 \neq 0$                       |
| > <b>tmp1 := cpcoeff (x1^5+x3*x4^2);</b> |                                     |
|                                          | $tmp1 := \frac{4 h2^3}{3}$          |
| > <b>contradict (tmp1, h2);</b>          |                                     |
| Contradiction on case level 1, so:       |                                     |
|                                          | $f1 + h2 = 0$                       |
| Variables to be uneliminated:            |                                     |
|                                          | "f1 := 'f1'"                        |
| Proceed on case level 0 with:            |                                     |
|                                          | $6 \neq 0$                          |
| On account of:                           |                                     |
|                                          | $f1 + h2 = 0$                       |
|                                          | $\{1 \neq 0\}$                      |
| h2 is set to:                            |                                     |
|                                          | $-f1$                               |
| > <b>launchNZcase (f1);</b>              |                                     |
| Launching case level 1:                  |                                     |

```

                                 $f1 \neq 0$ 
Assume from now on that:
                                 $6f1 \neq 0$ 
> tmp1 := cpcoeff (x1*x3^2*x4^5);
                                 $tmp1 := 3f1^4(-q1 + f1h3)$ 
> elimsolve (tmp1, q1);
                                 $\{-1 \neq 0\}$ 
q1 is set to:
                                 $f1h3$ 
> tmp1 := cpcoeff (x1^3*x3*x4^2*T);
                                 $tmp1 := f1^2(-f2 - 4h3 + 4e1)$ 
> elimsolve (tmp1, e1);
                                 $\{4 \neq 0\}$ 
e1 is set to:
                                 $\frac{f2}{4} + h3$ 
> tmp1 := cpcoeff (x1^5*x3^2*x4);
                                 $tmp1 := -\frac{3f1^2(3f2 + 4h3)}{2}$ 
> elimsolve (tmp1, h3);
                                 $\{4 \neq 0\}$ 
h3 is set to:
                                 $-\frac{3f2}{4}$ 
> tmp1 := cpcoeff (x1^5*x3^3);
                                 $tmp1 := \frac{f1(-17f2^2 - 16h4f1 - 24q2 + 8f1f3)}{8}$ 
> elimsolve (tmp1, q2);
                                 $\{-24 \neq 0\}$ 
q2 is set to:
                                 $-\frac{17f2^2}{24} - \frac{2h4f1}{3} + \frac{f1f3}{3}$ 
> tmp1 := cpcoeff (x4^4*T^2);
                                 $tmp1 := -\frac{(4f1f3 - 4n1 + 3f2^2 + 4h4f1)f1^2}{4}$ 
> elimsolve (tmp1, n1);
                                 $\{-4 \neq 0\}$ 
n1 is set to:
                                 $f1f3 + \frac{3f2^2}{4} + h4f1$ 
> tmp1 := cpcoeff (x3^3*x4^5);

```

$$tmp1 := \frac{3 f1^5 (-4 l1 + 2 f4 f1 - f2 f3 - f2 e2 + 4 e3 f1 - 2 n2)}{2}$$

> elimsolve (tmp1, n2);

$$\{-2 \neq 0\}$$

n2 is set to:

$$-2 l1 + f4 f1 - \frac{f2 f3}{2} - \frac{f2 e2}{2} + 2 e3 f1$$

> tmp1 := cpcoeff (x1\*x3^3\*x4^4);

$$tmp1 := \frac{3 f1^4 (8 f1 f3 + 3 f2^2 + 8 h4 f1)}{8}$$

> elimsolve (tmp1, h4);

$$\{8 f1 \neq 0\}$$

h4 is set to:

$$-\frac{8 f1 f3 + 3 f2^2}{8 f1}$$

> tmp1 := cpcoeff (x1^5\*x2\*x3\*x4);

$$tmp1 := -4 f1^2 (2 e2 + f3)$$

> elimsolve (tmp1, f3);

$$\{1 \neq 0\}$$

f3 is set to:

$$-2 e2$$

> tmp1 := cpcoeff (x1^3\*x3^2\*x4\*T);

$$tmp1 := 6 e2 f1^2$$

> elimsolve (tmp1, e2);

$$\{1 \neq 0\}$$

e2 is set to:

$$0$$

> tmp1 := cpcoeff (x3\*x4^3\*T^2);

$$tmp1 := -2 (-l1 + f4 f1) f1^2$$

> elimsolve (tmp1, l1);

$$\{-1 \neq 0\}$$

l1 is set to:

$$f4 f1$$

> tmp1 := cpcoeff (x1\*x2\*x4^2\*T^2);

$$tmp1 := 2 e3 f1^2$$

> elimsolve (tmp1, e3);

$$\{1 \neq 0\}$$

e3 is set to:

$$0$$

> tmp1 := cpcoeff (x1\*x3^4\*x4^3);

$$tmp1 := -9 f1^4 q3$$

> elimsolve (tmp1, q3);



```

{1 ≠ 0}
q3 is set to:
0
> tmp1 := cpcoeff (x1^2*x3^3*x4^3);
tmp1 :=  $\frac{3 f2 f1^4}{2}$ 
> elimsolve (tmp1, f2);
{1 ≠ 0}
f2 is set to:
0
> tmp1 := cpcoeff (x1^2*x2*x3*x4^2*T);
tmp1 :=  $-2 f1^3 (e4 + 1)$ 
> elimsolve (tmp1, e4);
{1 ≠ 0}
e4 is set to:
-1
> tmp1 := cpcoeff (x3^5*x4^3);
tmp1 :=  $-3 f1^5 n4$ 
> elimsolve (tmp1, n4);
{1 ≠ 0}
n4 is set to:
0
> tmp1 := cpcoeff (x1^4*x3^4);
tmp1 :=  $-n3 f1^2$ 
> elimsolve (tmp1, n3);
{1 ≠ 0}
n3 is set to:
0
> tmp1 := cpcoeff (x1*x3^4*x4*T);
tmp1 :=  $-f4^2 f1^3$ 
> elimsolve (tmp1, f4);
{1 ≠ 0}
f4 is set to:
0
> tmp1 := cpcoeff (x1*x2*x3^2*x4^2*T);
tmp1 :=  $-2 l4 f1^3$ 
> elimsolve (tmp1, l4);
{1 ≠ 0}
l4 is set to:
0
> tmp1 := cpcoeff (x2^2*x4^2*T^2);
tmp1 :=  $3 k3 f1^2$ 
> elimsolve (tmp1, k3);

```

|                                    |                    |
|------------------------------------|--------------------|
|                                    | $\{1 \neq 0\}$     |
| k3 is set to:                      |                    |
|                                    | 0                  |
| > tmp1 := cpcoeff (x1^5*x2^2*x3);  |                    |
|                                    | $tmp1 := -3 f1 l2$ |
| > elimsolve (tmp1, l2);            |                    |
|                                    | $\{1 \neq 0\}$     |
| l2 is set to:                      |                    |
|                                    | 0                  |
| > tmp1 := cpcoeff (x3^4*x4^4);     |                    |
|                                    | $tmp1 := 3 f1^6$   |
| > contradict (tmp1);               |                    |
| Contradiction on case level 1, so: |                    |
|                                    | $f1 = 0$           |
| Variables to be uneliminated:      |                    |
|                                    | "l2 := 'l2'"       |
|                                    | "k3 := 'k3'"       |
|                                    | "l4 := 'l4'"       |
|                                    | "f4 := 'f4'"       |
|                                    | "n3 := 'n3'"       |
|                                    | "n4 := 'n4'"       |
|                                    | "e4 := 'e4'"       |
|                                    | "f2 := 'f2'"       |
|                                    | "q3 := 'q3'"       |
|                                    | "e3 := 'e3'"       |
|                                    | "l1 := 'l1'"       |
|                                    | "e2 := 'e2'"       |
|                                    | "f3 := 'f3'"       |
|                                    | "h4 := 'h4'"       |
|                                    | "n2 := 'n2'"       |
|                                    | "n1 := 'n1'"       |
|                                    | "q2 := 'q2'"       |
|                                    | "h3 := 'h3'"       |
|                                    | "e1 := 'e1'"       |
|                                    | "q1 := 'q1'"       |
| Proceed on case level 0 with:      |                    |
|                                    | $6 \neq 0$         |
| On account of:                     |                    |
|                                    | $f1 = 0$           |
|                                    | $\{1 \neq 0\}$     |
| f1 is set to:                      |                    |
|                                    | 0                  |

```

> tmp1 := cpcoeff (x1^4*x3^2*x4^2);
                                      $tmp1 := -9 q1^2$ 
> elimsolve (tmp1, q1);
                                      $\{1 \neq 0\}$ 
q1 is set to:
                                     0
> launchNZcase (n1);
Launching case level 1:
                                      $n1 \neq 0$ 
Assume from now on that:
                                      $6 n1 \neq 0$ 
> tmp1 := cpcoeff (x1^4*x3^4);
                                      $tmp1 := -n1 (n1 + f2^2 + 3 q2)$ 
> elimsolve (tmp1, q2);
                                      $\{3 \neq 0\}$ 
q2 is set to:
                                      $-\frac{n1}{3} - \frac{f2^2}{3}$ 
> tmp1 := cpcoeff (x1^5*x2*x3^2);
                                      $tmp1 := -n1 (2 e1 + 3 f2 + 4 h3)$ 
> elimsolve (tmp1, h3);
                                      $\{4 \neq 0\}$ 
h3 is set to:
                                      $-\frac{e1}{2} - \frac{3 f2}{4}$ 
> launchNZcase (e1);
Launching case level 2:
                                      $e1 \neq 0$ 
Assume from now on that:
                                      $6 n1 e1 \neq 0$ 
> tmp1 := cpcoeff (x1^5*x2^2*x4);
                                      $tmp1 := 2 e1 (14 e1^2 + 15 e1 f2 + 3 f2^2 + 2 n1)$ 
> elimsolve (tmp1, n1);
                                      $\{2 \neq 0\}$ 
n1 is set to:
                                      $-7 e1^2 - \frac{15}{2} e1 f2 - \frac{3}{2} f2^2$ 
Nonzero constraint refines to:
                                      $6 (-14 e1^2 - 15 e1 f2 - 3 f2^2) e1 \neq 0$ 
> tmp1 := cpcoeff (x1^4*x2^2*x4^2);
                                      $tmp1 := 3 e1 (2 e1 + f2)^3$ 
> elimsolve (tmp1, f2);
                                      $\{1 \neq 0\}$ 
f2 is set to:

```

```

                                -2 e l
Nonzero constraint refines to:
                                12 e l^2 ≠ 0
> tmp1 := cpcoeff (x3^8);
                                tmp1 := 12 e l^5 (n2 + 3 q3)
> elimsolve (tmp1, n2);
                                {1 ≠ 0}
n2 is set to:
                                -3 q3
> tmp1 := cpcoeff (x1^3*x3^3*T);
                                tmp1 := 4 e l^3
> contradict (tmp1);
Contradiction on case level 2, so:
                                e l = 0
Variables to be uneliminated:
                                "n2 := 'n2'"
                                "f2 := 'f2'"
                                "n1 := 'n1'"
Proceed on case level 1 with:
                                6 n l ≠ 0
On account of:
                                e l = 0
                                {1 ≠ 0}
e l is set to:
                                0
> tmp1 := cpcoeff (x1*x3^2*x4*T^2);
                                tmp1 := - $\frac{27 f2^3}{8}$ 
> elimsolve (tmp1, f2);
                                {1 ≠ 0}
f2 is set to:
                                0
> tmp1 := cpcoeff (x1^1*x2^2*x3^3*x4^2);
                                tmp1 := 12 n l^3
> contradict (tmp1);
Contradiction on case level 1, so:
                                n l = 0
Variables to be uneliminated:
                                "f2 := 'f2'"
                                "e1 := 'e1'"
                                "h3 := 'h3'"
                                "q2 := 'q2'"
Proceed on case level 0 with:
                                6 ≠ 0

```

On account of:

$$n1 = 0$$

$$\{1 \neq 0\}$$

n1 is set to:

$$0$$

> **launchNZcase (e1);**

Launching case level 1:

$$e1 \neq 0$$

Assume from now on that:

$$6 e1 \neq 0$$

> **tmp1 := cpcoeff (x1^5\*x2\*x3^2);**

$$tmp1 := -2 e1 (f2^2 + 3 q2)$$

> **elimsolve (tmp1, q2);**

$$\{3 \neq 0\}$$

q2 is set to:

$$-\frac{f2^2}{3}$$

> **tmp1 := cpcoeff (x1^5\*x2^2\*x4);**

$$tmp1 := 2 e1 (12 e1^2 + 12 e1 f2 + 3 f2^2 - 4 e1 h3)$$

> **elimsolve (tmp1, h3);**

$$\{-4 e1 \neq 0\}$$

h3 is set to:

$$\frac{3 (2 e1 + f2)^2}{4 e1}$$

> **tmp1 := cpcoeff (x1^4\*x2^2\*x4^2);**

$$tmp1 := 3 e1 (2 e1 + f2)^3$$

> **elimsolve (tmp1, f2);**

$$\{1 \neq 0\}$$

f2 is set to:

$$-2 e1$$

> **tmp1 := cpcoeff (x1^3\*x3^3\*T);**

$$tmp1 := -8 e1^3$$

> **contradict (tmp1);**

Contradiction on case level 1, so:

$$e1 = 0$$

Variables to be uneliminated:

$$"f2 := 'f2'"$$

$$"h3 := 'h3'"$$

$$"q2 := 'q2'"$$

Proceed on case level 0 with:

$$6 \neq 0$$

On account of:

$$e1 = 0$$

$$\{1 \neq 0\}$$

e1 is set to:

$$0$$

> **launchNZcase (f2);**

Launching case level 1:

$$f2 \neq 0$$

Assume from now on that:

$$6f2 \neq 0$$

> **tmp1 := cpcoeff (x1^3\*x2\*x3\*x4\*T);**

$$tmp1 := 2f2(4f2^2 + 5h3f2 + 4h3^2 + 3q2)$$

> **elimsolve (tmp1, q2);**

$$\{3 \neq 0\}$$

q2 is set to:

$$-\frac{4}{3}f2^2 - \frac{5}{3}h3f2 - \frac{4}{3}h3^2$$

> **tmp1 := cpcoeff (x1^2\*x2\*x3\*x4^2\*T);**

$$tmp1 := 3f2^4$$

> **contradict (tmp1);**

Contradiction on case level 1, so:

$$f2 = 0$$

Variables to be uneliminated:

$$"q2 := 'q2'"$$

Proceed on case level 0 with:

$$6 \neq 0$$

On account of:

$$f2 = 0$$

$$\{1 \neq 0\}$$

f2 is set to:

$$0$$

> **tmp1 := cpcoeff (x3^2\*x4^2\*T^2);**

$$tmp1 := -3(4h3^2 + 3q2)^2$$

> **elimsolve (tmp1, q2);**

$$\{3 \neq 0\}$$

q2 is set to:

$$-\frac{4h3^2}{3}$$

> **tmp1 := cpcoeff (x1^3\*x3^3\*T);**

$$tmp1 := 8h3^3$$

> **elimsolve (tmp1, h3);**

$$\{1 \neq 0\}$$

h3 is set to:

$$0$$

> **launchNZcase (l1);**

Launching case level 1:

$$l1 \neq 0$$

Assume from now on that:

$$6\,l\,l \neq 0$$

> **tmp1 := cpcoeff (x1\*x2^5\*x4^2);**

$$tmp1 := 6\,l\,l^2\,(2\,l\,l + n2)$$

> **elimsolve (tmp1, n2);**

$$\{1 \neq 0\}$$

n2 is set to:

$$-2\,l\,l$$

> **tmp1 := cpcoeff (x2^2\*x4^2\*T^2);**

$$tmp1 := -4\,l\,l^2$$

> **contradict (tmp1);**

Contradiction on case level 1, so:

$$l\,l = 0$$

Variables to be uneliminated:

$$n2 := 'n2'$$

Proceed on case level 0 with:

$$6 \neq 0$$

On account of:

$$l\,l = 0$$

$$\{1 \neq 0\}$$

l1 is set to:

$$0$$

> **tmp1 := cpcoeff (x2^2\*x4^2\*T^2);**

$$tmp1 := -4\,n2^2$$

> **elimsolve (tmp1, n2);**

$$\{1 \neq 0\}$$

n2 is set to:

$$0$$

> **tmp1 := cpcoeff (x3^4\*T^2);**

$$tmp1 := -9\,q3^2$$

> **elimsolve (tmp1, q3);**

$$\{1 \neq 0\}$$

q3 is set to:

$$0$$

> **launchNZcase (k1);**

Launching case level 1:

$$k\,l \neq 0$$

Assume from now on that:

$$6\,k\,l \neq 0$$

> **tmp1 := cpcoeff (x1^4\*x2^4);**

$$tmp1 := -3\,k\,l\,(l2 + 4\,e2^2 + 3\,k\,l)$$

> **elimsolve (tmp1, l2);**

$$\{1 \neq 0\}$$

l2 is set to:

$$-4\,e2^2 - 3\,k\,l$$

```

> launchNZcase (3*k1+4*e2^2);
Launching case level 2:


$$4 e2^2 + 3 k1 \neq 0$$


Assume from now on that:


$$6 k1 (4 e2^2 + 3 k1) \neq 0$$

> tmp1 := cpcoeff (x1^3*x2^3*T);

$$tmp1 := 4 e2^2 f3 + 3 k1 f3 + 8 e2^3$$

> elimsolve (tmp1, f3);

$$\{4 e2^2 + 3 k1 \neq 0\}$$

f3 is set to:

$$-\frac{8 e2^3}{4 e2^2 + 3 k1}$$

> tmp1 := cpcoeff (x2^7*x4);

$$tmp1 := \frac{288 e2^5 k1^2 (-n3 + 4 e2^2)}{(4 e2^2 + 3 k1)^2}$$

> tmp2 := cpcoeff (x2^3*x4*T^2);

$$tmp2 := \frac{96 e2^4 k1 n3}{(4 e2^2 + 3 k1)^2}$$

> tmp3 := factor (tmp1 + 3*e2*k1*tmp2);

$$tmp3 := \frac{1152 e2^7 k1^2}{(4 e2^2 + 3 k1)^2}$$

> elimsolve (tmp3, e2);

$$\{1 \neq 0\}$$

e2 is set to:

$$0$$

Nonzero constraint refines to:

$$18 k1^2 \neq 0$$

> tmp1 := cpcoeff (x1*x2^6*x3);

$$tmp1 := -36 k1^2 (-n3 + 3 k1)$$

> tmp2 := cpcoeff (x1^2*x2^3*x3*T);

$$tmp2 := 6 k1 n3$$

> tmp3 := factor (tmp1 - 6*k1*tmp2);

$$tmp3 := -108 k1^3$$

> contradict (tmp3, k1);
Contradiction on case level 2, so:

$$4 e2^2 + 3 k1 = 0$$

Variables to be uneliminated:

$$"e2 := 'e2'"$$


$$"f3 := 'f3'"$$

Proceed on case level 1 with:

$$6 k1 \neq 0$$


```



On account of:

$$4 e2^2 + 3 k1 = 0$$
$$\{3 \neq 0\}$$

k1 is set to:

$$-\frac{4 e2^2}{3}$$

Nonzero constraint refines to:

$$-12 e2 \neq 0$$

> **tmp1 := cpcoeff (x1^3\*x2^3\*T);**

$$tmp1 := 8 e2^3$$

> **contradict (tmp1);**

Contradiction on case level 1, so:

$$k1 = 0$$

Variables to be uneliminated:

"k1 := 'k1'"

"l2 := 'l2'"

Proceed on case level 0 with:

$$6 \neq 0$$

On account of:

$$k1 = 0$$

$$\{1 \neq 0\}$$

k1 is set to:

$$0$$

> **launchNZcase (l2);**

Launching case level 1:

$$l2 \neq 0$$

Assume from now on that:

$$6 l2 \neq 0$$

> **tmp1 := cpcoeff (x1^3\*x2^3\*T);**

$$tmp1 := -4 l2 e2 - l2 f3 - 8 e2^3$$

> **elimsolve (tmp1, f3);**

$$\{l2 \neq 0\}$$

f3 is set to:

$$-\frac{4 e2 (l2 + 2 e2^2)}{l2}$$

> **tmp1 := cpcoeff (x2^4\*x3\*x4\*T);**

$$tmp1 := \frac{6 (4 e2^2 + l2)^3 (n3 + l2)}{l2}$$

> **tmp2 := cpcoeff (x2^3\*x4\*T^2);**

$$tmp2 := -\frac{2 (4 e2^2 + l2)^3 n3}{l2^2}$$

> **tmp3 := factor (tmp1 + 3\*l2\*tmp2);**

$$tmp3 := 6 (4 e2^2 + l2)^3$$

```
> elimsolve (tmp3,12);
```

 $\{1 \neq 0\}$ 

12 is set to:

$$-4 e 2^2$$

Nonzero constraint refines to:

$$-12\,e2 \neq 0$$

```
> tmp1 := cpcoeff (x1*x2^2*x3*T^2);
```

$$tmp1 := 4 \ e2 \ (n3 + 2 \ e2^2)$$

```
> elimsolve (tmp1, n3);
```

 $\{1 \neq 0\}$ 

n3 is set to:

$$-2\,e2^2$$

```
> tmp1 := cpcoeff (x2^3*x3^3*T);
```

$$tmp1 := -288\ e2^6$$

```
> contradict (tmp1);
```

Contradiction on case level 1, so:

$$l2 = 0$$

Variables to be uneliminated:

"n3 := 'n3'"

"12 := '12'"

"f3 := 'f3'"

Proceed on case level 0 with:

$$6 \neq 0$$

On account of:

$$l2 = 0$$
 $\{1 \neq 0\}$ 

12 is set to:

0

```
> tmp1 := cpcoeff (x1^3*x2^3*T);
```

$$tmp1 := -8 \, e2^3$$

```
> elimsolve (tmp1, e2);
```

 $\{1 \neq 0\}$ 

e2 is set to:

0

```
> launchNZcase (f3);
```

Launching case level 1:

$$f_3 \neq 0$$

Assume from now on that:

$$6.f3 \neq 0$$

```
> tmp1 := cpcoeff (x2^3*x4*T^2);
```

$$tmp1 := -2 \cdot f3^2 \cdot n3$$

```
> elimsolve (tmp1, n3);
```

 $\{1 \neq 0\}$ 

n3 is set to:

```

[
  0
  > tmp1 := cpcoeff (x2^2*x3^2*T^2);
                                     tmp1 := 3 f3^2 q4
  > elimsolve (tmp1, q4);
                                     {1 ≠ 0}
  q4 is set to:
                                     0
  > tmp1 := cpcoeff (x2^3*x3*T^2);
                                     tmp1 := 2 f3^2 n4
  > elimsolve (tmp1, n4);
                                     {1 ≠ 0}
  n4 is set to:
                                     0
  > tmp1 := cpcoeff (x1*x2^2*x3*T^2);
                                     tmp1 := 2 f3^2 h4
  > elimsolve (tmp1, h4);
                                     {1 ≠ 0}
  h4 is set to:
                                     0
  > tmp1 := cpcoeff (x1*x2^3*T^2);
                                     tmp1 := -f3 (-f4 f3 + 2 l3 + 3 k2)
  > elimsolve (tmp1, l3);
                                     {2 ≠ 0}
  l3 is set to:
                                      $\frac{f4 f3}{2} - \frac{3 k2}{2}$ 
  > tmp1 := cpcoeff (x2^4*T^2);
                                     tmp1 :=  $-\frac{f4^2 f3^2}{4} - \frac{27 k2^2}{4} + f3^2 l4$ 
  > elimsolve (tmp1, l4);
                                     { $-4 f3^2 \neq 0$ }
  l4 is set to:
                                      $\frac{f4^2 f3^2 + 27 k2^2}{4 f3^2}$ 
  > tmp1 := cpcoeff (x2^6*T);
                                     tmp1 :=  $-27 k2^3$ 
  > elimsolve (tmp1, k2);
                                     {1 ≠ 0}
  k2 is set to:
                                     0
  > det (T - jacobian (H,[x1,x2,x3,x4]));
                                     T^4
]

```

> **H;**

$$\left[ 0, \frac{x_1^3}{3}, x_1^2 x_2 + e_3 x_1 x_2^2 + f_3 x_1 x_2 x_3 + k_3 x_2^3 + \frac{f_4 f_3 x_2^2 x_3}{2} - f_3^2 x_2^2 x_4, \right. \\ \left. x_1^2 x_3 + e_4 x_1 x_2^2 + f_4 x_1 x_2 x_3 - f_3 x_1 x_2 x_4 + k_4 x_2^3 + \frac{f_4^2 x_2^2 x_3}{4} - \frac{f_4 f_3 x_2^2 x_4}{2} \right]$$

> **G := [0, 0, x1\*x2\*x3-x2^2\*x4, x1^2\*x3-x1\*x2\*x4] +**  
 > **x1^3\*[0, f3/(3\*C^4), 0, 0] + x1^2\*x2\*[0, 0, 1, -C^2\*f4/(2\*f3)] +**  
 > **x1\*x2^2\*[0, 0, C^2\*e3/f3, C^4\*(e4/f3-f4\*e3/(2\*f3^2))] +**  
 > **x2^3\*[0, 0, C^4\*k3/f3^2, C^6\*(k4/f3^2-f4\*k3/(2\*f3^3))];**

$$G := [0, 0, x_1 x_2 x_3 - x_2^2 x_4, x_1^2 x_3 - x_1 x_2 x_4] + x_1^3 \left[ 0, \frac{f_3}{3 C^4}, 0, 0 \right] \\ + x_1^2 x_2 \left[ 0, 0, 1, -\frac{C^2 f_4}{2 f_3} \right] + x_1 x_2^2 \left[ 0, 0, \frac{C^2 e_3}{f_3}, C^4 \left( \frac{e_4}{f_3} - \frac{f_4 e_3}{2 f_3^2} \right) \right] \\ + x_2^3 \left[ 0, 0, \frac{C^4 k_3}{f_3^2}, C^6 \left( \frac{k_4}{f_3^2} - \frac{f_4 k_3}{2 f_3^3} \right) \right]$$

> **M := evalm ([C, 0, 0, 0], [0, f3/C, 0, 0],**  
 > **[0, 0, C\*f3, 0], [0, 0, -C^3\*f4/2, C^3\*f3]);**

$$M := \begin{bmatrix} C & 0 & 0 & 0 \\ 0 & \frac{f_3}{C} & 0 & 0 \\ 0 & 0 & C f_3 & 0 \\ 0 & 0 & -\frac{C^3 f_4}{2} & C^3 f_3 \end{bmatrix}$$

> **evalm(simplify(evalm(M^(-1) &\* subs({seq([x1,x2,x3,x4][i] =**  
 > **evalm(M&\*[x1,x2,x3,x4])[i], i=1..4)}, G) - H));**  
 [0, 0, 0, 0]

> **factor(evalm([0, 0, 0, 1] &\* jacobian(G, [x1,x2,x3,x4])^3 &\***  
 > **[x1,x2,x3,x4]));**

$$x_1^4 (2 x_1^2 f_3^3 x_3 - 2 x_1 f_3^3 x_2 x_4 + 2 x_1^3 f_3^3 + 4 x_1^2 f_3^2 x_2 C^2 e_3 + 6 x_1 f_3 x_2^2 C^4 k_3 \\ + x_2 x_1^2 C^2 f_4 f_3^2 - 4 x_1 x_2^2 C^4 f_3^2 e_4 + 2 x_1 x_2^2 C^4 f_3 f_4 e_3 - 6 x_2^3 C^6 k_4 f_3 + 3 x_2^3 C^6 f_4 k_3) \\ / (2 f_3^2 C^4)$$

> **contradict (1);**

Contradiction on case level 1, so:

$$f_3 = 0$$

Variables to be uneliminated:

"k2 := 'k2'"

"l4 := 'l4'"

"l3 := 'l3'"

"h4 := 'h4'"

"n4 := 'n4'"

"q4 := 'q4'"

```

                                "n3 := 'n3'"
Proceed on case level 0 with:
                                6 ≠ 0
On account of:
                                f3 = 0
                                {1 ≠ 0}
f3 is set to:
                                0
> tmp1 := cpcoeff (x2^2*x3^2*T^2);
                                tmp1 := -4 n3^2
> elimsolve (tmp1, n3);
                                {1 ≠ 0}
n3 is set to:
                                0
> tmp1 := cpcoeff (x2^6*T);
                                tmp1 := 3 k2 l3 (l3 + 3 k2)
> tmp2 := cpcoeff (x2^4*T^2);
                                tmp2 := -l3^2 - 3 k2 l3 - 9 k2^2
> tmp3 := factor (tmp1 + l3*tmp2);
                                tmp3 := -l3^3
> elimsolve (tmp3, l3);
                                {1 ≠ 0}
l3 is set to:
                                0
> tmp1 := cpcoeff (x2^4*T^2);
                                tmp1 := -9 k2^2
> elimsolve (tmp1, k2);
                                {1 ≠ 0}
k2 is set to:
                                0
> det (T - jacobian (H,[x1,x2,x3,x4]));
                                T^4
> H;
[ 0,  $\frac{x1^3}{3}$ ,  $x1^2 x2 + e3 x1 x2^2 + k3 x2^3$ ,
 $x1^2 x3 + e4 x1 x2^2 + f4 x1 x2 x3 + h4 x1 x3^2 + k4 x2^3 + l4 x2^2 x3 + n4 x2 x3^2 + q4 x3^3$  ]
> jacobian (H,[x1,x2,x3,x4]);
[0, 0, 0, 0]
[ $x1^2$ , 0, 0, 0]
[ $2 x1 x2 + e3 x2^2$ ,  $x1^2 + 2 e3 x1 x2 + 3 k3 x2^2$ , 0, 0]
[ $2 x1 x3 + e4 x2^2 + f4 x2 x3 + h4 x3^2$ ,  $2 e4 x1 x2 + f4 x1 x3 + 3 k4 x2^2 + 2 l4 x2 x3 + n4 x3^2$ ,

```

$$x1^2 + f4 x1 x2 + 2 h4 x1 x3 + l4 x2^2 + 2 n4 x2 x3 + 3 q4 x3^2, 0]$$

> **contradict (1);**

Contradiction on case level 0, so:

$$6 = 0$$

Variables to be uneliminated:

"k2 := 'k2'"

"l3 := 'l3'"

"n3 := 'n3'"

"f3 := 'f3'"

"e2 := 'e2'"

"l2 := 'l2'"

"k1 := 'k1'"

"q3 := 'q3'"

"n2 := 'n2'"

"l1 := 'l1'"

"h3 := 'h3'"

"q2 := 'q2'"

"f2 := 'f2'"

"e1 := 'e1'"

"n1 := 'n1'"

"q1 := 'q1'"

"f1 := 'f1'"

"h2 := 'h2'"

"h1 := 'h1'"

"t1 := 't1'"

"s1 := 's1'"

"r1 := 'r1'"

"p1 := 'p1'"

"o1 := 'o1'"

"m1 := 'm1'"

"j1 := 'j1'"

"i1 := 'i1'"

"g1 := 'g1'"

"t2 := 't2'"

"s2 := 's2'"

"r2 := 'r2'"

"p2 := 'p2'"

"o2 := 'o2'"

"m2 := 'm2'"

"j2 := 'j2'"

```

"i2 := 'i2'"
"g2 := 'g2'"
"t3 := 't3'"
"s3 := 's3'"
"r3 := 'r3'"
"p3 := 'p3'"
"o3 := 'o3'"
"m3 := 'm3'"
"j3 := 'j3'"
"i3 := 'i3'"
"g3 := 'g3'"
"t4 := 't4'"
"s4 := 's4'"
"r4 := 'r4'"
"p4 := 'p4'"
"o4 := 'o4'"
"m4 := 'm4'"
"j4 := 'j4'"
"i4 := 'i4'"
"g4 := 'g4'"

```

That is all, folks! Check that all variables are uneliminated:

```

[[a1, b1, c1, d1, e1, f1, g1, h1, i1, j1, k1, l1, m1, n1, o1, p1, q1, r1, s1, t1],
 [a2, b2, c2, d2, e2, f2, g2, h2, i2, j2, k2, l2, m2, n2, o2, p2, q2, r2, s2, t2],
 [a3, b3, c3, d3, e3, f3, g3, h3, i3, j3, k3, l3, m3, n3, o3, p3, q3, r3, s3, t3],
 [a4, b4, c4, d4, e4, f4, g4, h4, i4, j4, k4, l4, m4, n4, o4, p4, q4, r4, s4, t4]]

```

**> startnewHcase ();**

Starting case H = H2:

```

[ x1^2 x4 + e1 x1 x2^2 + f1 x1 x2 x3 + g1 x1 x2 x4 + h1 x1 x3^2 + i1 x1 x3 x4 + j1 x1 x4^2 + k1 x2^3
  + l1 x2^2 x3 + m1 x2^2 x4 + n1 x2 x3^2 + o1 x2 x3 x4 + p1 x2 x4^2 + q1 x3^3 + r1 x3^2 x4 + s1 x3 x4^2
  + t1 x4^3, x1^3/3 + e2 x1 x2^2 + f2 x1 x2 x3 + g2 x1 x2 x4 + h2 x1 x3^2 + i2 x1 x3 x4 + j2 x1 x4^2
  + k2 x2^3 + l2 x2^2 x3 + m2 x2^2 x4 + n2 x2 x3^2 + o2 x2 x3 x4 + p2 x2 x4^2 + q2 x3^3 + r2 x3^2 x4
  + s2 x3 x4^2 + t2 x4^3, x1^2 x2 + e3 x1 x2^2 + f3 x1 x2 x3 + g3 x1 x2 x4 + h3 x1 x3^2 + i3 x1 x3 x4
  + j3 x1 x4^2 + k3 x2^3 + l3 x2^2 x3 + m3 x2^2 x4 + n3 x2 x3^2 + o3 x2 x3 x4 + p3 x2 x4^2 + q3 x3^3
  + r3 x3^2 x4 + s3 x3 x4^2 + t3 x4^3, e4 x1 x2^2 + f4 x1 x2 x3 + g4 x1 x2 x4 + h4 x1 x3^2 + i4 x1 x3 x4
  + j4 x1 x4^2 + k4 x2^3 + l4 x2^2 x3 + m4 x2^2 x4 + n4 x2 x3^2 + o4 x2 x3 x4 + p4 x2 x4^2 + q4 x3^3
  + r4 x3^2 x4 + s4 x3 x4^2 + t4 x4^3 ]

```

```
> initcases (6);
```

We assume the following in our calculation:

$$6 \neq 0$$

```
> for i from 1 by -1 to 0 do
```

```
>   for j from 2-i by -1 to 0 do
```

```
>     for k from 0 to 2-i-j do
```

```
>       v := coeff (coeff (coeff (coeff (H[3],
```

```
>                                     x1,i),x2,j),x3,3-i-j-k),x4,k);
```

```
>       m := cpcoeff (x1^i * x2^j * x3^(2-i-j-k) * x4^k * T^3);
```

```
>       elimsolve (m,v);
```

```
>     od;
```

```
>   od;
```

```
> od;
```

$$\{1 \neq 0\}$$

f3 is set to:

$$-2 e2 - g4$$

$$\{2 \neq 0\}$$

h3 is set to:

$$-\frac{f2}{2} - \frac{i4}{2}$$

$$\{1 \neq 0\}$$

i3 is set to:

$$-2 j4 - 2 - g2$$

$$\{1 \neq 0\}$$

l3 is set to:

$$-m4 - e1 - 3 k2$$

$$\{2 \neq 0\}$$

n3 is set to:

$$-l2 - \frac{f1}{2} - \frac{o4}{2}$$

$$\{1 \neq 0\}$$

o3 is set to:

$$-2 p4 - 2 m2 - g1$$

$$\{3 \neq 0\}$$

q3 is set to:

$$-\frac{h1}{3} - \frac{r4}{3} - \frac{n2}{3}$$

$$\{2 \neq 0\}$$

r3 is set to:

$$-s4 - \frac{i1}{2} - \frac{o2}{2}$$

$$\{1 \neq 0\}$$

s3 is set to:

$$-p2 - j1 - 3 t4$$



```

> for i from 1 by -1 to 0 do
>   for j from 2-i by -1 to 0 do
>     for k from 0 to 2-i-j do
>       v := coeff (coeff (coeff (coeff (H[2],
>                                     x1,i),x2,j),x3,3-i-j-k),x4,k);
>       m := cpcoeff (x1^(i+2) * x2^j * x3^(2-i-j-k) * x4^k *
>                     T^2);
>       elimsolve (m,v);
>     od;
>   od;
> od;

```

f2 is set to:  $\{1 \neq 0\}$

$$-2\,el$$

h2 is set to:  $\{2 \neq 0\}$

$$-\frac{fl}{2}$$

i2 is set to:  $\{1 \neq 0\}$

$$-gl$$

l2 is set to:  $\{-1 \neq 0\}$

$$-4\,e2^2 - 2\,e2\,g4 - e4 - g3\,f4 - g4^2 - 3\,kl - 2\,fl - 2\,e4\,g2 + 4\,el\,e3$$

n2 is set to:  $\{-2 \neq 0\}$

$$f4\,j4 + \frac{f4}{2} - g4\,i4 - l1 - 2\,h1 - h4\,g3 - e2\,i4 + 2\,e2\,el + e3\,fl + e4\,gl$$

$$\{-1 \neq 0\}$$

o2 is set to:

$$-4\,g4\,j4 - 3\,g4 - 2\,g4\,g2 - 2\,j3\,f4 + 2\,e3\,gl - 2\,il - 2\,ml - 4\,j4\,e2 - 4\,e2 - 4\,e2\,g2 + 2\,el\,g3 \\ - g3\,i4 - 4\,e4\,j2$$

$$\{3 \neq 0\}$$

q2 is set to:

$$-\frac{n1}{3} + \frac{2\,el\,i4}{3} + \frac{4\,h4\,j4}{3} + h4 + \frac{2\,h4\,g2}{3} - \frac{i4^2}{3} - \frac{4\,el^2}{3} - \frac{2\,fl\,e2}{3} - \frac{fl\,g4}{3} + \frac{f4\,gl}{3}$$

$$\{-2 \neq 0\}$$

r2 is set to:

$$2\,el\,j4 - j4\,i4 - 2\,j3\,h4 - j2\,f4 - \frac{o1}{2} - \frac{i4}{2} + 2\,el + 2\,el\,g2 - gl\,e2 + \frac{g3\,fl}{2}$$

$$\{-1 \neq 0\}$$

s2 is set to:

$$-p1 - 2\,g2\,j4 - 4\,j4^2 - 5\,j4 - 2\,j3\,i4 - 2\,g2 - g2^2 + g3\,gl - 4 - 2\,j2\,g4$$

```

> for i from 1 by -1 to 0 do

```

```

> for j from 2-i by -1 to 0 do
>   for k from 0 to 2-i-j do
>     v := coeff (coeff (coeff (coeff (H[1],
>                                     x1,i),x2,j),x3,3-i-j-k),x4,k);
>     m := cpcoeff (x1^(i+4) * x2^j * x3^(2-i-j-k) * x4^k * T);
>     elimsolve (m,v);
>   od;
> od;
> od;

```

```

f1 is set to:

```

$$\{1 \neq 0\}$$

```

h1 is set to:

```

$$-2 e4$$

```

i1 is set to:

```

$$\{1 \neq 0\}$$

```

l1 is set to:

```

$$-g4$$

```

n1 is set to:

```

$$-4 e2 e1 - 2 e1 g4 - 2 f4 - 3 k4 + 4 e3 e4 - 2 e4 g1 - f4 g2$$

```

o1 is set to:

```

$$2 e1^2 - e1 i4 + e3 f4 + e4 g4 - h4 g2 - 2 h4 - l4$$

```

p1 is set to:

```

$$-2 m4 - 4 e1 j4 - 8 e1 - 2 e1 g2 - 4 e4 j1 + 2 e3 g4 - g2 i4 + 2 g3 e4 - 2 i4 - 2 j2 f4 - 2 g1 e2$$

```

q1 is set to:

```

$$-\frac{2 e2 f4}{3} - \frac{n4}{3} - \frac{4 e4 e1}{3} + \frac{2 e4 i4}{3} + \frac{2 h4 g1}{3}$$

```

r1 is set to:

```

$$g1 e1 + 2 e4 j4 + 4 e4 + e4 g2 - \frac{o4}{2} - e2 g4 + \frac{g3 f4}{2} - 2 j2 h4 - f4 j1$$

```

s1 is set to:

```

$$-2 g1 j4 - 4 g1 - g1 g2 - p4 + g3 g4 - 2 j2 i4 - 2 j1 g4$$

```

> for i from 1 by -1 to 0 do
>   for j from 2-i by -1 to 0 do
>     for k from 0 to 2-i-j do
>       v := coeff (coeff (coeff (coeff (H[4],

```

```

>                                     x1,i),x2,j),x3,3-i-j-k),x4,k);
>      m := cpcoeff (x1^(i+6) * x2^j * x3^(2-i-j-k) * x4^k);
>      elimsolve (m,v);
>      od;
>      od;
>      od;

```

```

                                     {1 ≠ 0}
f4 is set to:

```

0

{1 ≠ 0}

```

h4 is set to:

```

0

{1 ≠ 0}

```

i4 is set to:

```

0

{1 ≠ 0}

```

l4 is set to:

```

$-4 e4 (g4 + e2)$

{-1 ≠ 0}

```

n4 is set to:

```

$2 e4 e1$

{1 ≠ 0}

```

o4 is set to:

```

$-8 e4 j4 - 2 g4^2 - 4 e4 - 2 e4 g2 - 2 e2 g4$

{1 ≠ 0}

```

q4 is set to:

```

0

{-1 ≠ 0}

```

r4 is set to:

```

$e1 g4$

{1 ≠ 0}

```

s4 is set to:

```

$-g4 (4 j4 + 2 + g2)$

```

> launchNZcase (e1);

```

```

Launching case level 1:

```

$e1 \neq 0$

```

Assume from now on that:

```

$6 e1 \neq 0$

```

> tmp1 := cpcoeff (x3^3*x1^5);

```

$tmp1 := 4 e4 e1^2$

```

> elimsolve (tmp1,e4);

```

{1 ≠ 0}

```

e4 is set to:

```

0

```

> tmp1 := cpcoeff (x3^3*x1^3*T);

```

```

[                                      $tmp1 := 4 e1^3$ 
> contradict (tmp1);
Contradiction on case level 1, so:
                                      $e1 = 0$ 
Variables to be uneliminated:
                                     "e4 := 'e4'"
Proceed on case level 0 with:
                                      $6 \neq 0$ 
On account of:
                                      $e1 = 0$ 
                                      $\{1 \neq 0\}$ 
e1 is set to:
                                     0
> launchNZcase (e4);
Launching case level 1:
                                      $e4 \neq 0$ 
Assume from now on that:
                                      $6 e4 \neq 0$ 
> tmp1 := cpcoeff (x1^3*x3^3*T);
                                      $tmp1 := 6 e4 (k4 - 2 e3 e4 + e4 g1)$ 
> elimsolve (tmp1, k4);
                                      $\{1 \neq 0\}$ 
k4 is set to:
                                      $-e4 (-2 e3 + g1)$ 
> tmp1 := cpcoeff (x1^3*x2^1*x3^2*T);
                                      $tmp1 := -3 e4 (4 e4 j4 + 2 e4 g2 + 3 g4^2 + 2 k1)$ 
> elimsolve (tmp1, k1);
                                      $\{2 \neq 0\}$ 
k1 is set to:
                                      $-2 e4 j4 - e4 g2 - \frac{3 g4^2}{2}$ 
> tmp1 := cpcoeff (x1^1*x3^3*T^2);
                                      $tmp1 := -2 e4 (4 e2^2 + 6 e2 g4 - g4^2 - 2 e4 j4 - e4)$ 
> tmp2 := cpcoeff (x1^5*x2^2*x3^1);
                                      $tmp2 := 6 e4 (4 e2^2 + 6 e2 g4 + g4^2 - e4)$ 
> tmp3 := factor (3*tmp1 + tmp2);
                                      $tmp3 := 12 e4 (g4^2 + e4 j4)$ 
> elimsolve (tmp3, j4);
                                      $\{e4 \neq 0\}$ 
j4 is set to:
                                      $-\frac{g4^2}{e4}$ 
> tmp1 := cpcoeff (x1^3*x3^2*x4*T);

```

$$tmp1 := -4 e4 m1 - 3 g4^2 e2 + 4 g4 e2^2 - 11 g4 g2 e4 + 4 e3 g1 e4 - 4 e2 g2 e4 + \frac{61 g4^3}{2}$$

$$- 8 e4^2 j2 - 28 e4 g4$$

> **elimsolve** (tmp1, m1);

$$\{-8 e4 \neq 0\}$$

m1 is set to:

$$\frac{-6 g4^2 e2 + 8 g4 e2^2 - 22 g4 g2 e4 + 8 e3 g1 e4 - 8 e2 g2 e4 + 61 g4^3 - 16 e4^2 j2 - 56 e4 g4}{8 e4}$$

> **tmp1 := cpcoeff** (x1\*x3^3\*T^2);

$$tmp1 := -2 e4 (4 e2^2 + 6 e2 g4 + g4^2 - e4)$$

> **elimsolve** (tmp1, e4);

$$\{-1 \neq 0\}$$

e4 is set to:

$$4 e2^2 + 6 e2 g4 + g4^2$$

Nonzero constraint refines to:

$$24 e2^2 + 36 e2 g4 + 6 g4^2 \neq 0$$

> **launchNZcase** (3\*g4+4\*e2);

Launching case level 2:

$$3 g4 + 4 e2 \neq 0$$

Assume from now on that:

$$6 (4 e2^2 + 6 e2 g4 + g4^2) (3 g4 + 4 e2) \neq 0$$

> **tmp1 := cpcoeff** (x1^5\*x2\*x3\*x4);

$$tmp1 := \frac{3 (3 g4 + 4 e2) (16 e2^2 + 8 g2 e2^2 + 18 e2 g4 + 12 g2 e2 g4 - 9 g4^2 + 2 g2 g4^2)}{2}$$

> **elimsolve** (tmp1, g2);

$$\{8 e2^2 + 12 e2 g4 + 2 g4^2 \neq 0\}$$

g2 is set to:

$$-\frac{(2 e2 + 3 g4) (8 e2 - 3 g4)}{2 (4 e2^2 + 6 e2 g4 + g4^2)}$$

> **launchNZcase** (g4);

Launching case level 3:

$$g4 \neq 0$$

Assume from now on that:

$$6 (4 e2^2 + 6 e2 g4 + g4^2) (3 g4 + 4 e2) g4 \neq 0$$

> **launchNZcase** (e2 + 2\*g4);

Launching case level 4:

$$e2 + 2 g4 \neq 0$$

Assume from now on that:

$$6 (4 e2^2 + 6 e2 g4 + g4^2) (3 g4 + 4 e2) g4 (e2 + 2 g4) \neq 0$$

> **tmp1 := cpcoeff** (x1^5\*x3\*x4^2);

$$tmp1 := -\frac{g4^2 (e2 + 2 g4) (2 e2 - g4)}{4 e2^2 + 6 e2 g4 + g4^2}$$

> **elimsolve** (tmp1, e2);

```

{2 ≠ 0}
e2 is set to:

$$\frac{g^4}{2}$$

Nonzero constraint refines to:

$$750 g^4 \neq 0$$

> tmp1 := cpcoeff (x1^2*x3^3*x4*T);

$$tmp1 := -256 g^4$$

> contradict (tmp1,'e2');
Contradiction on case level 4, so:

$$e2 + 2 g^4 = 0$$

Variables to be uneliminated:
"e2 := 'e2'"
Proceed on case level 3 with:

$$6 (4 e2^2 + 6 e2 g^4 + g^4^2) (3 g^4 + 4 e2) g^4 \neq 0$$

On account of:

$$e2 + 2 g^4 = 0$$


$$\{1 \neq 0\}$$

e2 is set to:

$$-2 g^4$$

Nonzero constraint refines to:

$$-150 g^4^3 \neq 0$$

> tmp1 := cpcoeff (x1*x2*x3^4*T);

$$tmp1 := -1200 g^4^6$$

> contradict (tmp1);
Contradiction on case level 3, so:

$$g^4 = 0$$

Variables to be uneliminated:
"e2 := 'e2'"
Proceed on case level 2 with:

$$6 (4 e2^2 + 6 e2 g^4 + g^4^2) (3 g^4 + 4 e2) \neq 0$$

On account of:

$$g^4 = 0$$


$$\{1 \neq 0\}$$

g4 is set to:

$$0$$

Nonzero constraint refines to:

$$24 e2^2 \neq 0$$

> tmp1 := cpcoeff (x3^4*T^2);

$$tmp1 := -64 e2^5$$

> contradict (tmp1,'e2');
Contradiction on case level 2, so:

$$3 g^4 + 4 e2 = 0$$

Variables to be uneliminated:
"g4 := 'g4'"

```

Proceed on case level 1 with:

$$24 e^2 + 36 e^2 g^4 + 6 g^4 \neq 0$$

$$3g^4 + 4e^2 = 0$$

$$\{4 \neq 0\}$$

$$-\frac{3g^4}{4}$$

Nonzero constraint refines to:

```
> tmp1 := cpcoeff (x1^4*x2^2*x3^2);
```

$$tmp1 := -\frac{15\,g4^5}{2}$$

$$e4 = 0$$

$$6 \neq 0$$

$$e4 = 0$$

$\{1 \neq 0\}$

e4 is set to:

```
> tmp1 := cpcoeff (x3^4*T^2);
```

$$tmp1 := -9 \, k4^2$$

$$\{1 \neq 0\}$$

0

$$tmp1 := g4 (g4^2 + 5 e2 g4 + 4 e2^2 + 3 kl)$$

$$tmp2 := 2\,g4\,(4\,g4^2 + 5\,e2\,g4 + 4\,e2^2 + 3\,kl)$$

$$tmp3 := -6 \, g4^3$$

```

> elimsolve (tmp3,g4);
                                     {1 ≠ 0}
g4 is set to:
                                     0
> tmp1 := cpcoeff (x2^2*x3^2*T^2);
                                      $tmp1 := -3 (4 e2^2 + 3 kl)^2$ 
> elimsolve (tmp1, k1);
                                     {3 ≠ 0}
k1 is set to:
                                      $-\frac{4 e2^2}{3}$ 
> tmp1 := cpcoeff (x1^3*x2^3*T);
                                      $tmp1 := 8 e2^3$ 
> elimsolve (tmp1,e2);
                                     {1 ≠ 0}
e2 is set to:
                                     0
> tmp1 := cpcoeff (x2*x3^2*x4*T^2);
                                      $tmp1 := 2 m4 (m4 + 6 k2)$ 
> tmp2 := cpcoeff (x1^2*x2^2*x3*x4*T^1);
                                      $tmp2 := -2 m4 (-m4 + 3 k2)$ 
> tmp3 := factor (tmp1 + 2*tmp2);
                                      $tmp3 := 6 m4^2$ 
> elimsolve (tmp3, m4);
                                     {1 ≠ 0}
m4 is set to:
                                     0
> tmp1 := cpcoeff (x2^4*T^2);
                                      $tmp1 := -9 k2^2$ 
> elimsolve (tmp1, k2);
                                     {1 ≠ 0}
k2 is set to:
                                     0
> tmp1 := cpcoeff (x3^2*x4^2*T^2);
                                      $tmp1 := -4 (e3 gl - m1)^2$ 
> elimsolve (tmp1, m1);
                                     {-1 ≠ 0}
m1 is set to:
                                      $e3 gl$ 
> launchNZcase (g1);
Launching case level 1:
                                      $gl \neq 0$ 
Assume from now on that:

```



```

[
  > tmp1 := cpcoeff (x1*x3*x4^2*T^2);
                                      $6\,g1 \neq 0$ 
                                      $tmp1 := -g1\,(p4 + 2\,m2)$ 
  > elimsolve (tmp1, m2);
                                      $\{2 \neq 0\}$ 
  m2 is set to:
                                      $-\frac{p4}{2}$ 
  > tmp1 := cpcoeff (x1*x2^2*x4*T^2);
                                      $tmp1 := 3\,k3\,g1$ 
  > elimsolve (tmp1, k3);
                                      $\{1 \neq 0\}$ 
  k3 is set to:
                                     0
  > tmp1 := cpcoeff (x2*x3*x4^2*T^2);
                                      $tmp1 := 2\,g1^2\,e3$ 
  > elimsolve (tmp1, e3);
                                      $\{1 \neq 0\}$ 
  e3 is set to:
                                     0
  > tmp1 := cpcoeff (x1^3*x2*x4^2*T);
                                      $tmp1 := -2\,g1\,p4$ 
  > elimsolve (tmp1, p4);
                                      $\{1 \neq 0\}$ 
  p4 is set to:
                                     0
  > tmp1 := cpcoeff (x2^2*x4^2*T^2);
                                      $tmp1 := -g1^2$ 
  > contradict (tmp1);
  Contradiction on case level 1, so:
                                      $g1 = 0$ 
  Variables to be uneliminated:
                                     "p4 := 'p4'"
                                     "e3 := 'e3'"
                                     "k3 := 'k3'"
                                     "m2 := 'm2'"
  Proceed on case level 0 with:
                                      $6 \neq 0$ 
  On account of:
                                      $g1 = 0$ 
                                      $\{1 \neq 0\}$ 
  g1 is set to:
                                     0
  > tmp1 := cpcoeff (x1^2*x2*x3*x4^4);

```

```

[
    tmp1 := 6 (p4 + m2) p4^2
> tmp2 := cpcoeff (x1^2*x3*x4^3*T);
    tmp2 := -2 m2 p4
> tmp3 := factor (tmp1 + 3*p4*tmp2);
    tmp3 := 6 p4^3
> elimsolve (tmp3, p4);
    {1 ≠ 0}
p4 is set to:
    0
> tmp1 := cpcoeff (x3*x4^3*T^2);
    tmp1 := -2 m2 (p1 + 2 g2 j4 + 4 j4^2 + 5 j4 + 4 + 2 g2 + g2^2)
> tmp2 := cpcoeff (x2^2*x4^2*T^2);
    tmp2 := -4 m2^2 + 3 k3 p1 + 6 k3 g2 j4 + 12 k3 j4^2 + 15 k3 j4 + 12 k3 + 6 k3 g2 + 3 k3 g2^2
> tmp3 := factor (3*k3*tmp1 + 2*m2*tmp2);
    tmp3 := -8 m2^3
> elimsolve (tmp3, m2);
    {1 ≠ 0}
m2 is set to:
    0
> launchNZcase (j4);
Launching case level 1:
    j4 ≠ 0
Assume from now on that:
    6 j4 ≠ 0
> tmp1 := cpcoeff (x1^4*x4^4);
    tmp1 := j4 (12 j4^2 + 15 j4 + 4 j4 p1 + 7 p1 + 2 g2 p1 + 12)
> tmp2 := cpcoeff (x1^3*x4^3*T);
    tmp2 := -8 - 2 j4 p1 - 4 p1 - 12 j4 - g2 p1 - 12 j4^2 - 8 j4^3
> tmp3 := factor (tmp1 + 2*j4*tmp2);
    tmp3 := -j4 (16 j4^3 + 12 j4^2 + 9 j4 + p1 + 4)
> elimsolve (tmp3, p1);
    {1 ≠ 0}
p1 is set to:
    -16 j4^3 - 12 j4^2 - 9 j4 - 4
> launchNZcase (16*j4^3+12*j4^2+9*j4+4);
Launching case level 2:
    16 j4^3 + 12 j4^2 + 9 j4 + 4 ≠ 0
Assume from now on that:
    6 j4 (16 j4^3 + 12 j4^2 + 9 j4 + 4) ≠ 0
> tmp1 := cpcoeff (x1^3*x4^3*T);
    tmp1 := 8 + 9 g2 j4 + 4 g2 + 32 j4 + 54 j4^2 + 80 j4^3 + 12 g2 j4^2 + 32 j4^4 + 16 j4^3 g2
> elimsolve (tmp1, g2);
    {16 j4^3 + 12 j4^2 + 9 j4 + 4 ≠ 0}

```

g2 is set to:

$$-\frac{2(4 + 40j4^3 + 16j4 + 27j4^2 + 16j4^4)}{16j4^3 + 12j4^2 + 9j4 + 4}$$

> **launchNZcase (2\*j4+1+4\*j4^2);**

Launching case level 3:

$$2j4 + 1 + 4j4^2 \neq 0$$

Assume from now on that:

$$6j4(16j4^3 + 12j4^2 + 9j4 + 4)(2j4 + 1 + 4j4^2) \neq 0$$

> **tmp1 := cpcoeff (x1\*x3\*x4^6);**

$$tmp1 := -\frac{288j4^3(2j4 + 1 + 4j4^2)^5}{(16j4^3 + 12j4^2 + 9j4 + 4)^2}$$

> **tmp1 := contradict (tmp1);**

Contradiction on case level 3, so:

$$2j4 + 1 + 4j4^2 = 0$$

Proceed on case level 2 with:

$$6j4(16j4^3 + 12j4^2 + 9j4 + 4) \neq 0$$

On account of:

$$2j4 + 1 + 4j4^2 = 0$$

the following return value can be used as an equation:

$$tmp1 := 2j4 + 1 + 4j4^2$$

> **tmp2 := cpcoeff (x2\*x4^3\*T^2);**

$$tmp2 := -4(32 + 320m3j4^3 + 5120m3j4^7 + 4096m3j4^8 + 2048m3j4^9 + 64m3j4^2 + 1024m3j4^4 + 4096m3j4^6 + 2432m3j4^5 + 8m3j4 + 240j4 + 930j4^2 + 2622j4^3 + 5529j4^4 + 11520j4^6 + 8934j4^5 + 11040j4^7 + 3584j4^9 + 7680j4^8) / (16j4^3 + 12j4^2 + 9j4 + 4)^2$$

> **tmp3 := factor (32\*m3\*j4\*tmp1^4 + (16\*j4^3+12\*j4^2+9\*j4+4)^2\*tmp2);**

$$tmp3 := -4(2 + 6j4 + 9j4^2 + 14j4^3)(16j4^3 + 12j4^2 + 9j4 + 4)^2$$

> **tmp4 := factor (tmp3 - quo(tmp3, tmp1, j4)\*tmp1);**

$$tmp4 := -\frac{81}{4} - 81j4$$

> **tmp5 := factor (81\*tmp1 + (4\*j4+1)\*tmp4);**

$$tmp5 := \frac{243}{4}$$

> **tmp1 := contradict (tmp5);**

Contradiction on case level 2, so:

$$16j4^3 + 12j4^2 + 9j4 + 4 = 0$$

Variables to be uneliminated:

$$"g2 := 'g2'"$$

Proceed on case level 1 with:

$$6j4 \neq 0$$

On account of:

$$16j4^3 + 12j4^2 + 9j4 + 4 = 0$$

the following return value can be used as an equation:

$$tmp1 := 16j4^3 + 12j4^2 + 9j4 + 4$$

> **tmp2 := cpcoeff (x1^3\*x4^3\*T) ;**

$$tmp2 := 8 + 9g2j4 + 4g2 + 32j4 + 54j4^2 + 80j4^3 + 12g2j4^2 + 32j4^4 + 16j4^3g2$$

> **tmp3 := factor (tmp2 + g2\*tmp1) ;**

$$tmp3 := 8 + 18g2j4 + 8g2 + 32j4 + 54j4^2 + 80j4^3 + 24g2j4^2 + 32j4^4 + 32j4^3g2$$

> **tmp4 := factor (tmp3 - quo(tmp3, tmp1, j4)\*tmp1) ;**

$$tmp4 := -6 - \frac{15}{2}j4 - 6j4^2$$

> **tmp5 := factor (3\*tmp1 + (8\*j4-4)\*tmp4) ;**

$$tmp5 := 9j4 + 36$$

> **tmp6 := factor (6\*tmp4 + (4\*j4-11)\*tmp5) ;**

$$tmp6 := -432$$

> **contradict (tmp6) ;**

Contradiction on case level 1, so:

$$j4 = 0$$

Variables to be uneliminated:

$$p1 := p1$$

Proceed on case level 0 with:

$$6 \neq 0$$

On account of:

$$j4 = 0$$

$$\{1 \neq 0\}$$

j4 is set to:

$$0$$

> **launchNZcase (p1+4) ;**

Launching case level 1:

$$p1 + 4 \neq 0$$

Assume from now on that:

$$6p1 + 24 \neq 0$$

> **launchNZcase (g2+4) ;**

Launching case level 2:

$$g2 + 4 \neq 0$$

Assume from now on that:

$$6(p1 + 4)(g2 + 4) \neq 0$$

> **tmp1 := cpcoeff (x1^3\*x4^3\*T) ;**

$$tmp1 := -8 - 4p1 - g2p1$$

> **elimsolve (tmp1, p1) ;**

$$\{g2 + 4 \neq 0\}$$

p1 is set to:

$$-\frac{8}{g2 + 4}$$

Nonzero constraint refines to:

$$6(4 + 2g2)(g2 + 4) \neq 0$$

> **tmp1 := cpcoeff (x3\*x4^5\*T) ;**

$$tmp1 := \frac{8(2+g2)^4}{(g2+4)^2}$$

> **contradict (tmp1);**

Contradiction on case level 2, so:

$$g2 + 4 = 0$$

Variables to be uneliminated:

"p1 := 'p1'"

Proceed on case level 1 with:

$$6p1 + 24 \neq 0$$

On account of:

$$g2 + 4 = 0$$

$$\{1 \neq 0\}$$

g2 is set to:

$$-4$$

> **tmp1 := cpcoeff (x1^3\*x4^3\*T);**

$$tmp1 := -8$$

> **contradict (tmp1);**

Contradiction on case level 1, so:

$$p1 + 4 = 0$$

Variables to be uneliminated:

"g2 := 'g2'"

Proceed on case level 0 with:

$$6 \neq 0$$

On account of:

$$p1 + 4 = 0$$

$$\{1 \neq 0\}$$

p1 is set to:

$$-4$$

> **tmp1 := cpcoeff (x1^3\*x4^3\*T);**

$$tmp1 := 8 + 4g2$$

> **elimsolve (tmp1, g2);**

$$\{1 \neq 0\}$$

g2 is set to:

$$-2$$

> **tmp1 := cpcoeff (x2\*x4^3\*T^2);**

$$tmp1 := -8$$

> **contradict (tmp1);**

Contradiction on case level 0, so:

$$6 = 0$$

Variables to be uneliminated:

"g2 := 'g2'"

"p1 := 'p1'"

"j4 := 'j4'"

"m2 := 'm2'"

"p4 := 'p4'"

"g1 := 'g1'"  
"m1 := 'm1'"  
"k2 := 'k2'"  
"m4 := 'm4'"  
"e2 := 'e2'"  
"k1 := 'k1'"  
"g4 := 'g4'"  
"k4 := 'k4'"  
"e4 := 'e4'"  
"e1 := 'e1'"  
"s4 := 's4'"  
"r4 := 'r4'"  
"q4 := 'q4'"  
"o4 := 'o4'"  
"n4 := 'n4'"  
"l4 := 'l4'"  
"i4 := 'i4'"  
"h4 := 'h4'"  
"f4 := 'f4'"  
"s1 := 's1'"  
"r1 := 'r1'"  
"q1 := 'q1'"  
"o1 := 'o1'"  
"n1 := 'n1'"  
"l1 := 'l1'"  
"i1 := 'i1'"  
"h1 := 'h1'"  
"f1 := 'f1'"  
"s2 := 's2'"  
"r2 := 'r2'"  
"q2 := 'q2'"  
"o2 := 'o2'"  
"n2 := 'n2'"  
"l2 := 'l2'"  
"i2 := 'i2'"  
"h2 := 'h2'"  
"f2 := 'f2'"  
"s3 := 's3'"  
"r3 := 'r3'"

```
"q3 := 'q3'"
```

```
"o3 := 'o3'"
```

```
"n3 := 'n3'"
```

```
"l3 := 'l3'"
```

```
"i3 := 'i3'"
```

```
"h3 := 'h3'"
```

```
"f3 := 'f3'"
```

That is all, folks! Check that all variables are uneliminated:

```
[[a1,b1,c1,d1,e1,f1,g1,h1,i1,j1,k1,l1,m1,n1,o1,p1,q1,r1,s1,t1],  
 [a2,b2,c2,d2,e2,f2,g2,h2,i2,j2,k2,l2,m2,n2,o2,p2,q2,r2,s2,t2],  
 [a3,b3,c3,d3,e3,f3,g3,h3,i3,j3,k3,l3,m3,n3,o3,p3,q3,r3,s3,t3],  
 [a4,b4,c4,d4,e4,f4,g4,h4,i4,j4,k4,l4,m4,n4,o4,p4,q4,r4,s4,t4]]
```

```
> startnewHcase ();
```

```
No cases for H remaining; all cases have been evaluated.
```

```
>
```
